# Supplementary material for: The Sloan Digital Sky Survey Reverberation Mapping Project: Systematic Investigations of Short-Timescale CIV Broad Absorption Line Variability
Source: arXiv:1811.00010 ancillary file (2018-10-31)

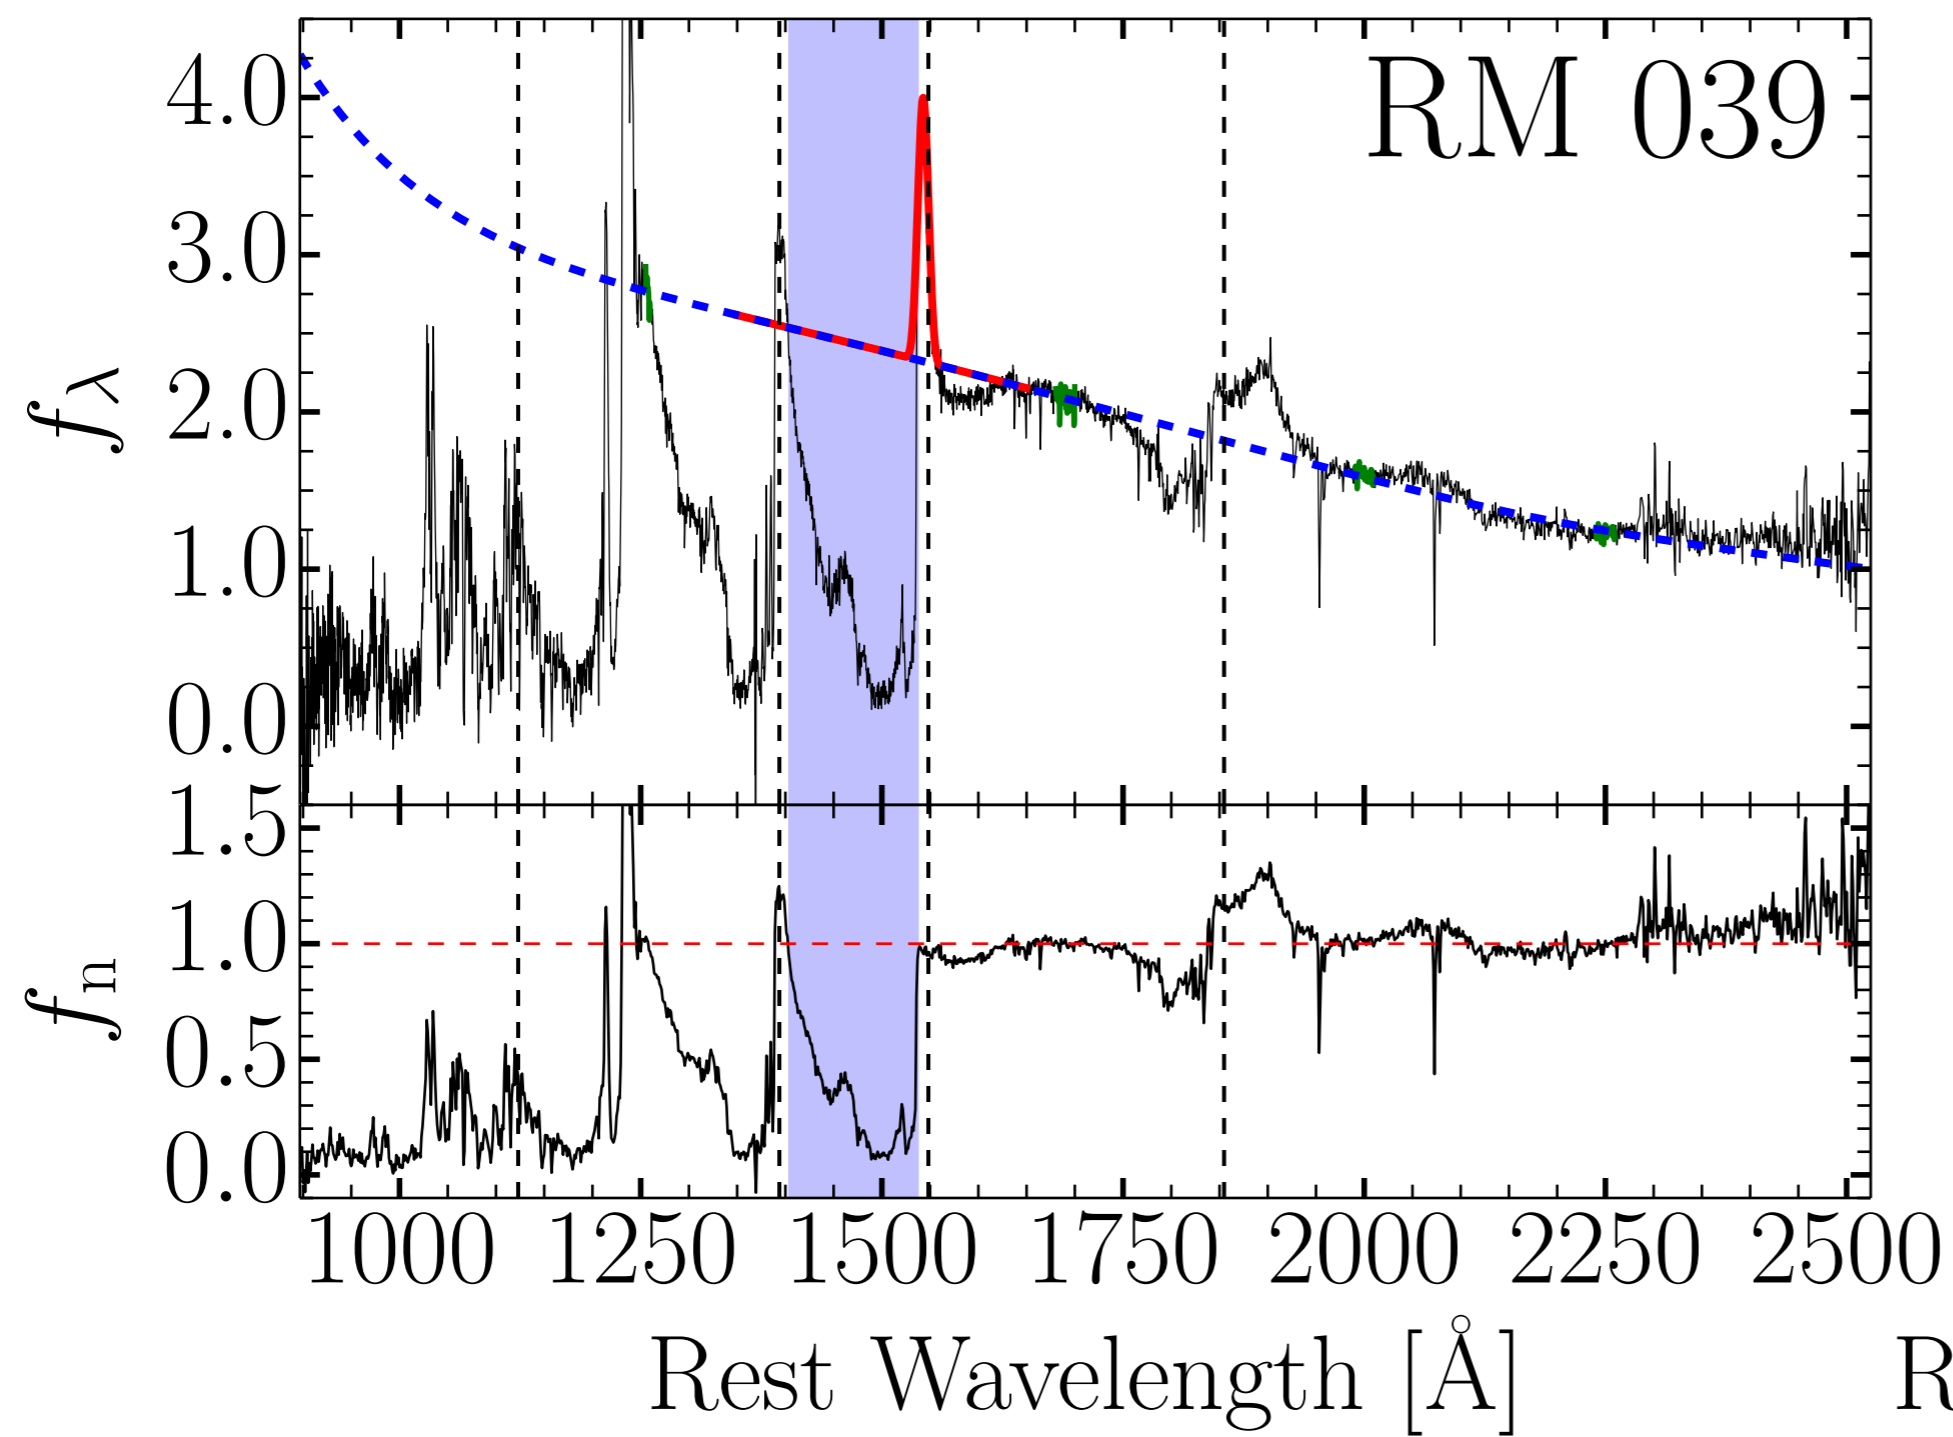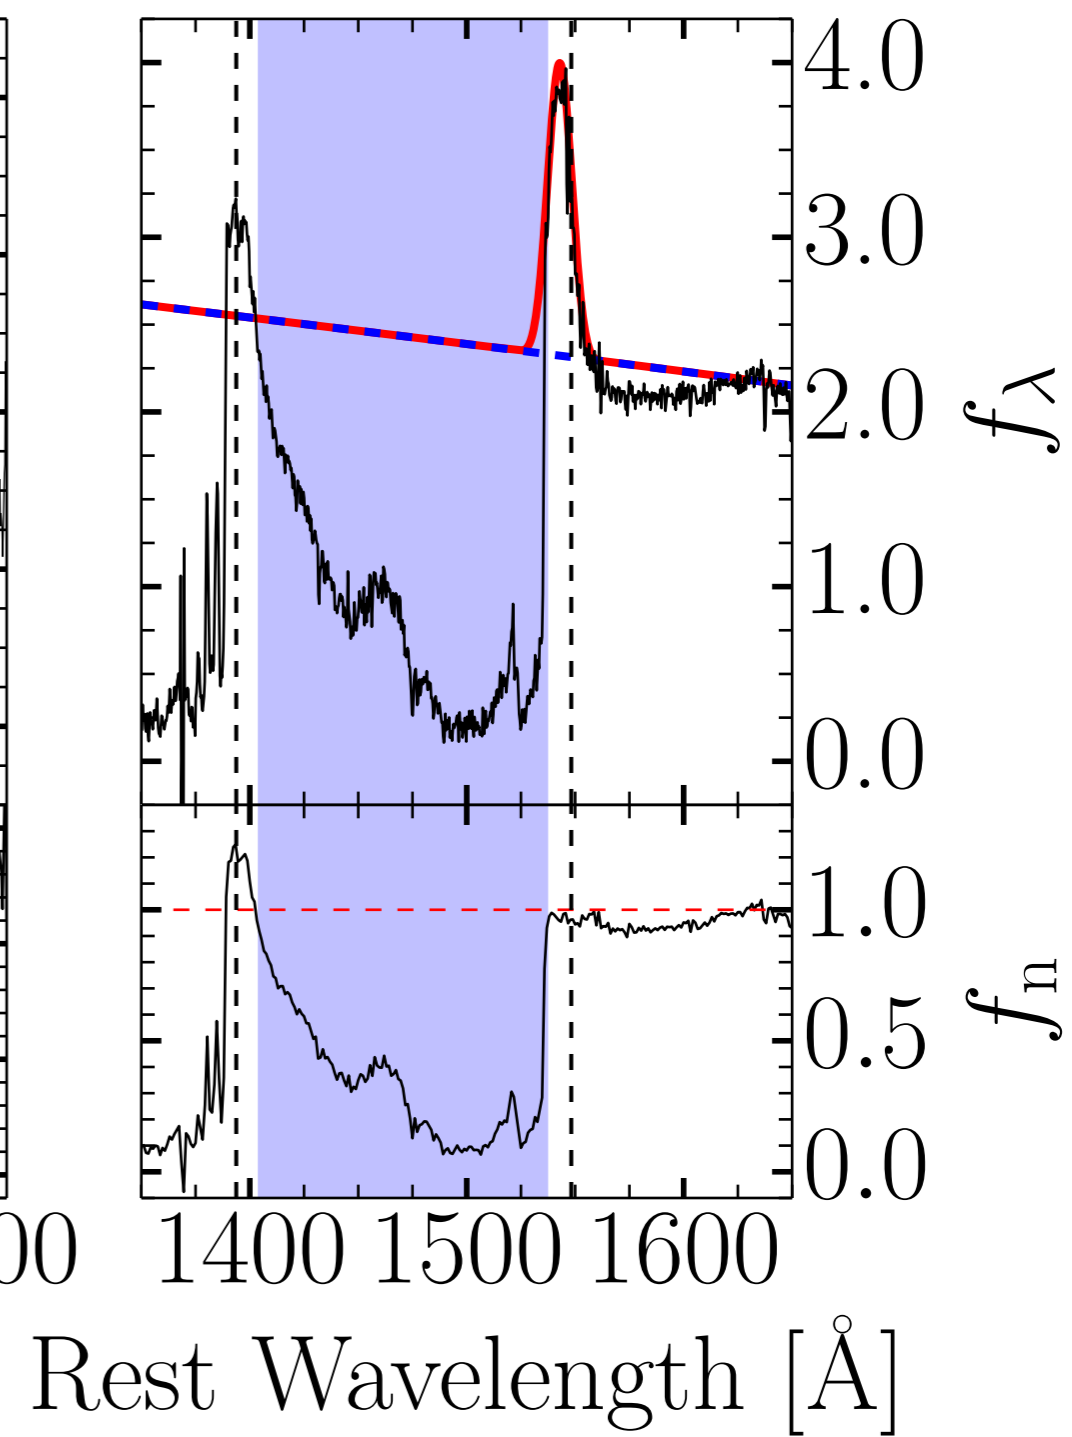

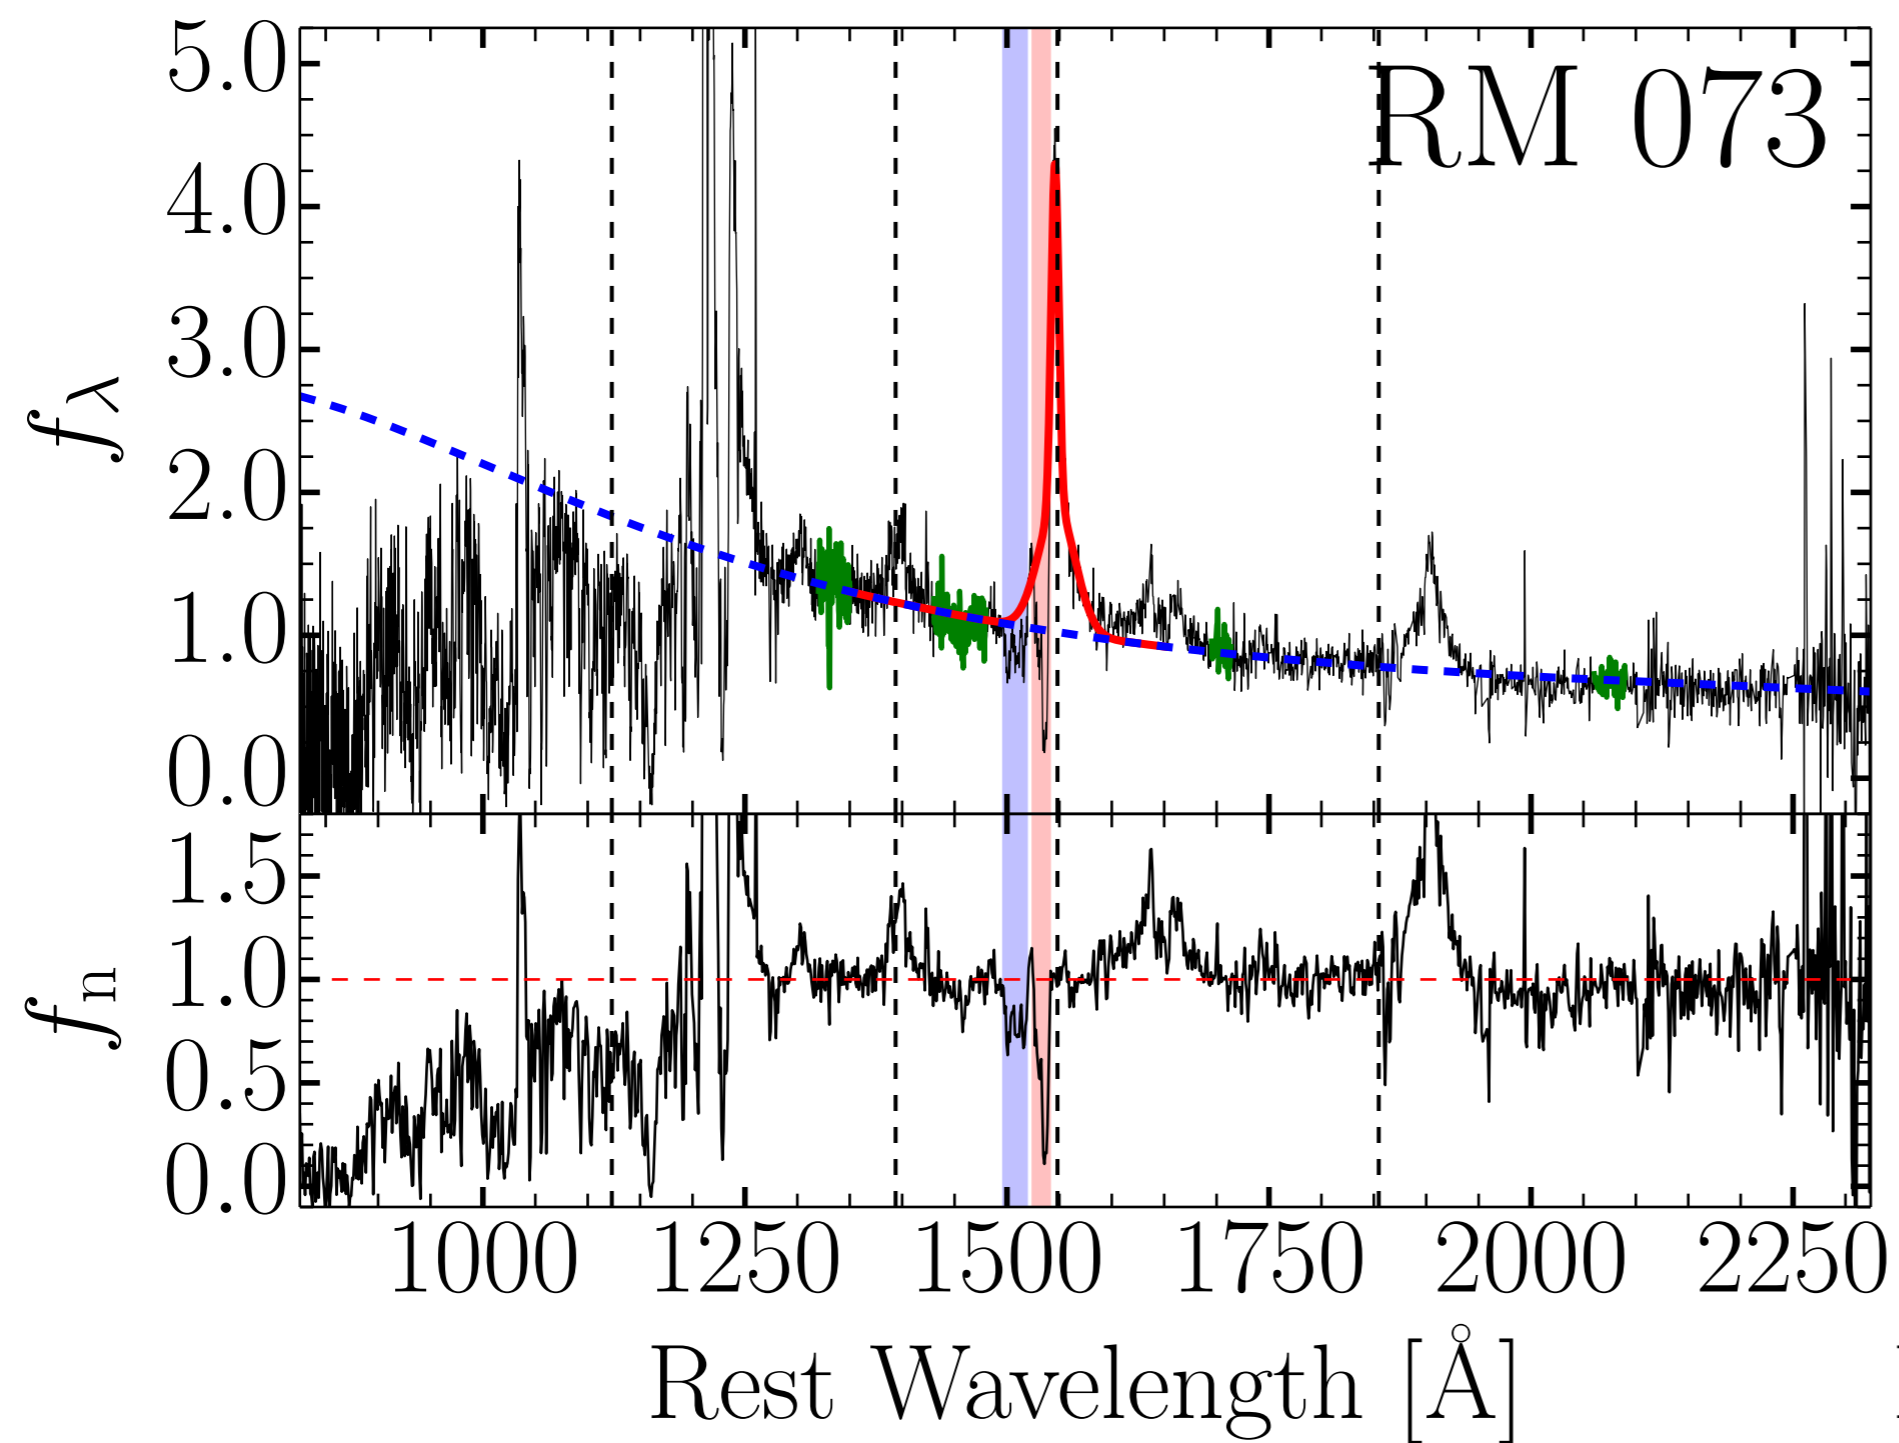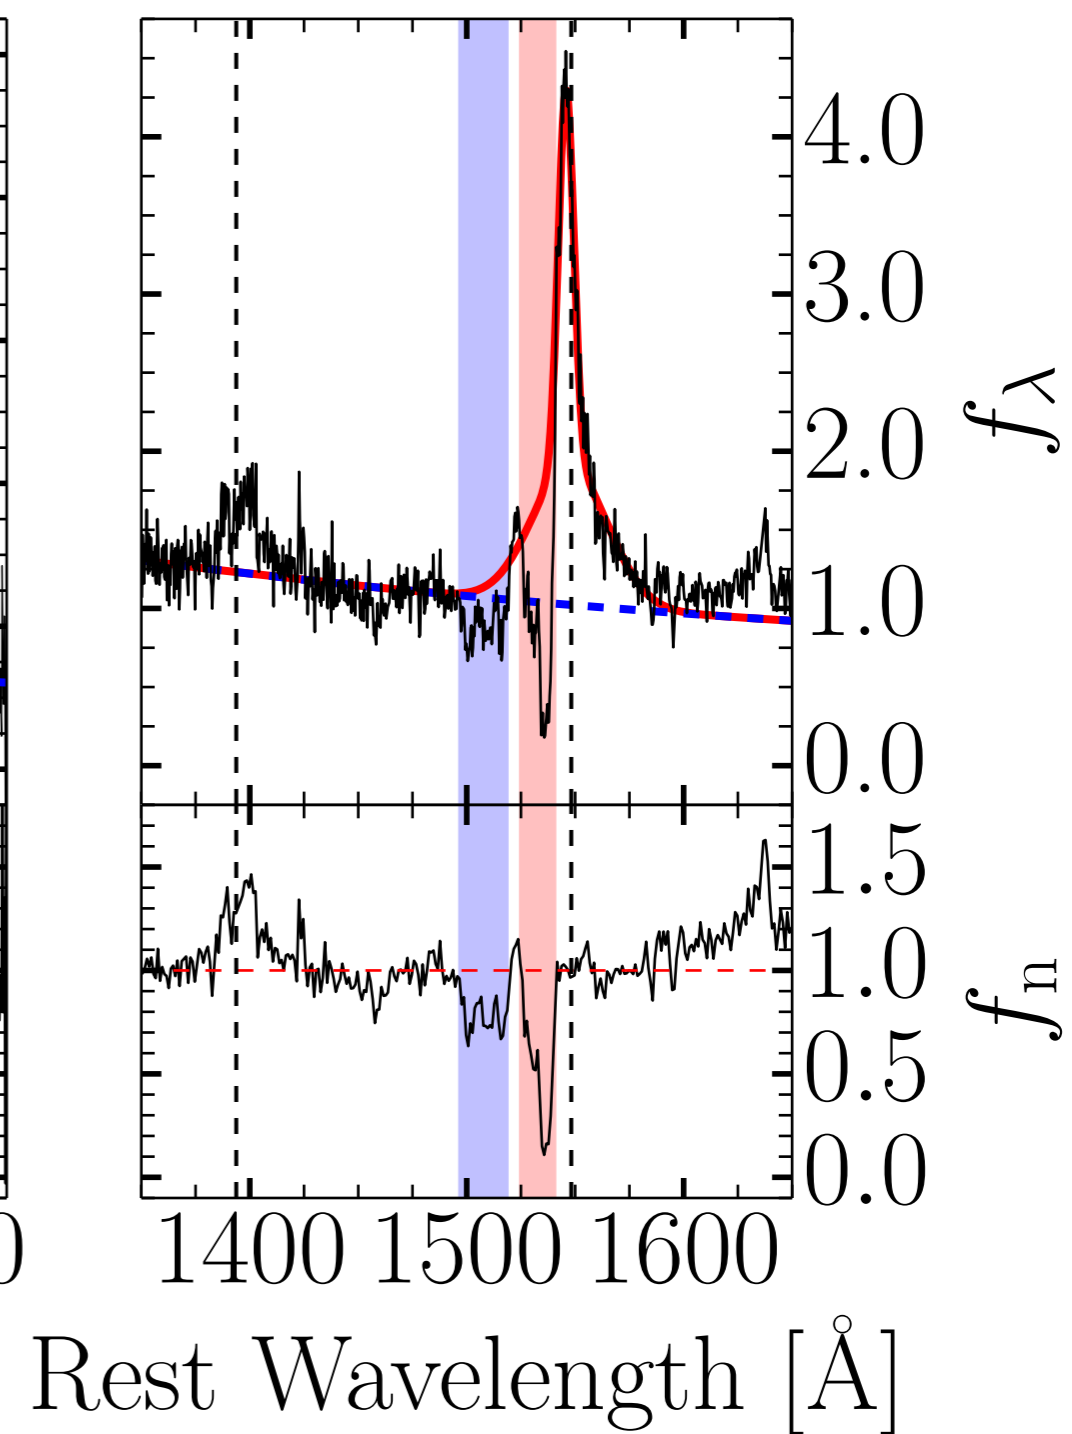

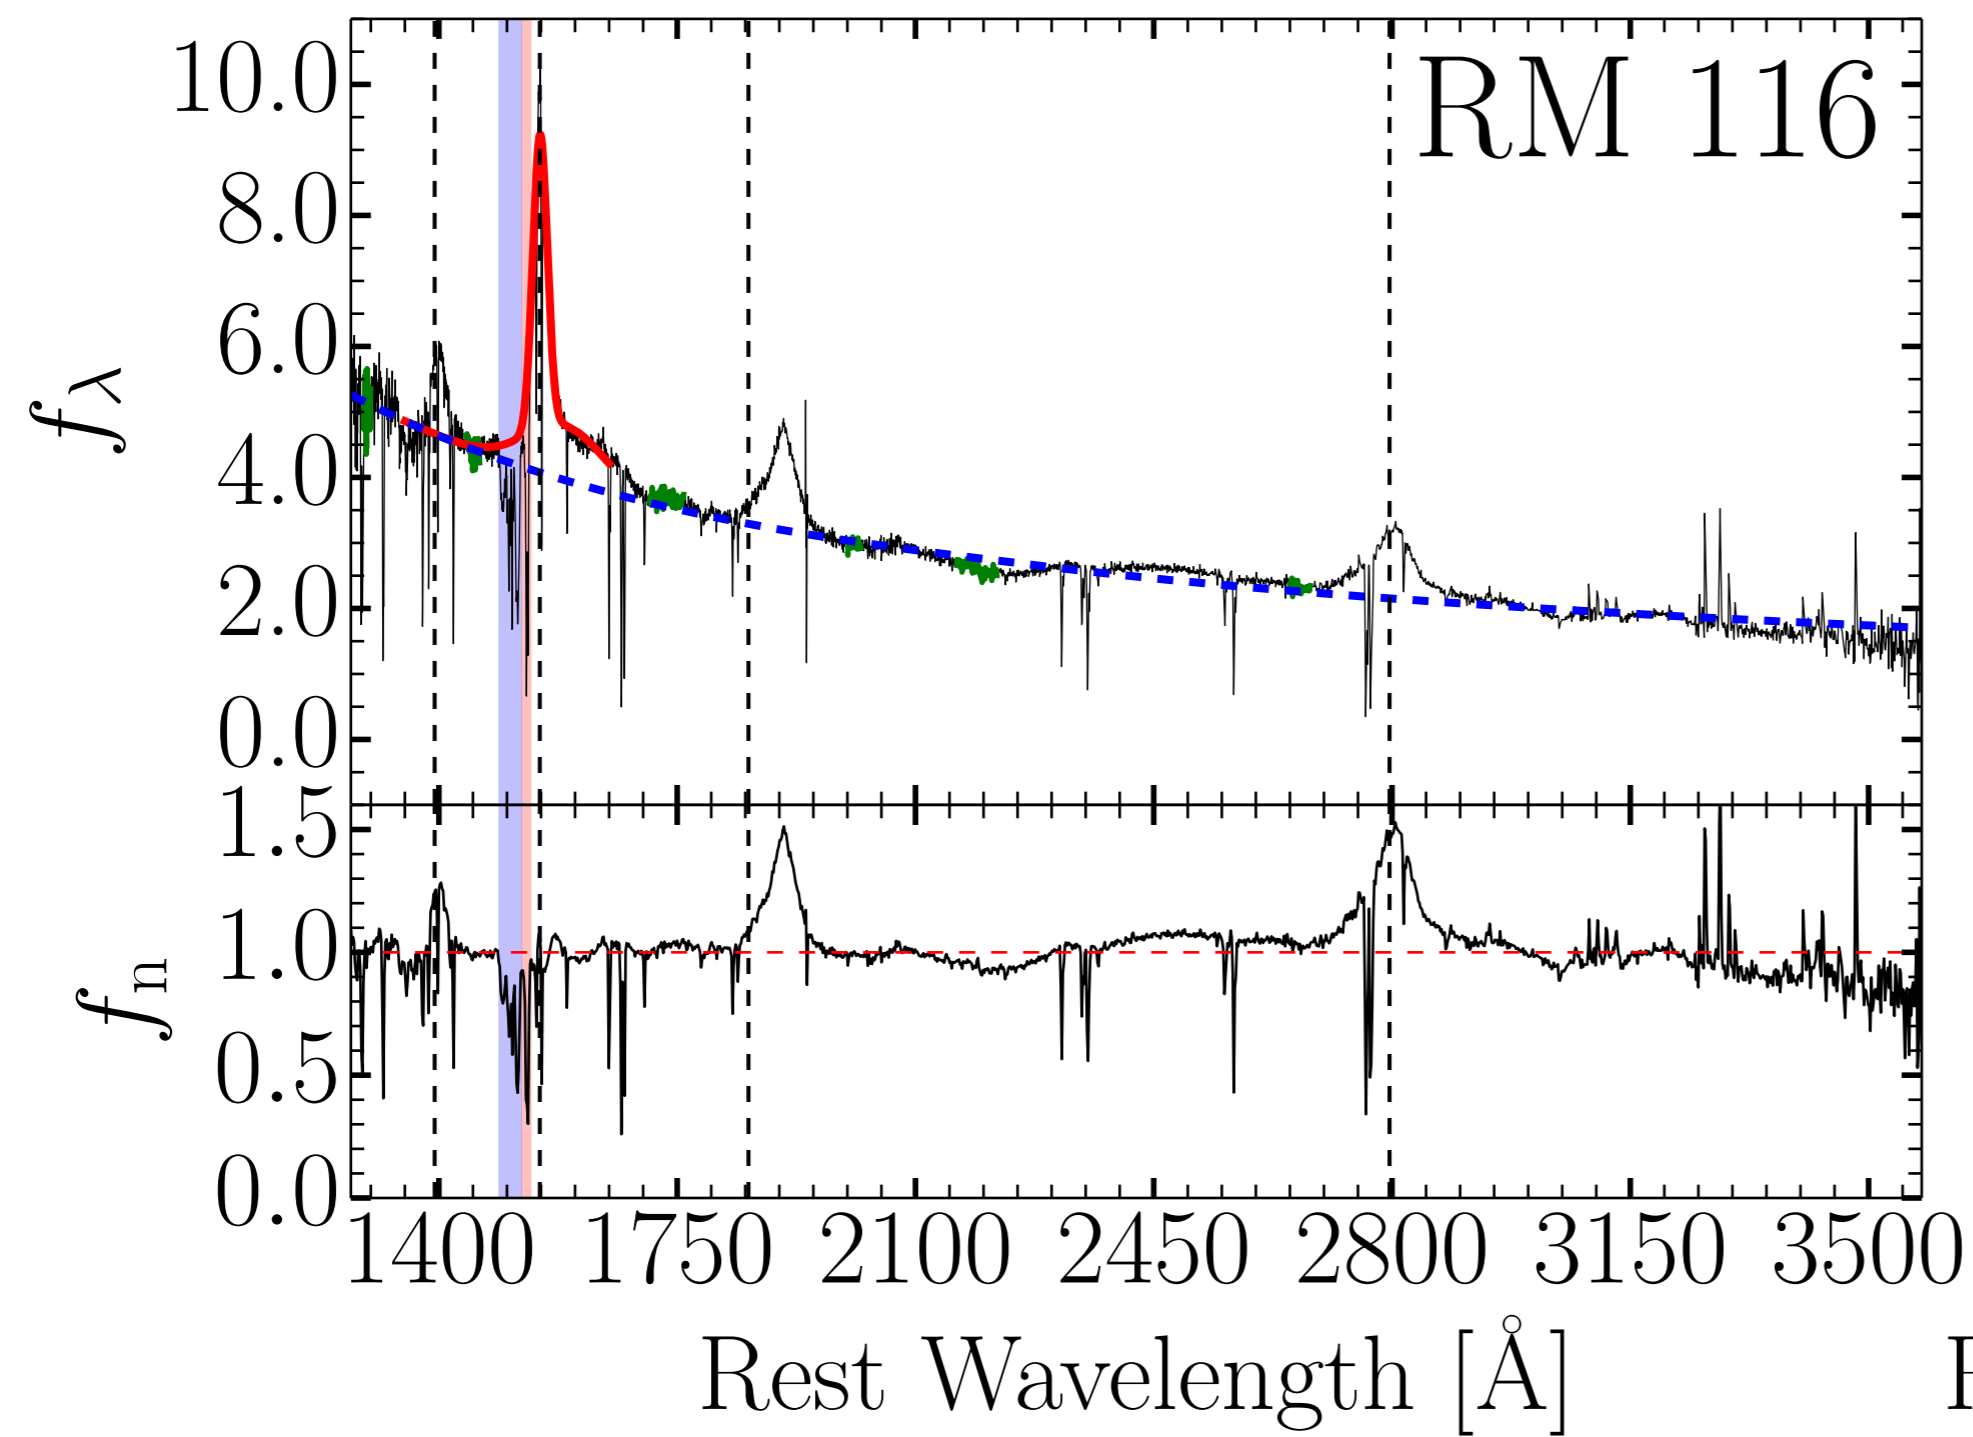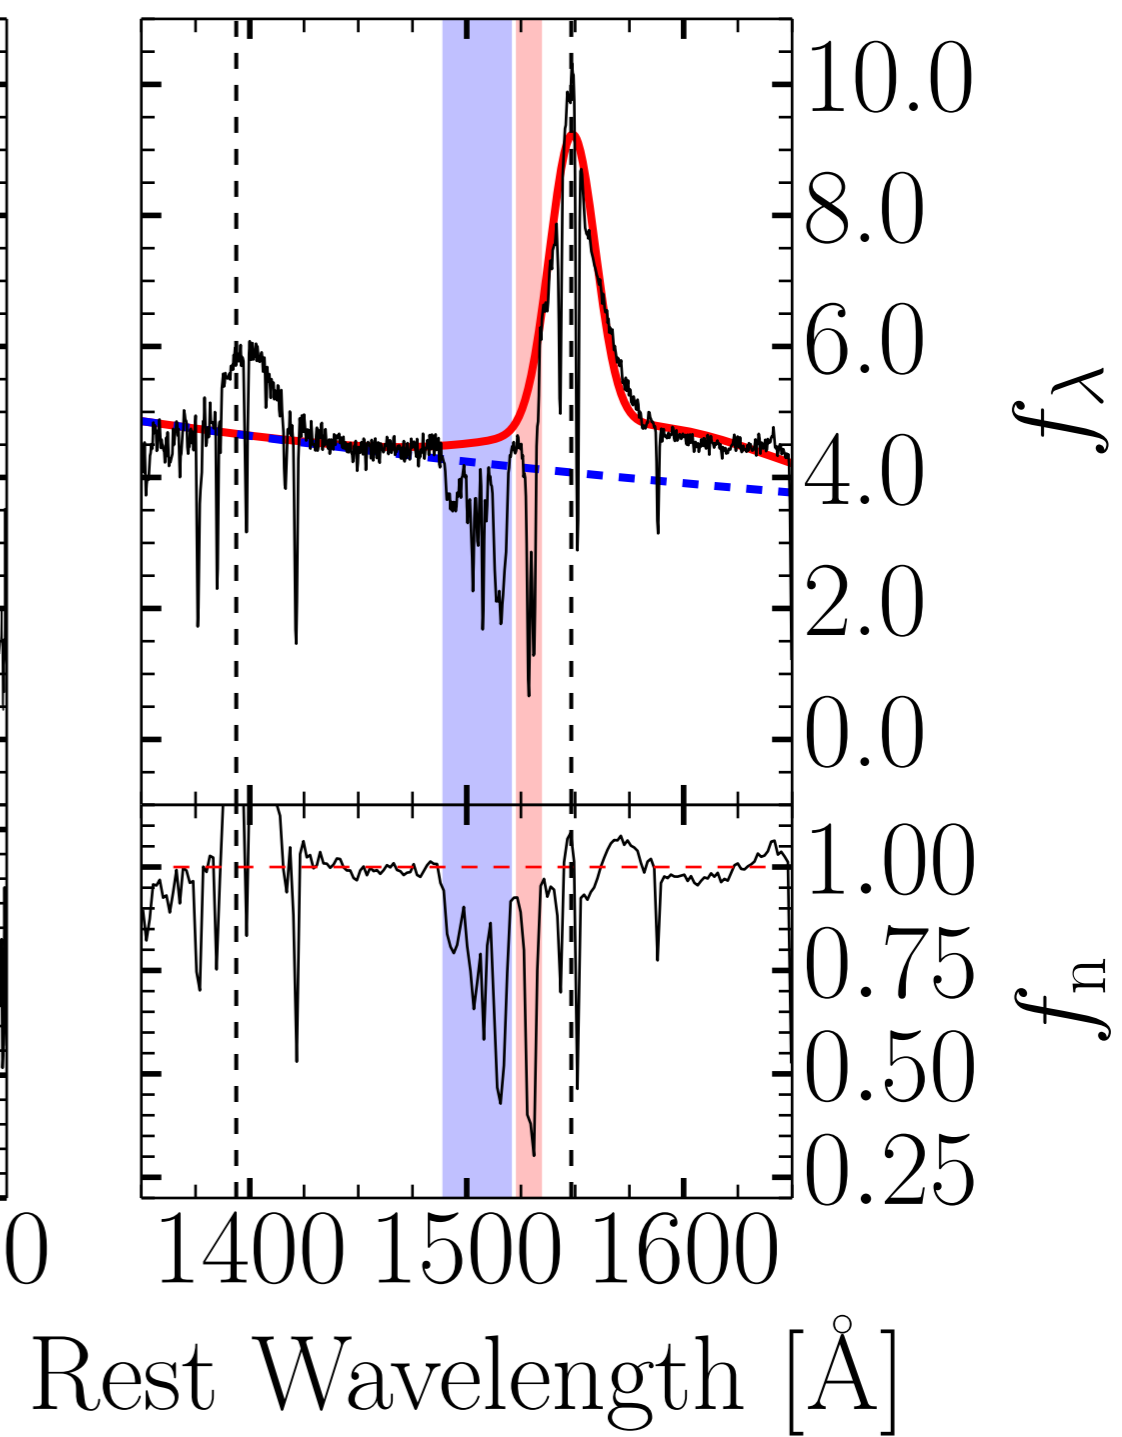

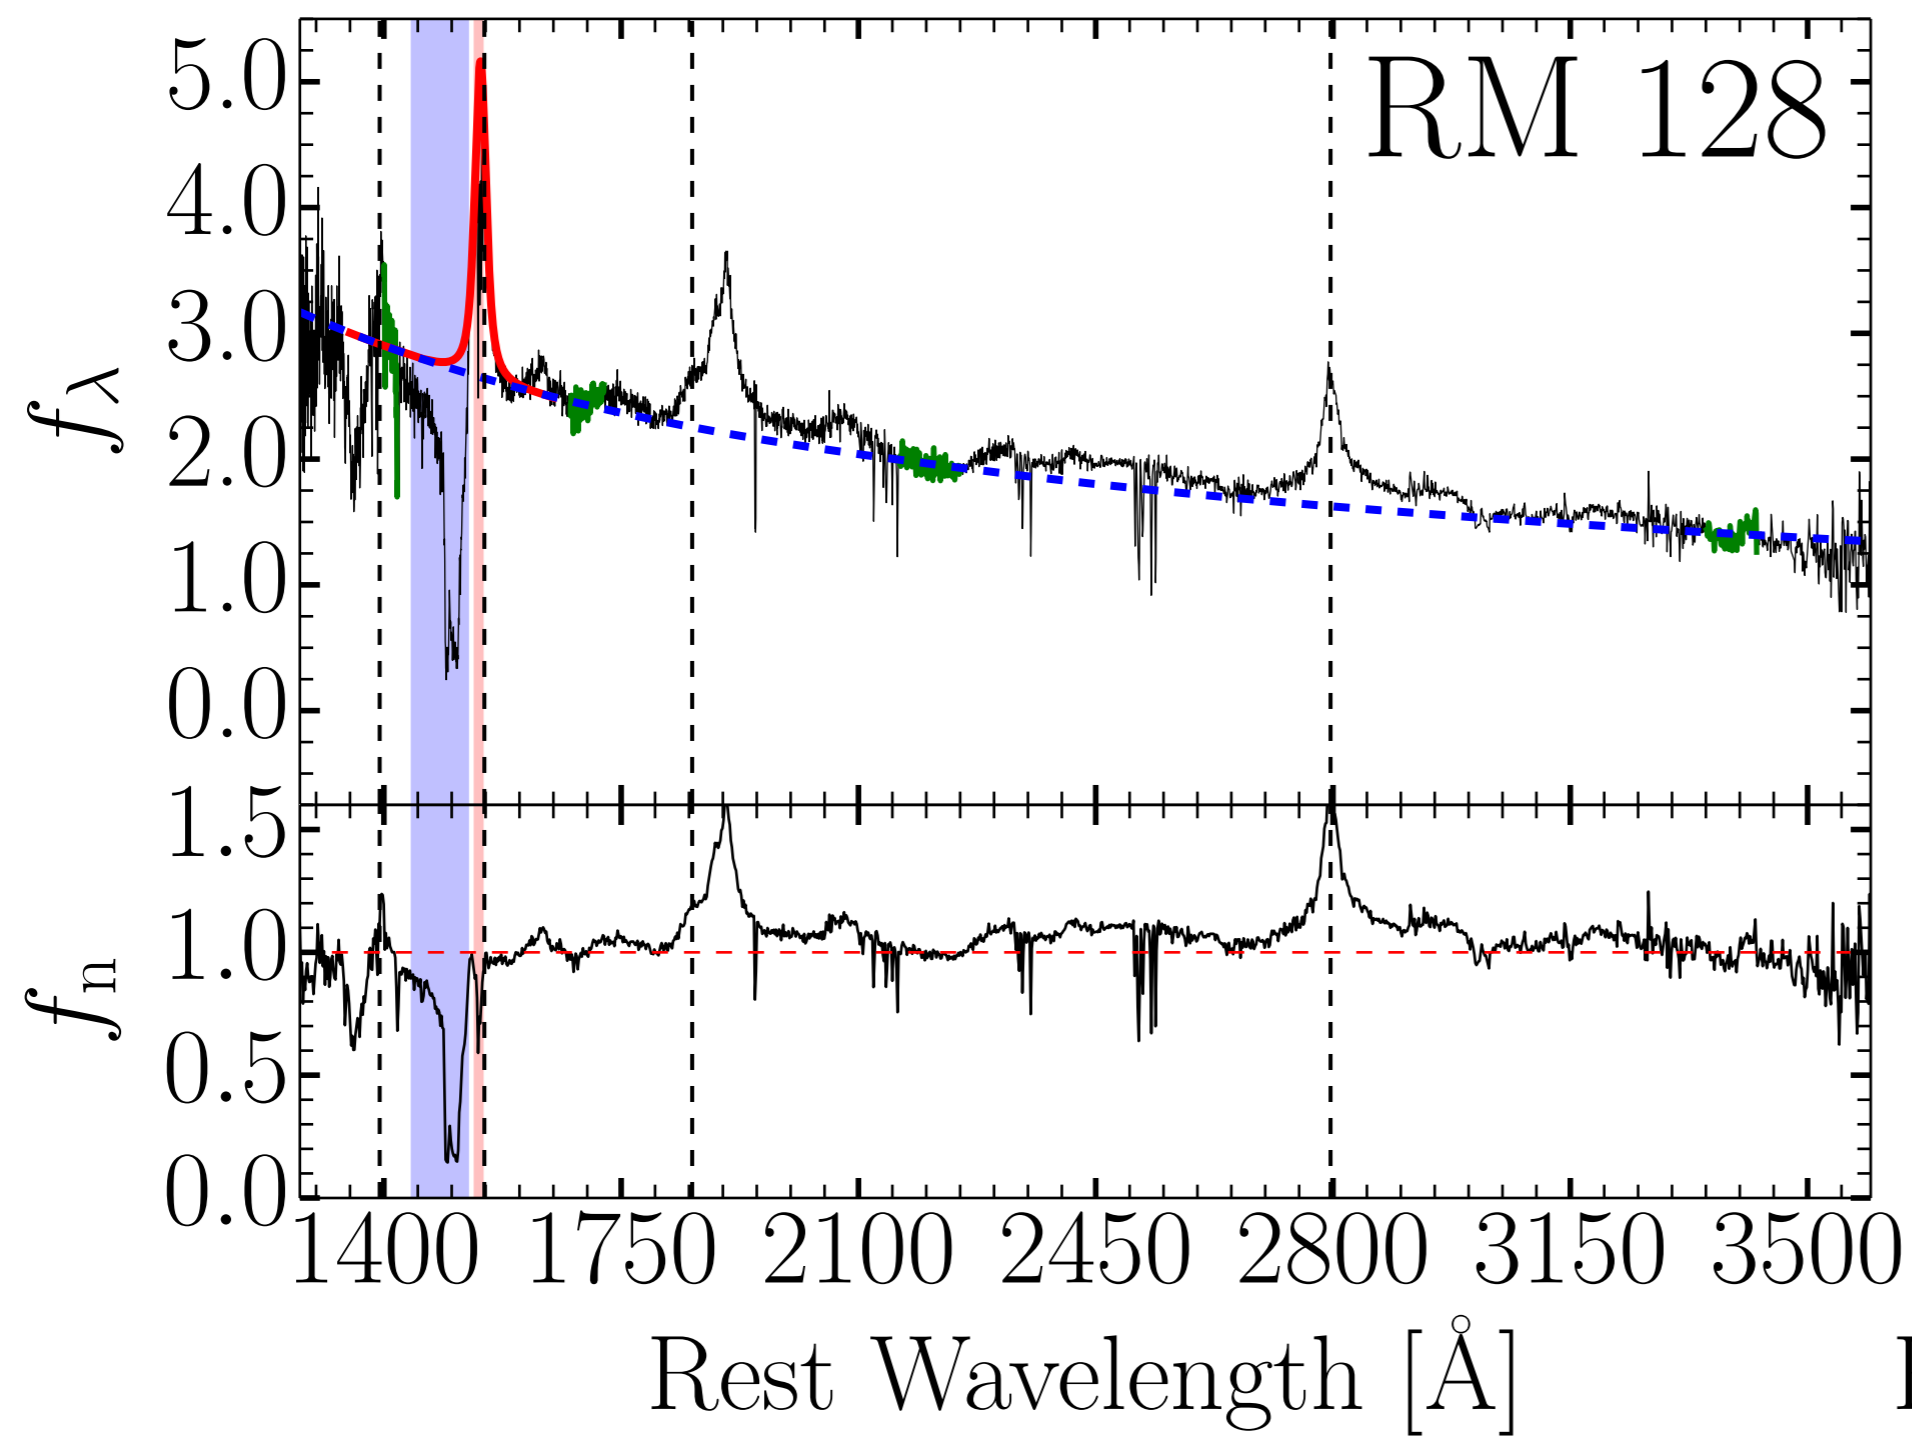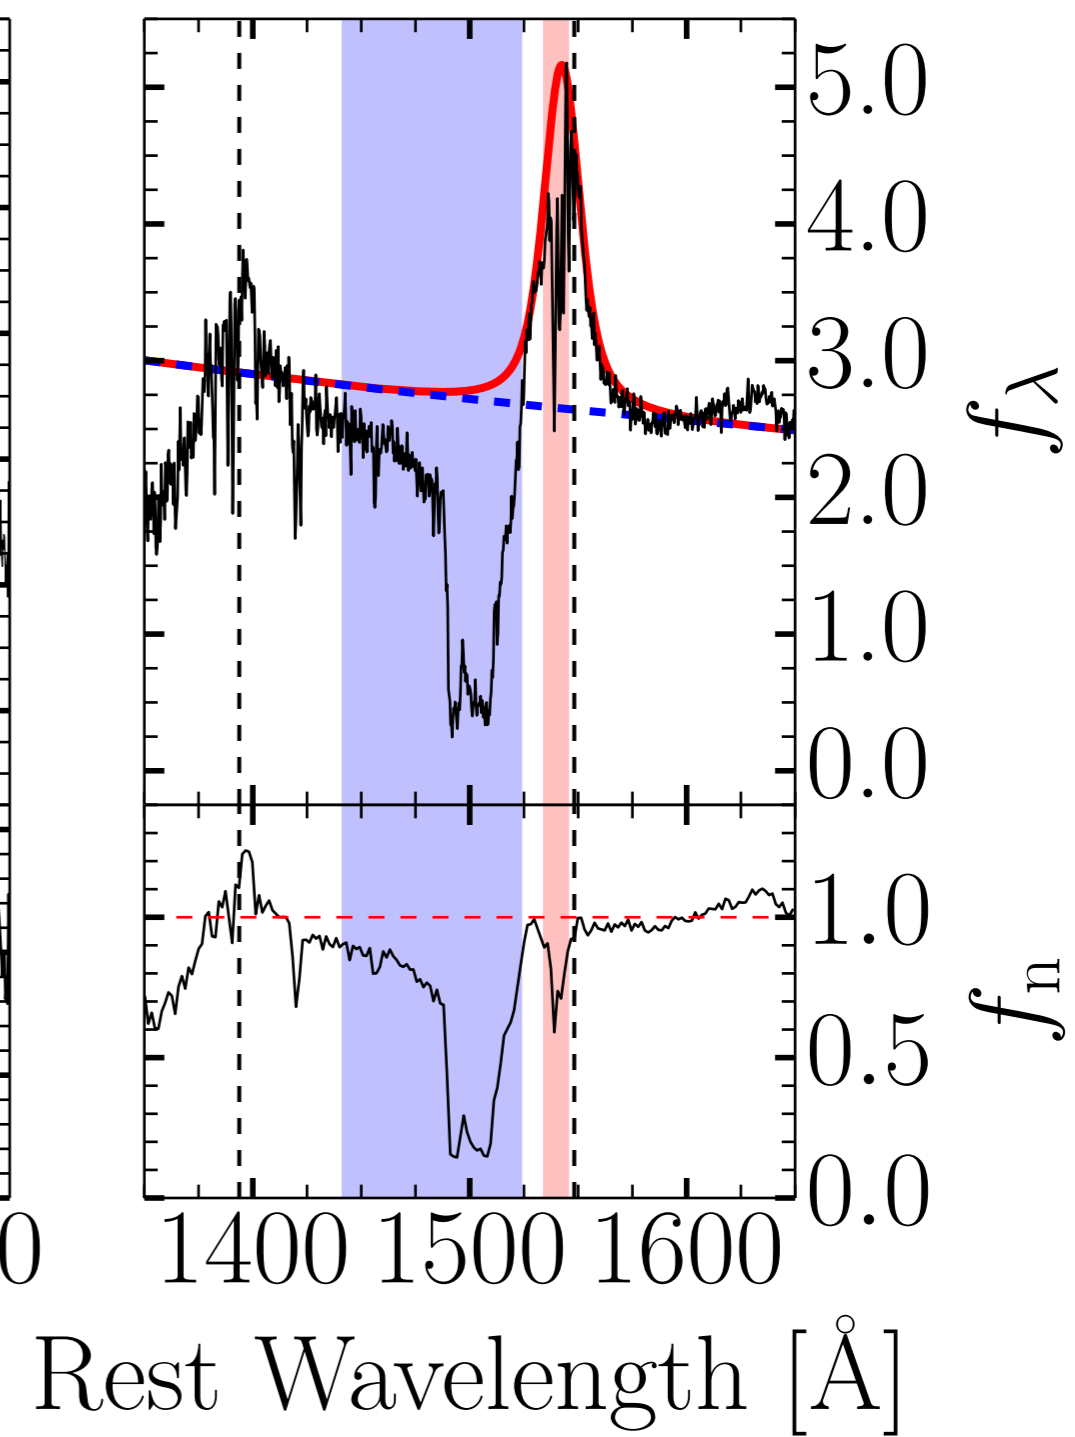

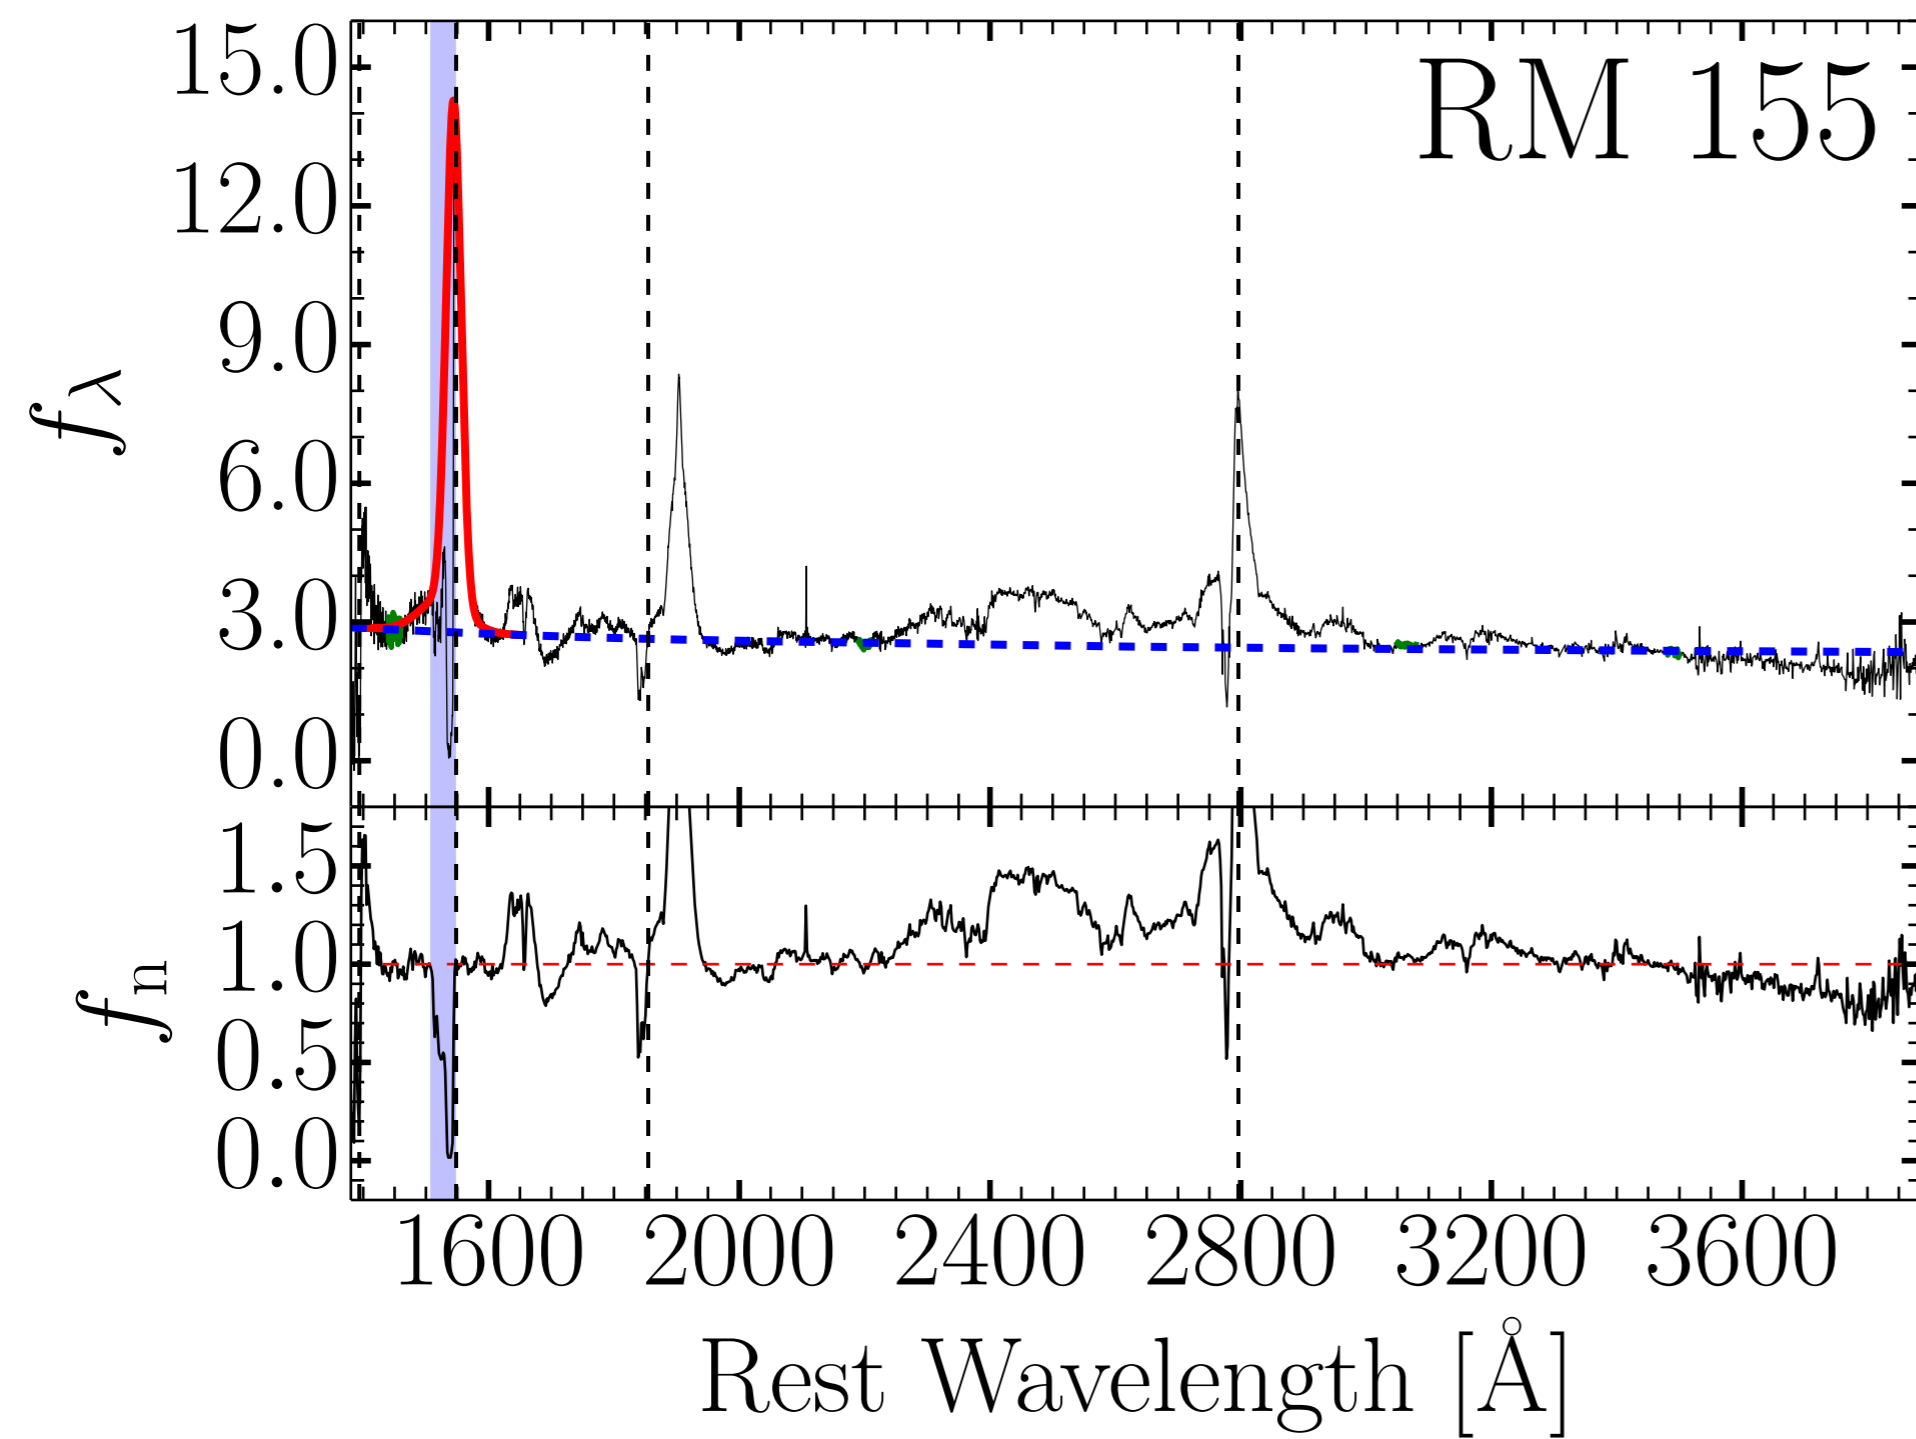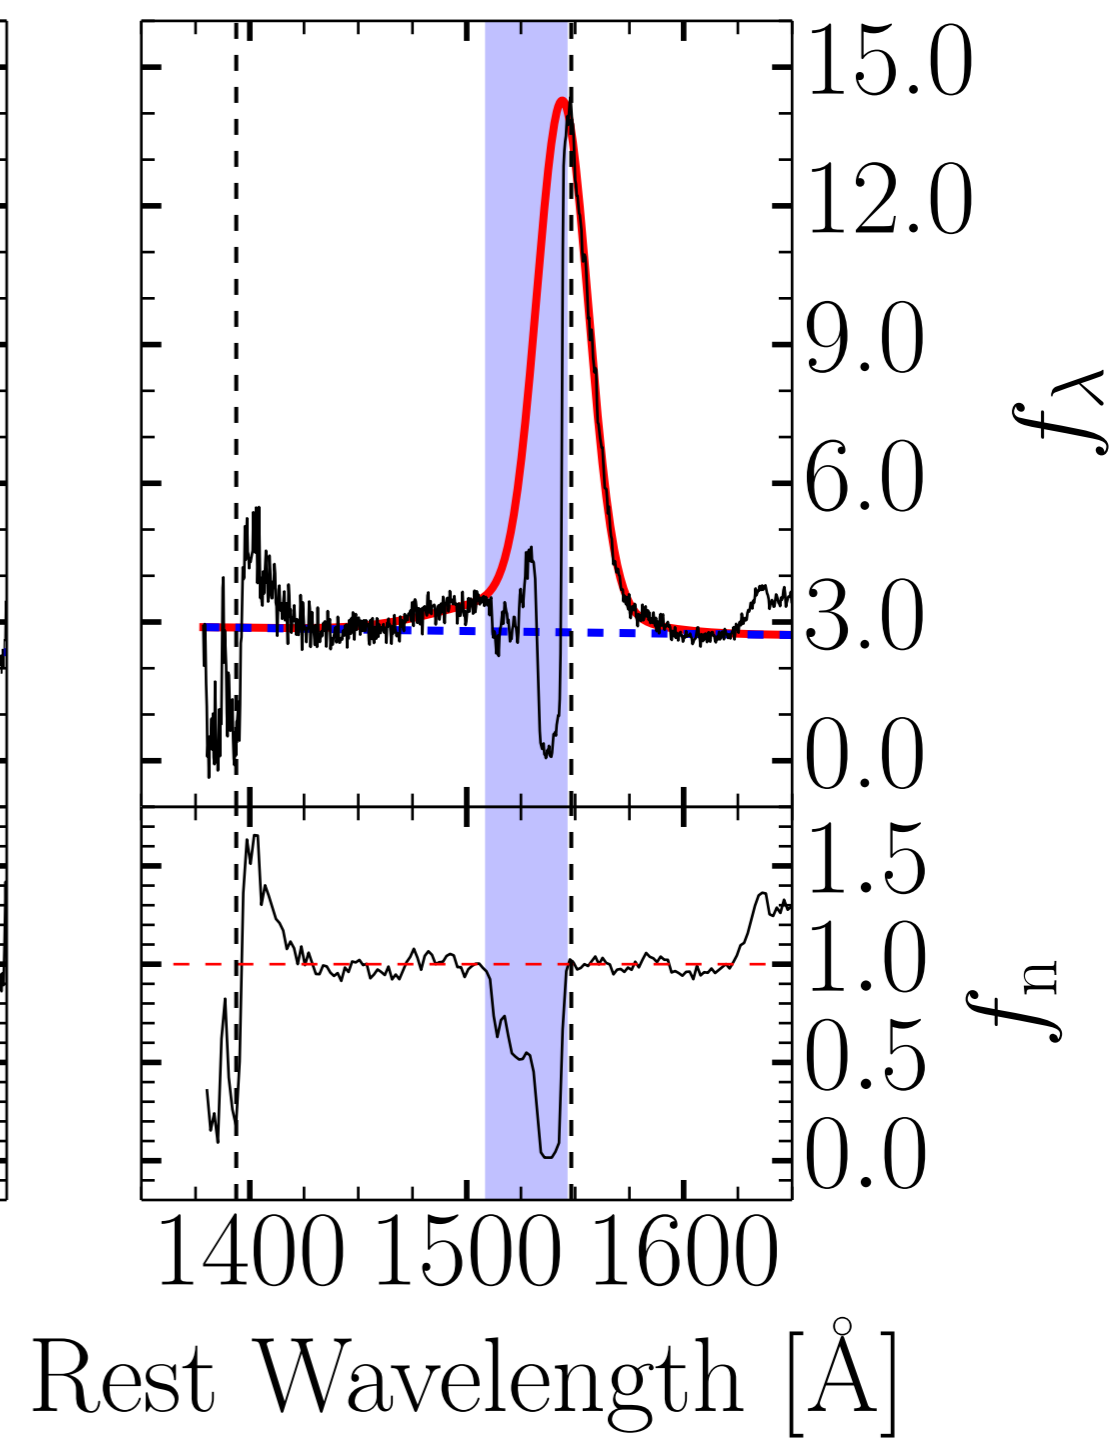

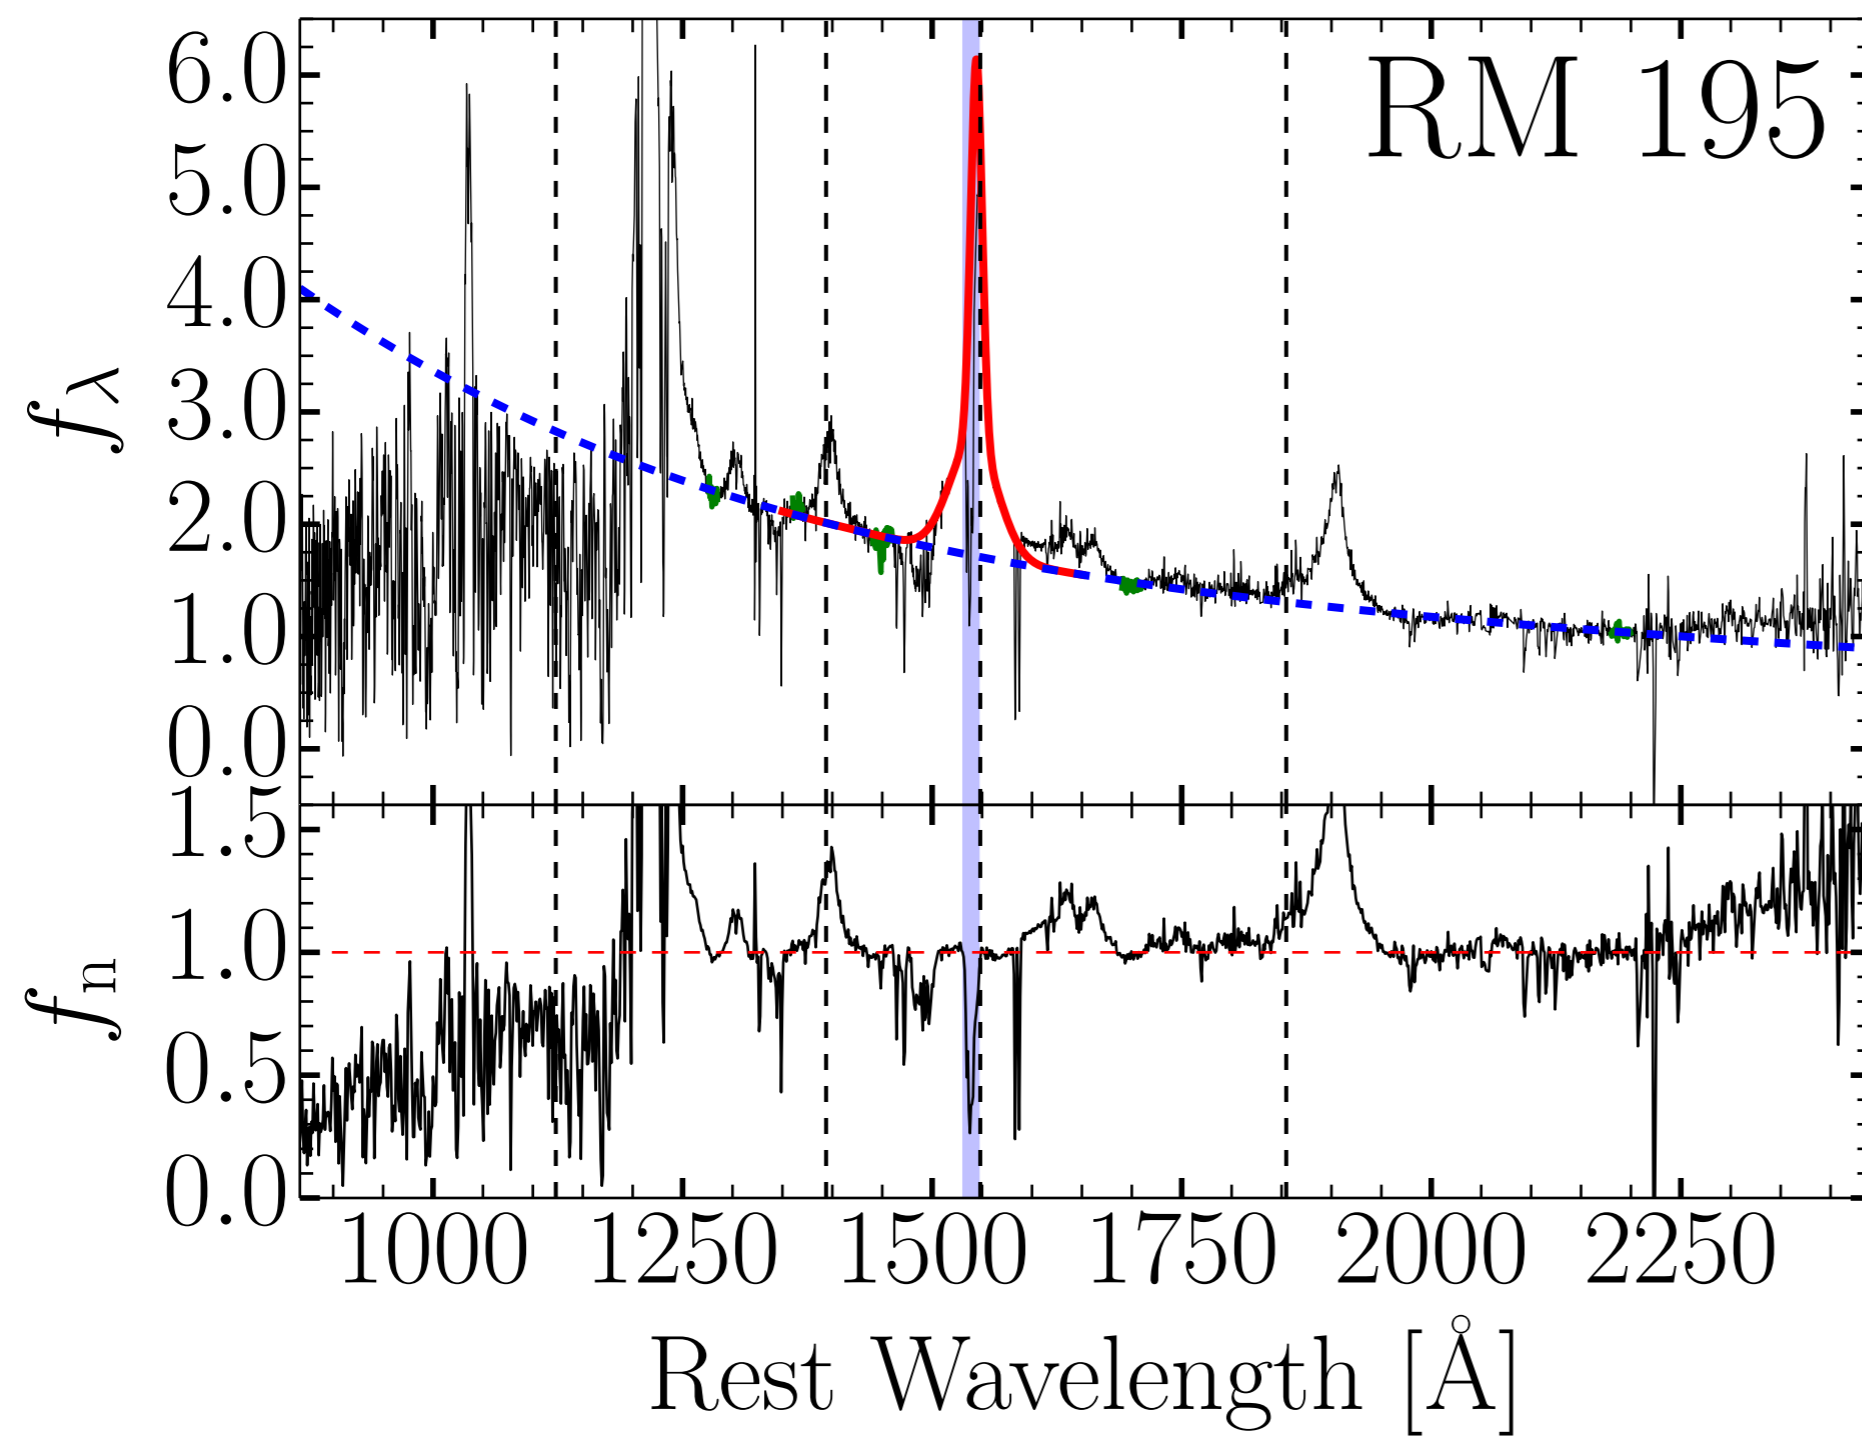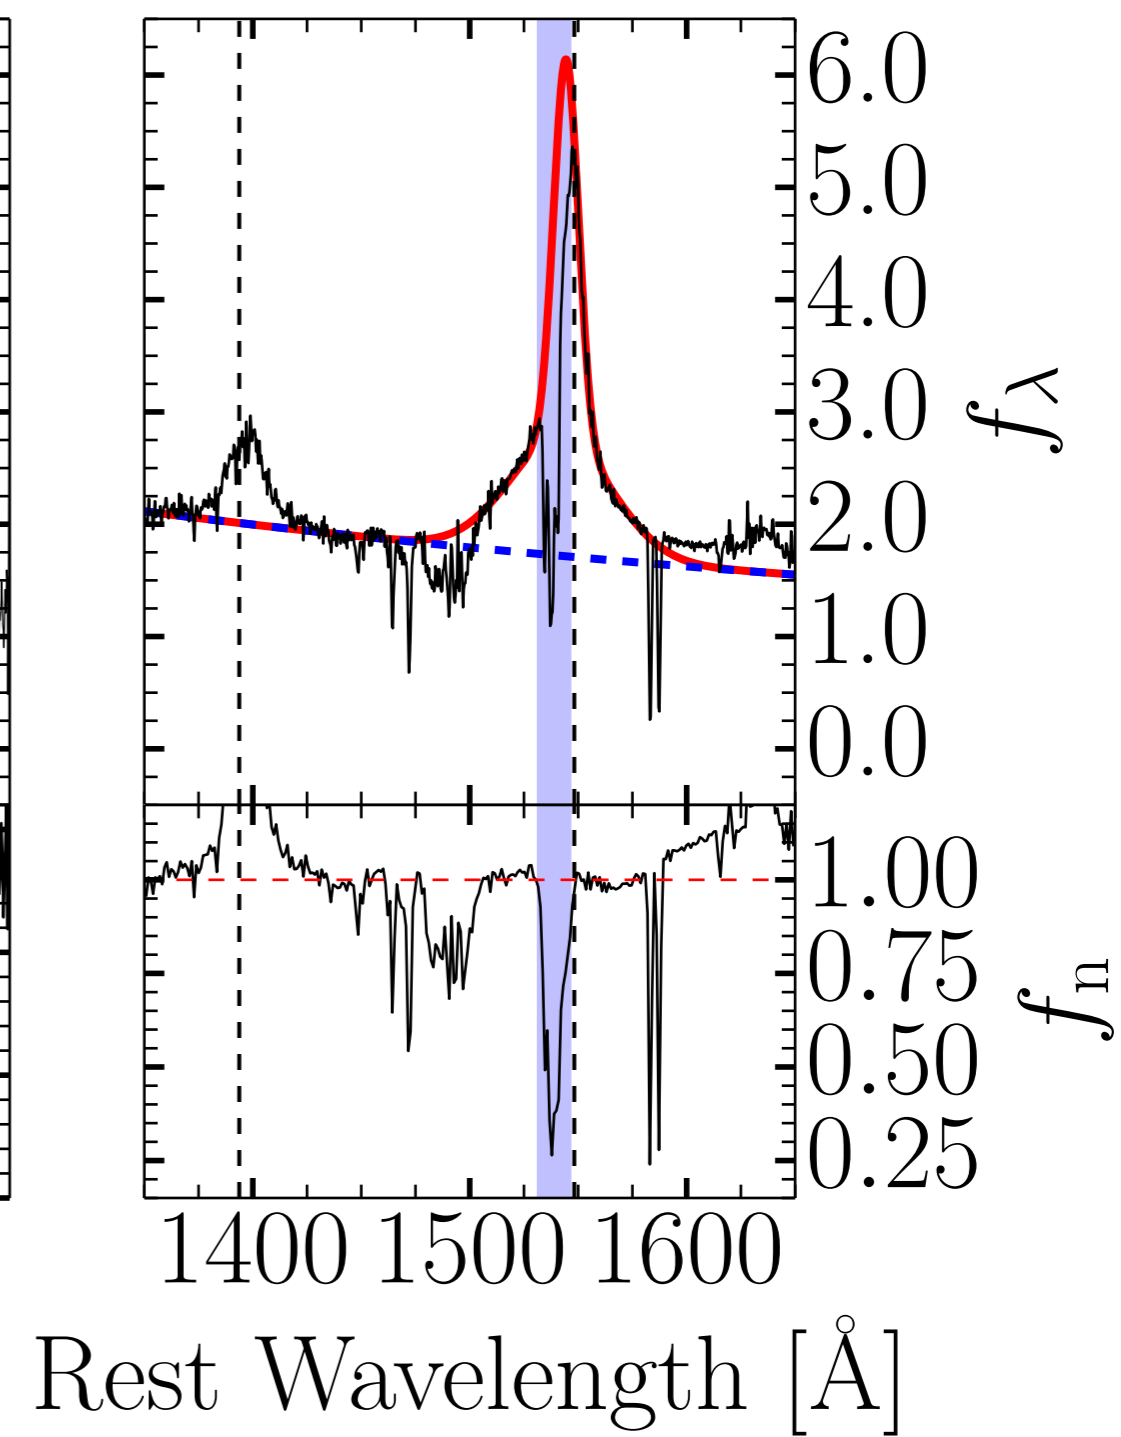

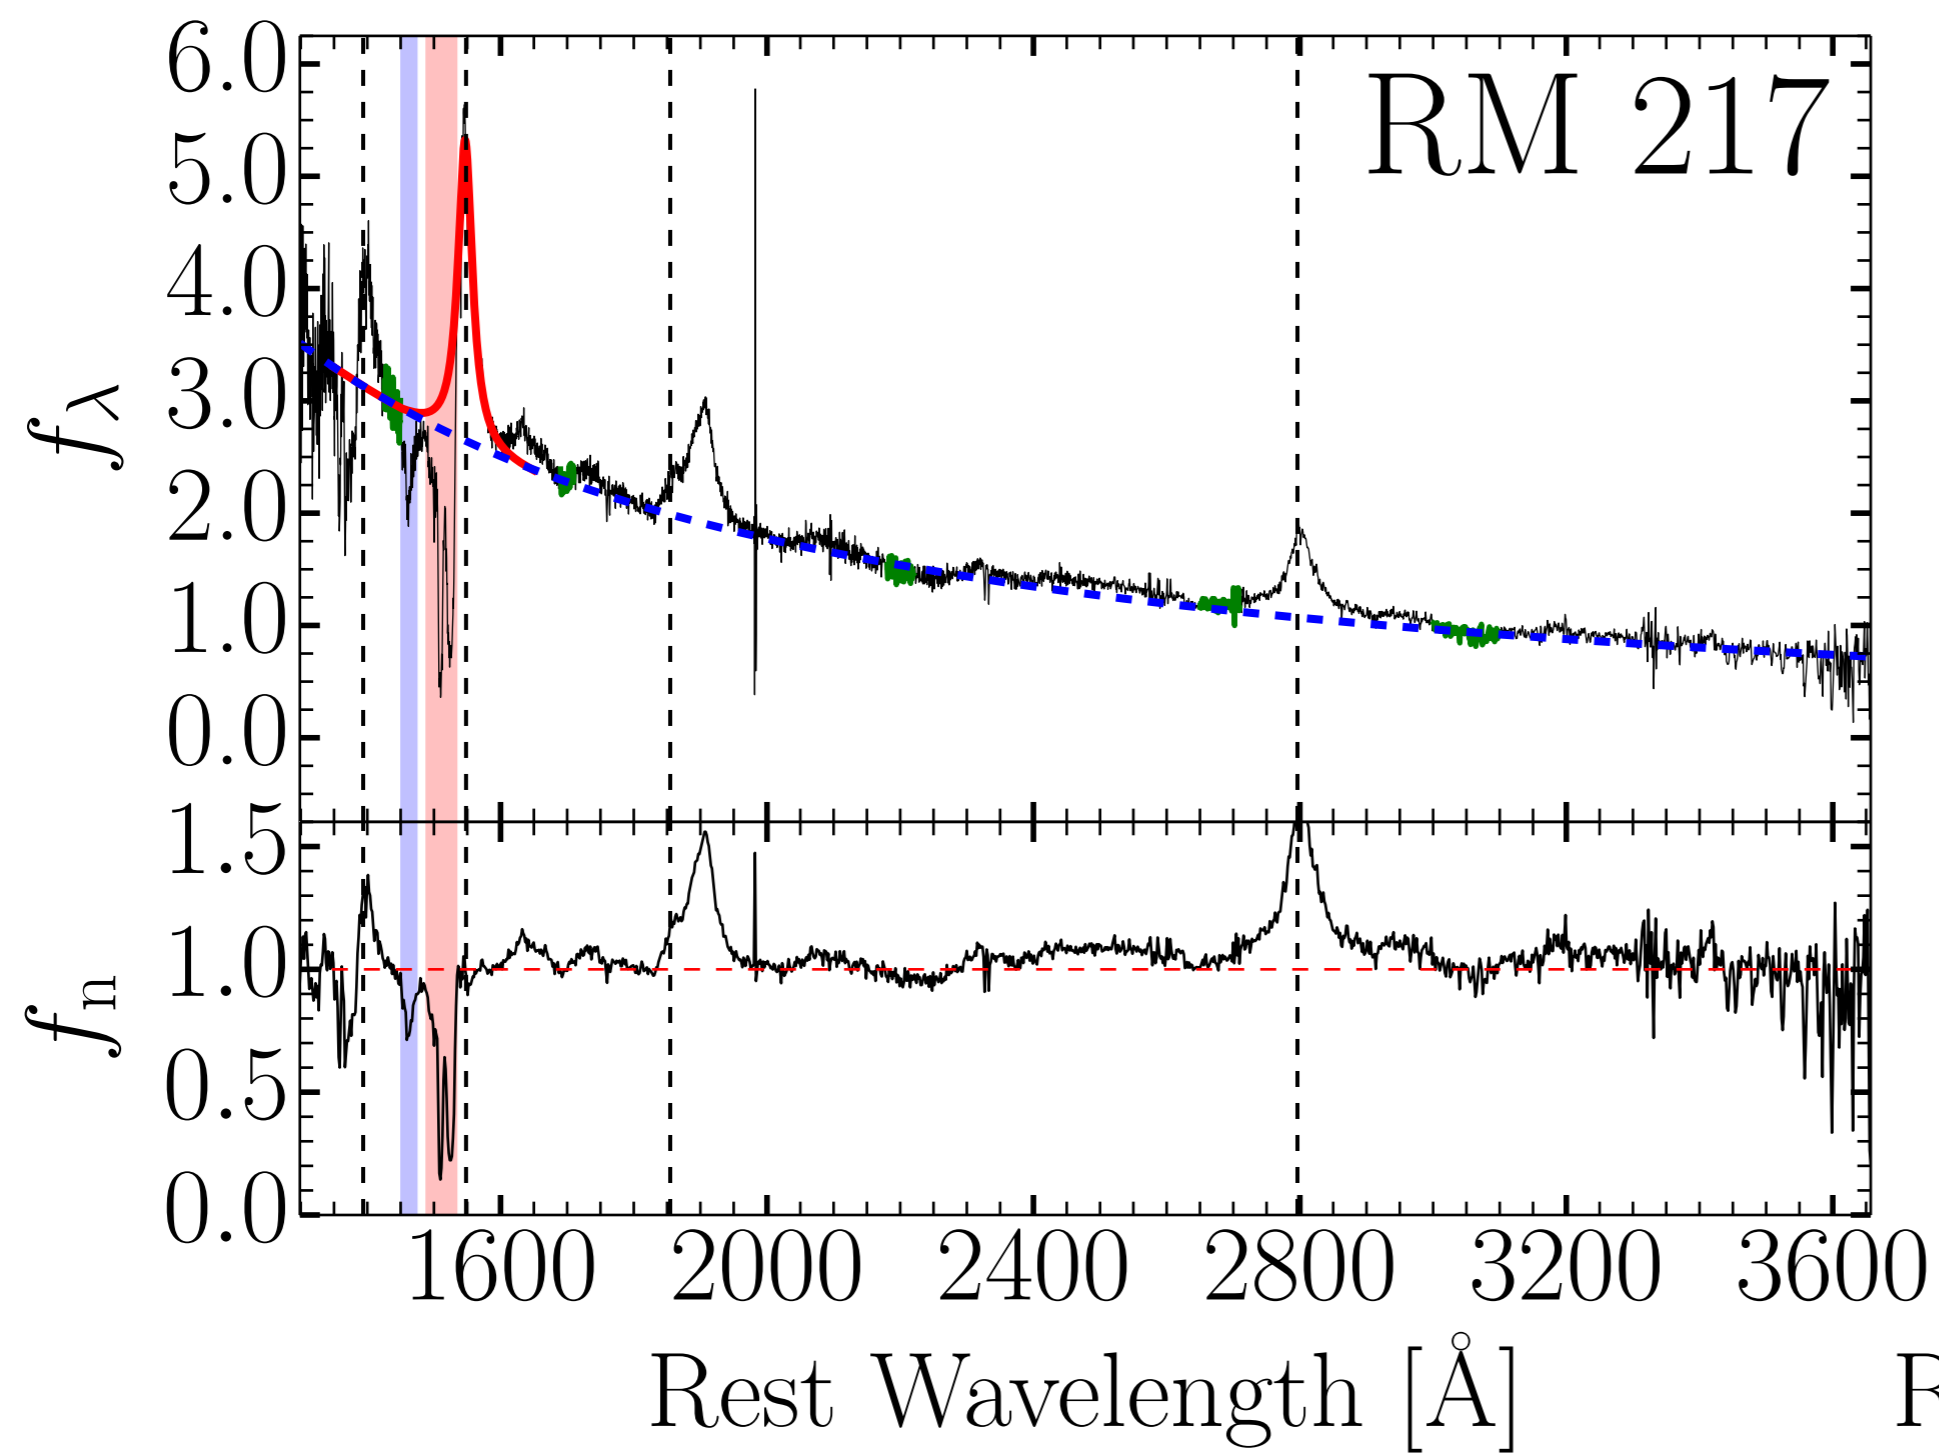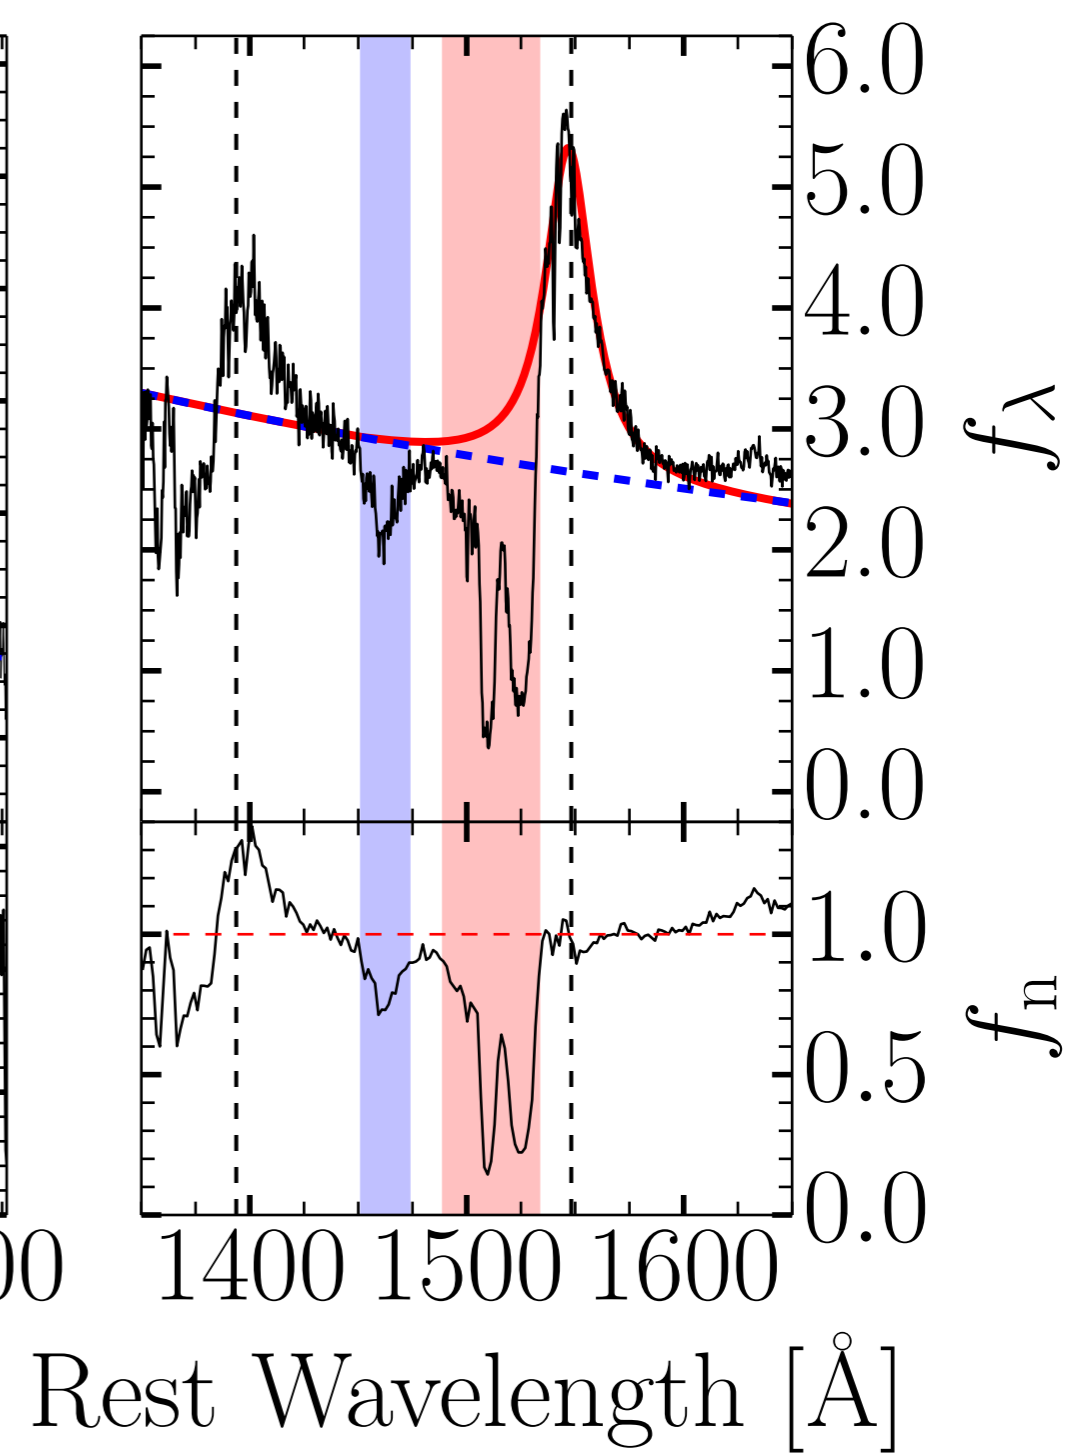

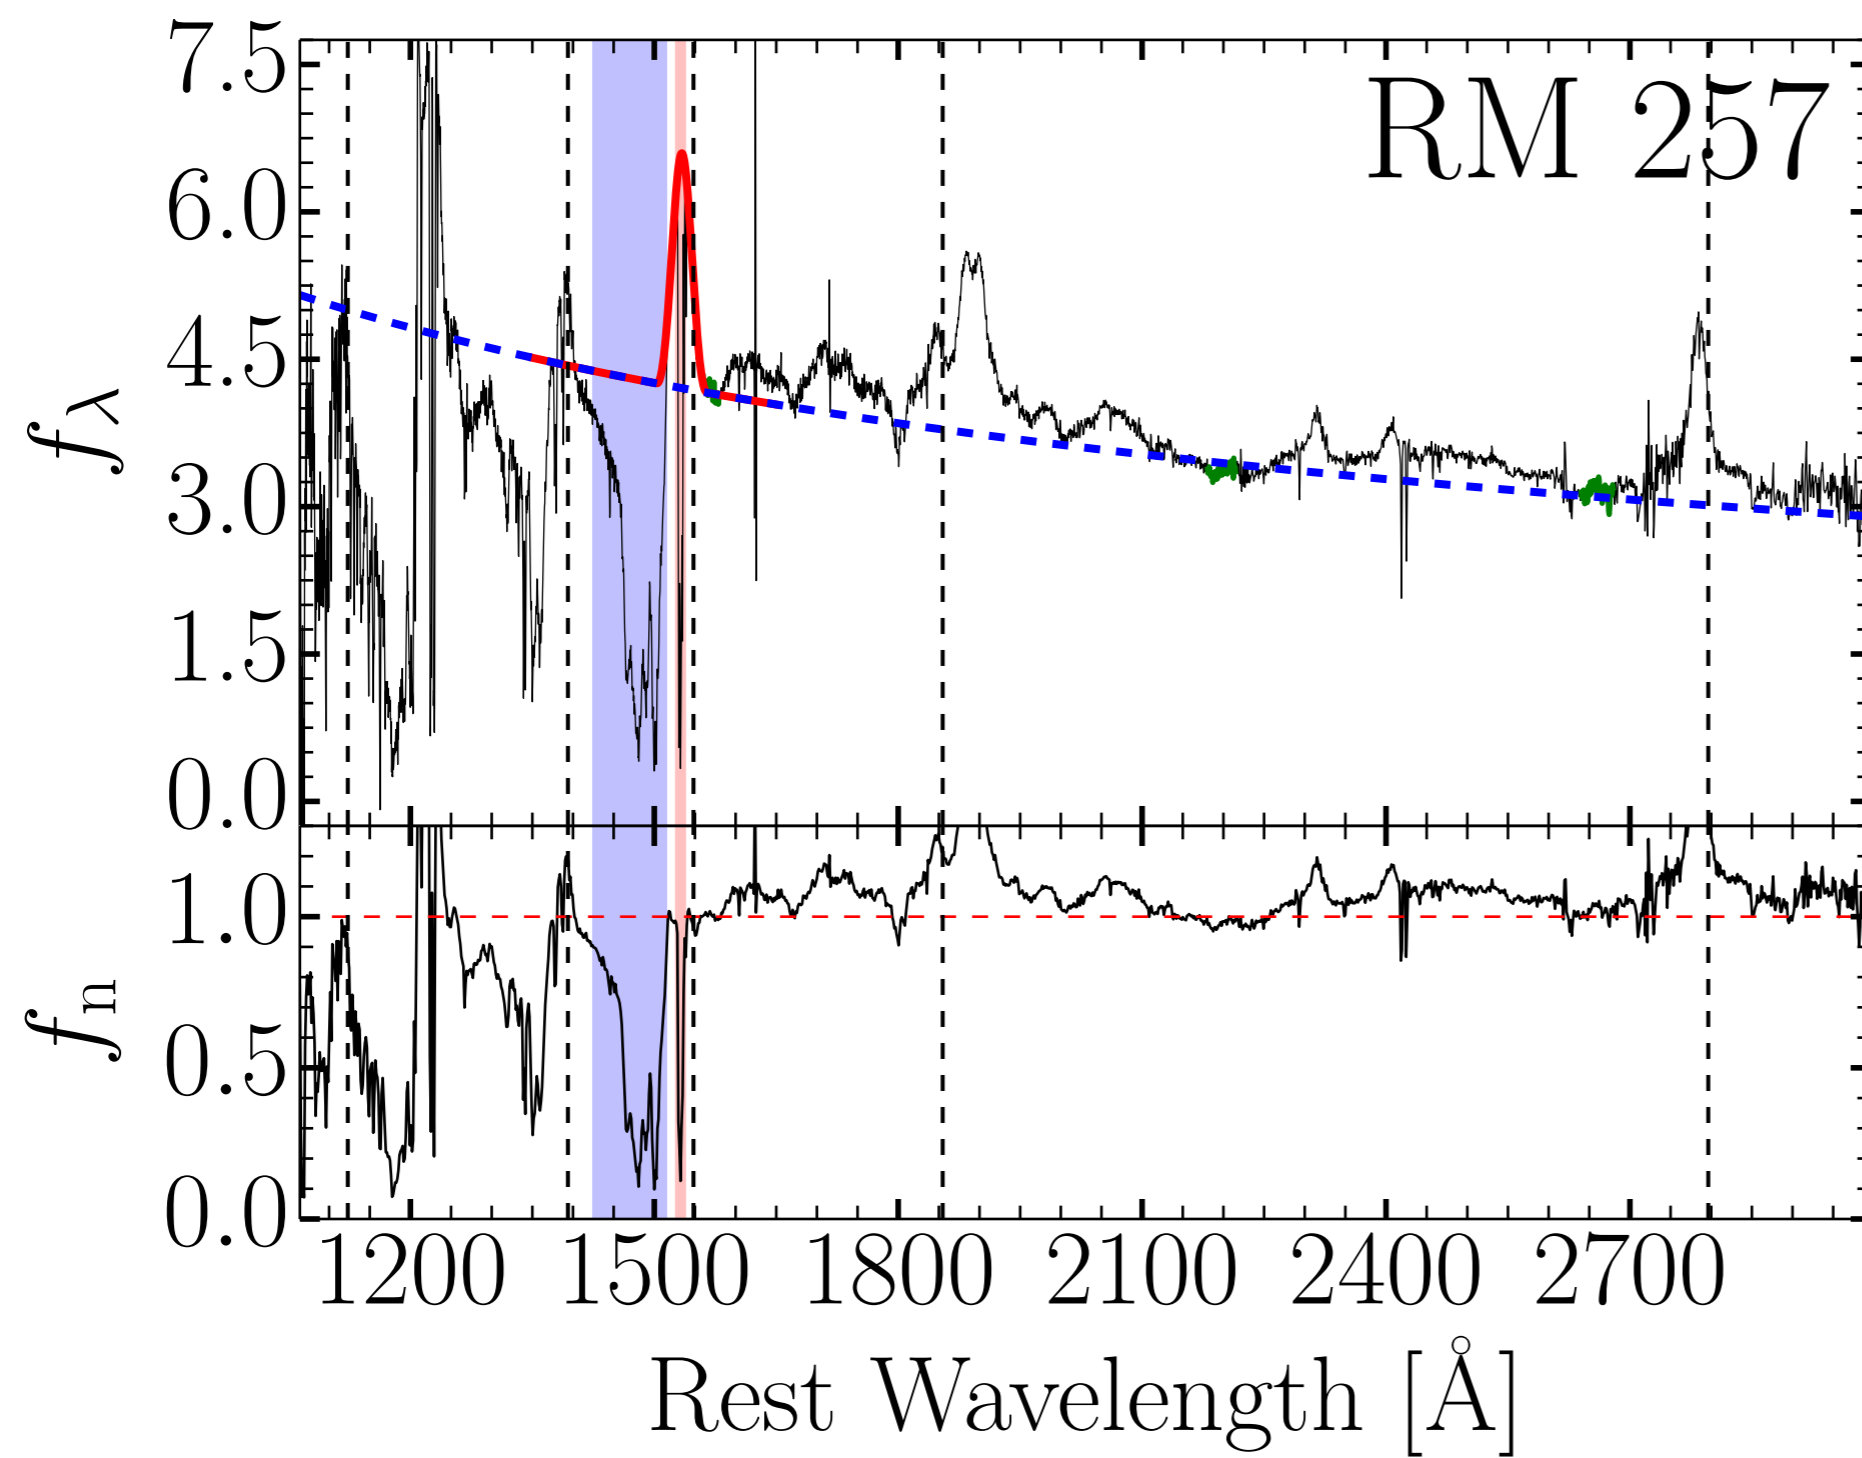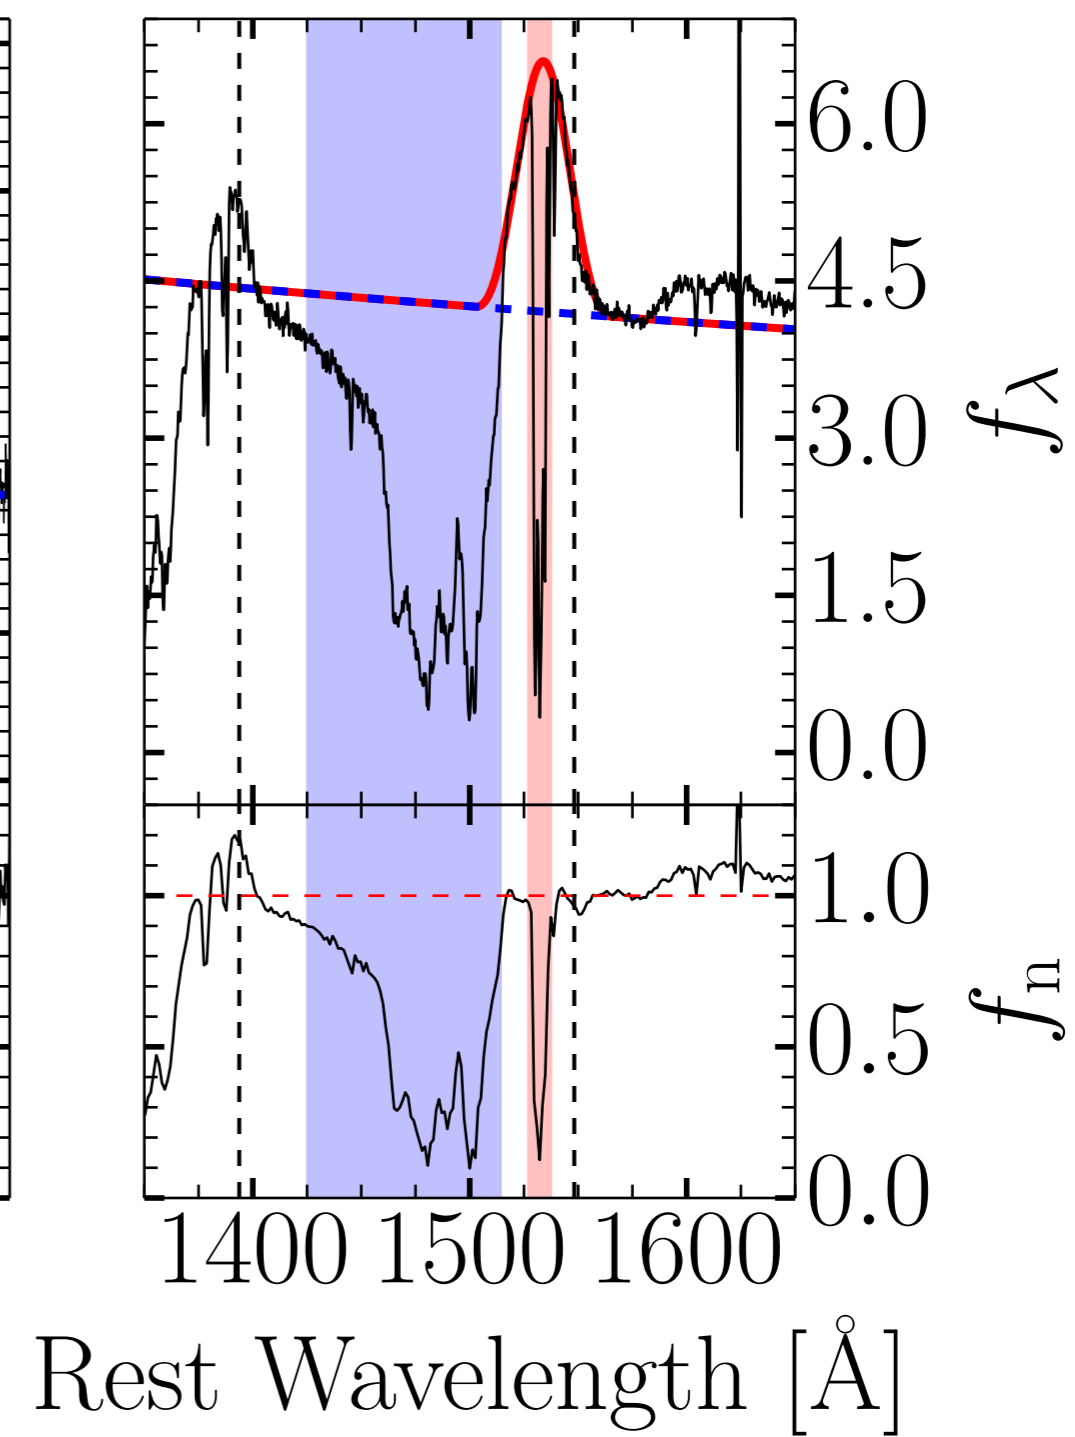

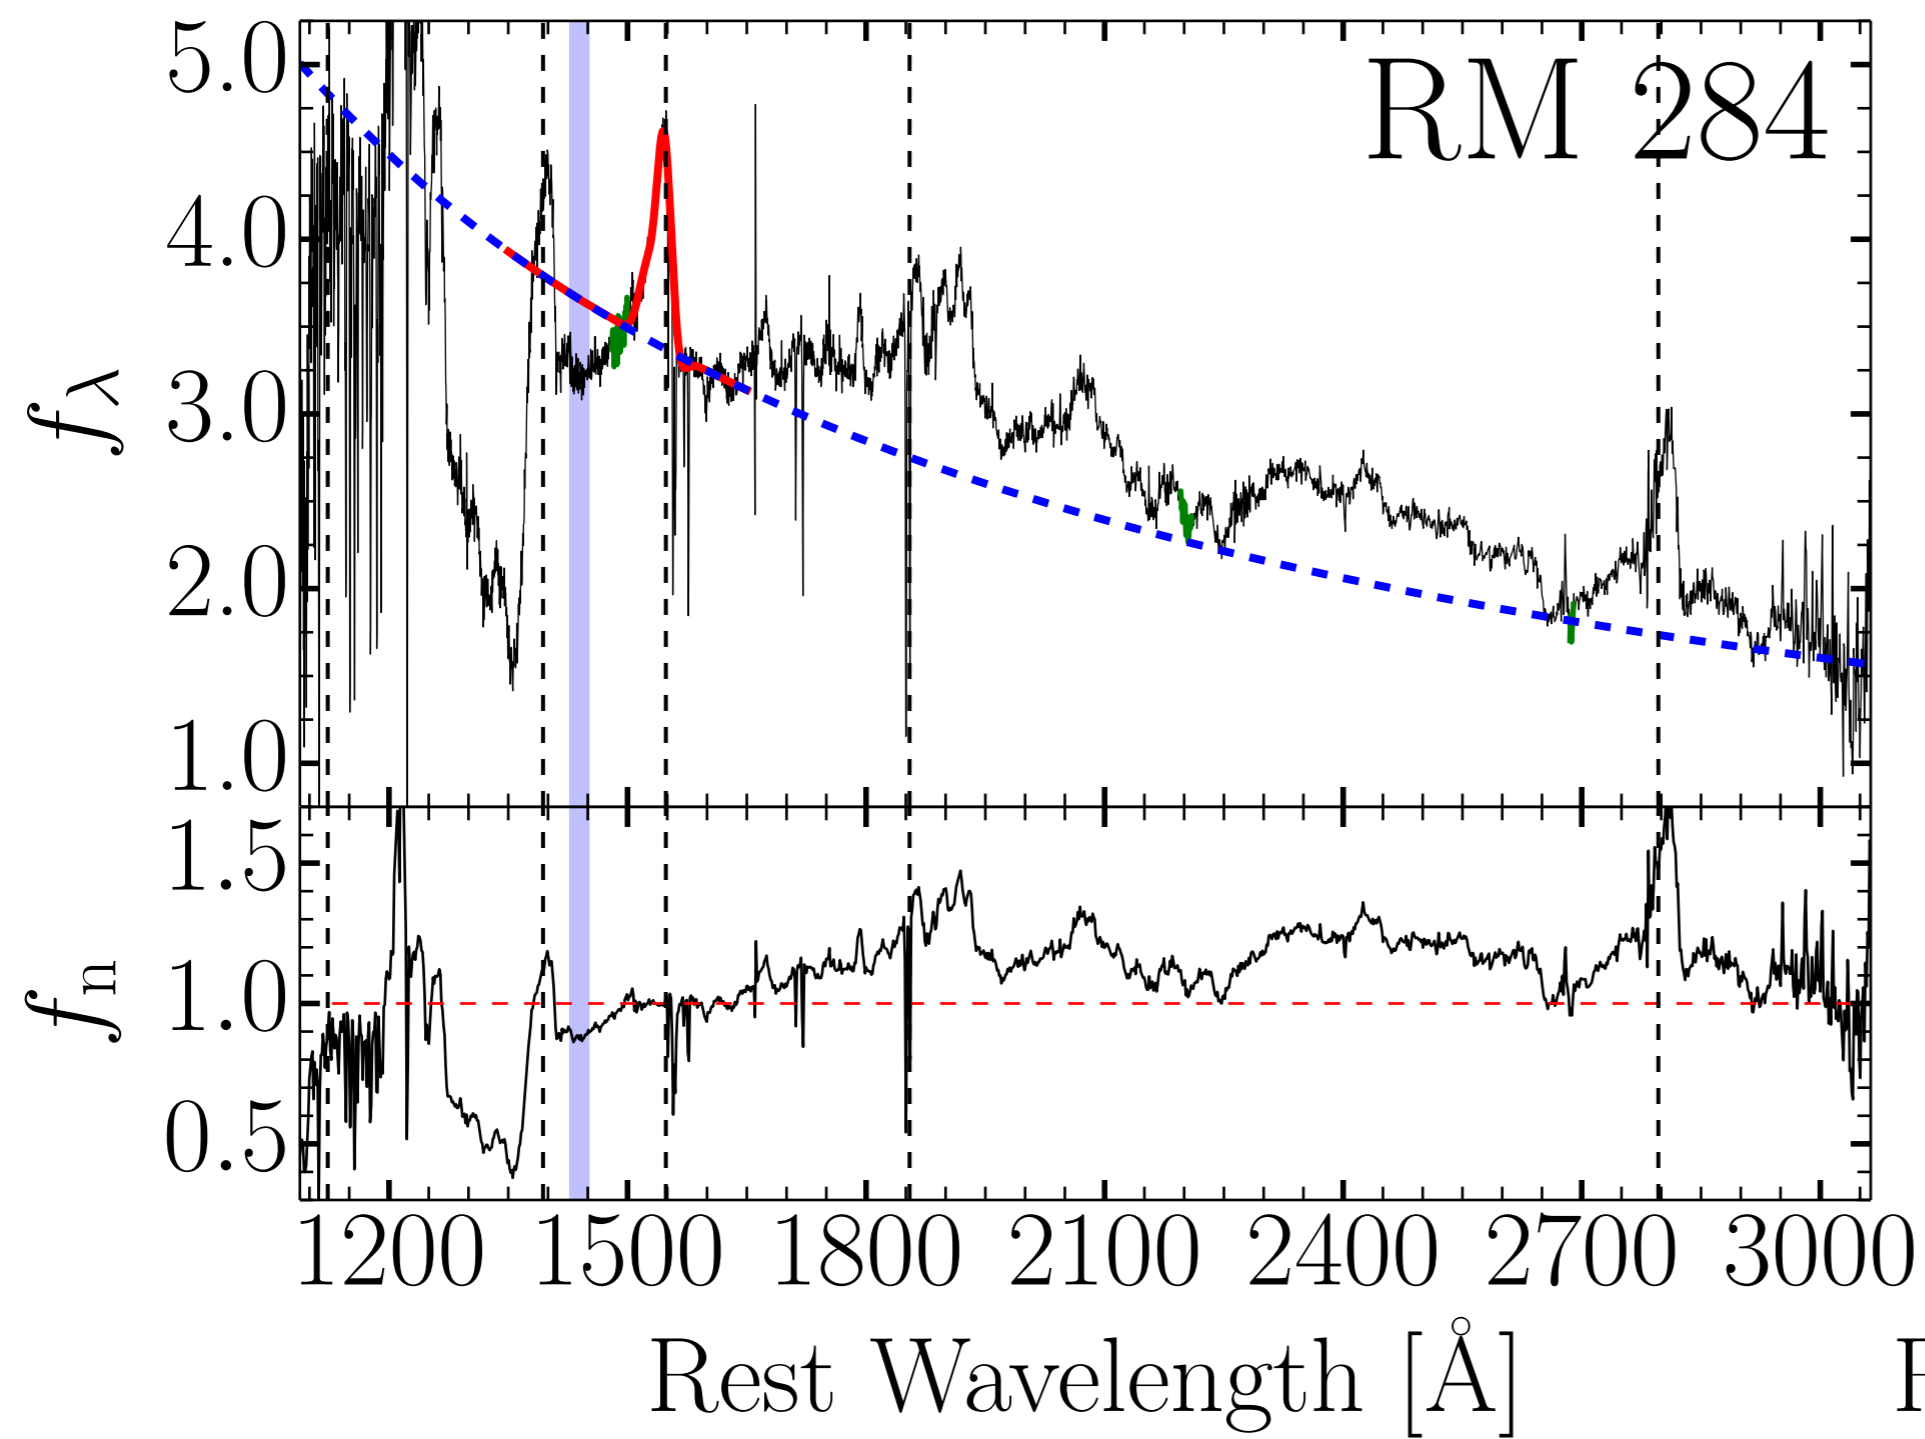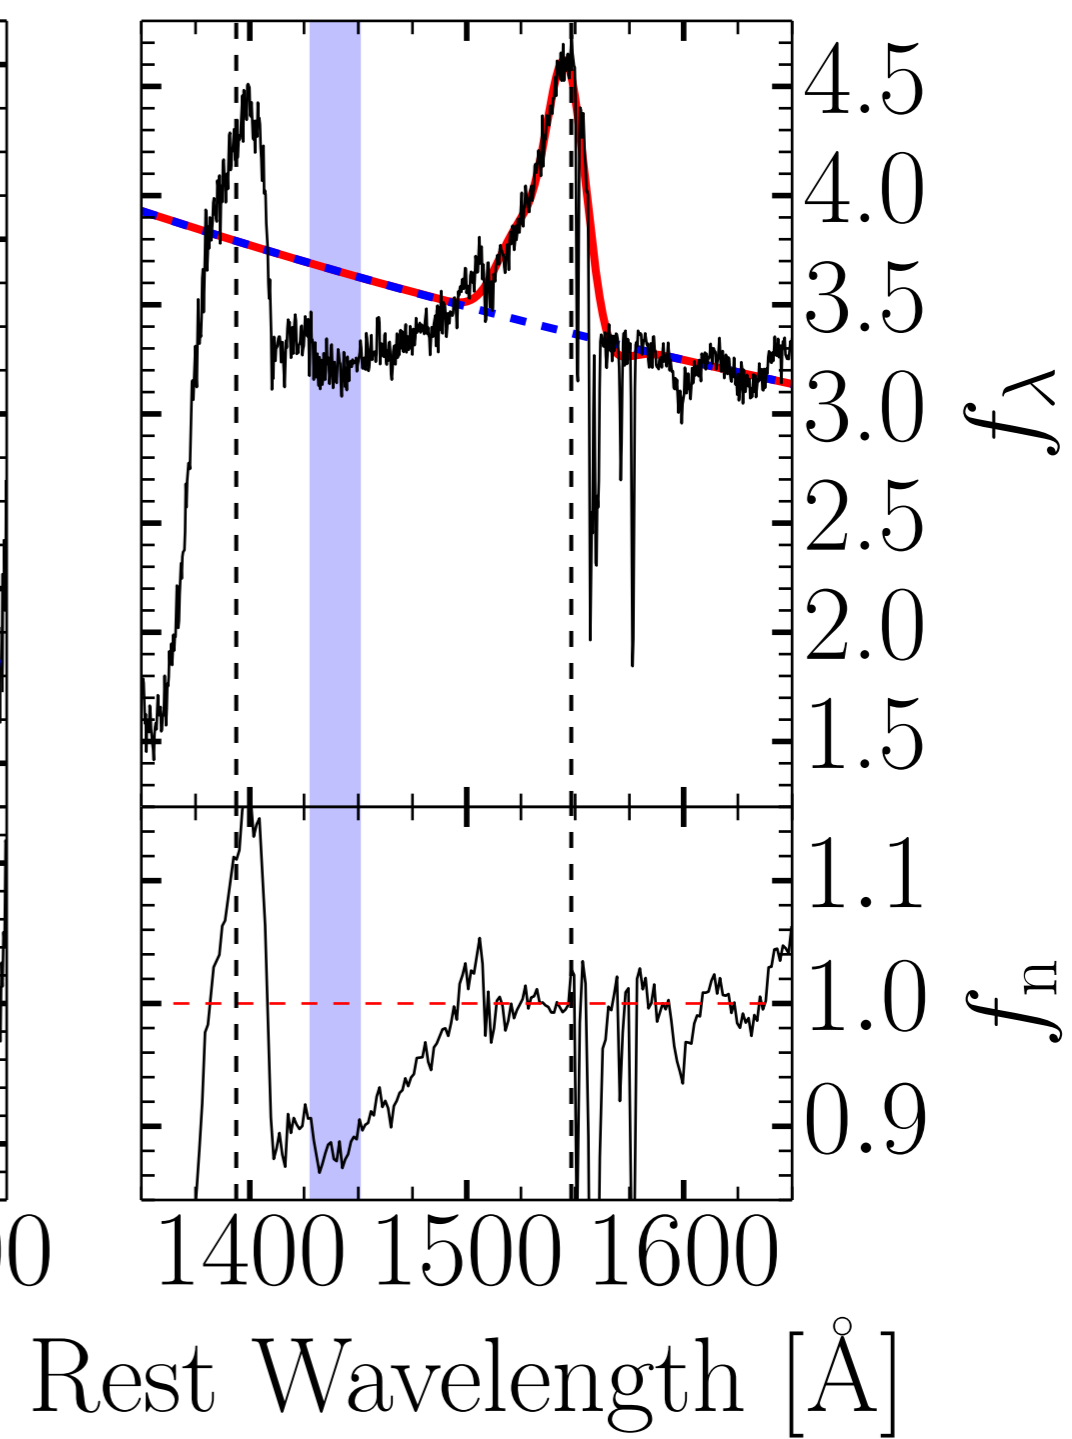

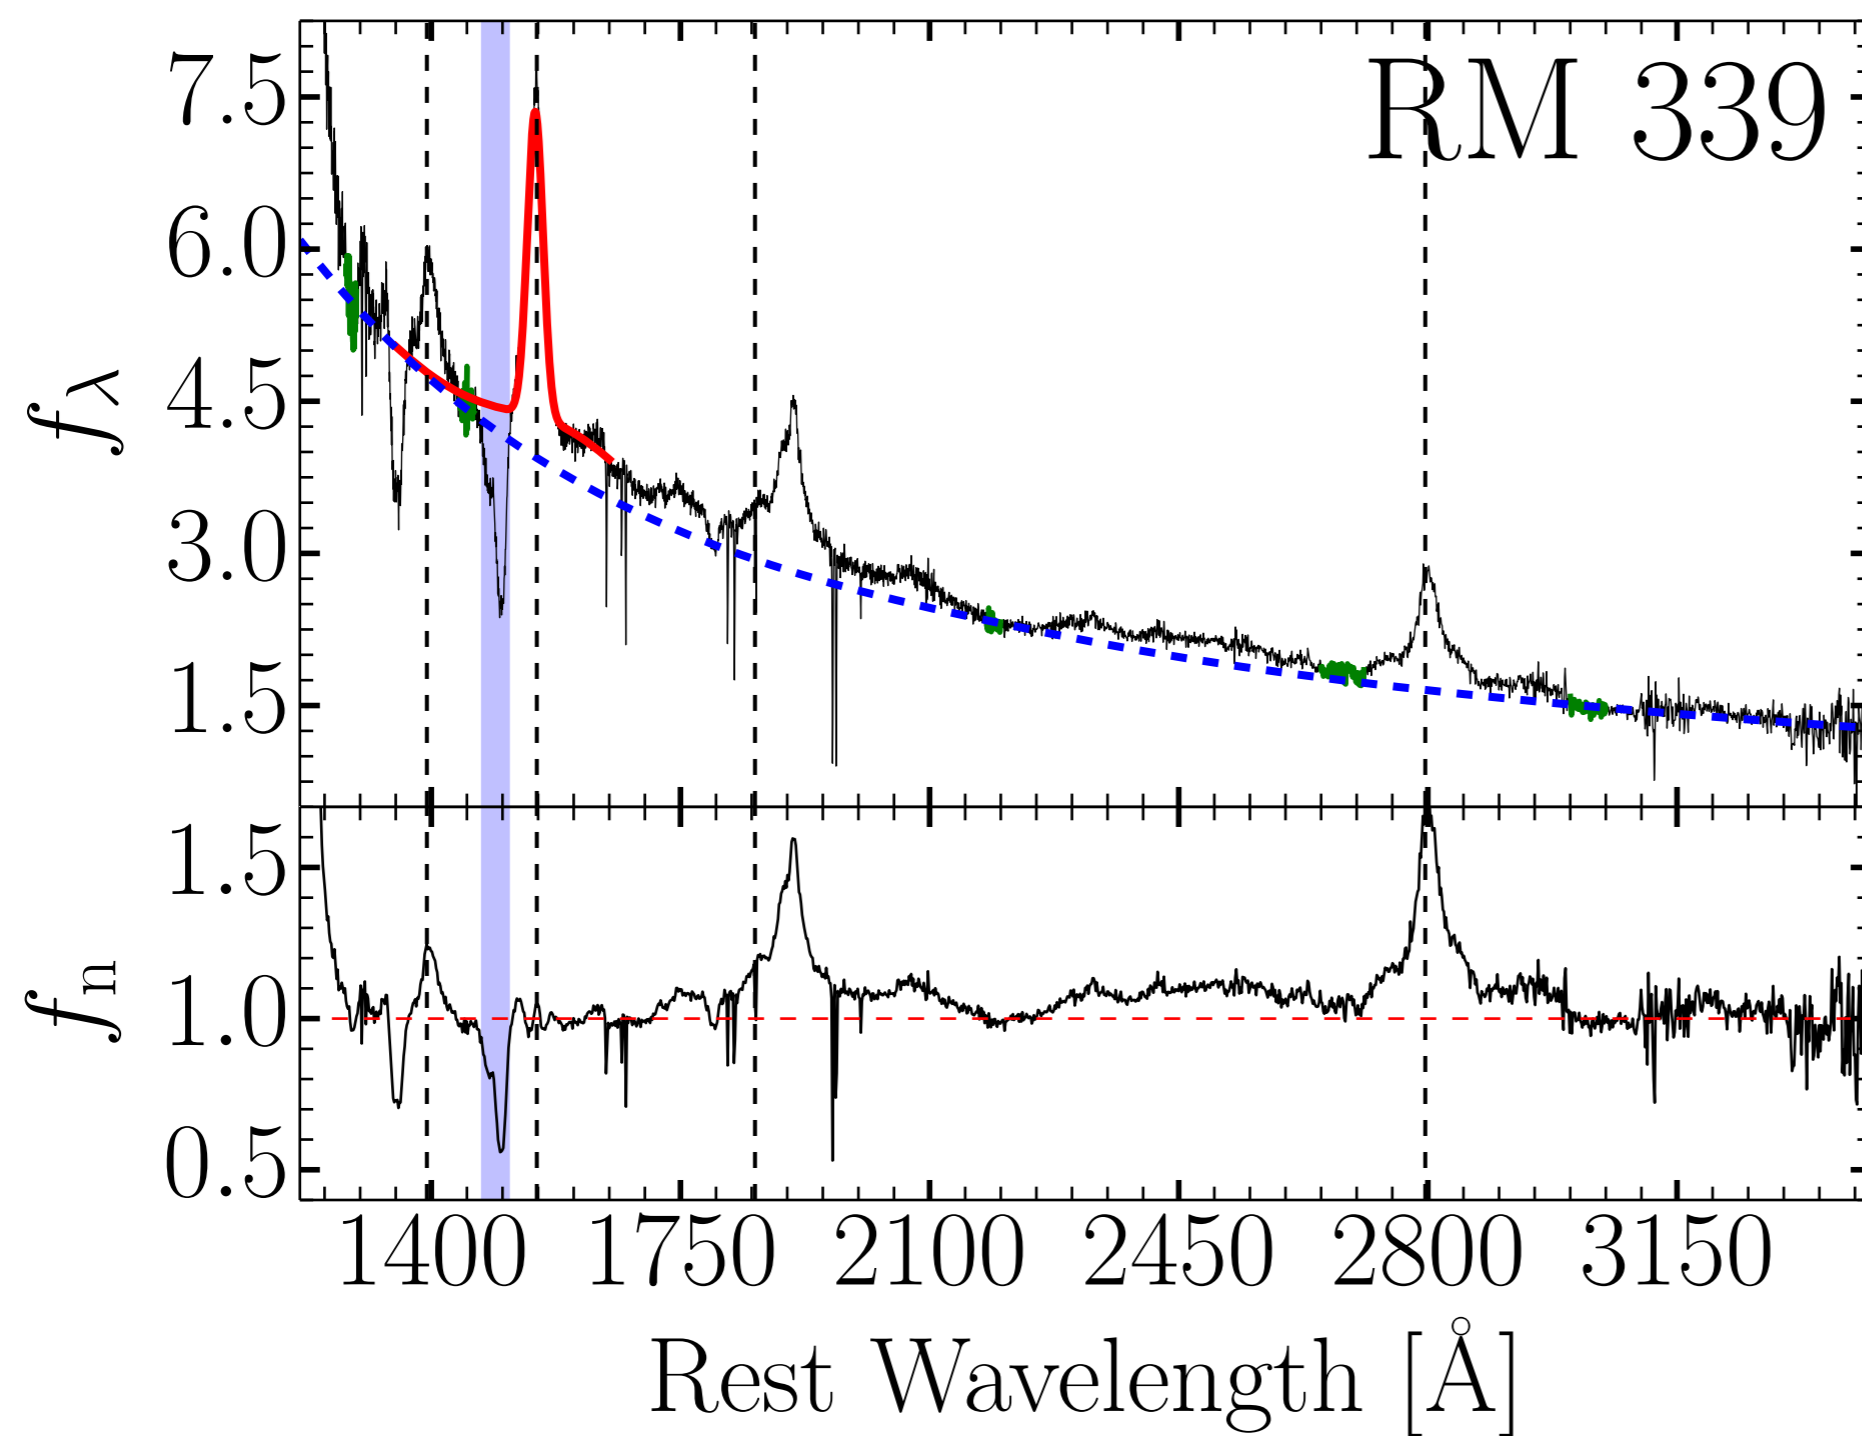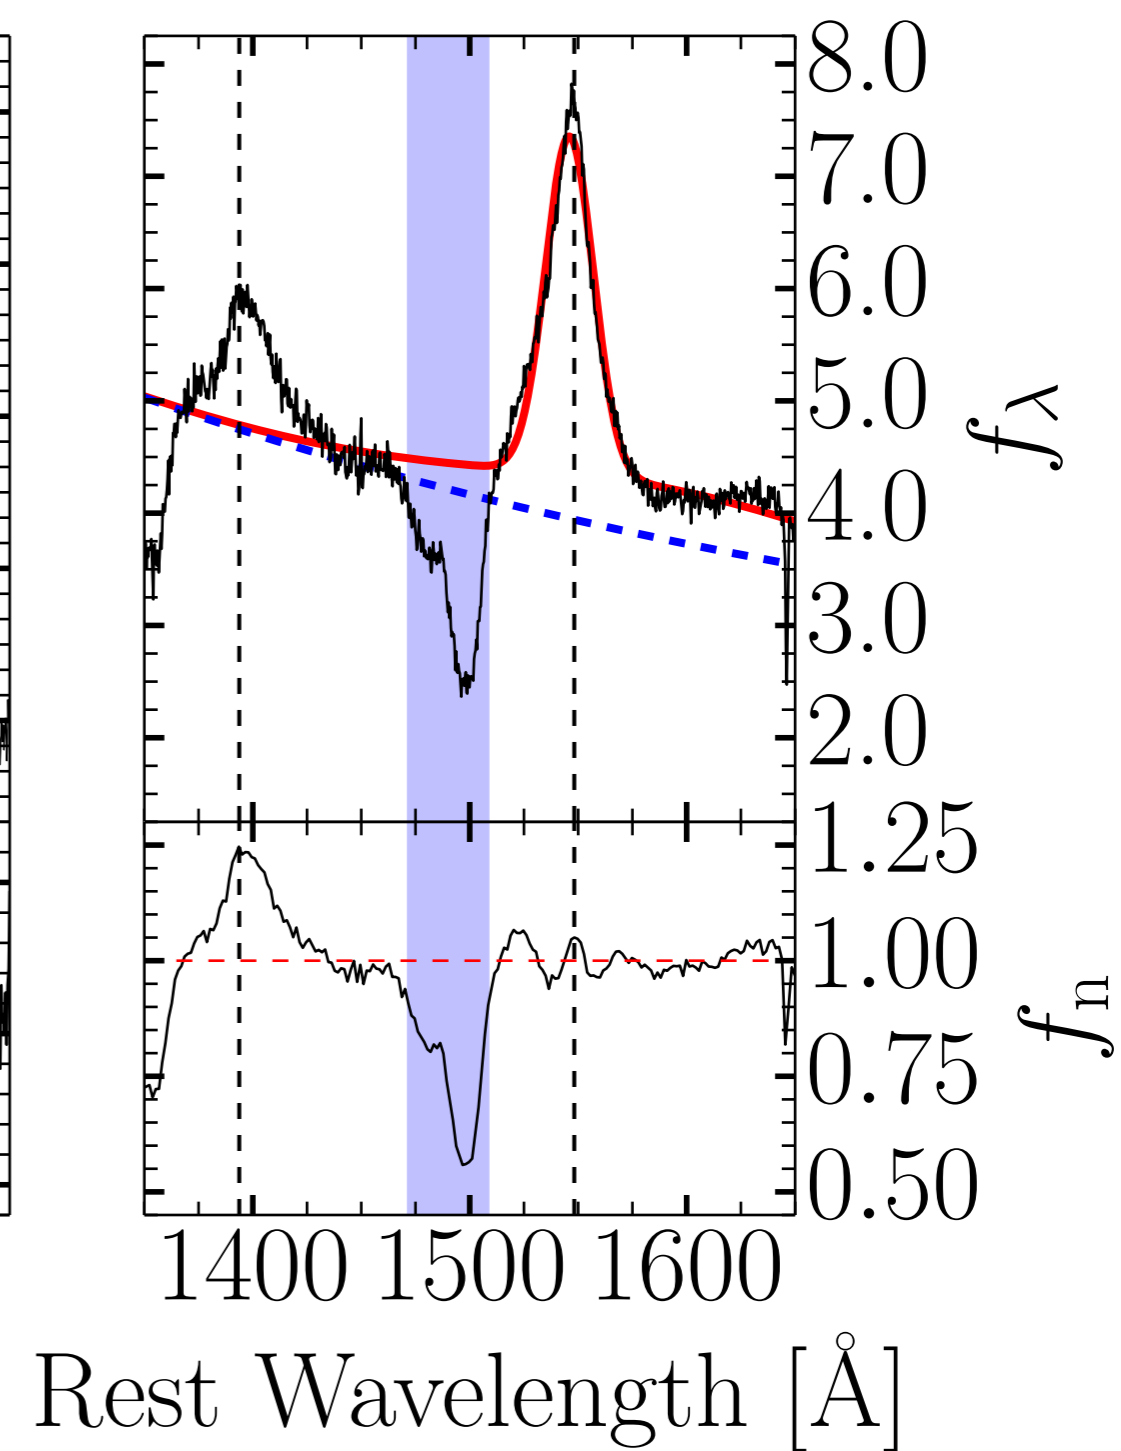

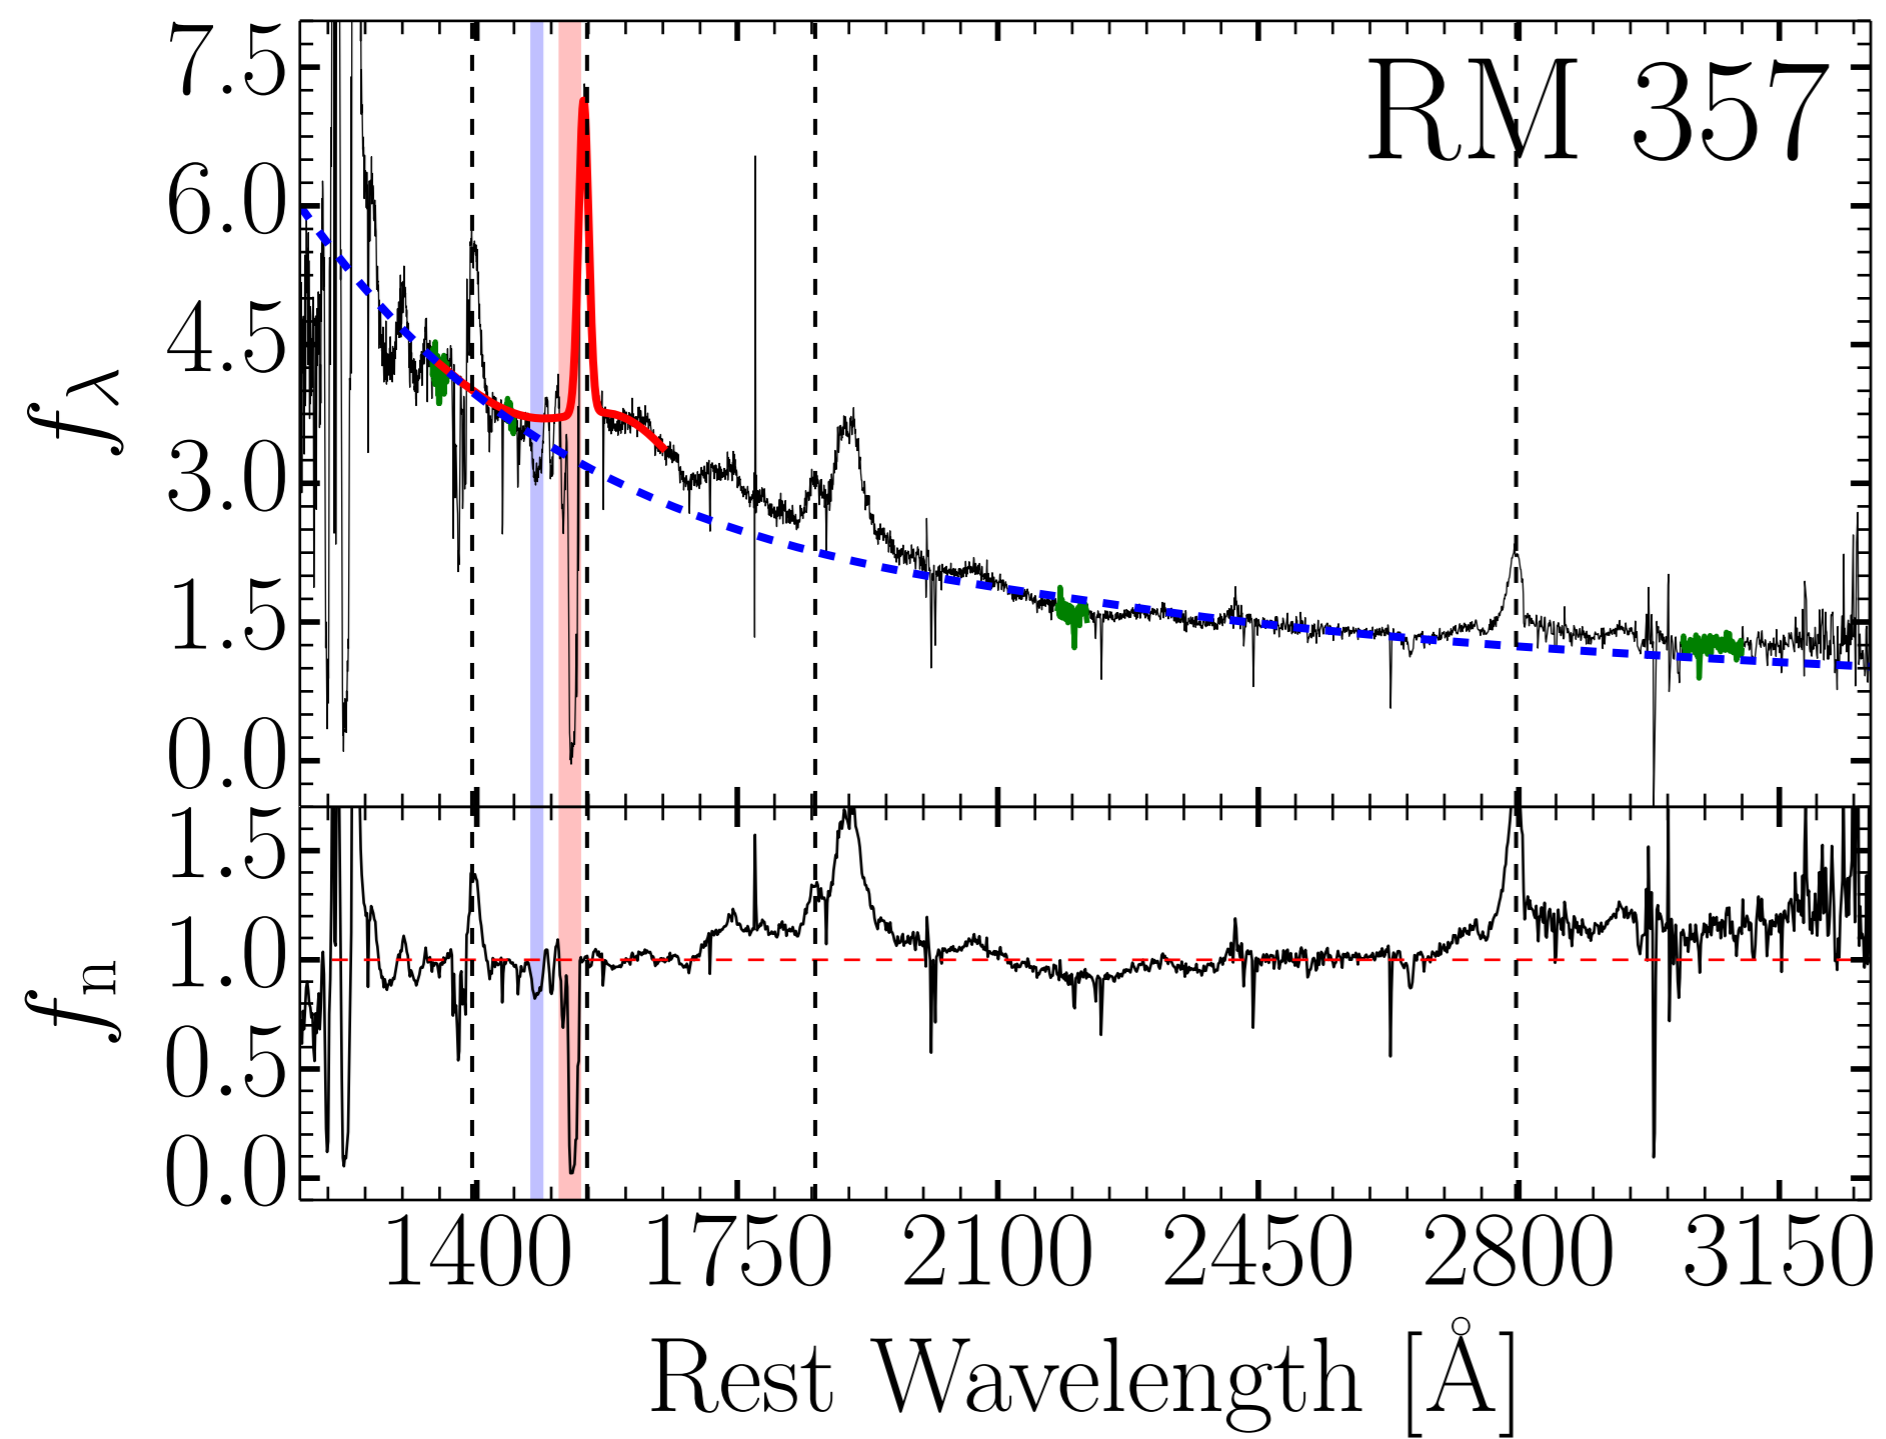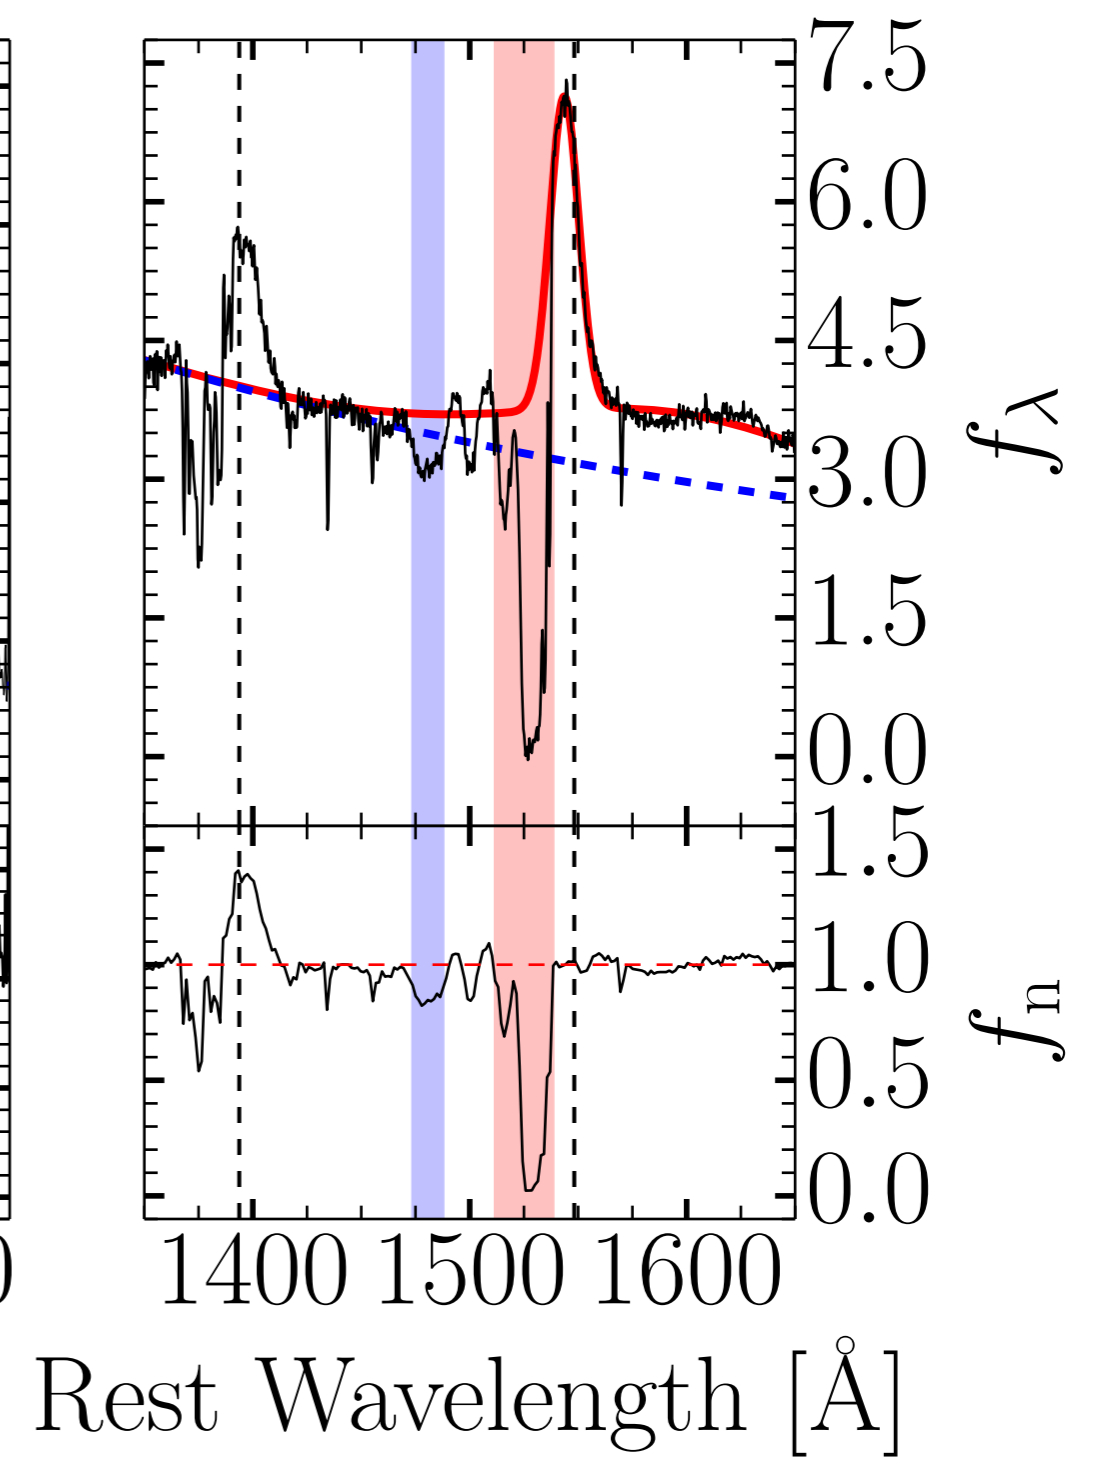

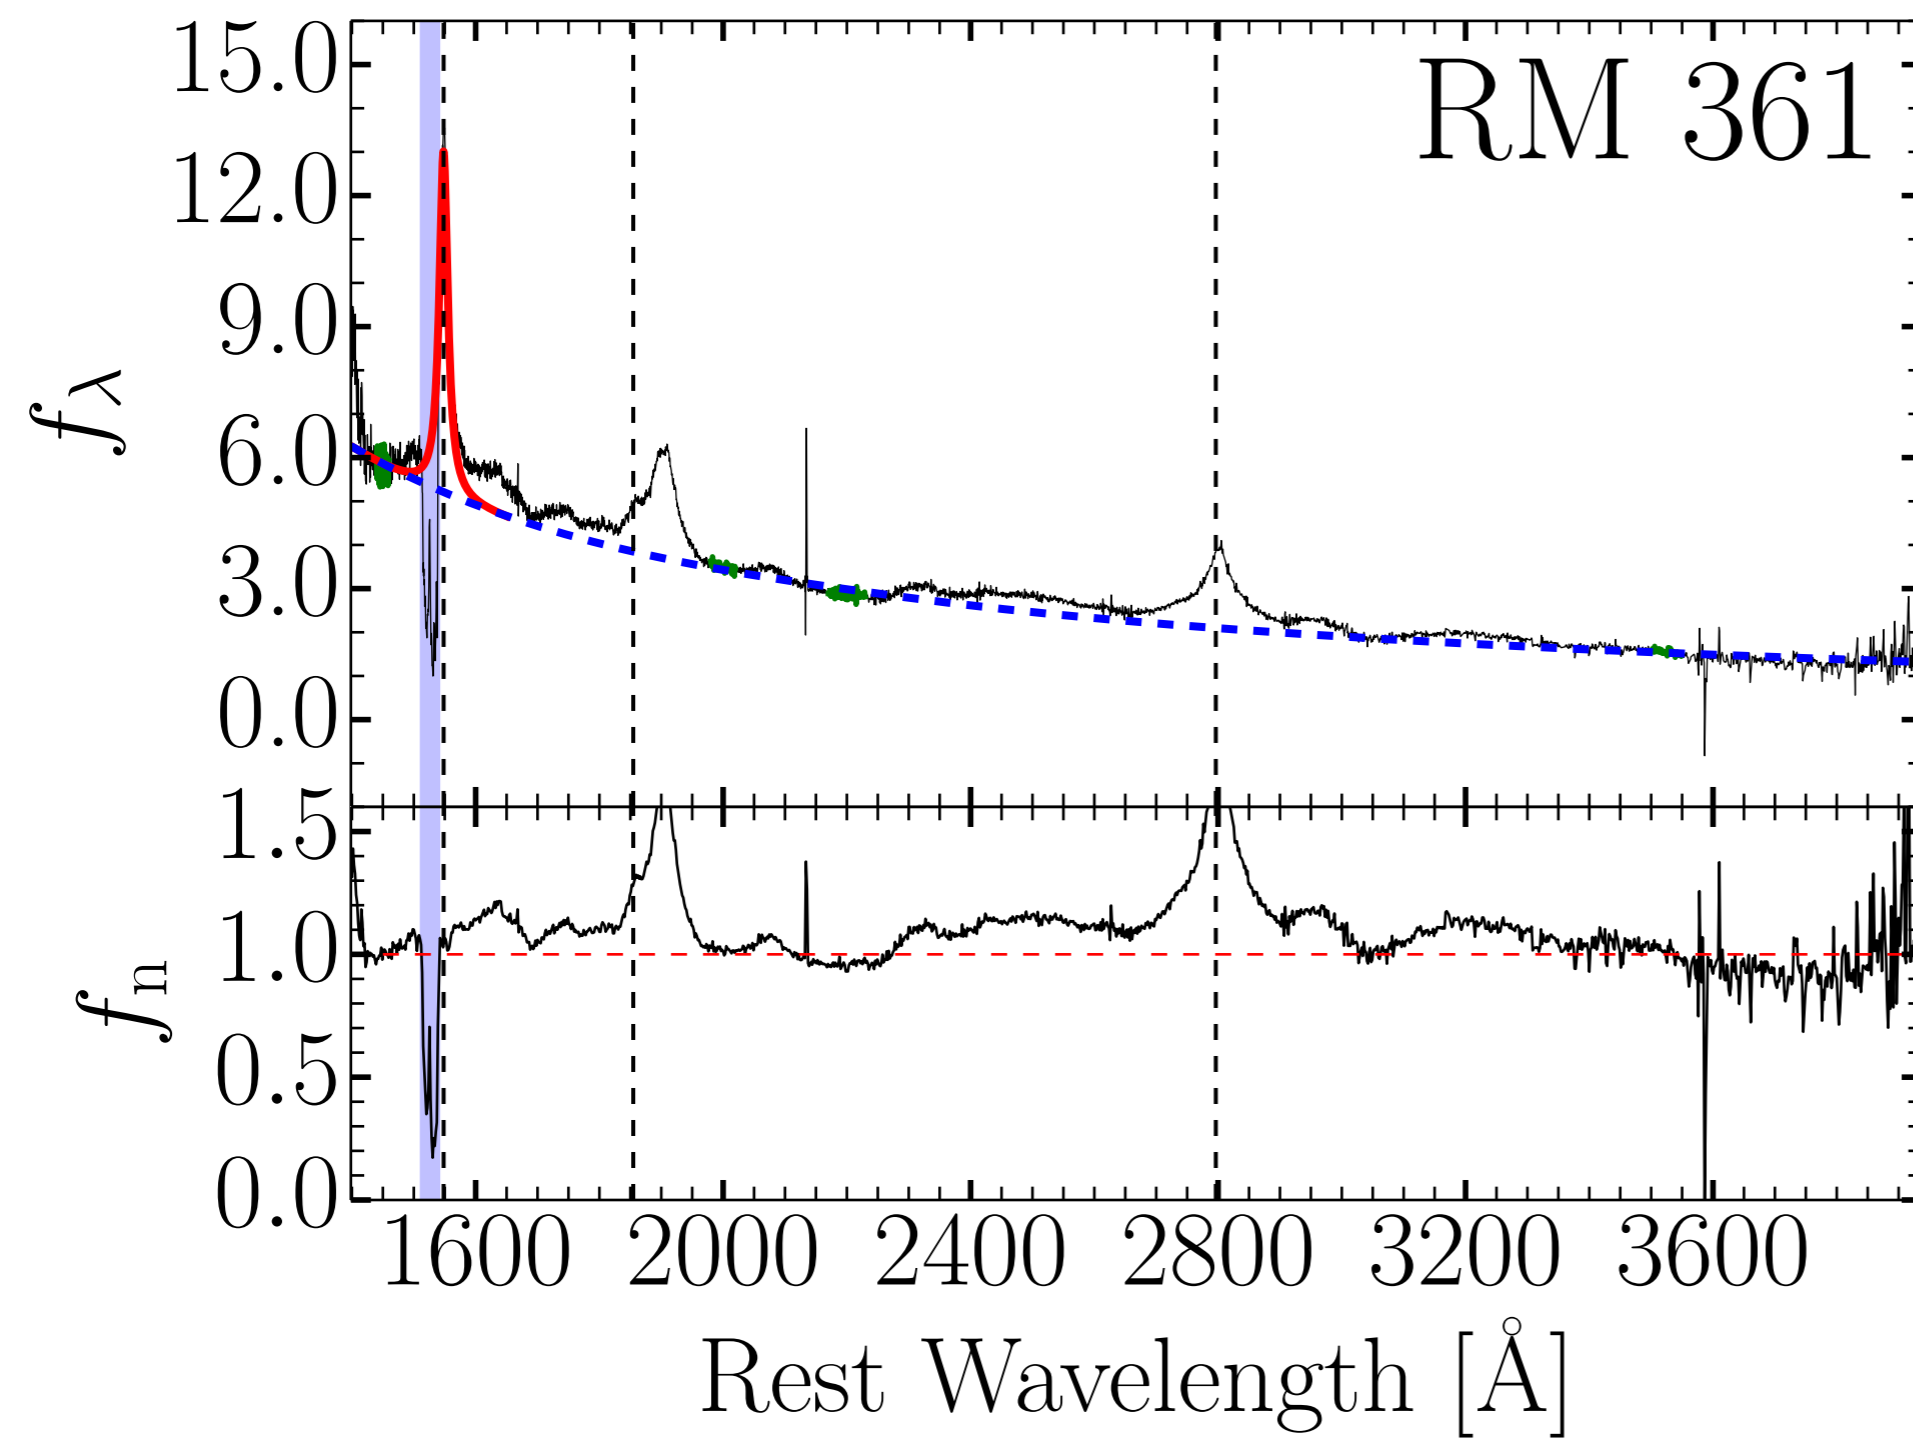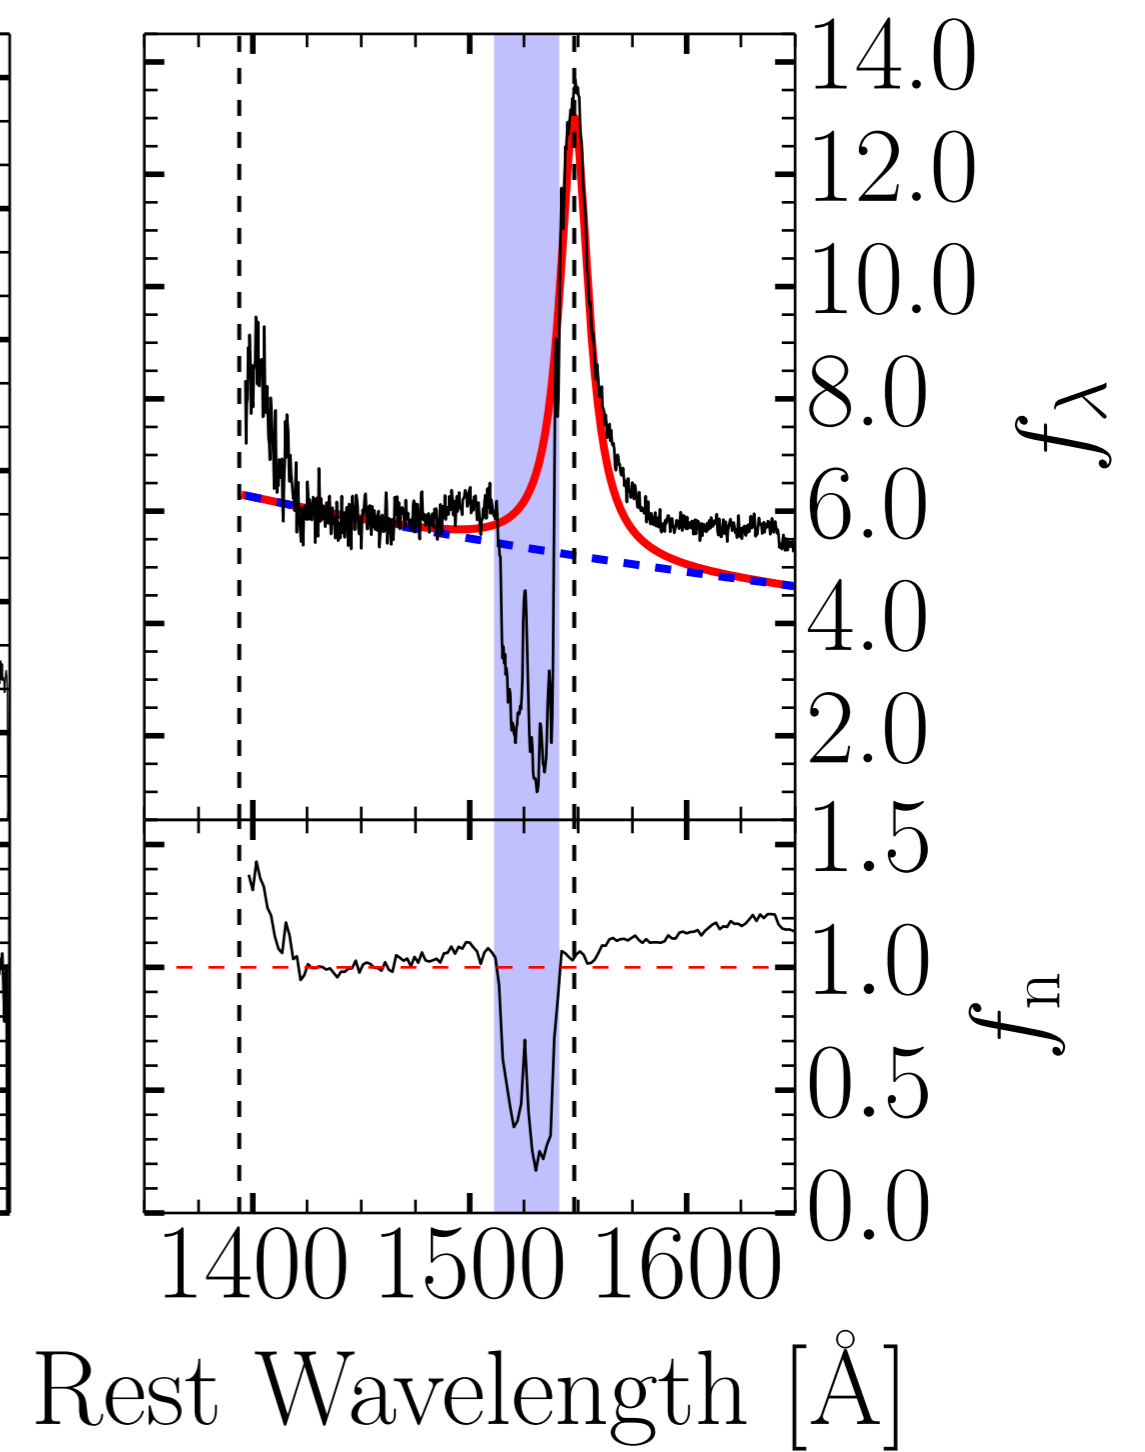

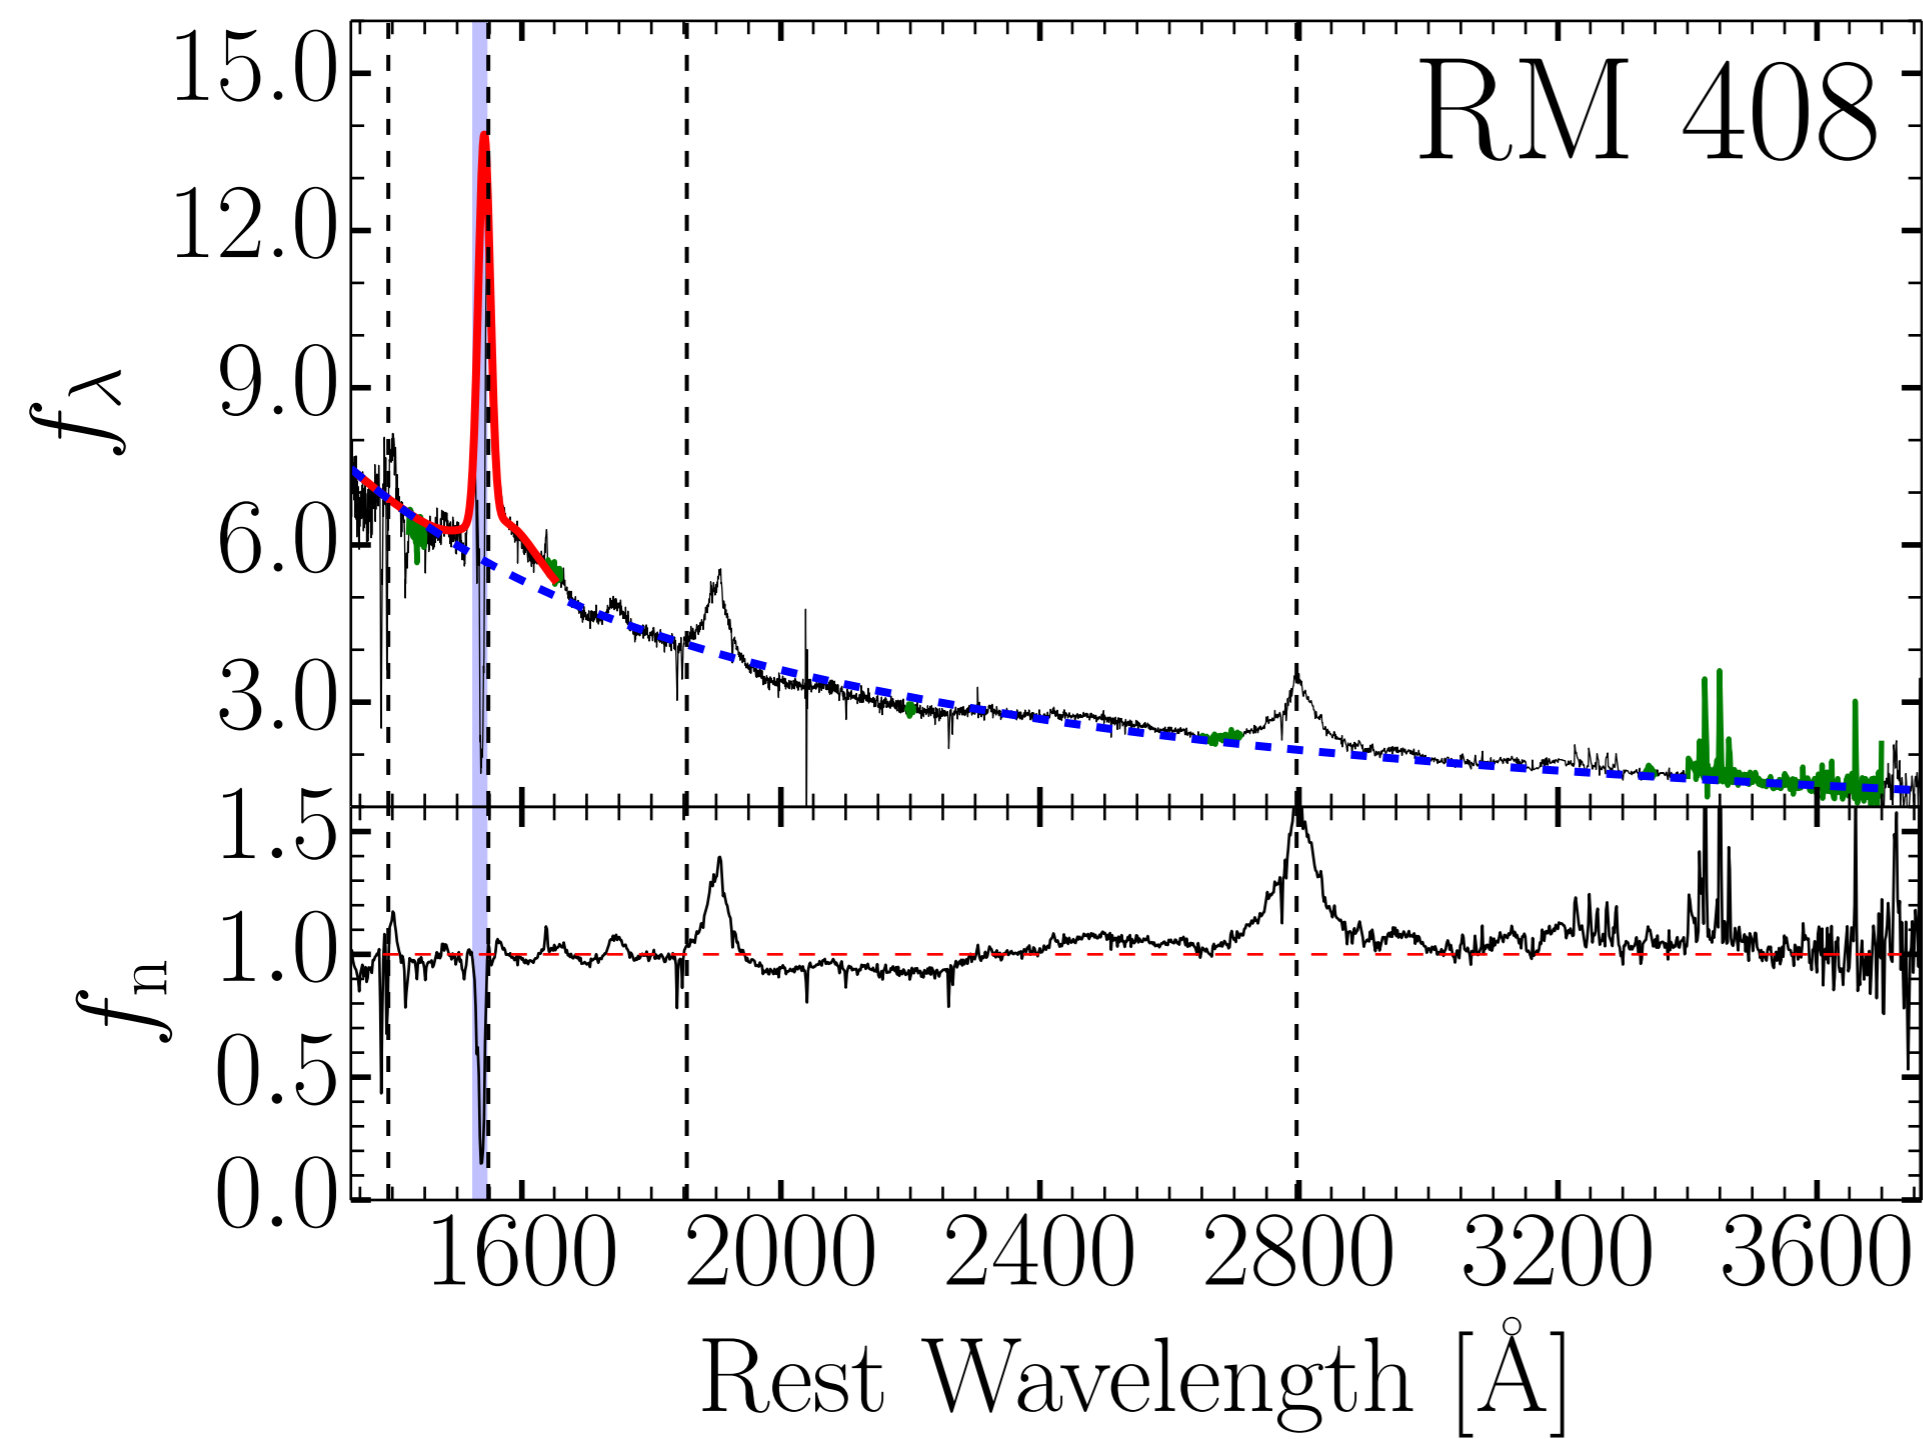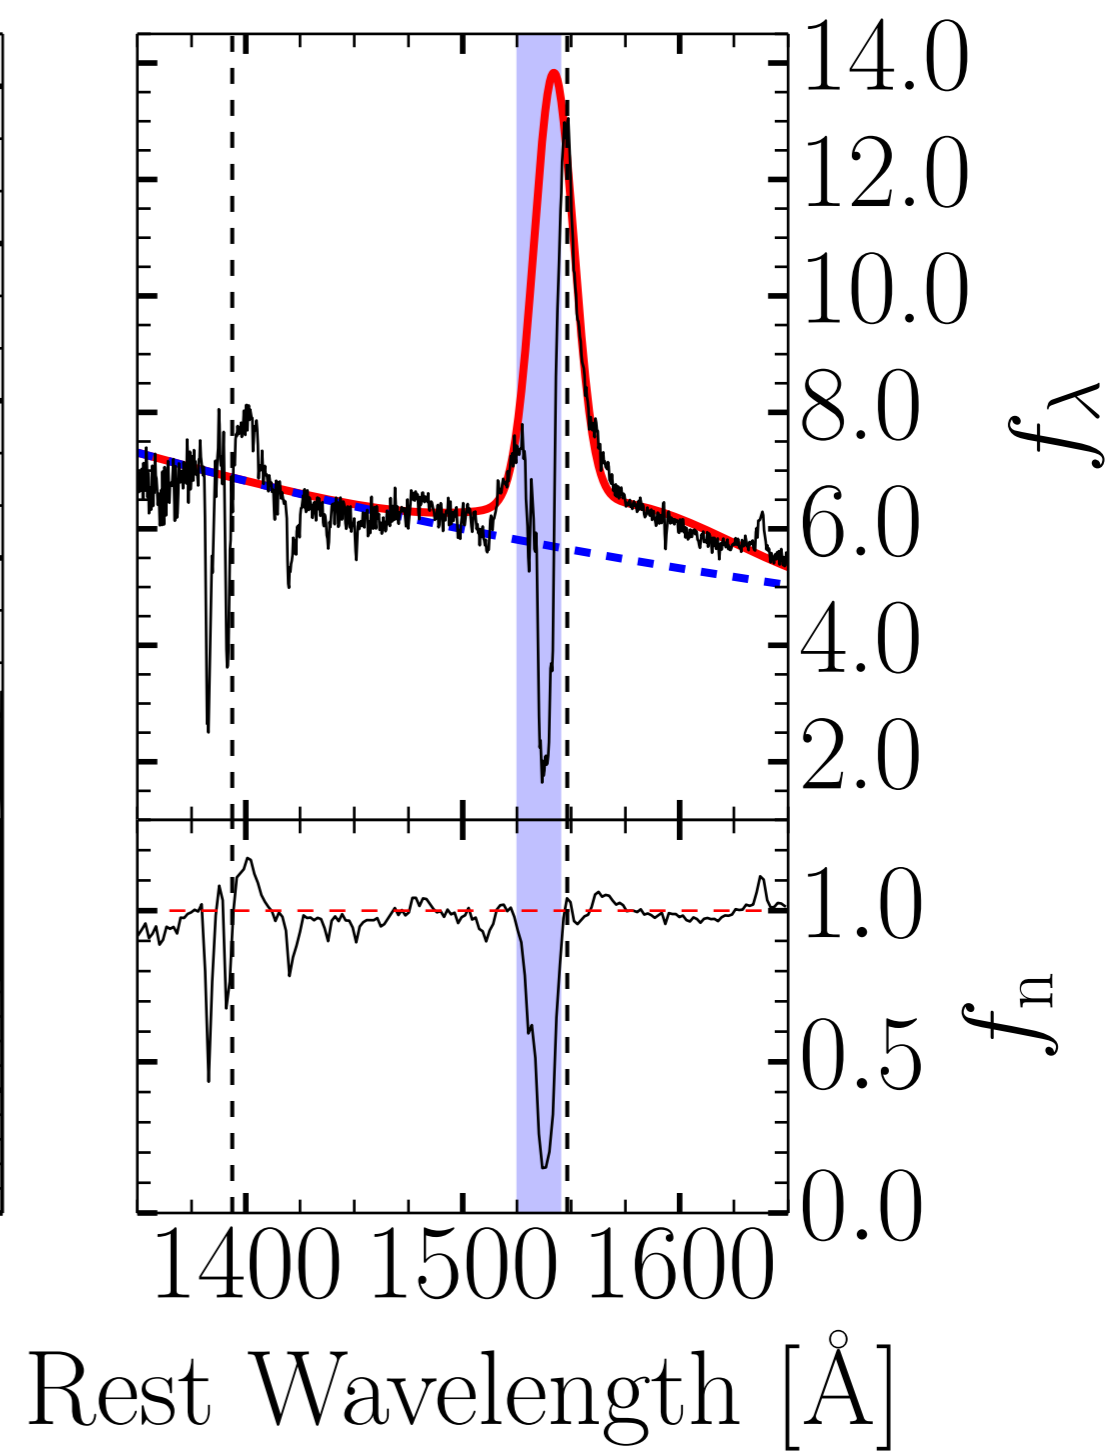

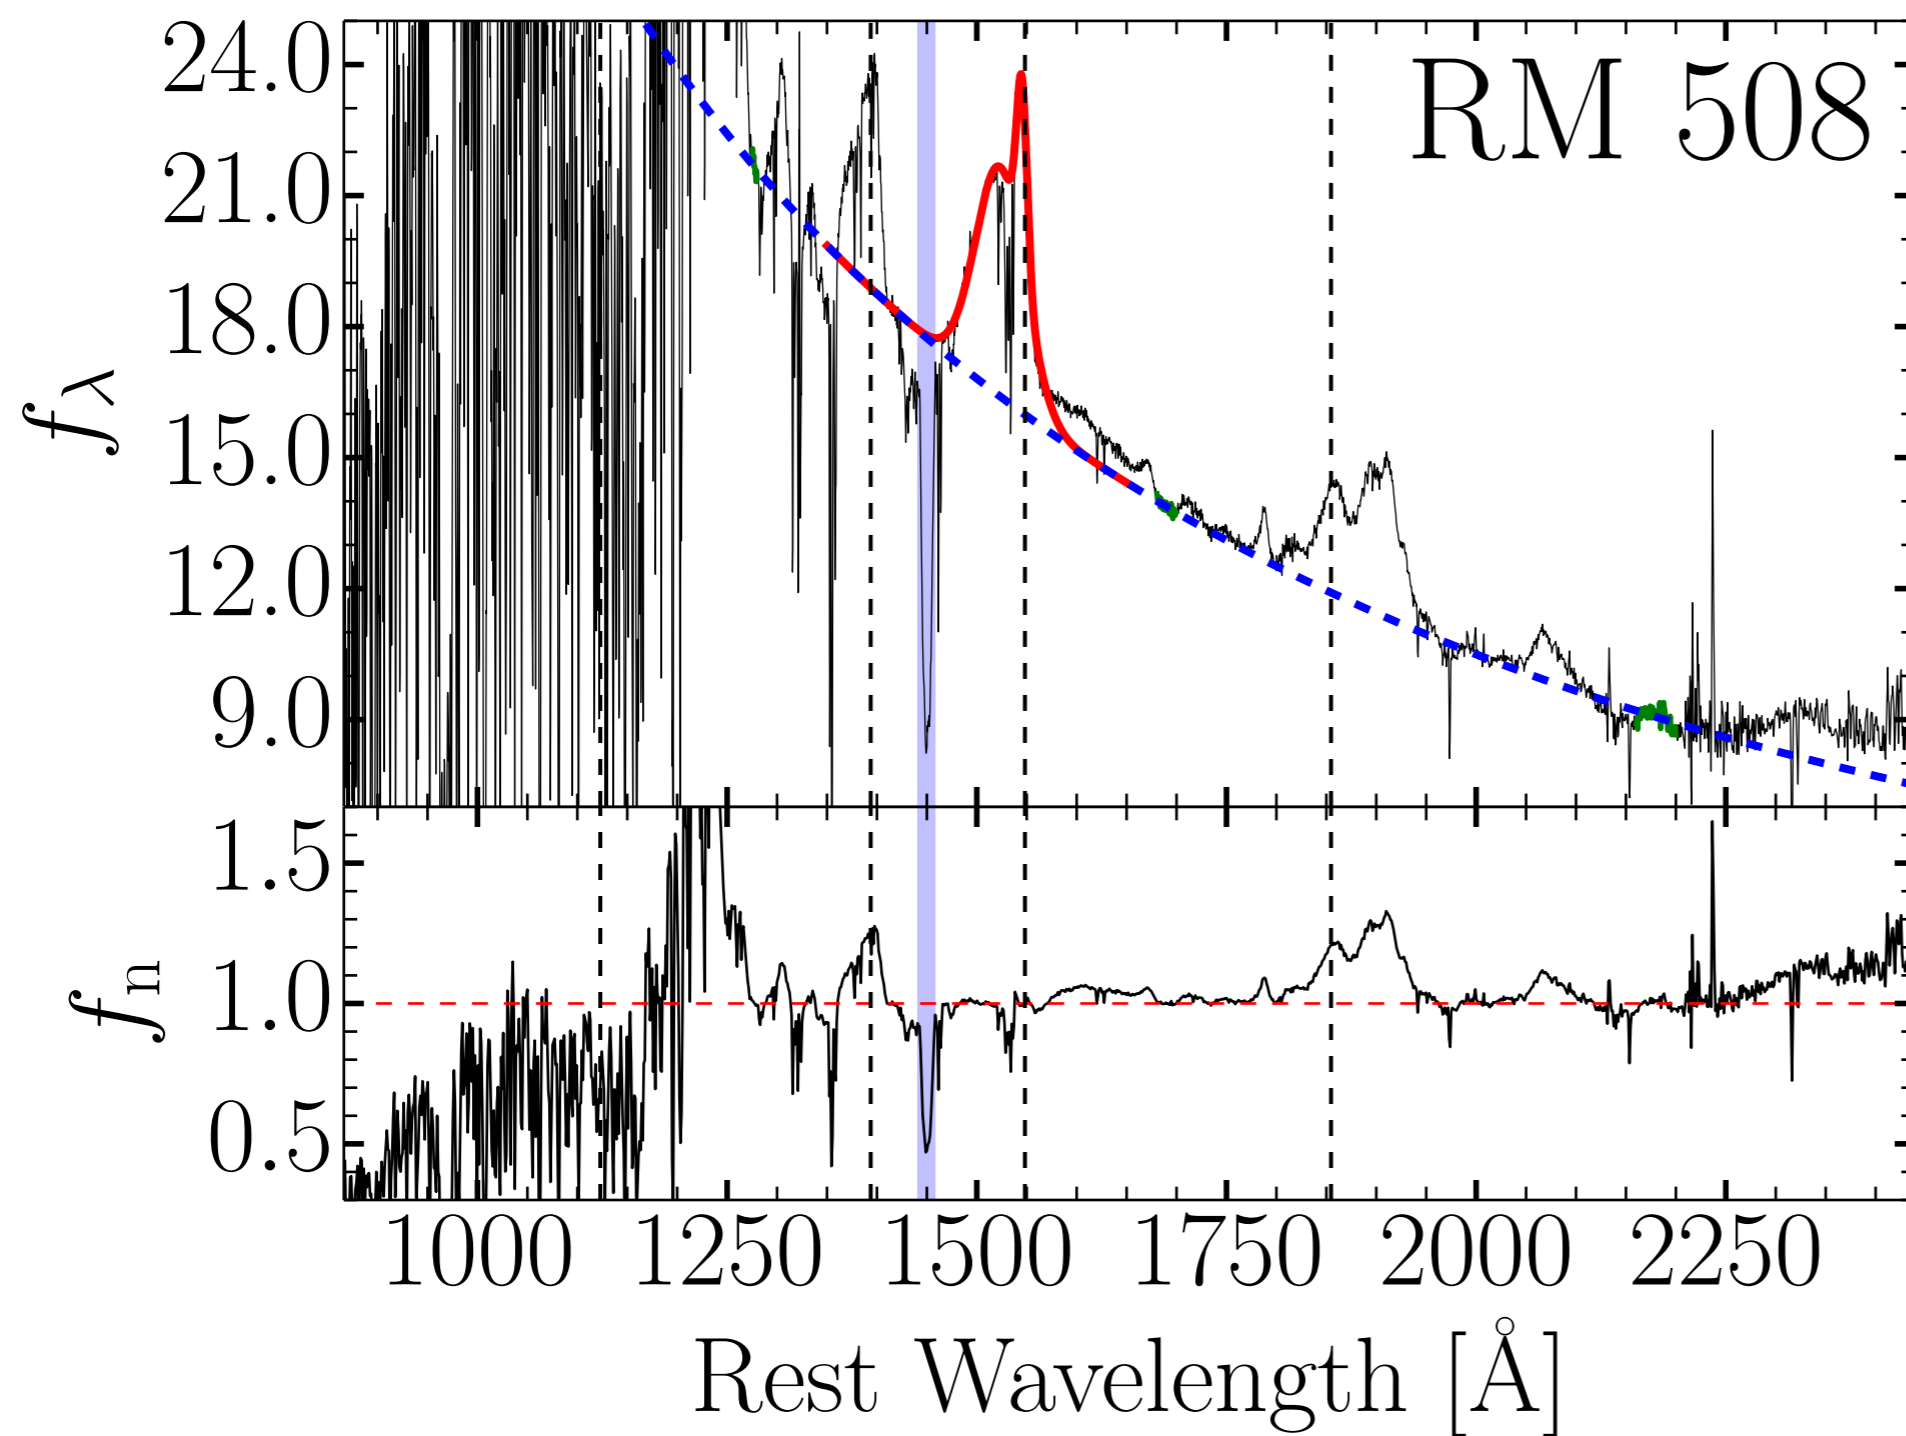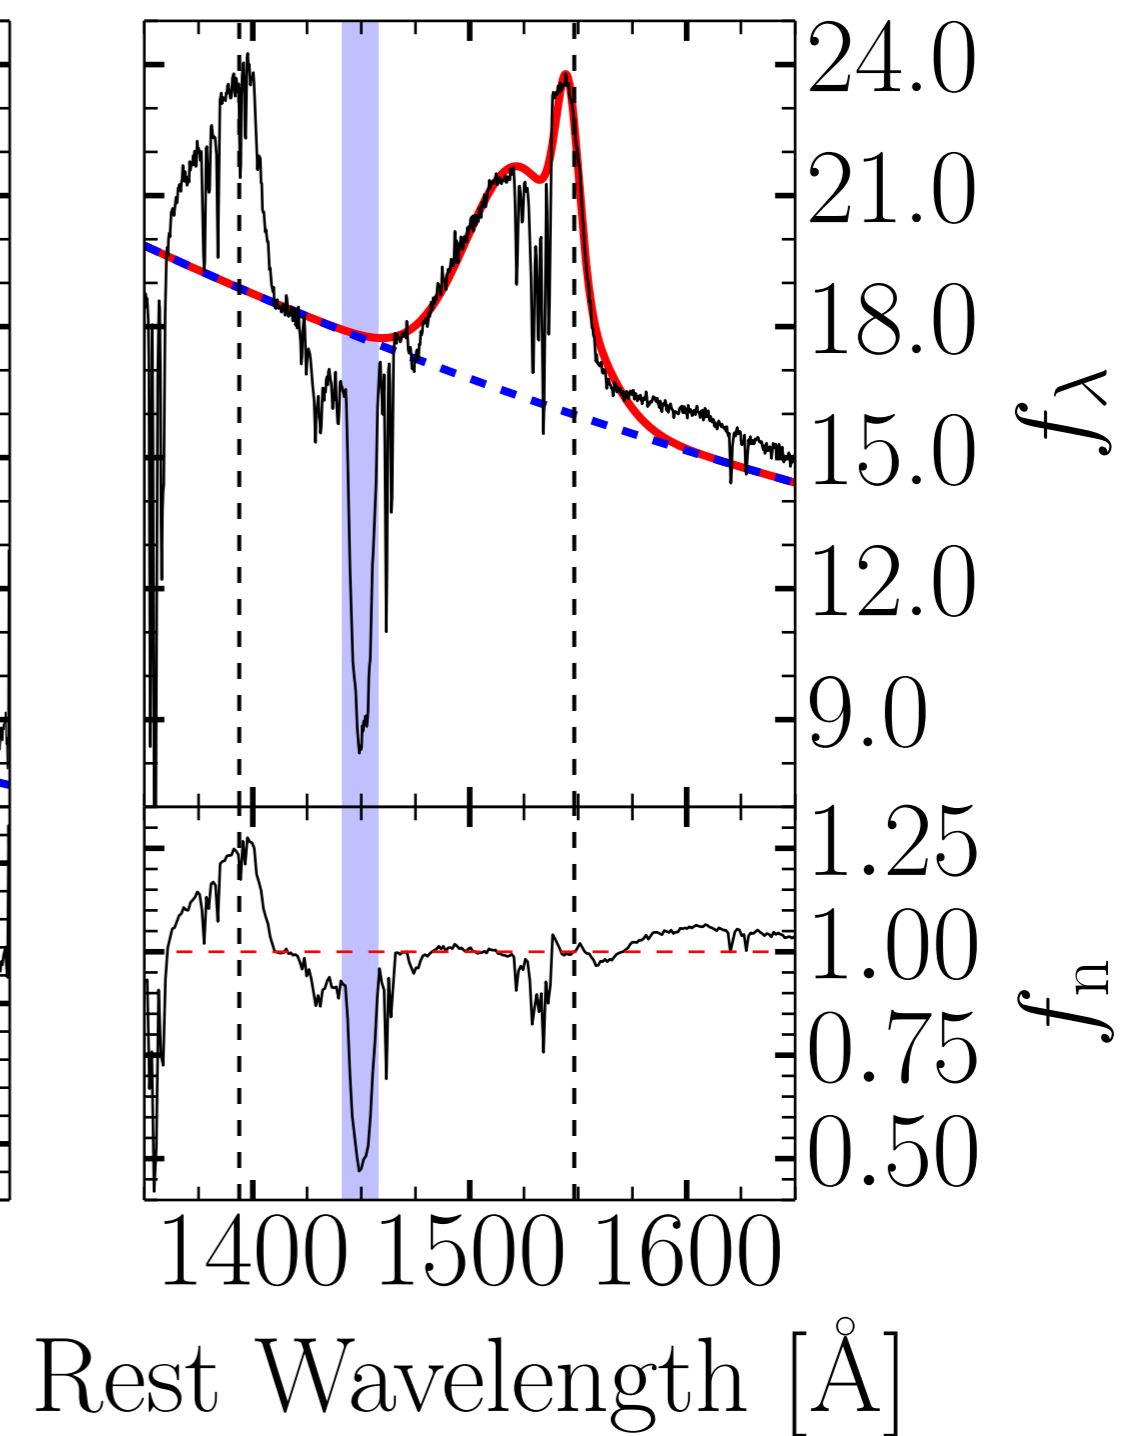

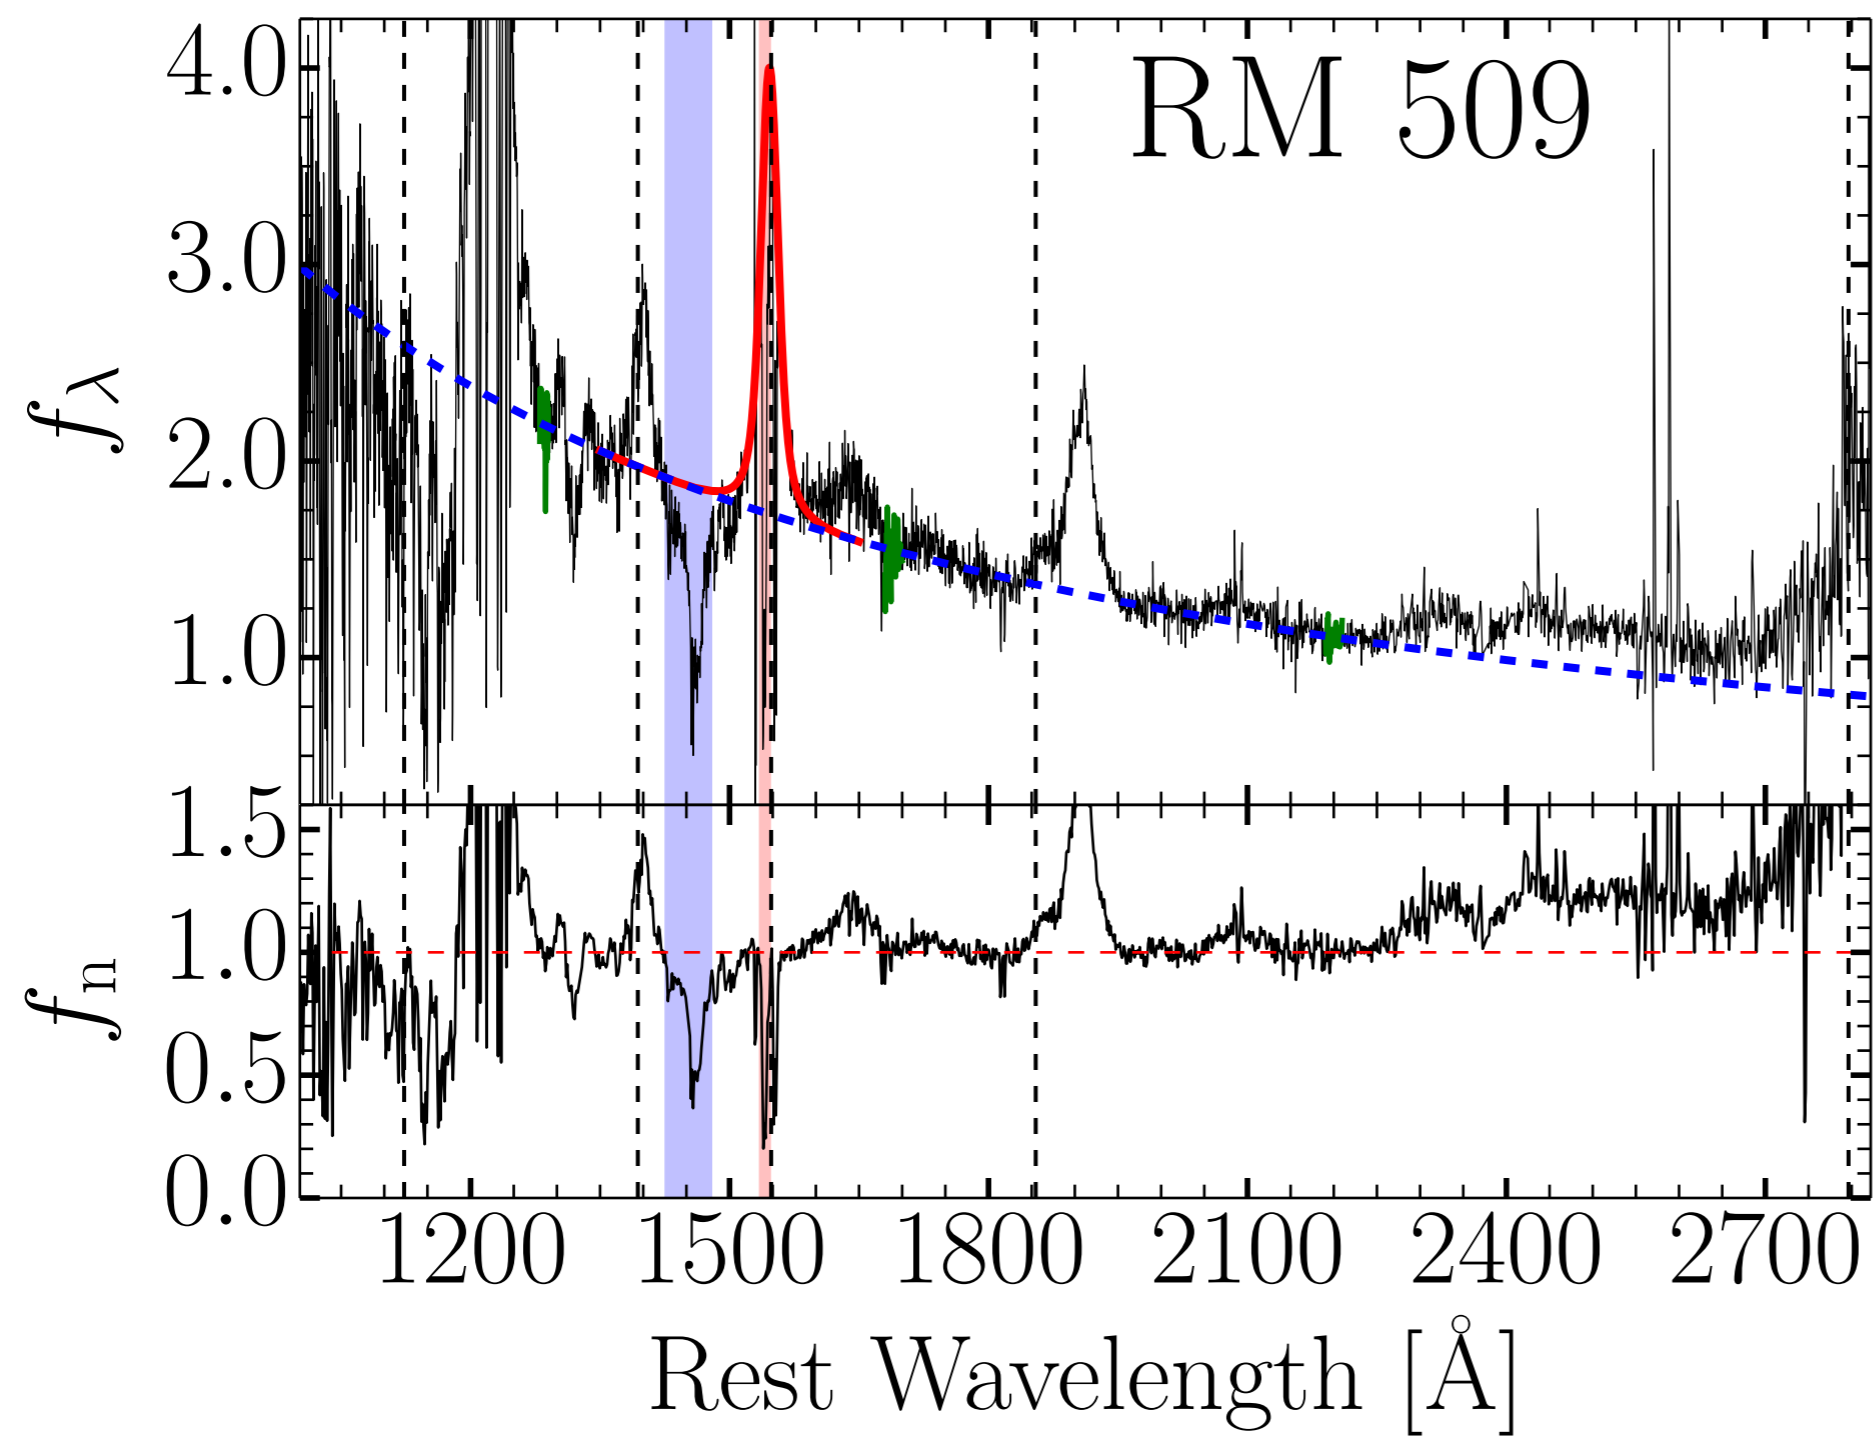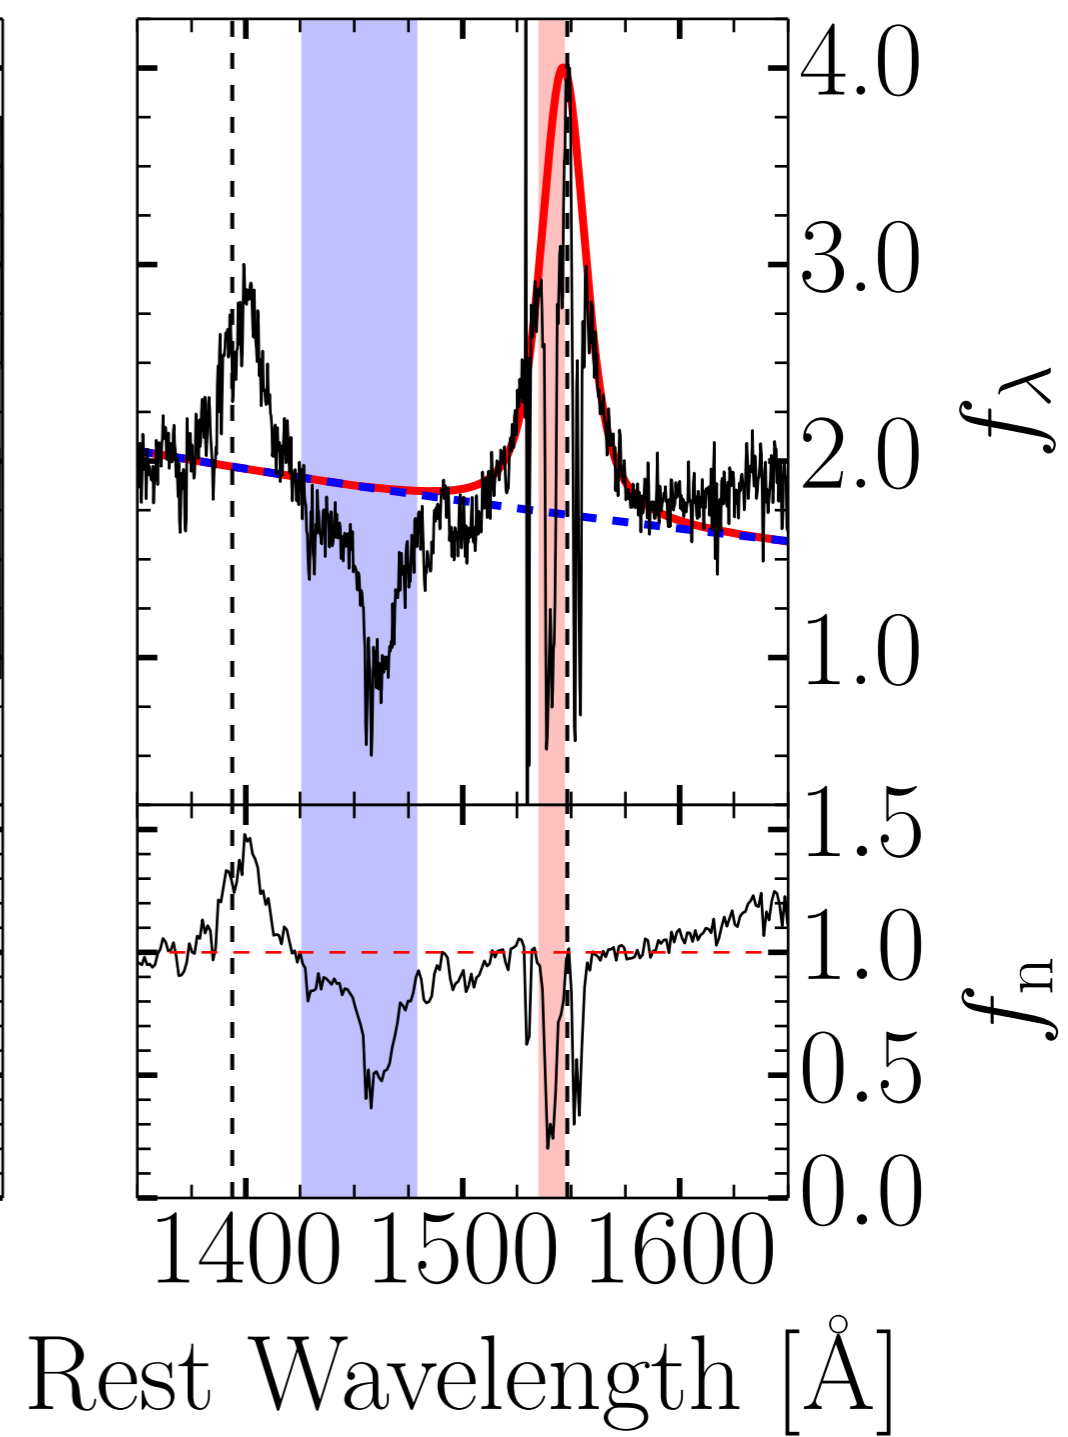

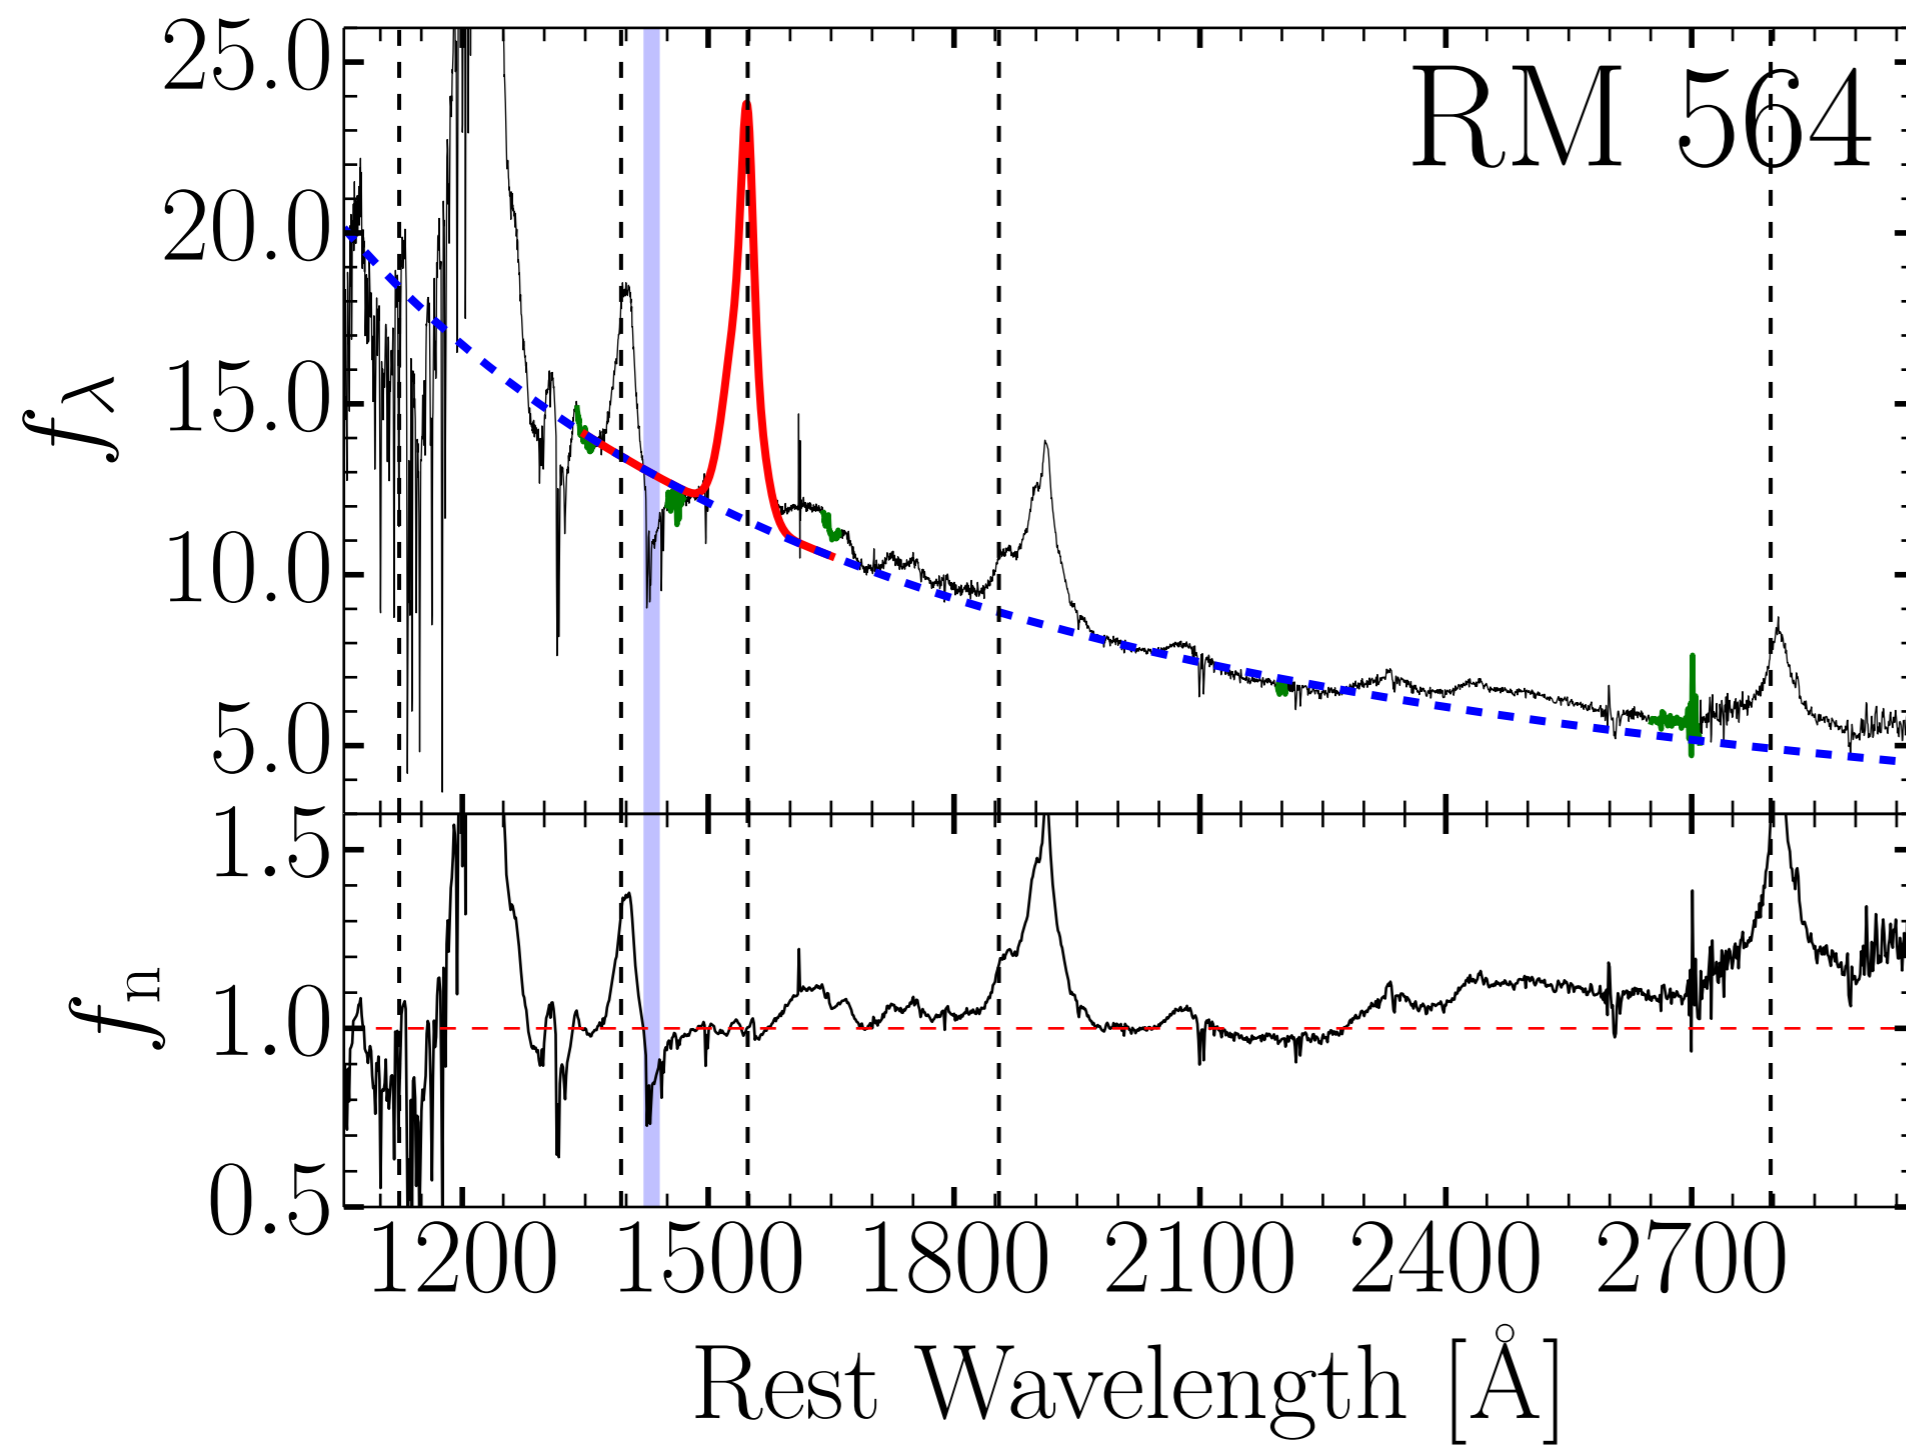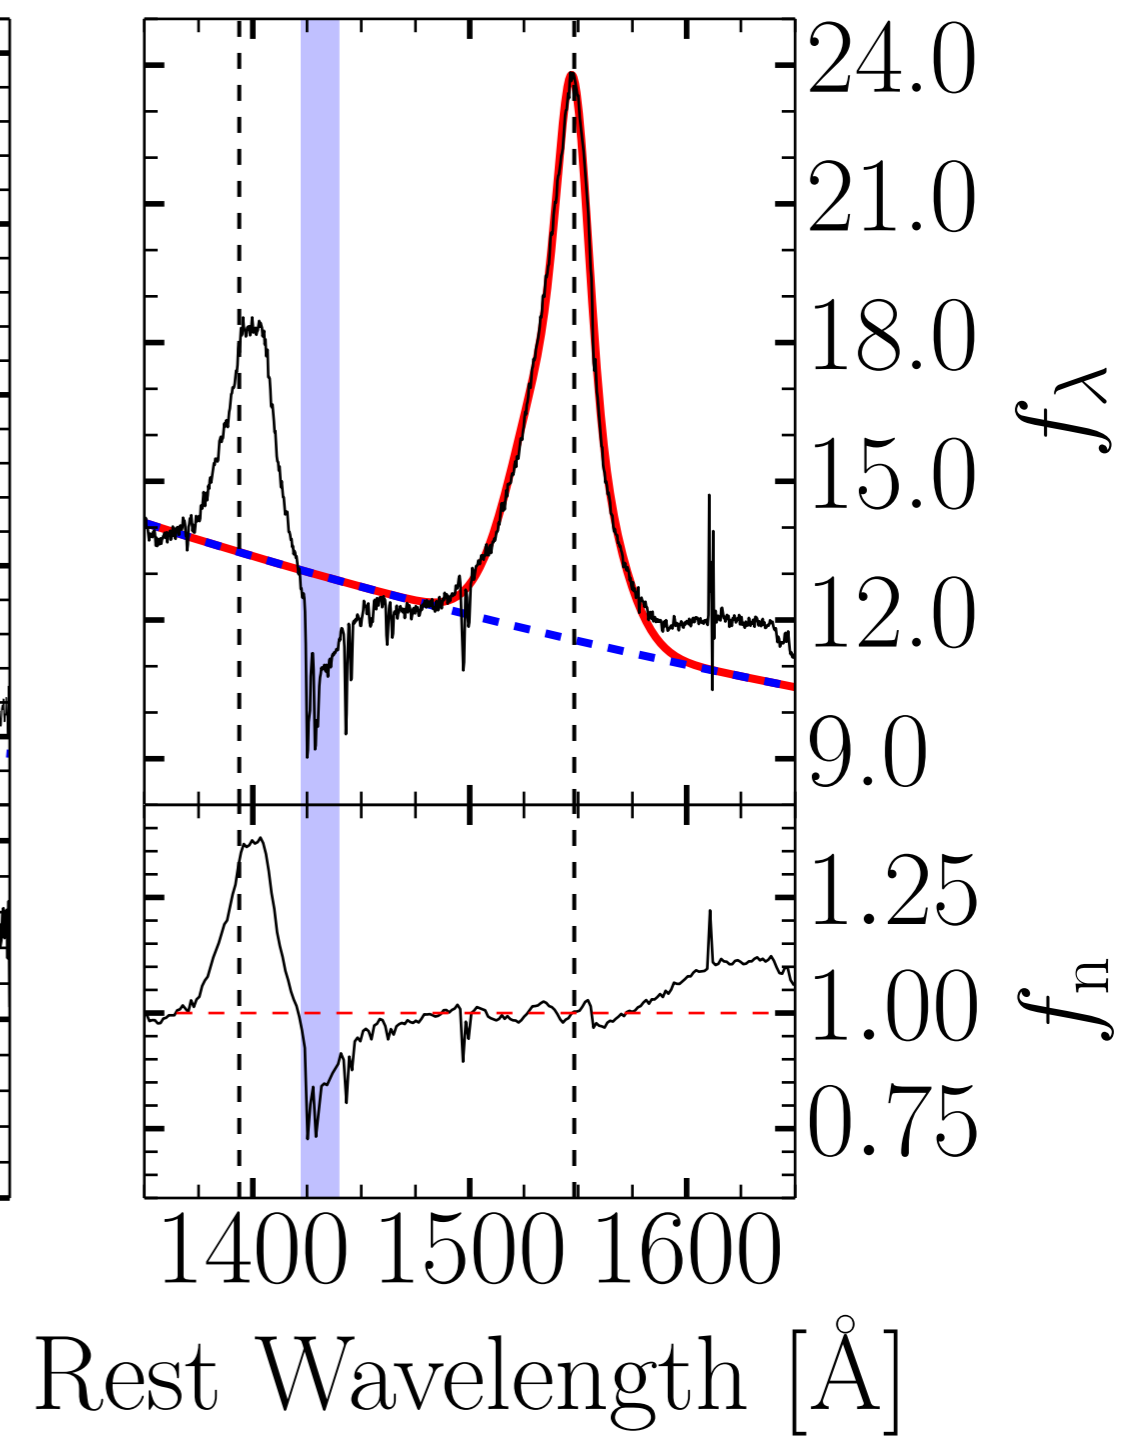

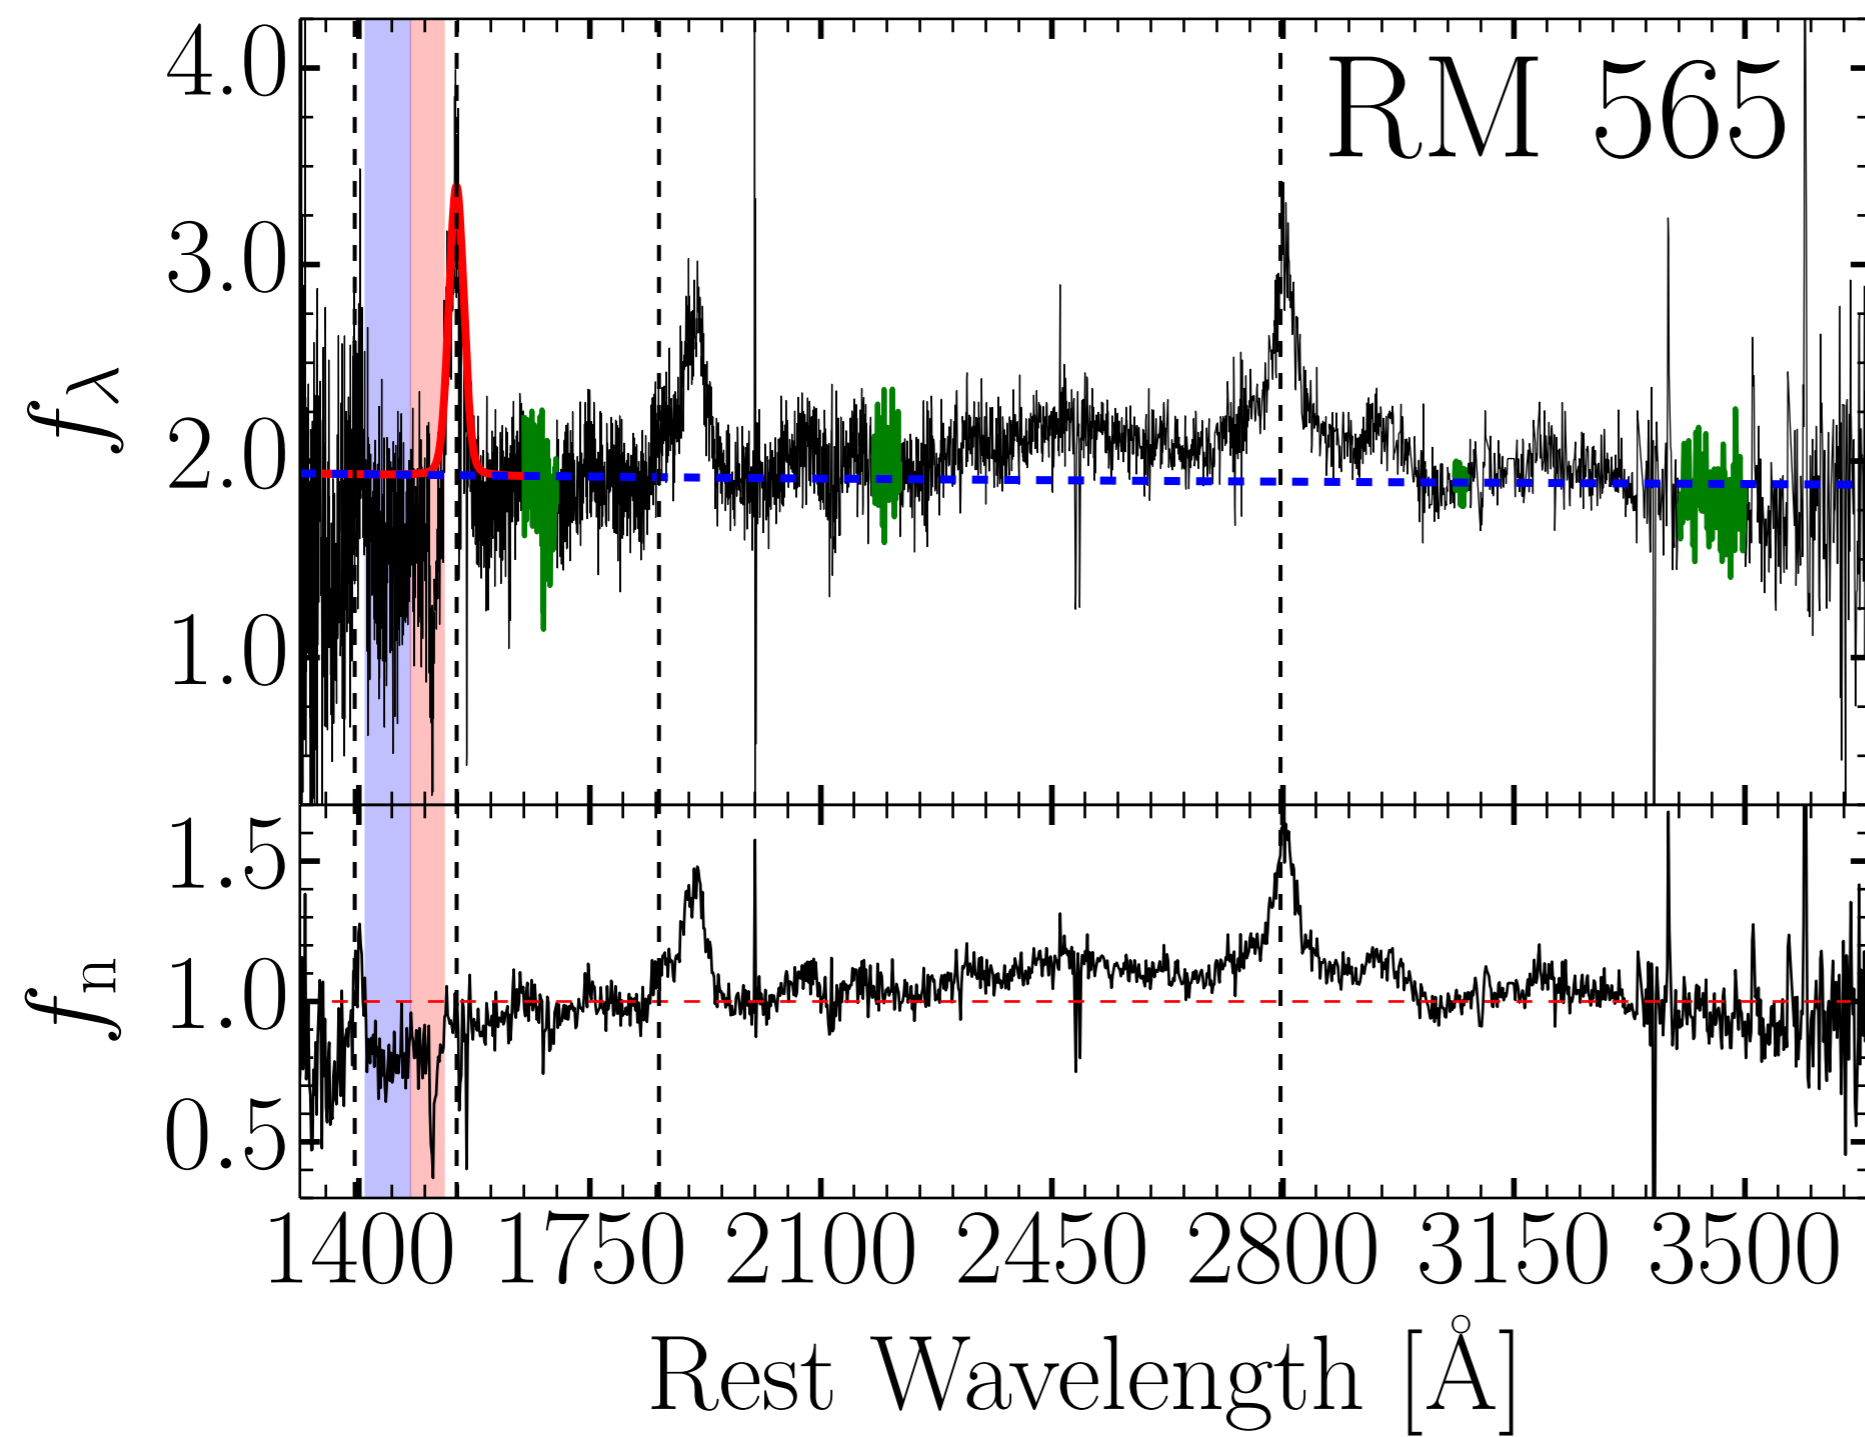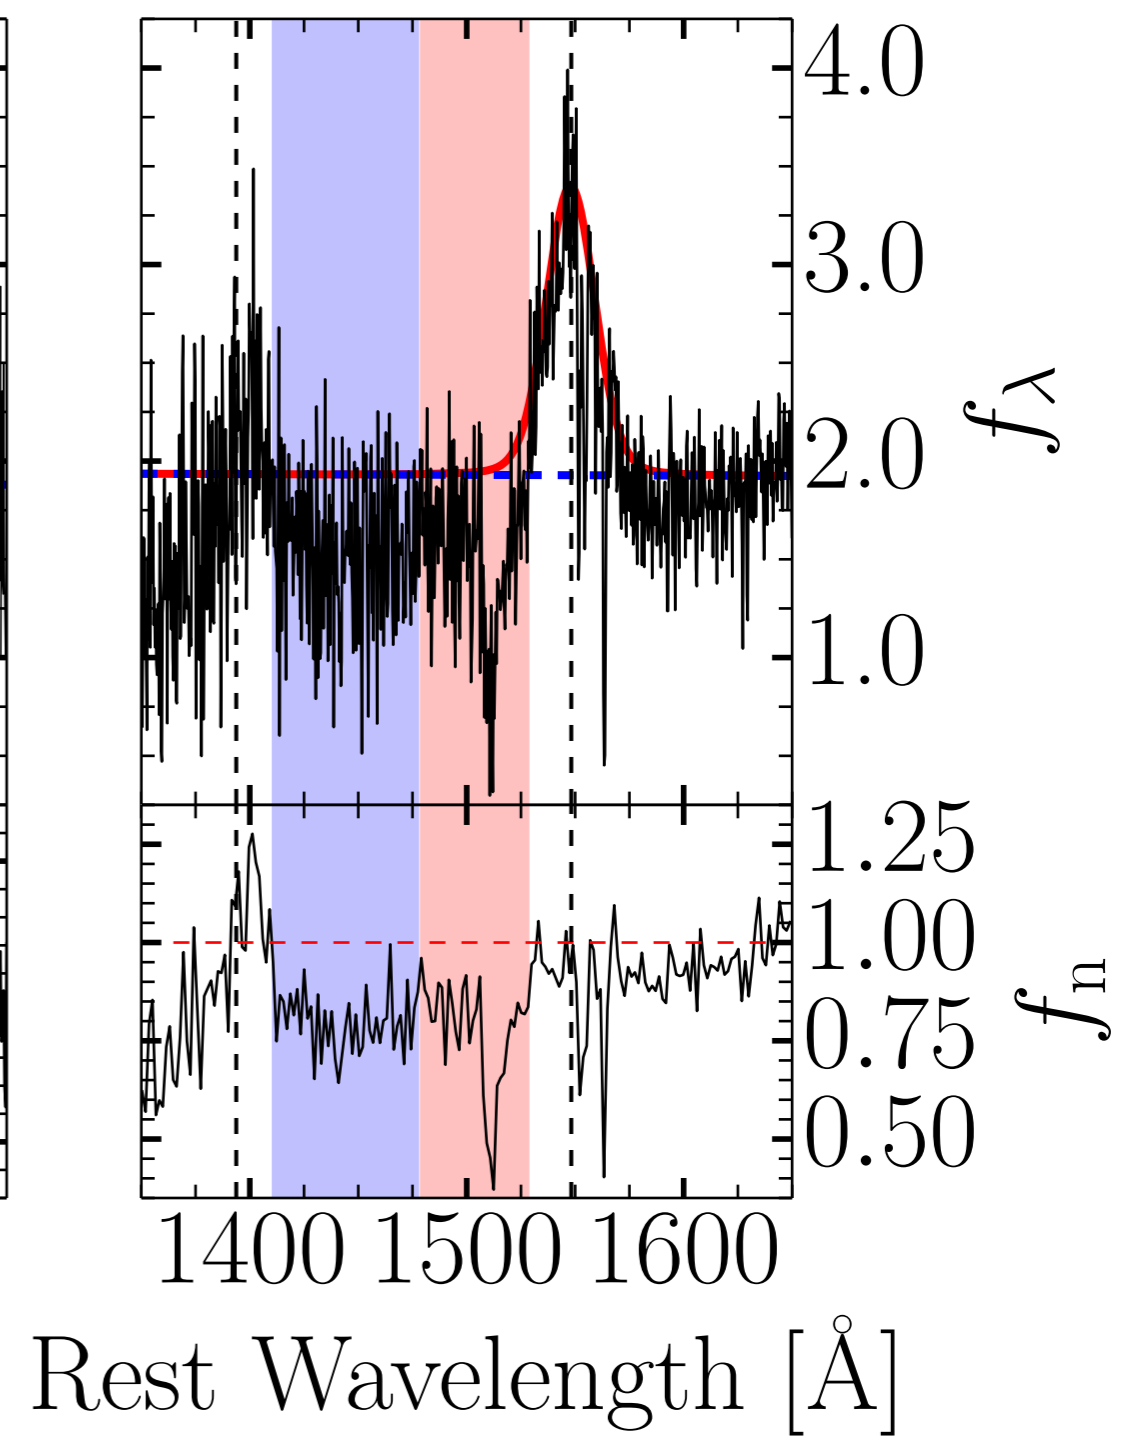

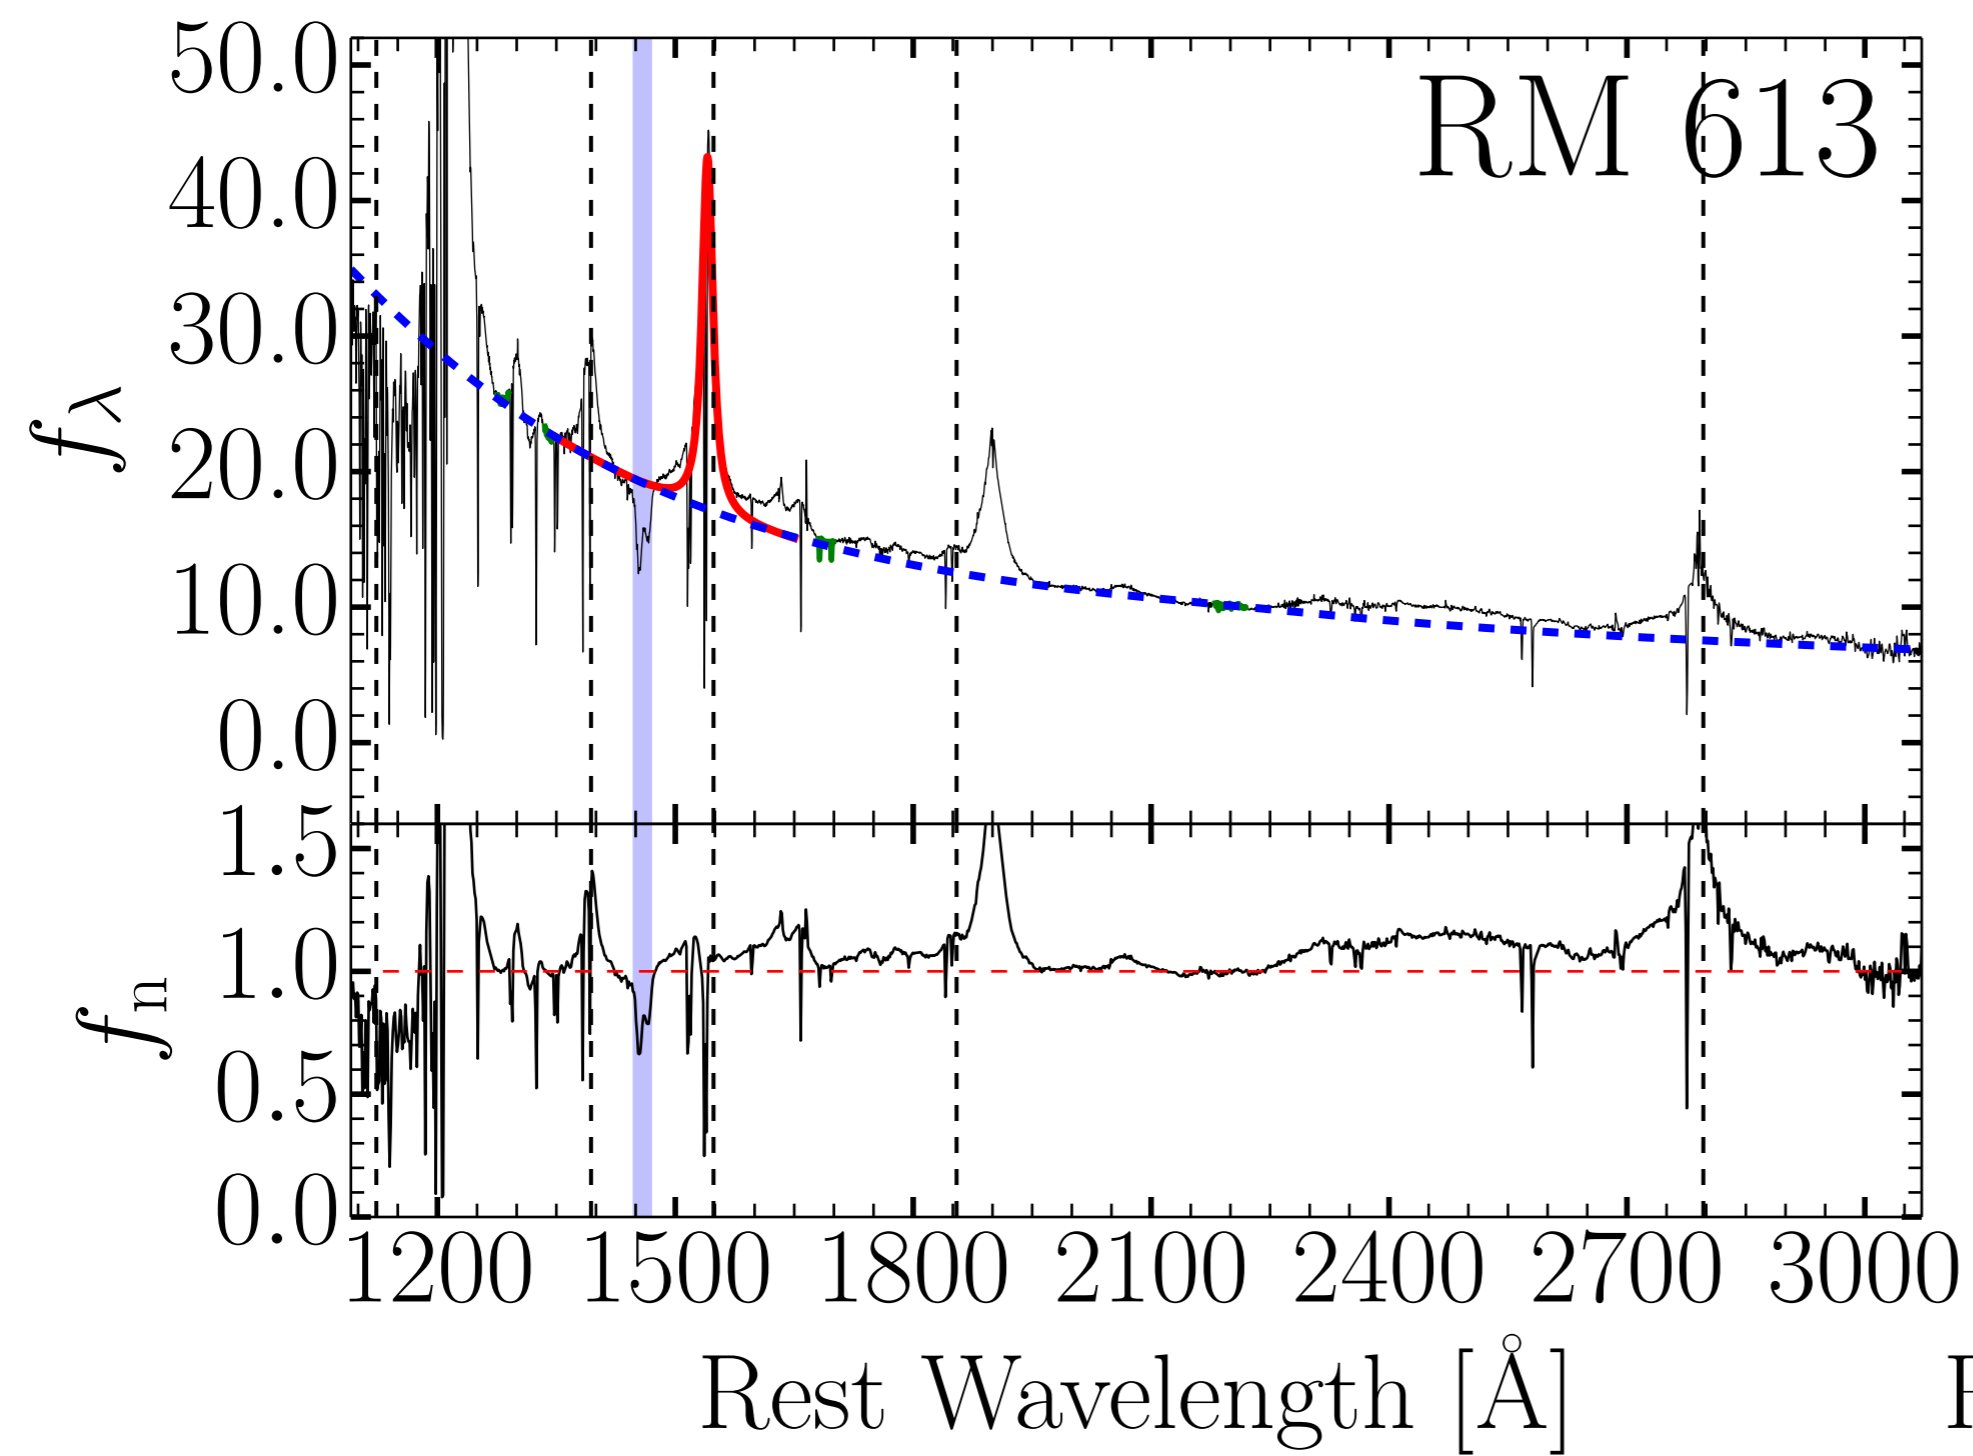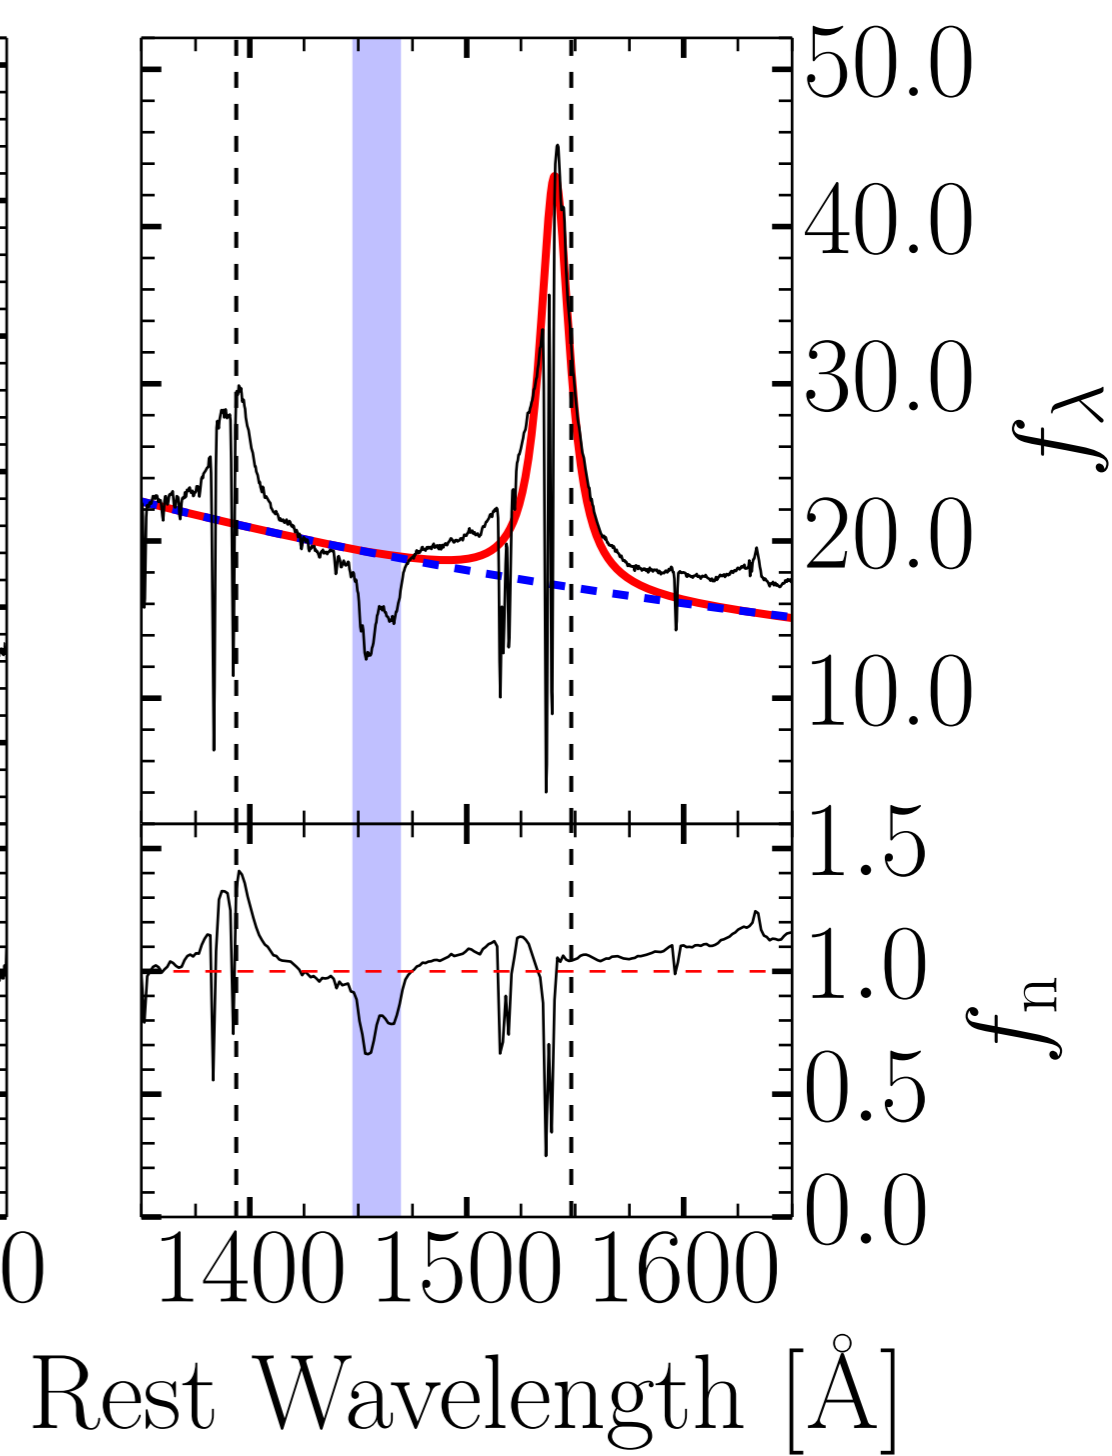

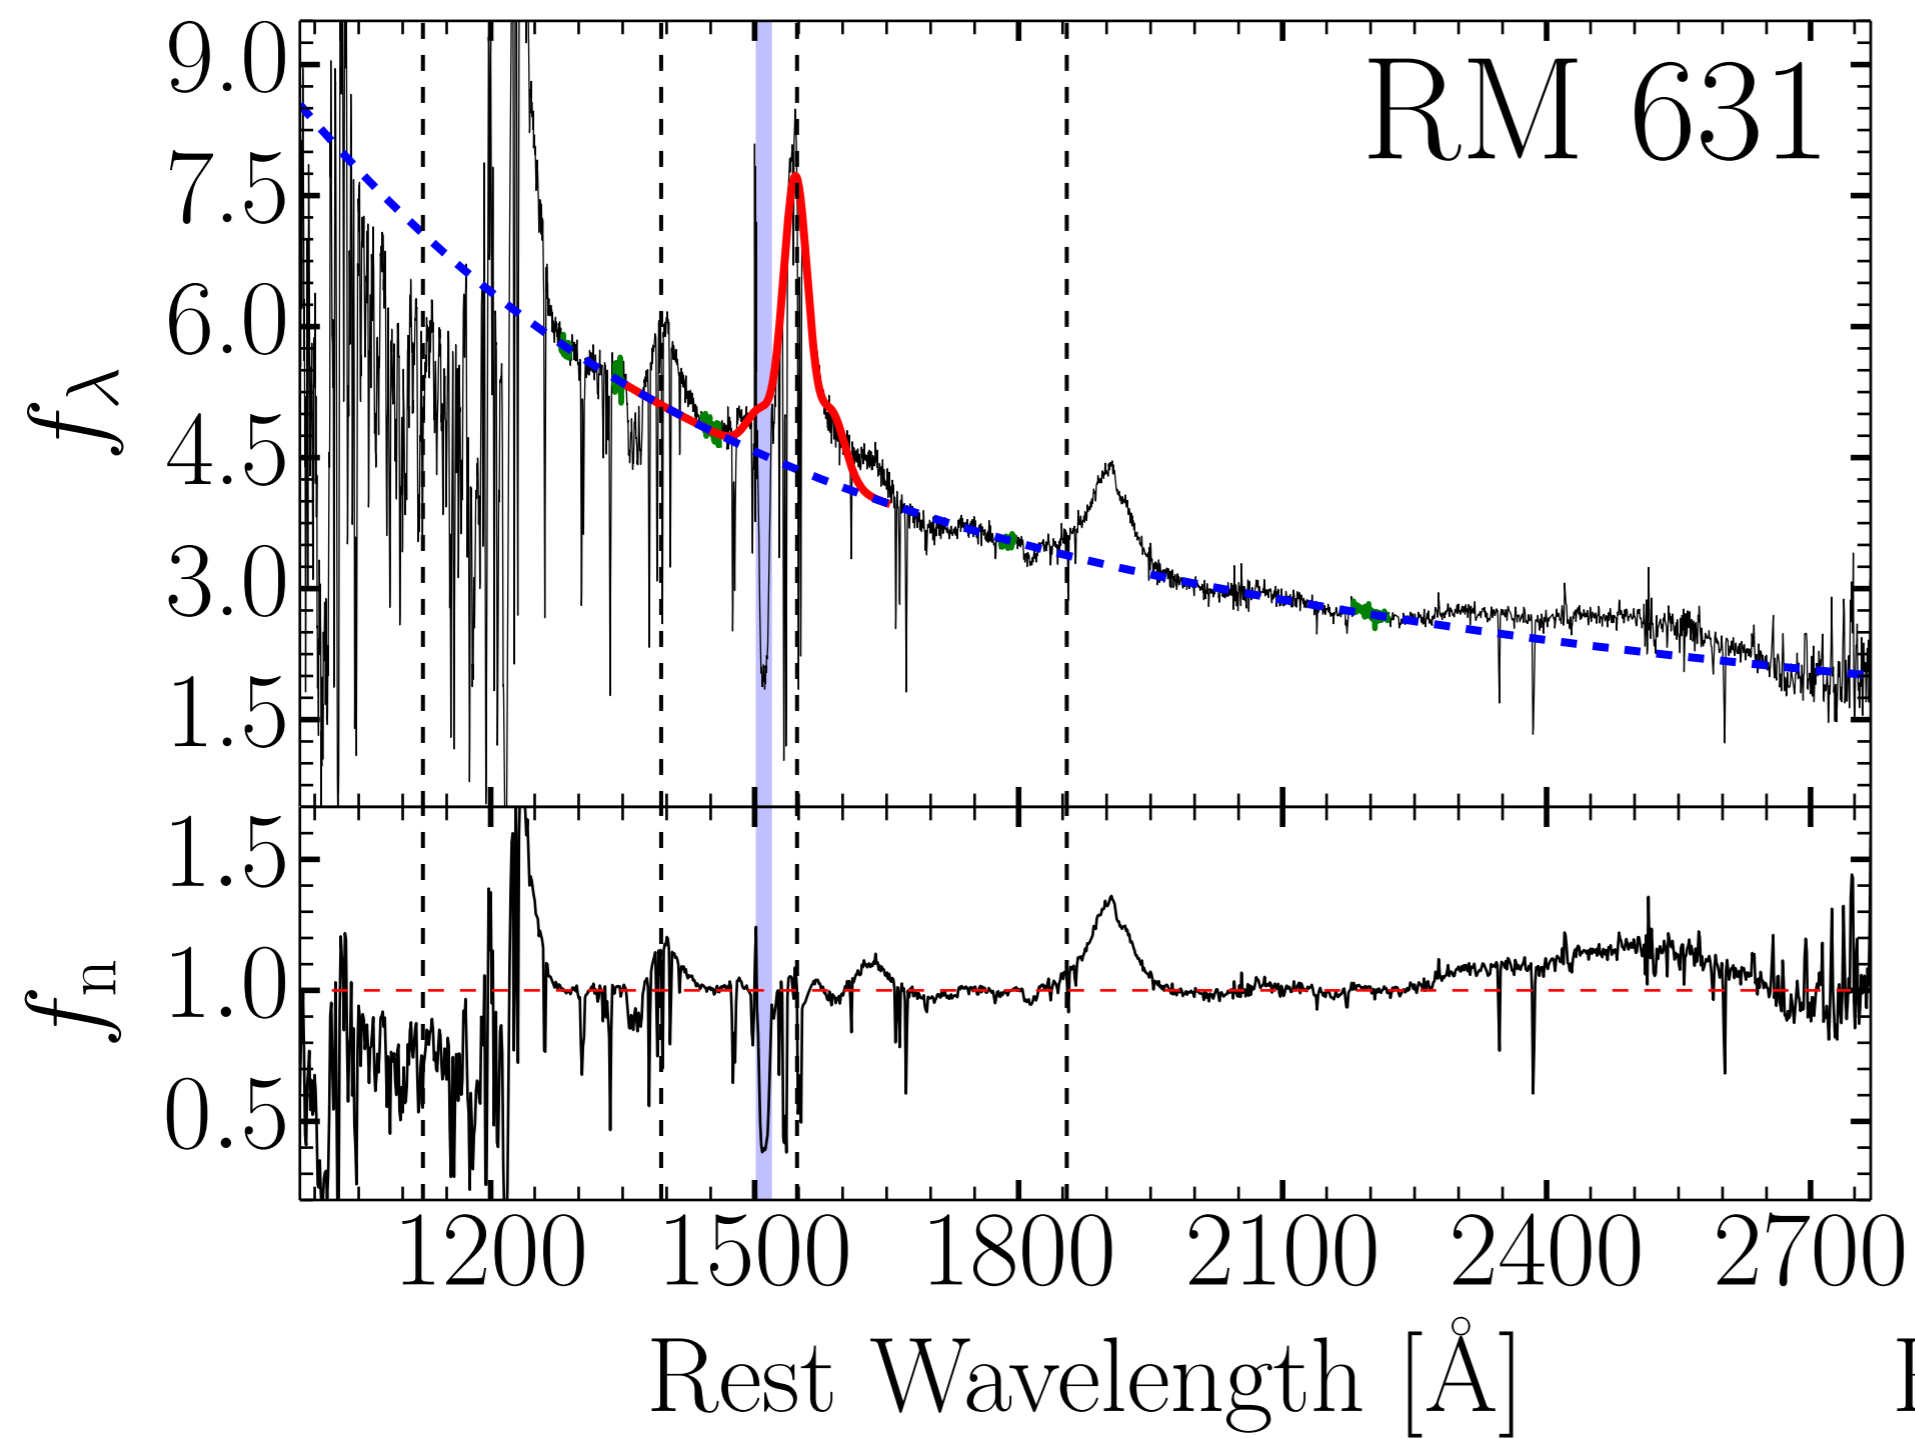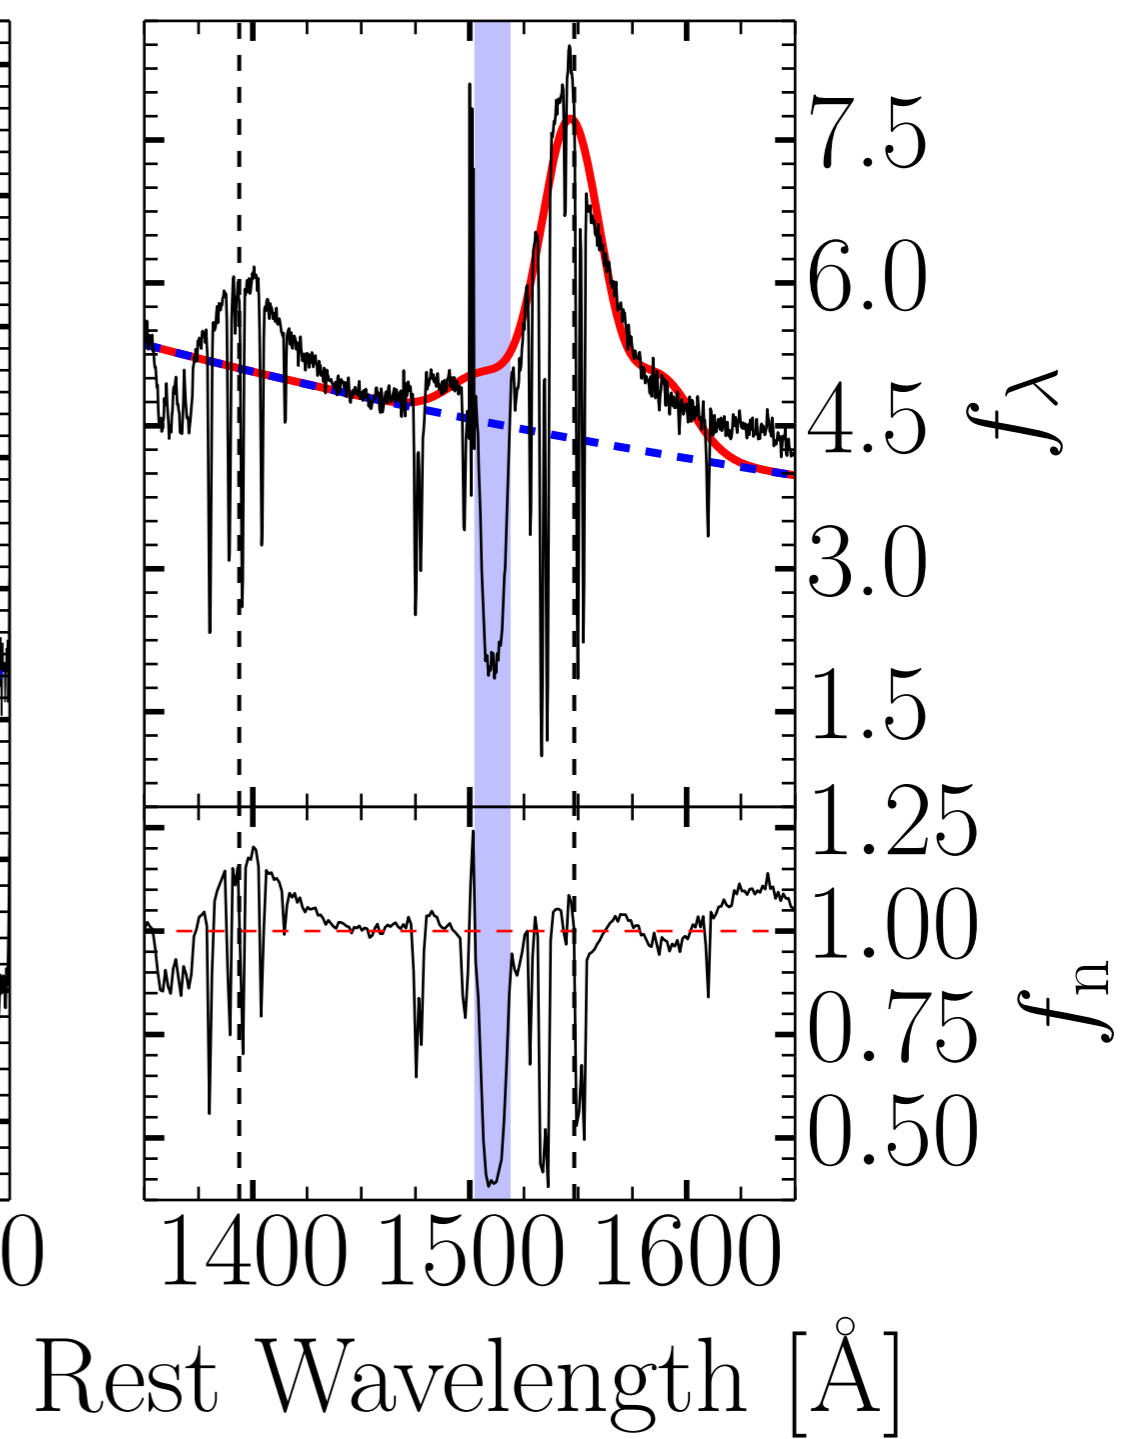

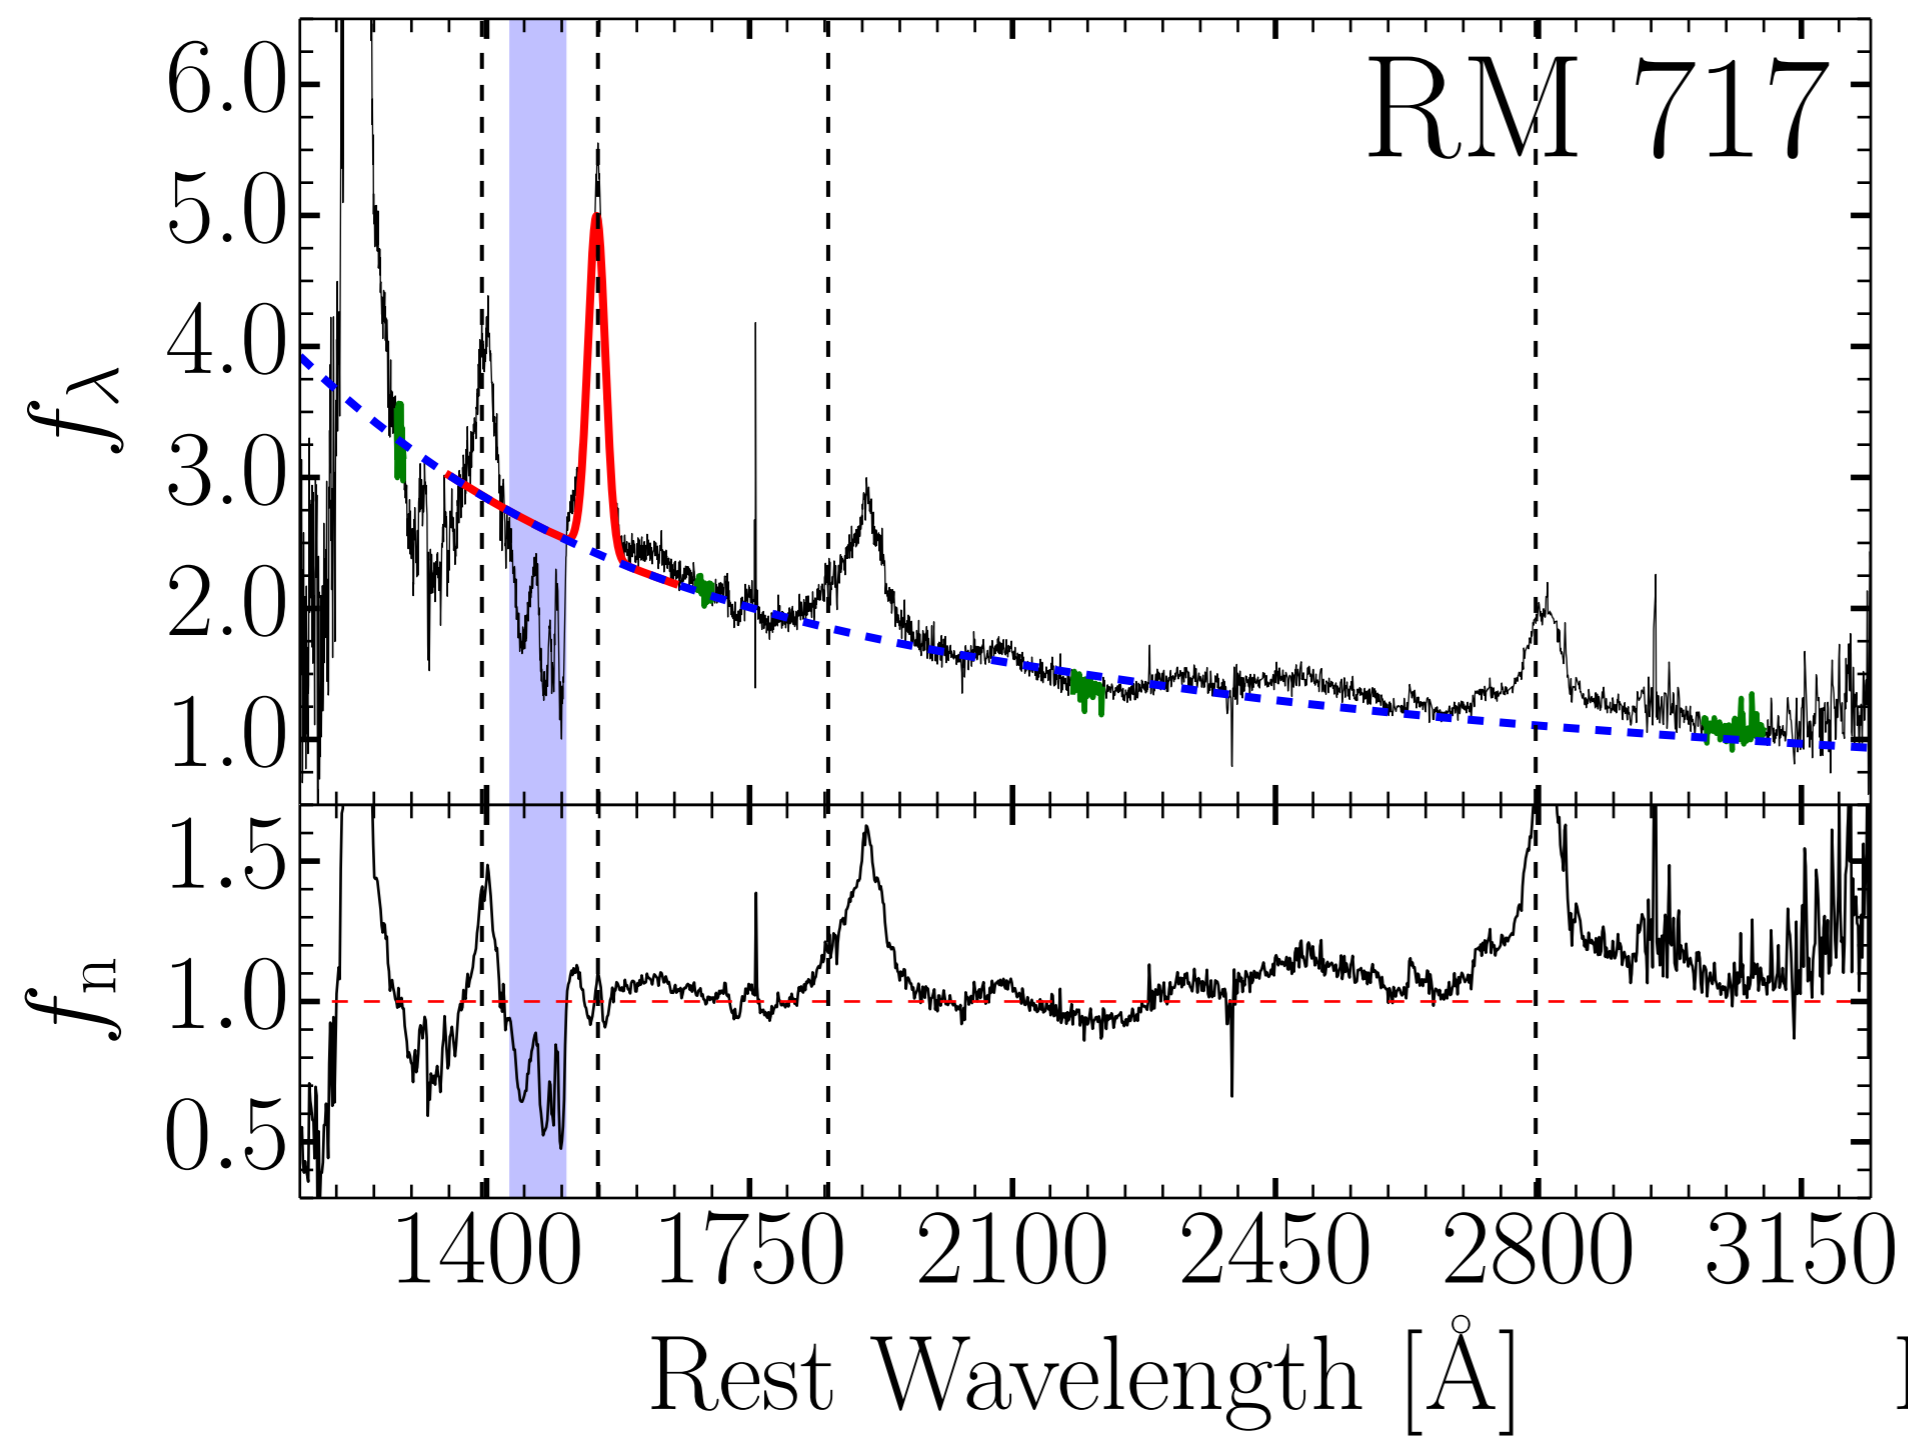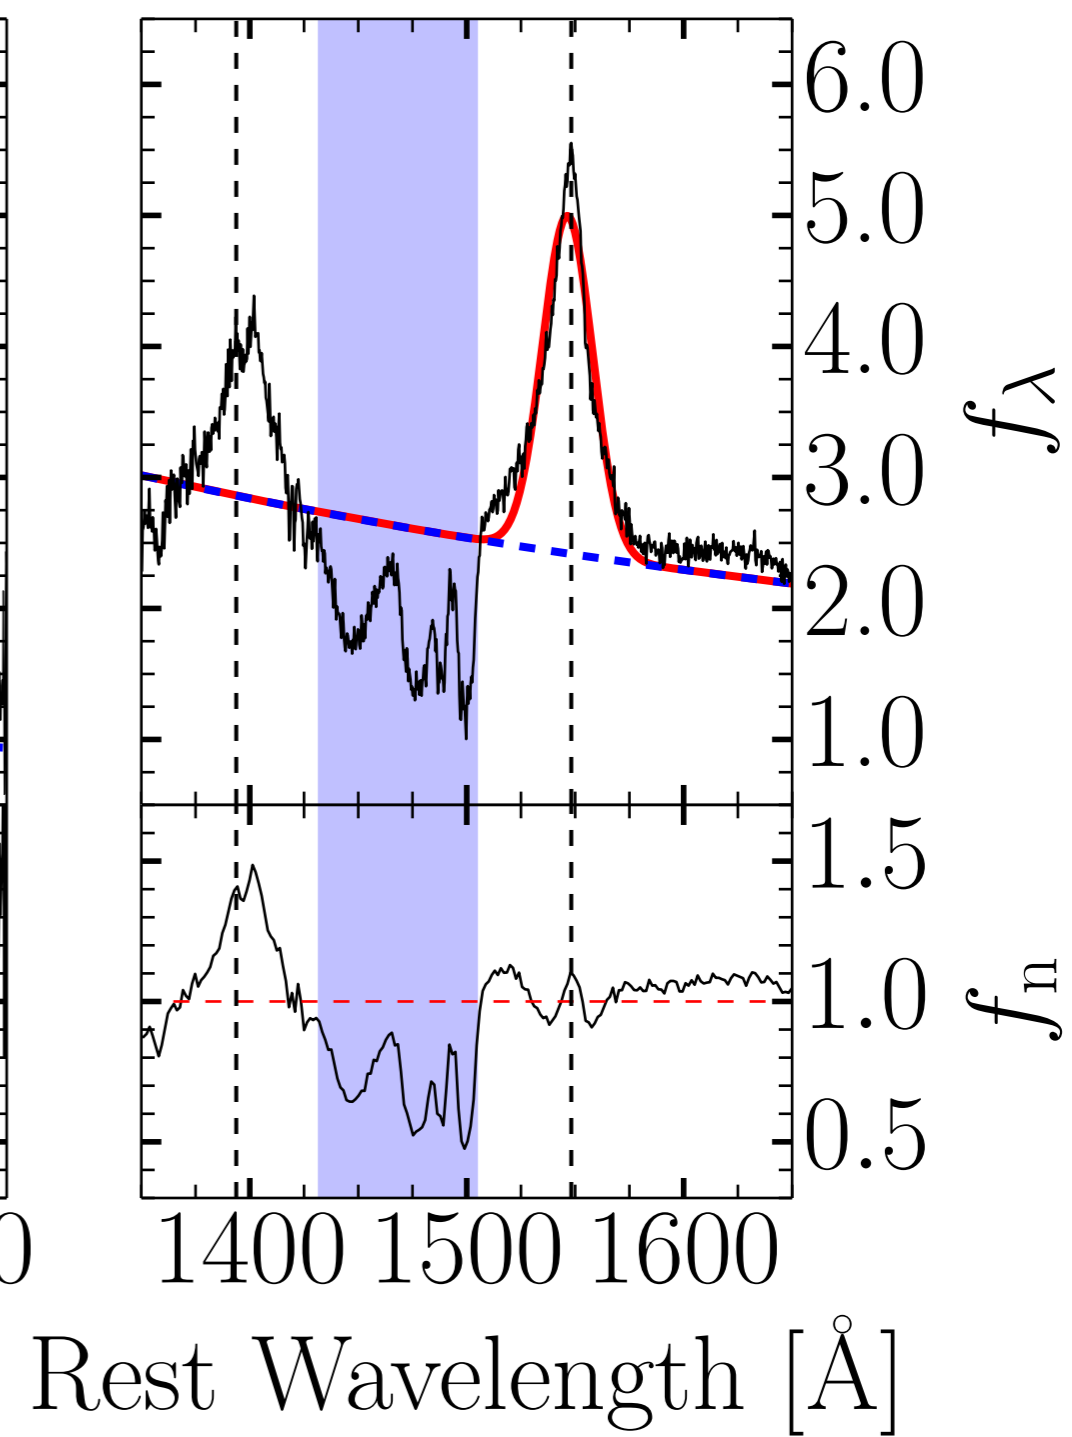

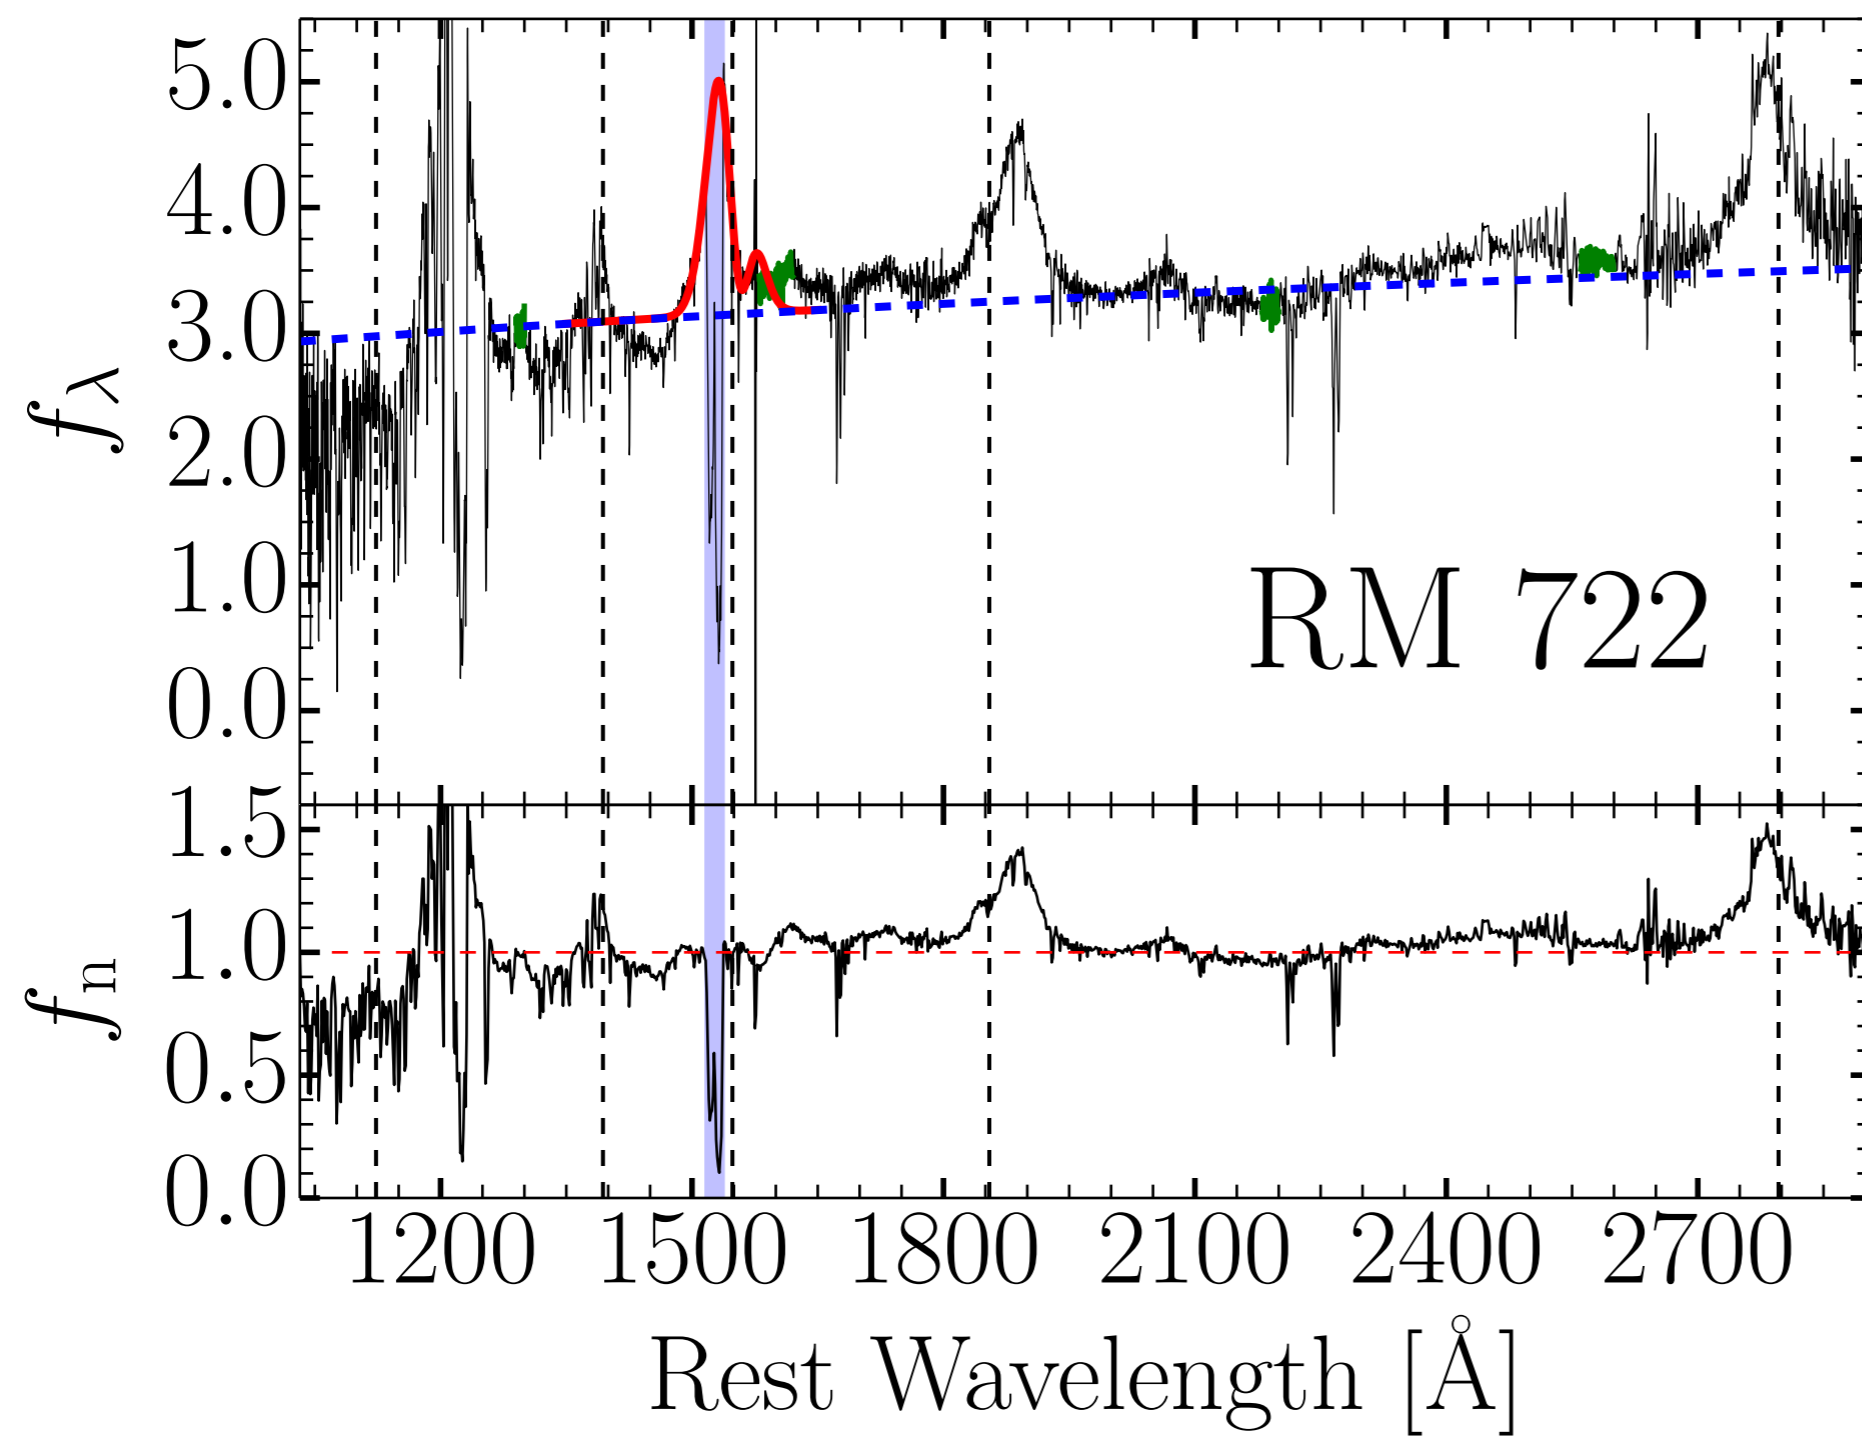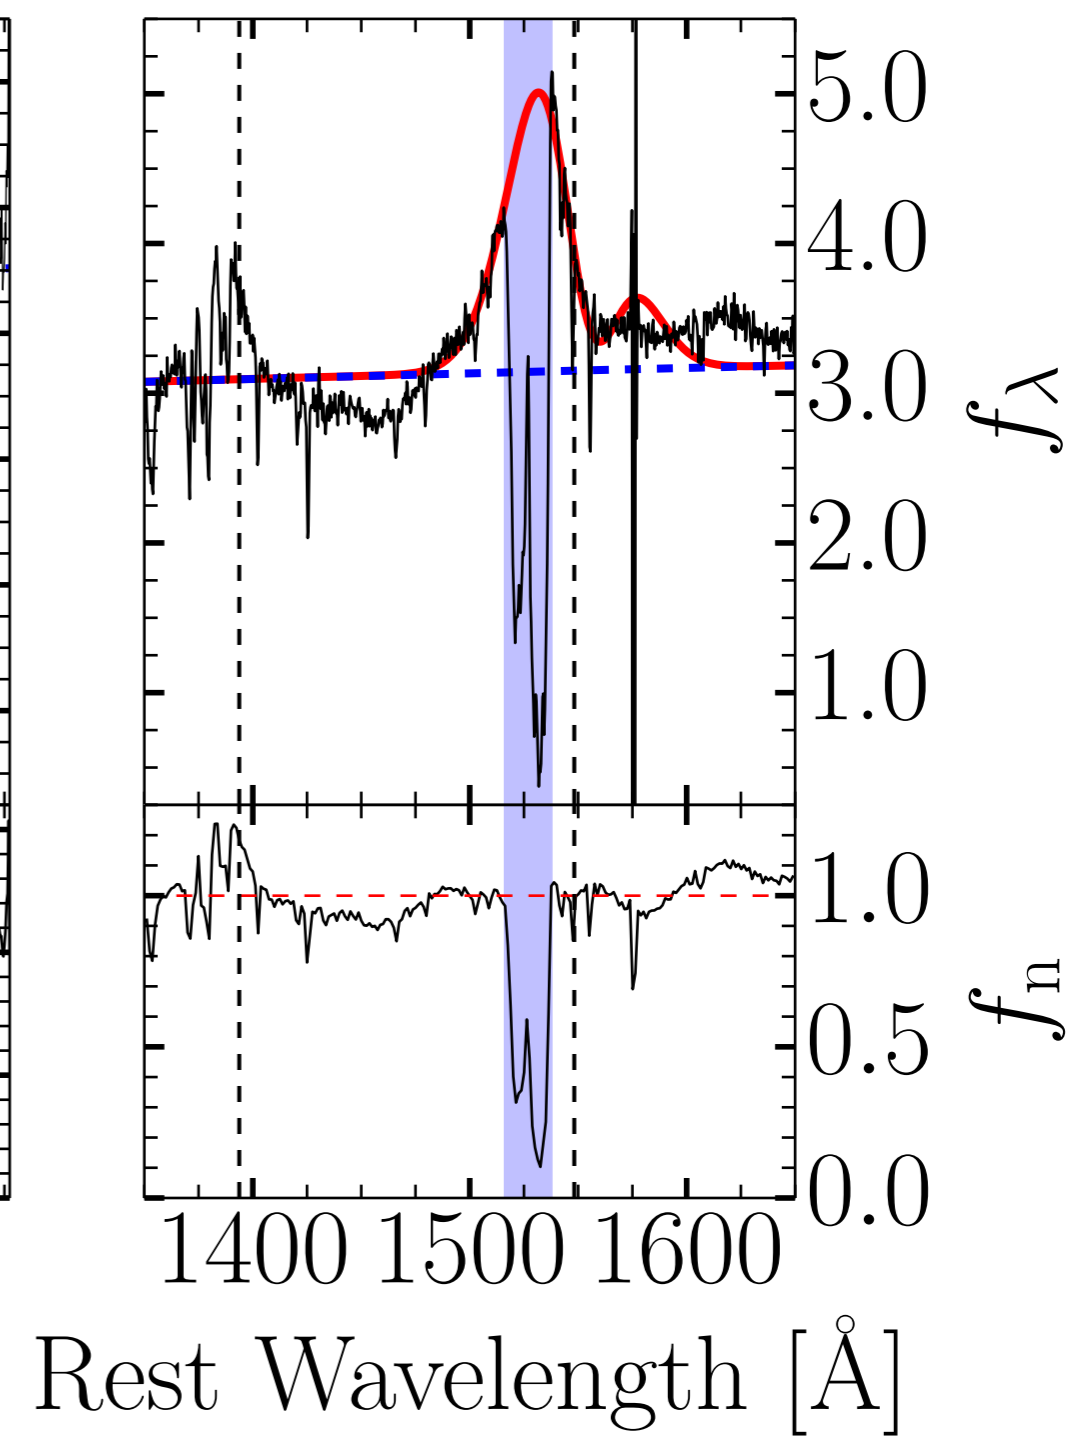

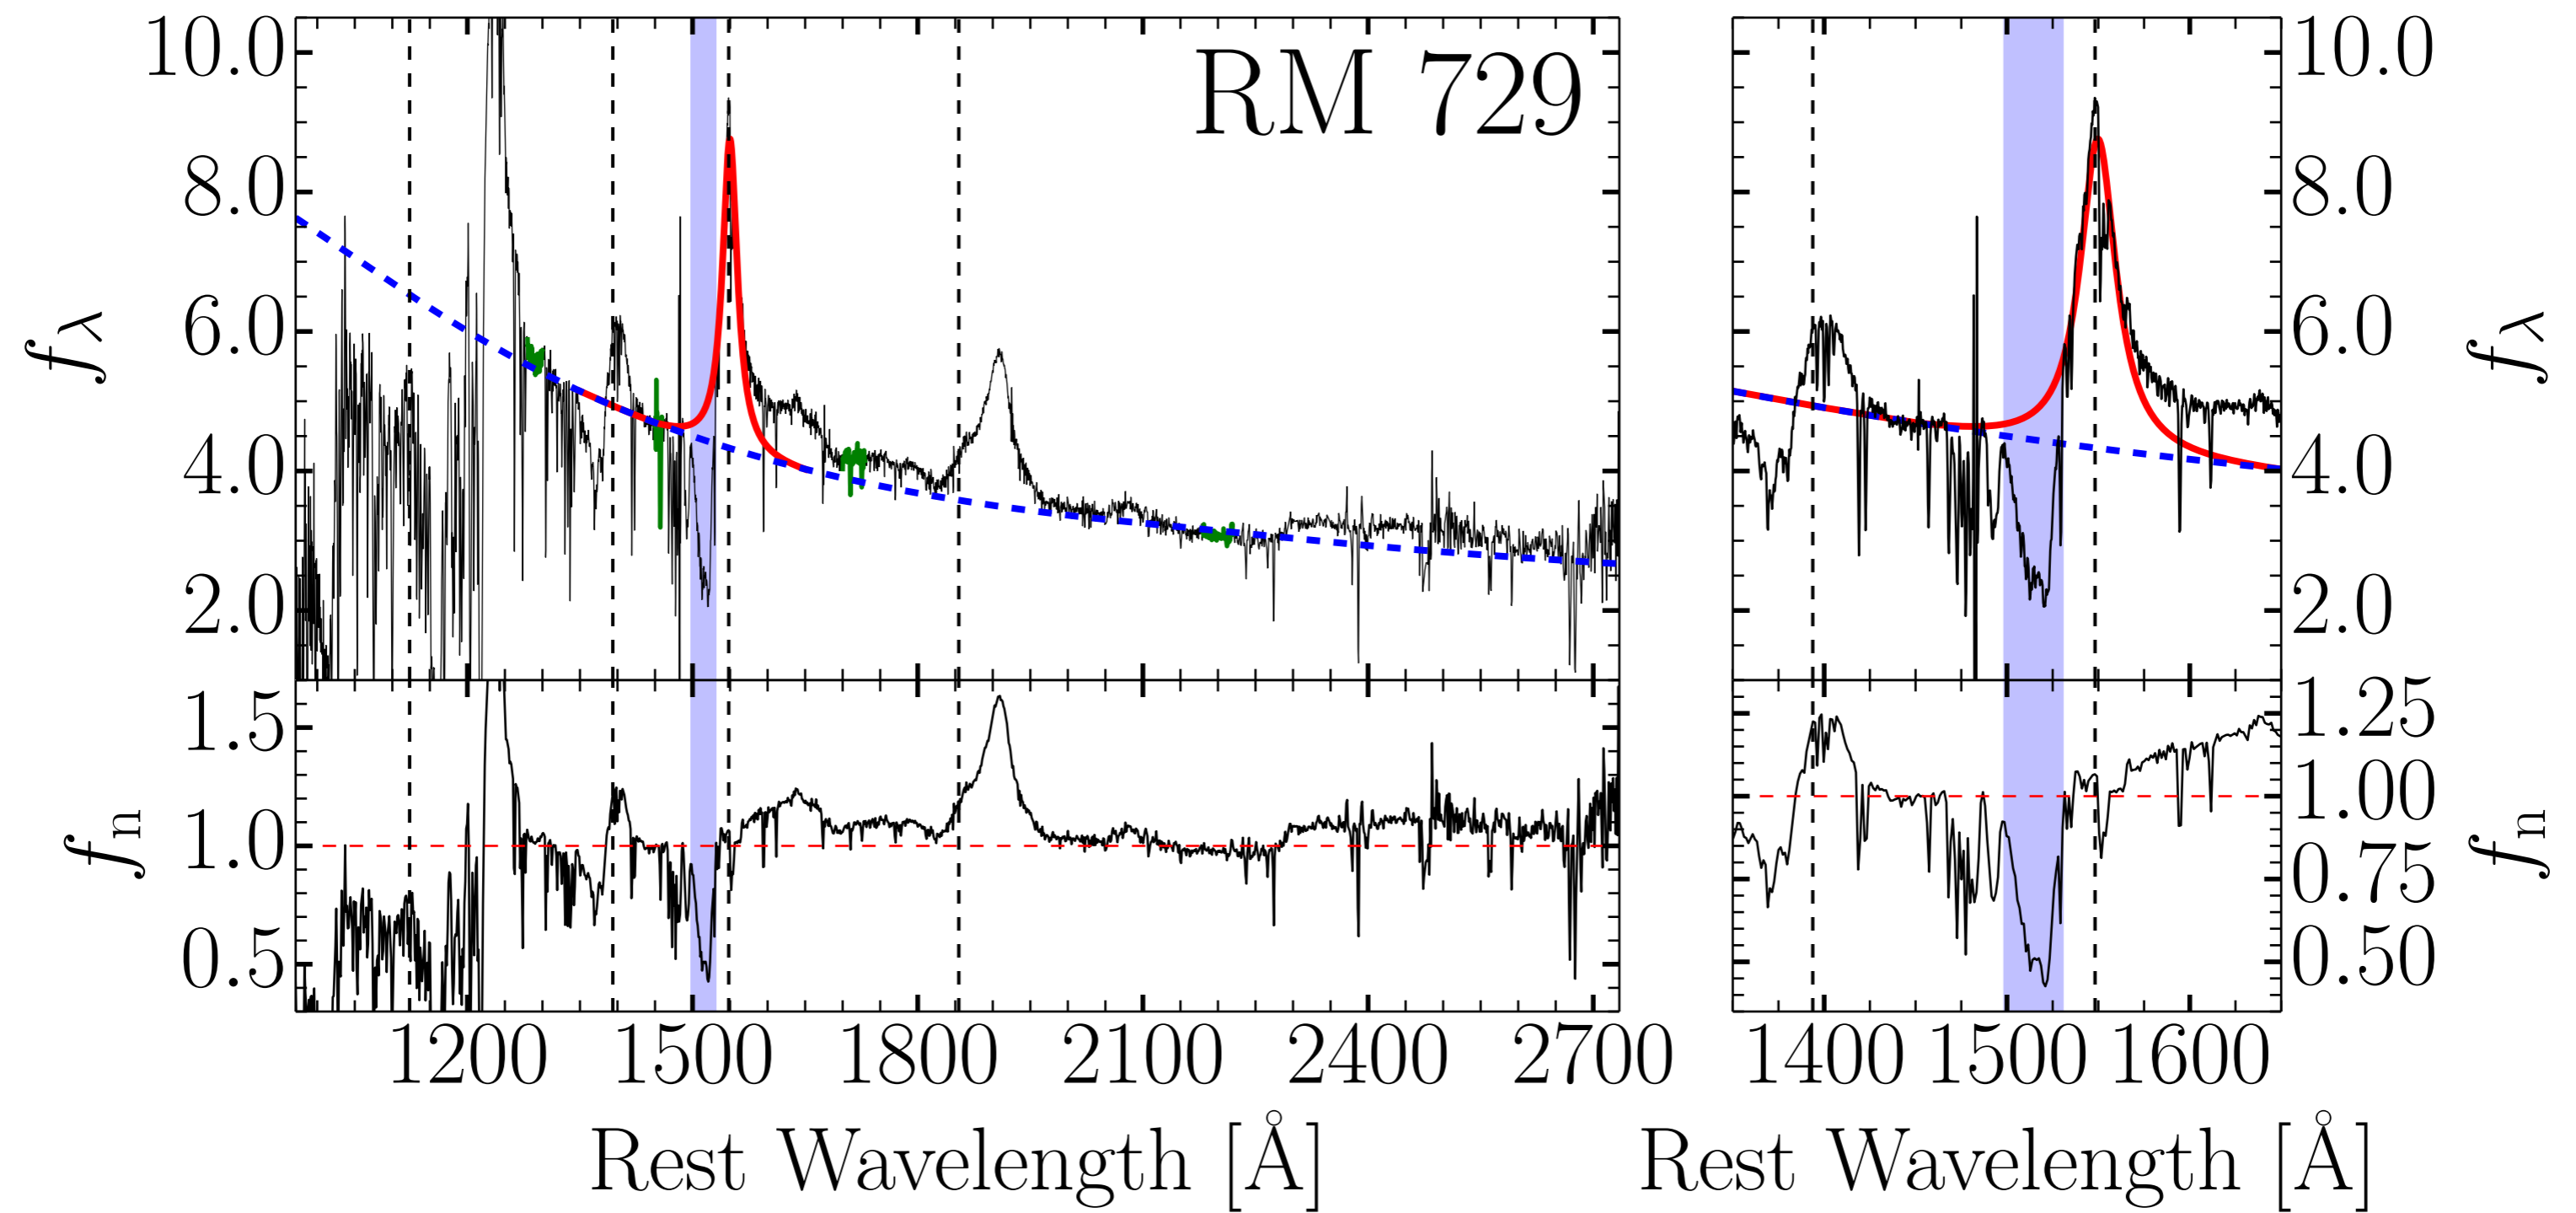

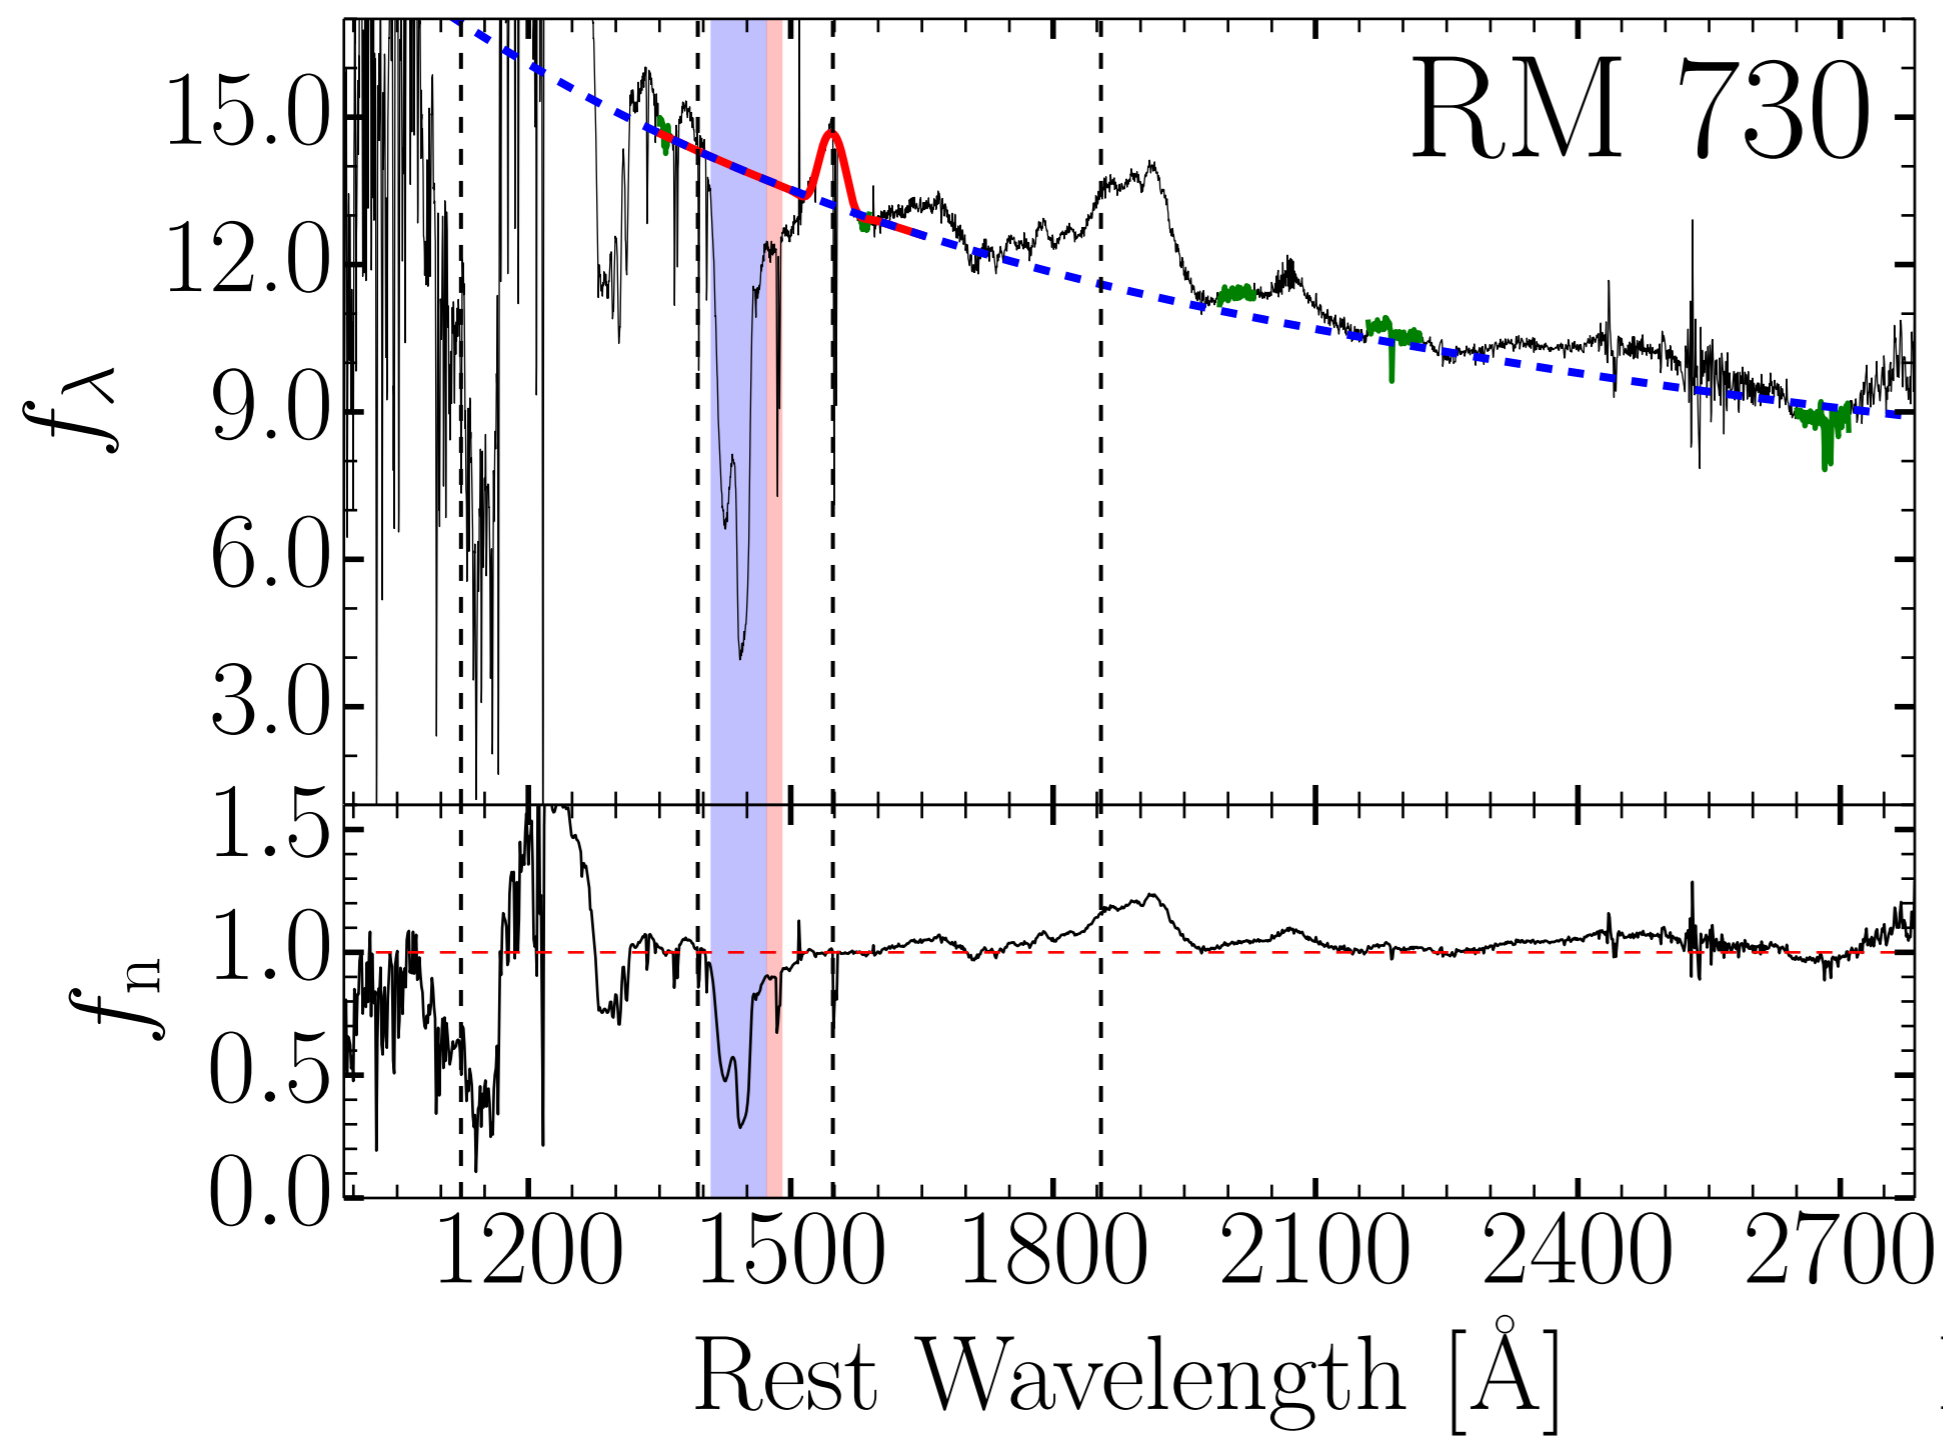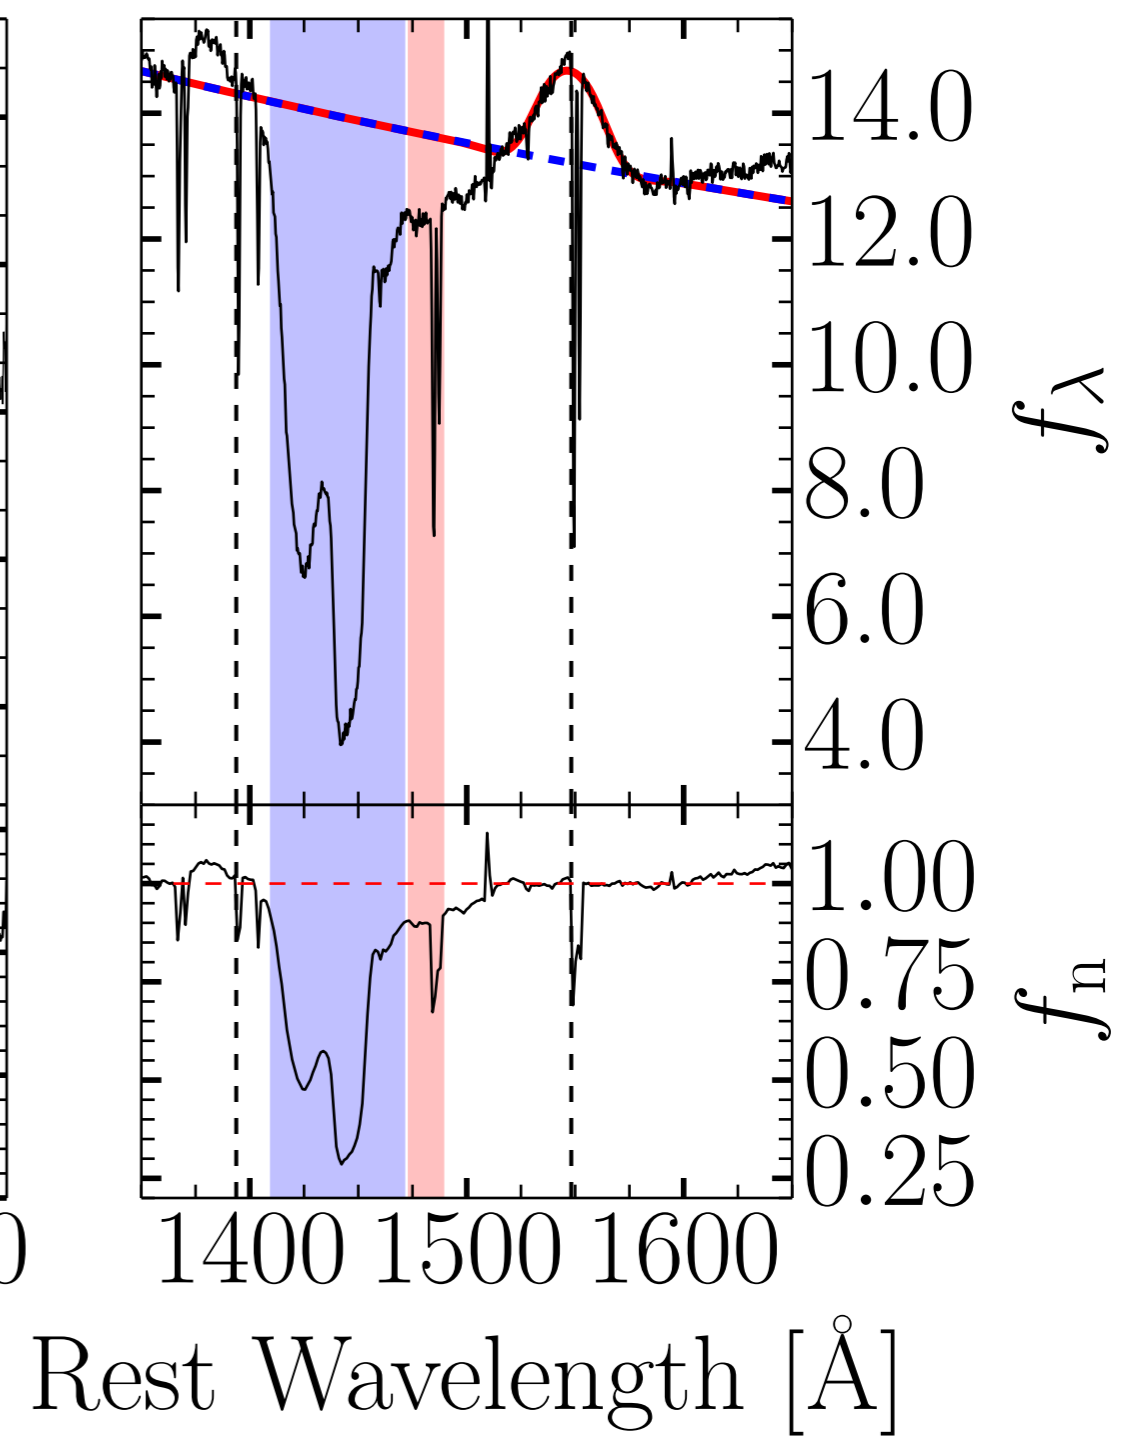

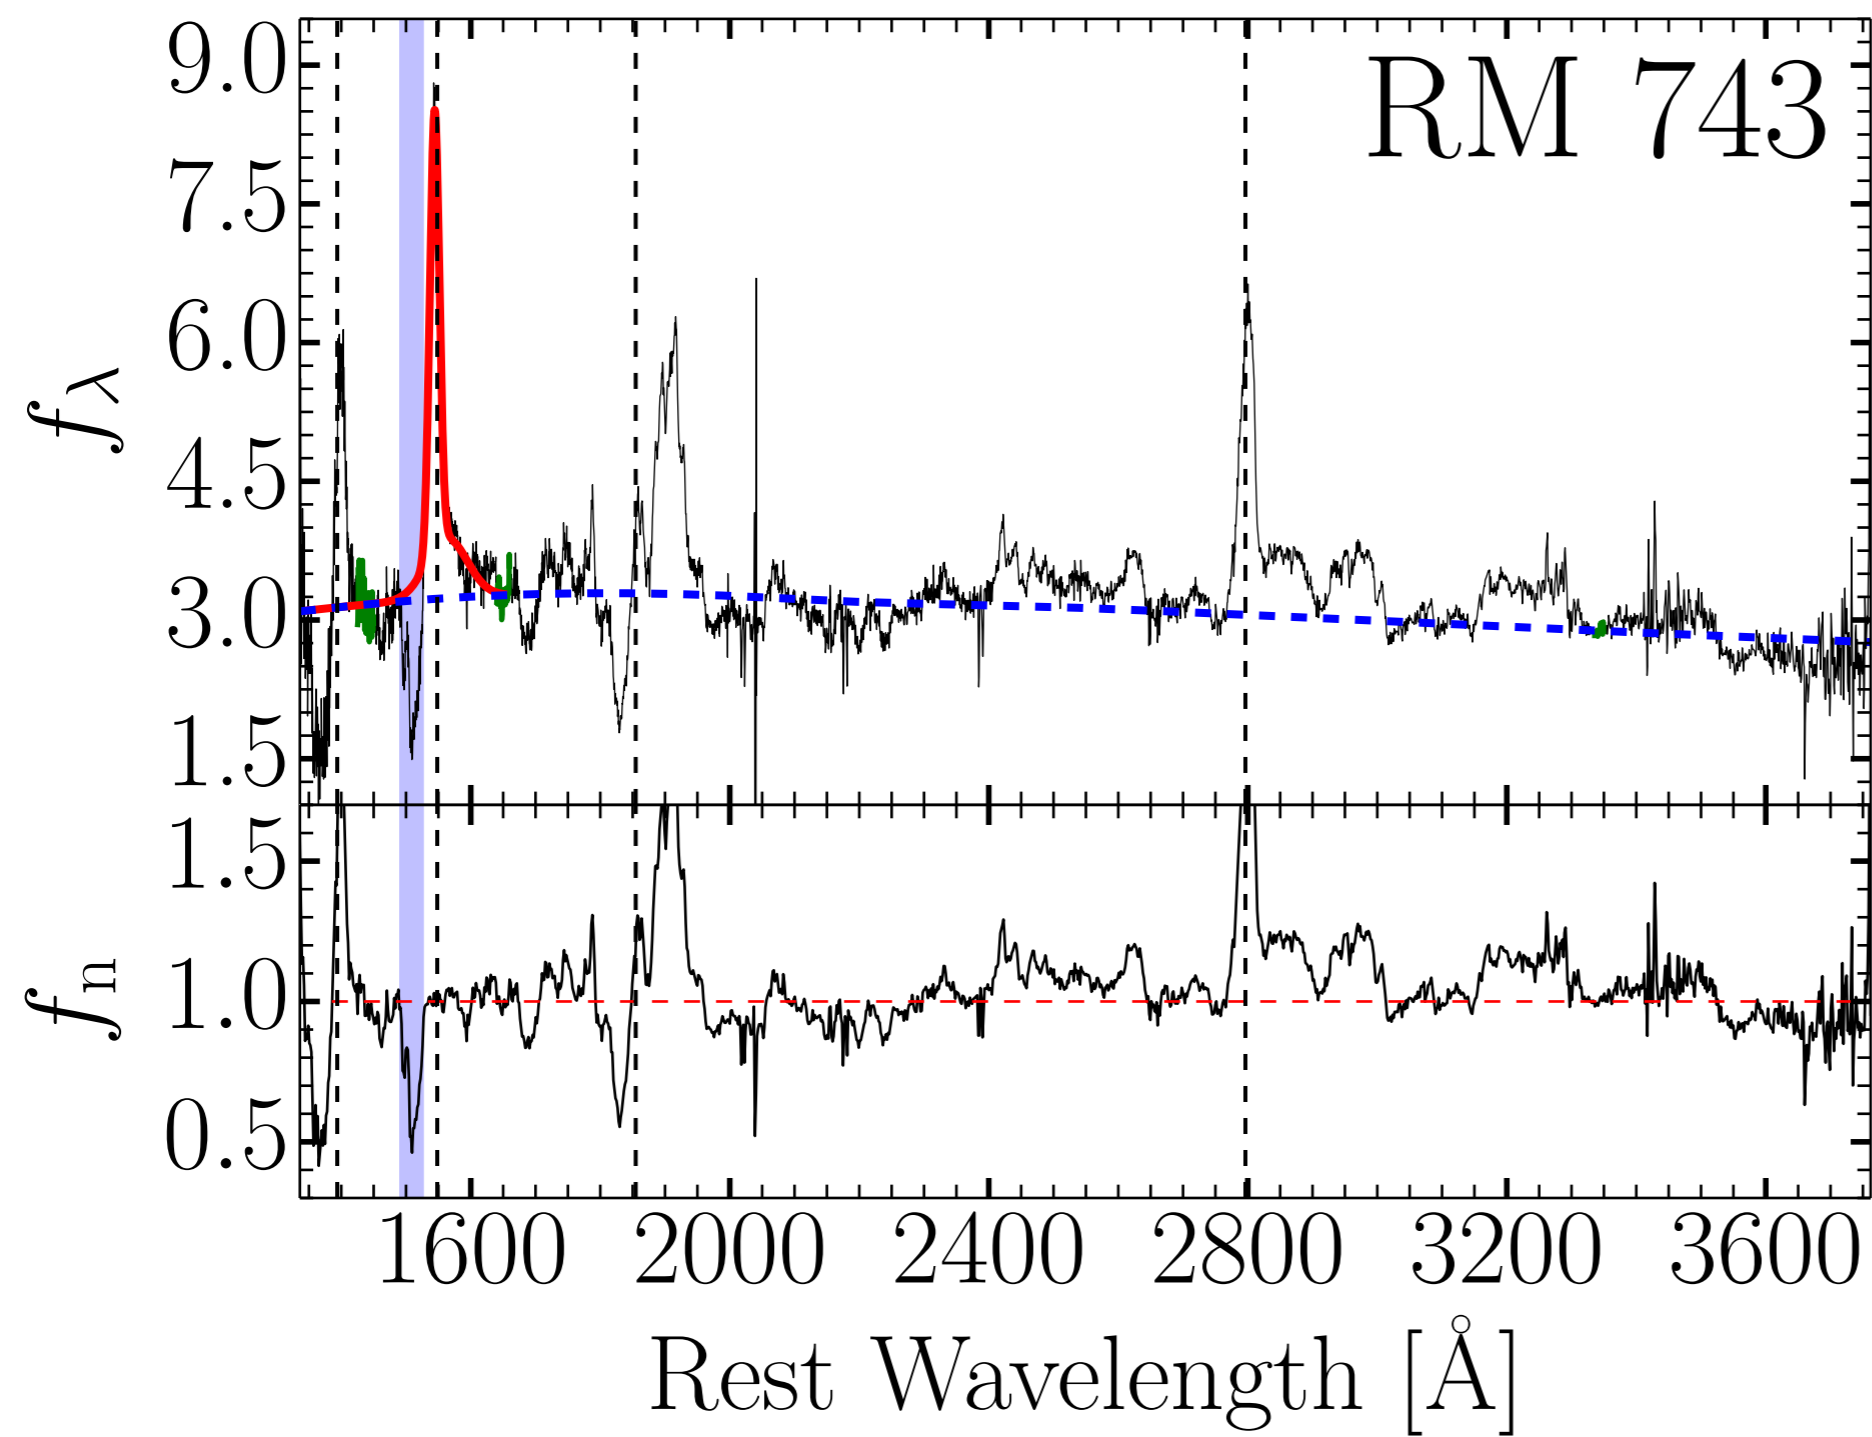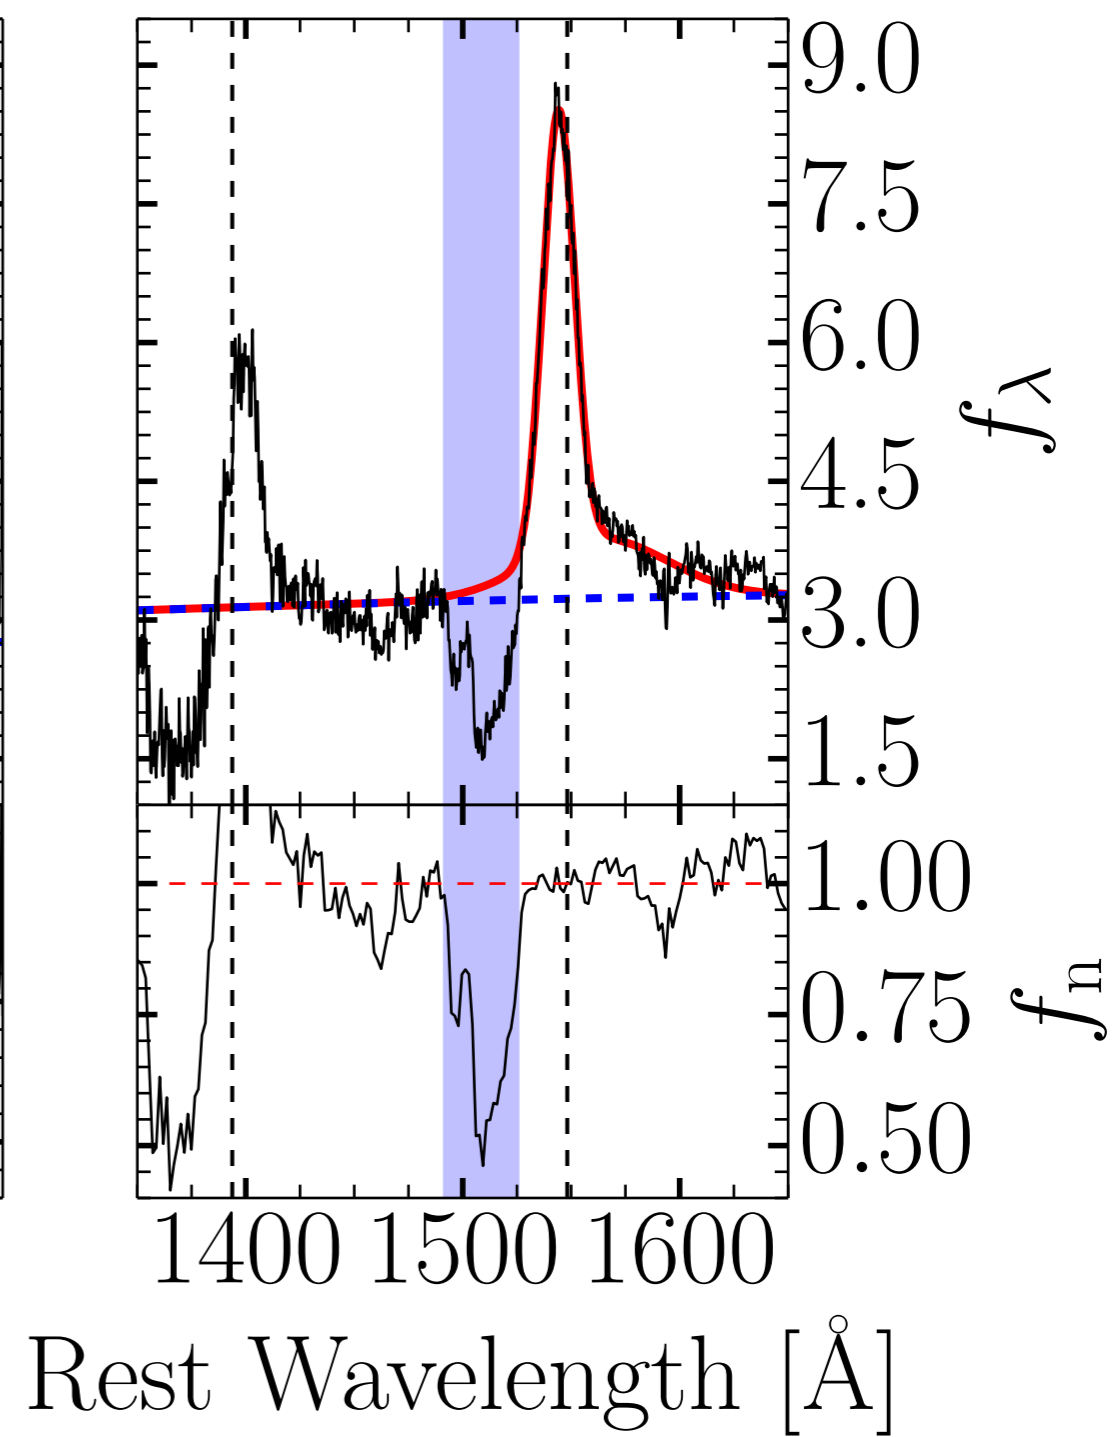

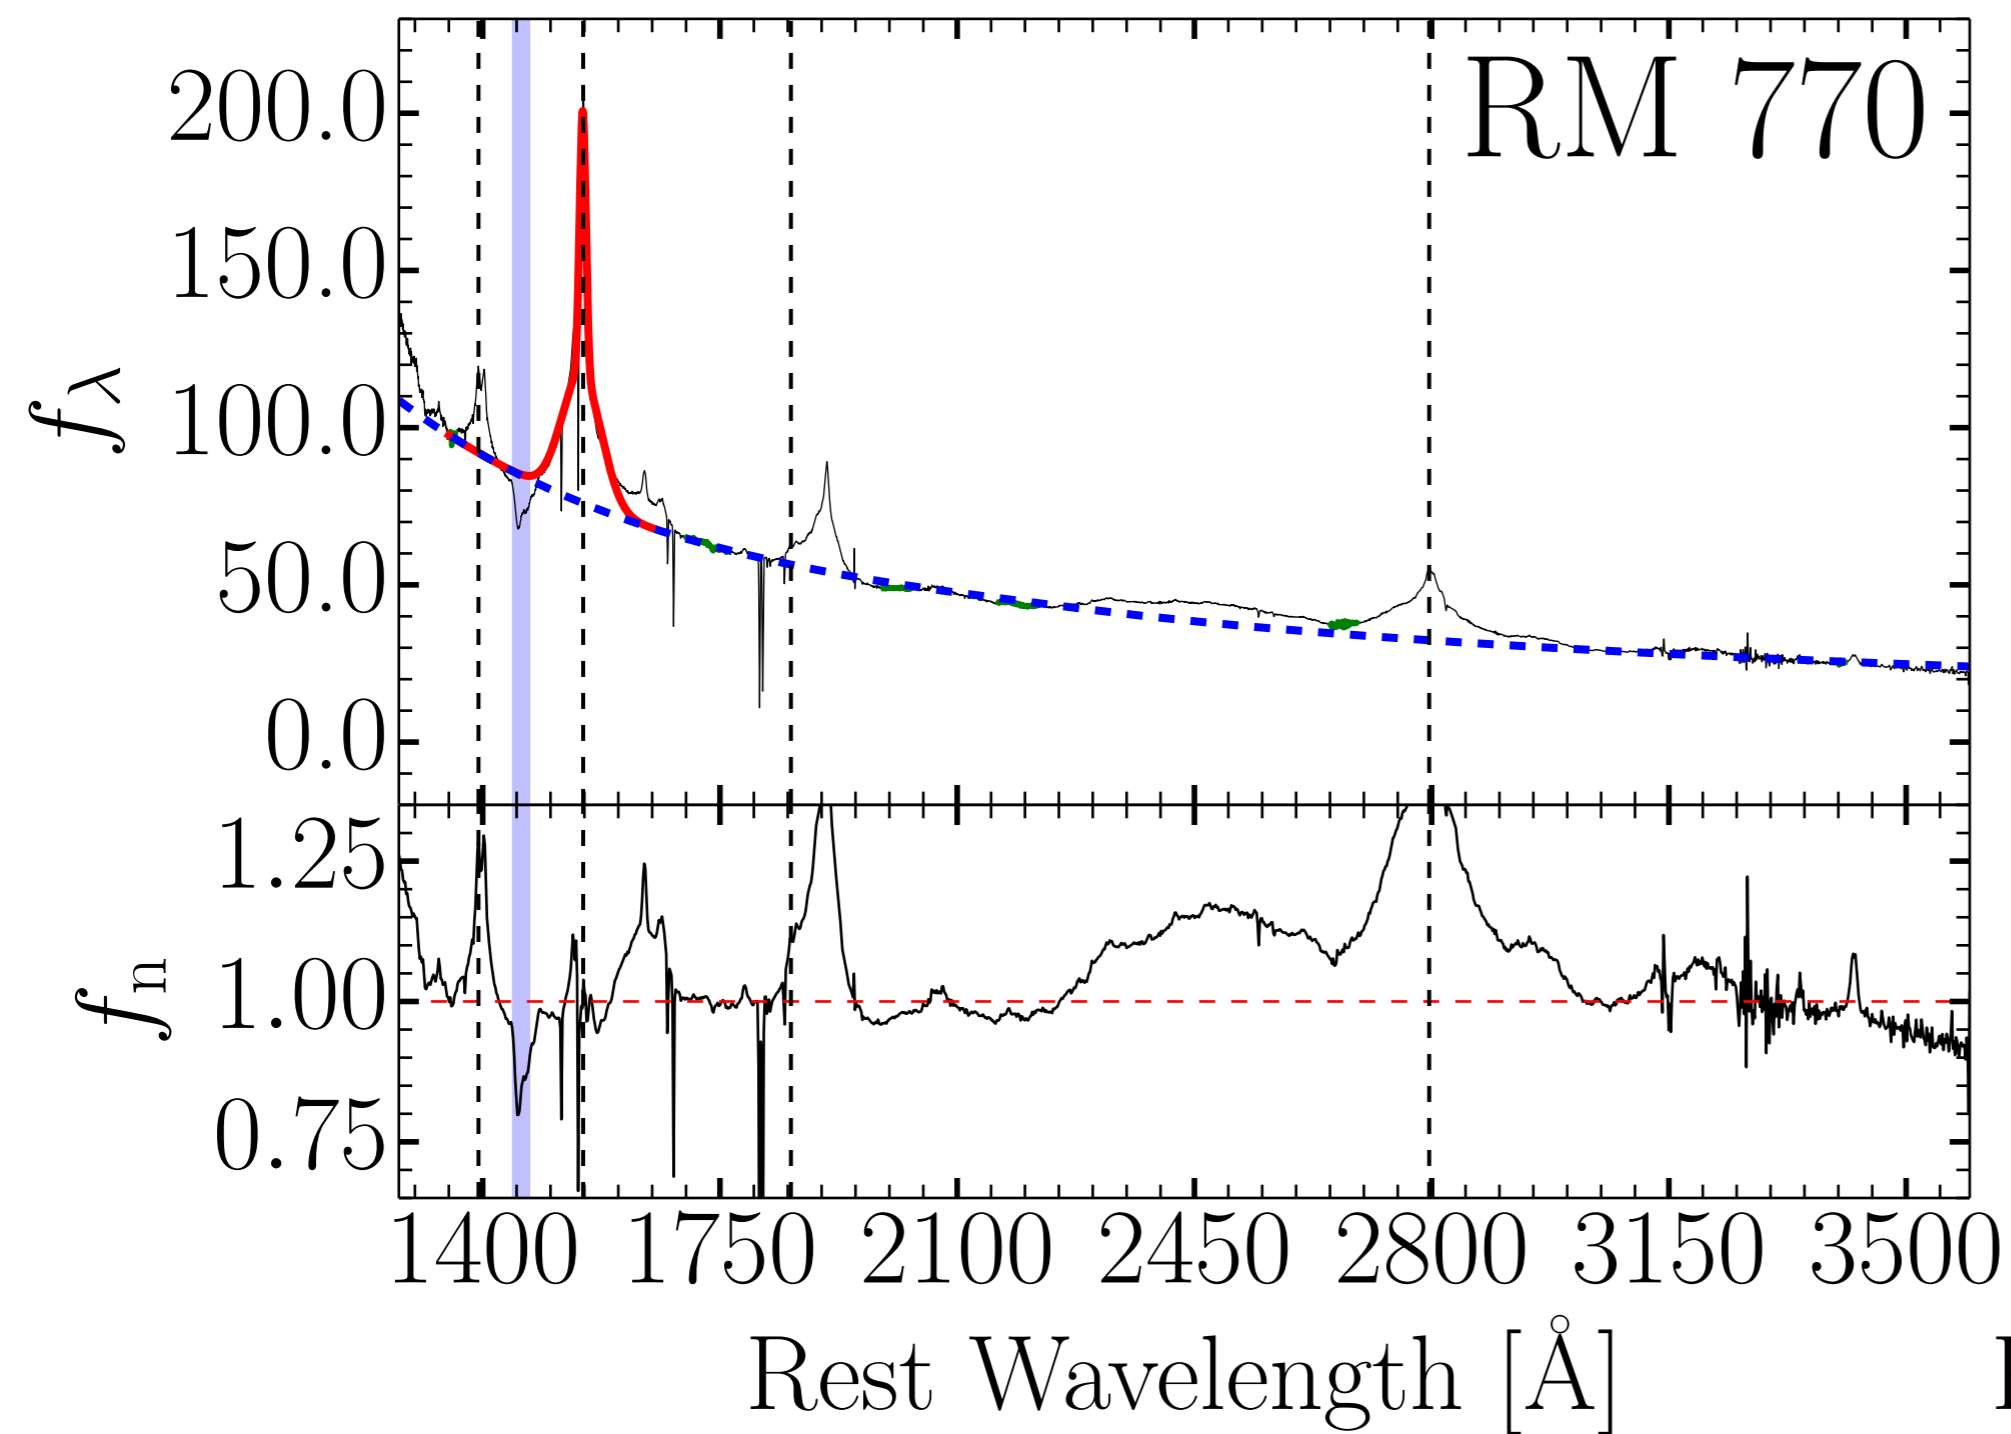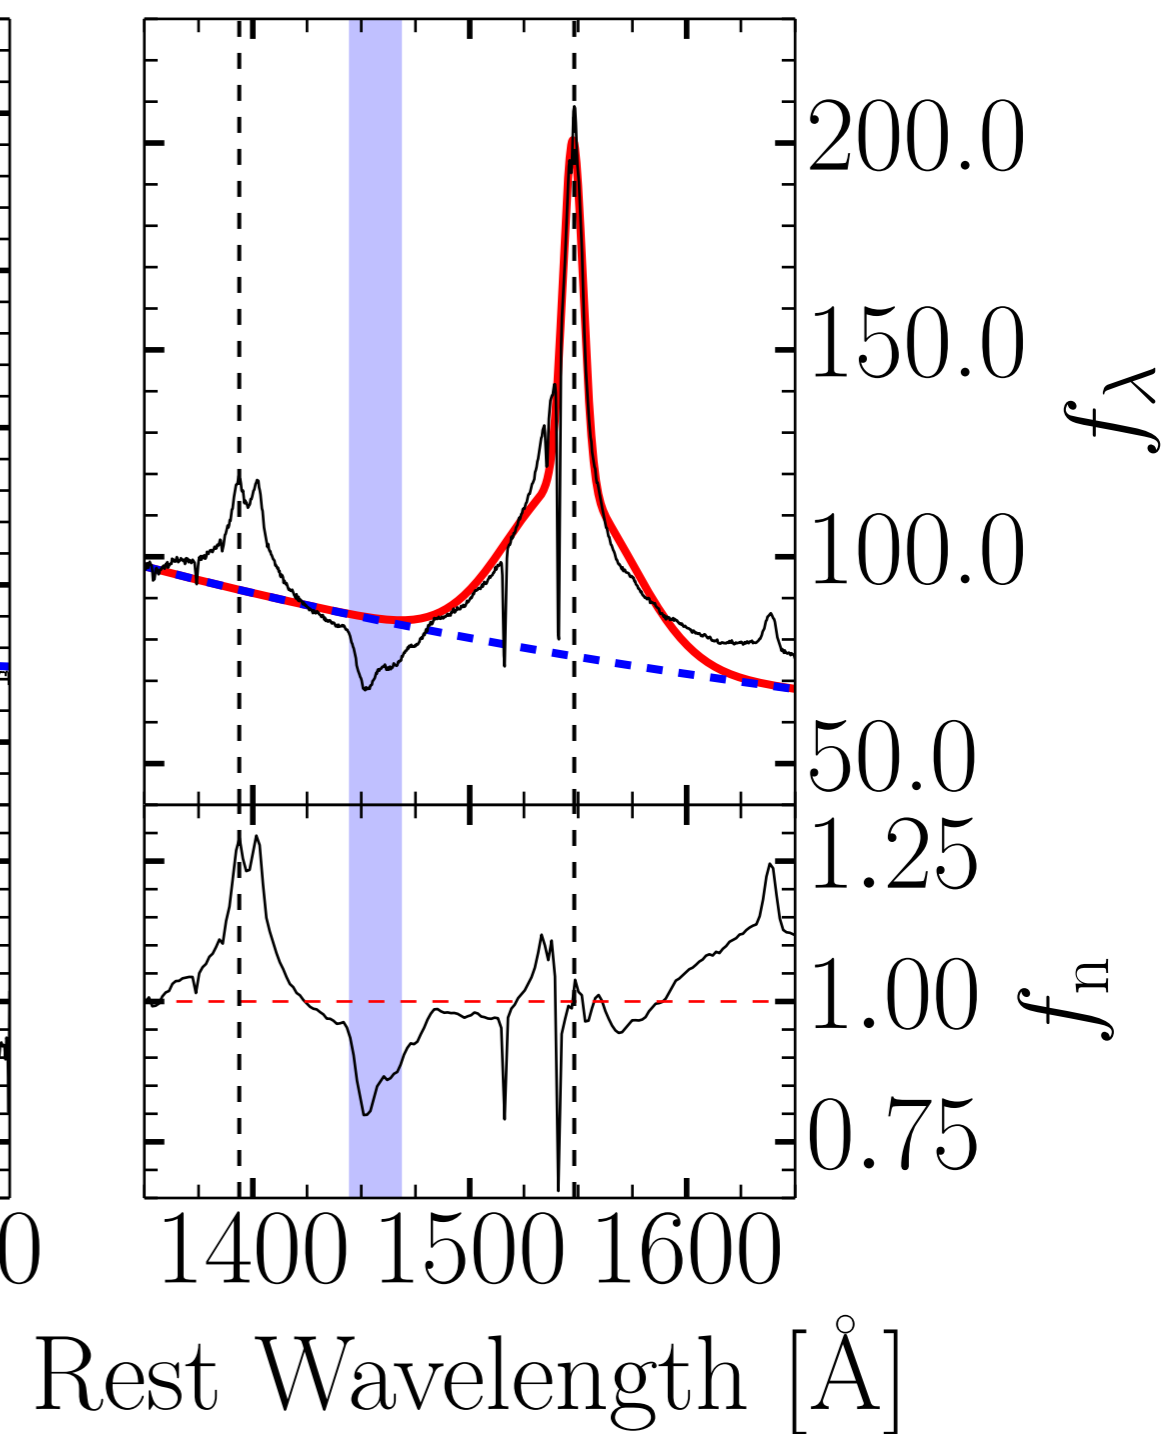

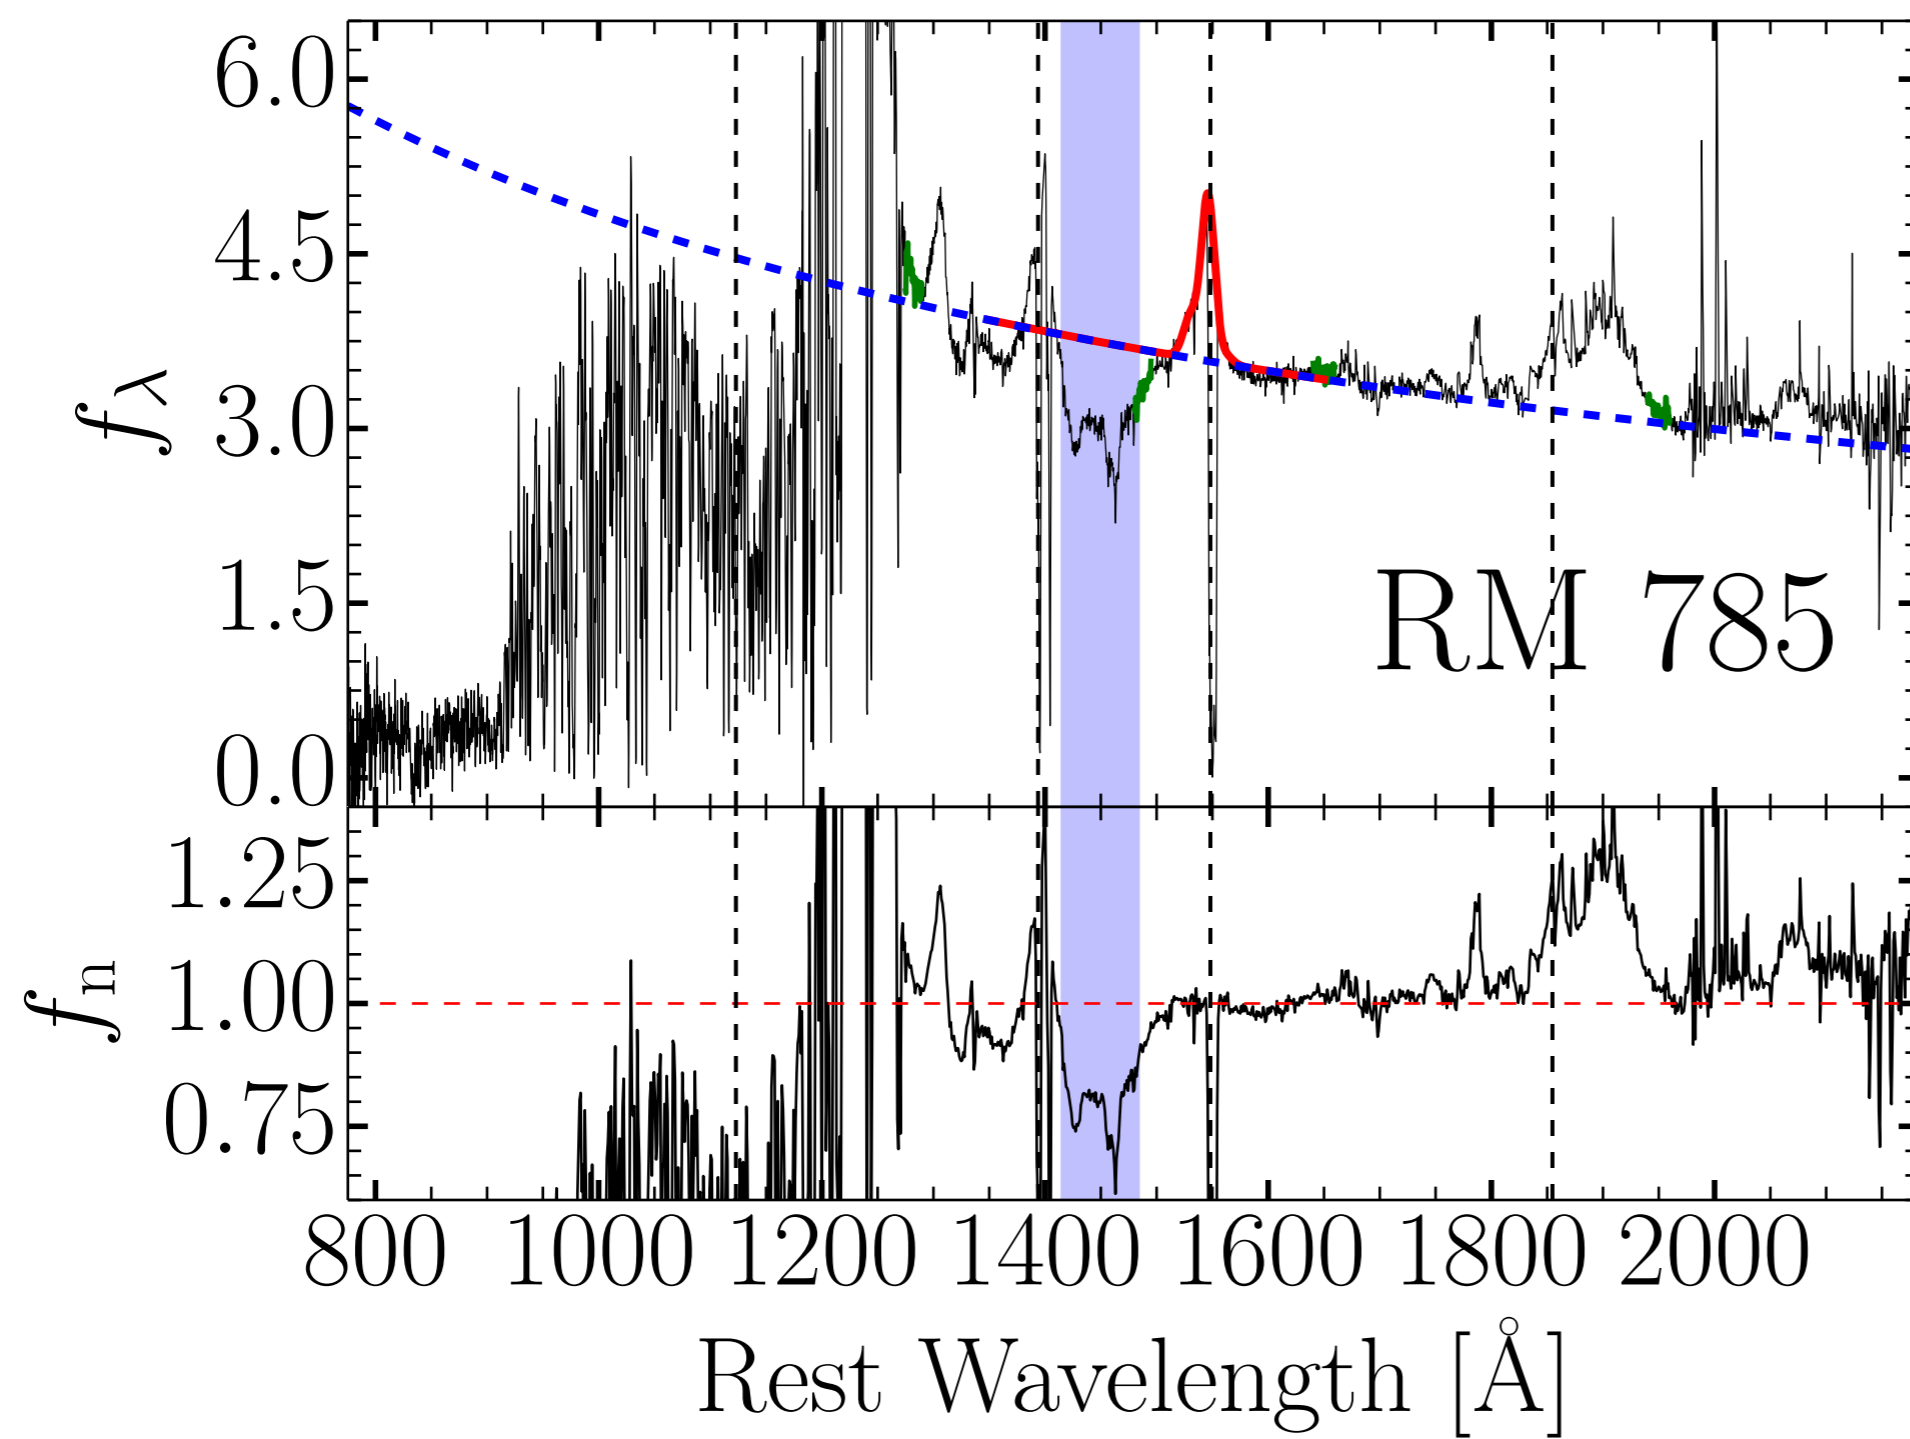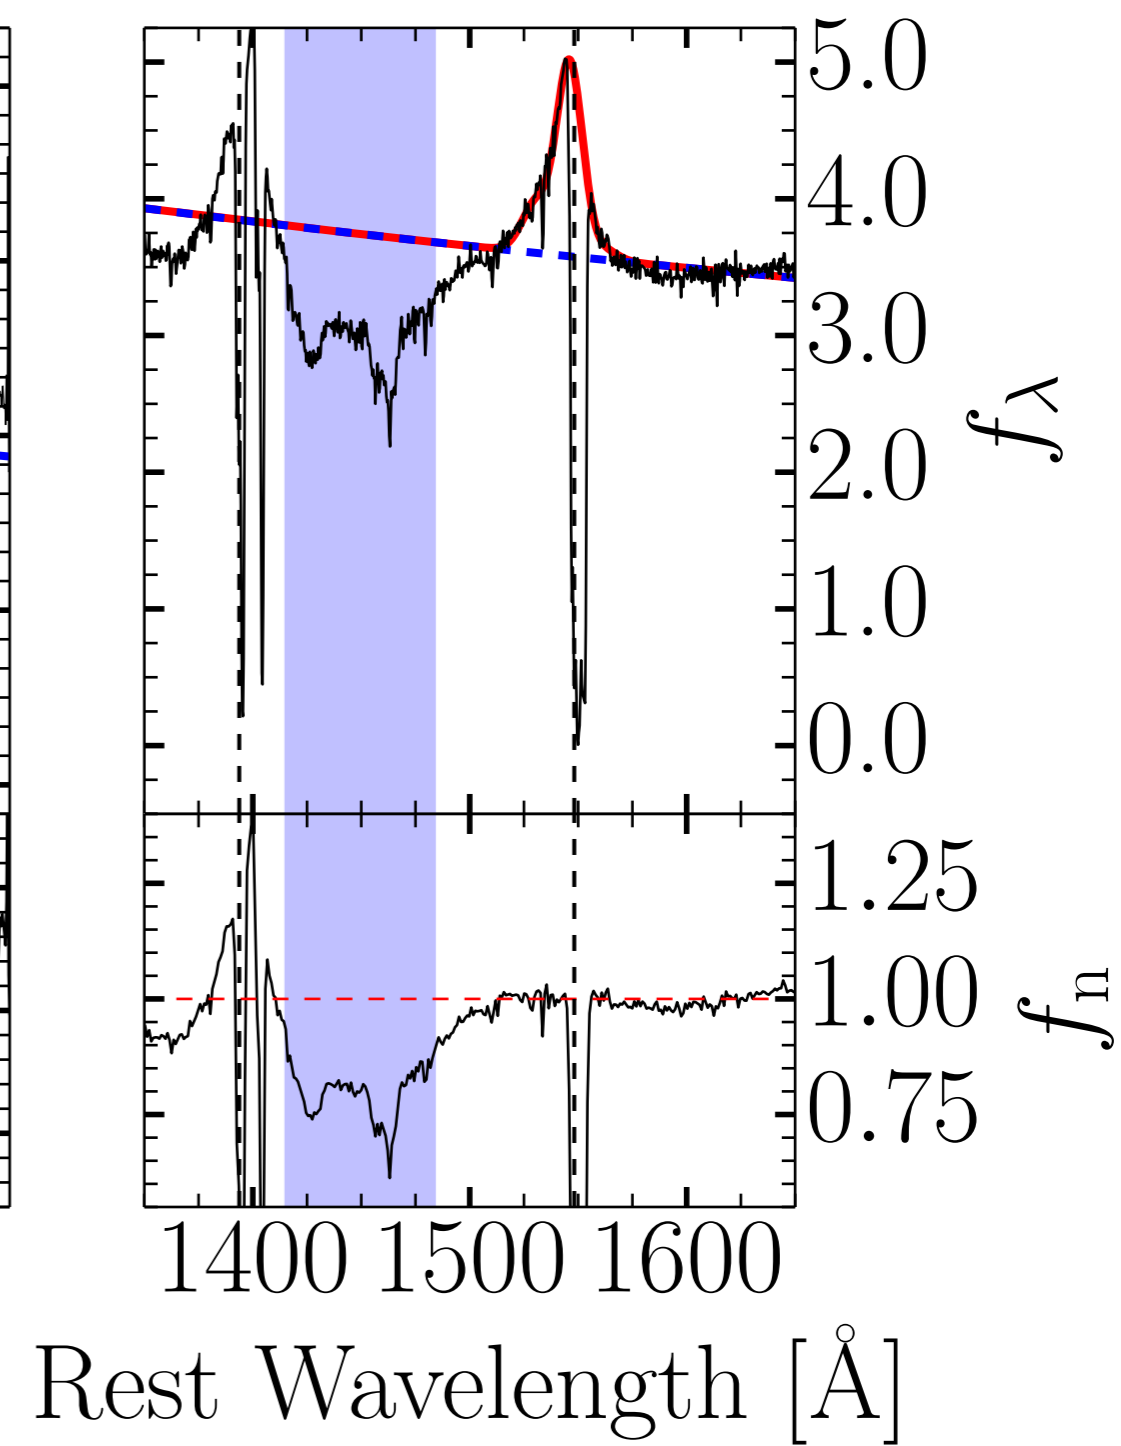

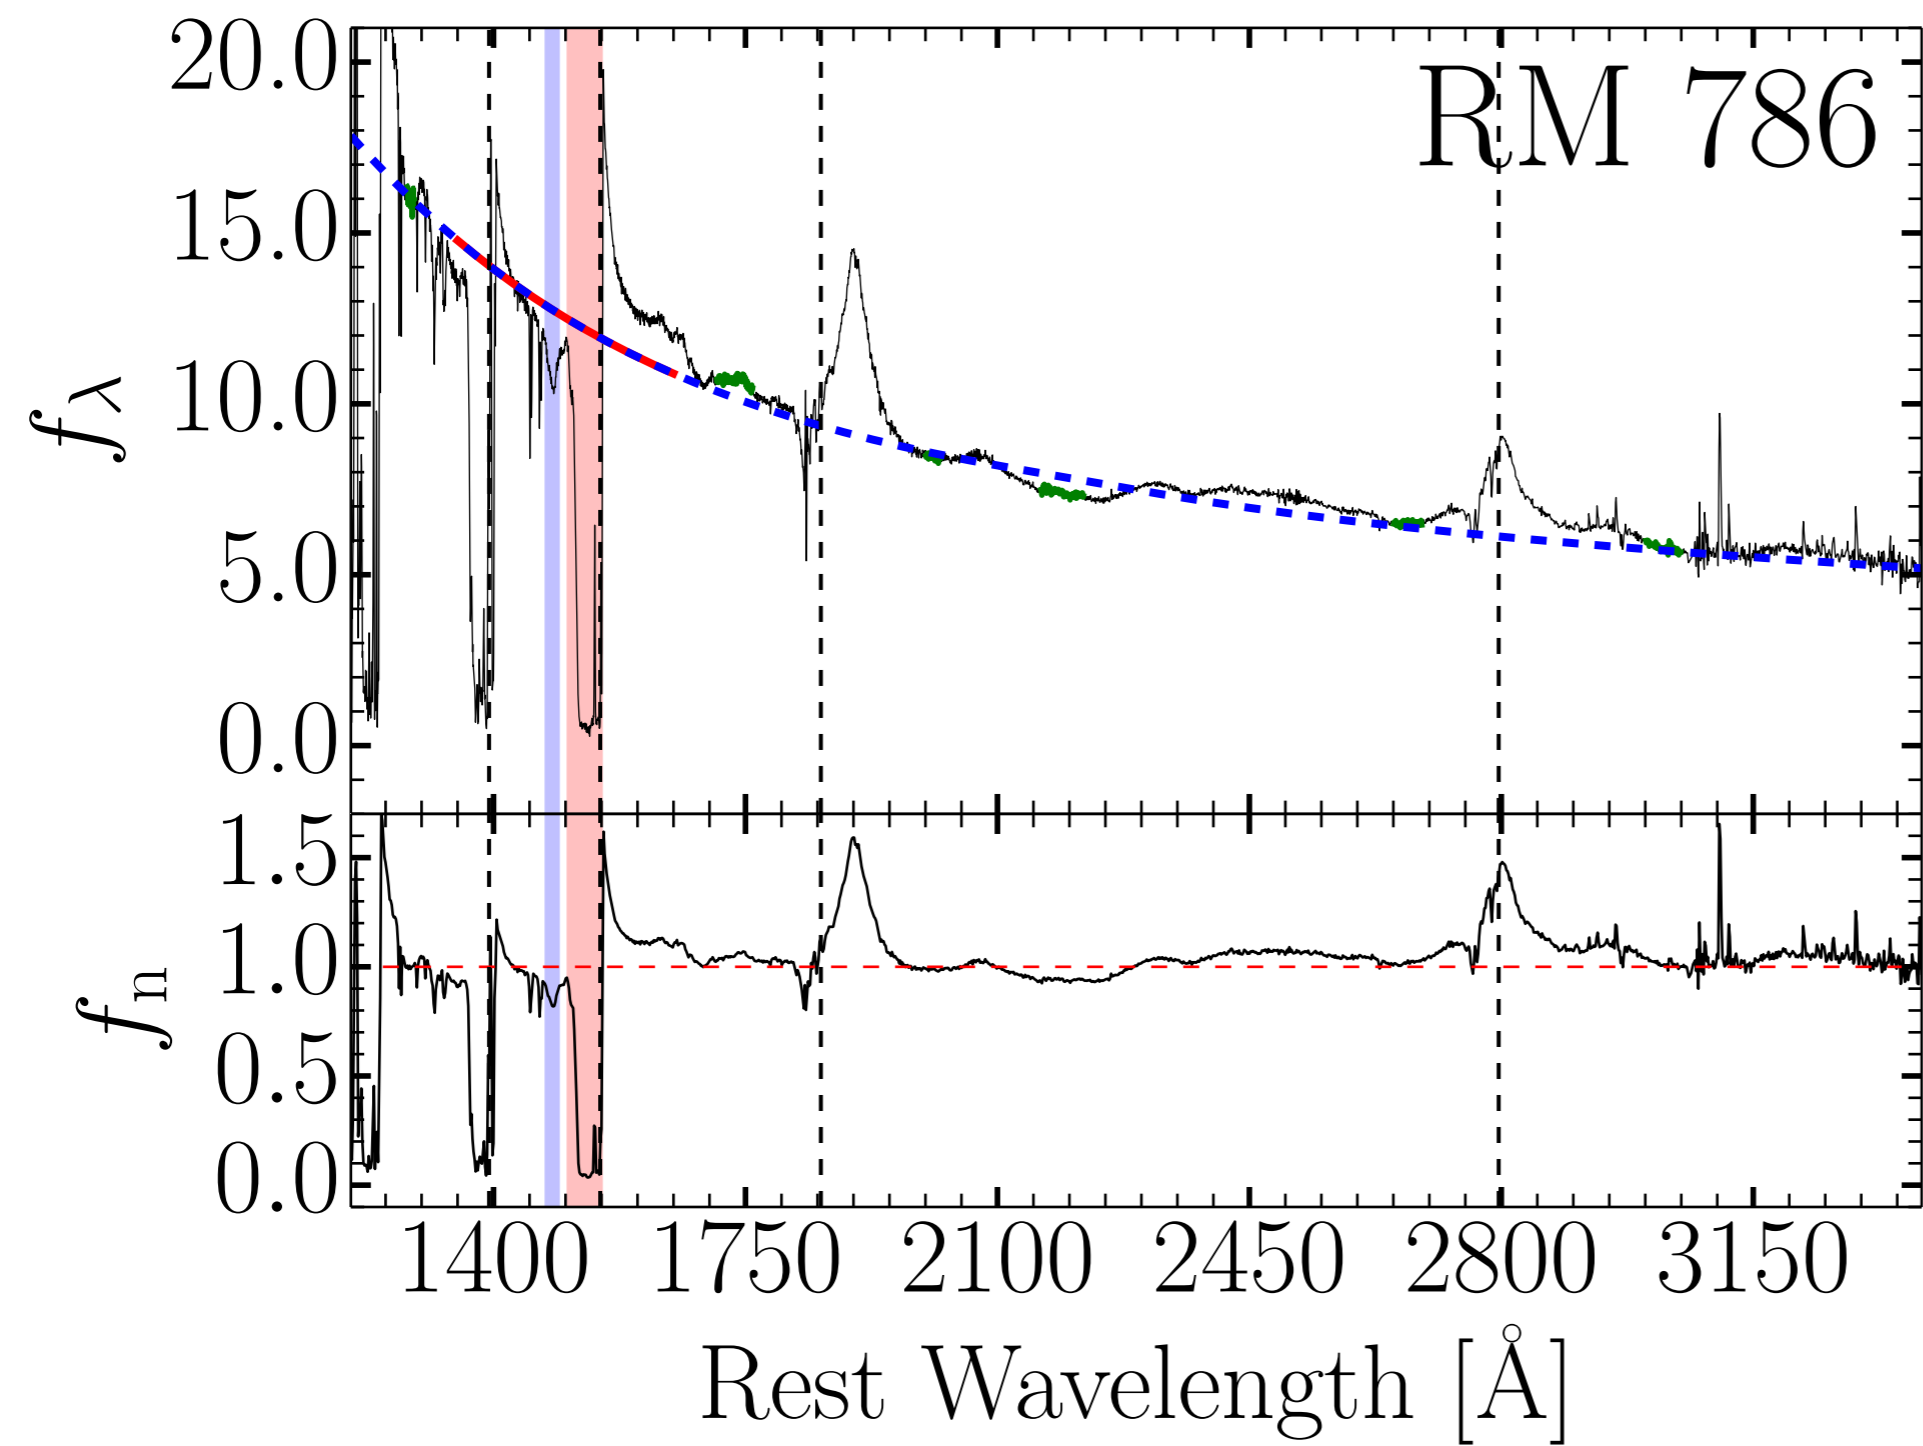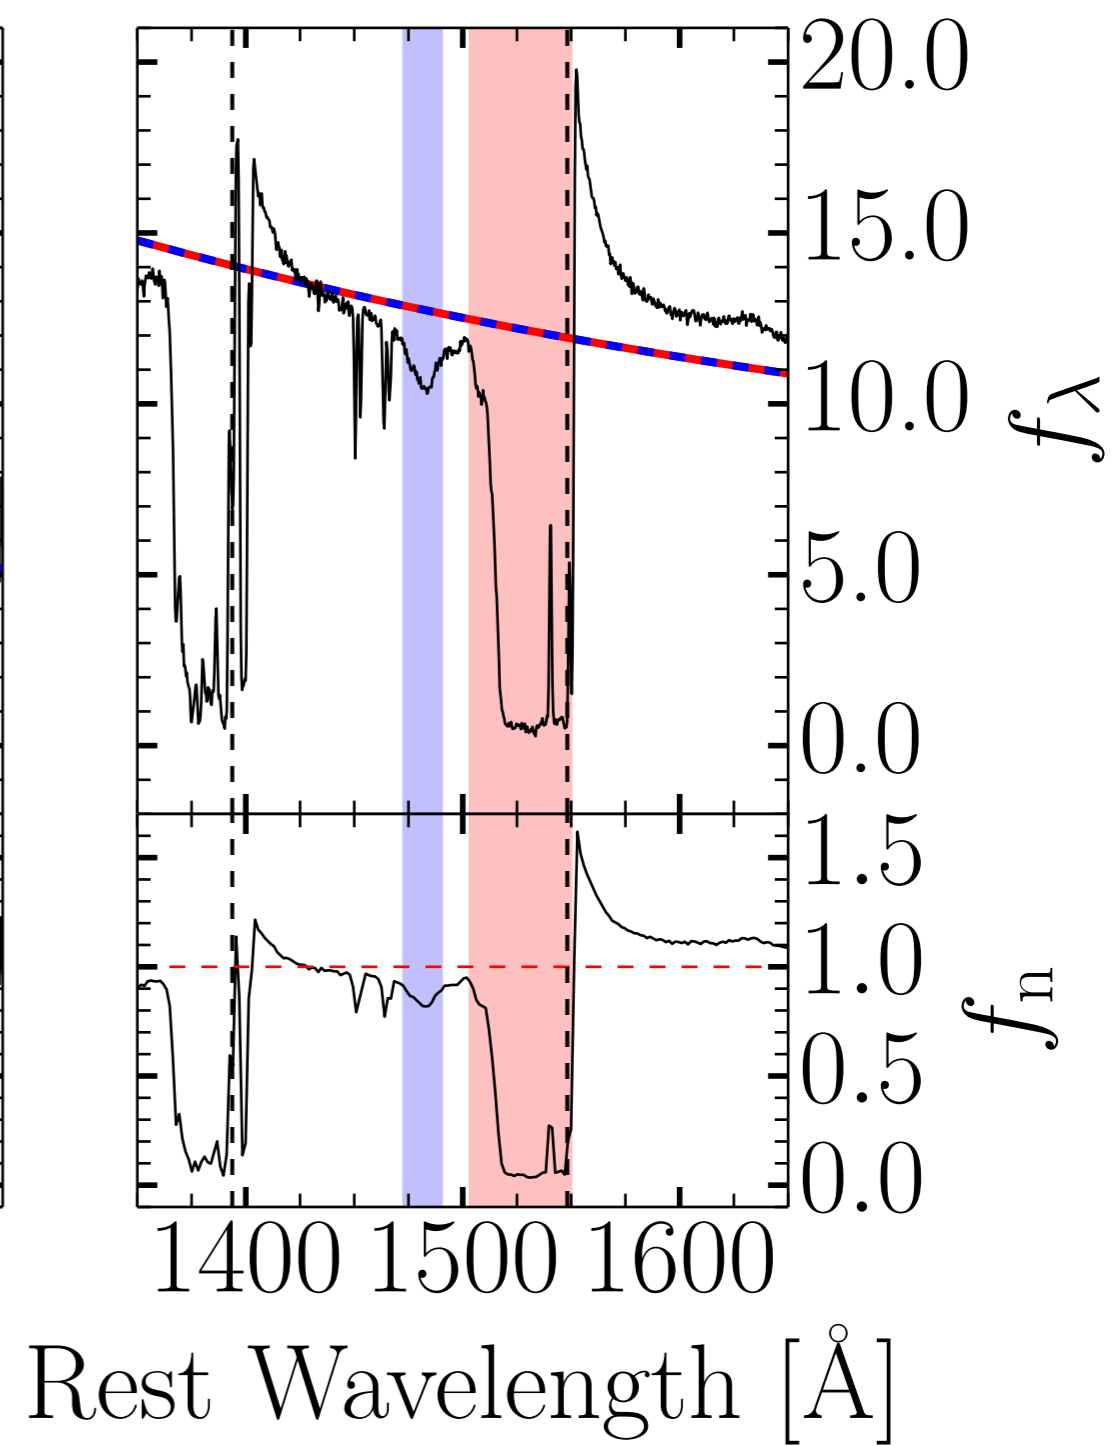

Supplement: Supplementary file 1 [file Figure3Set.pdf]
