# Supplementary material for: The Sloan Digital Sky Survey Reverberation Mapping Project: Systematic Investigations of Short-Timescale CIV Broad Absorption Line Variability
Source: arXiv:1811.00010 ancillary file (2018-10-31)

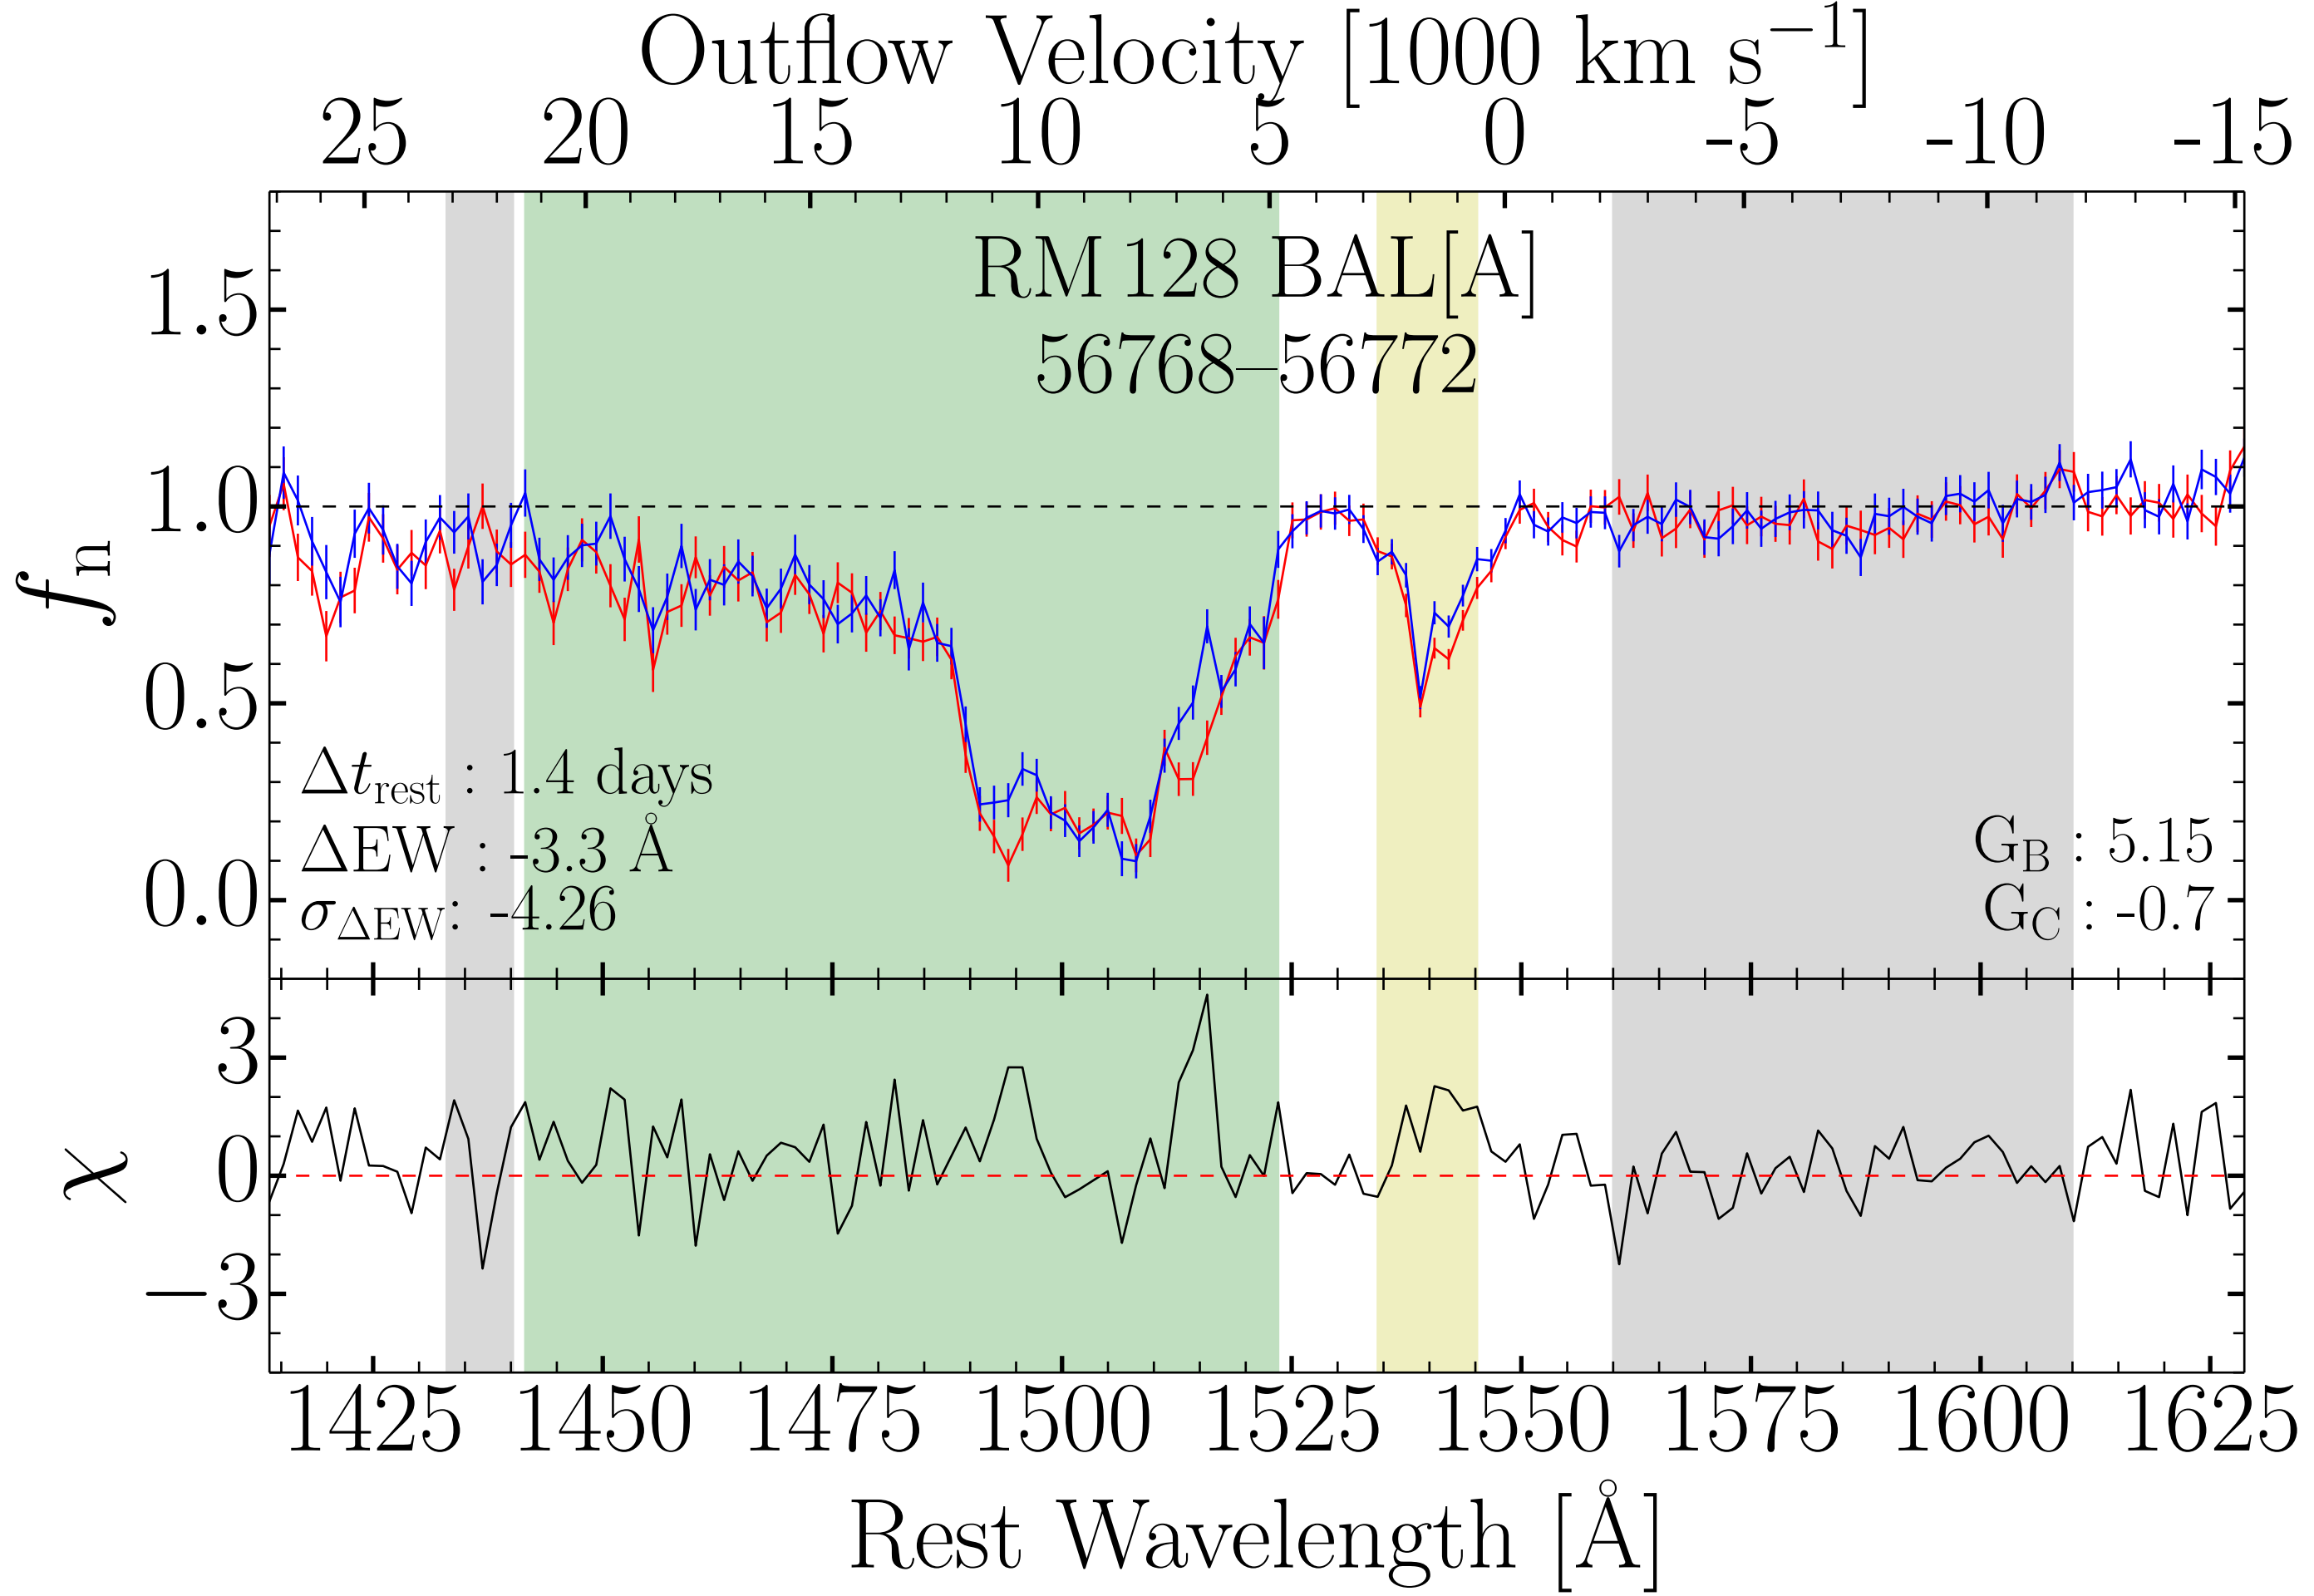

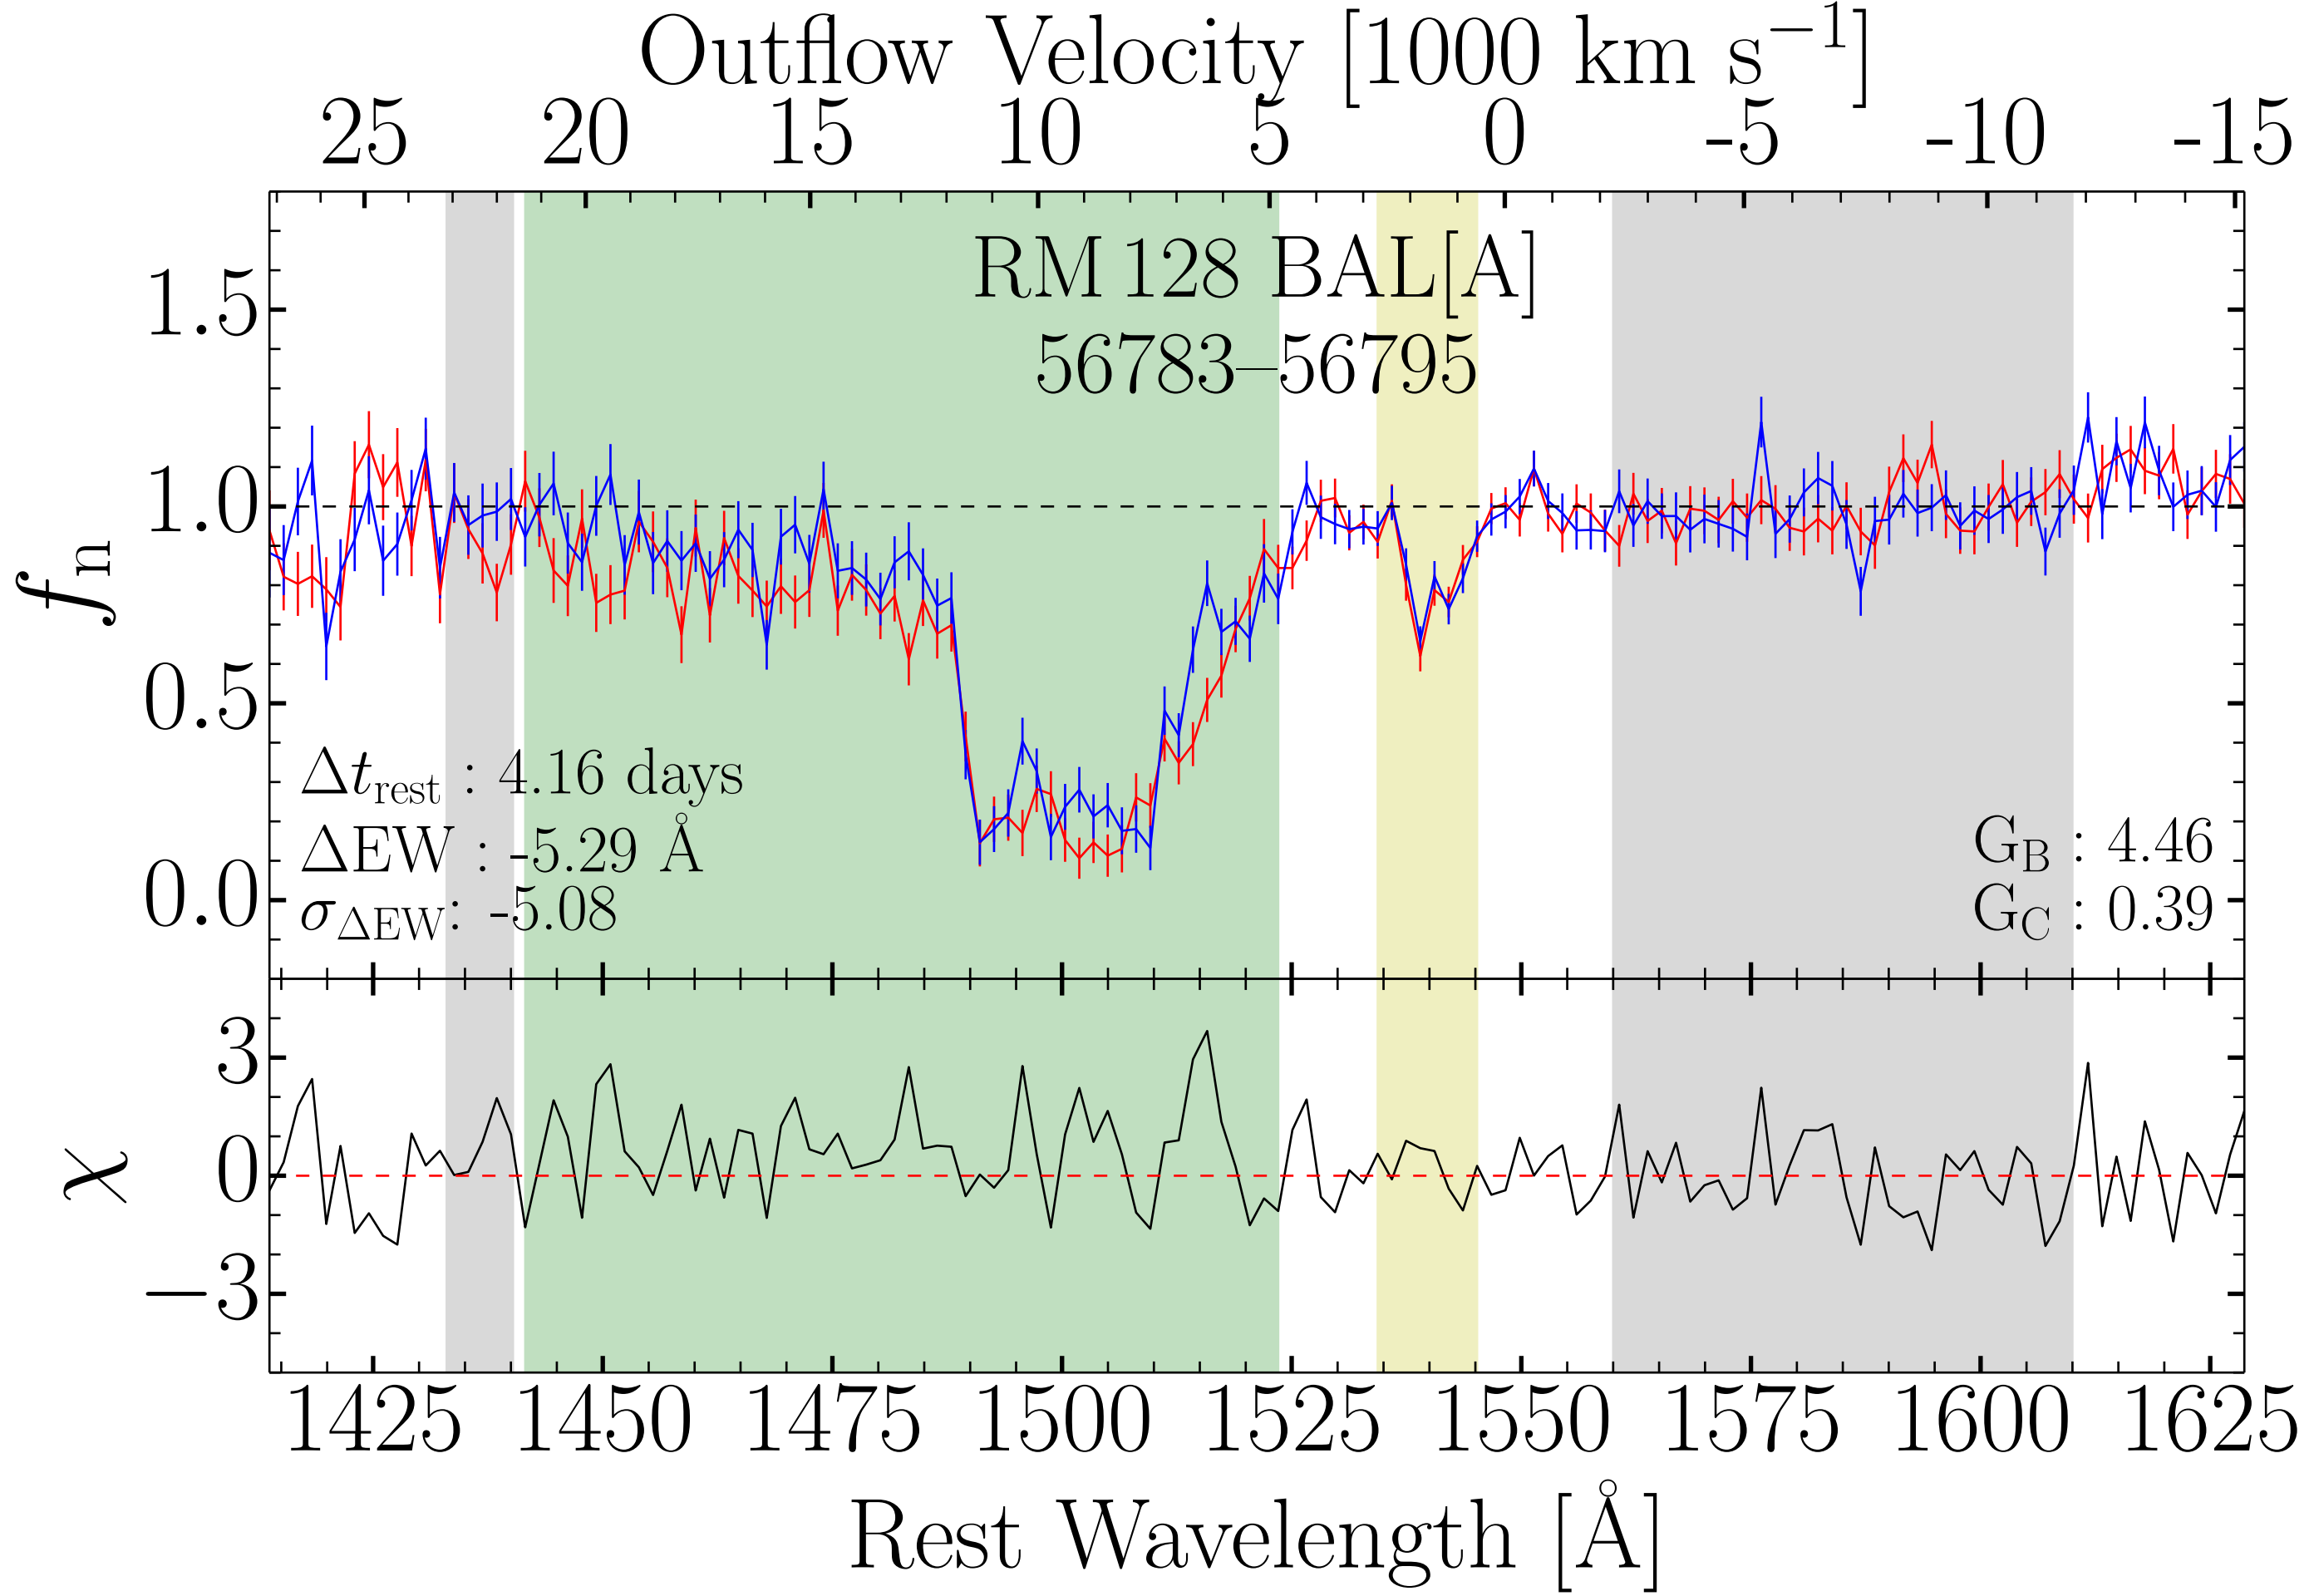

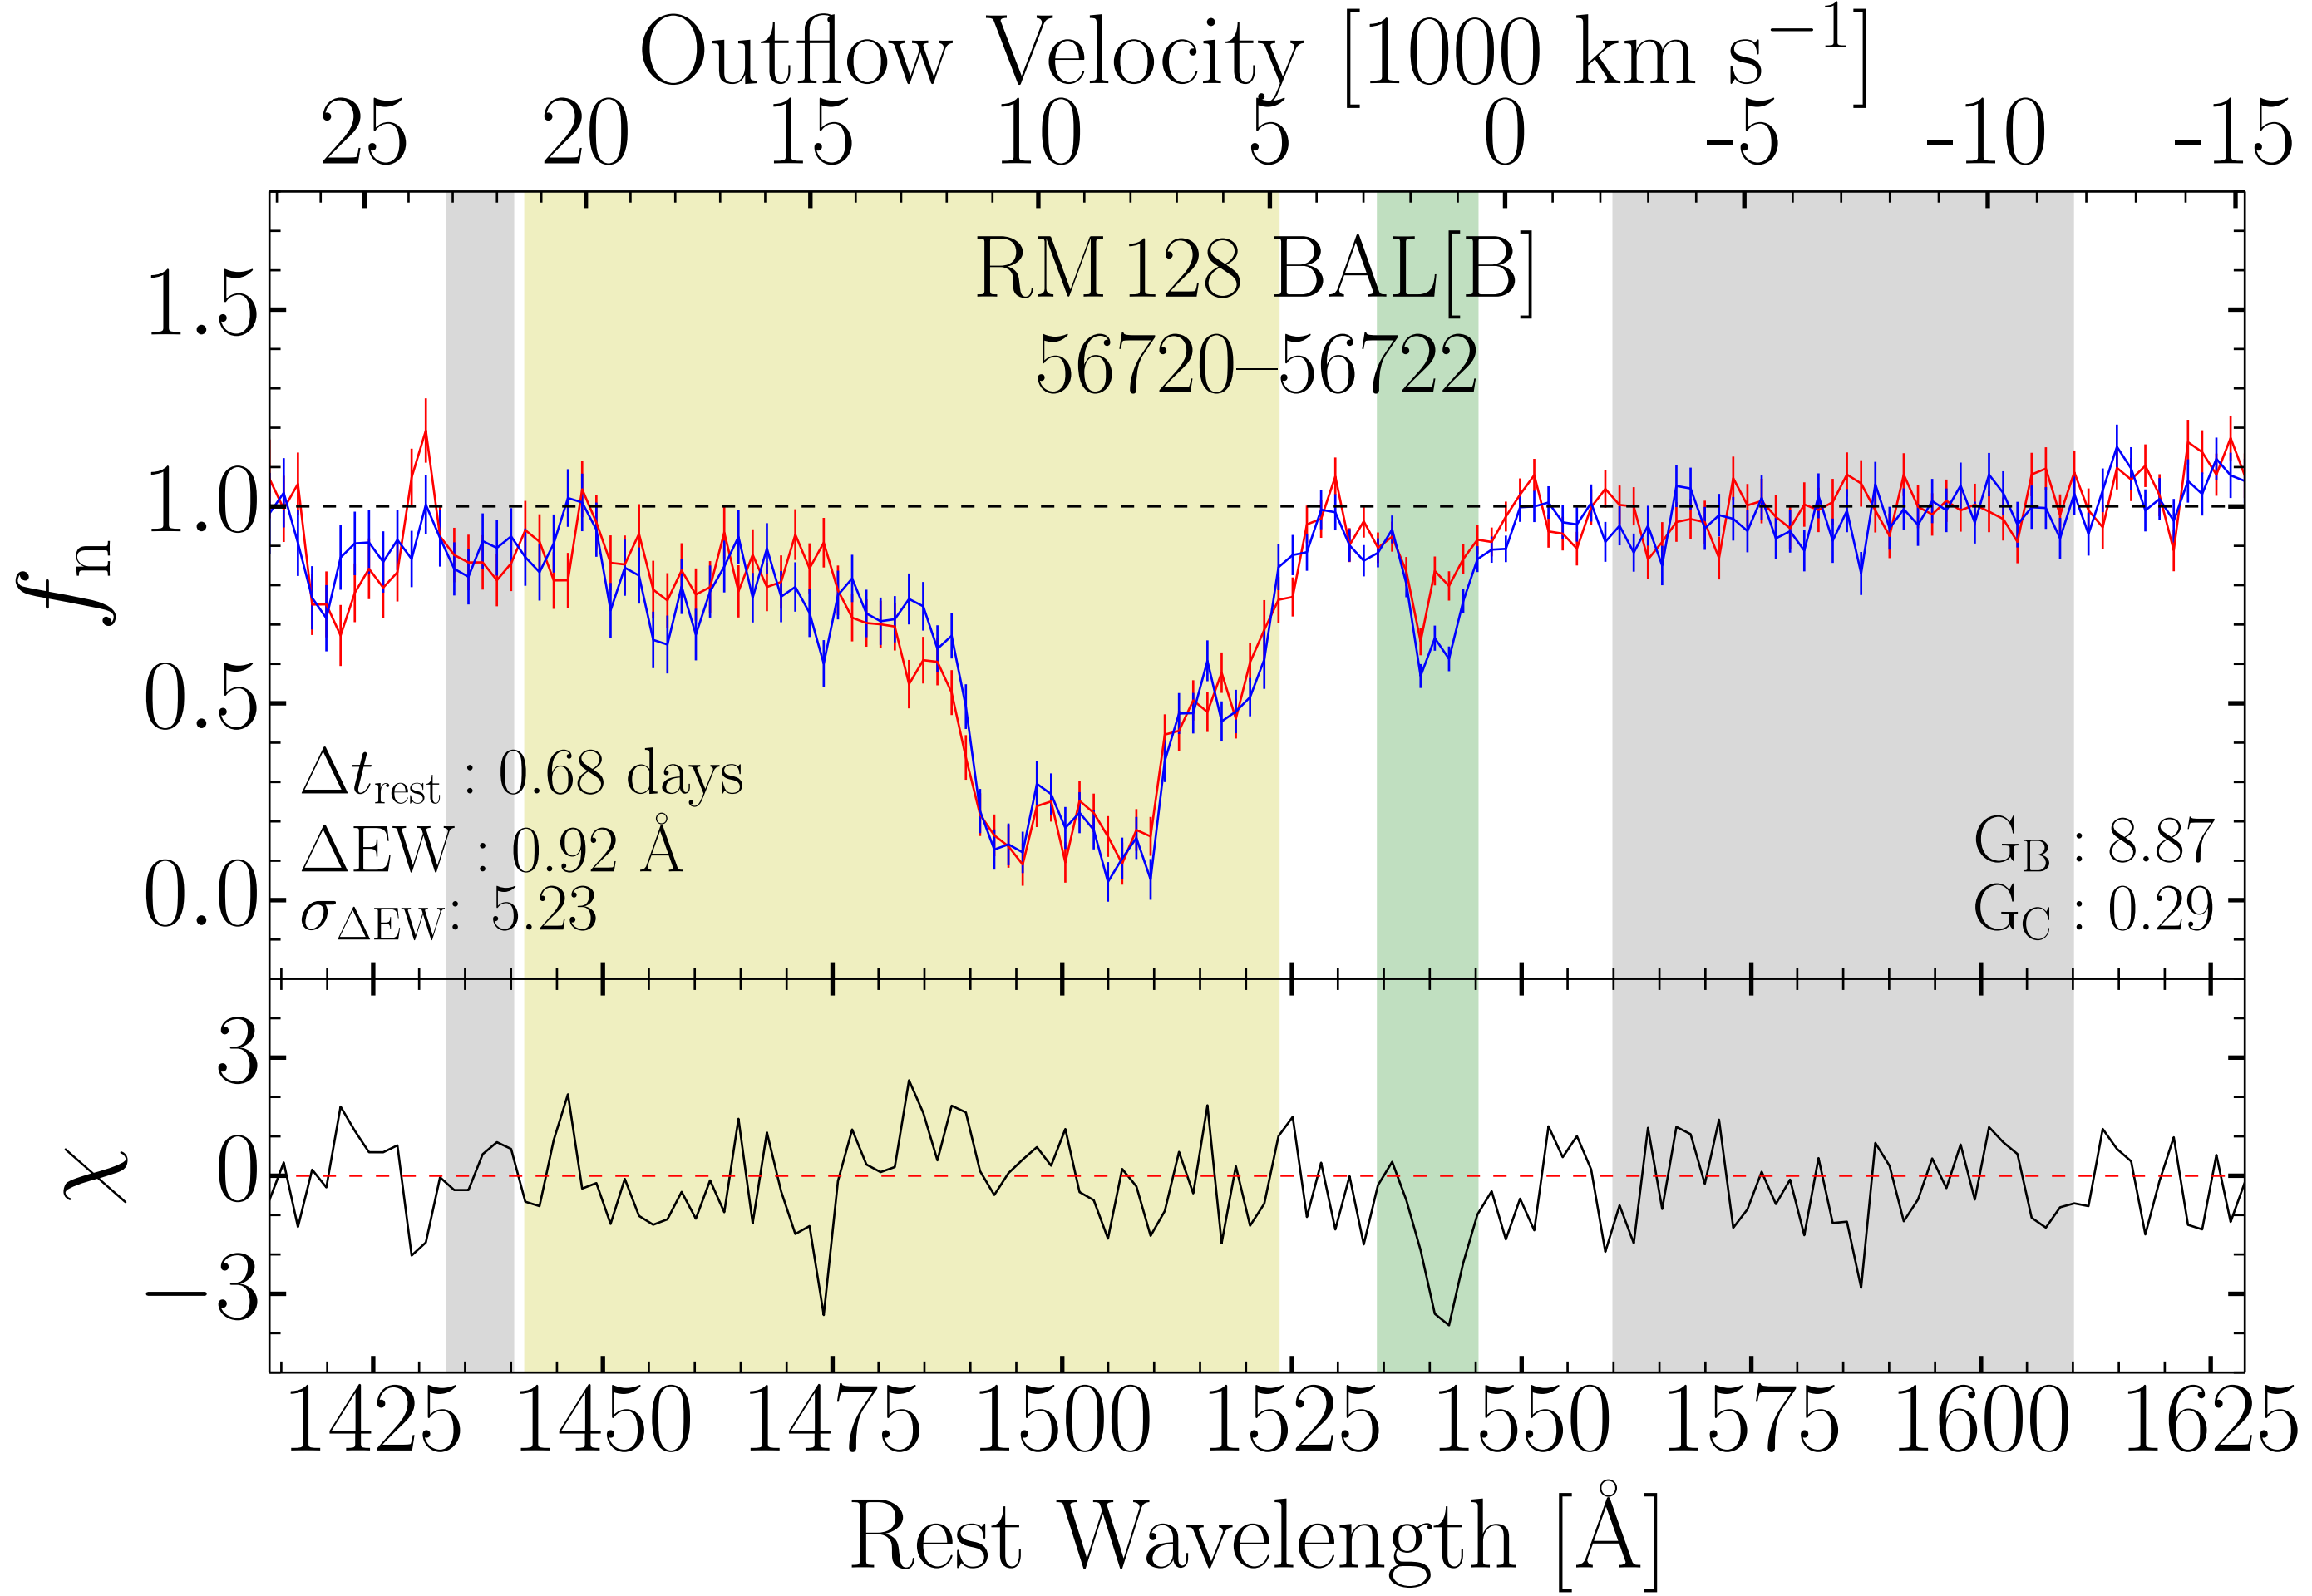

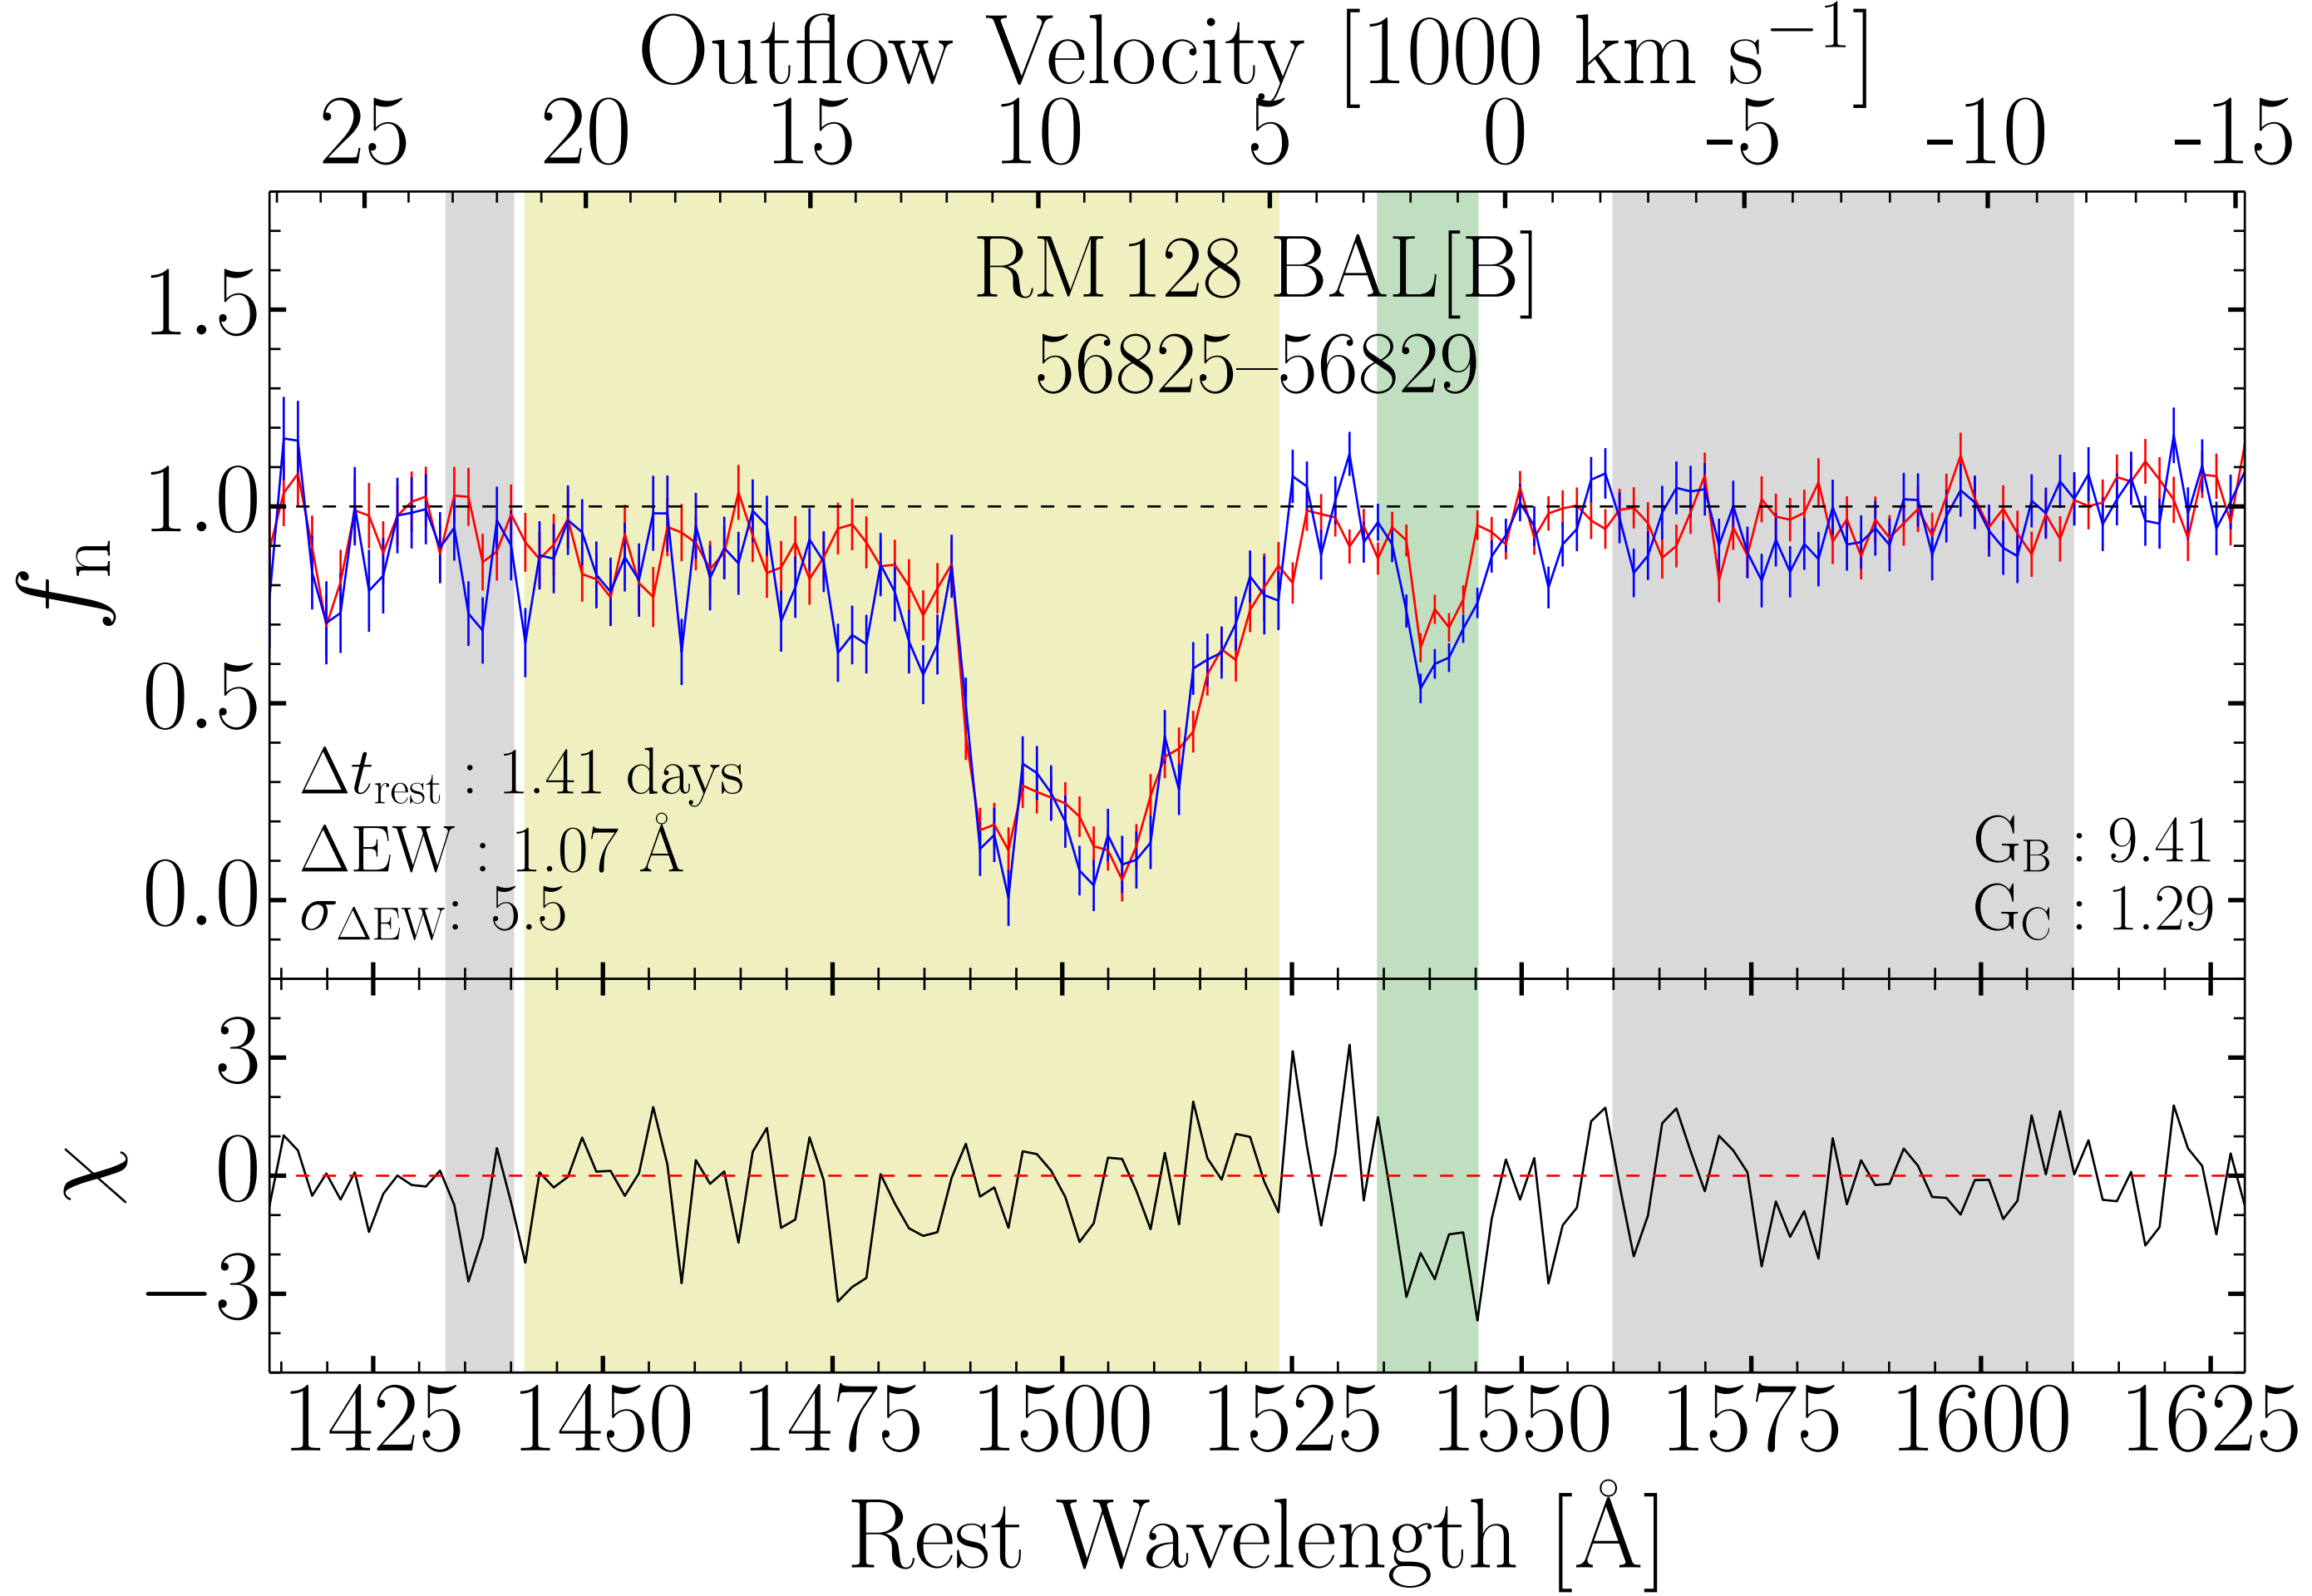

Outflow Velocity [ $1000 \text{ km s}^{-1}$ ]

25

20

15

10

5

0

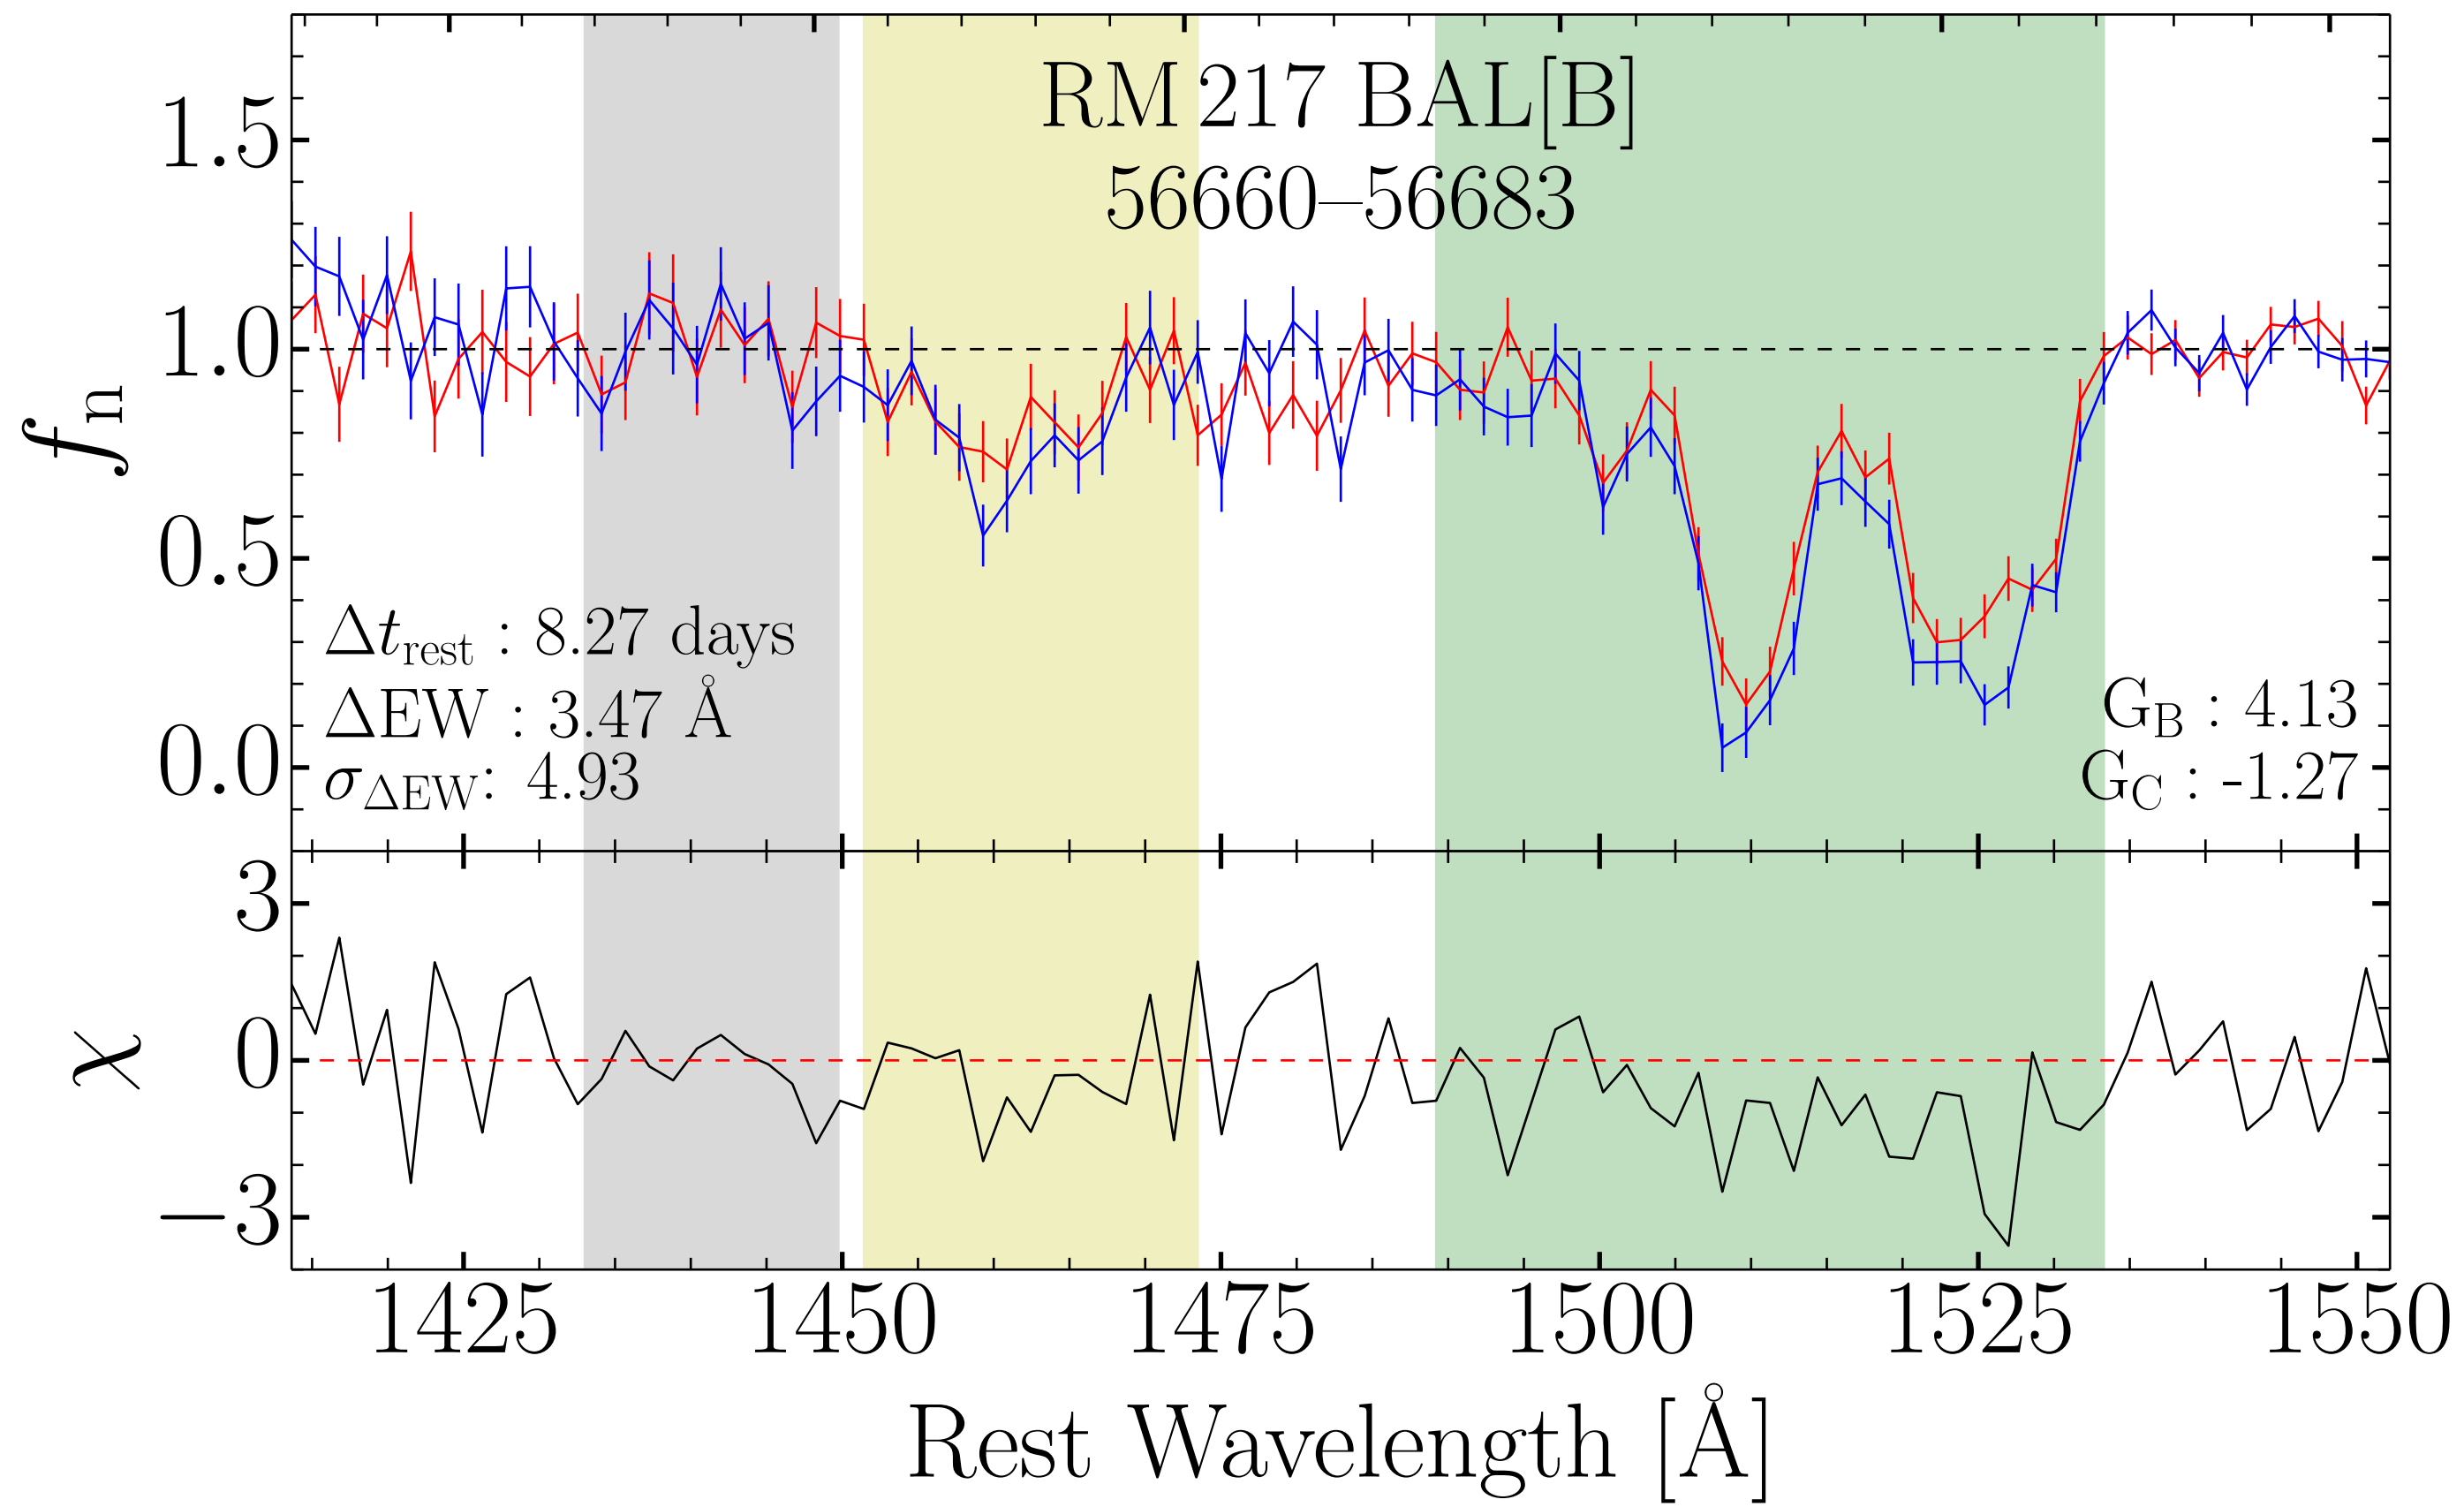

Outflow Velocity [1000 km s<sup>-1</sup>]

25

20

15

10

5

0

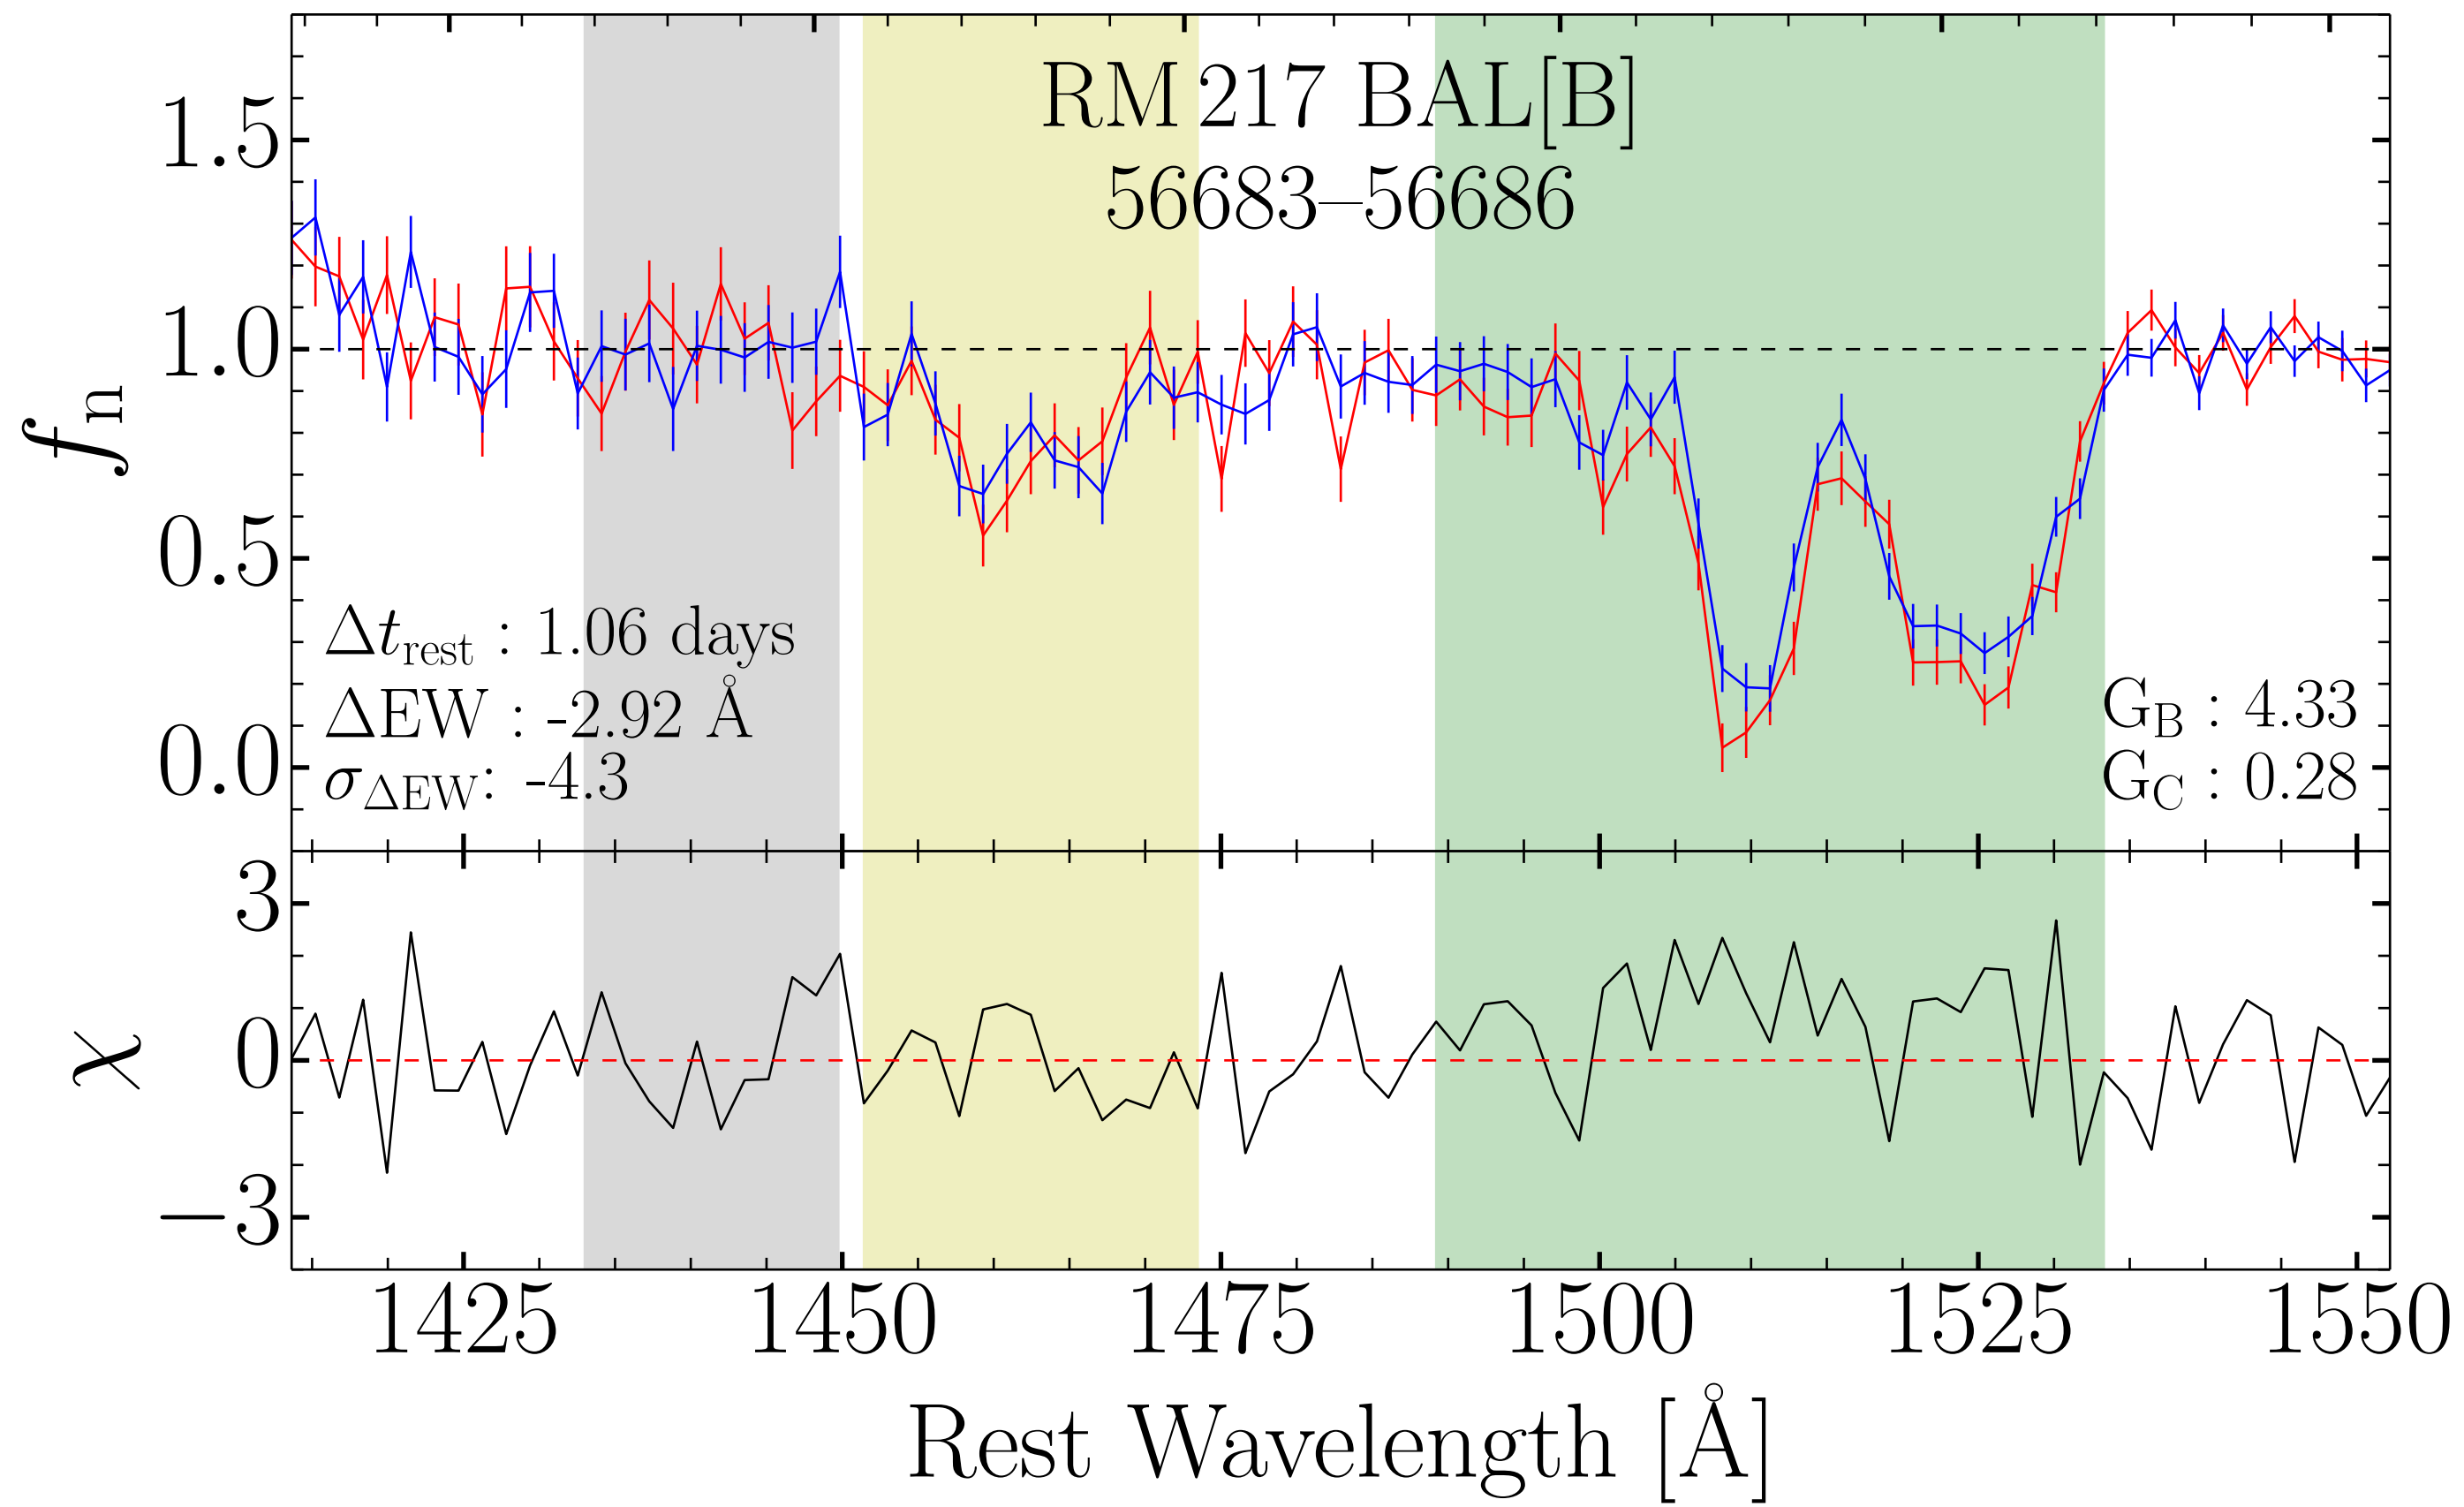

Outflow Velocity [1000 km s<sup>-1</sup>]

25

20

15

10

5

0

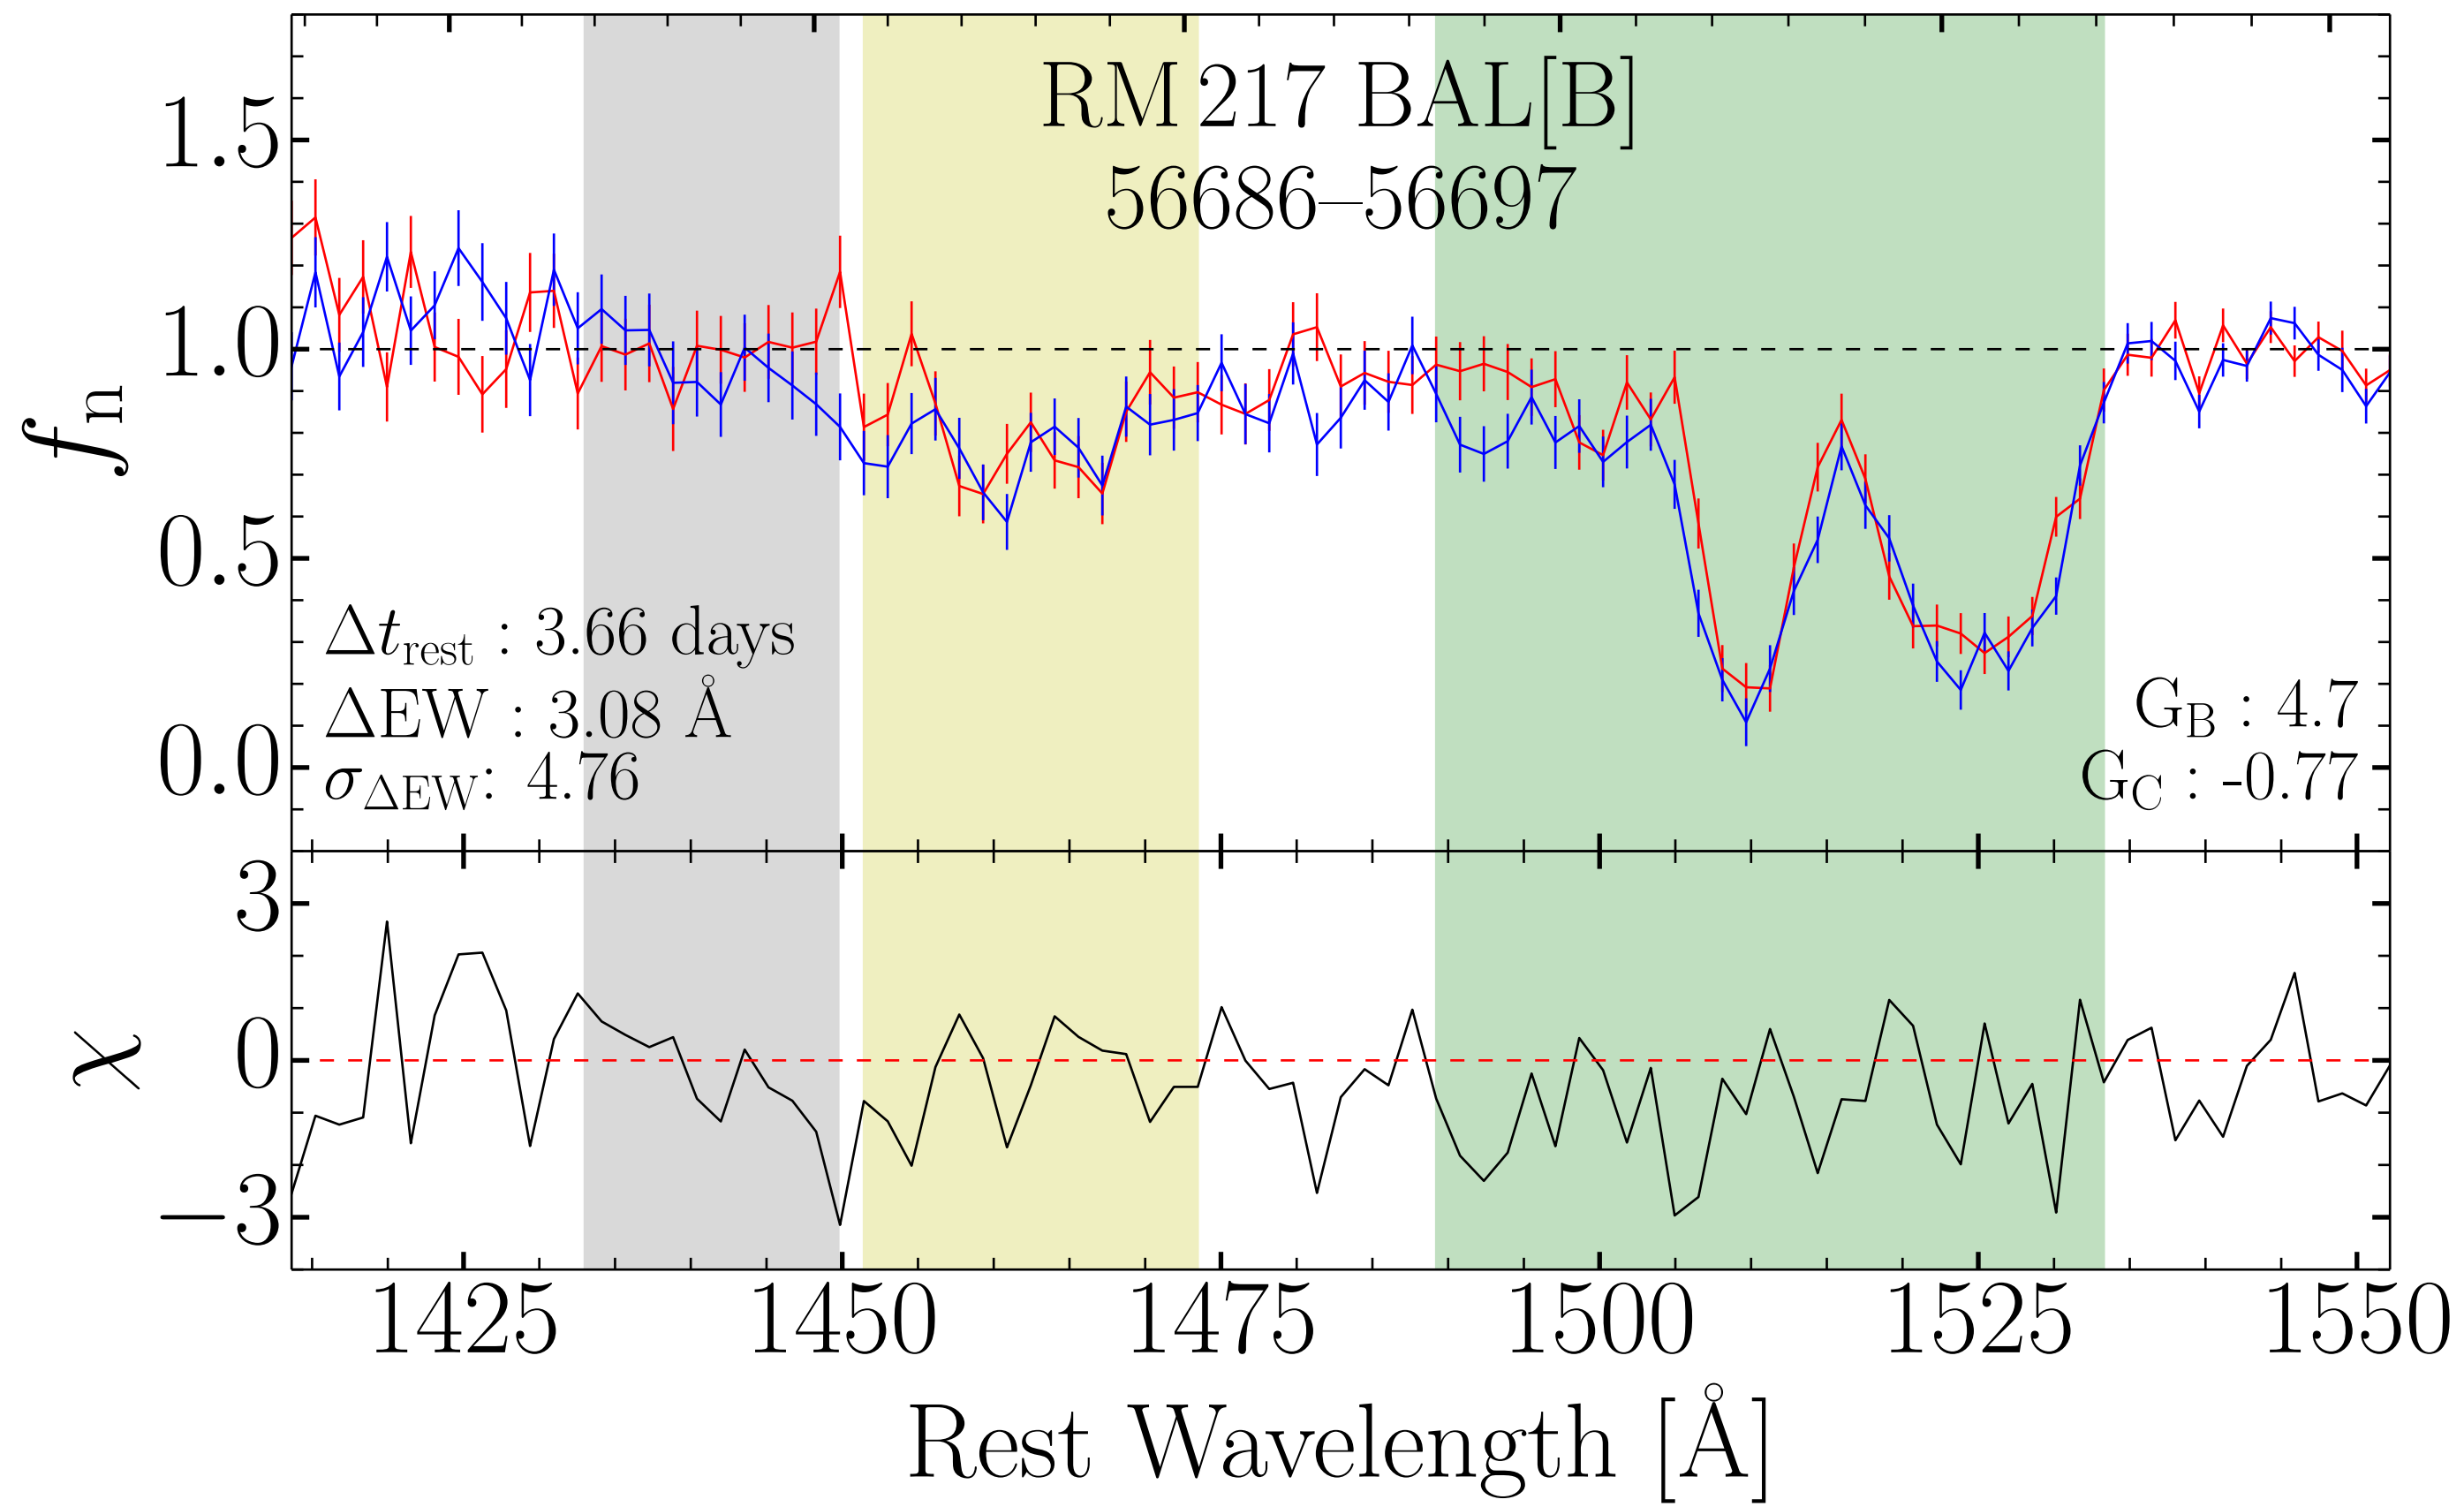

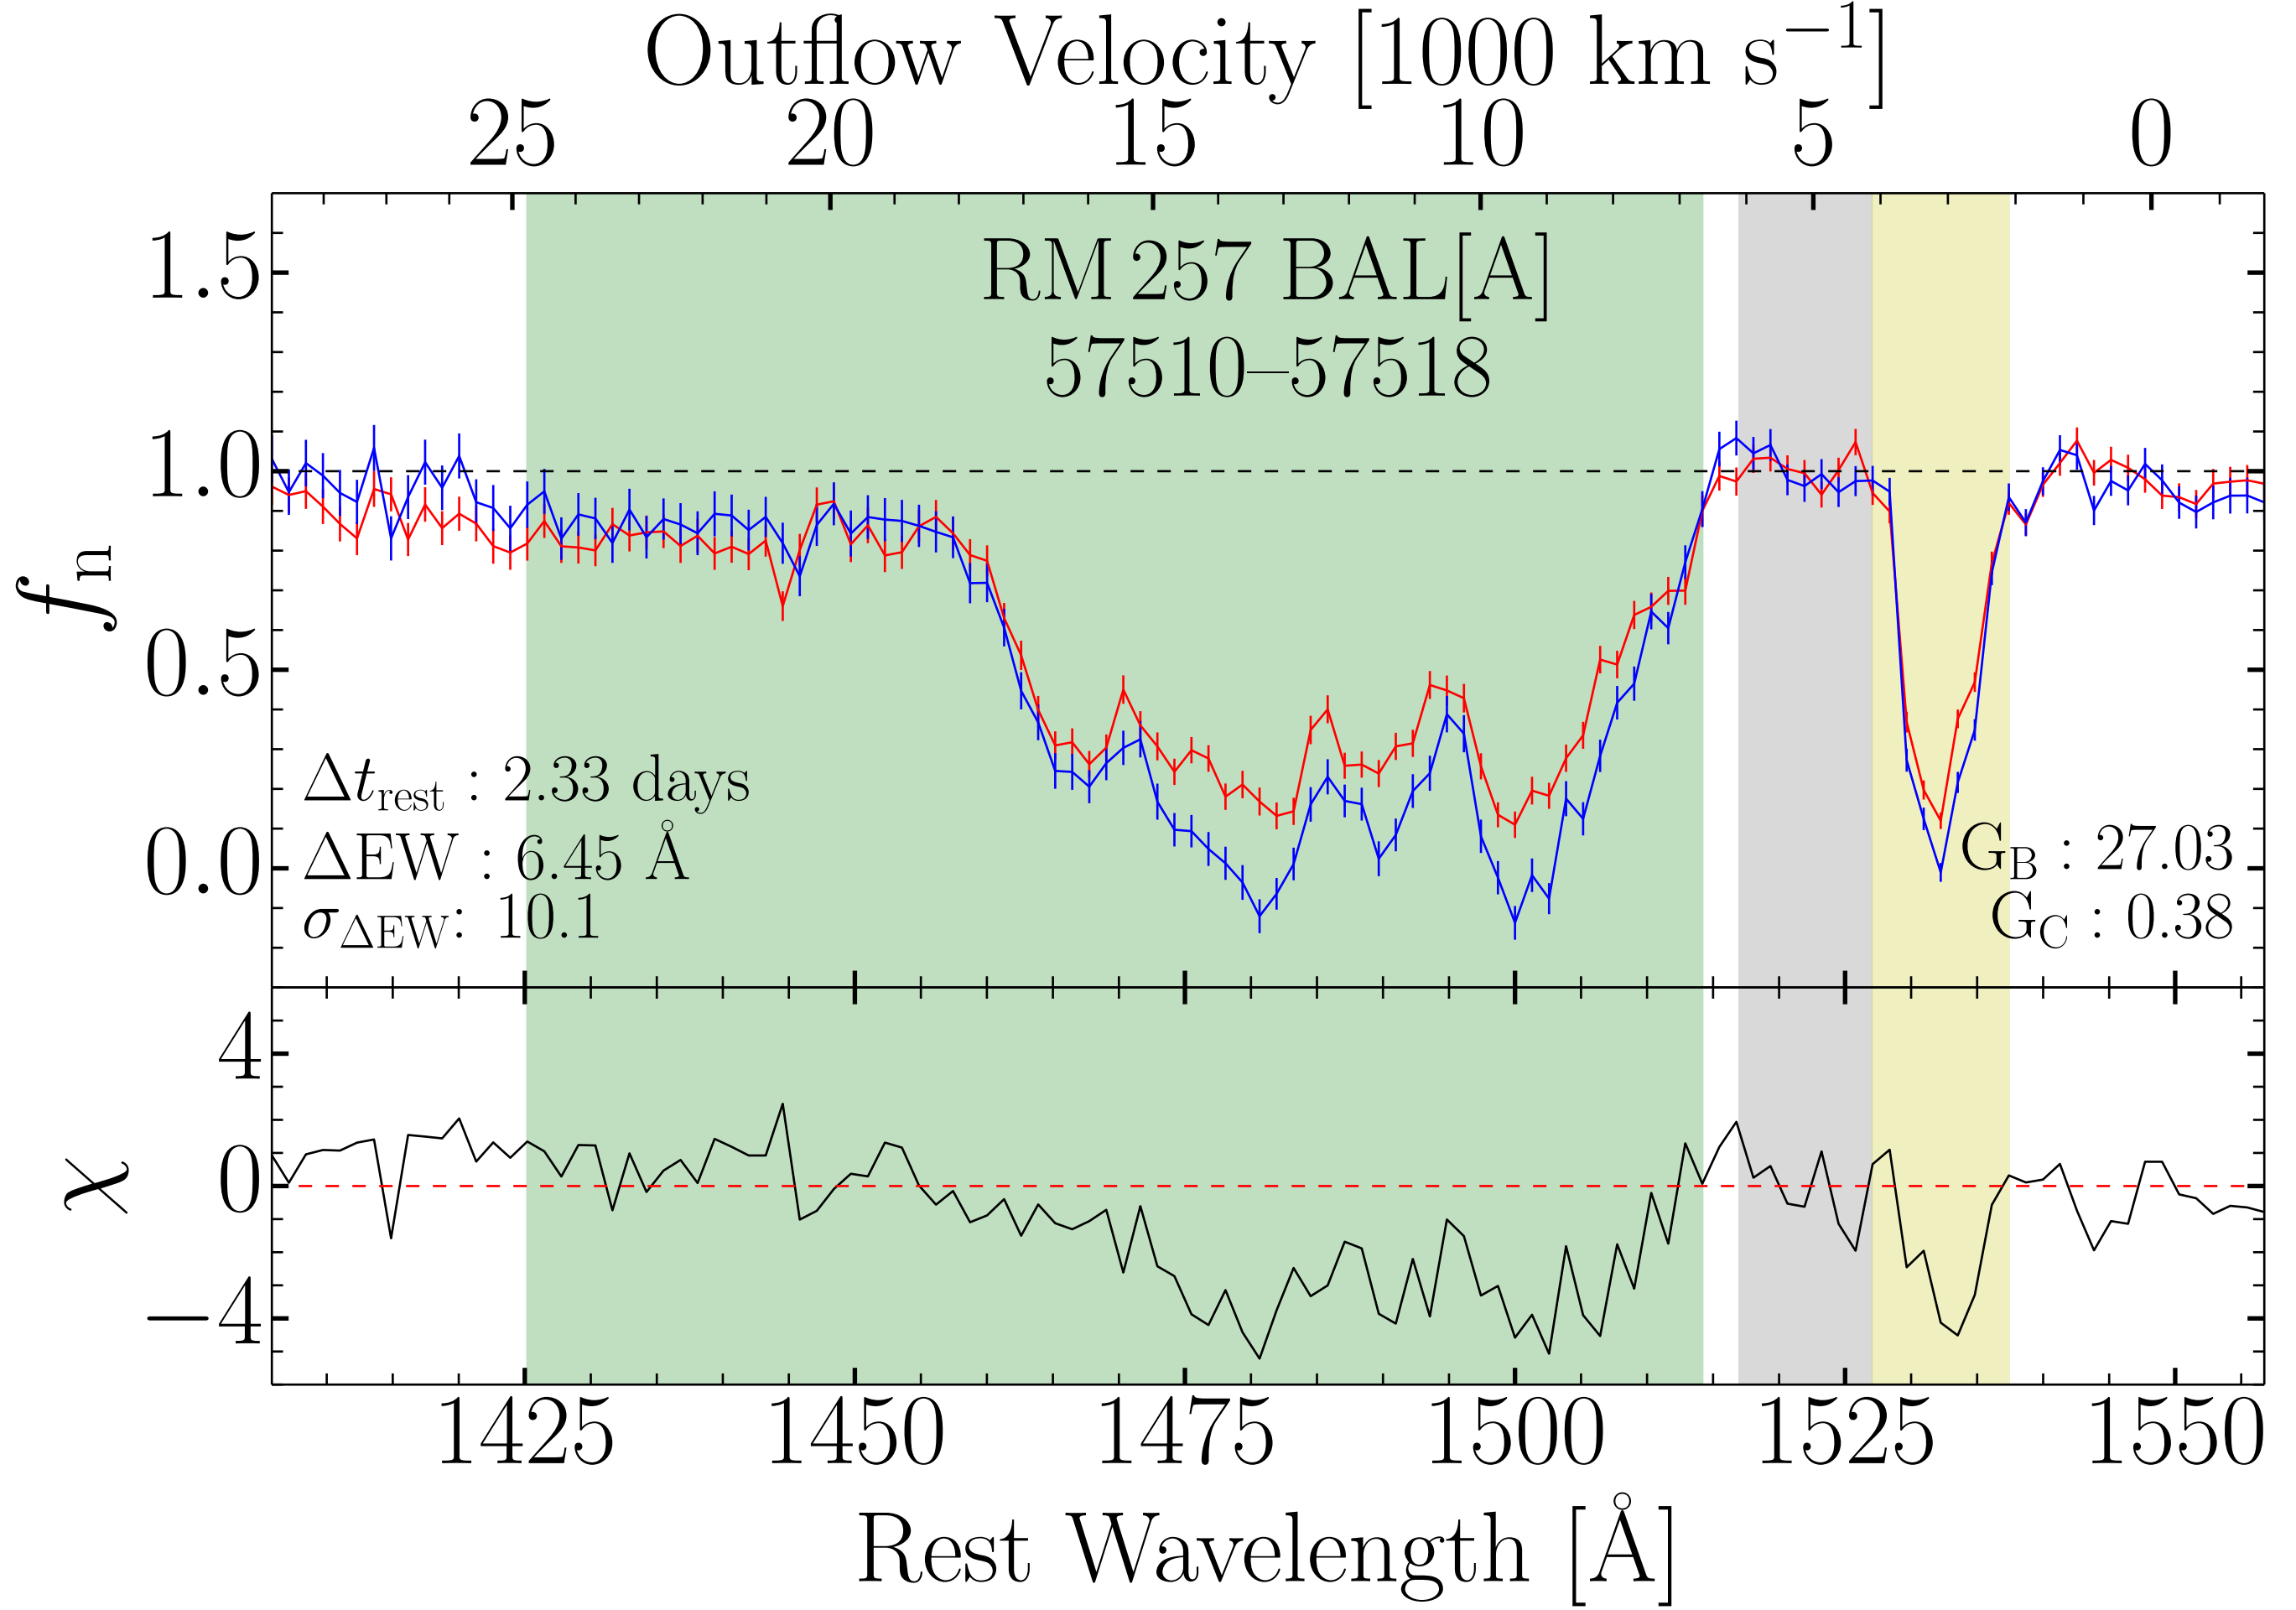



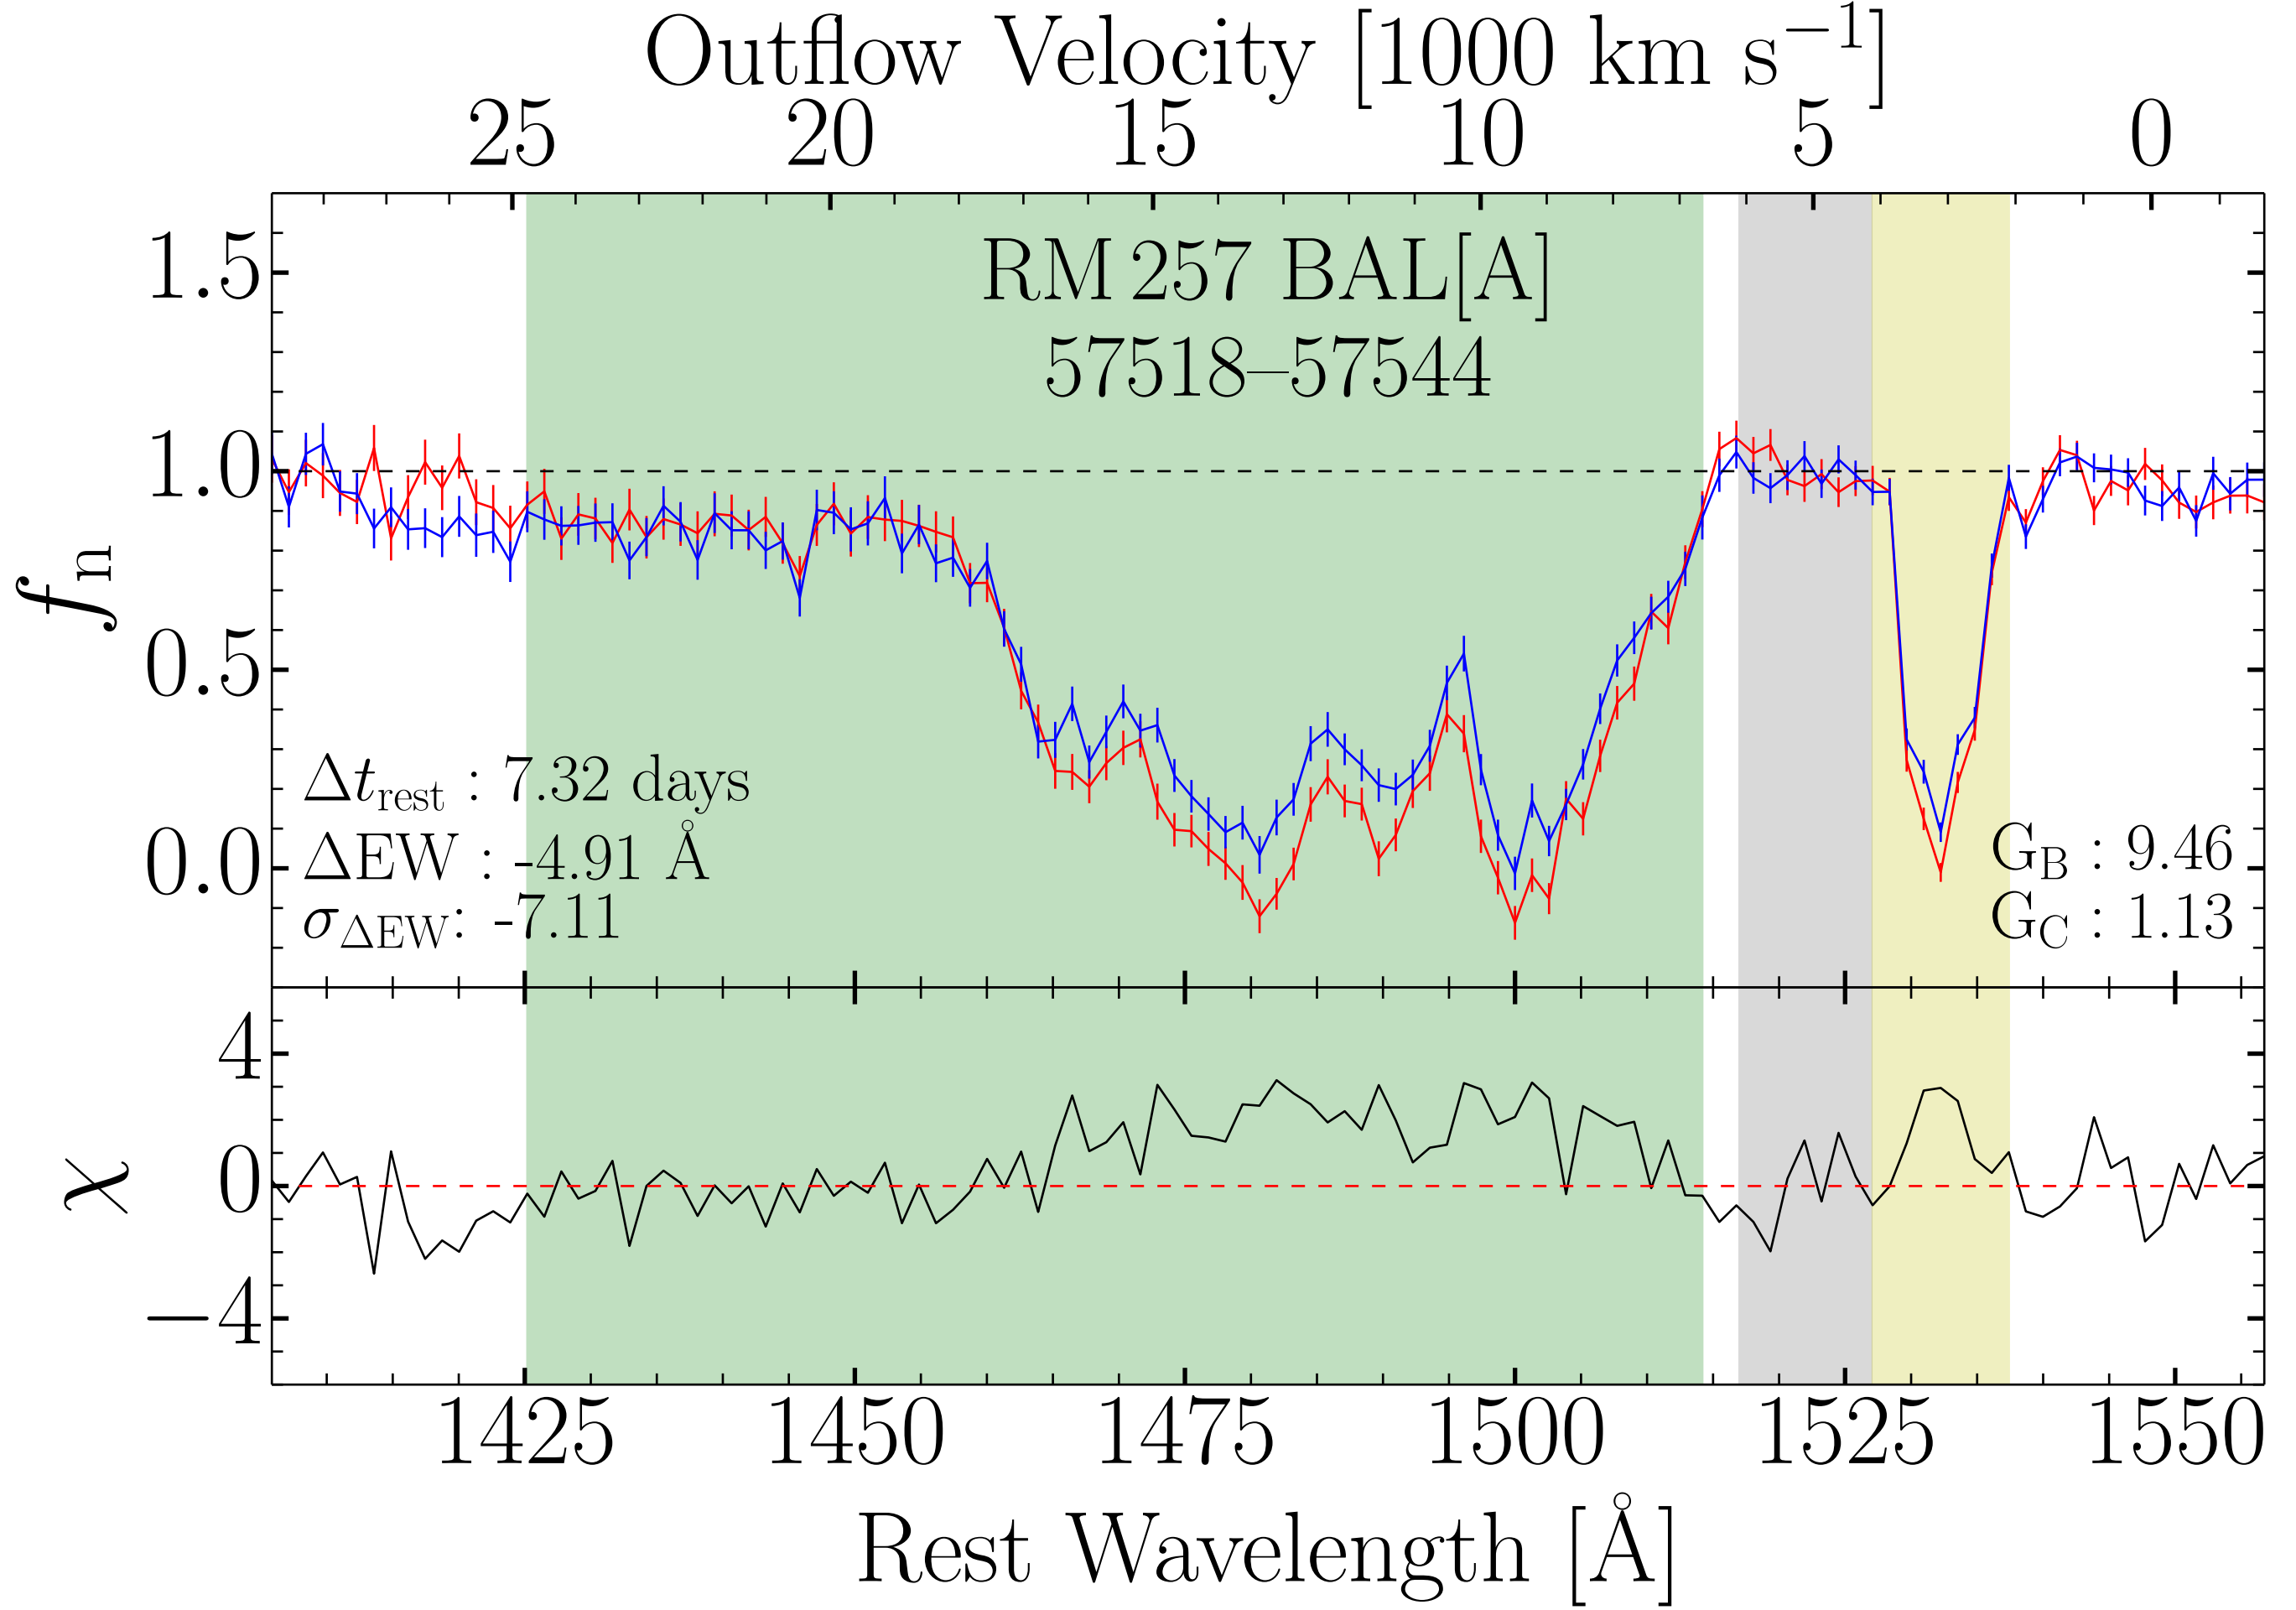

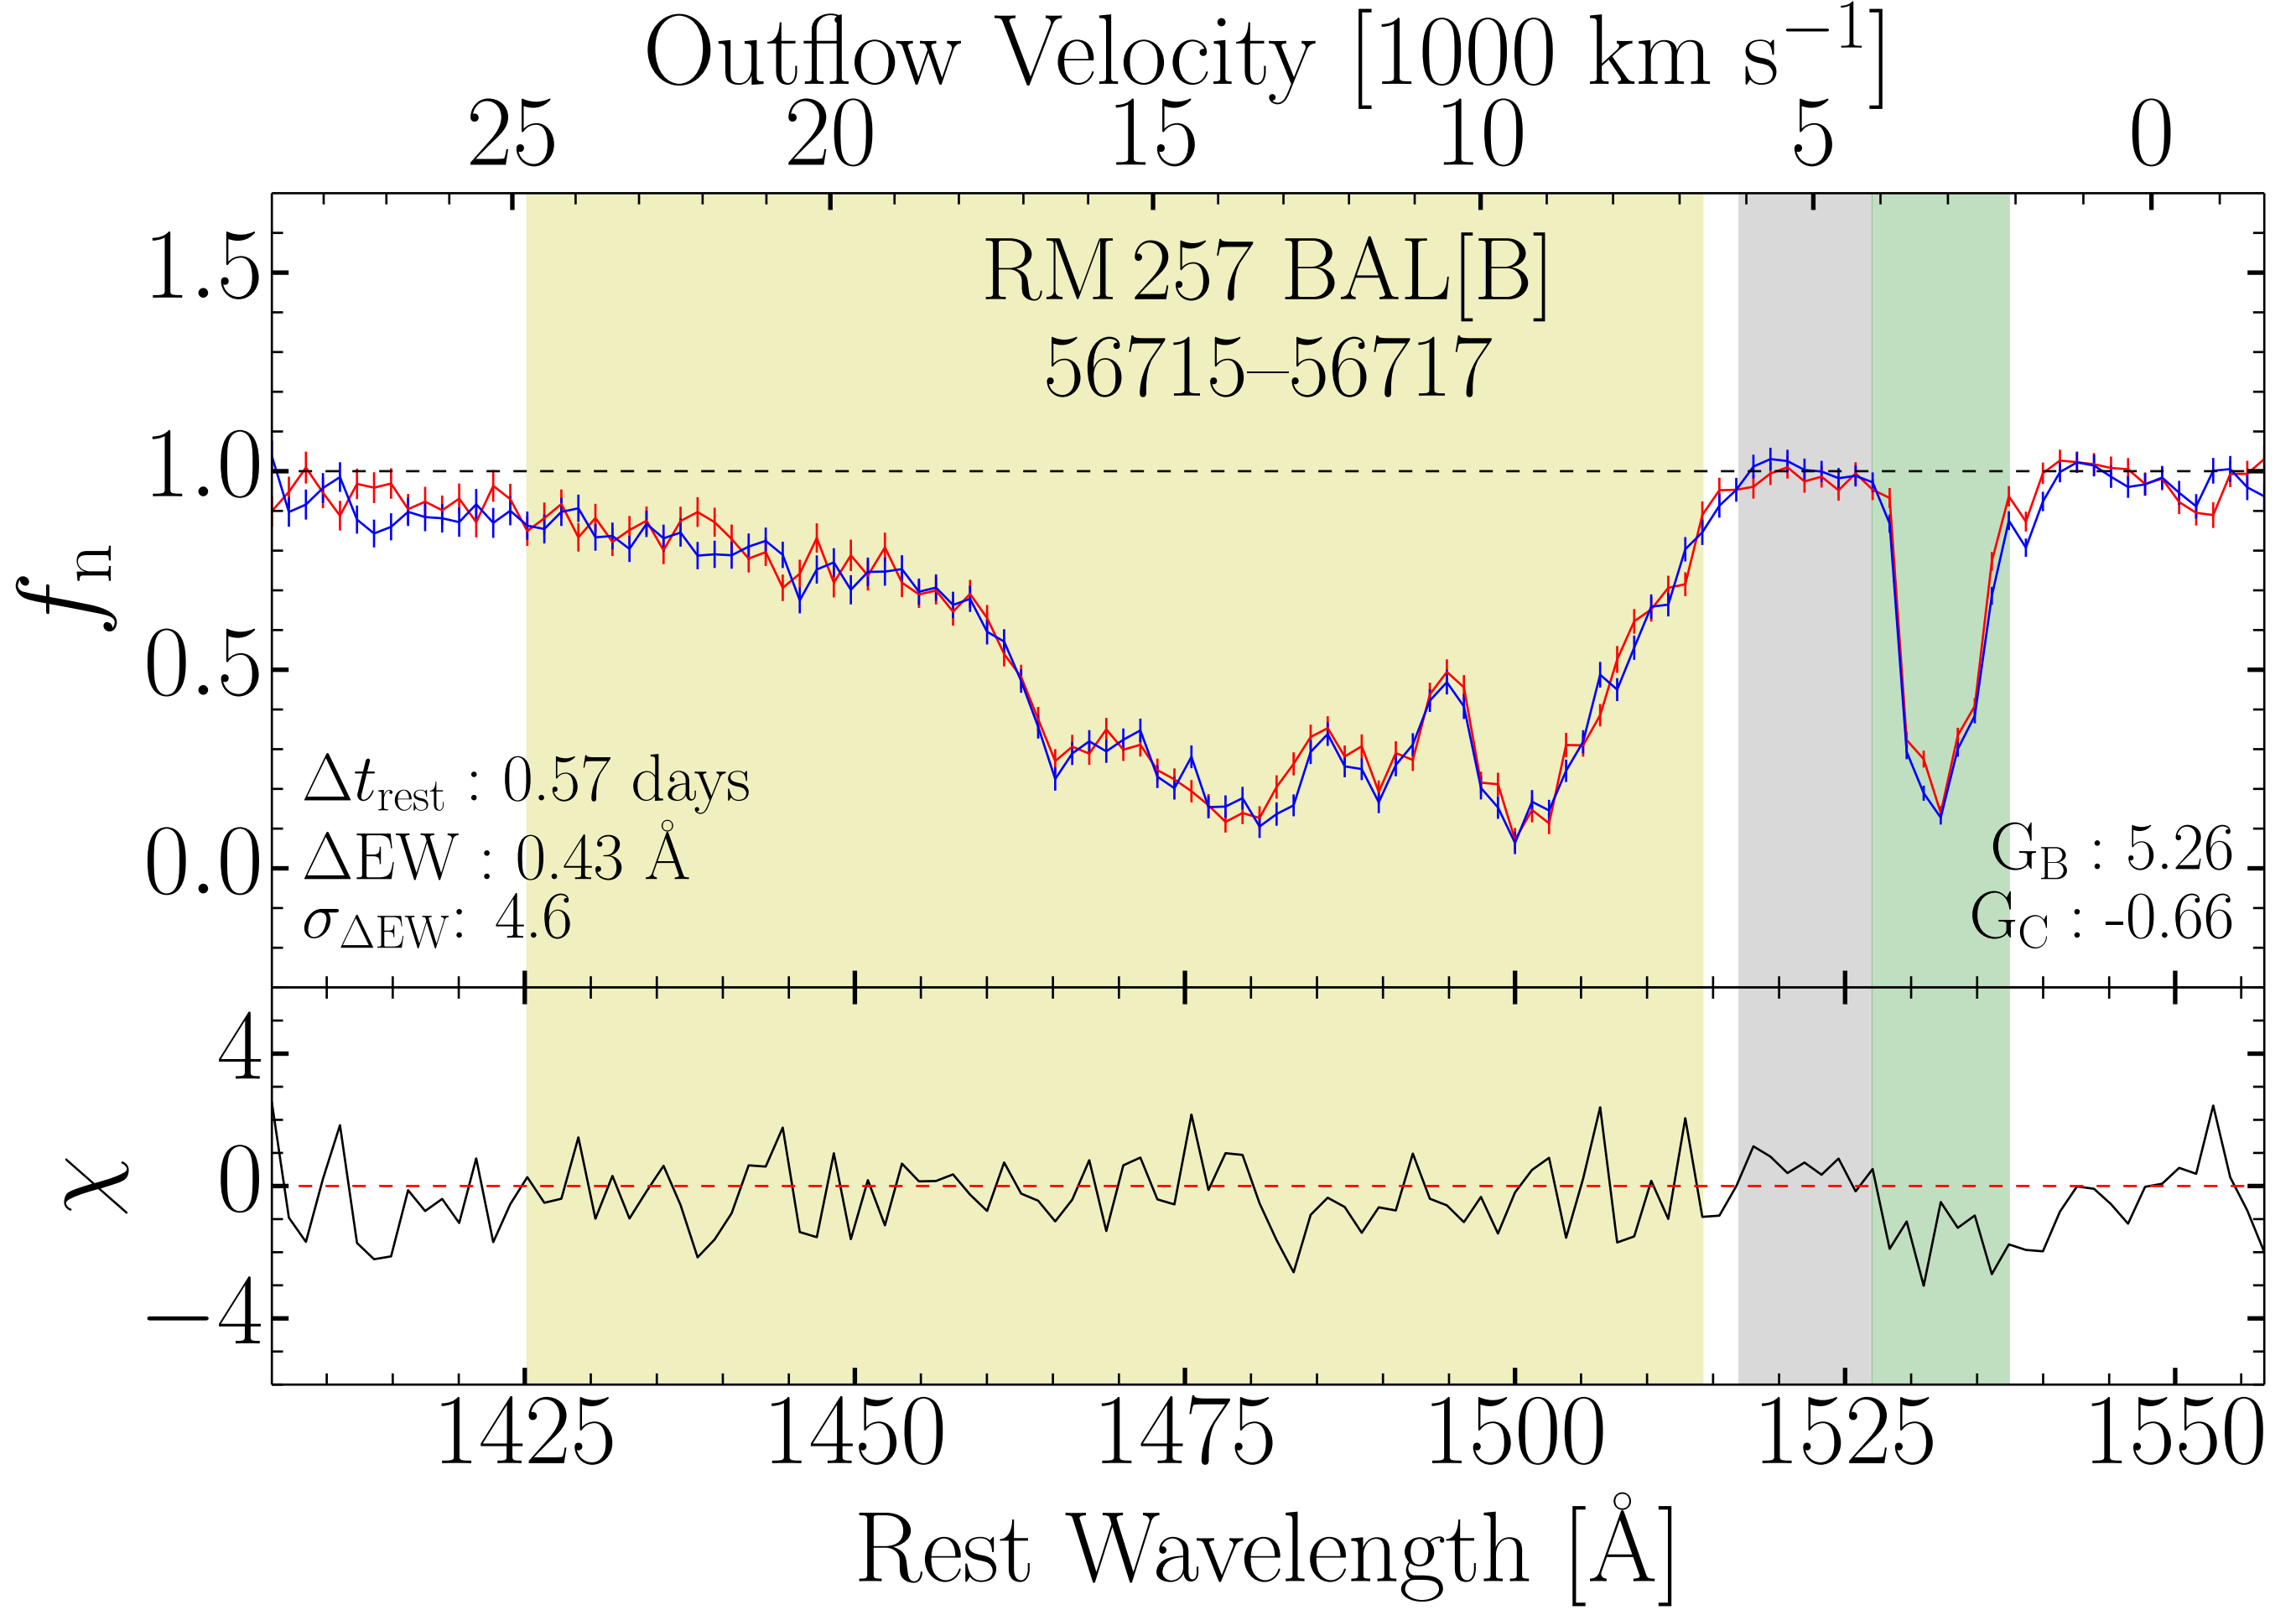

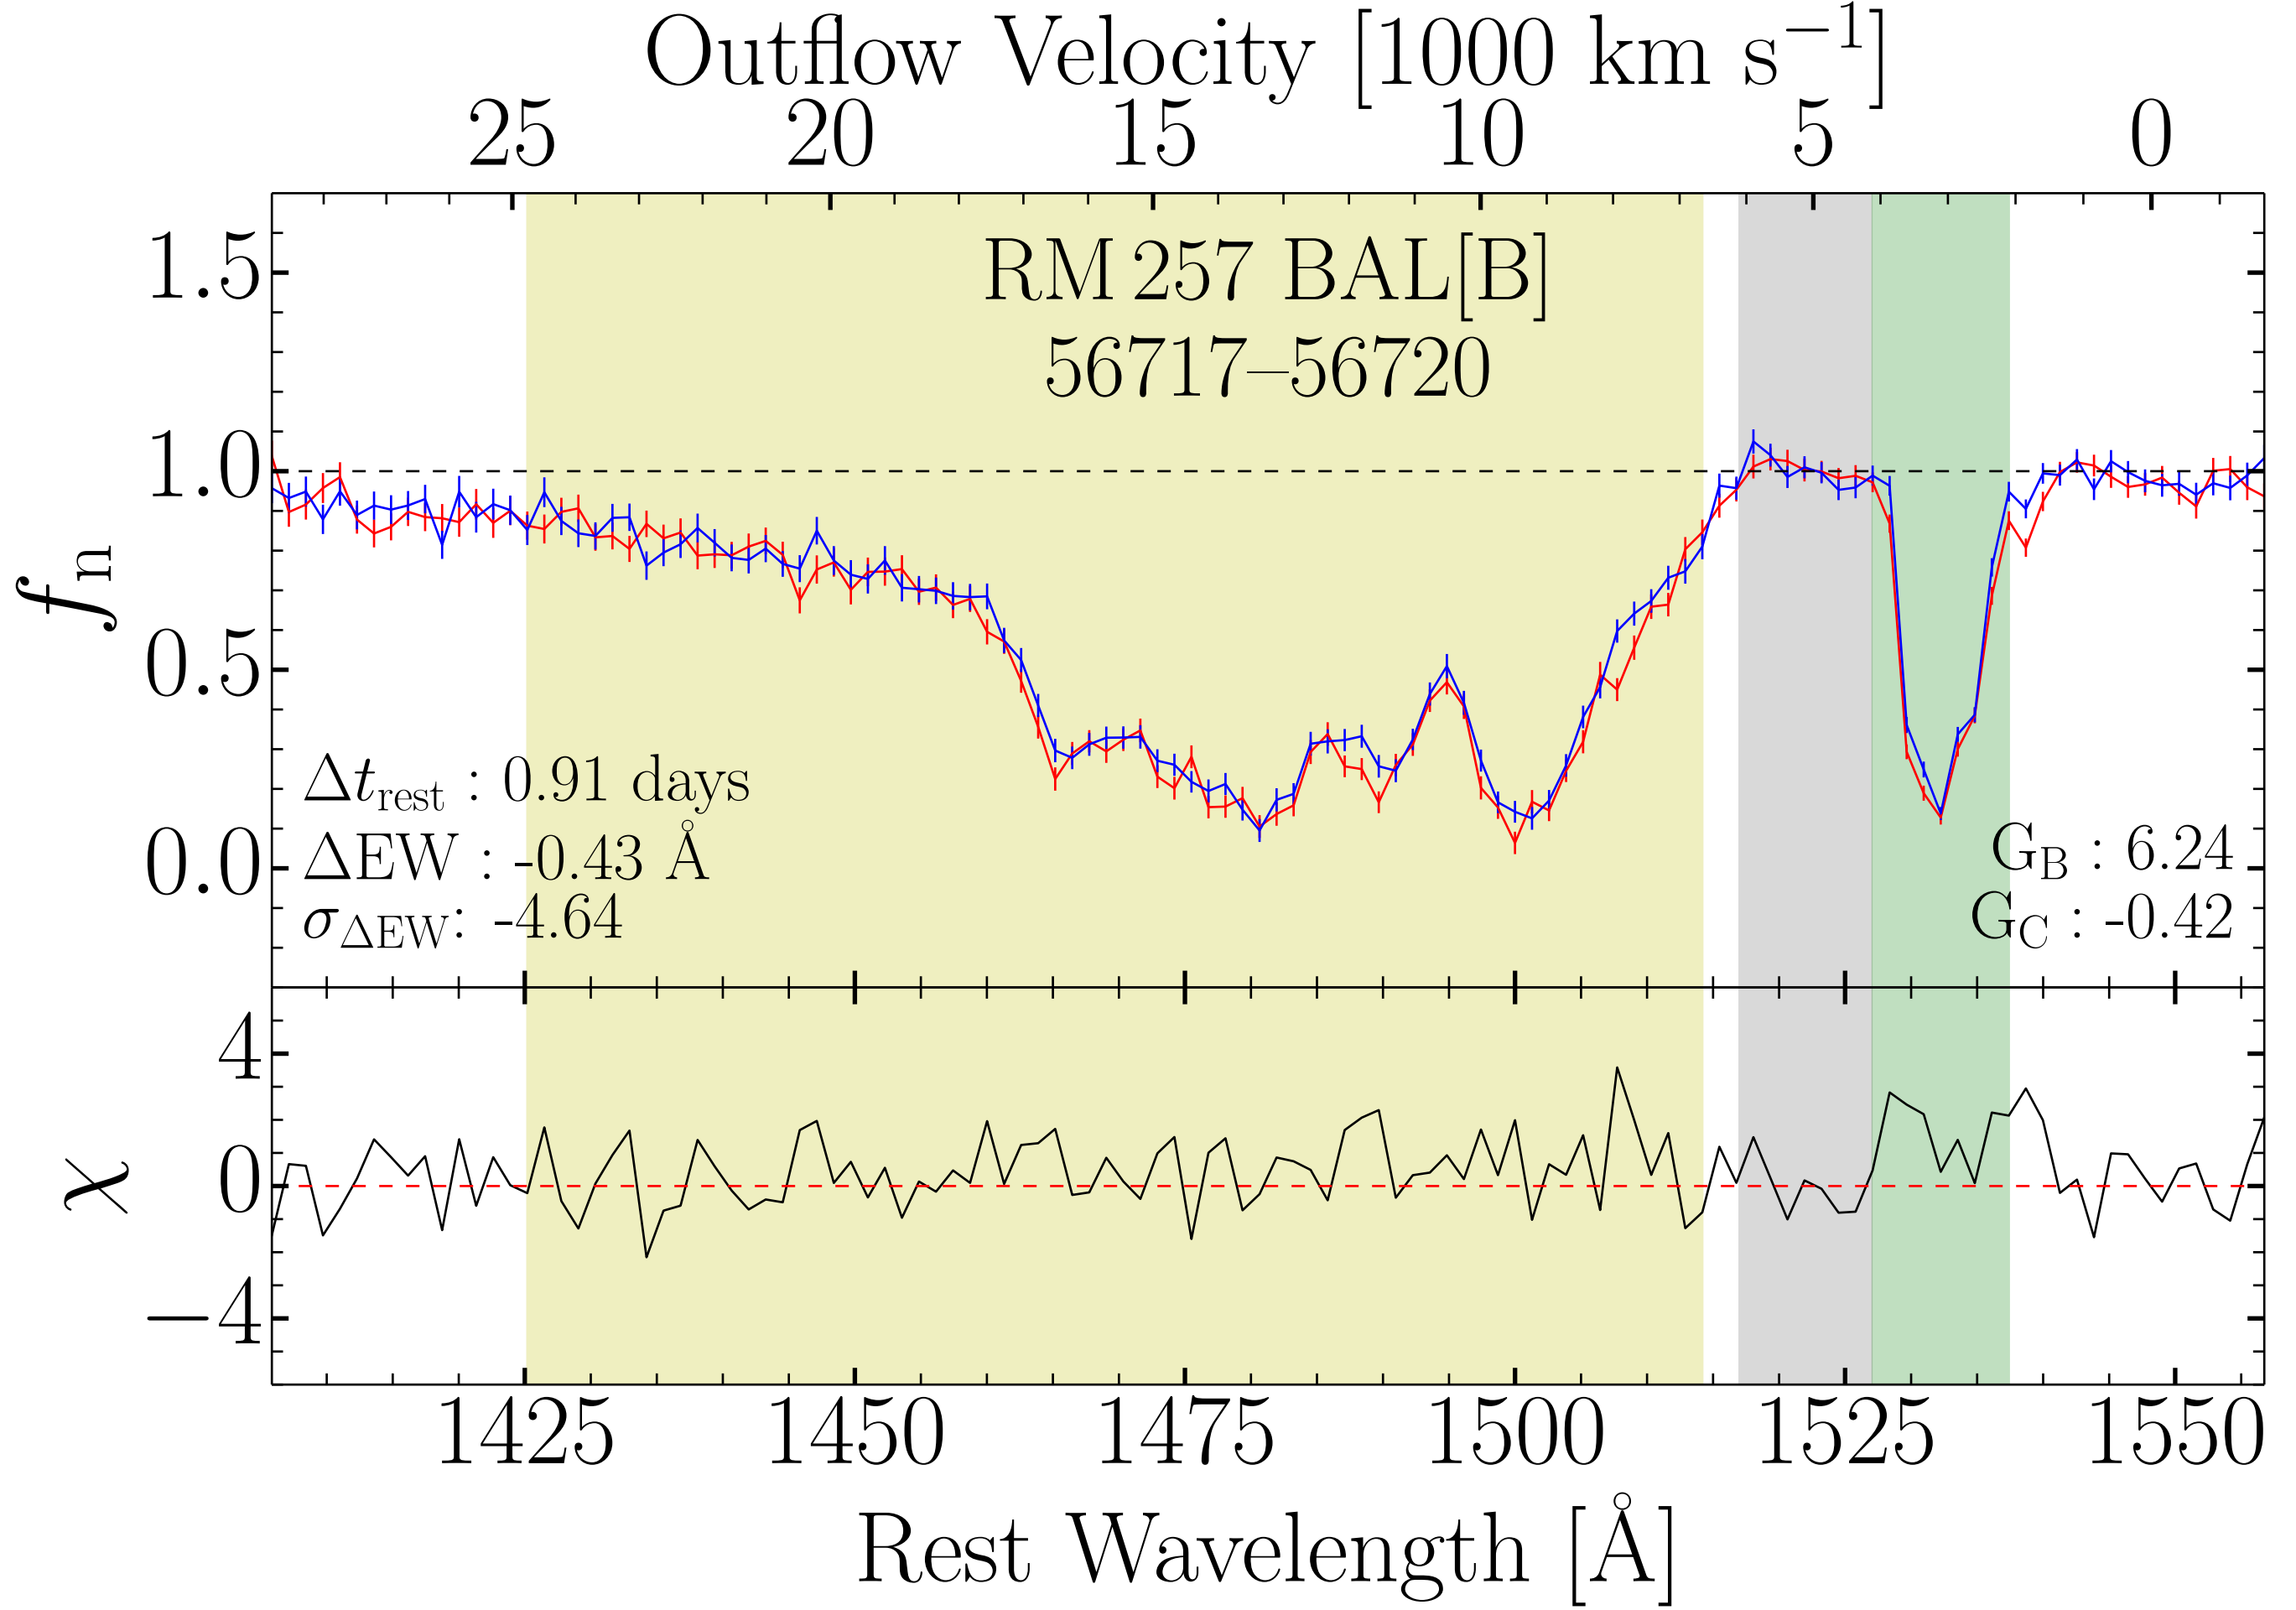

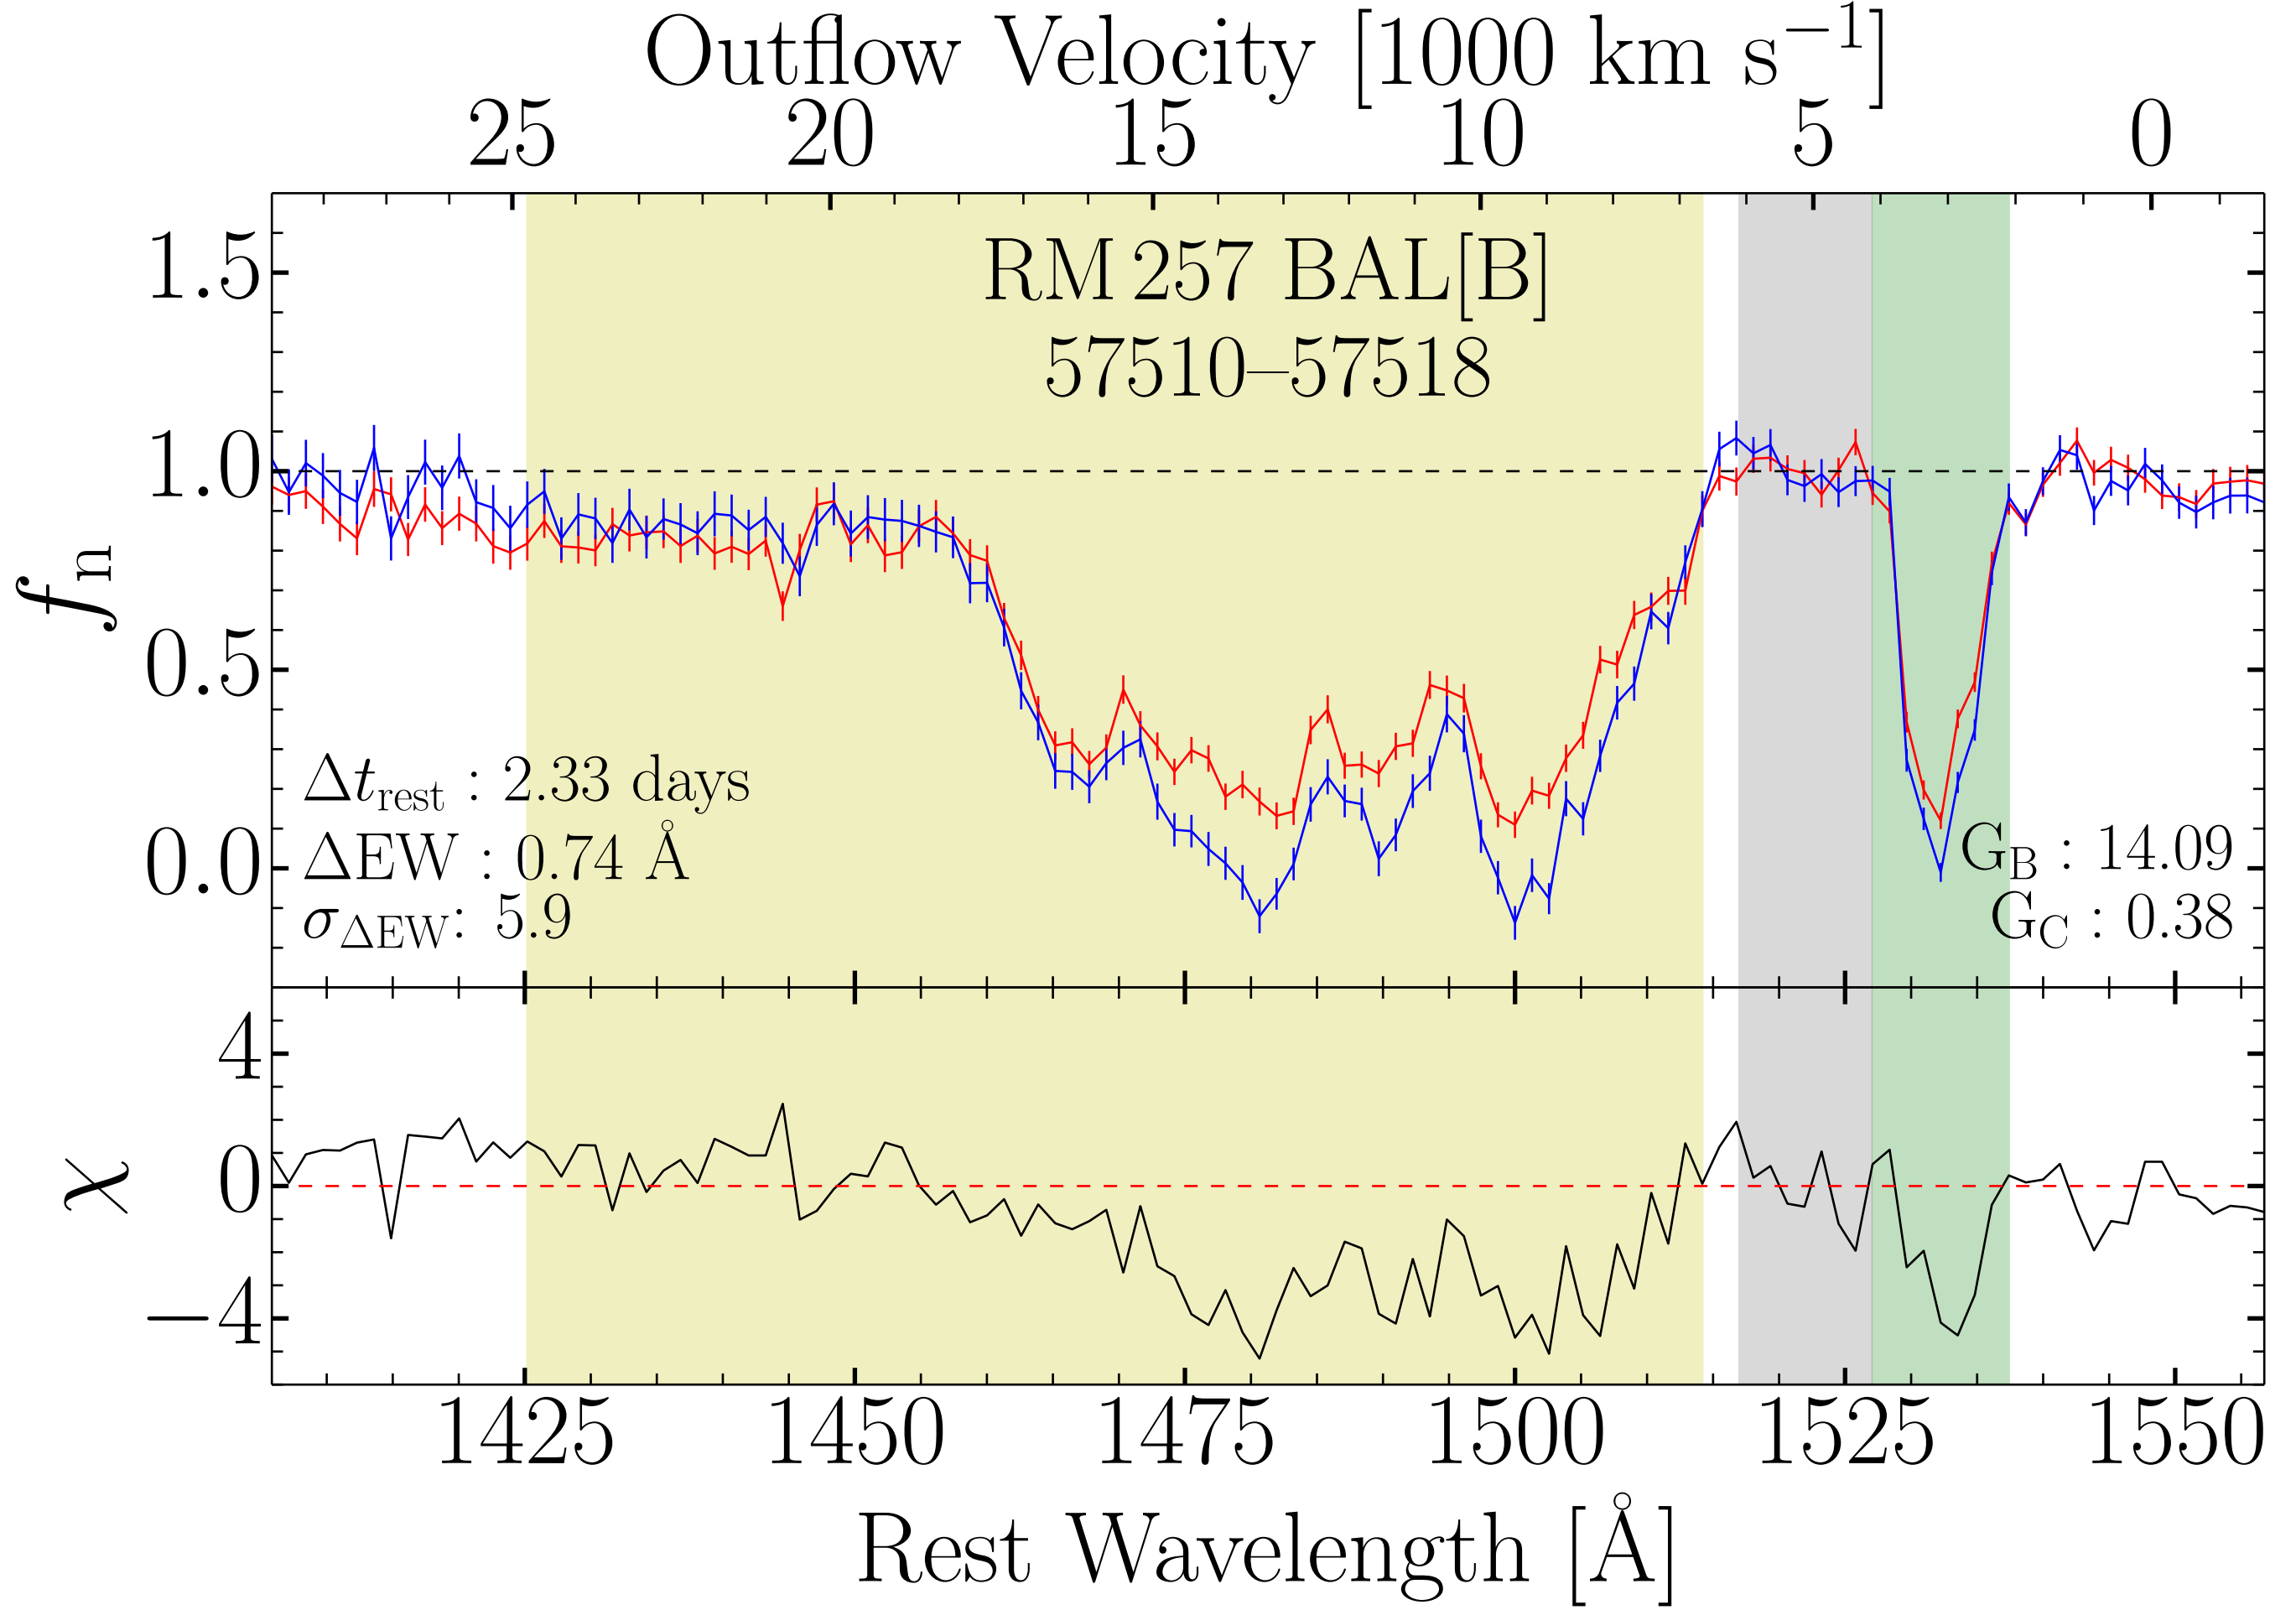

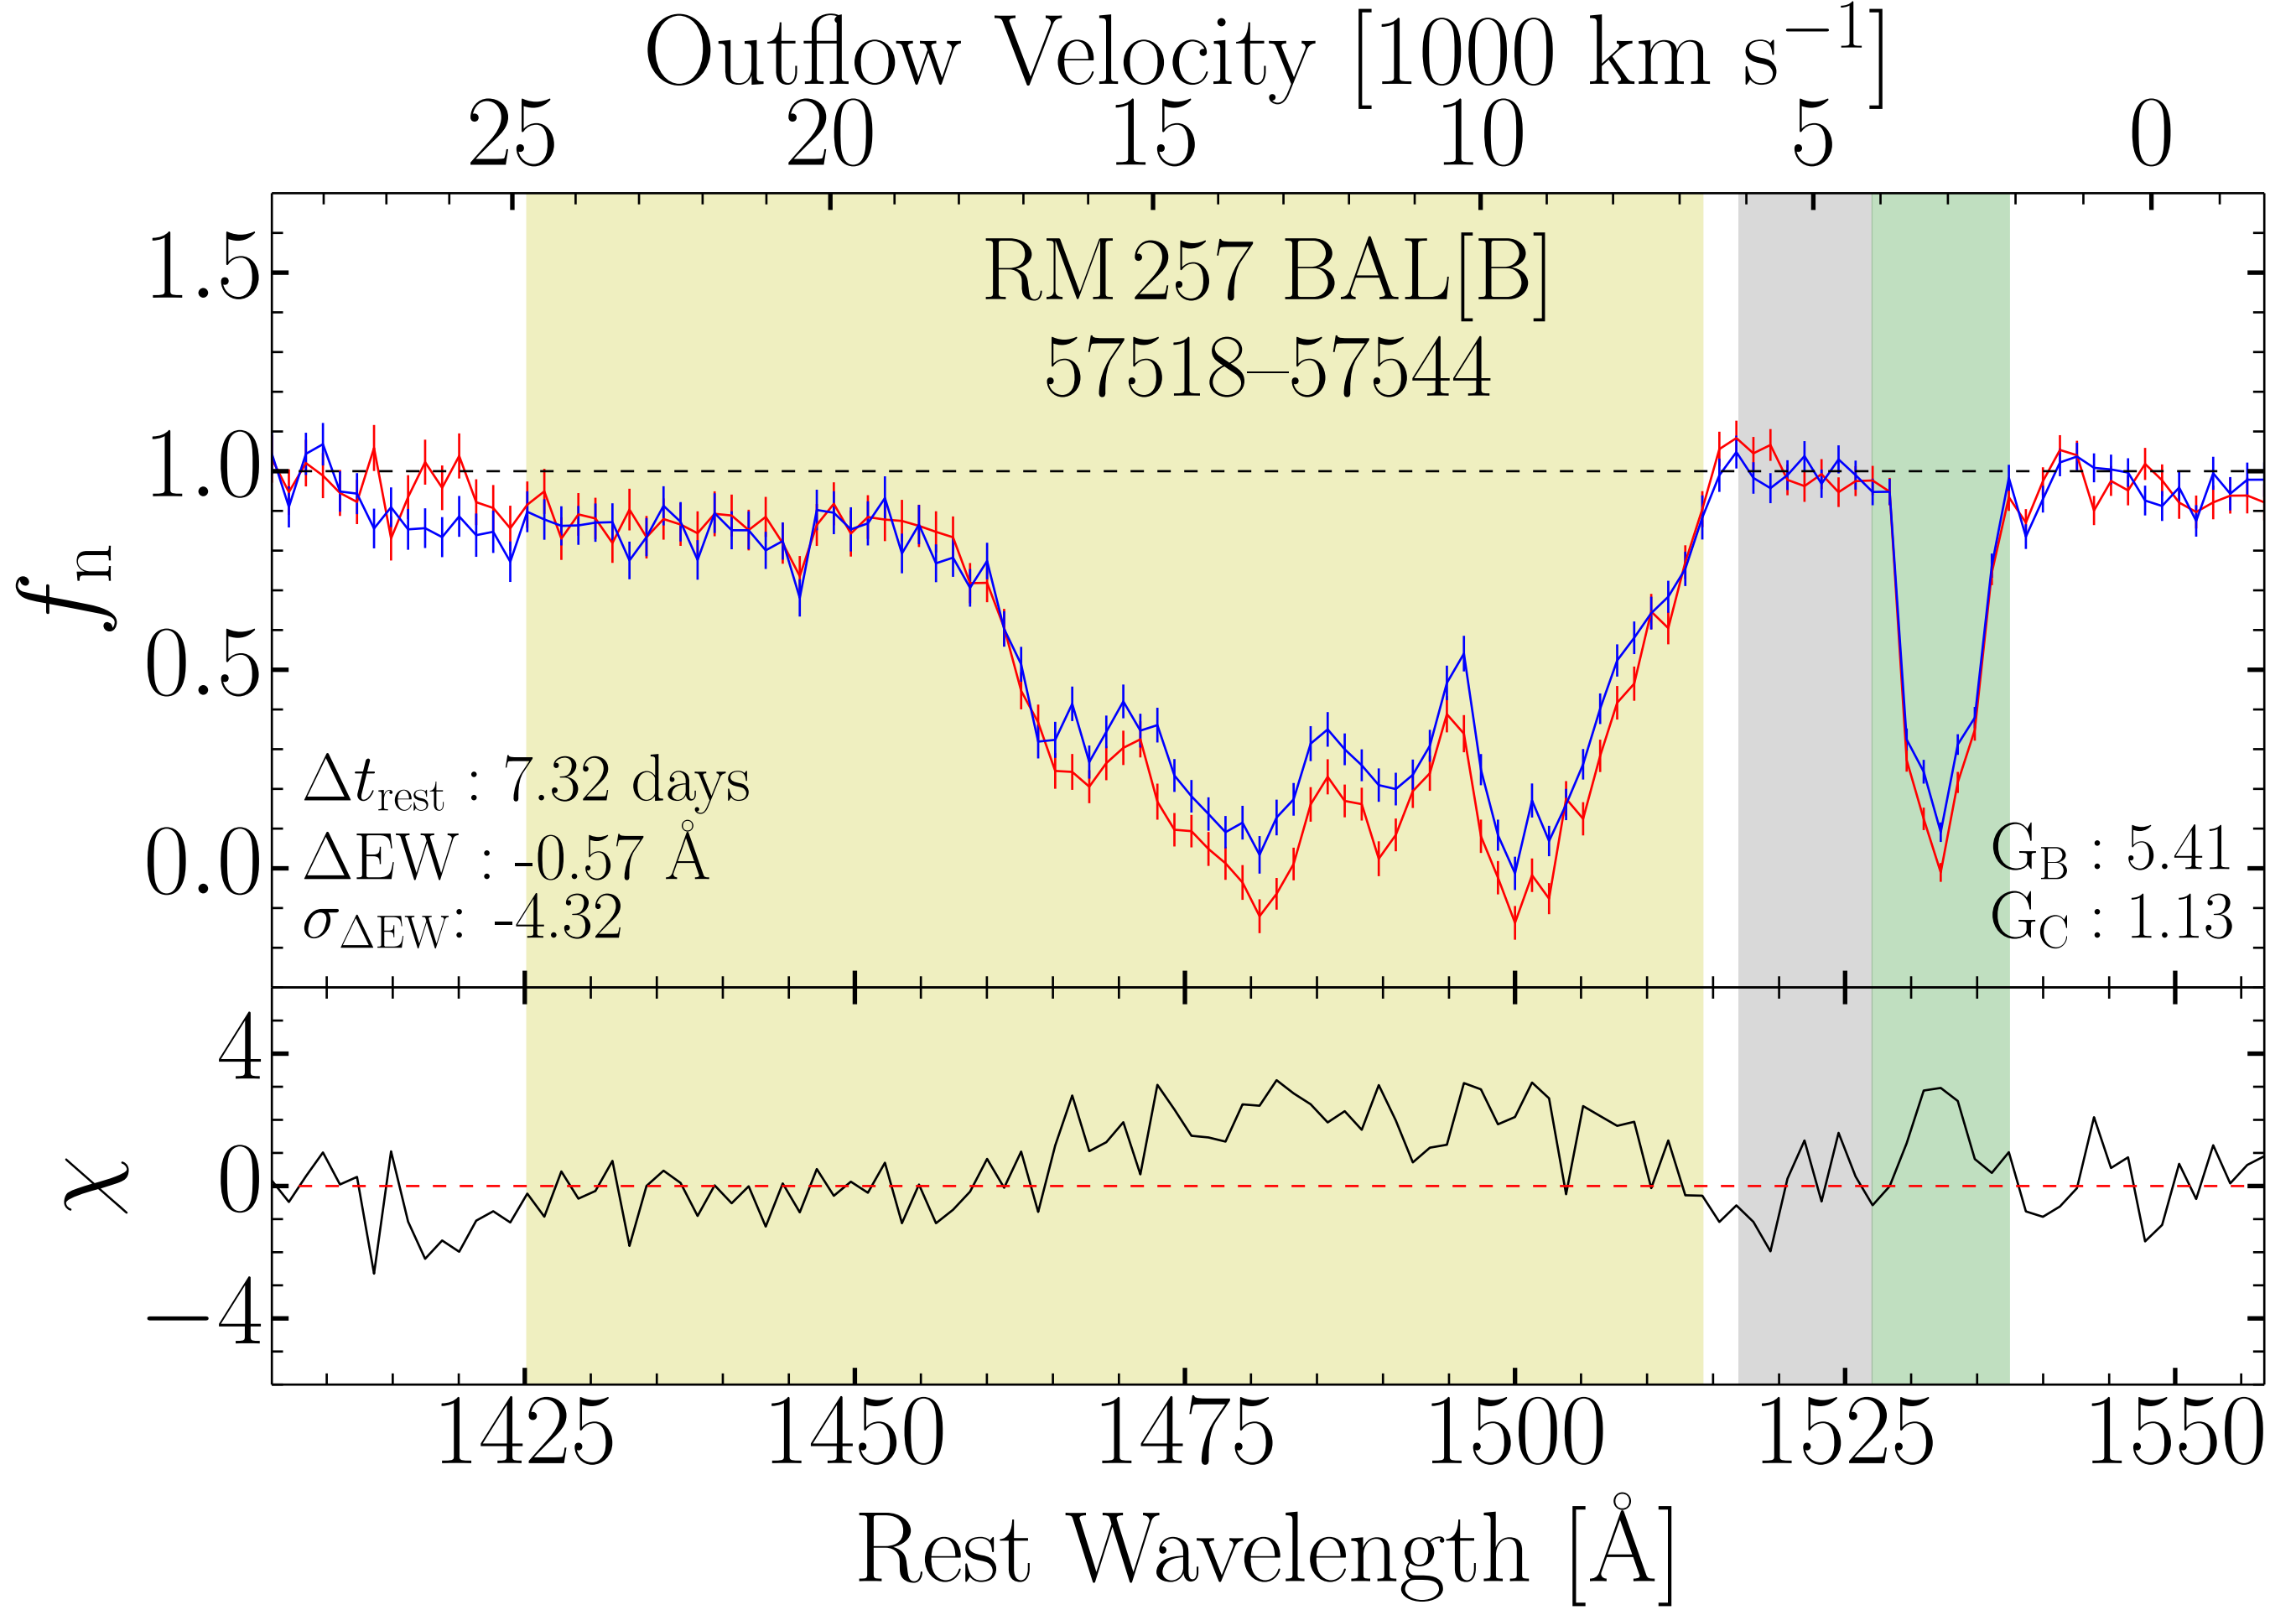

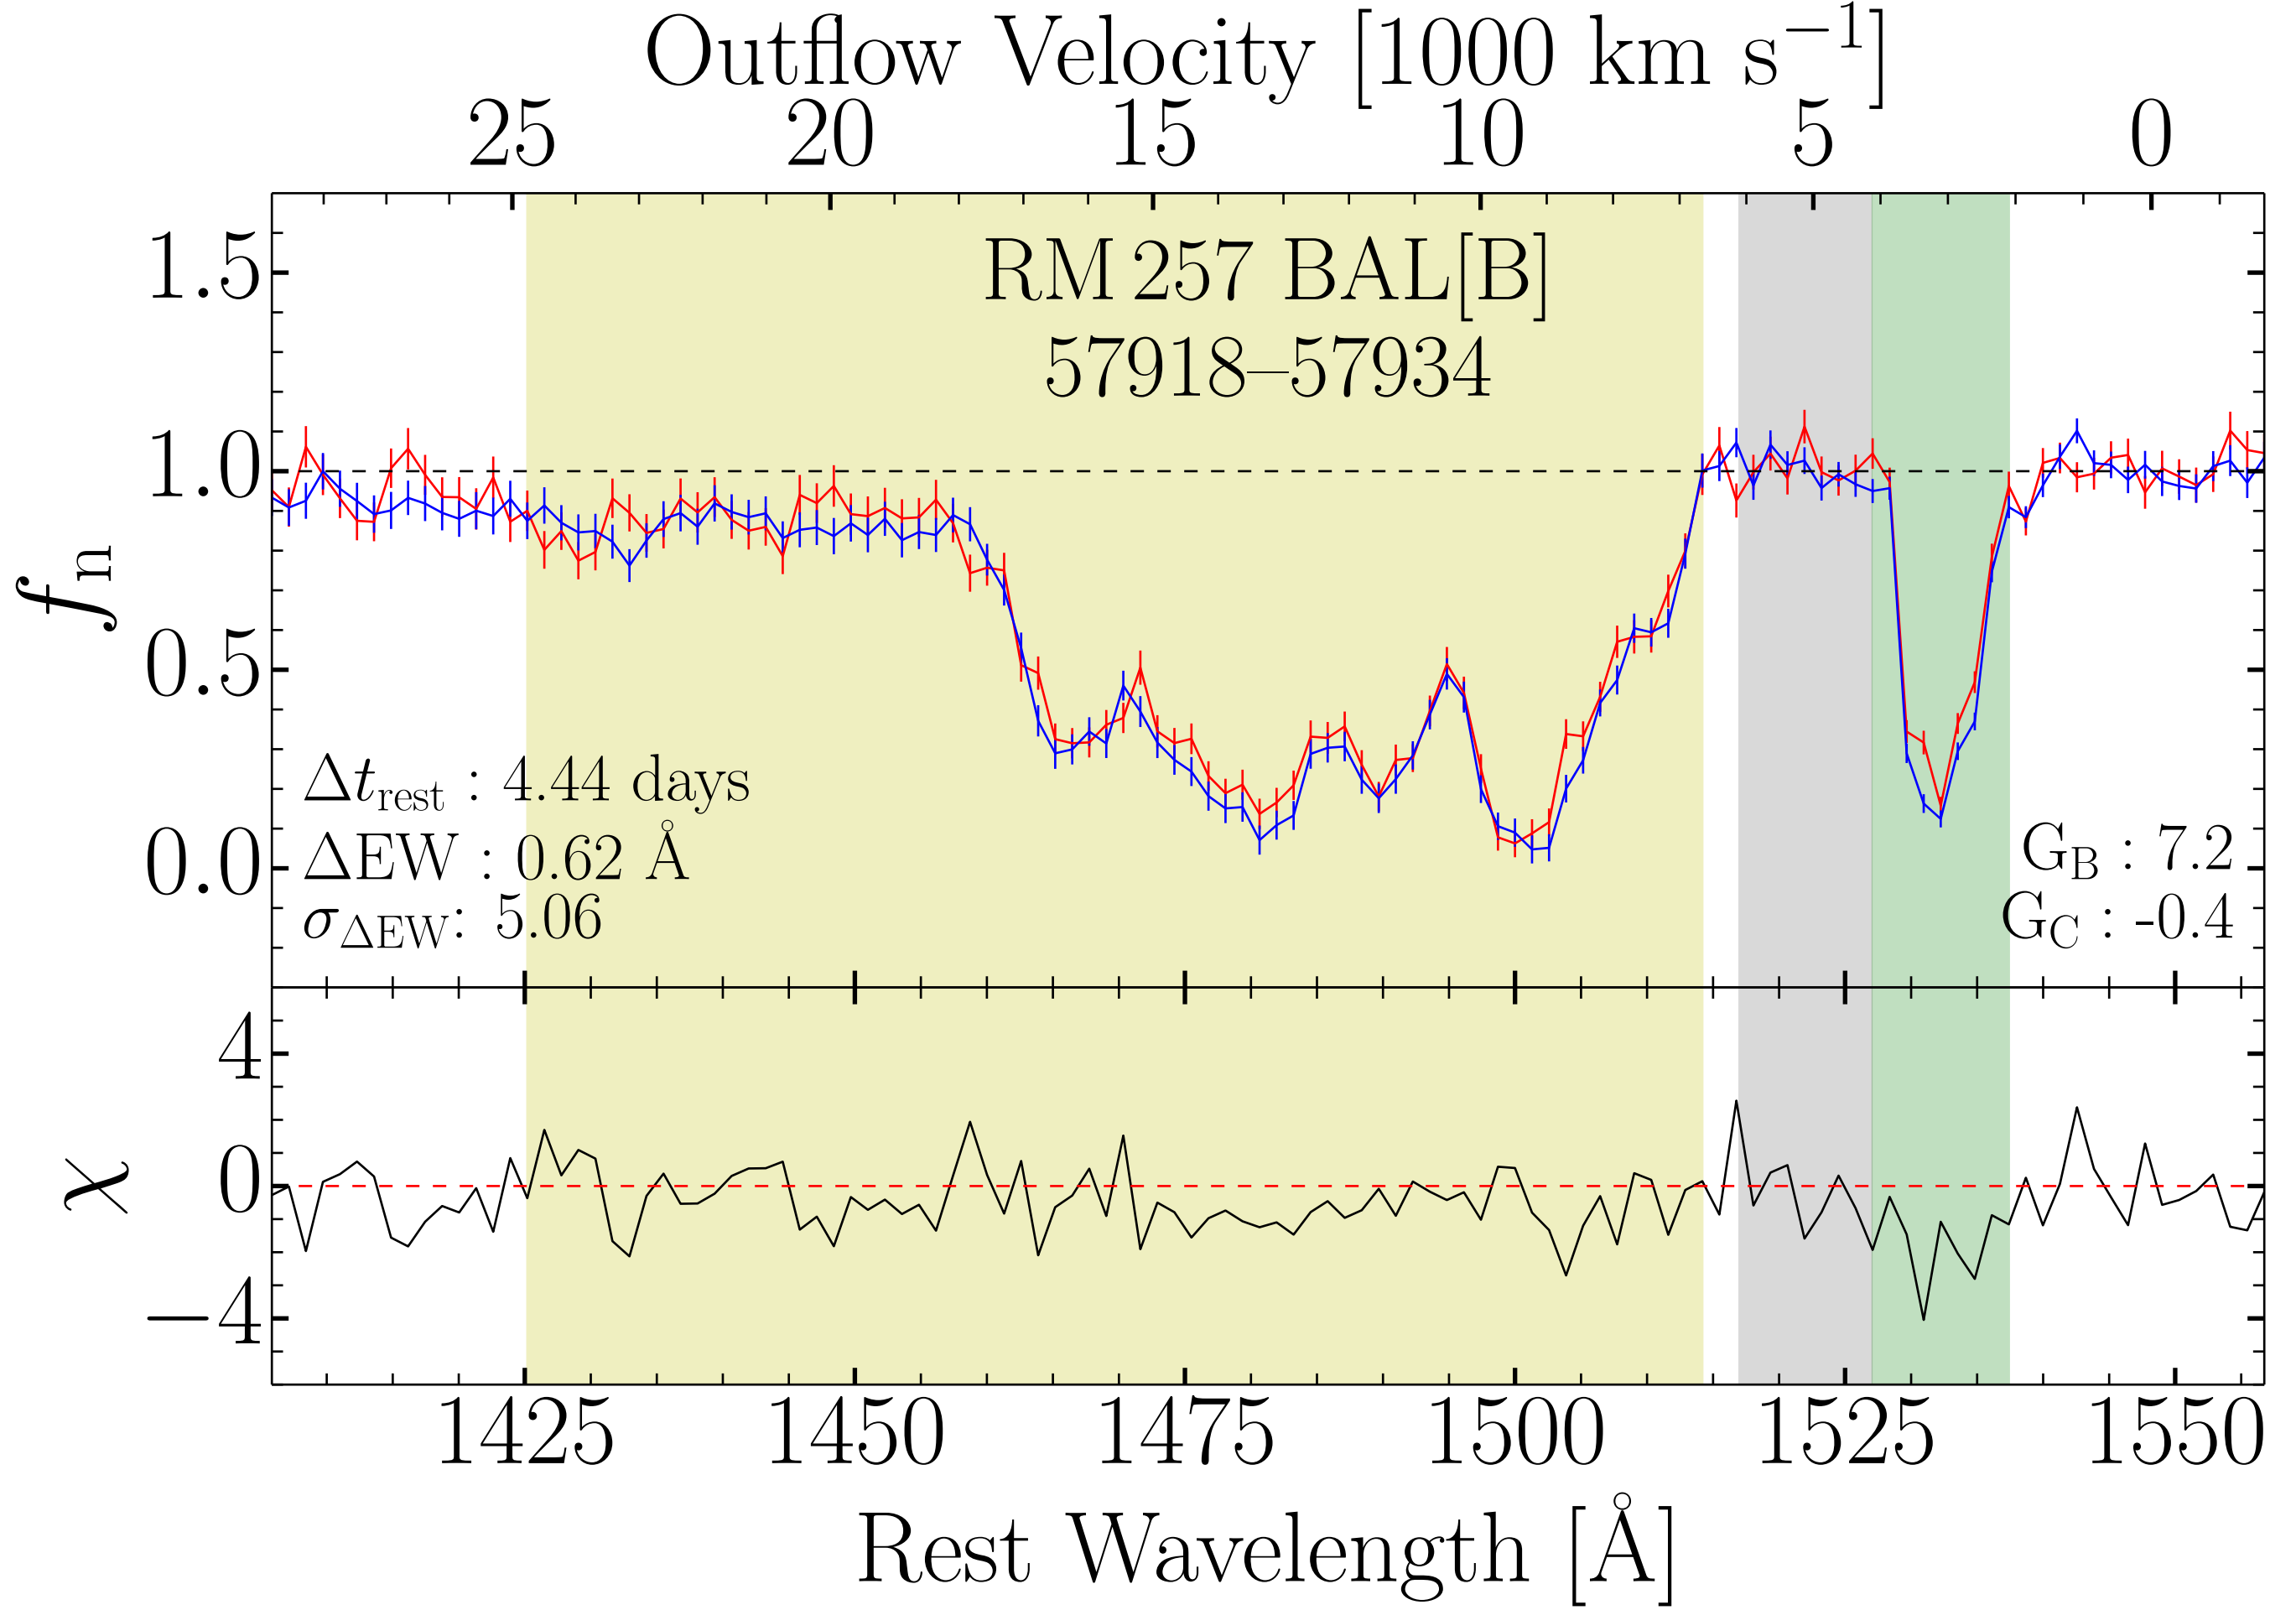

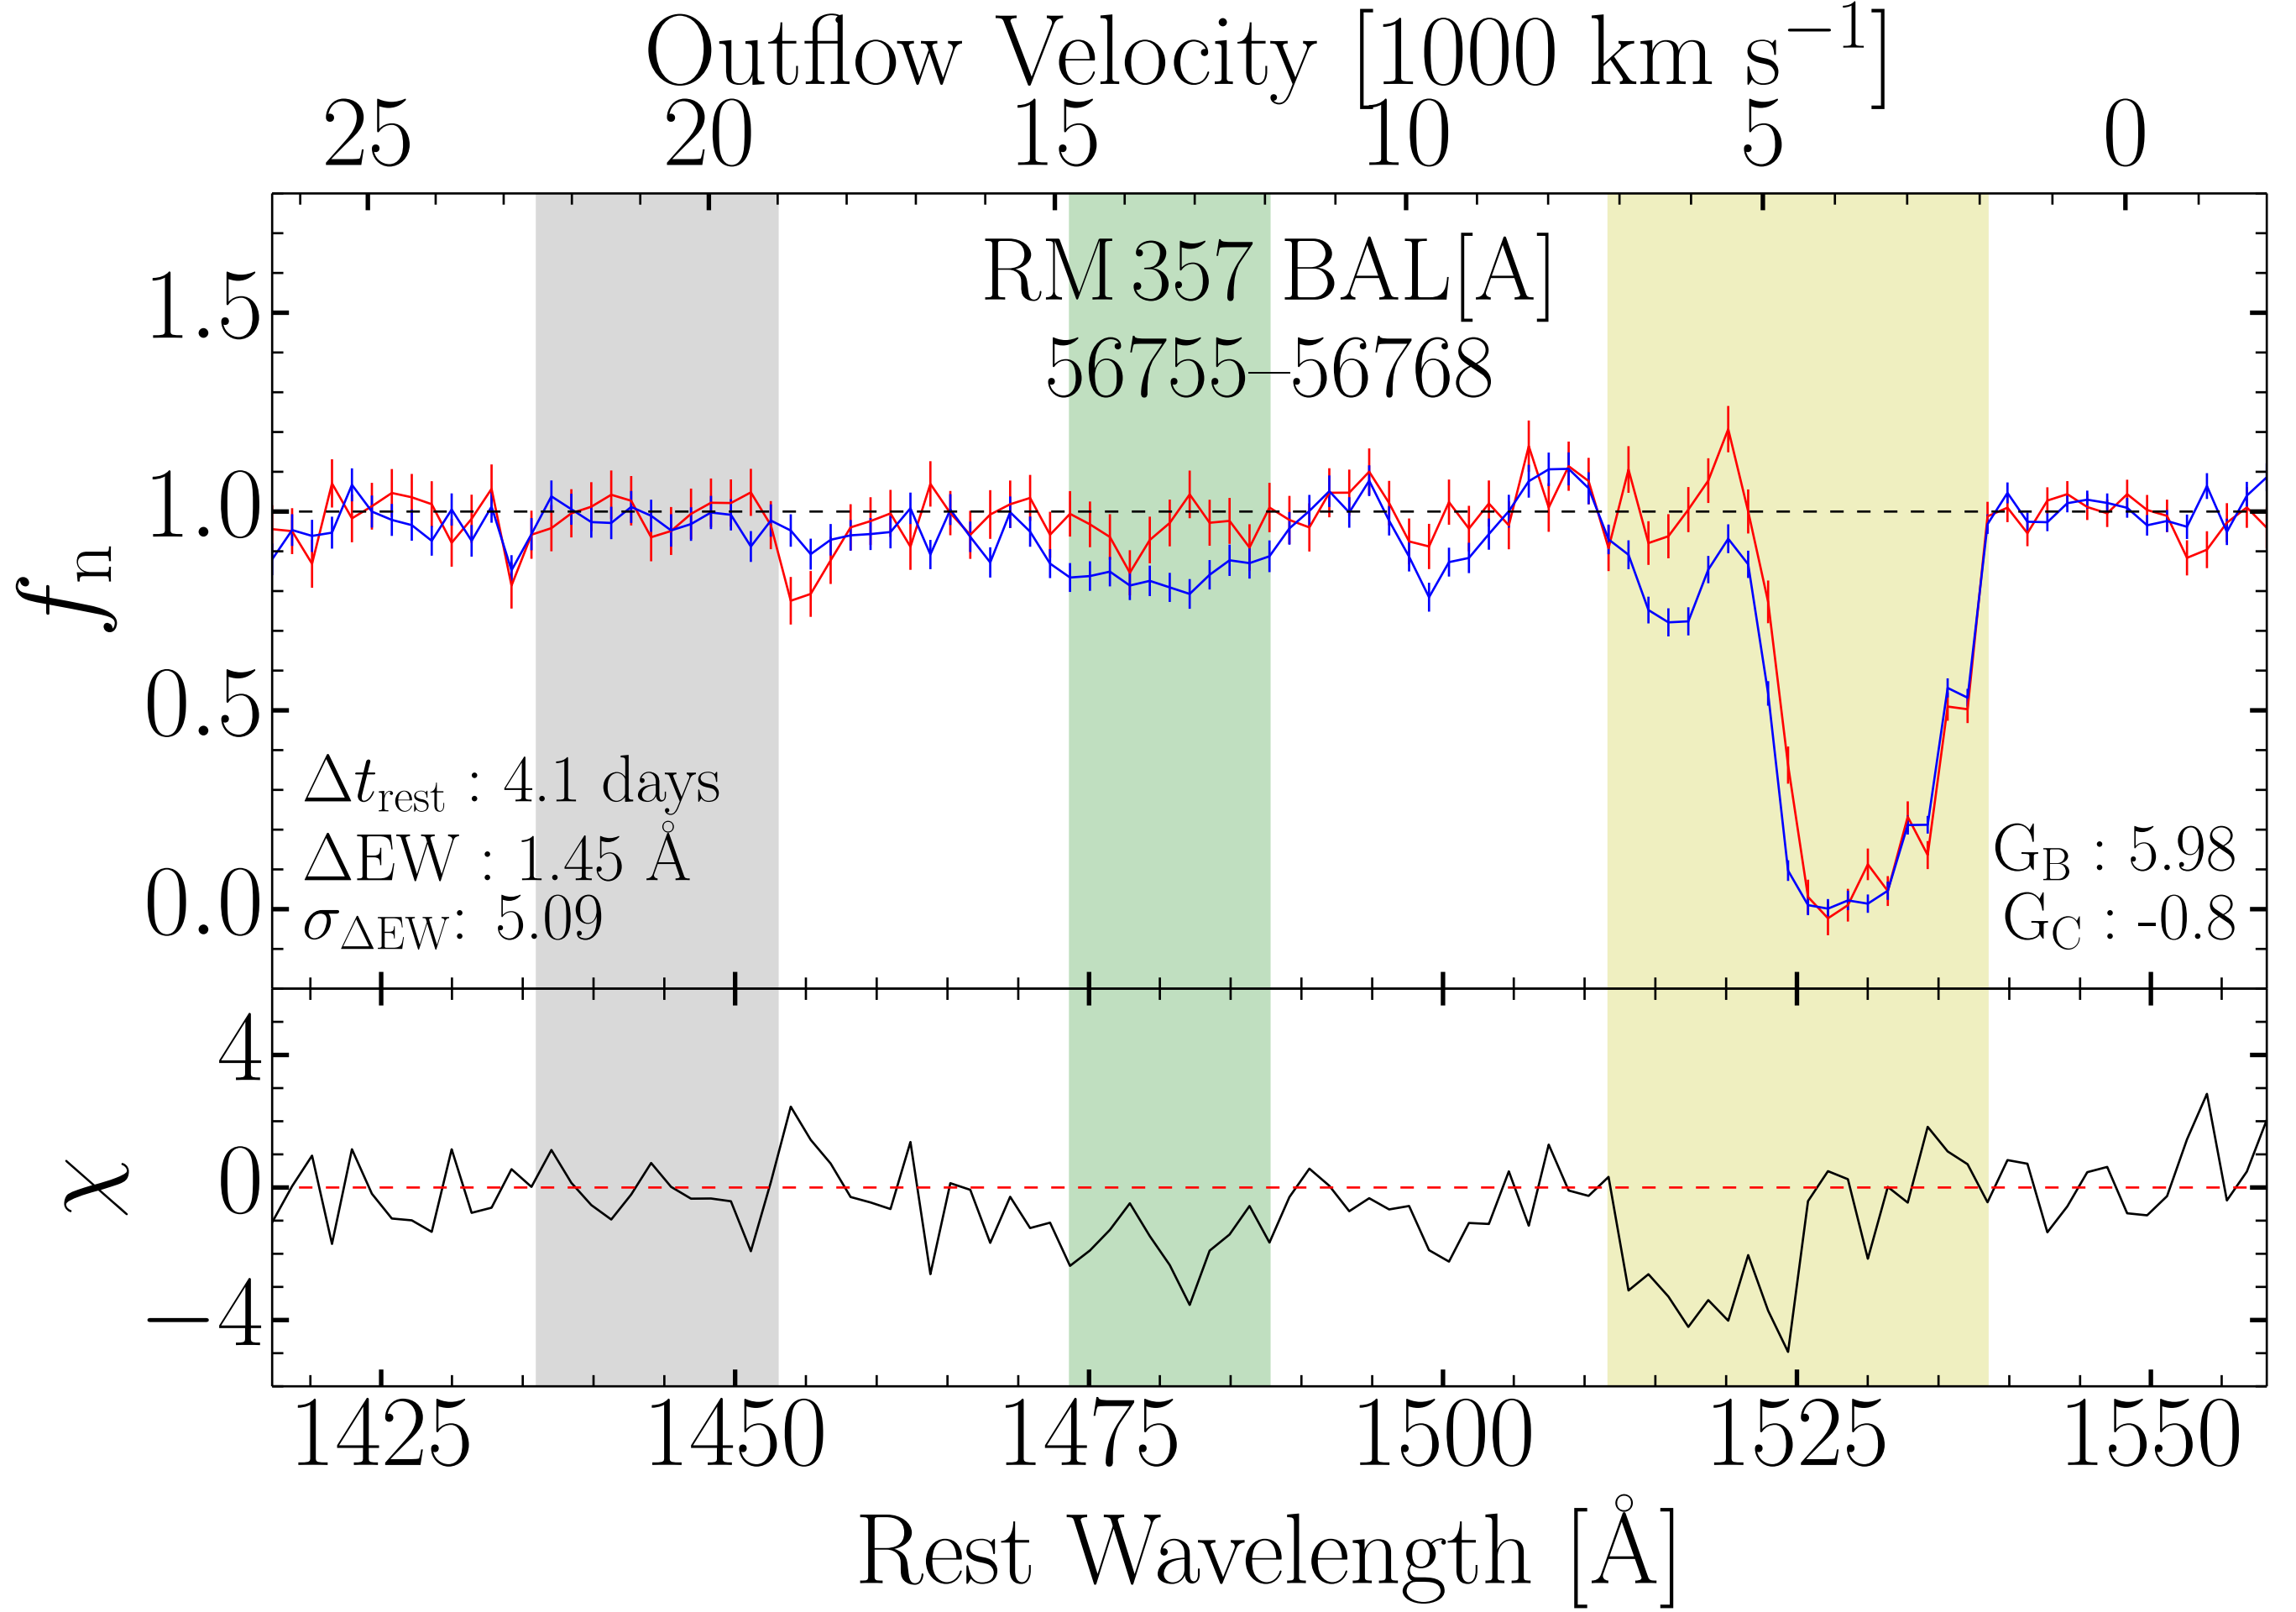

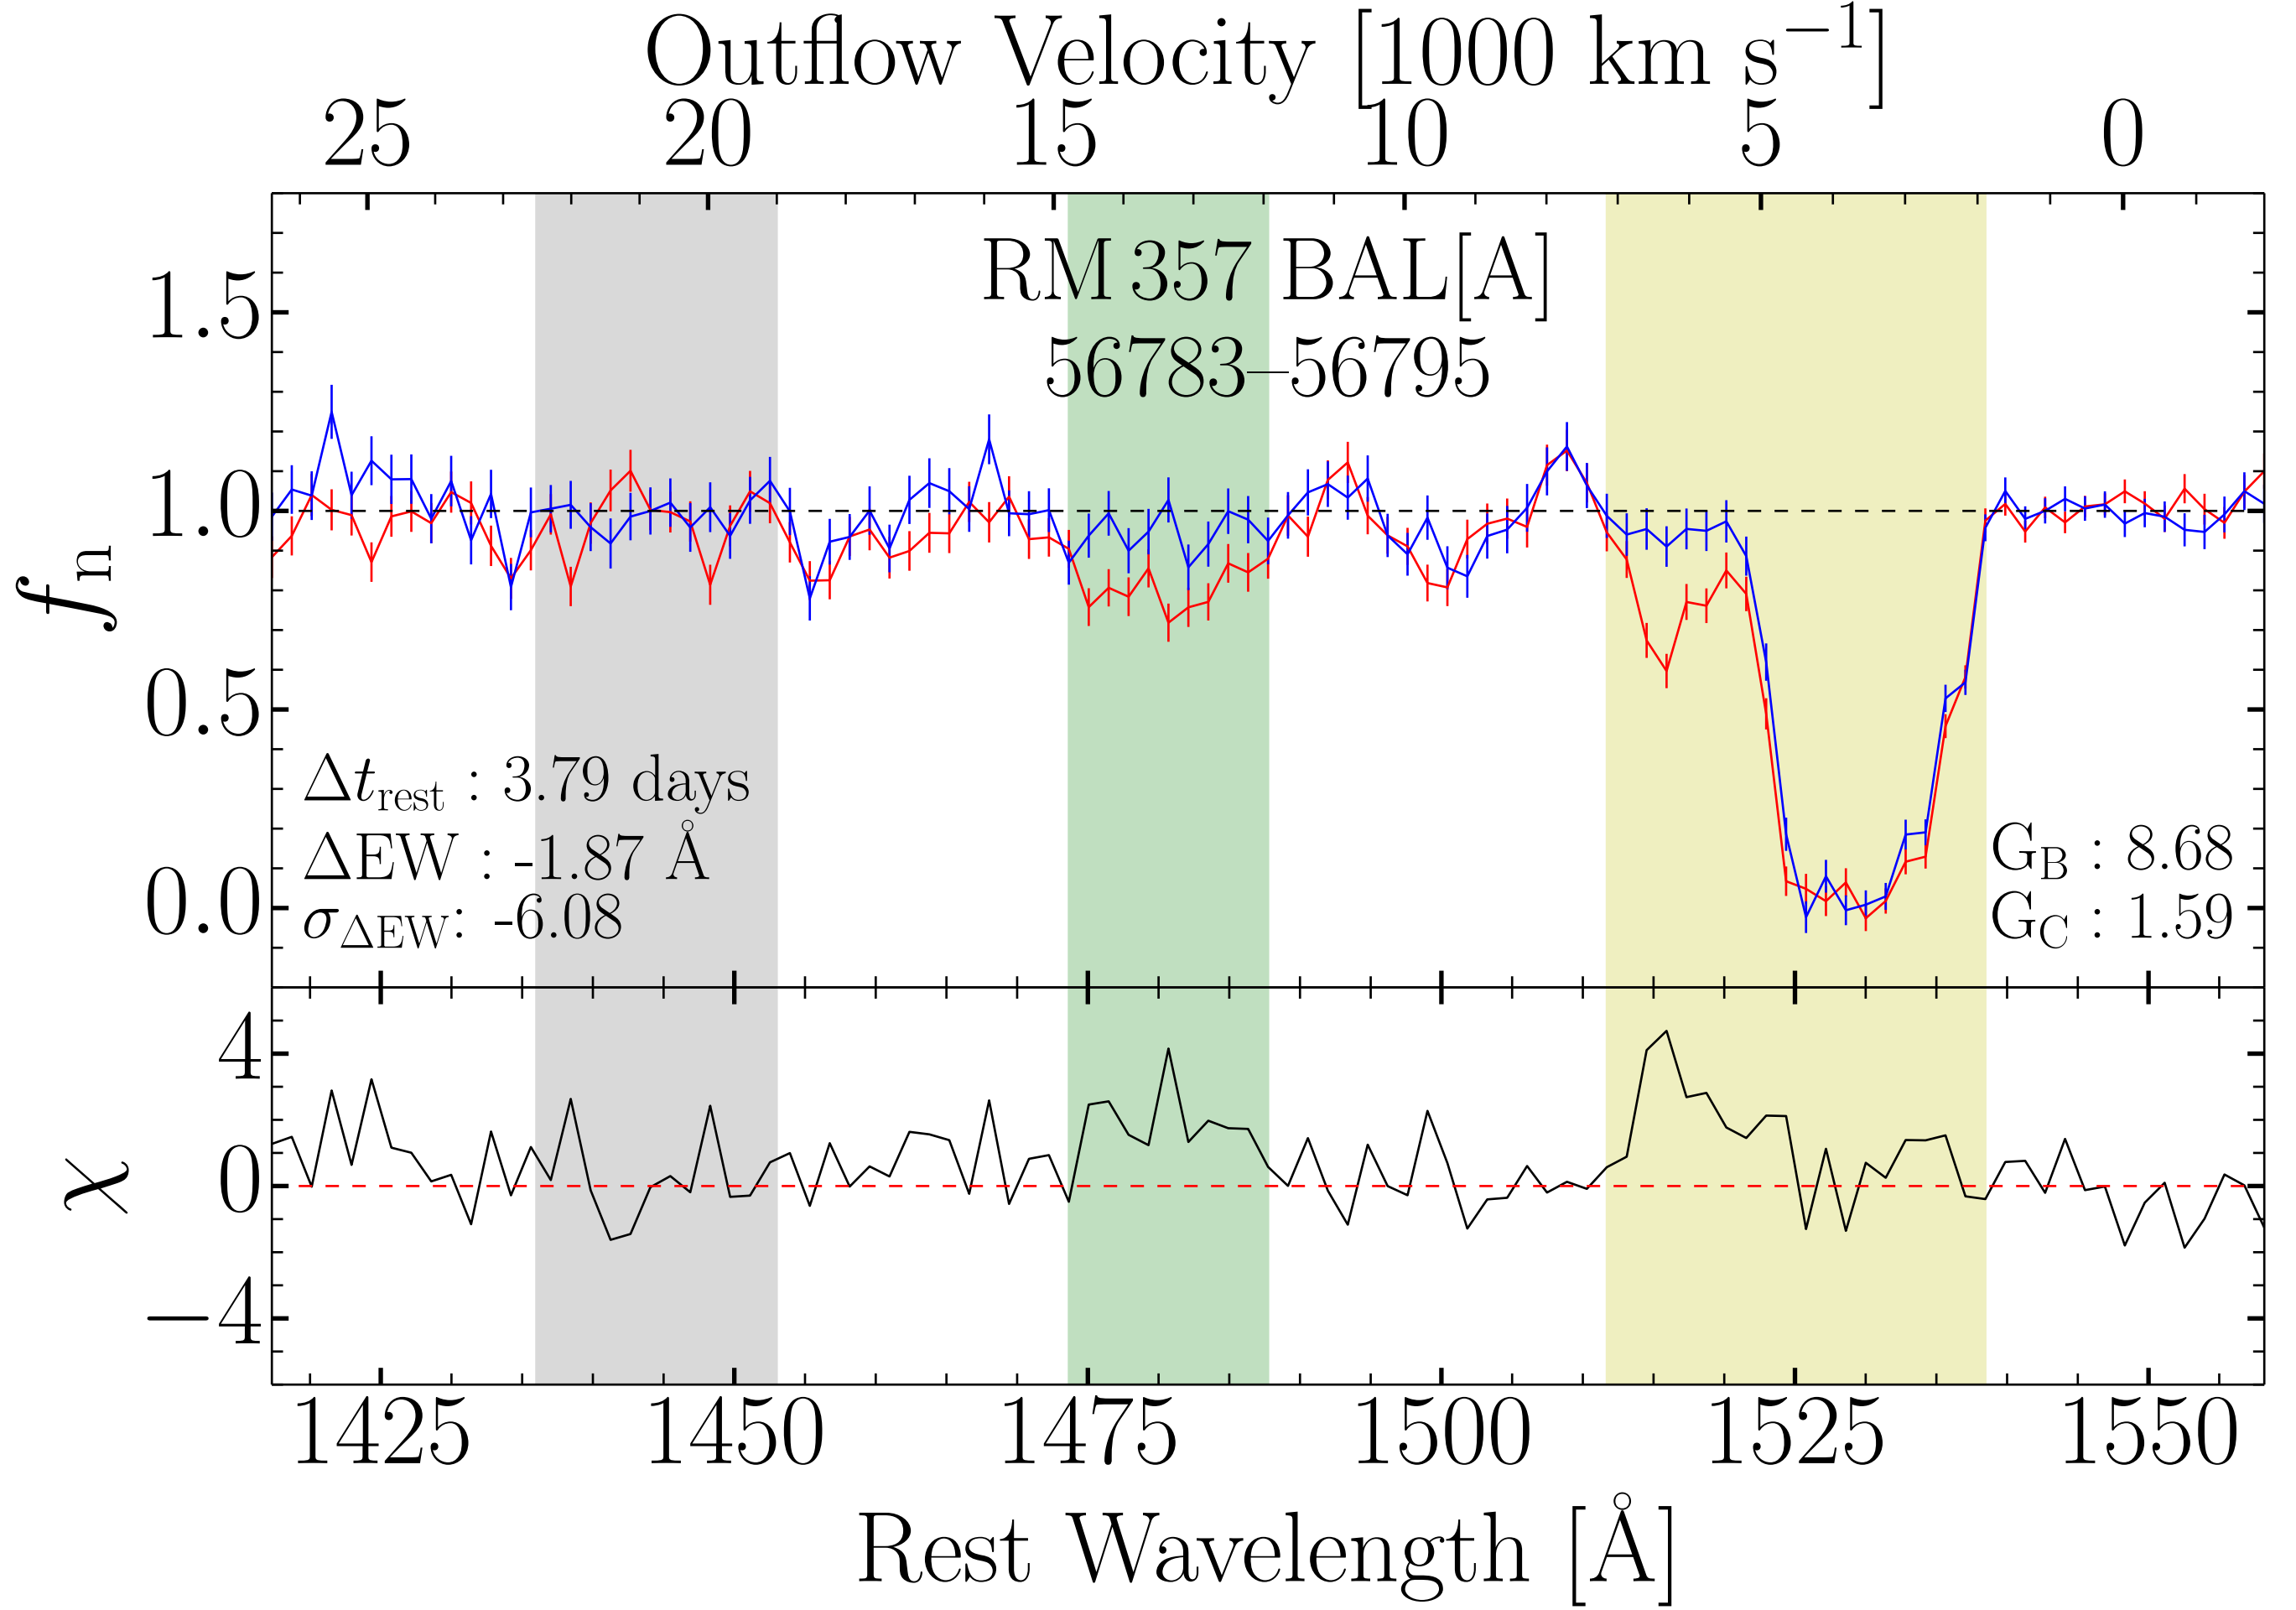



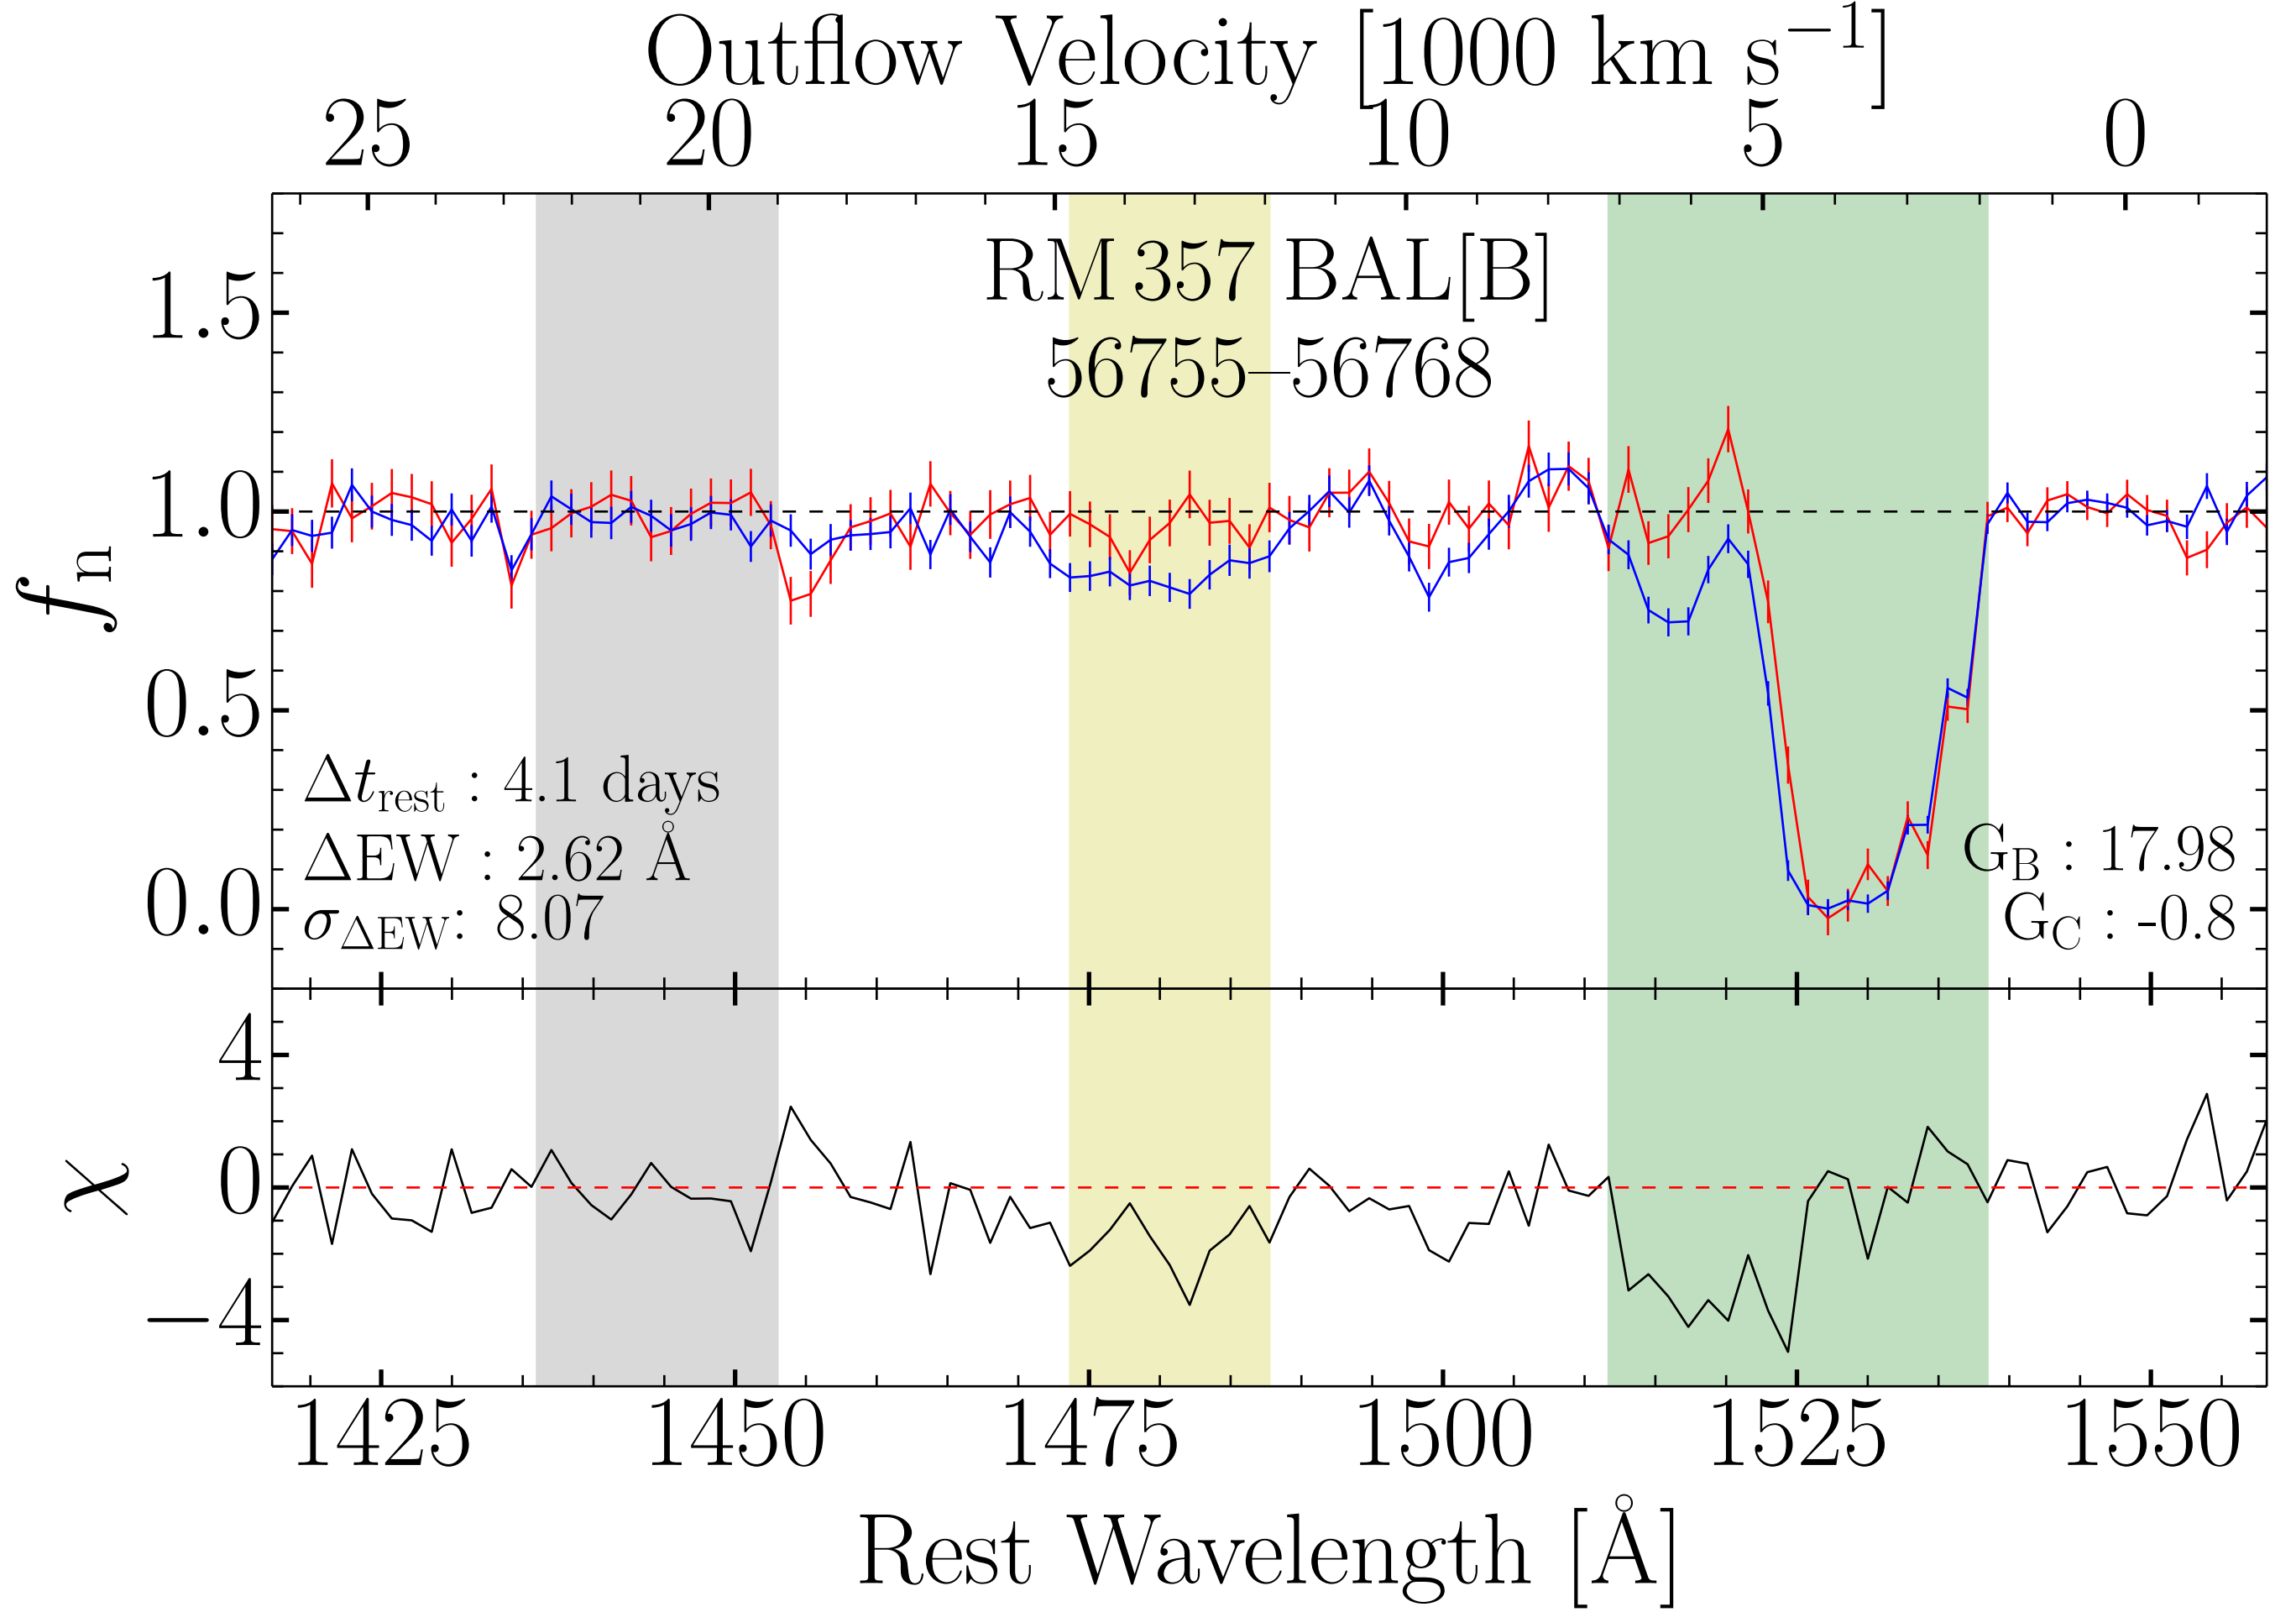

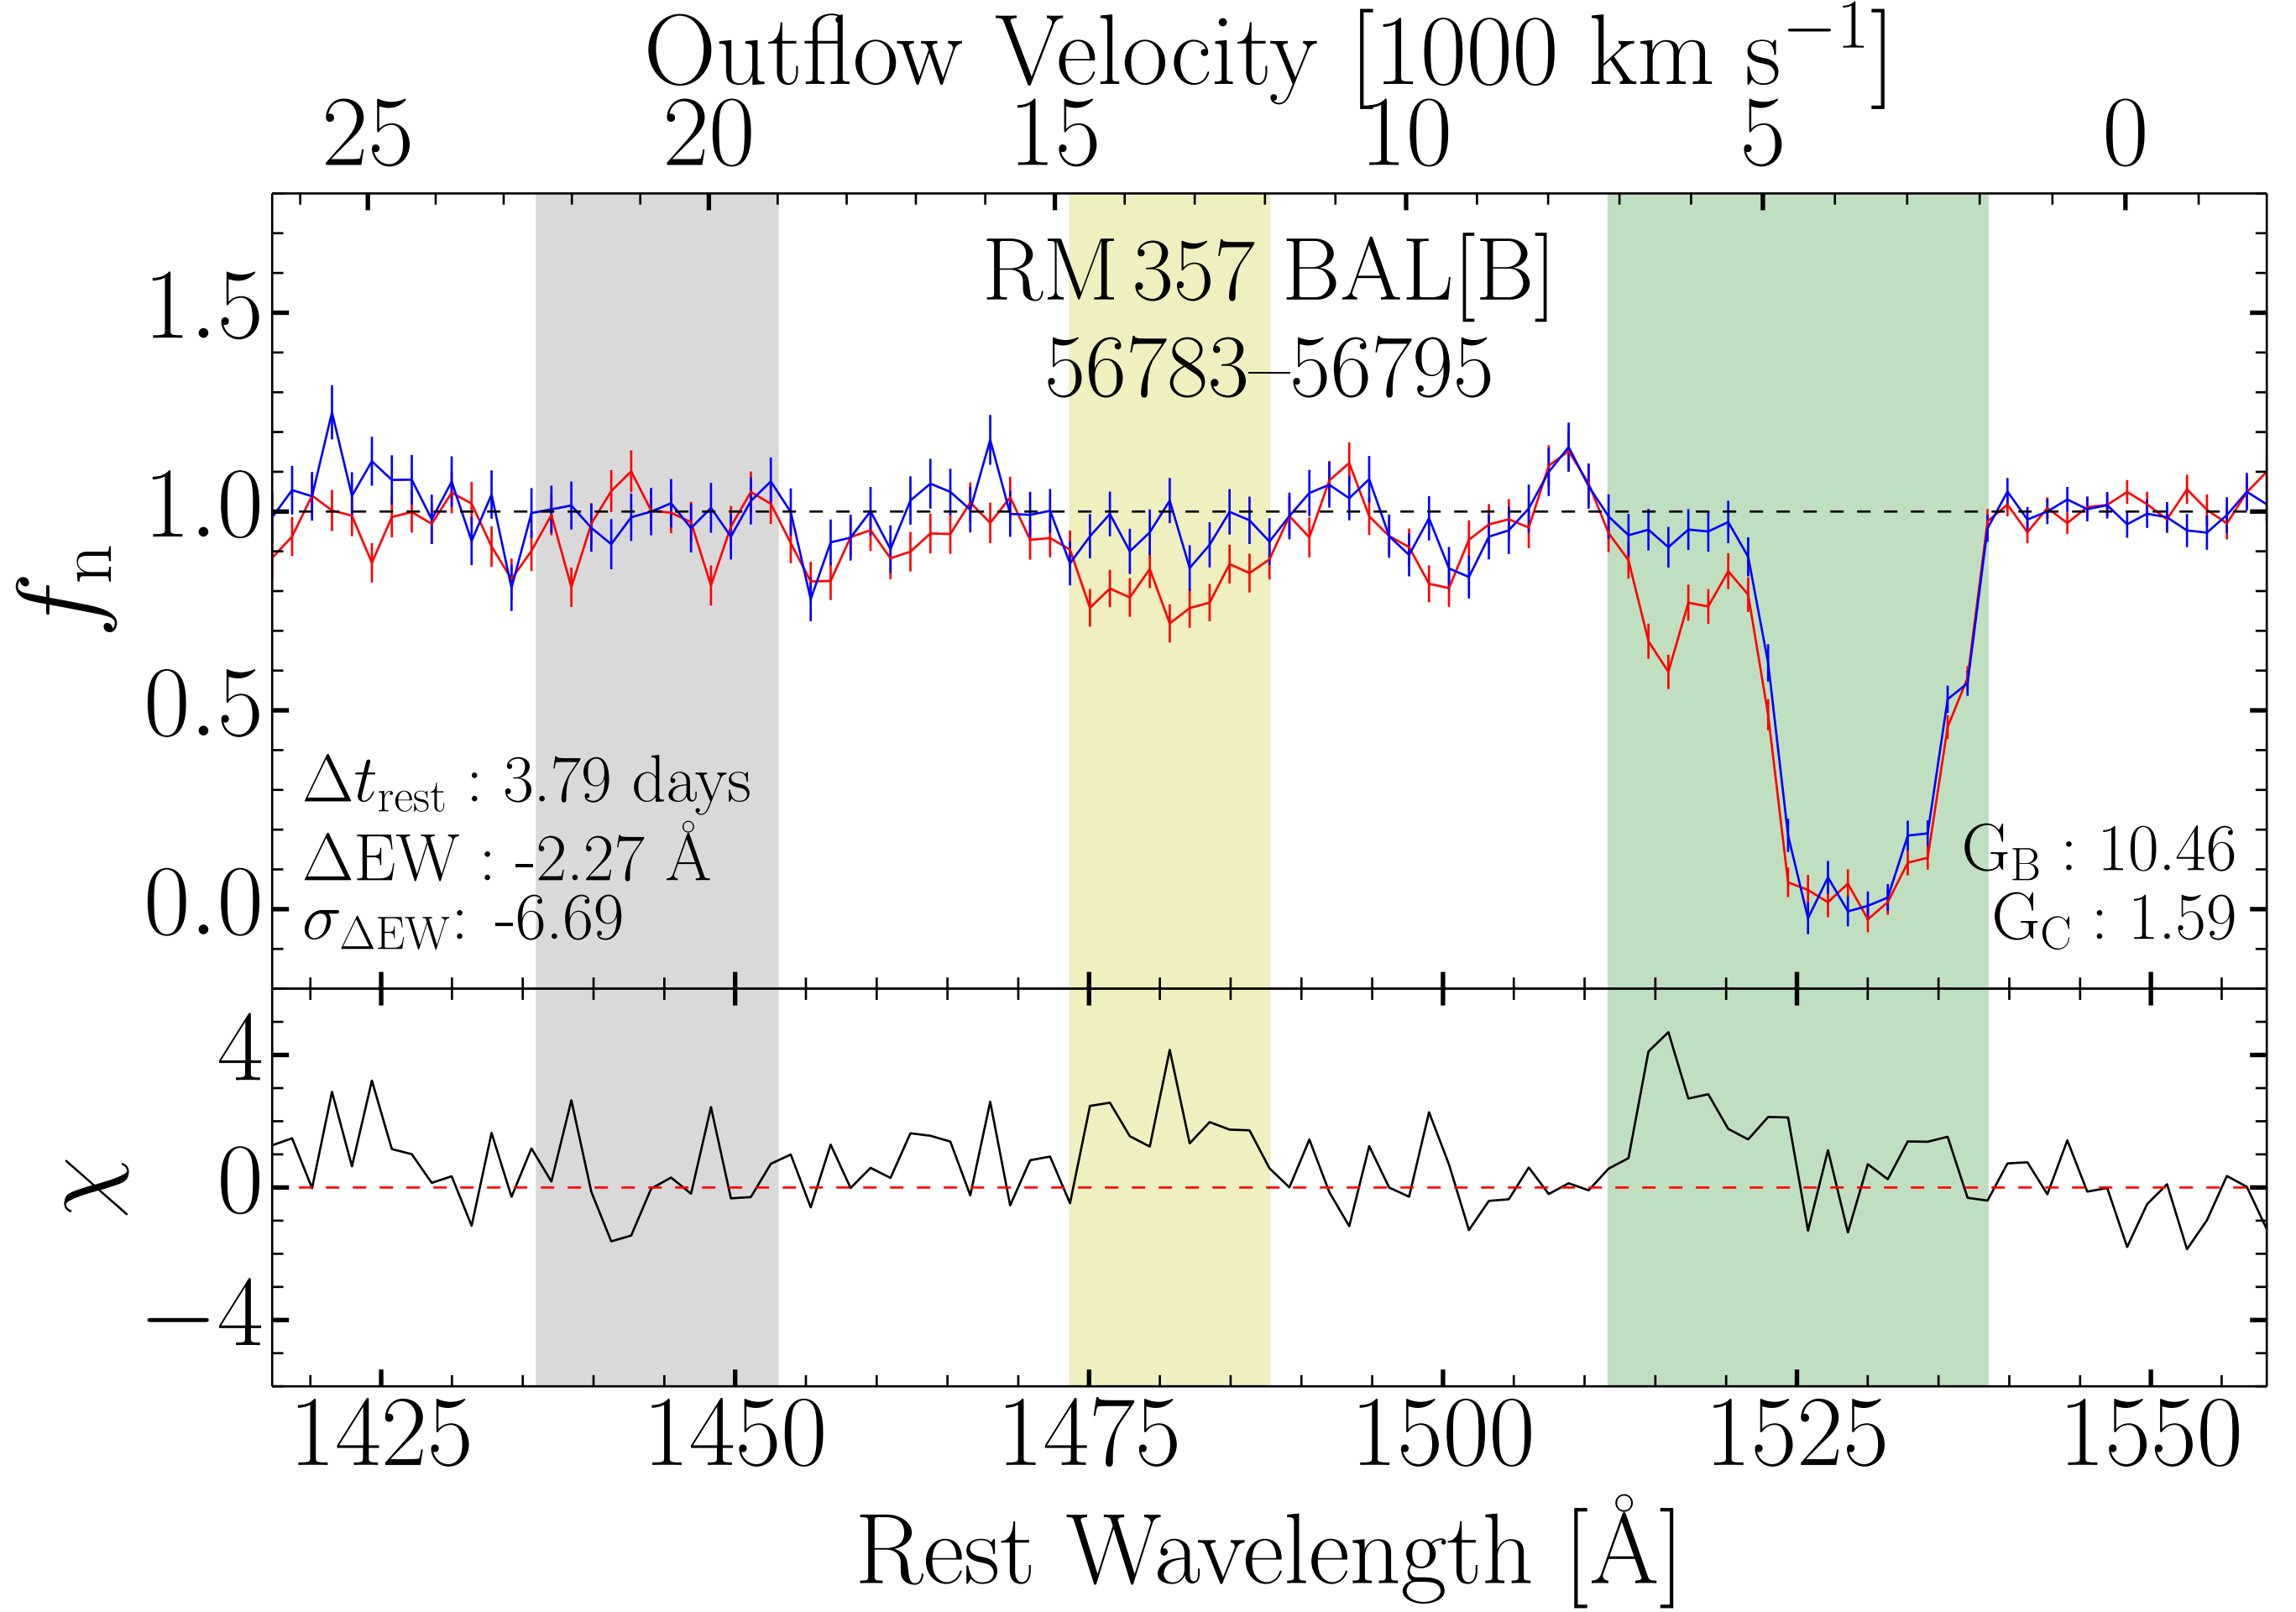

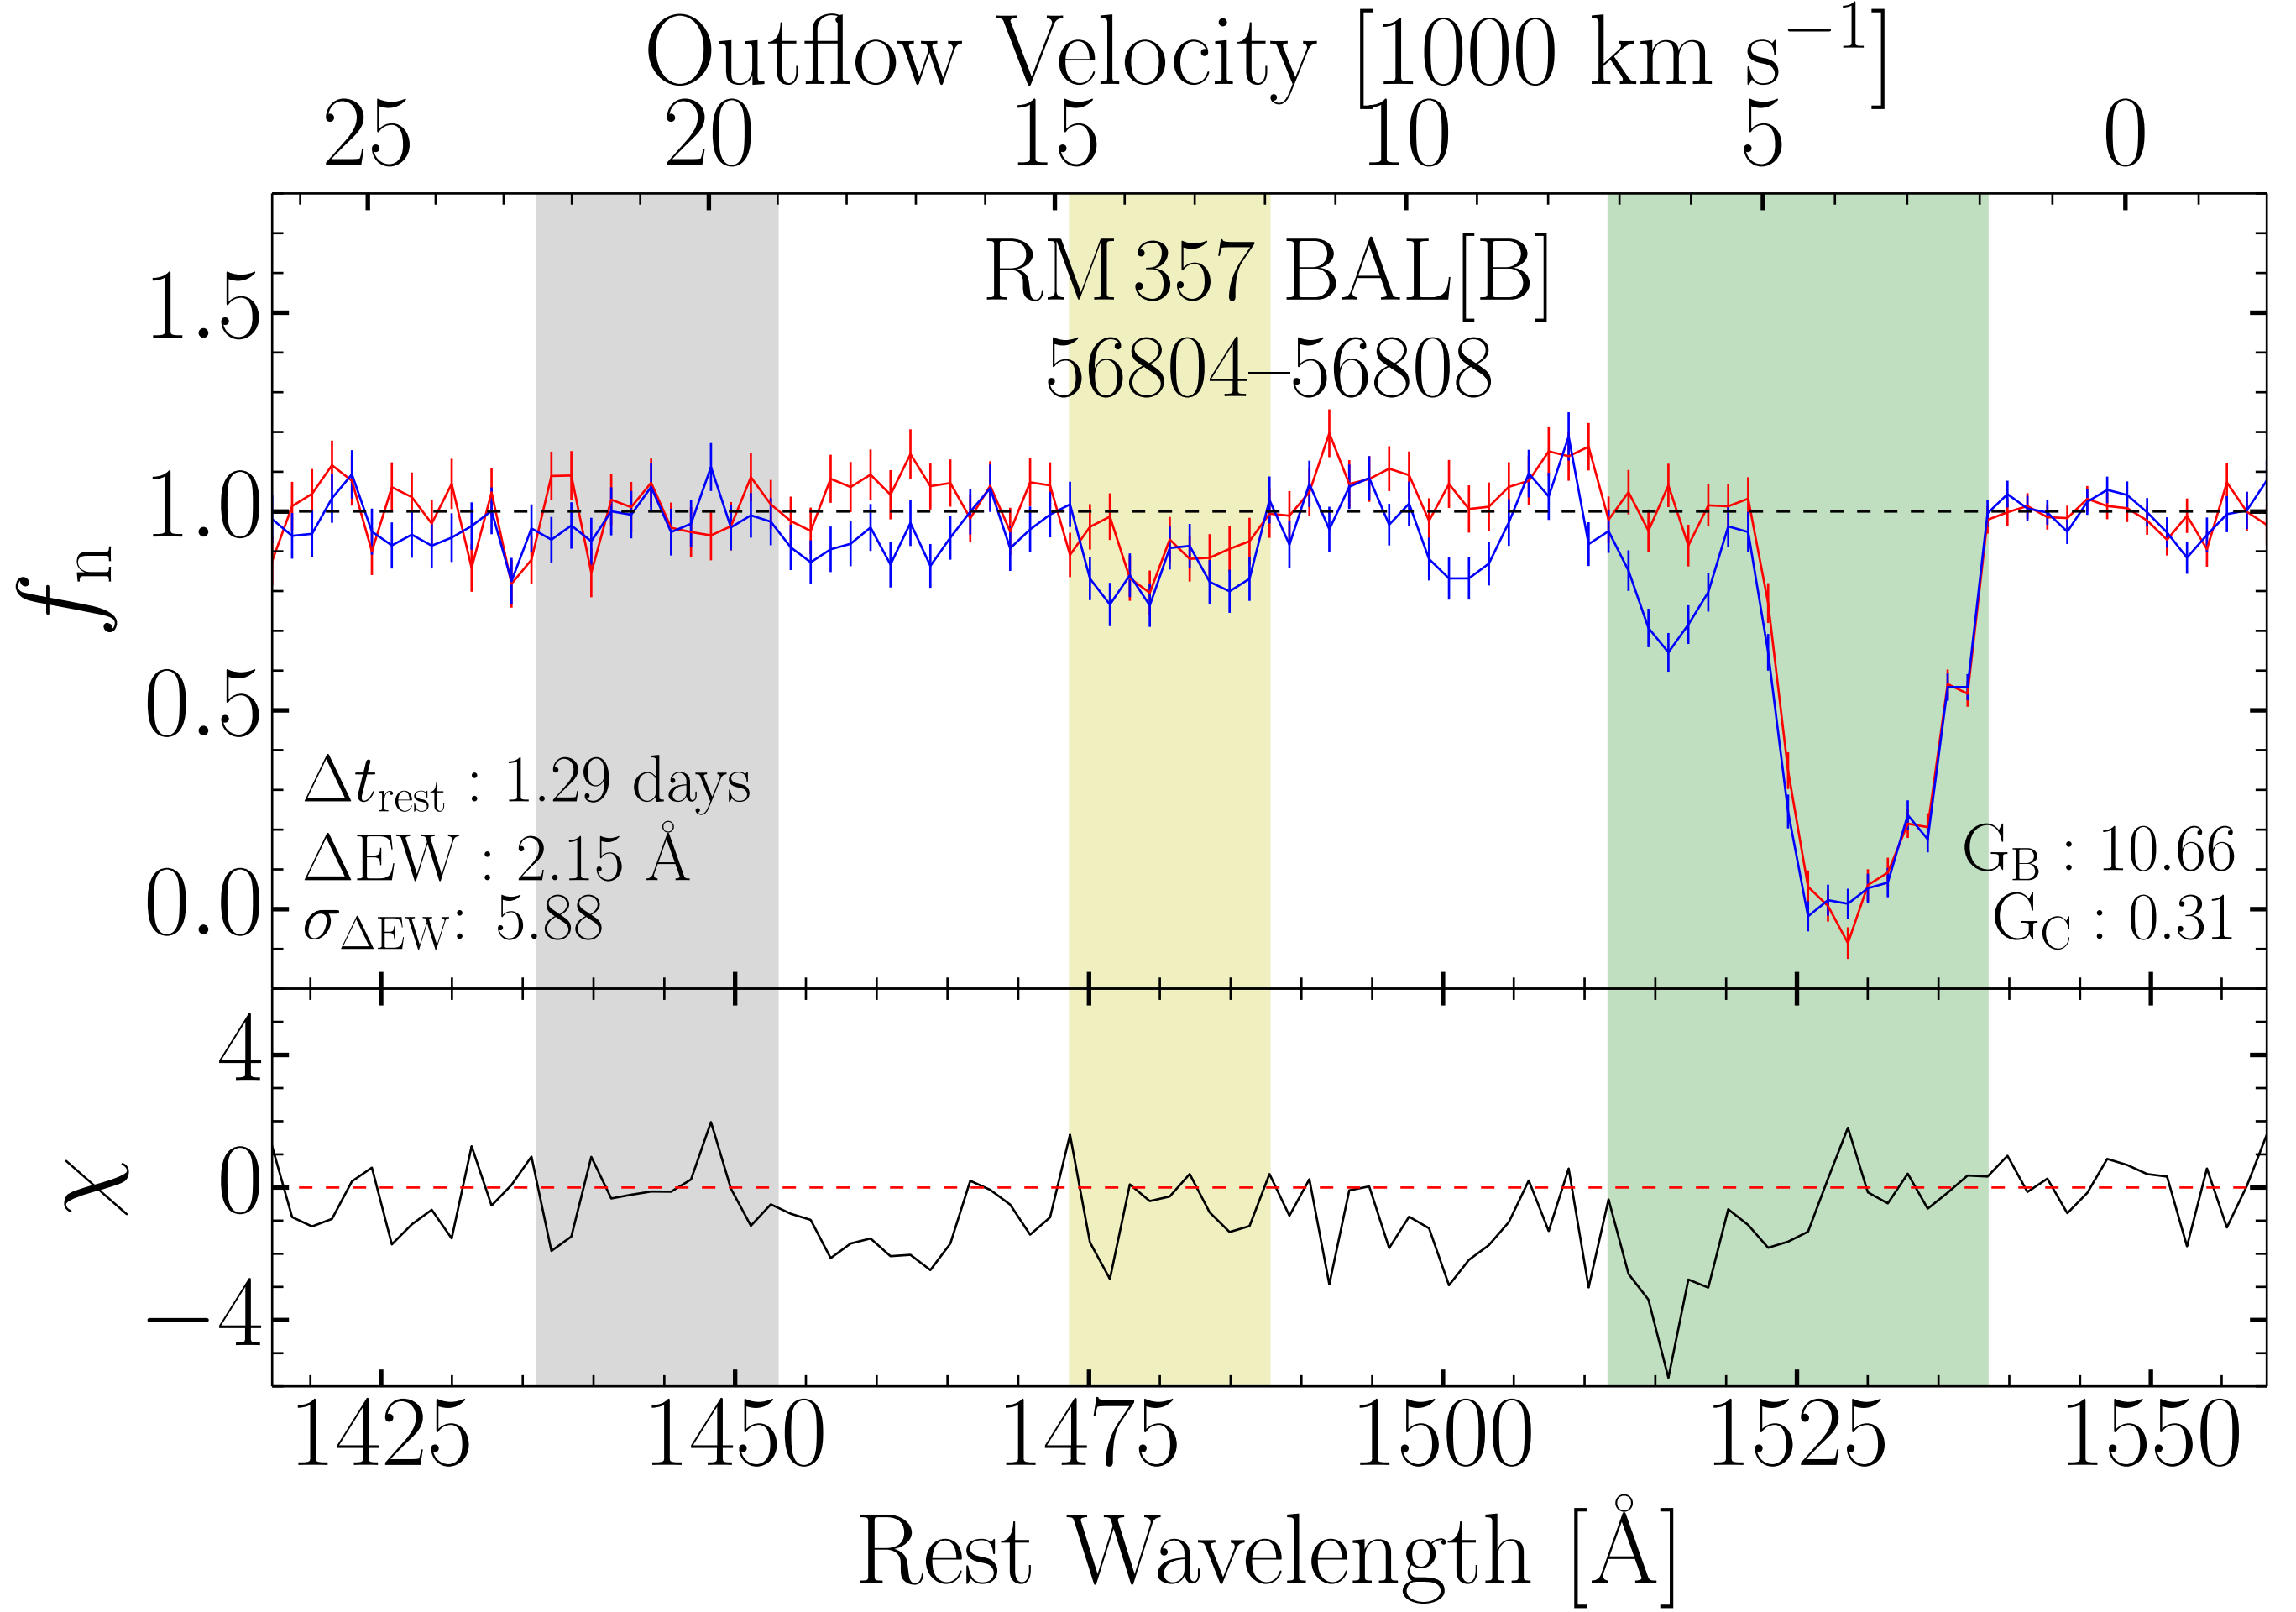

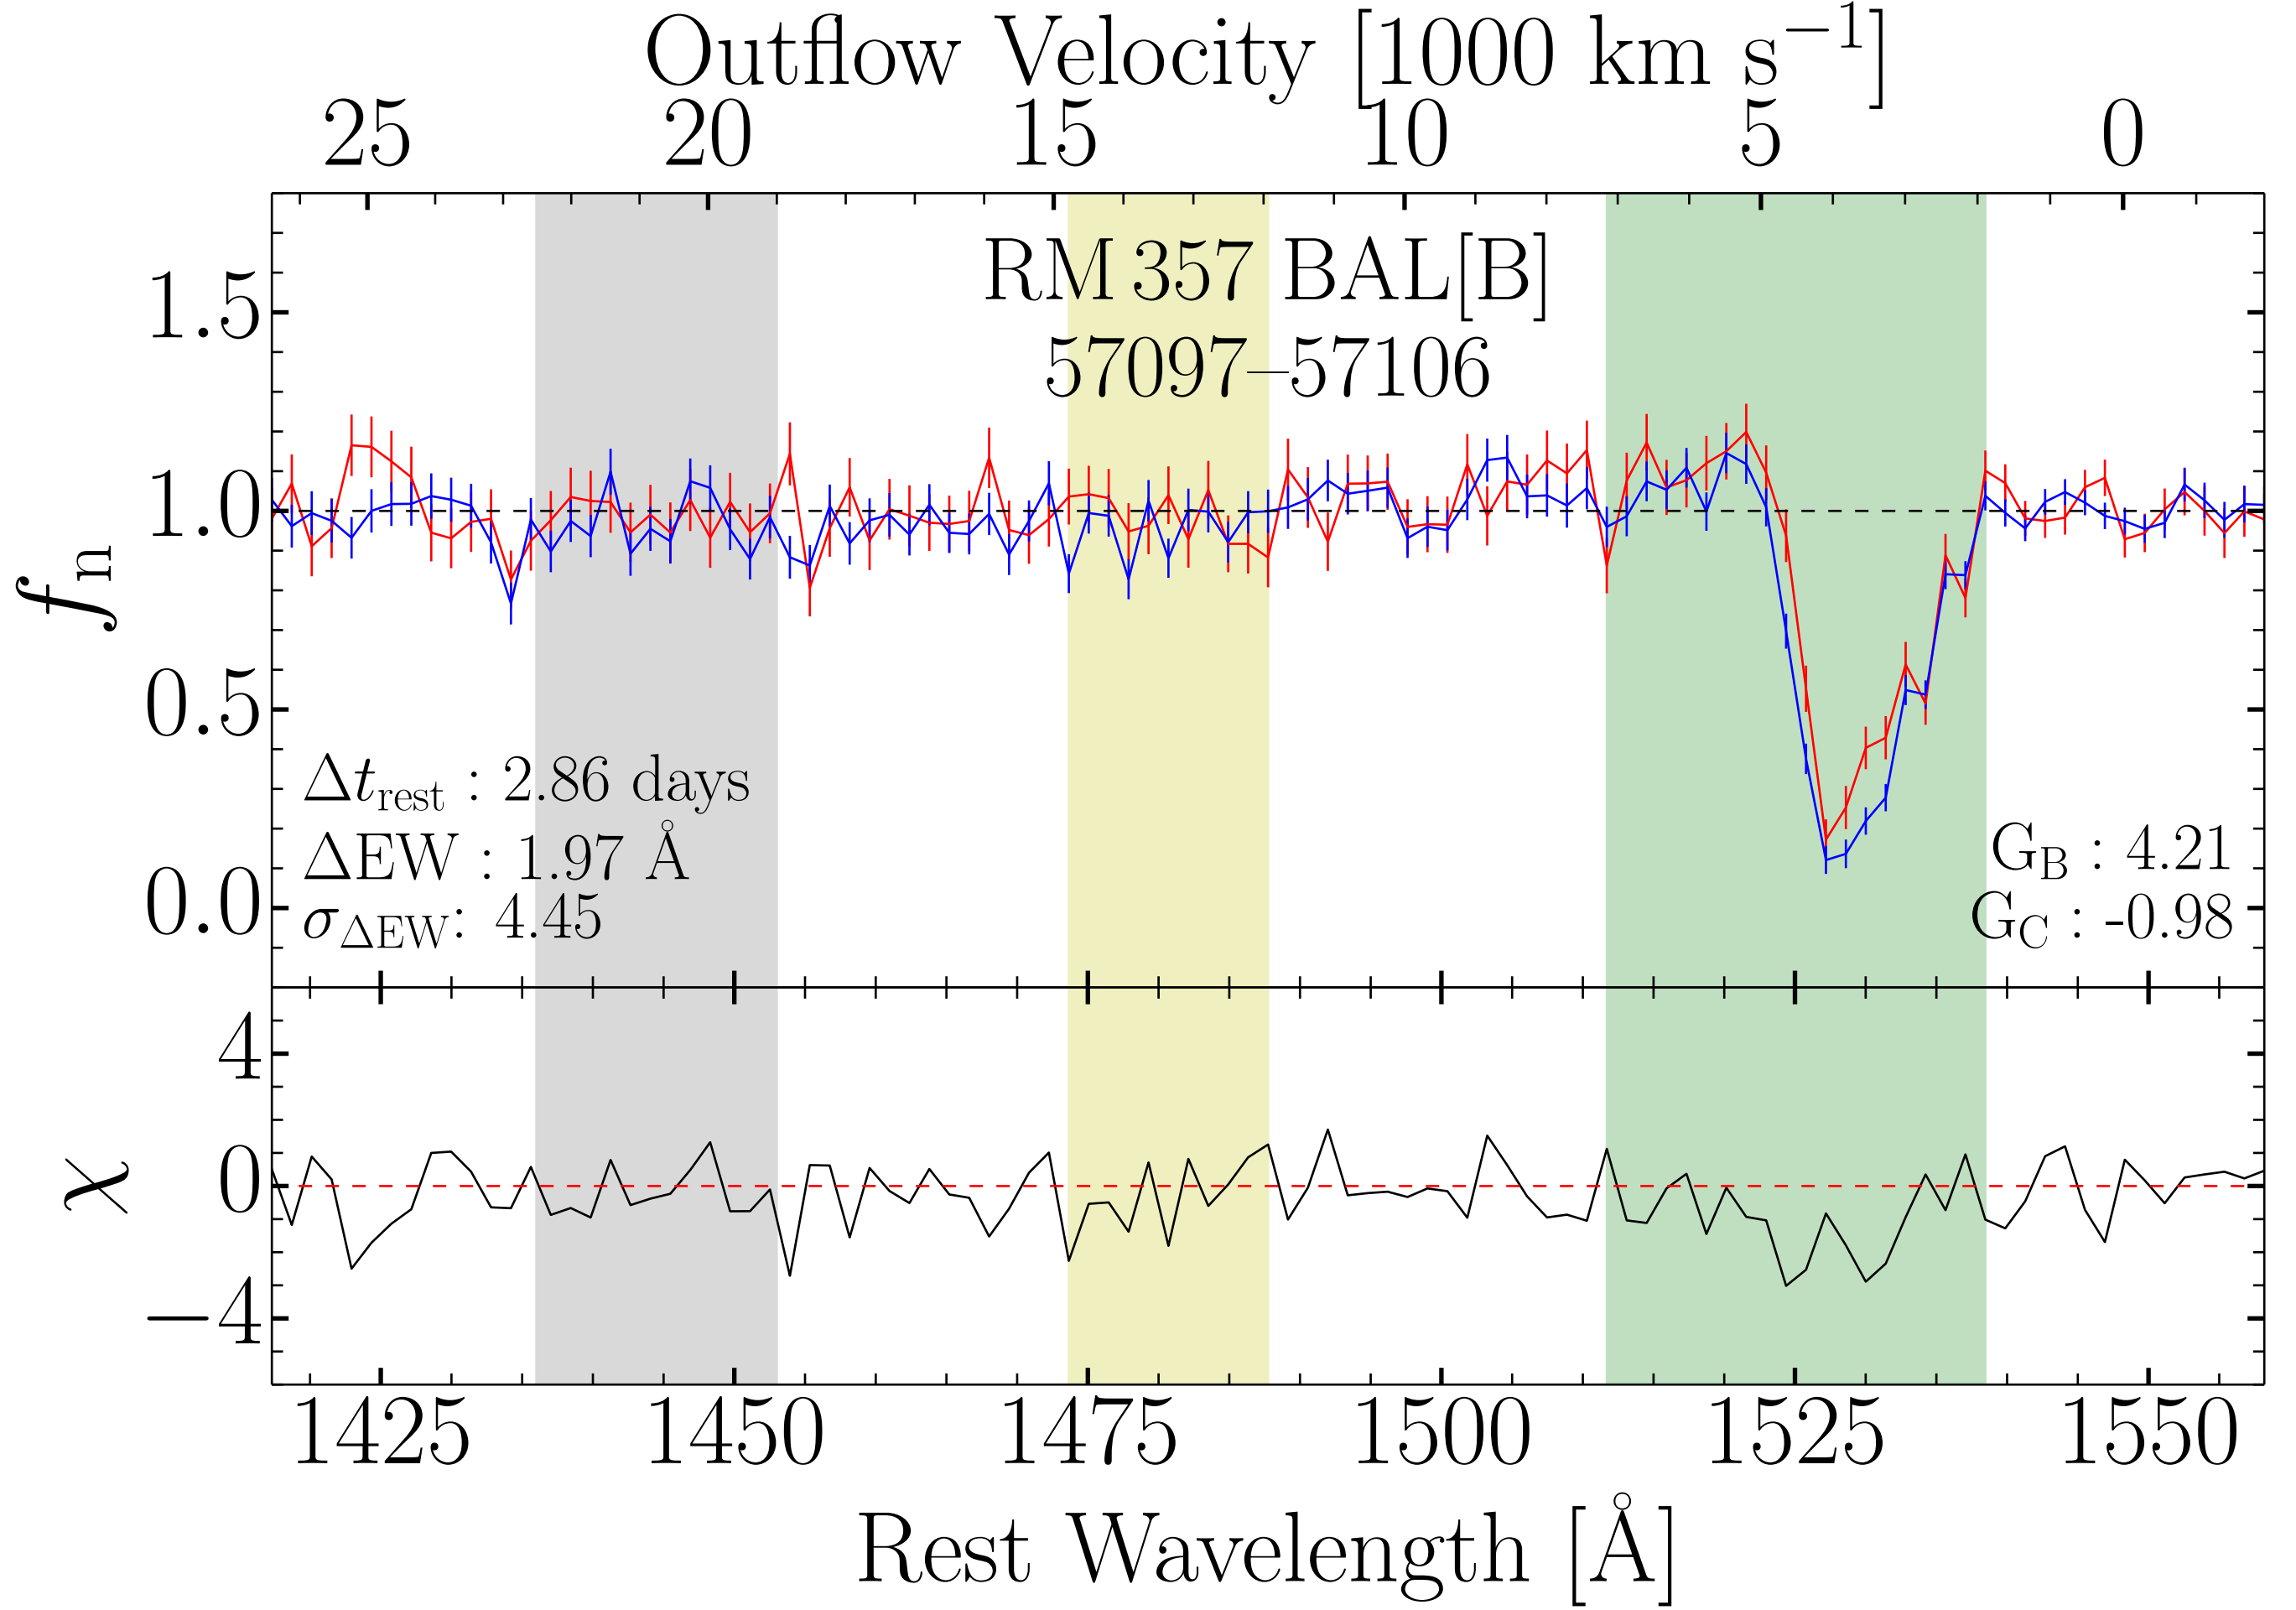

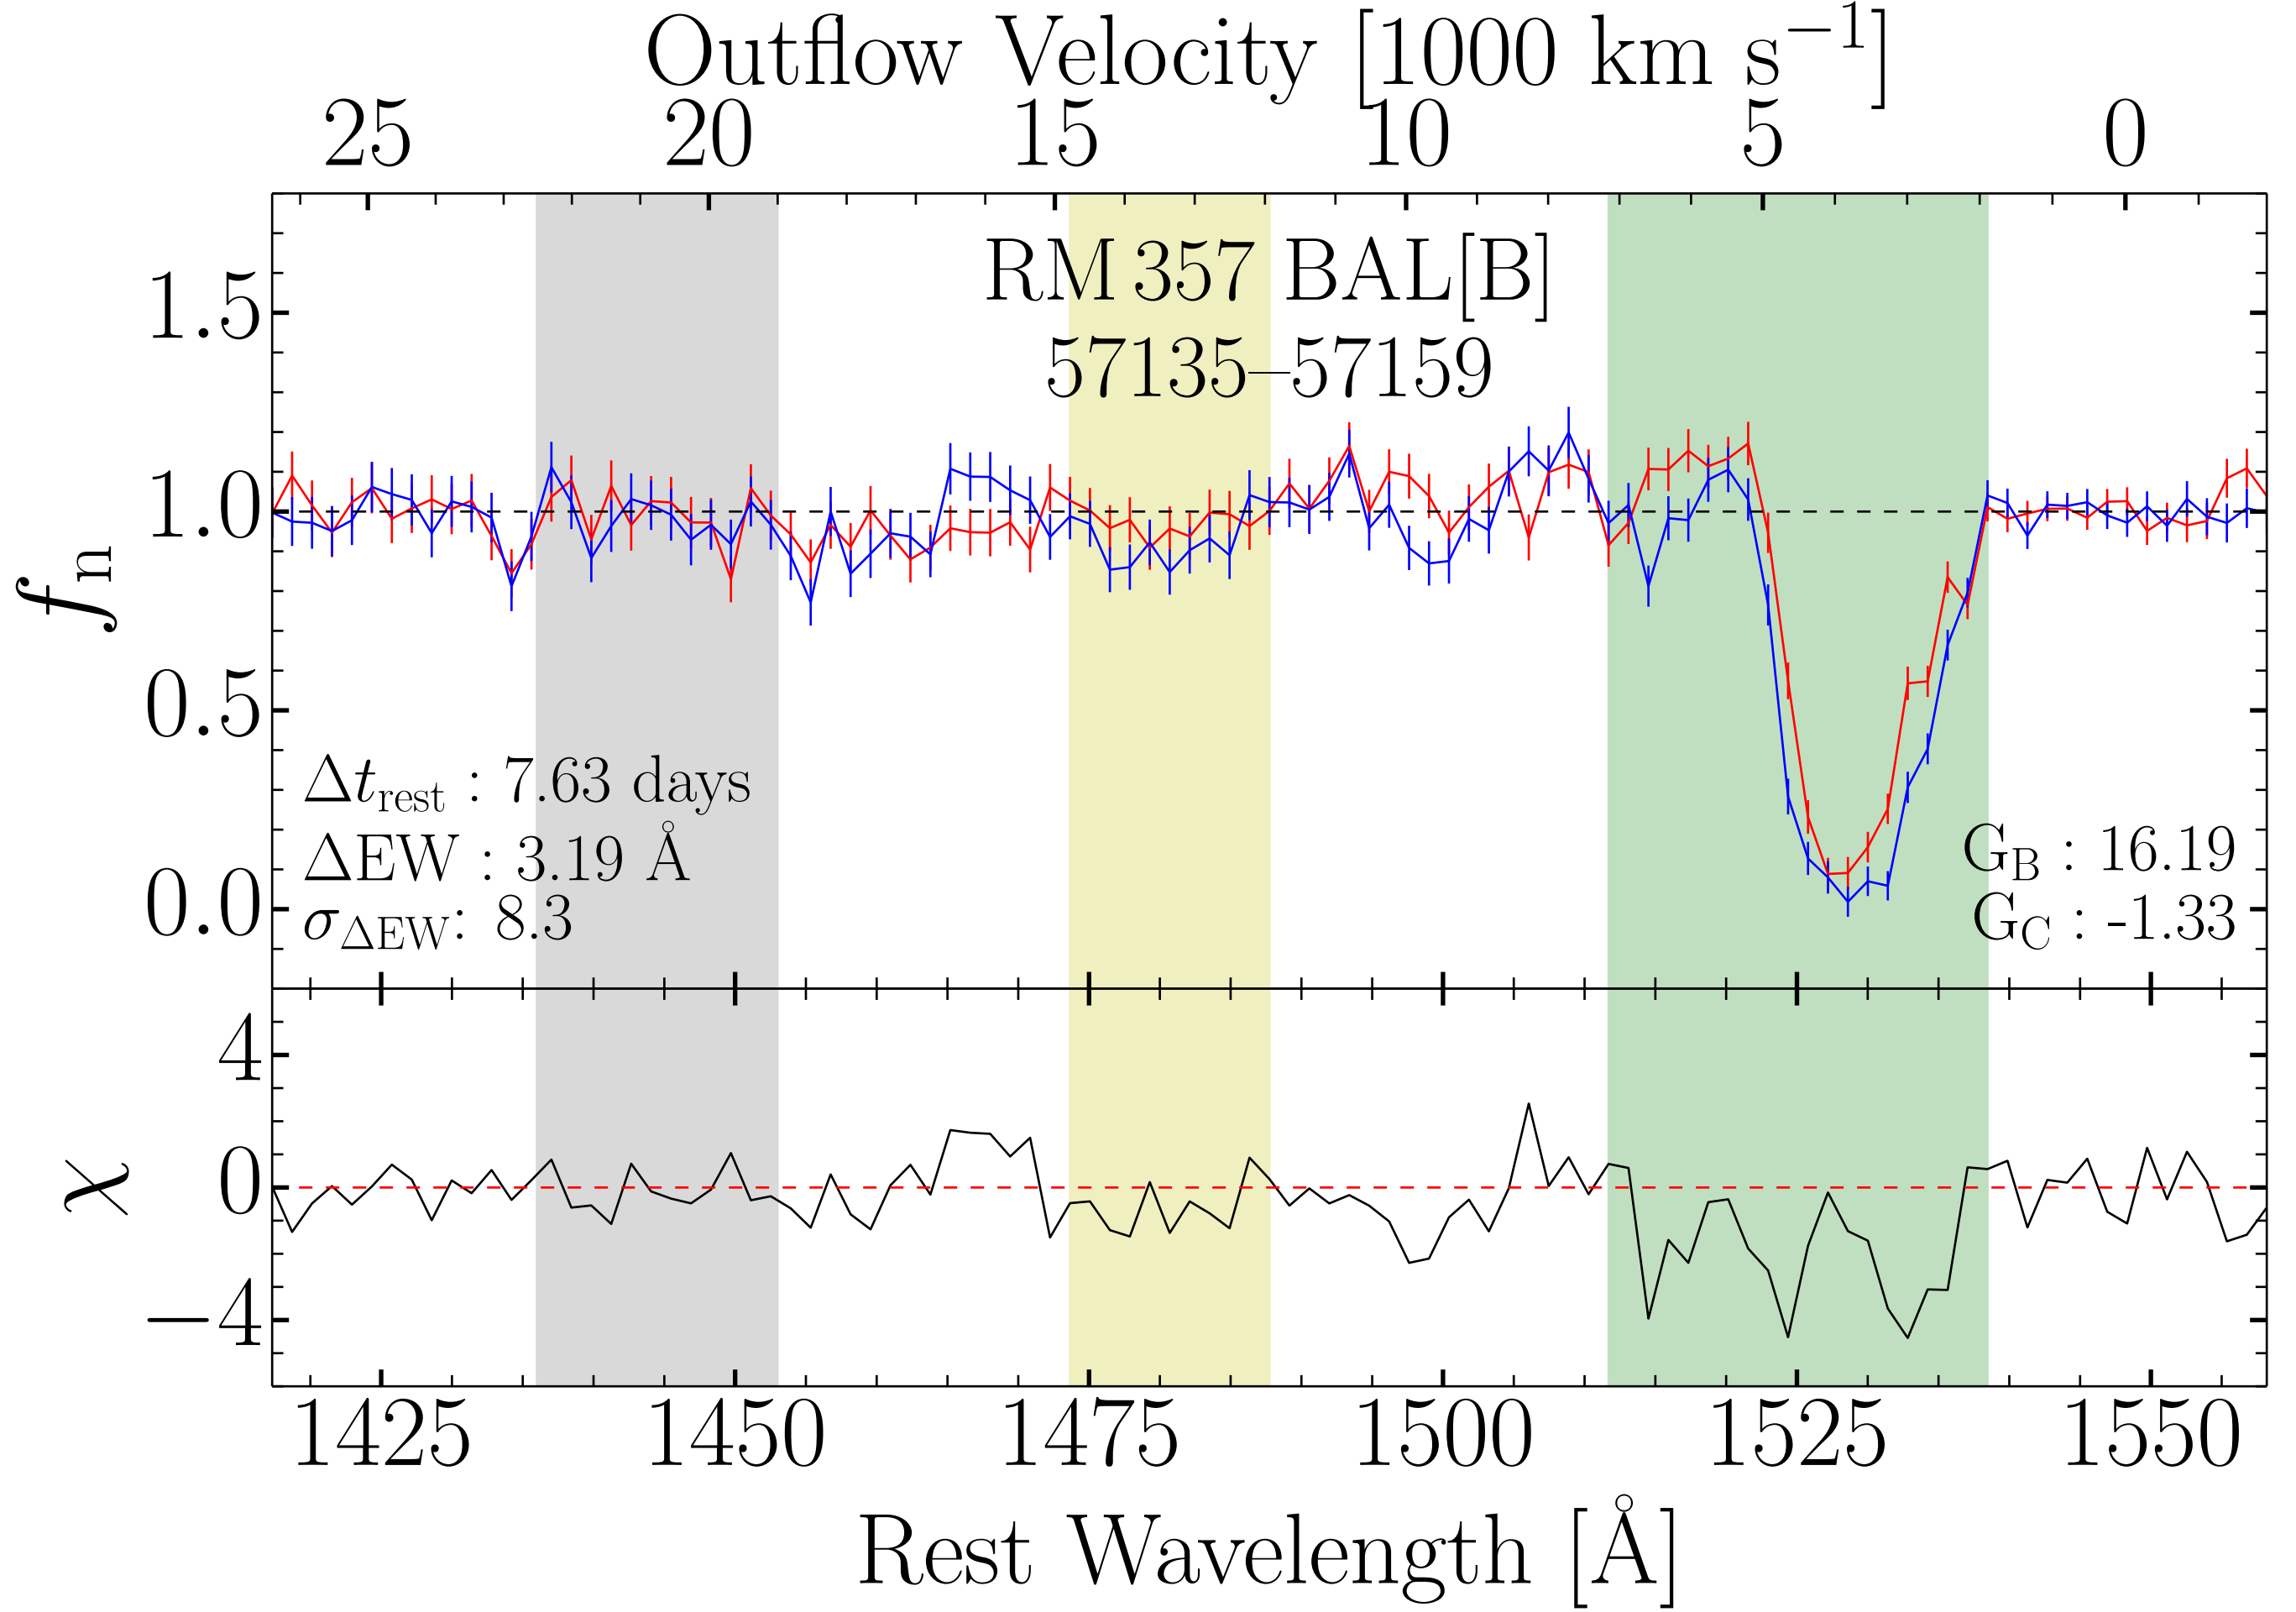

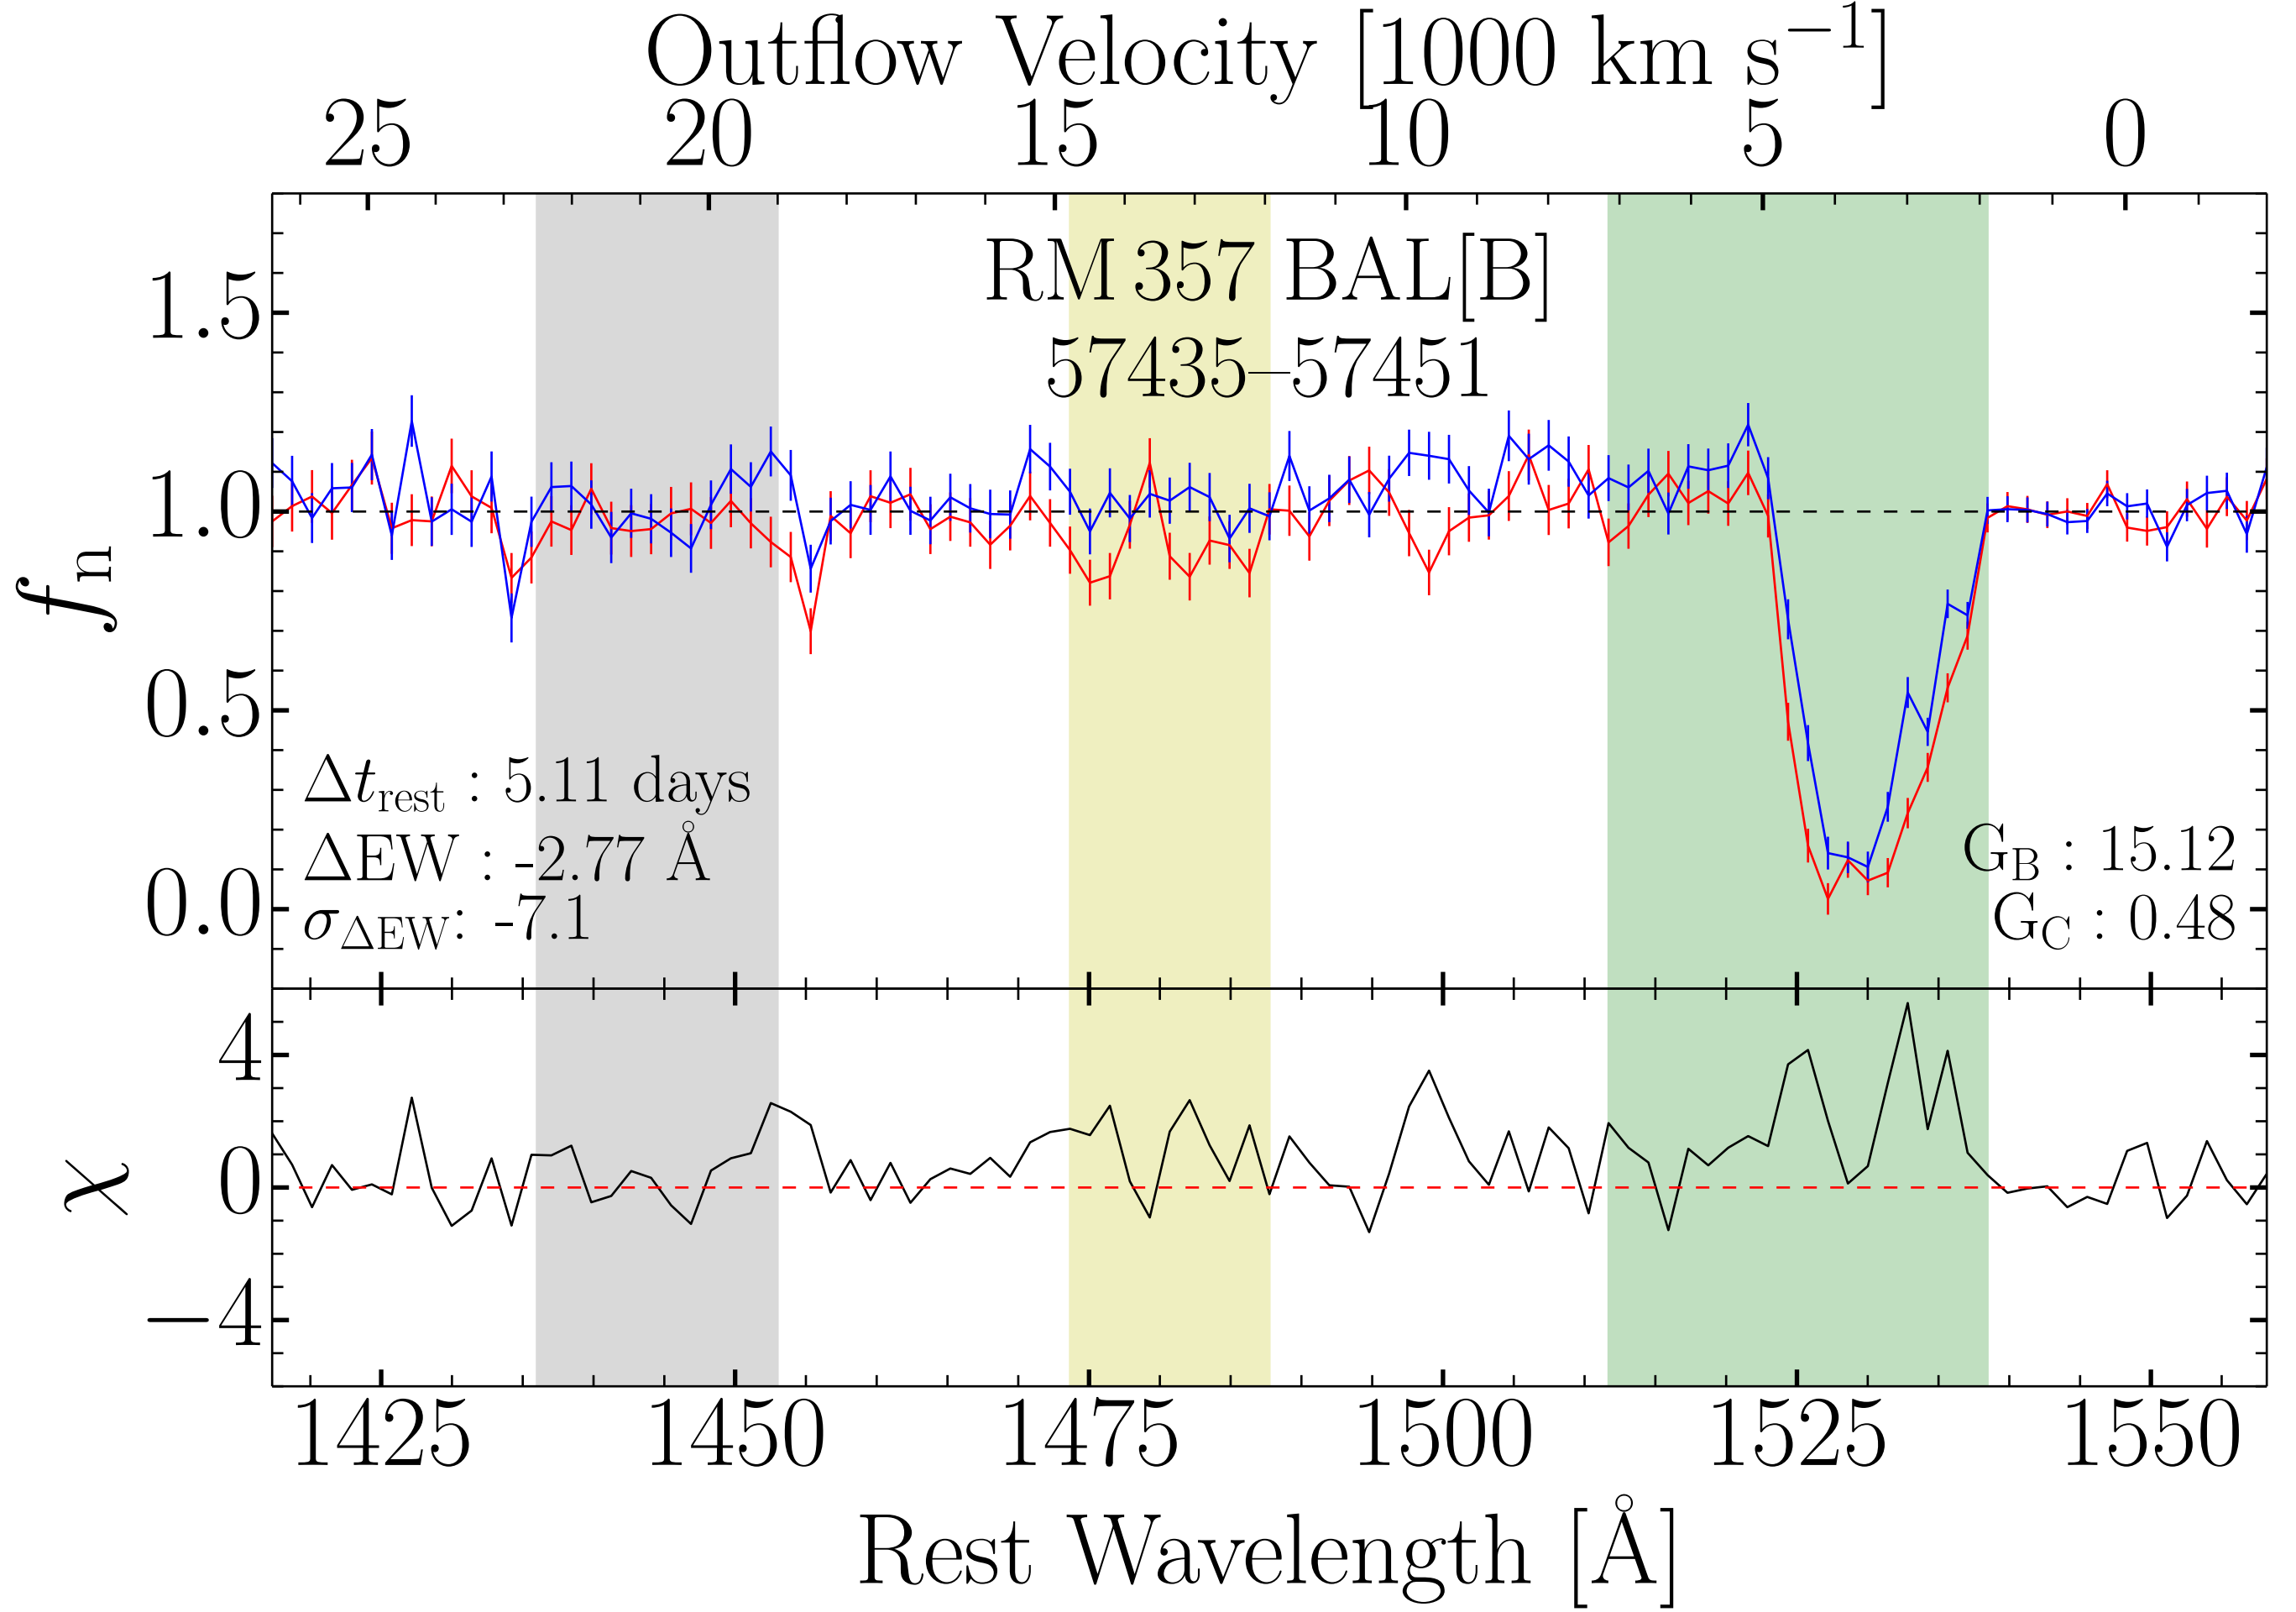

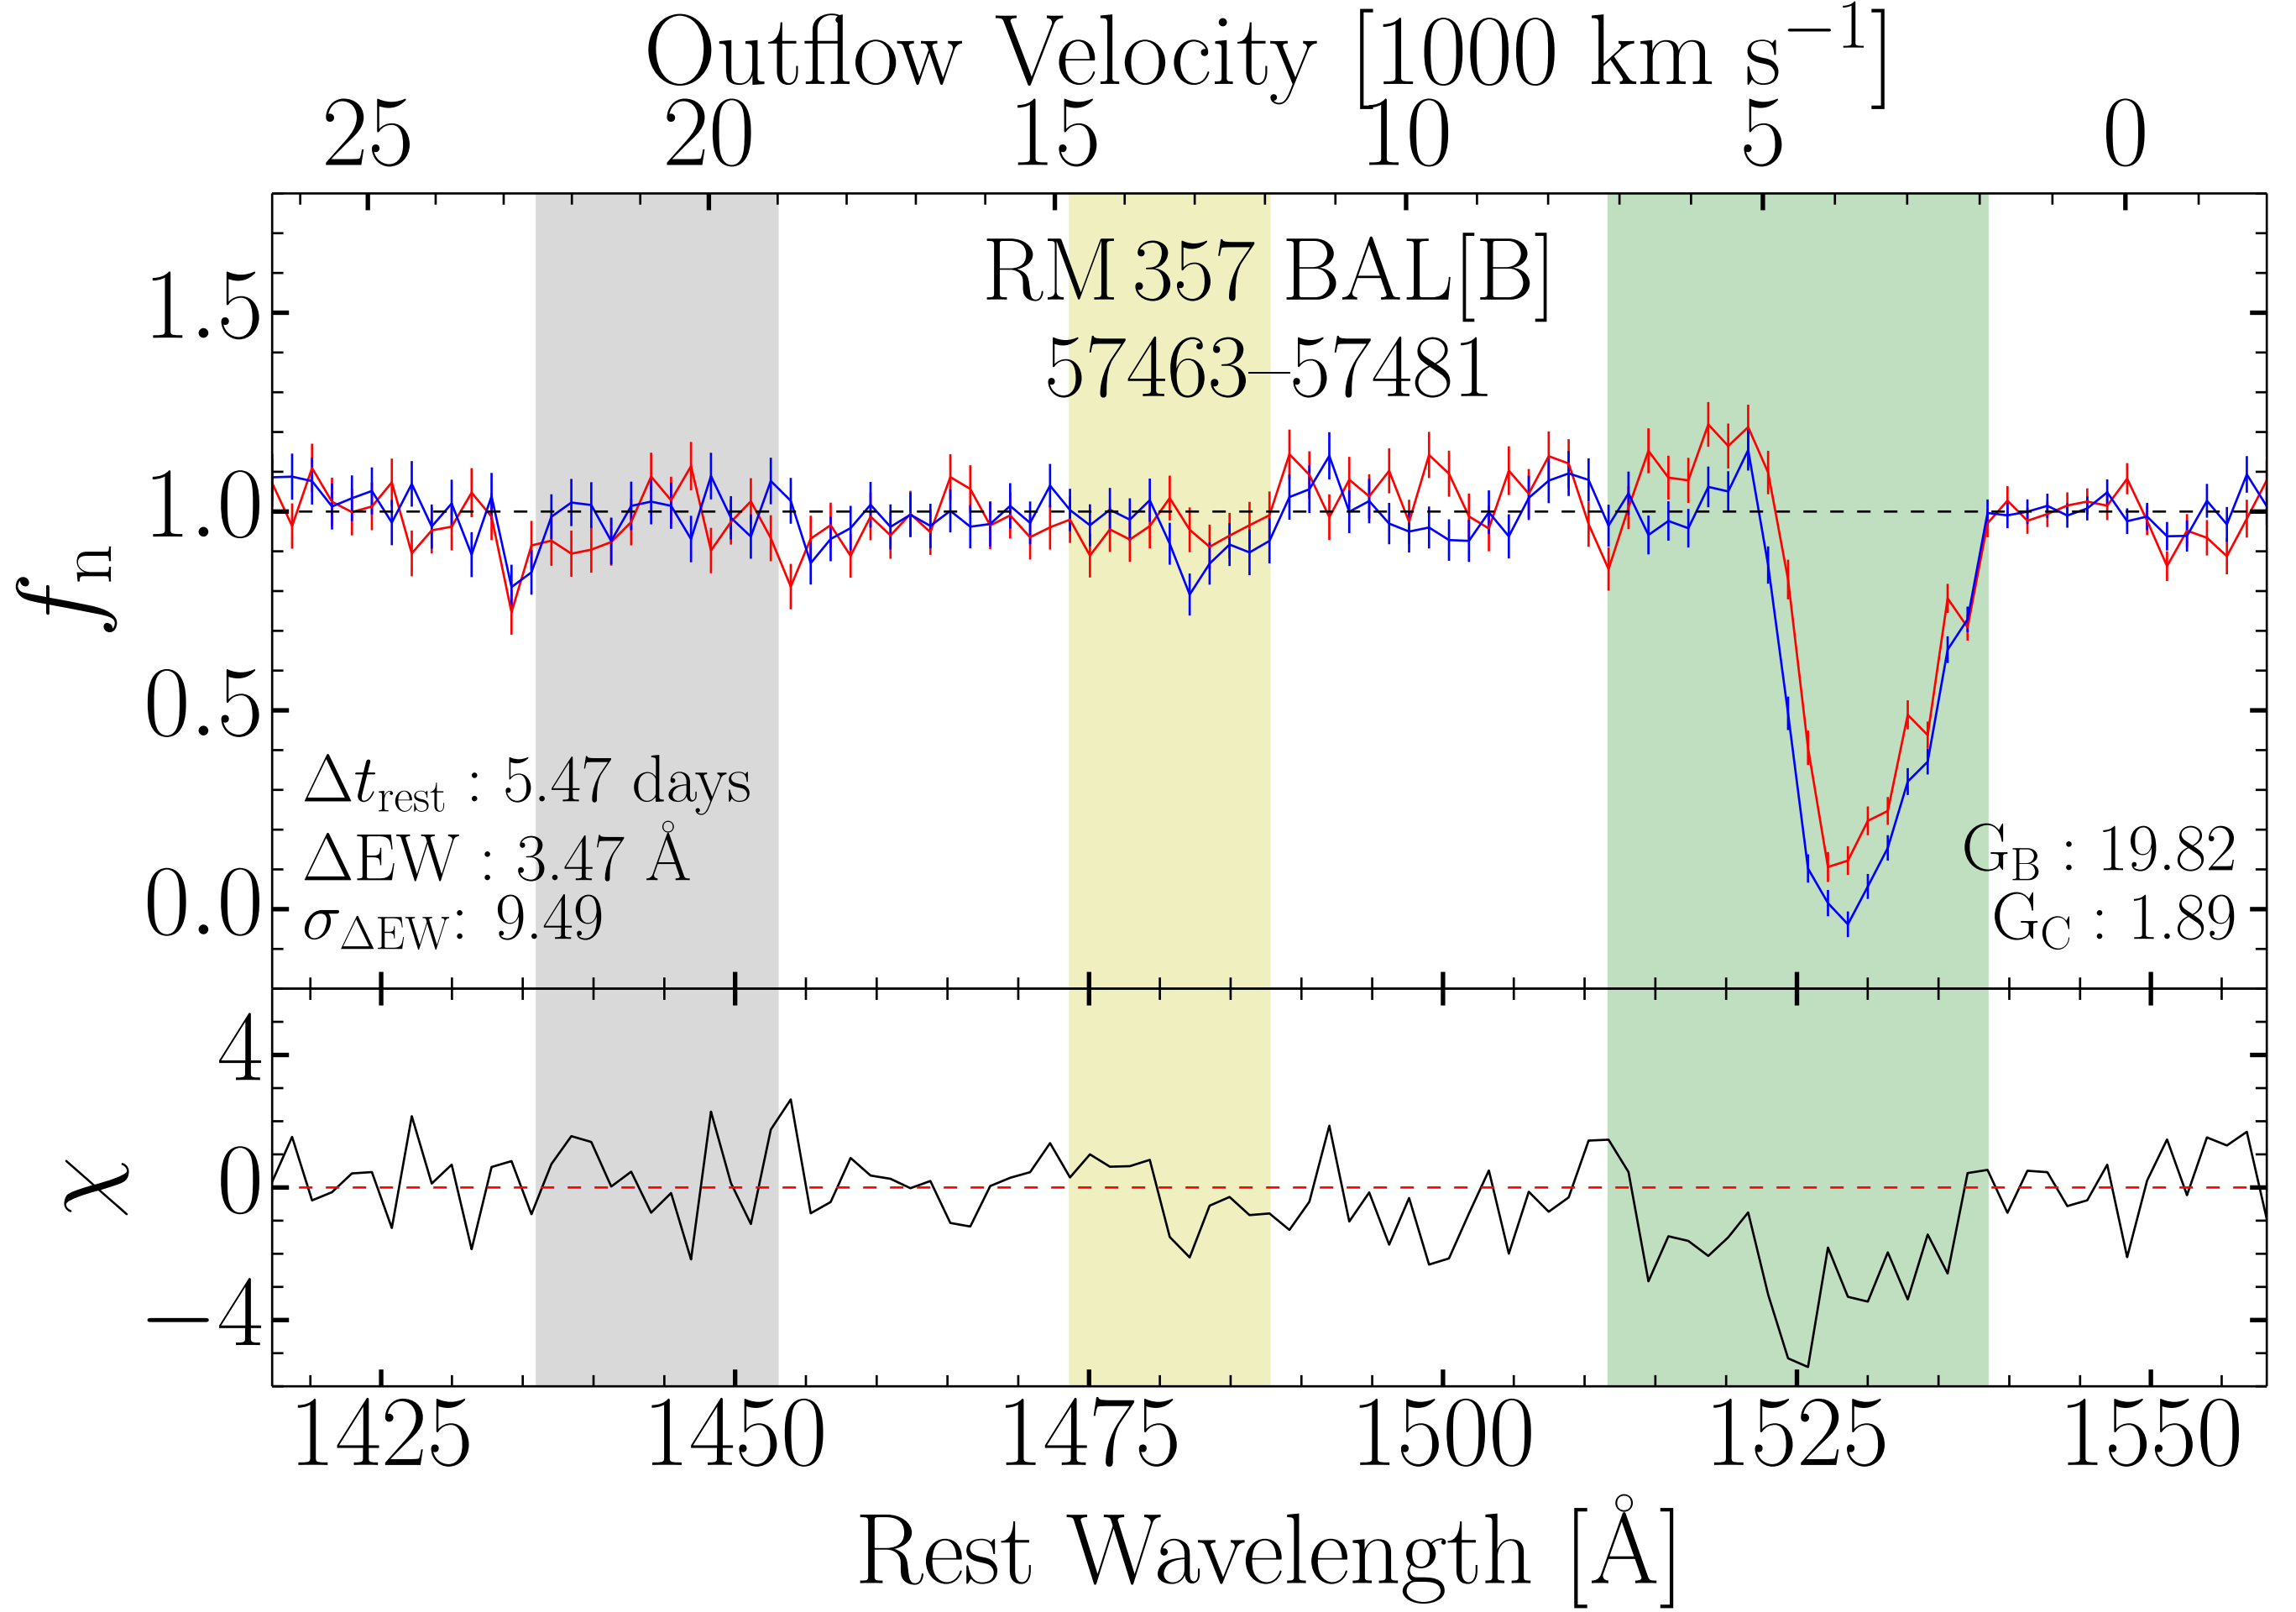

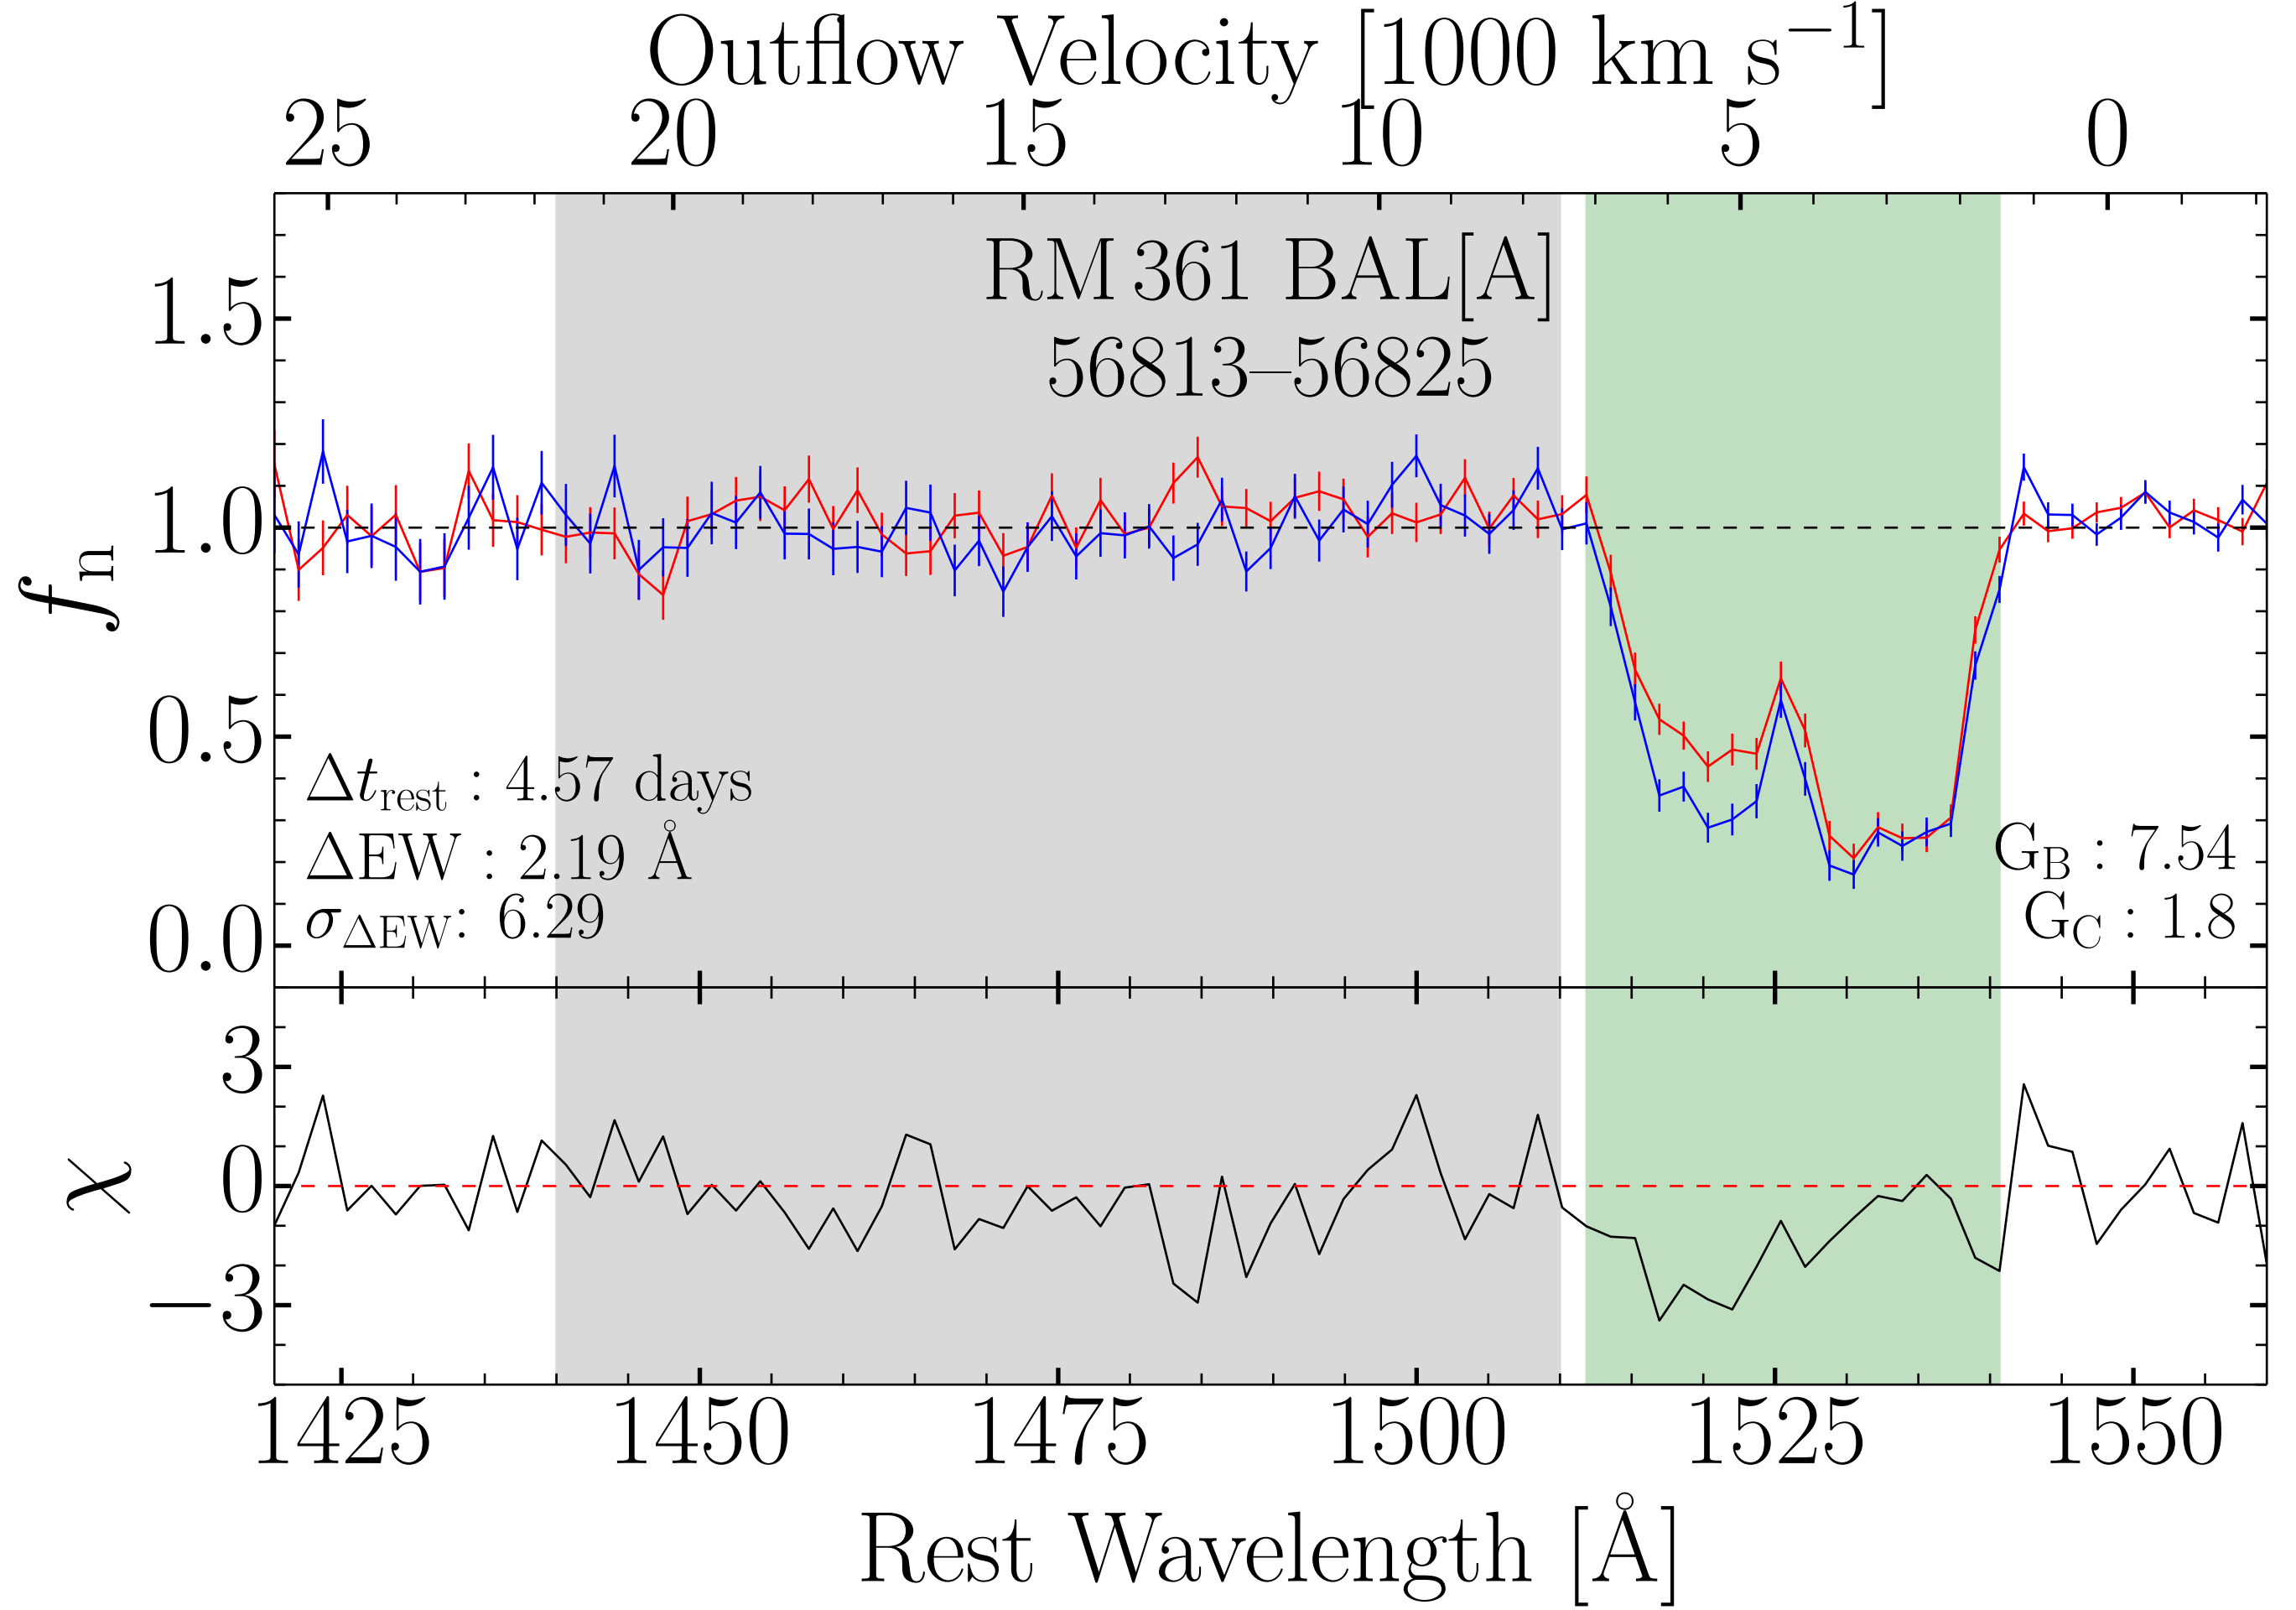



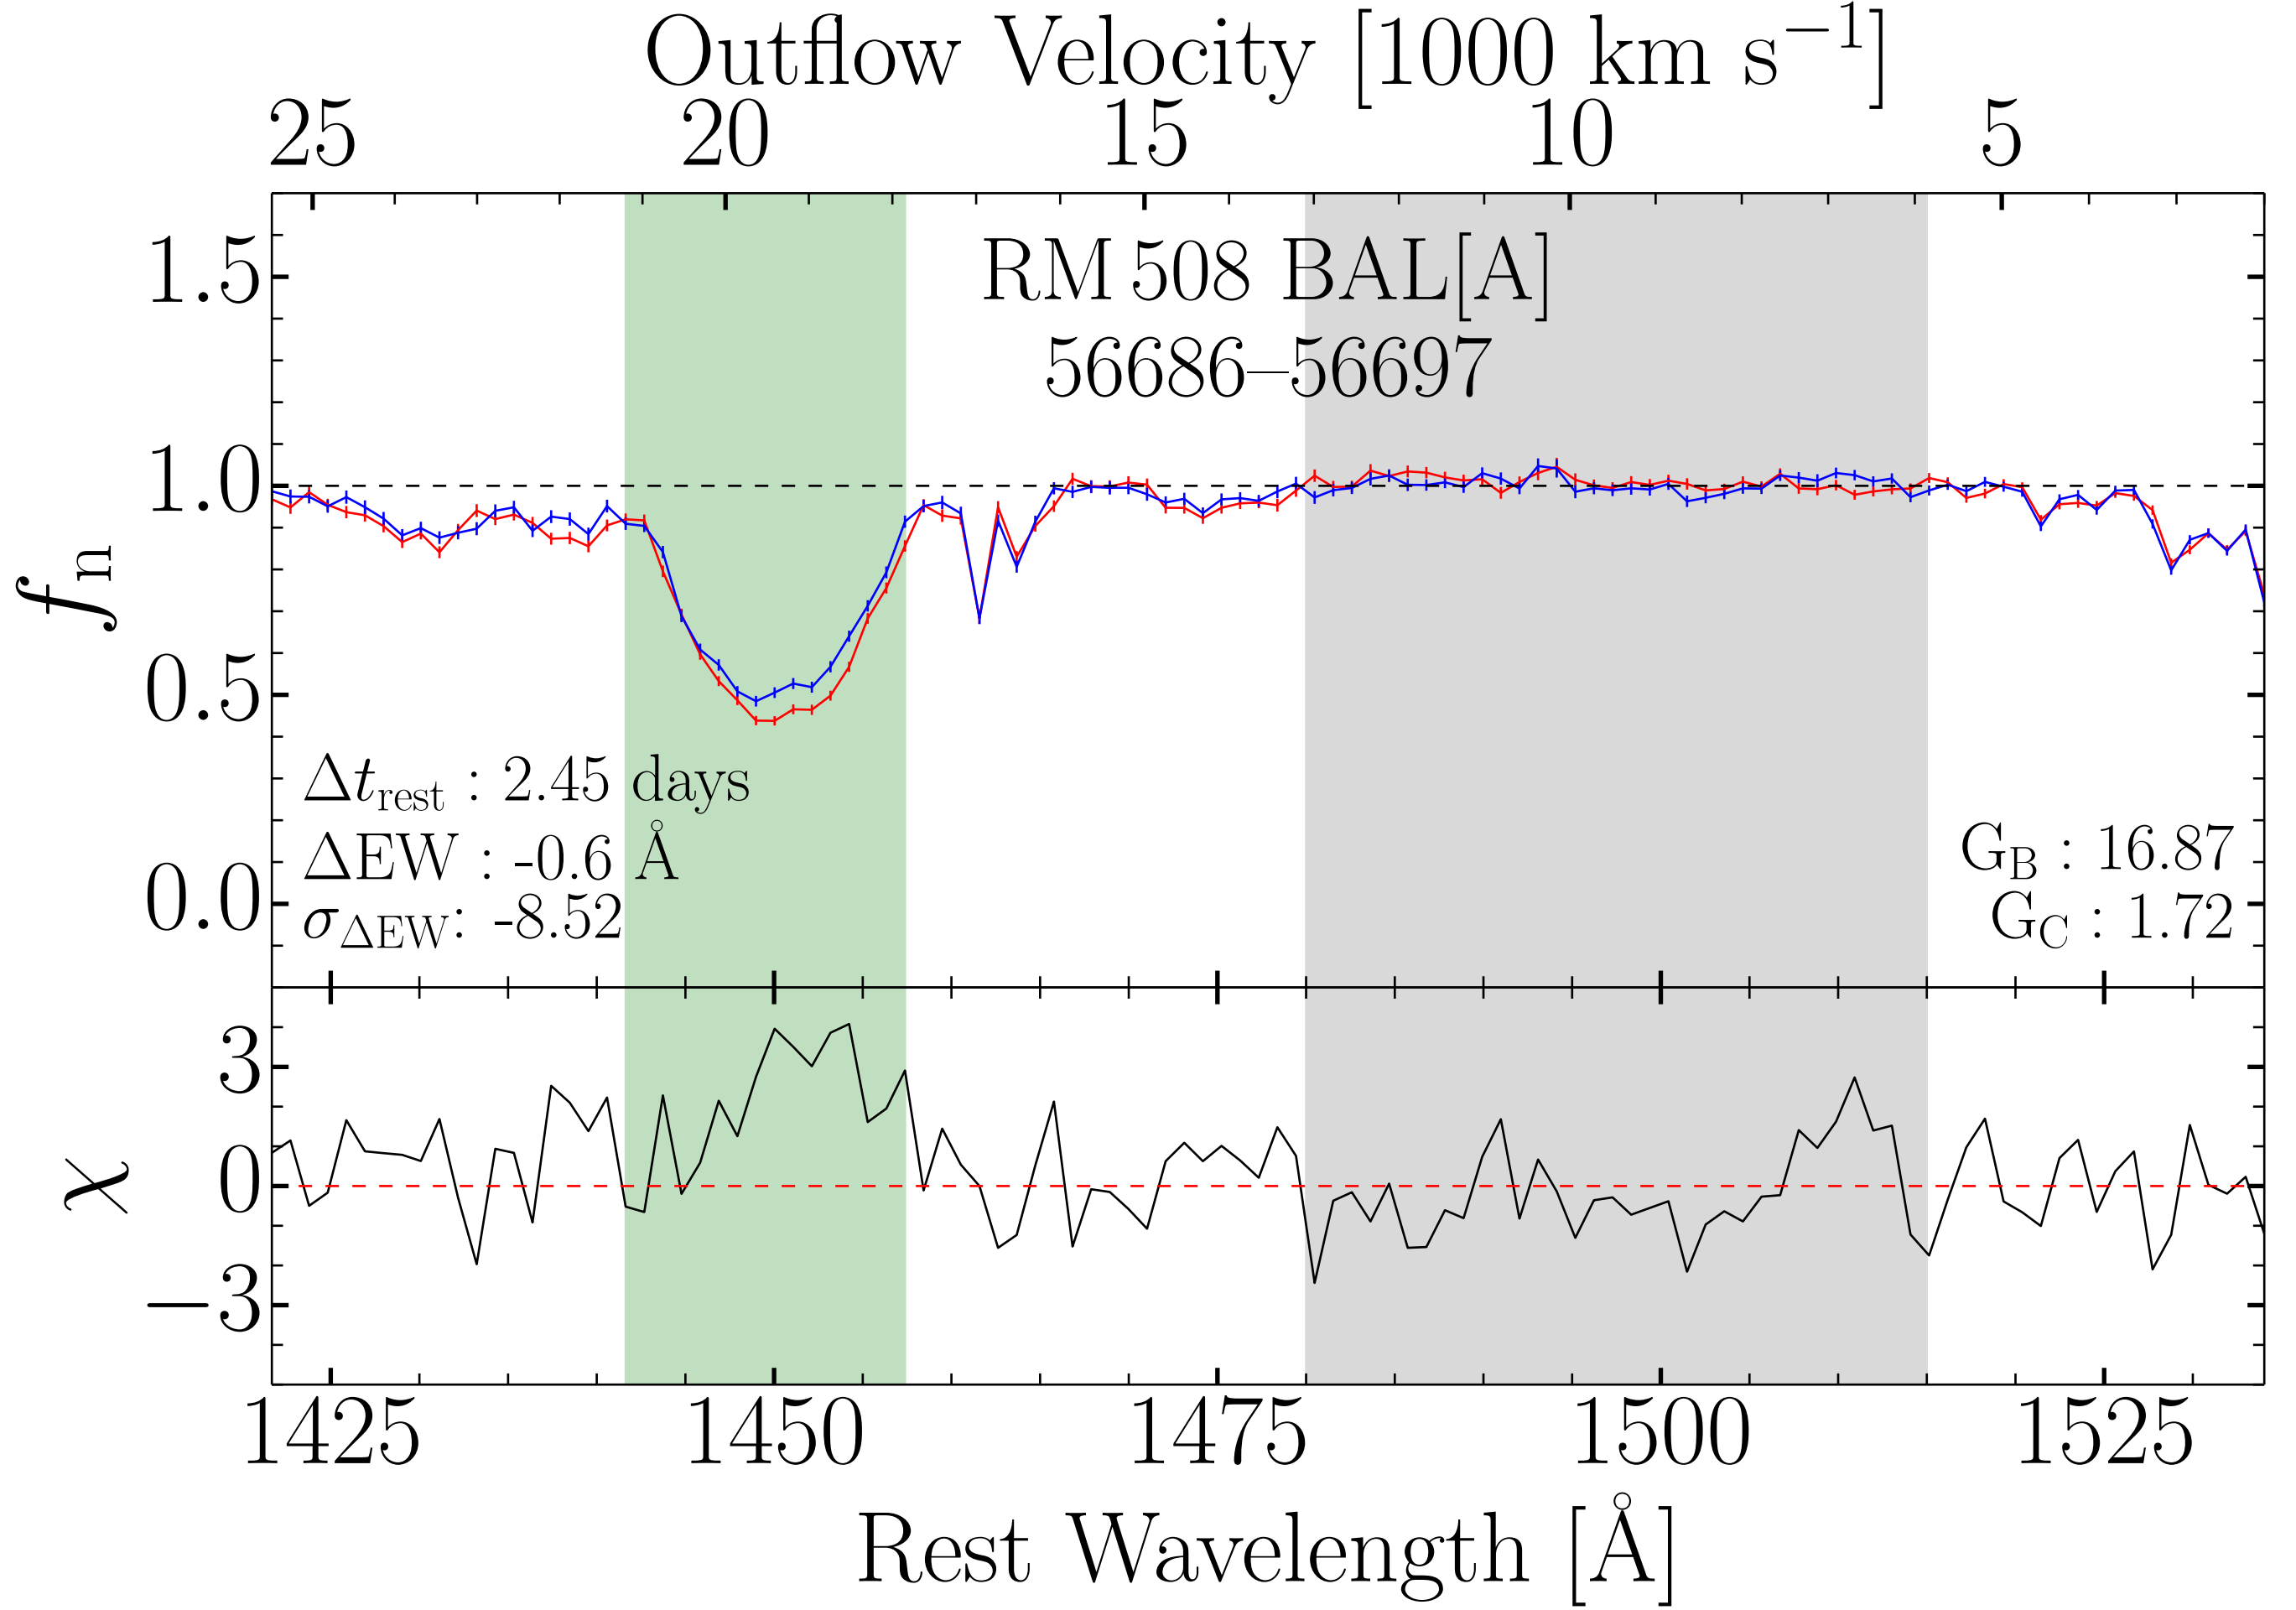

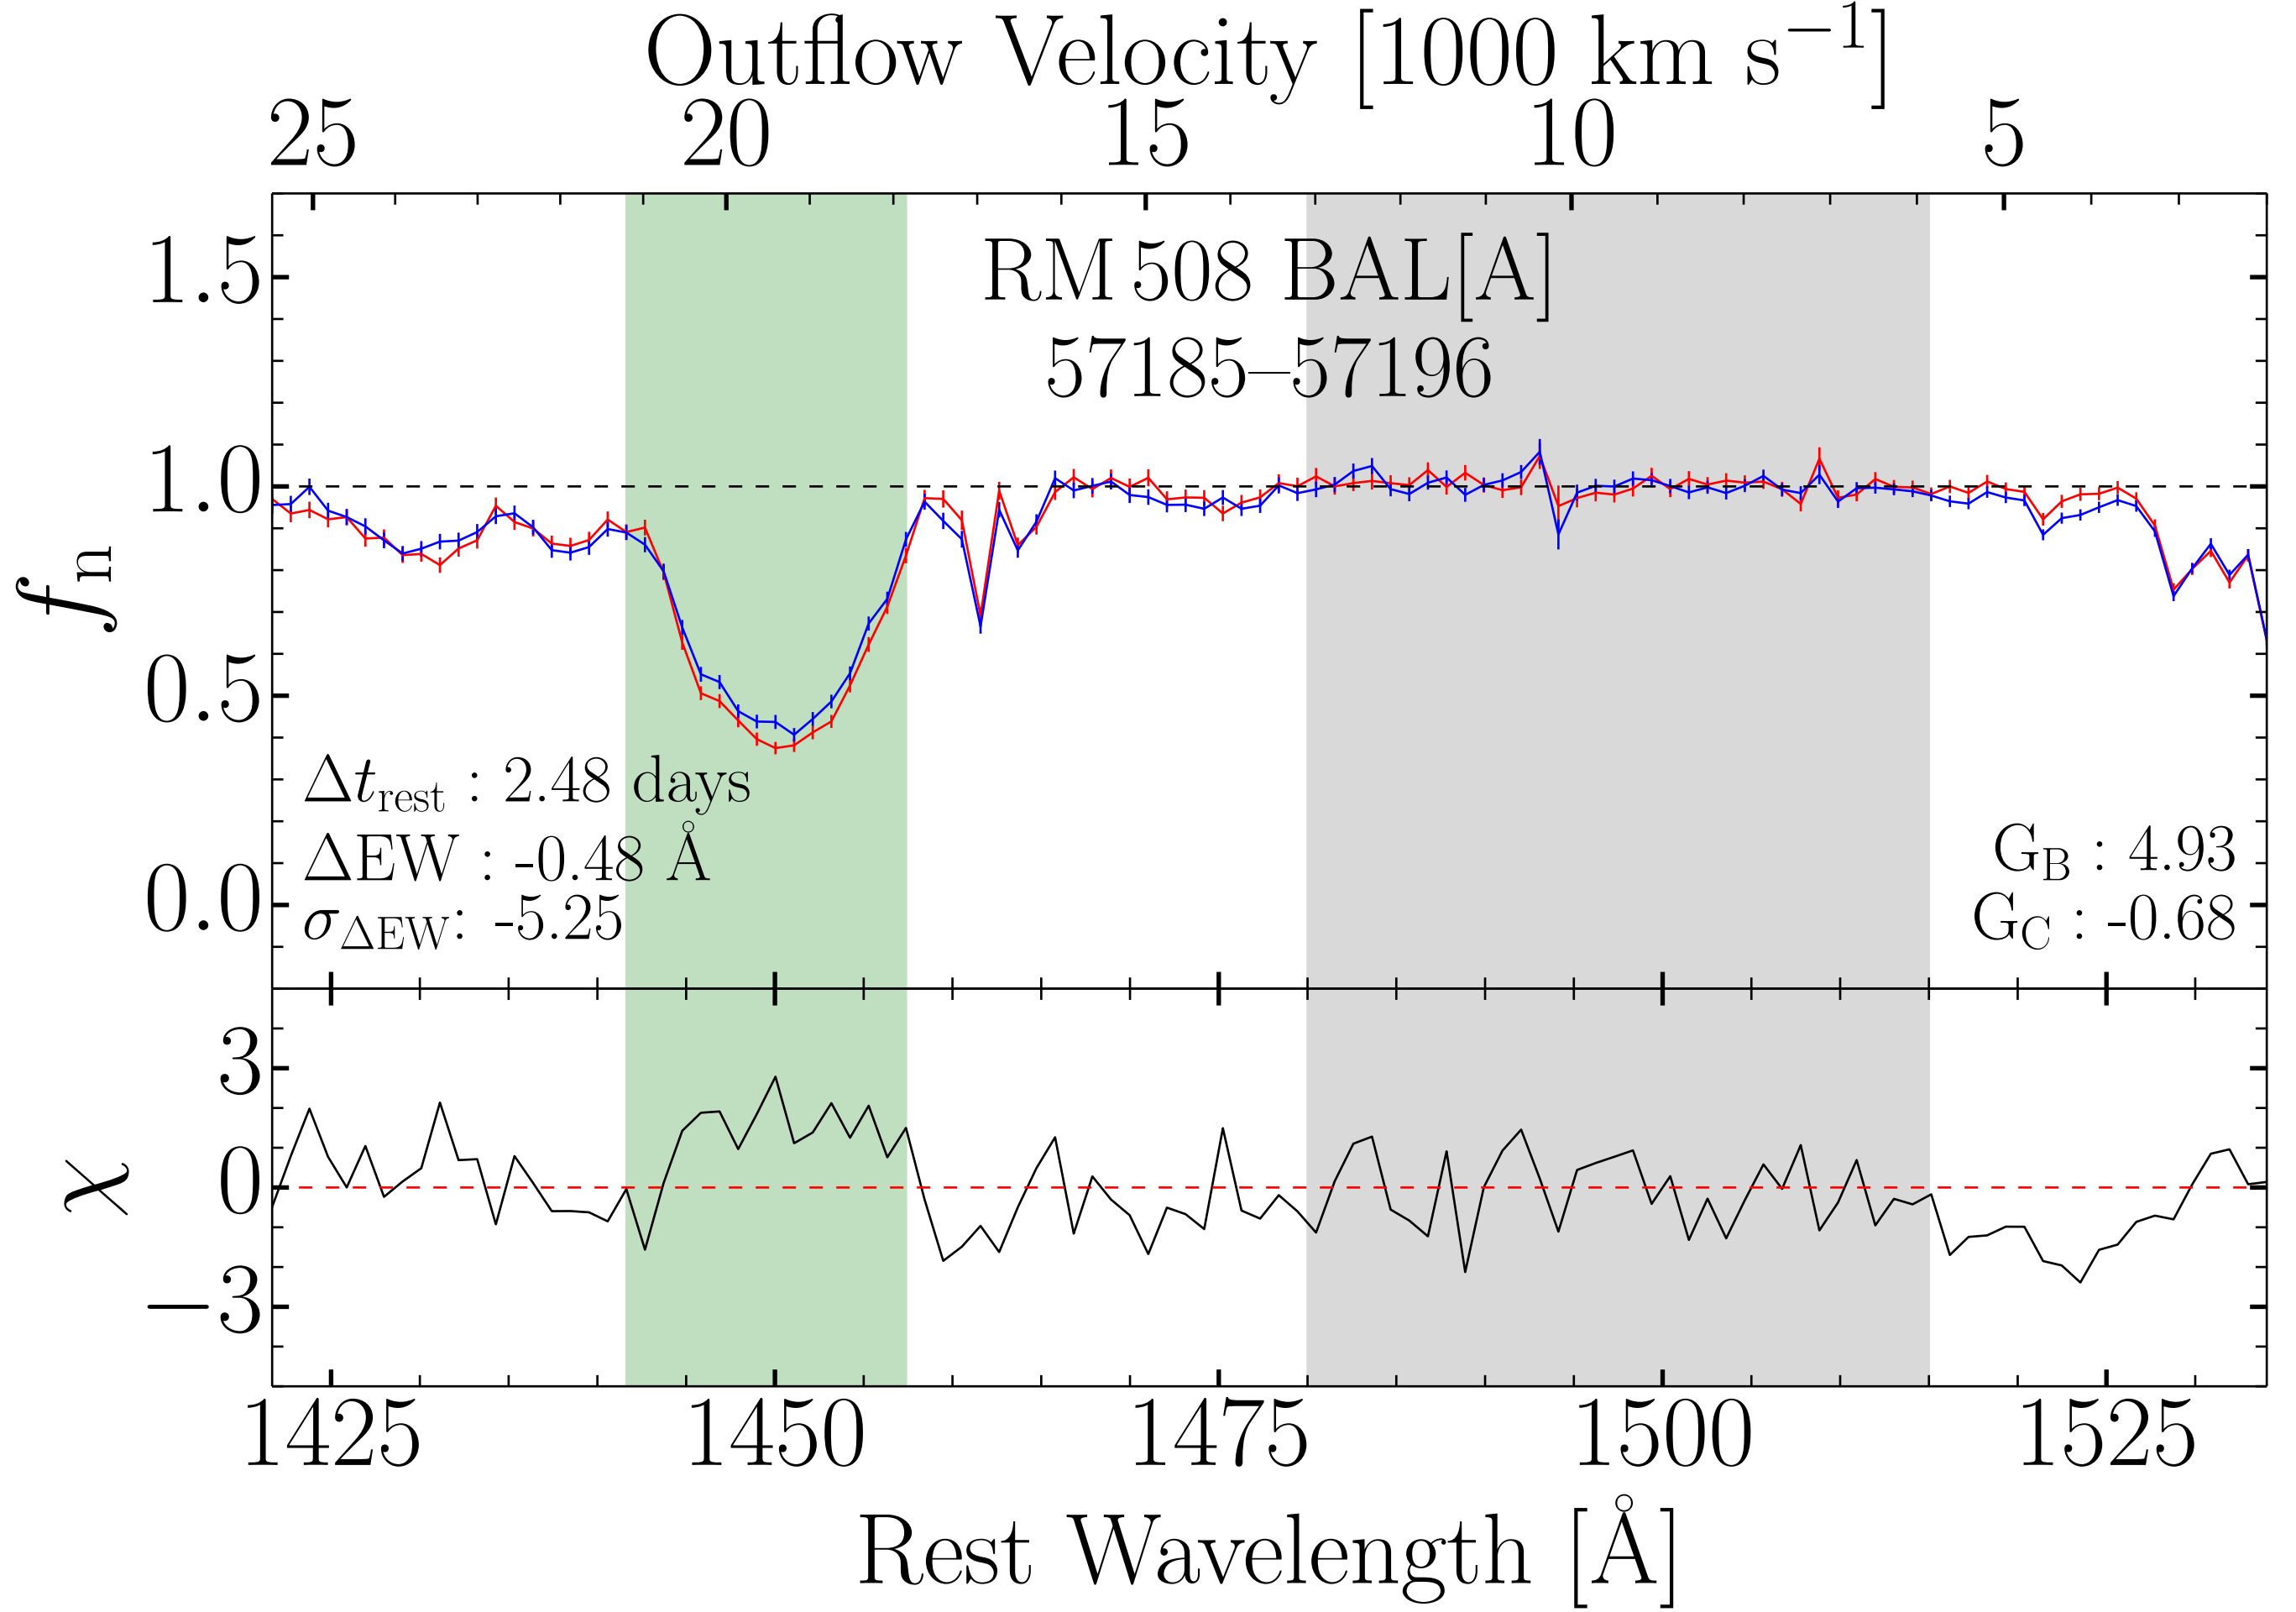

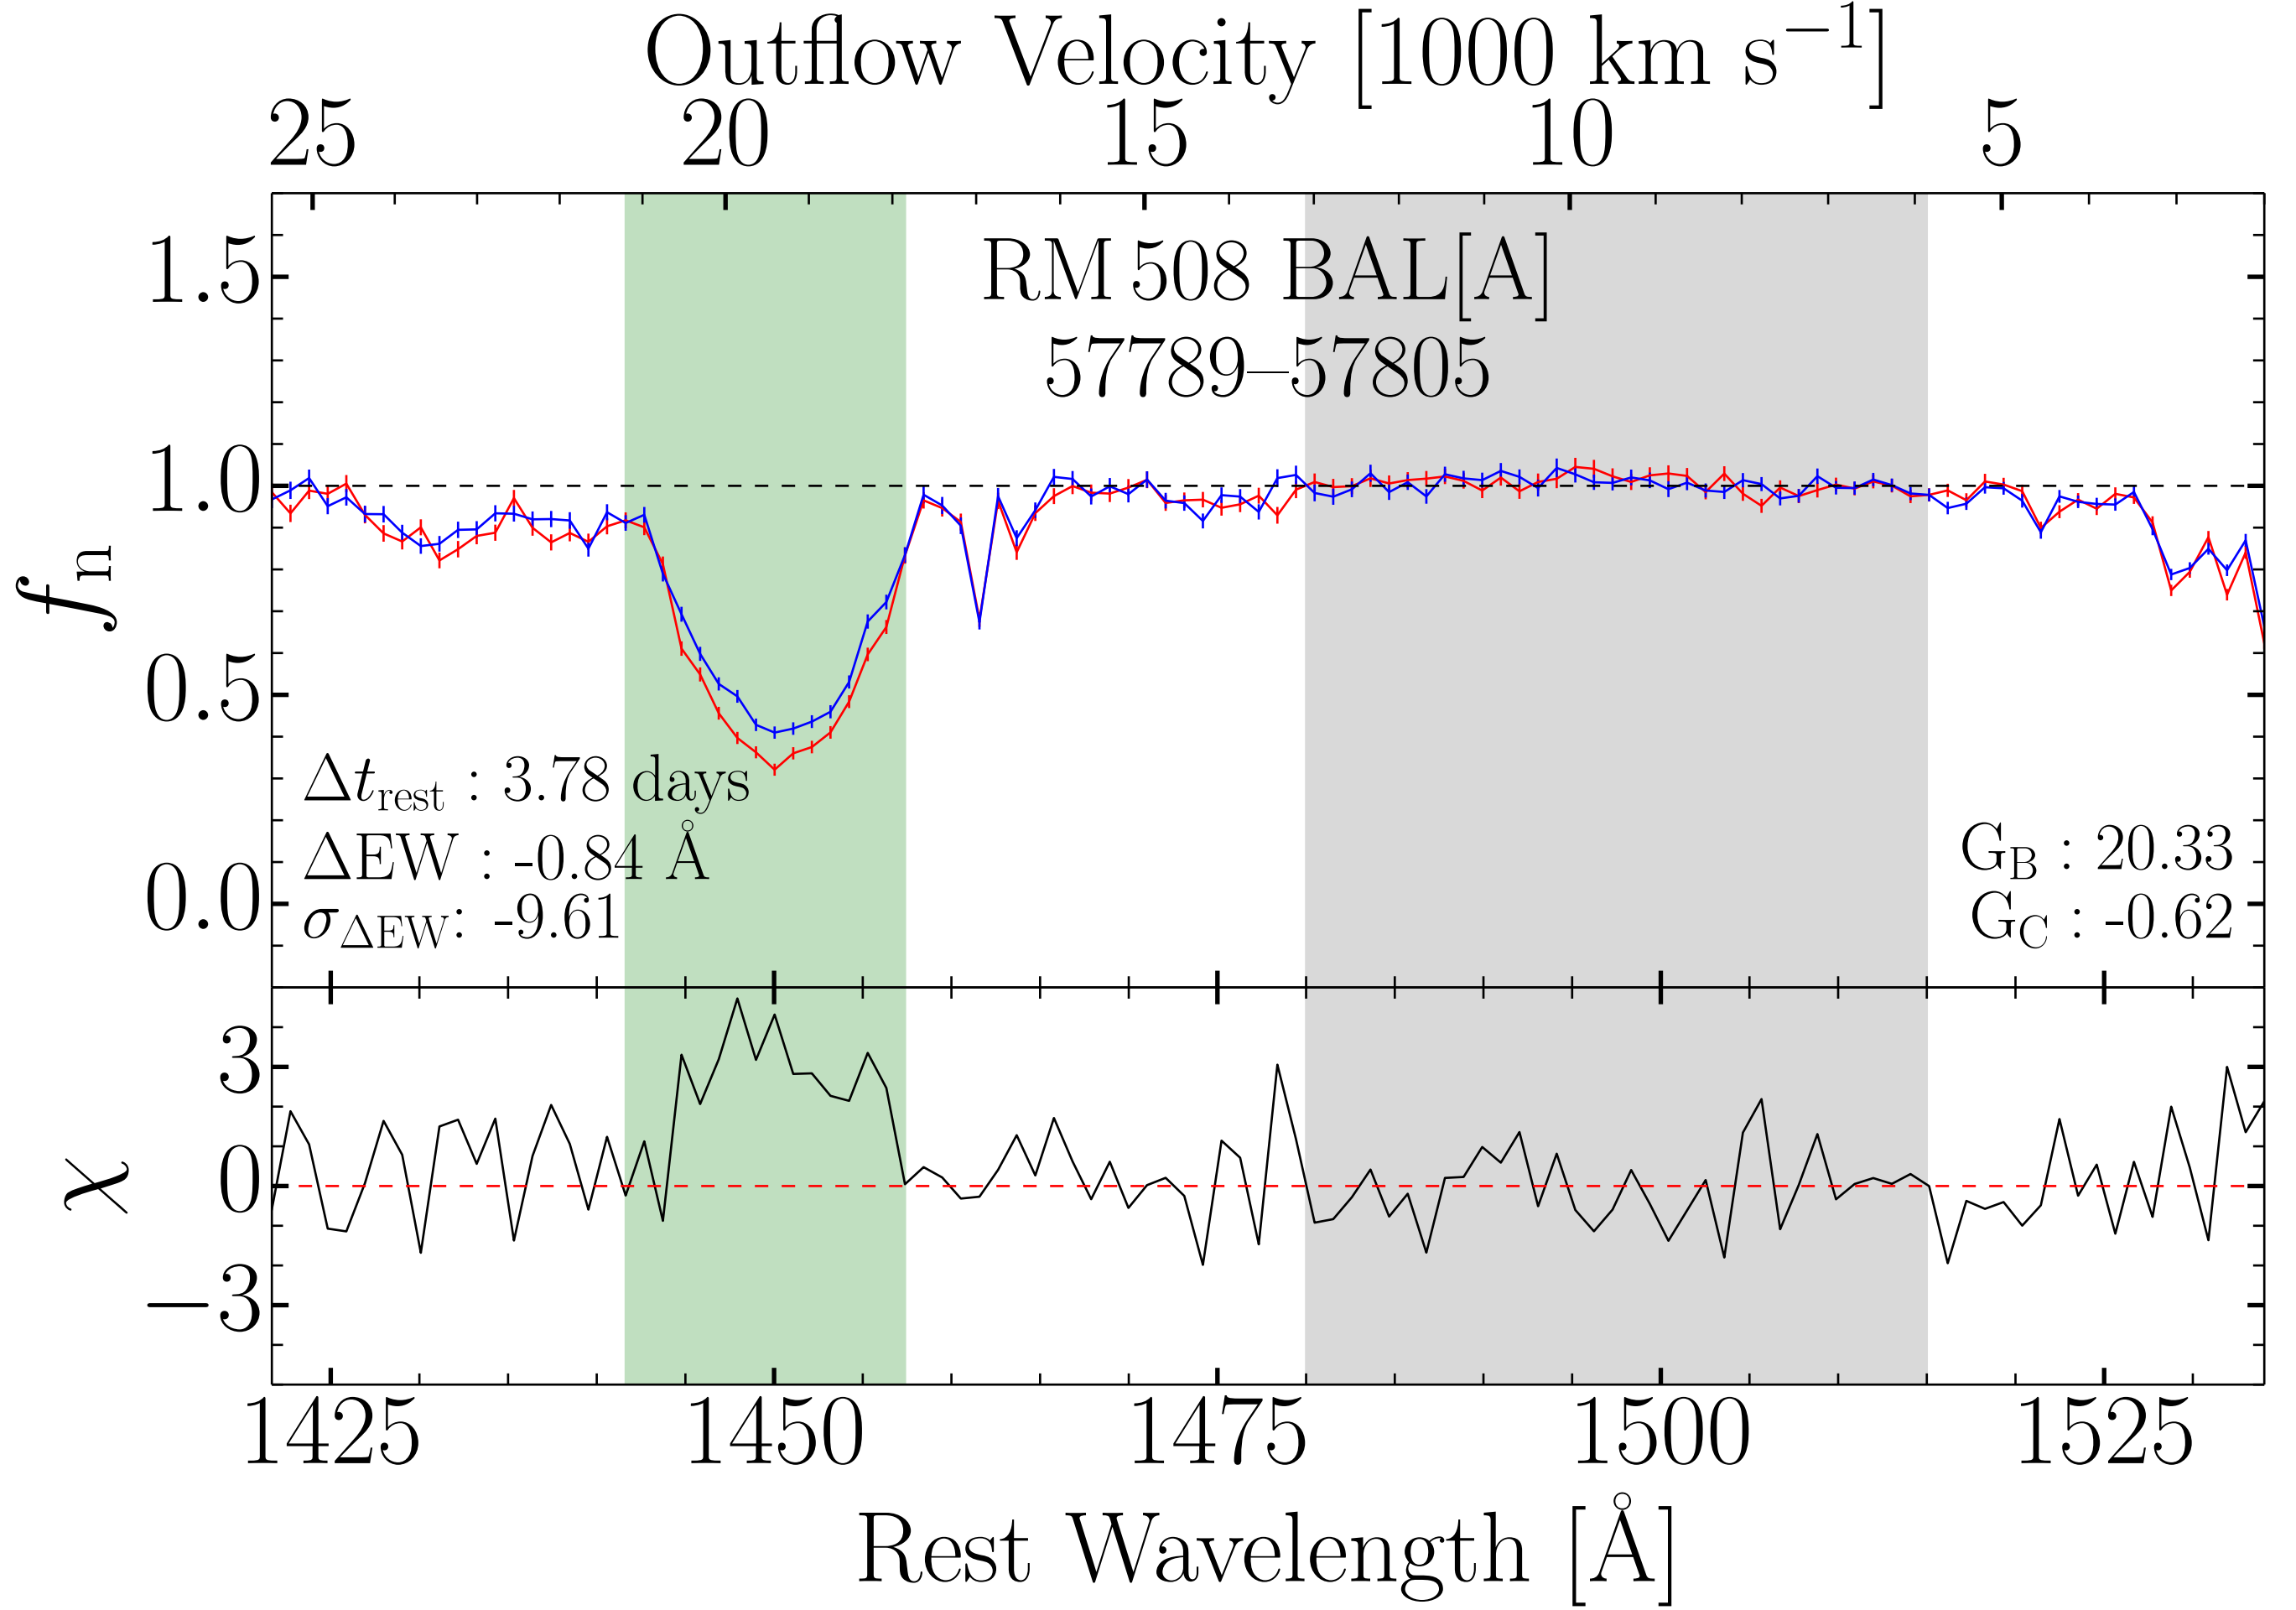

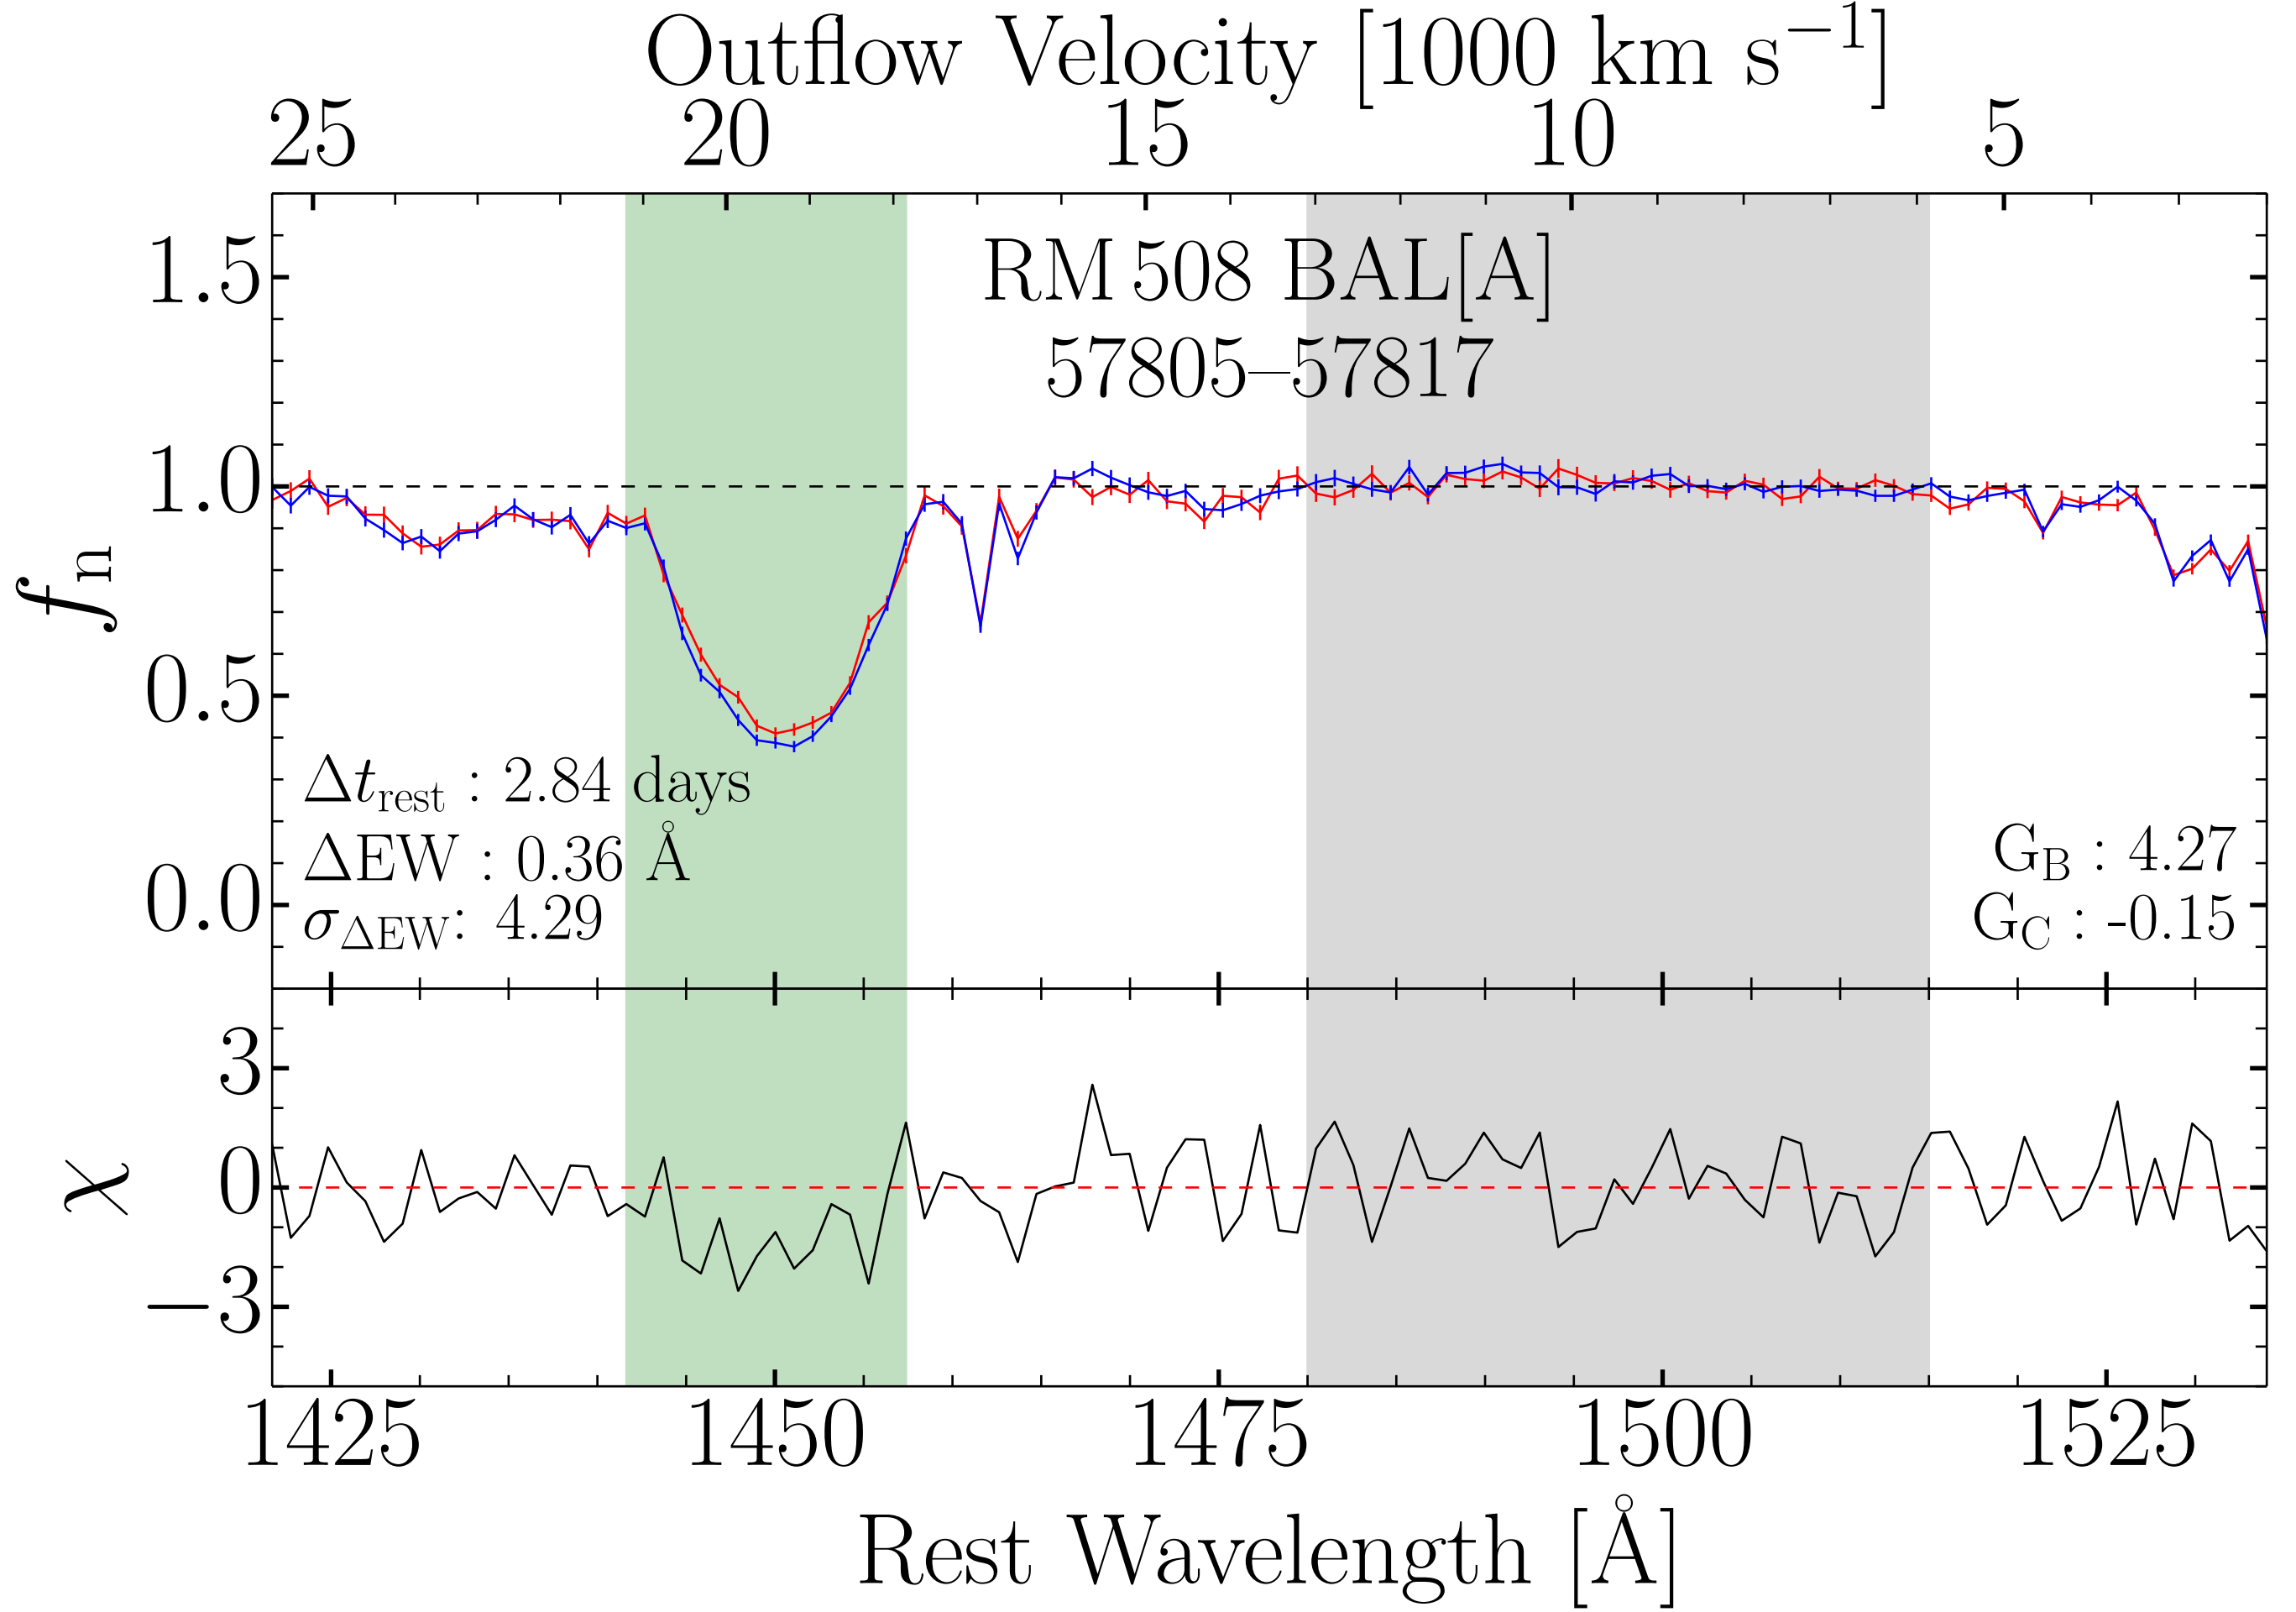

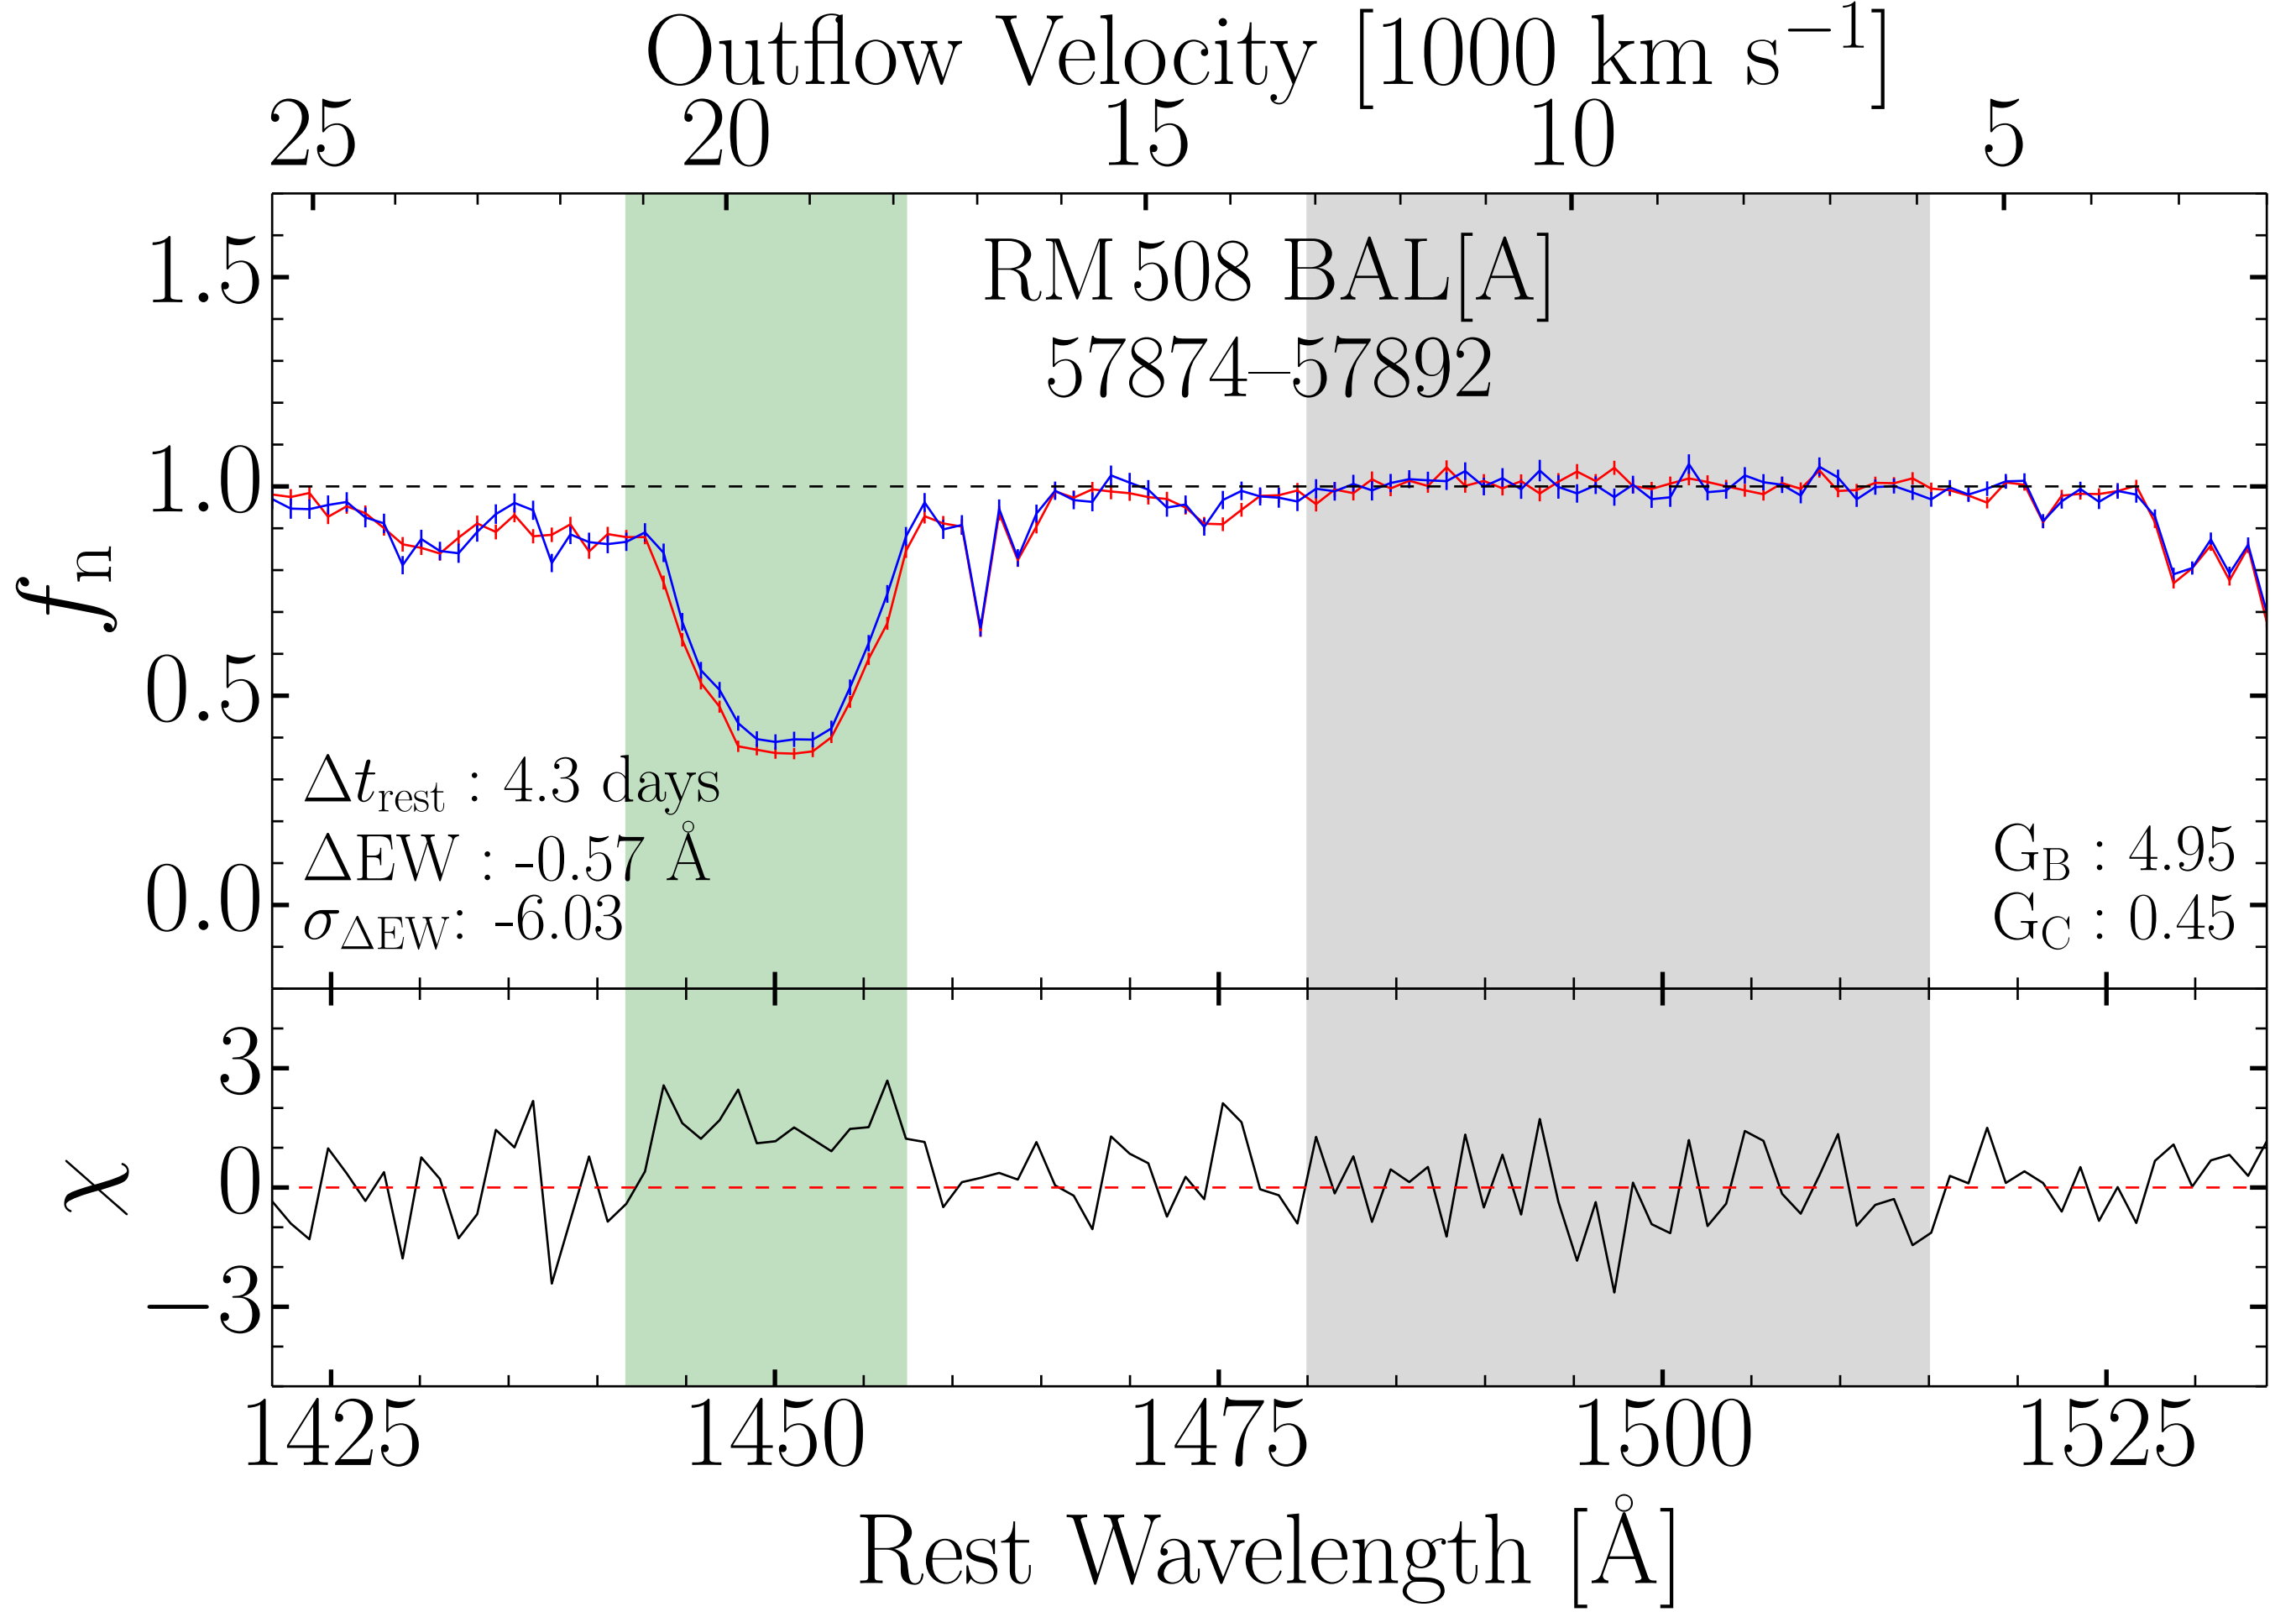

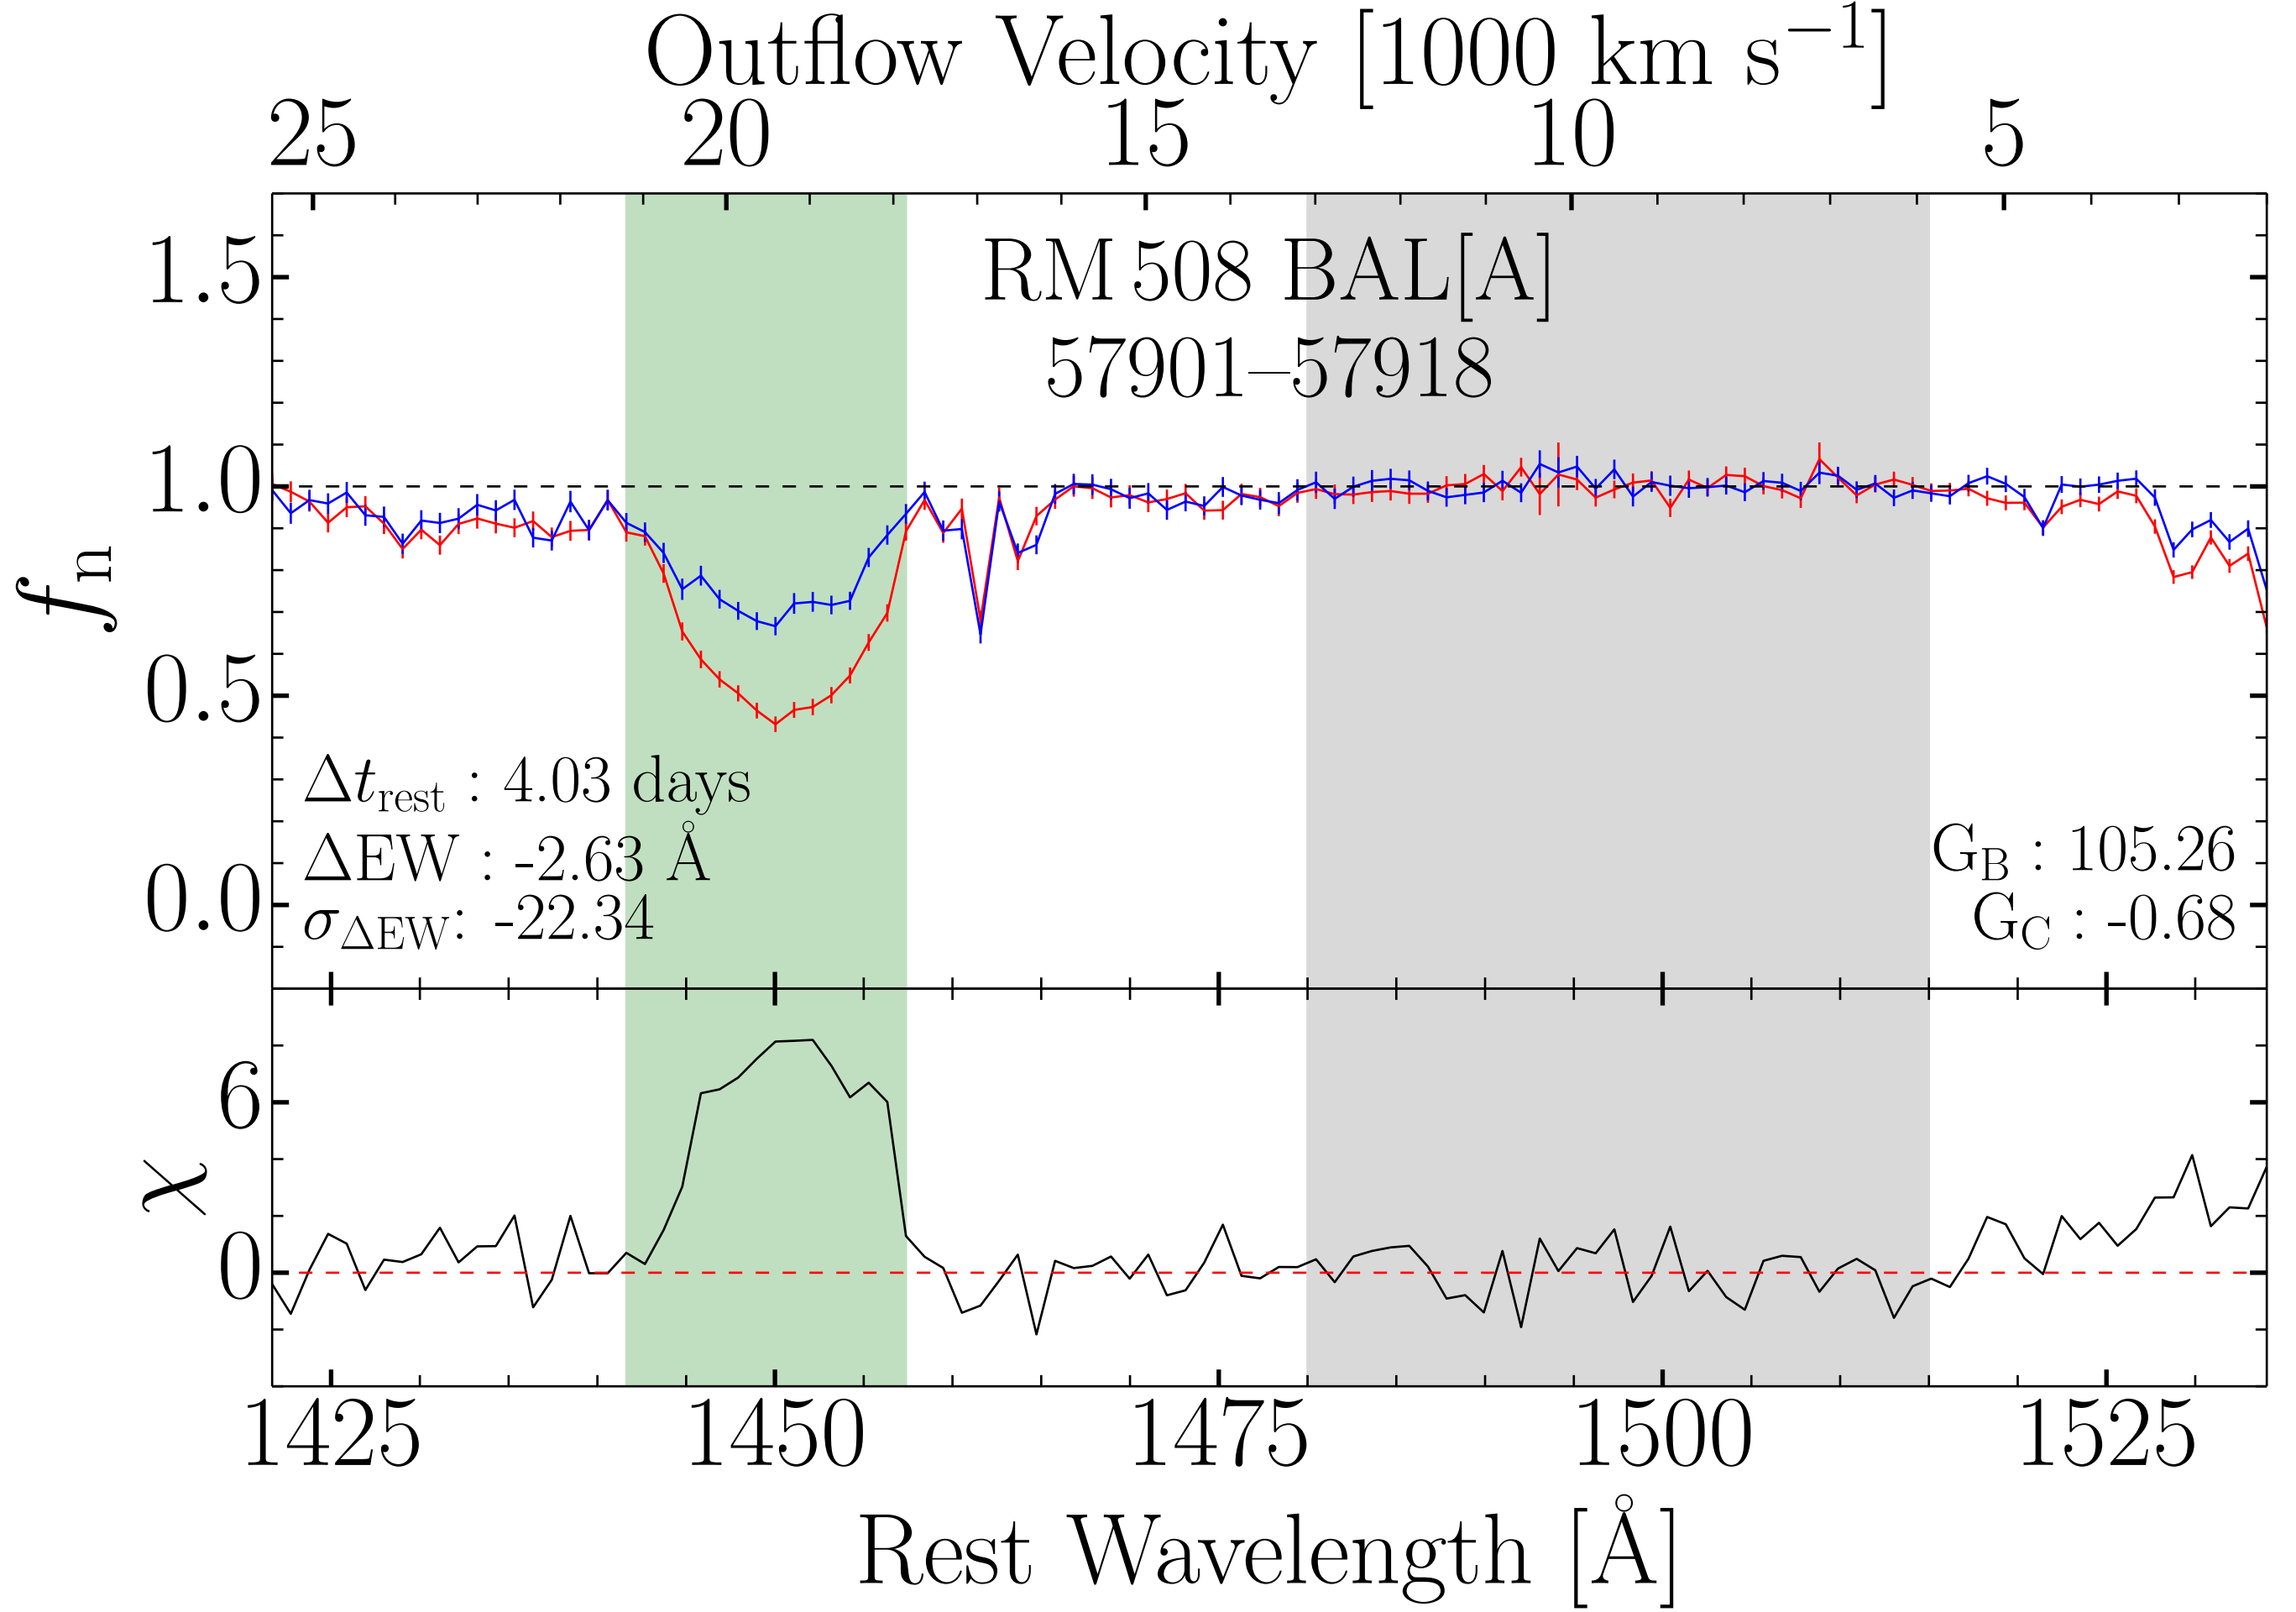

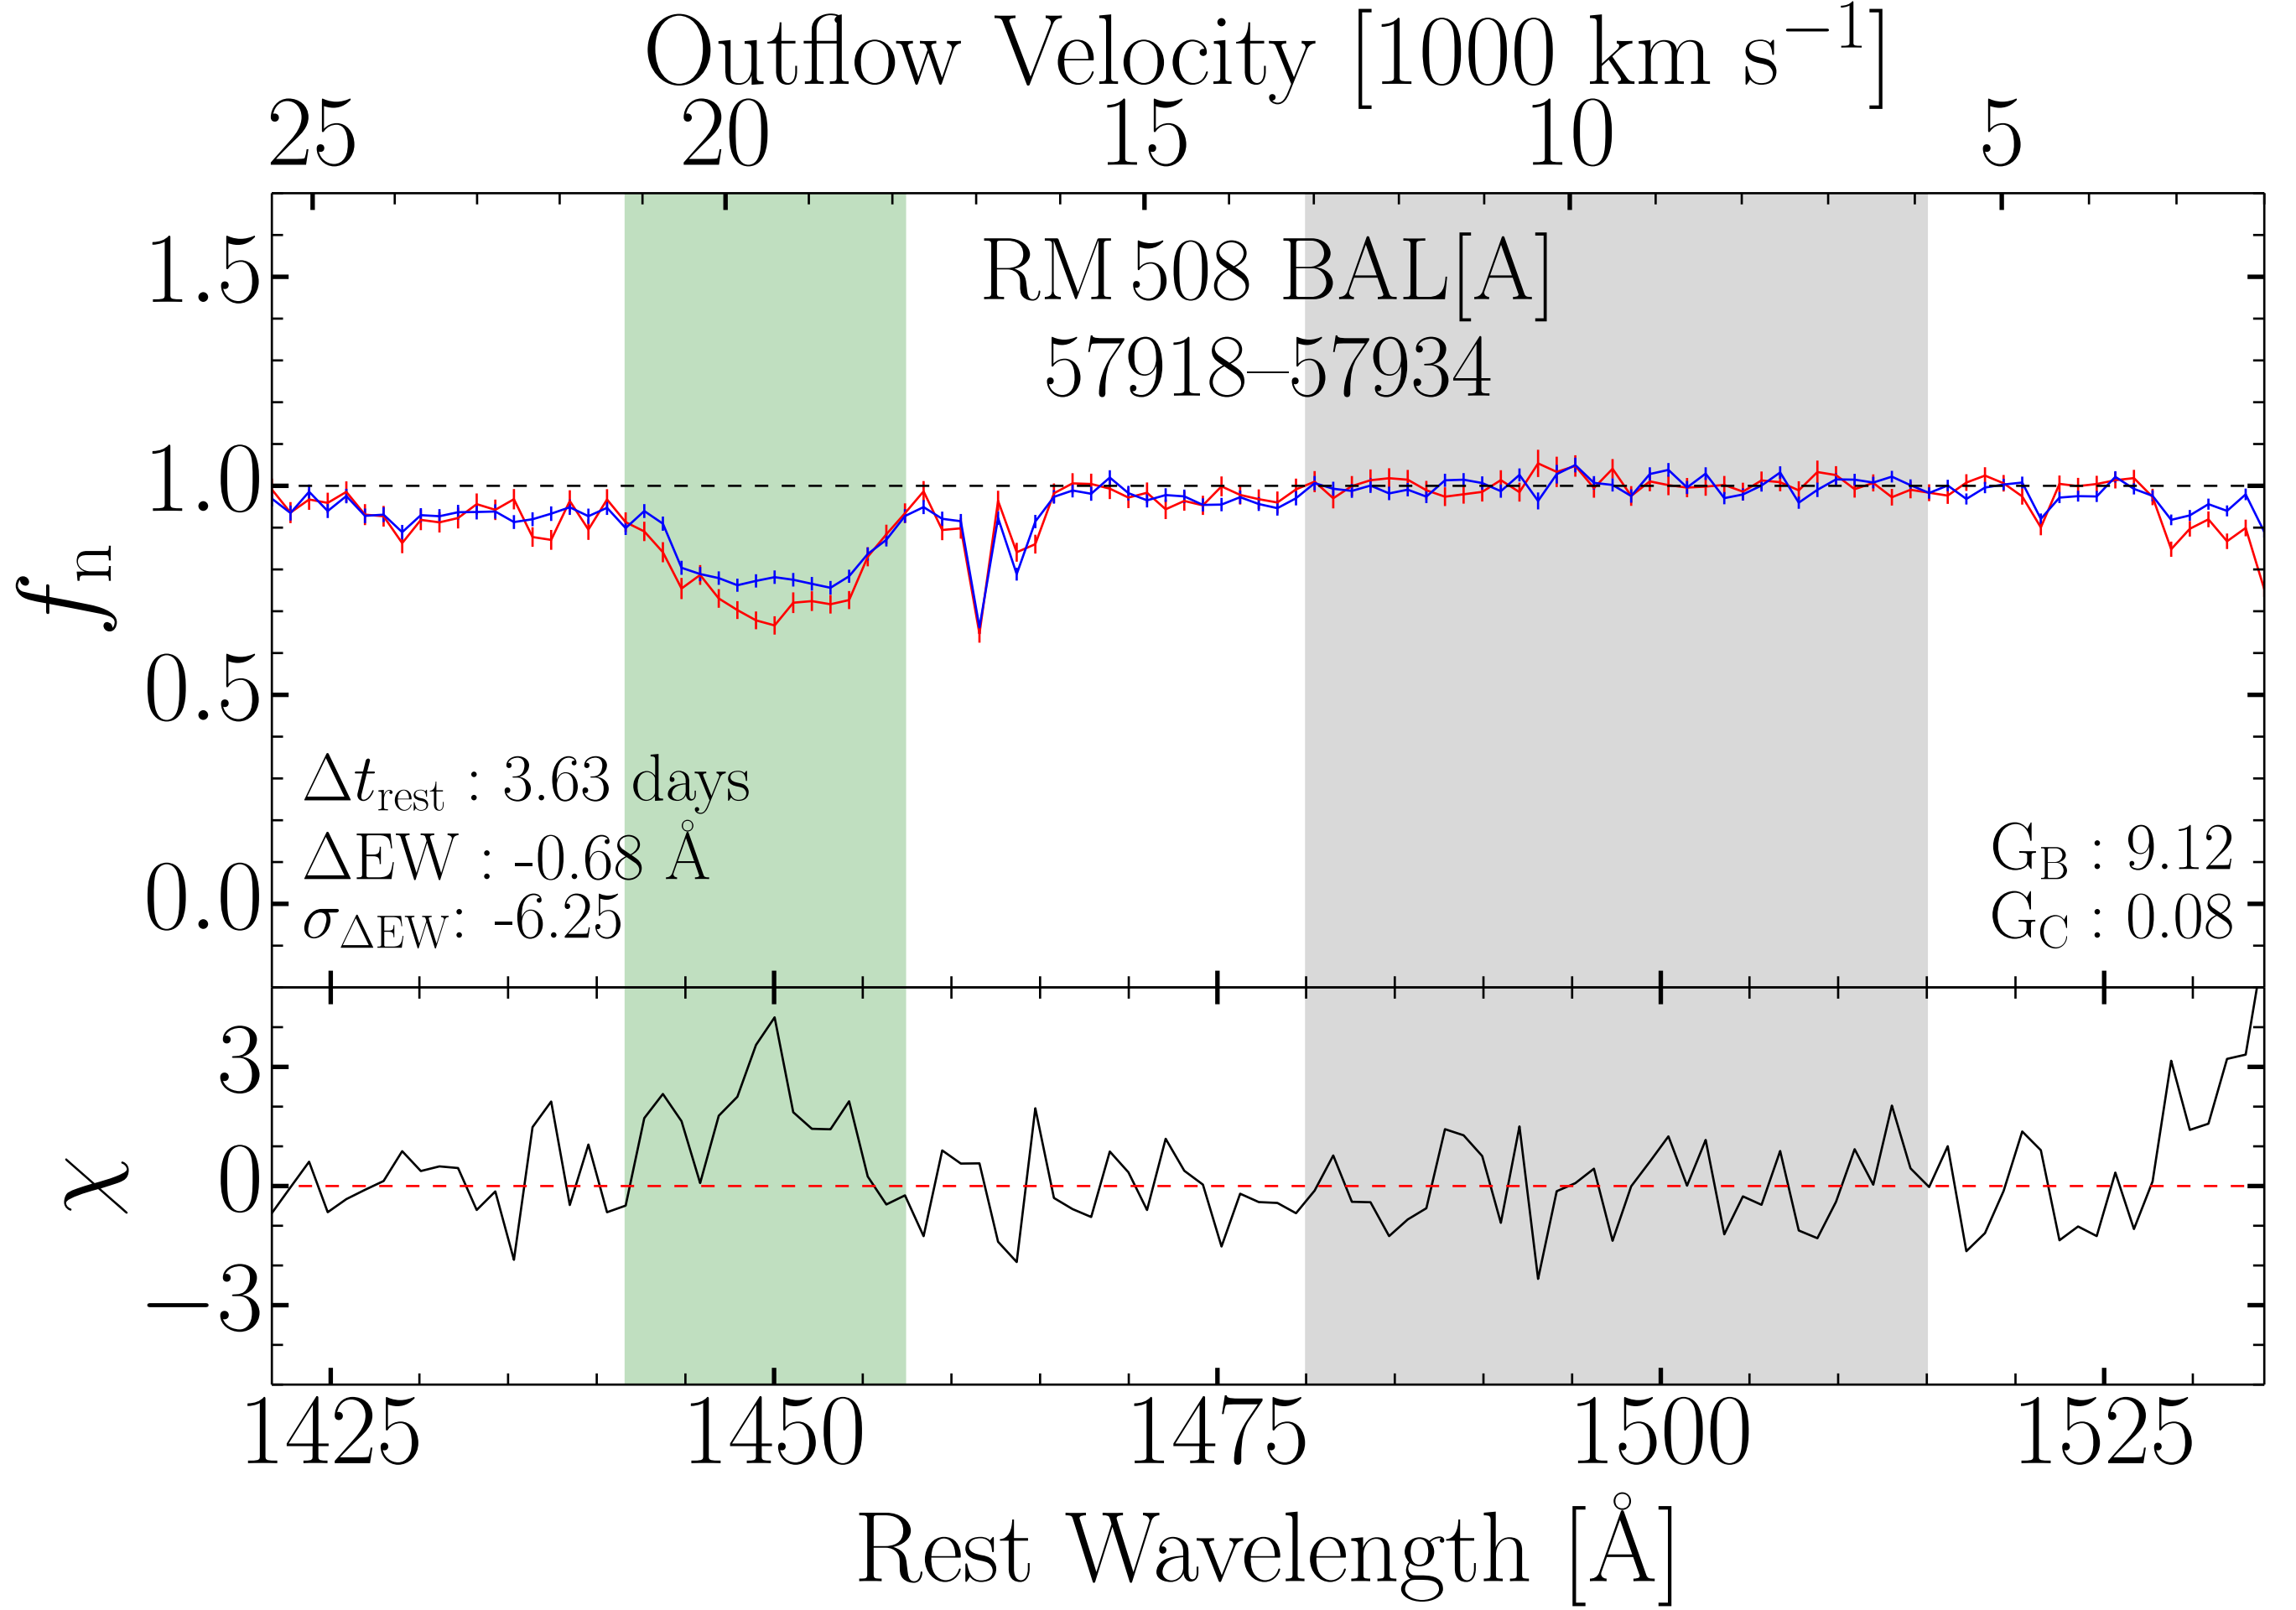

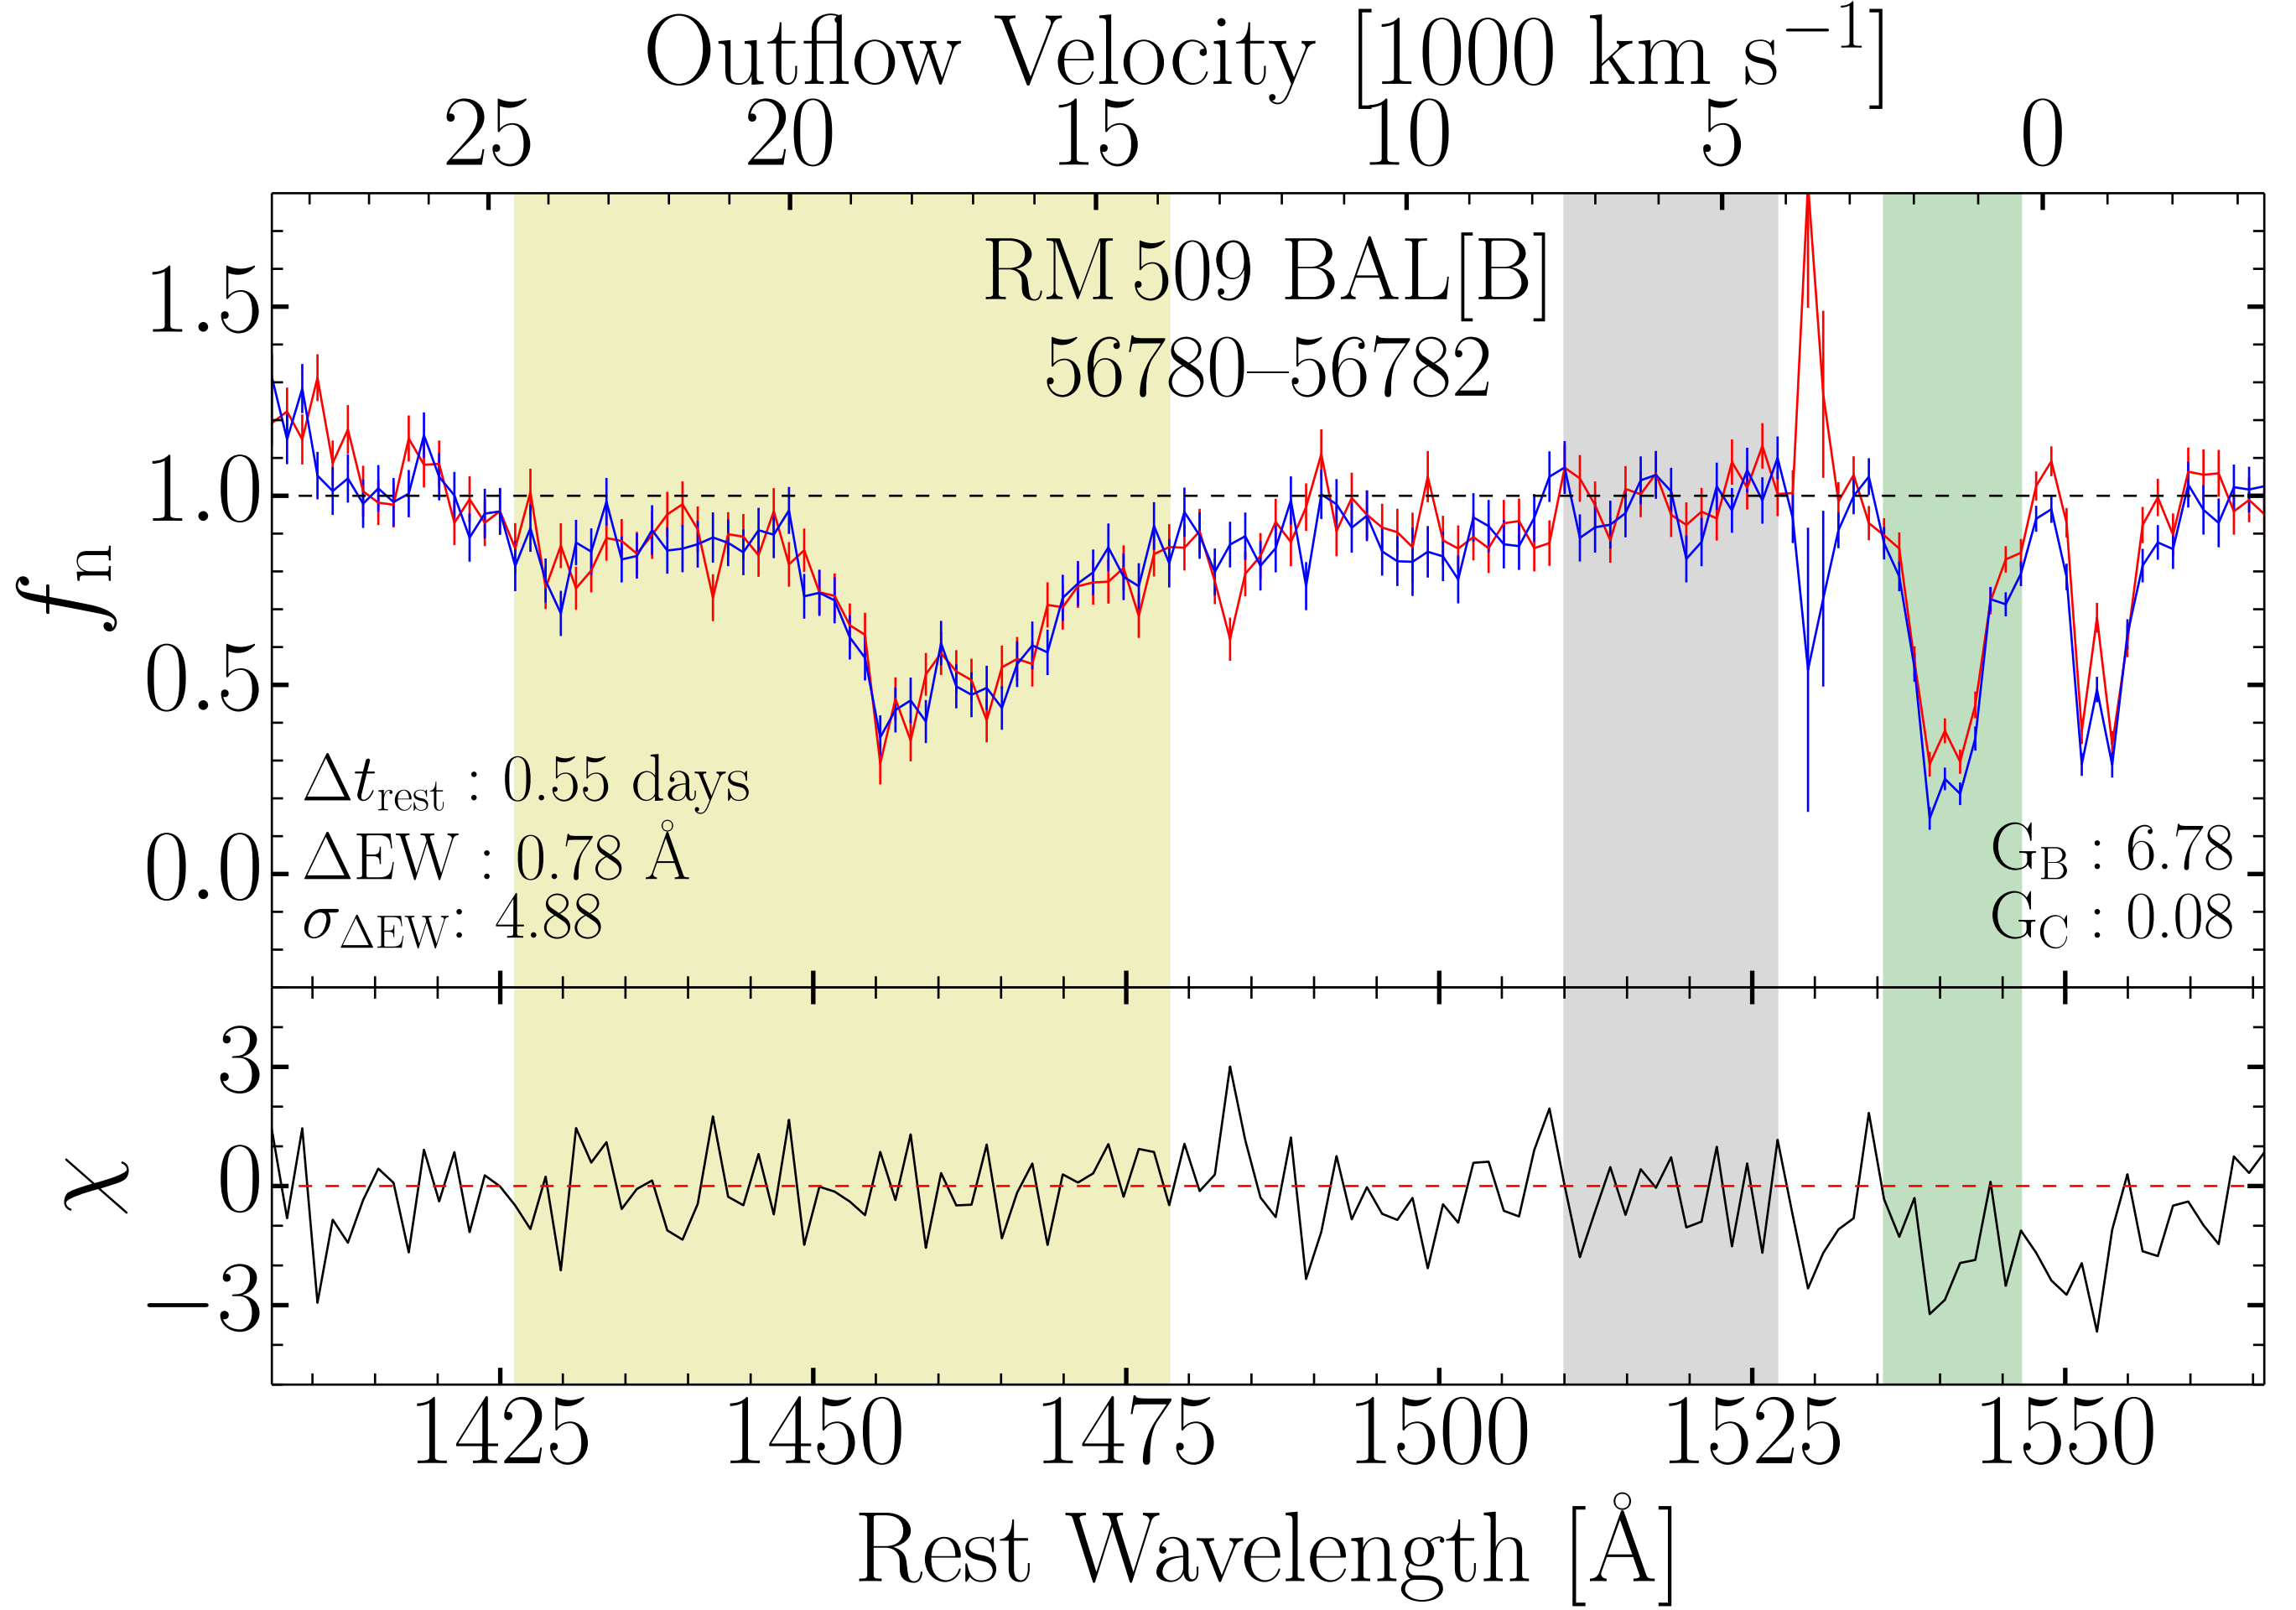



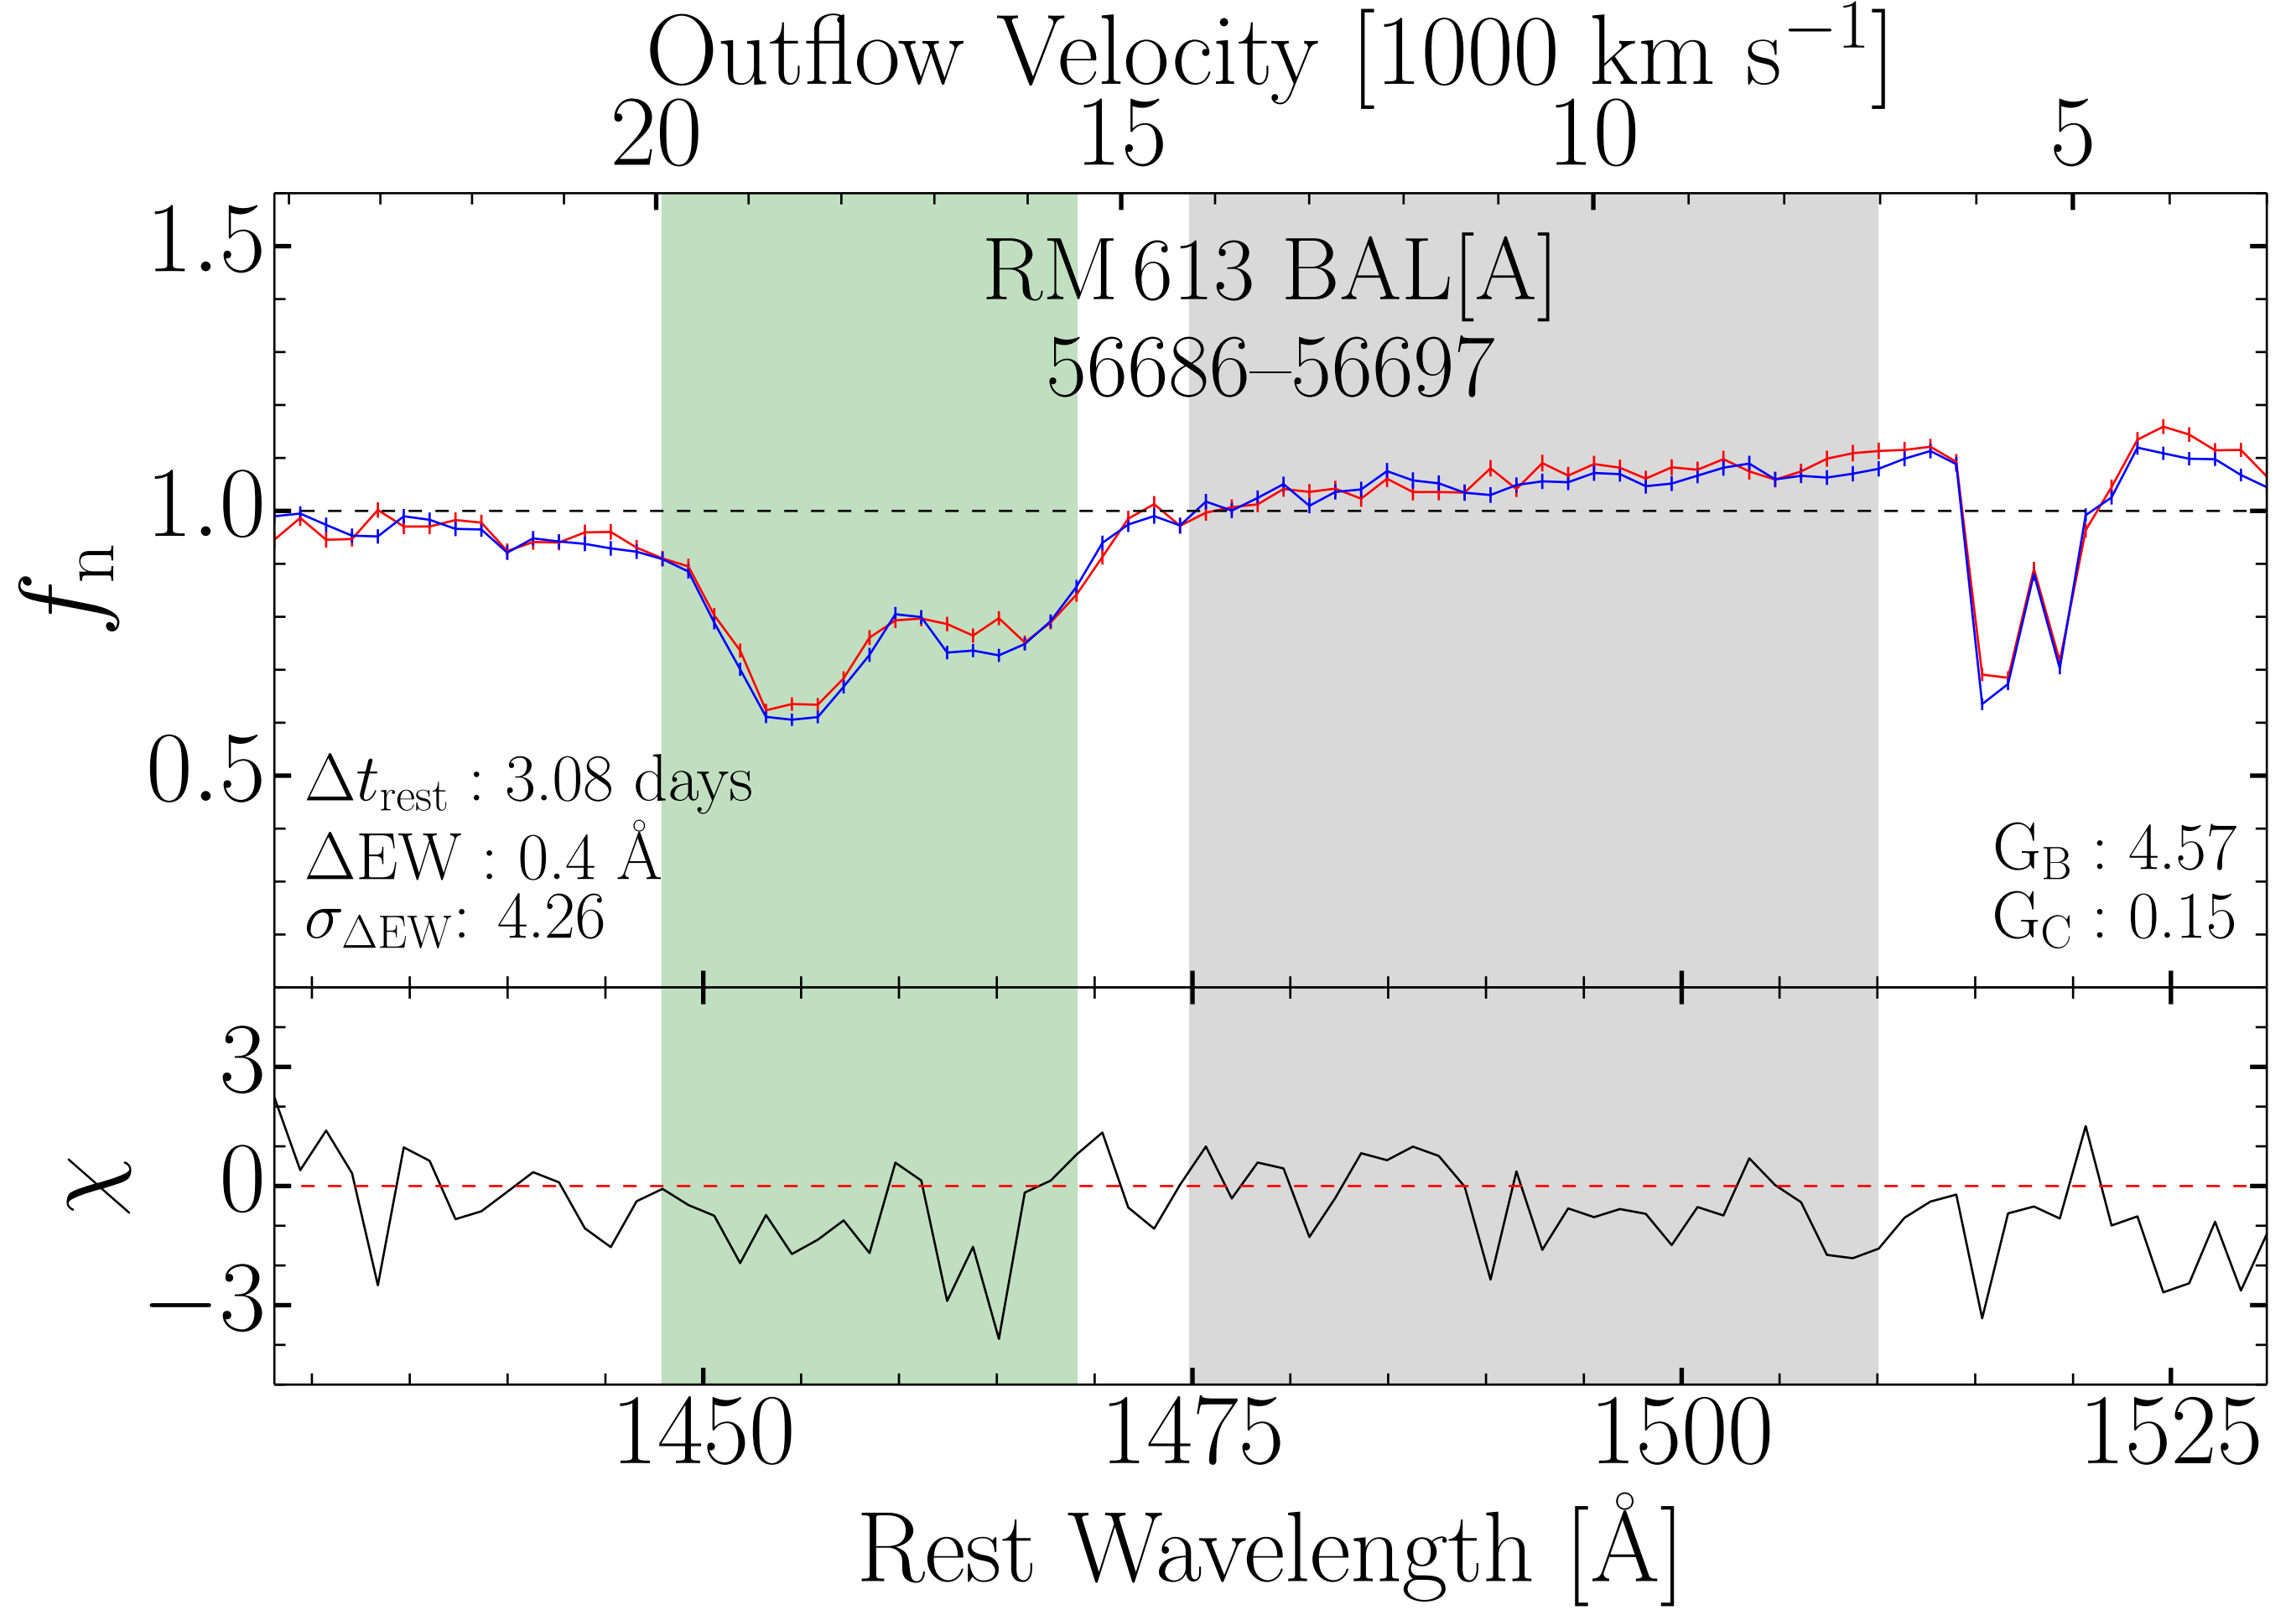

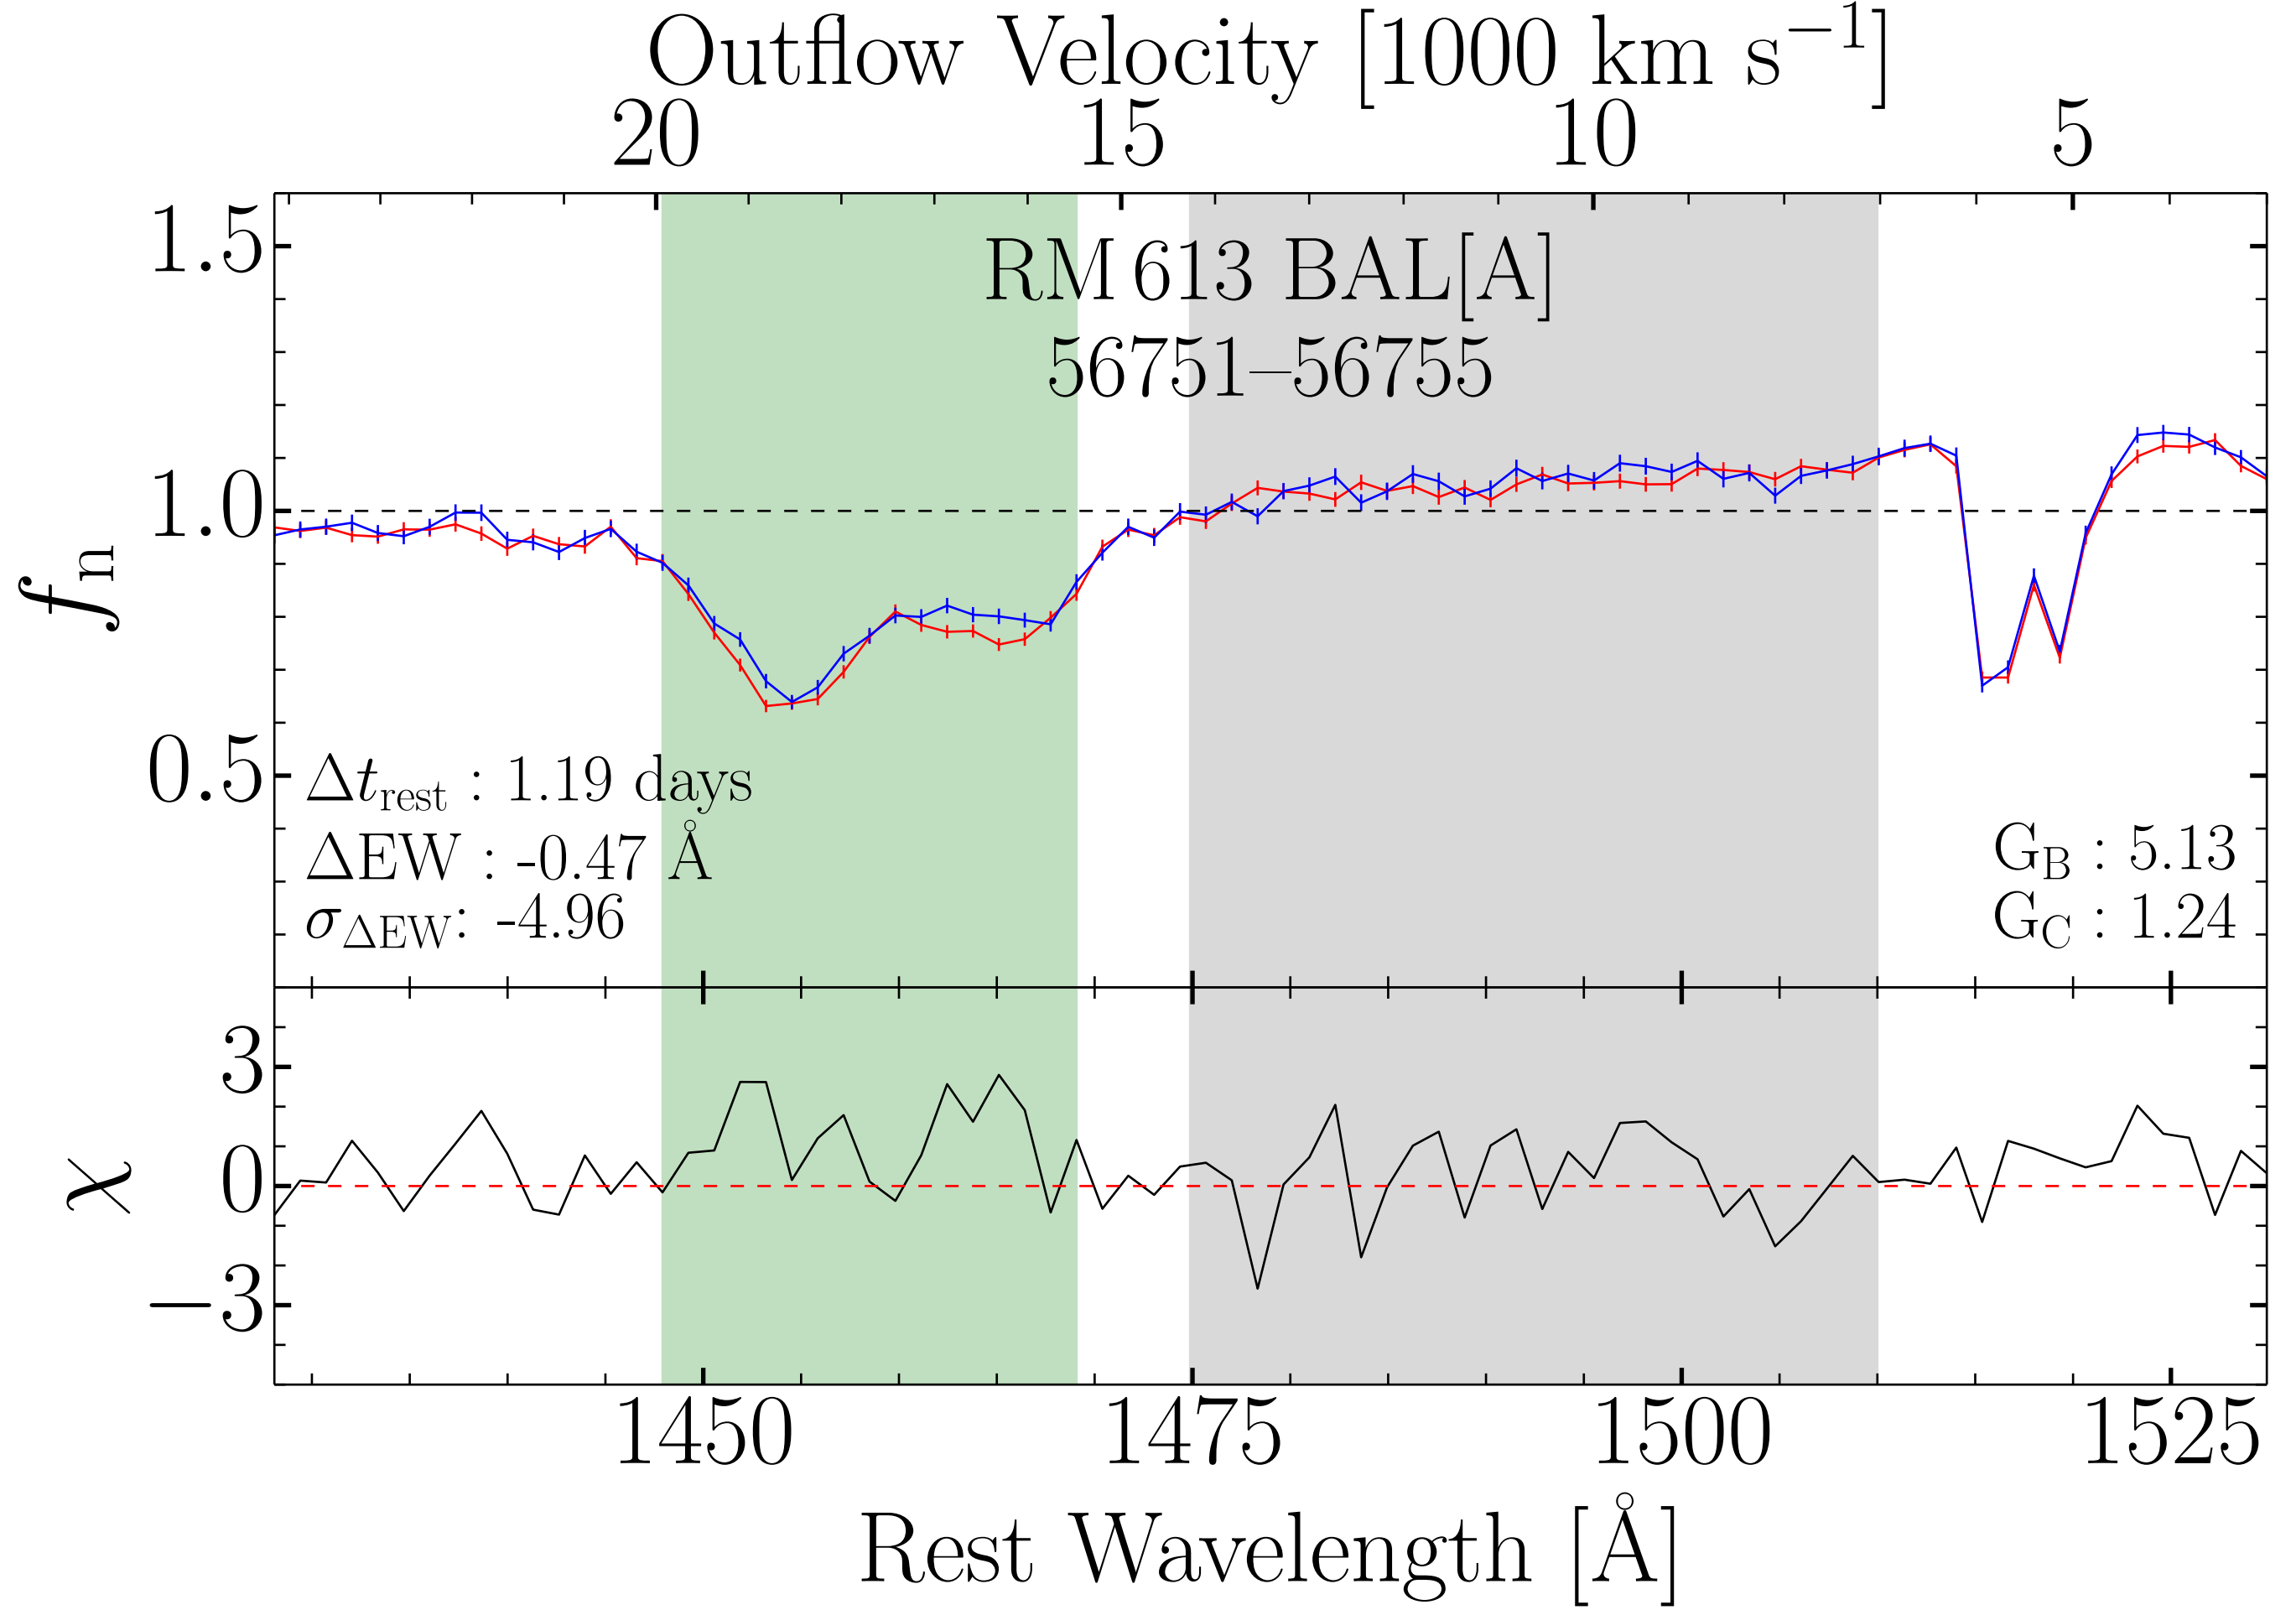

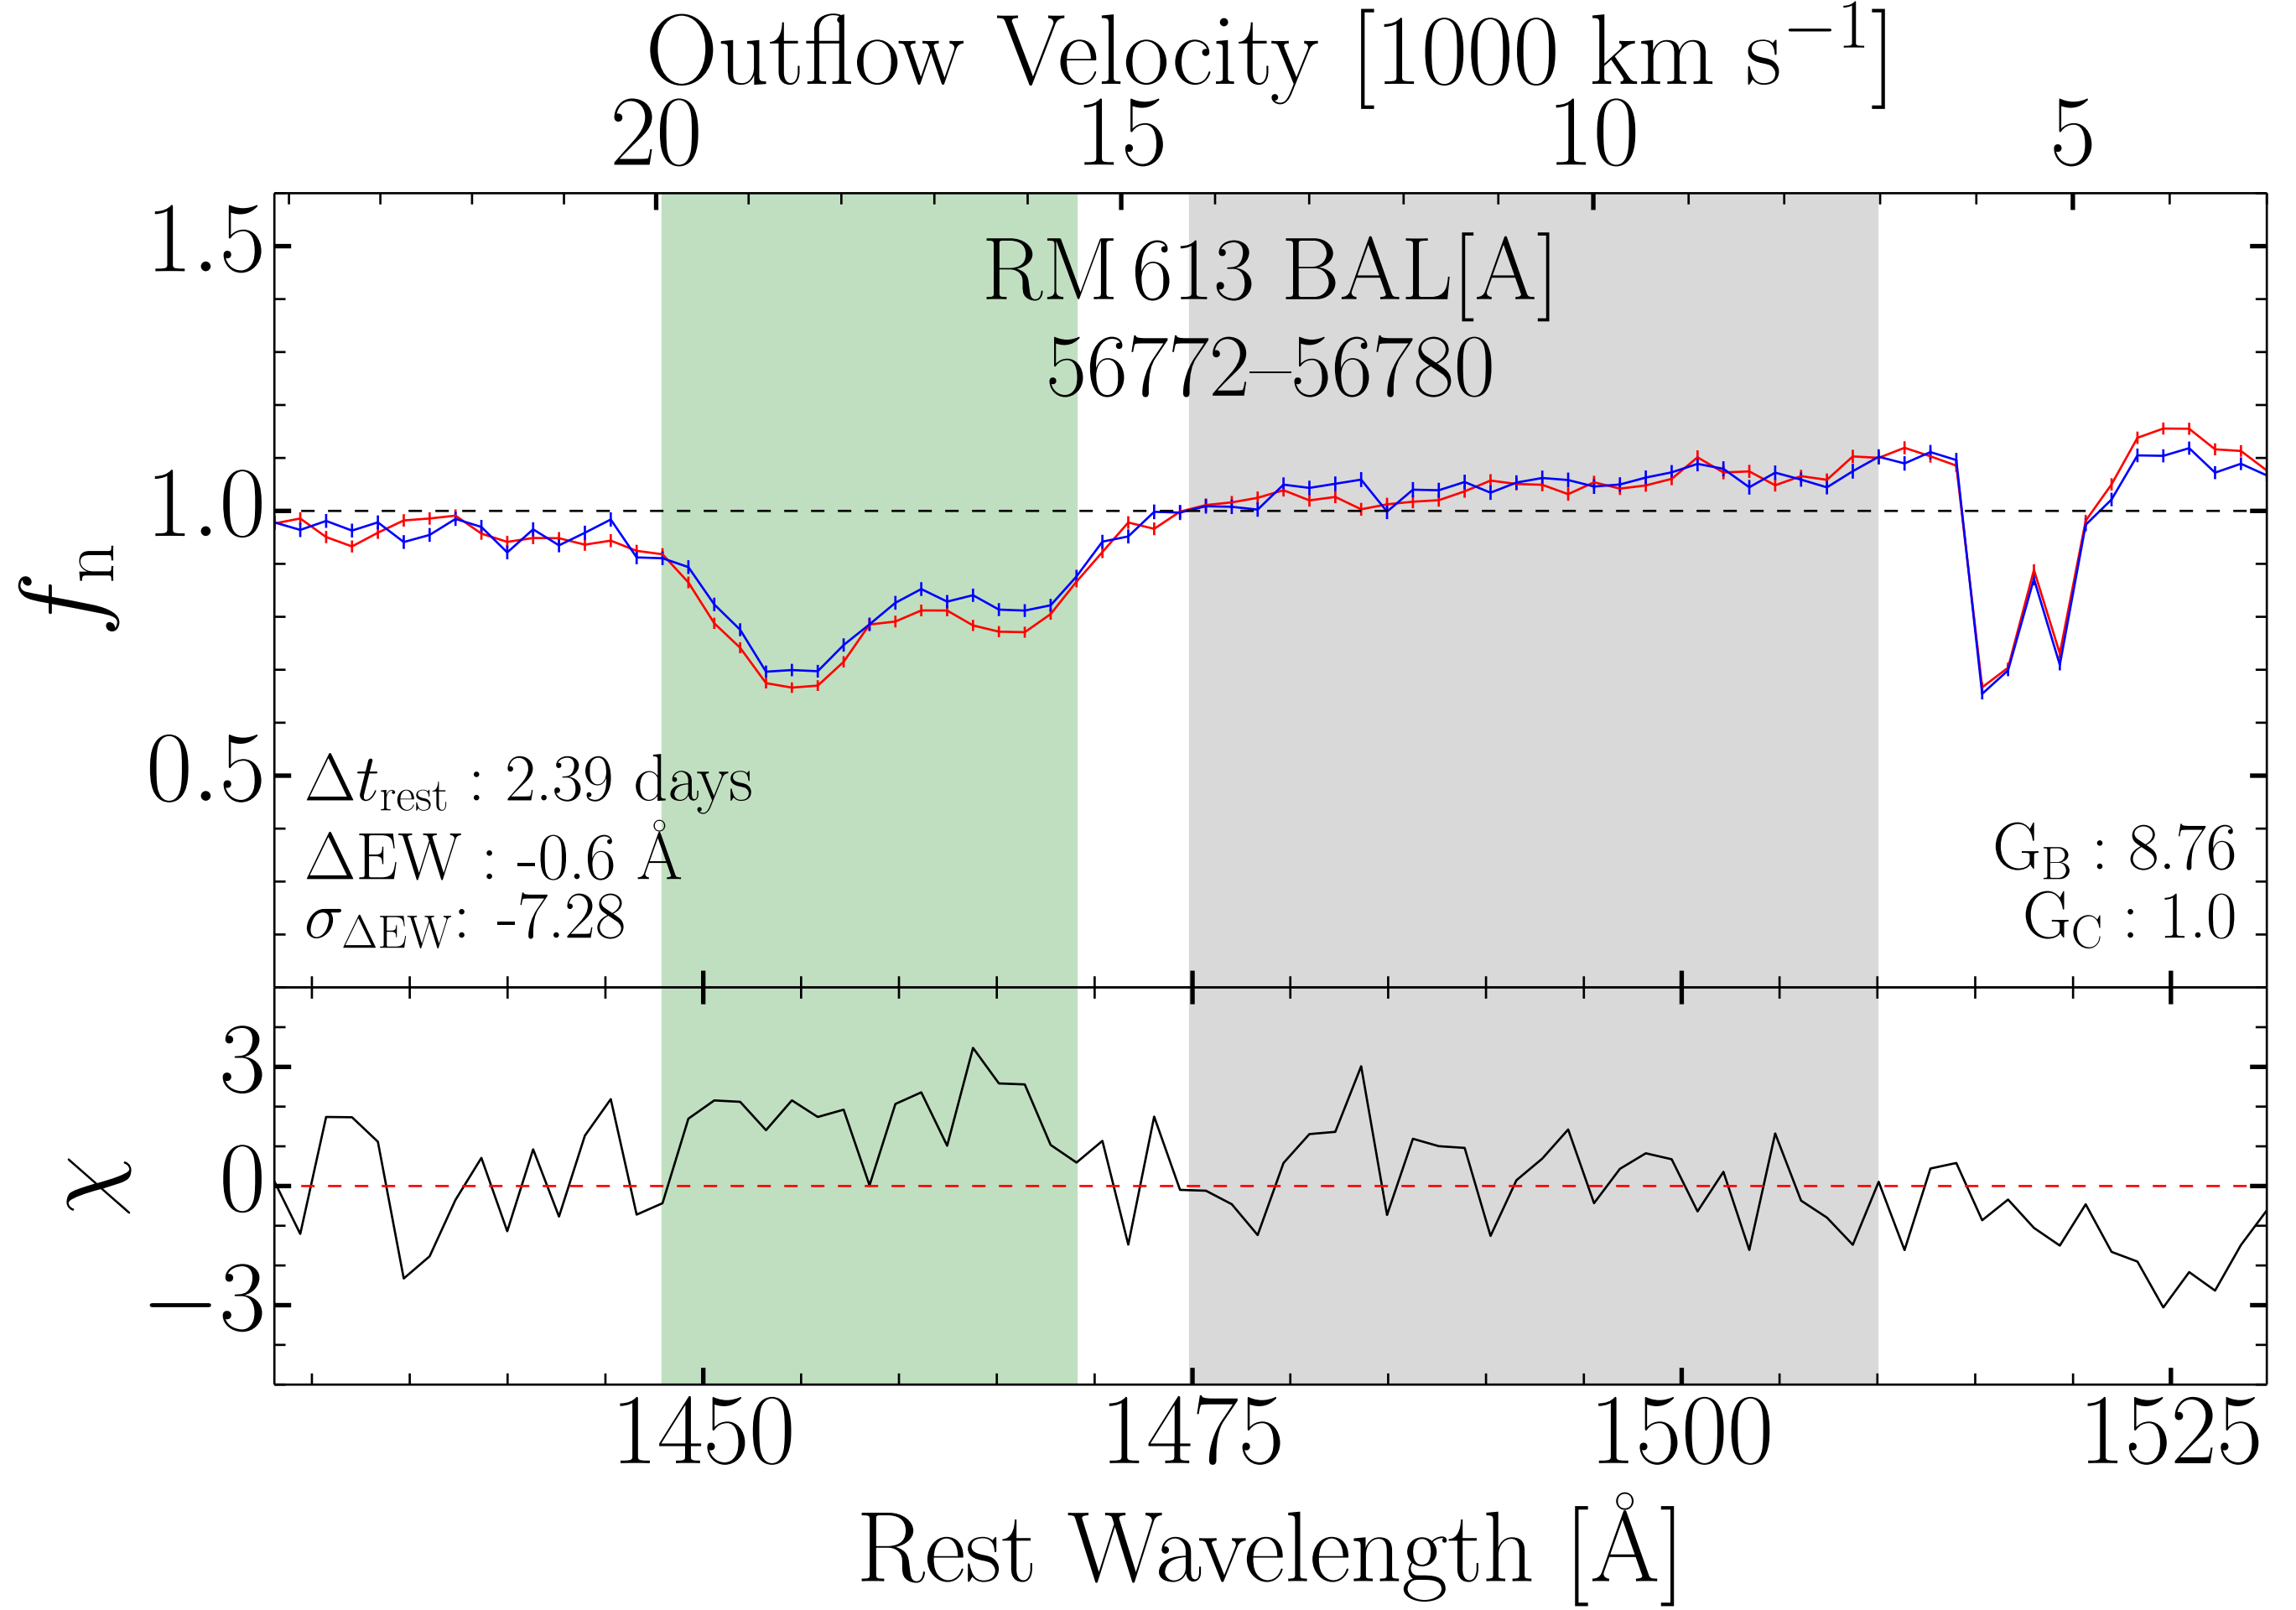

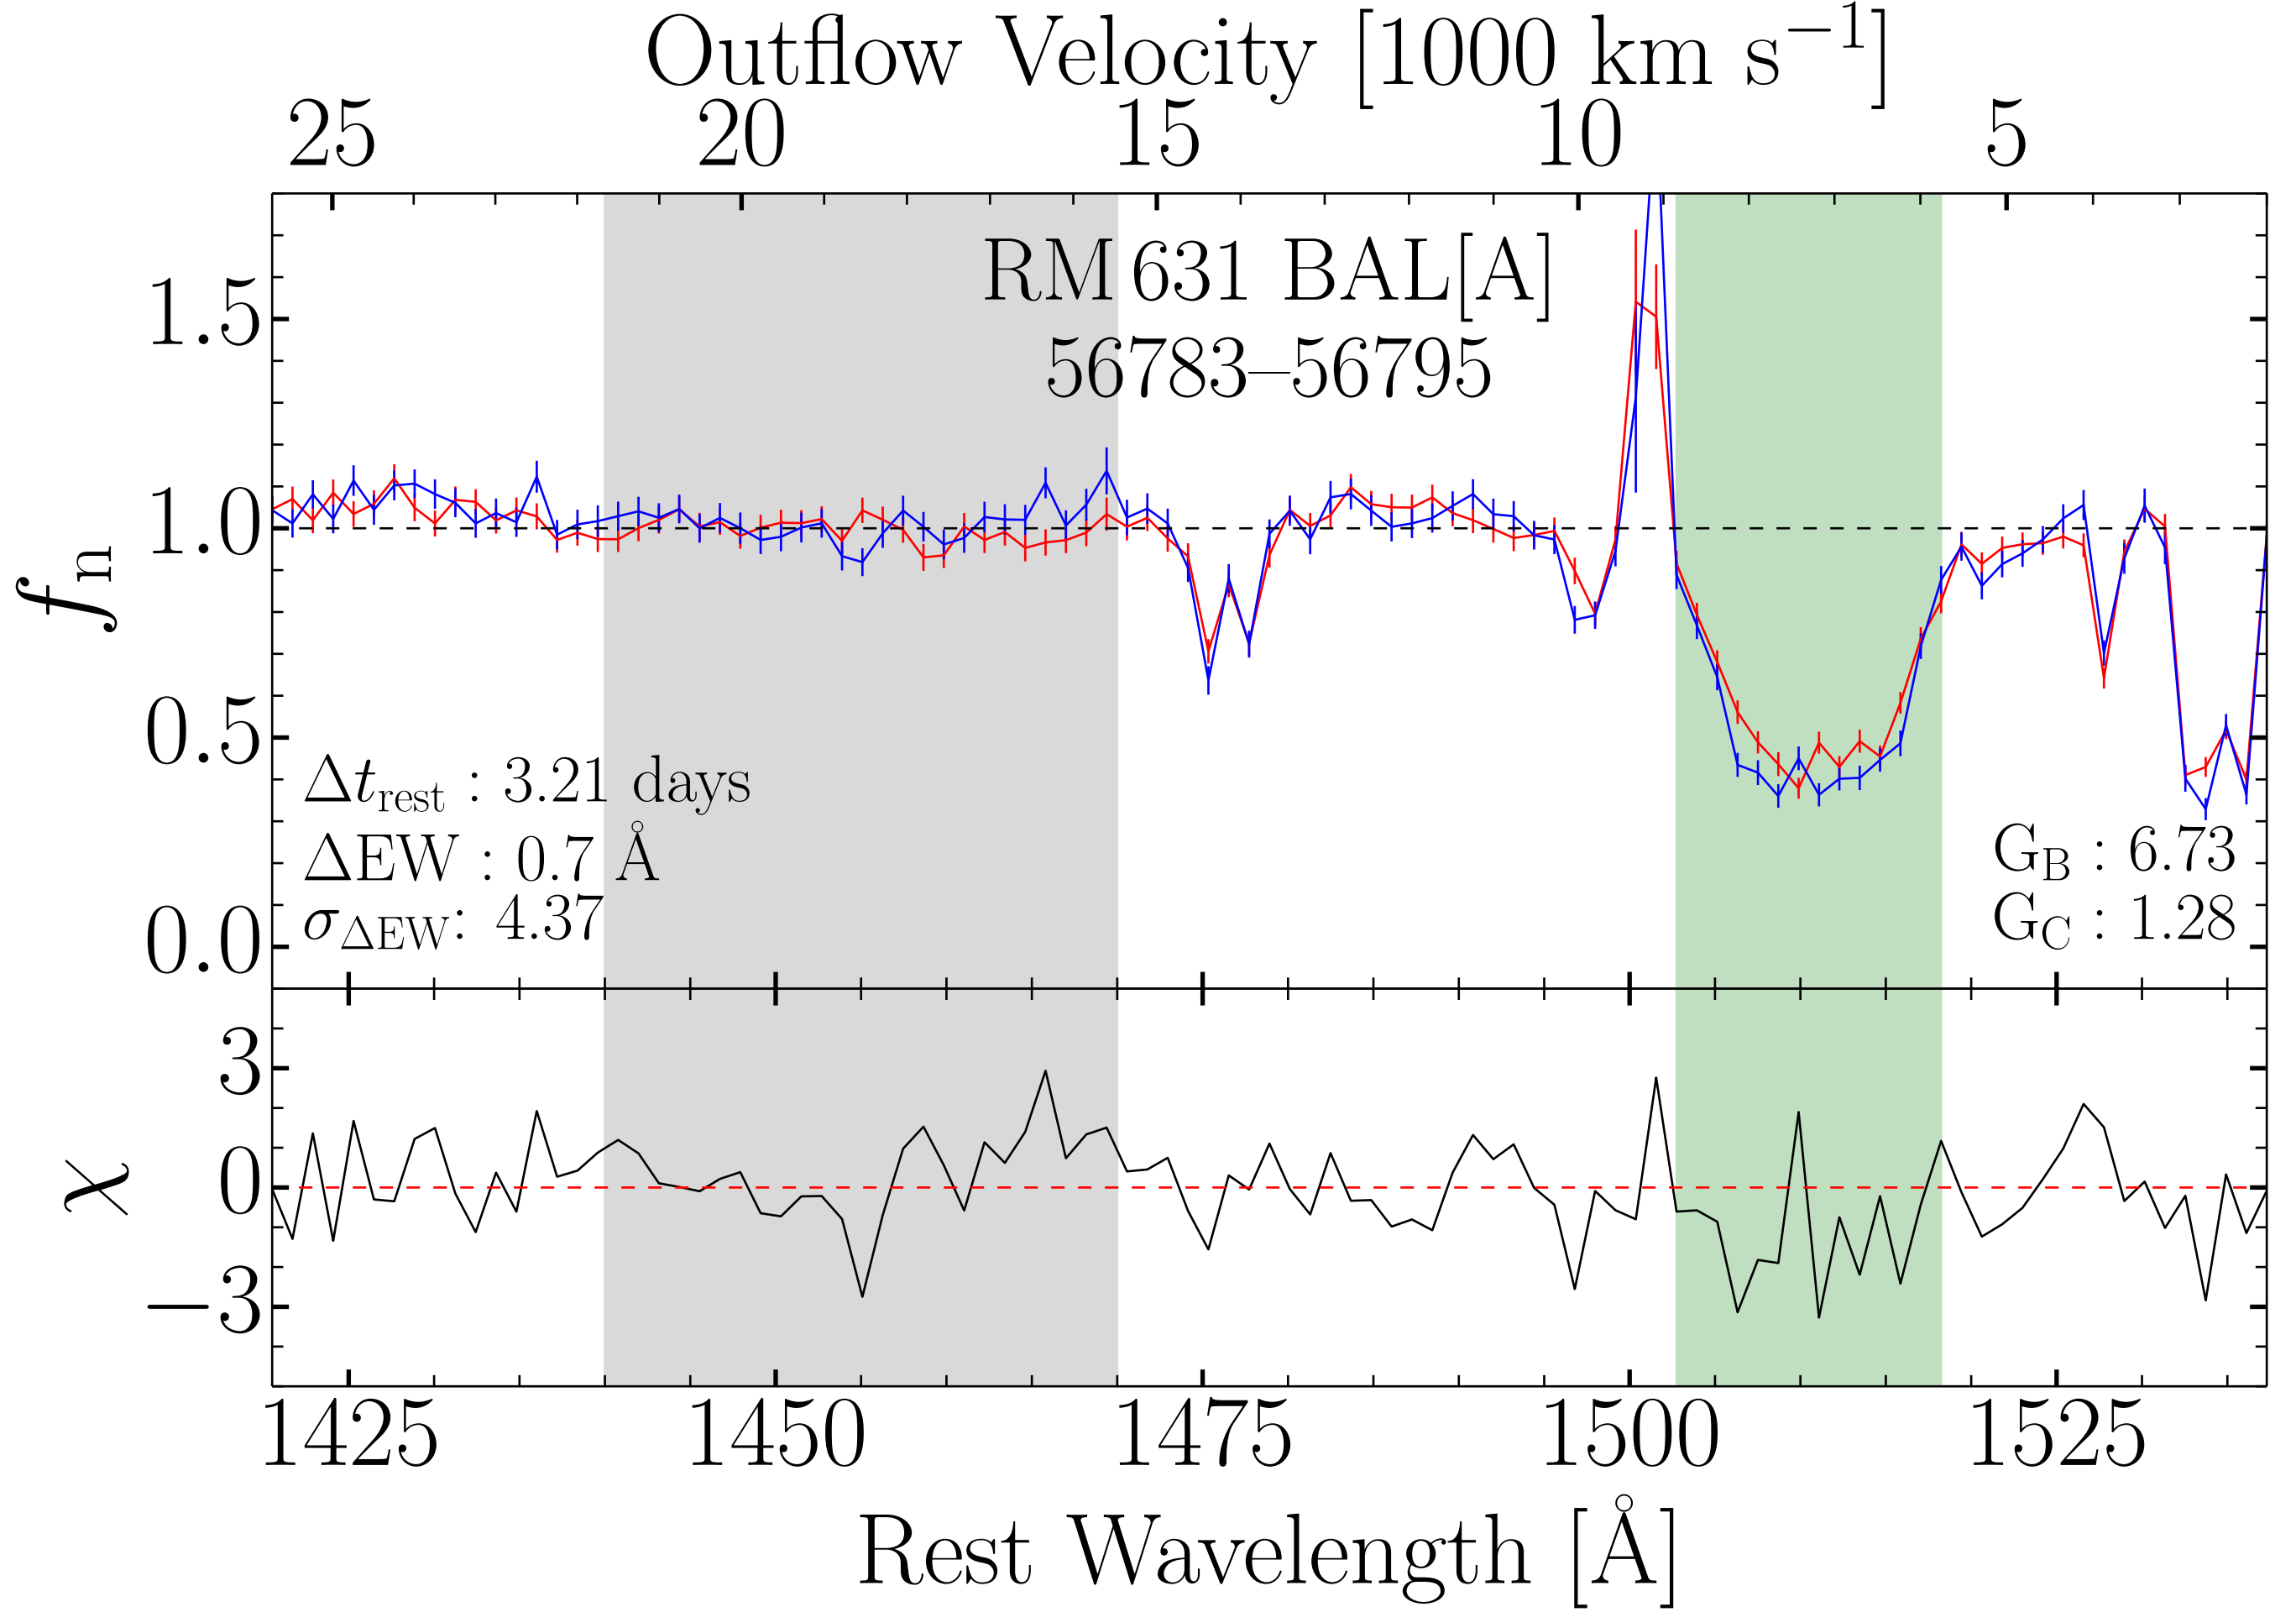

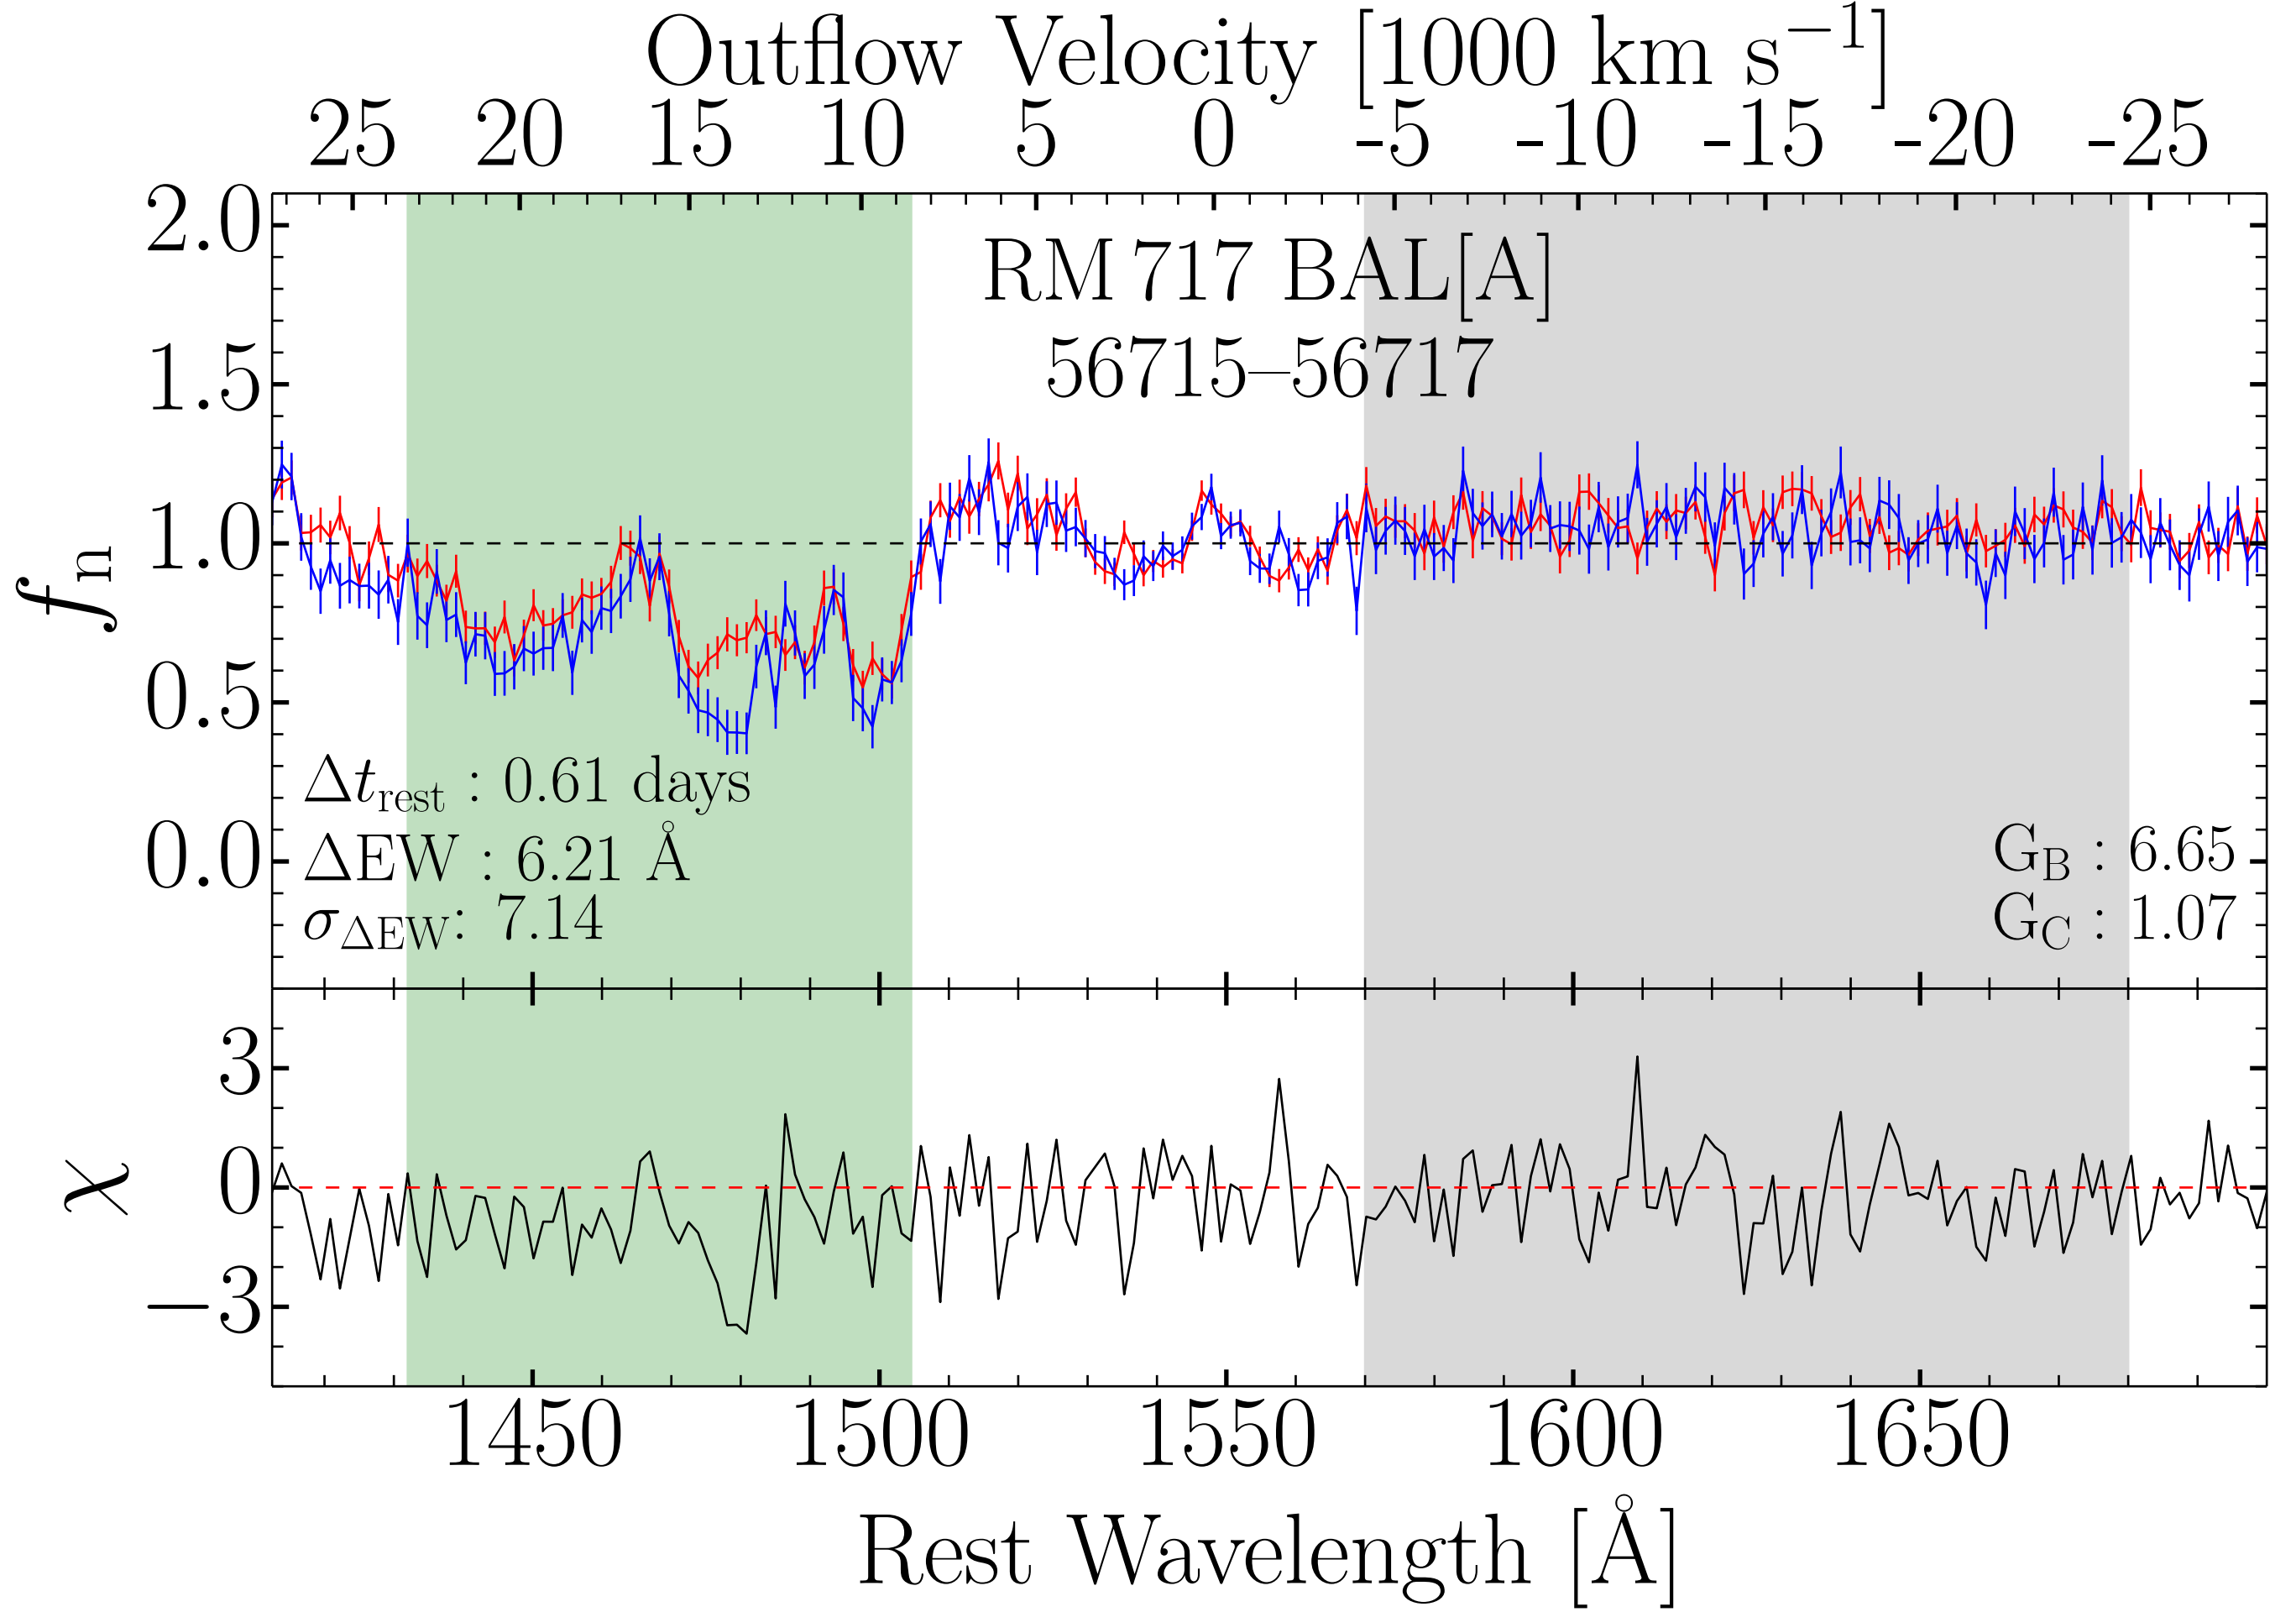

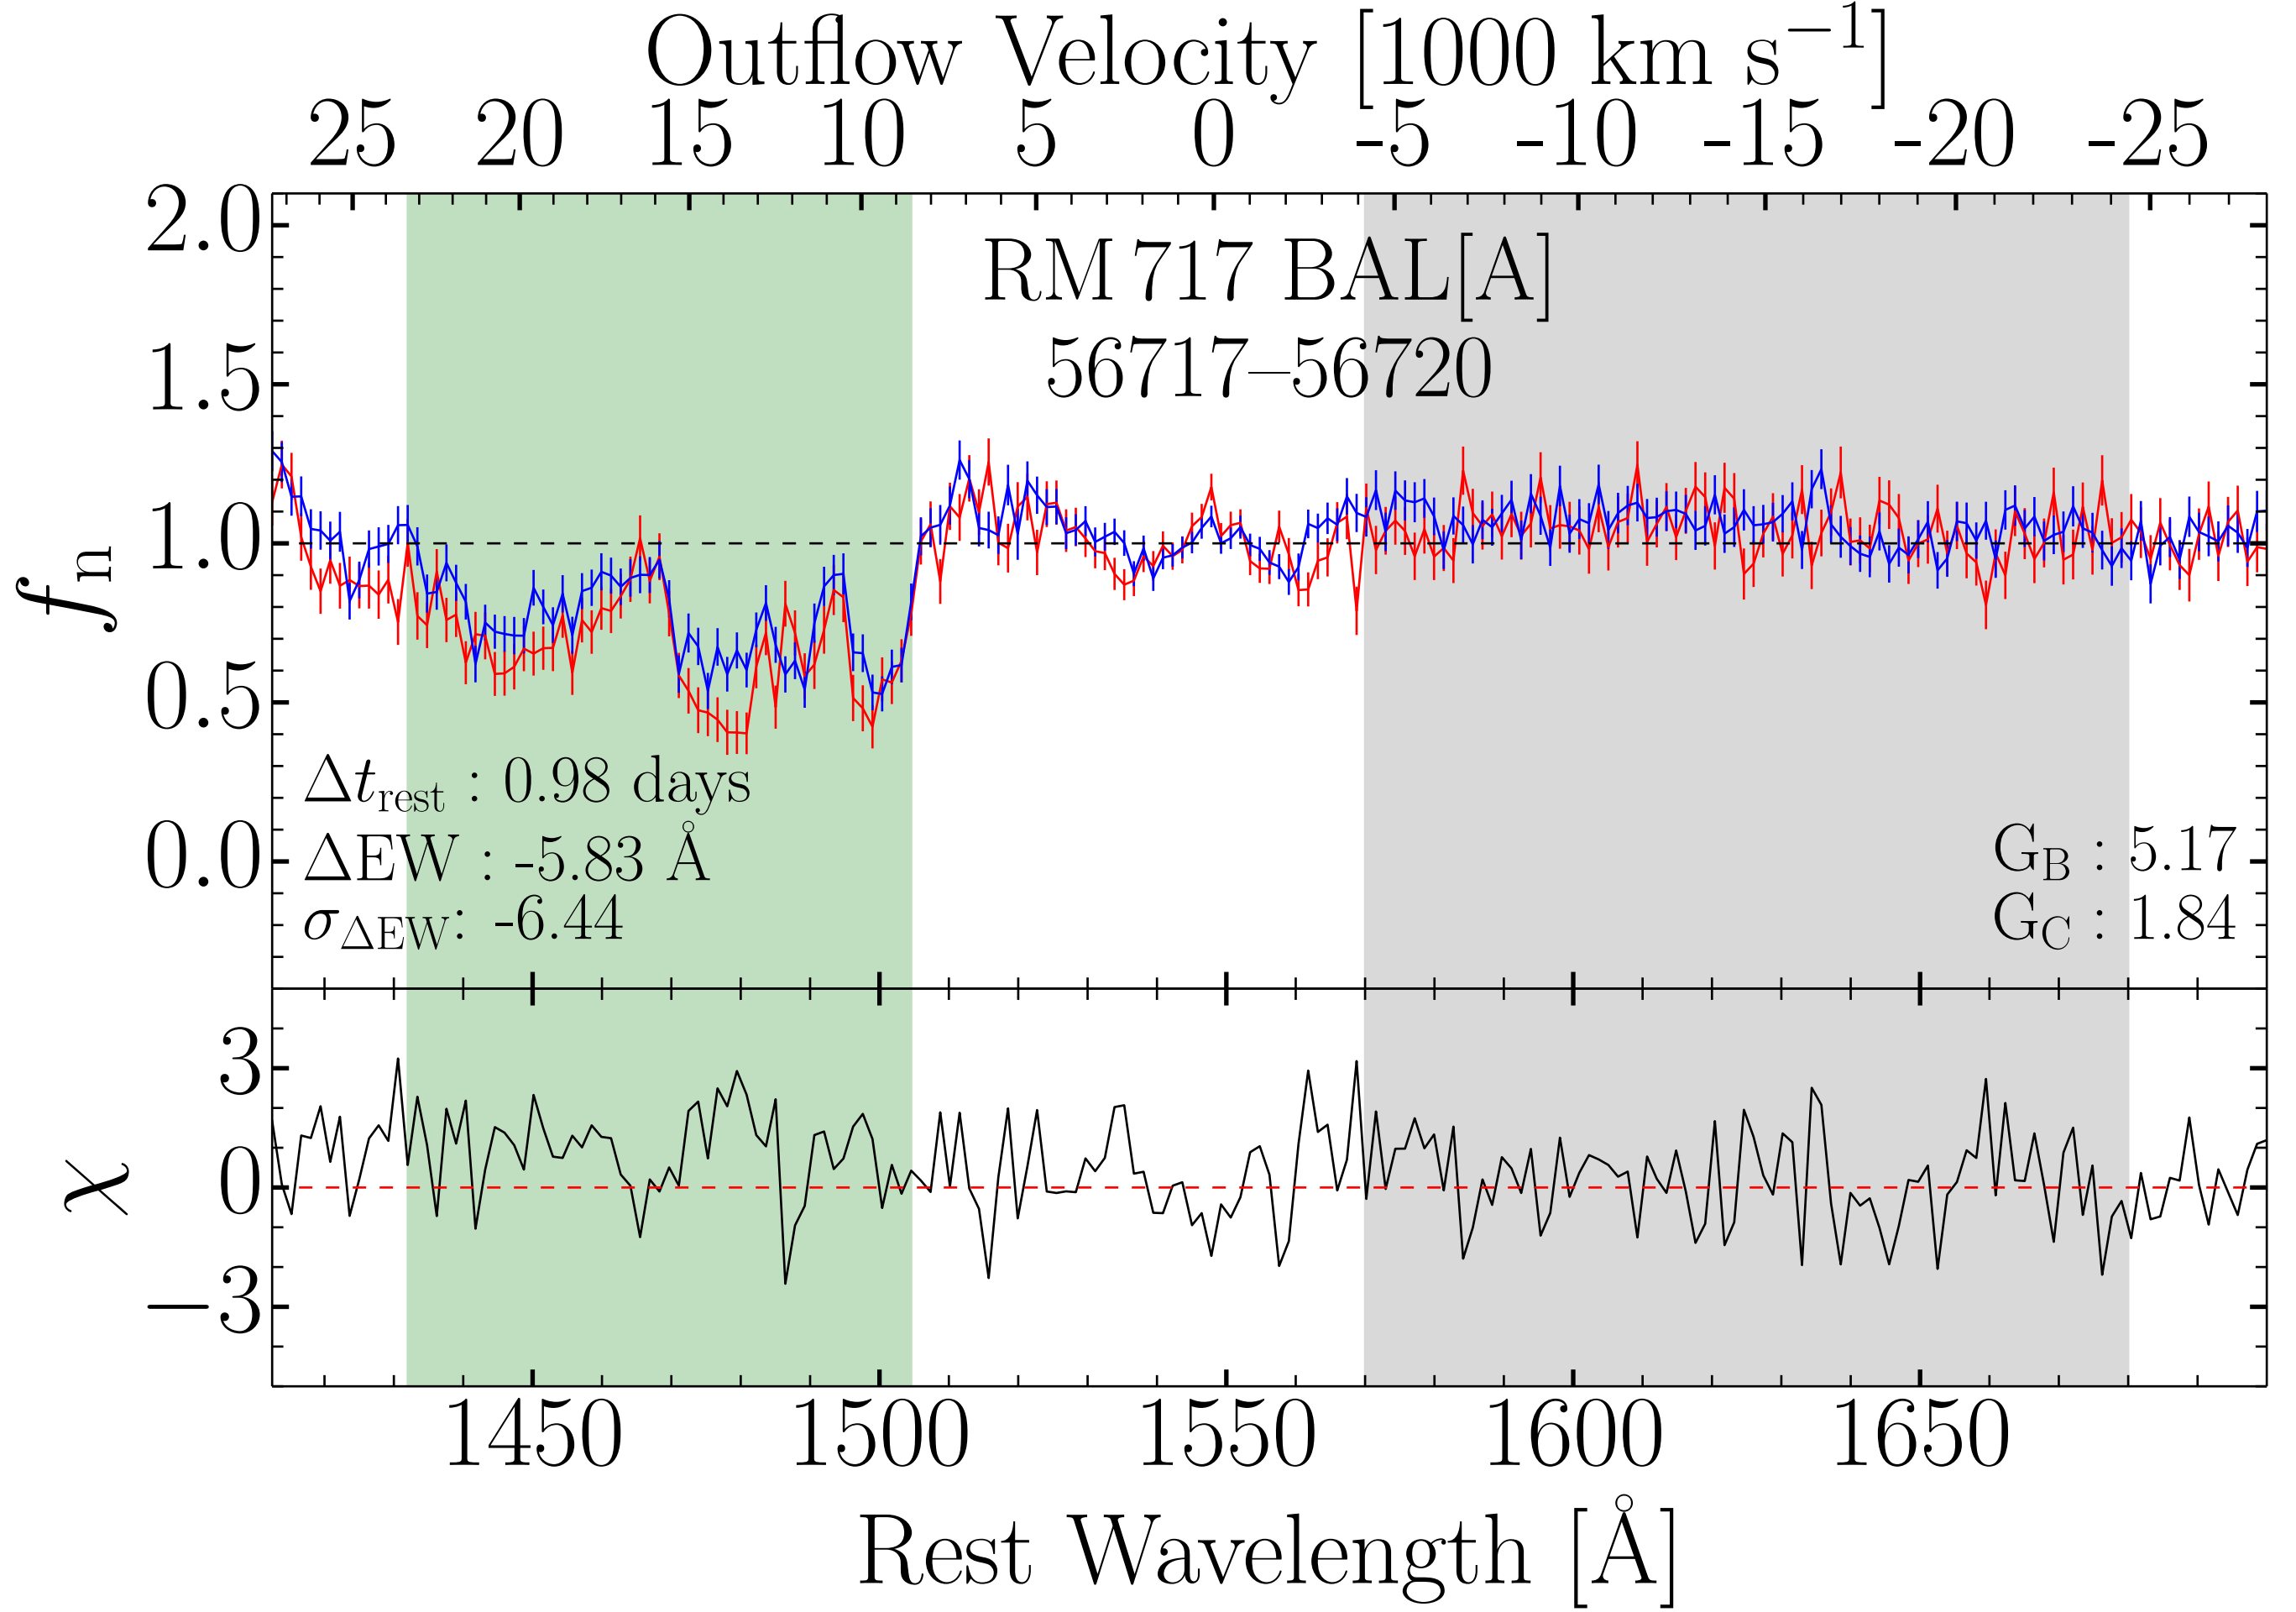

Outflow Velocity [1000 km s<sup>-1</sup>]

15

10

5

0

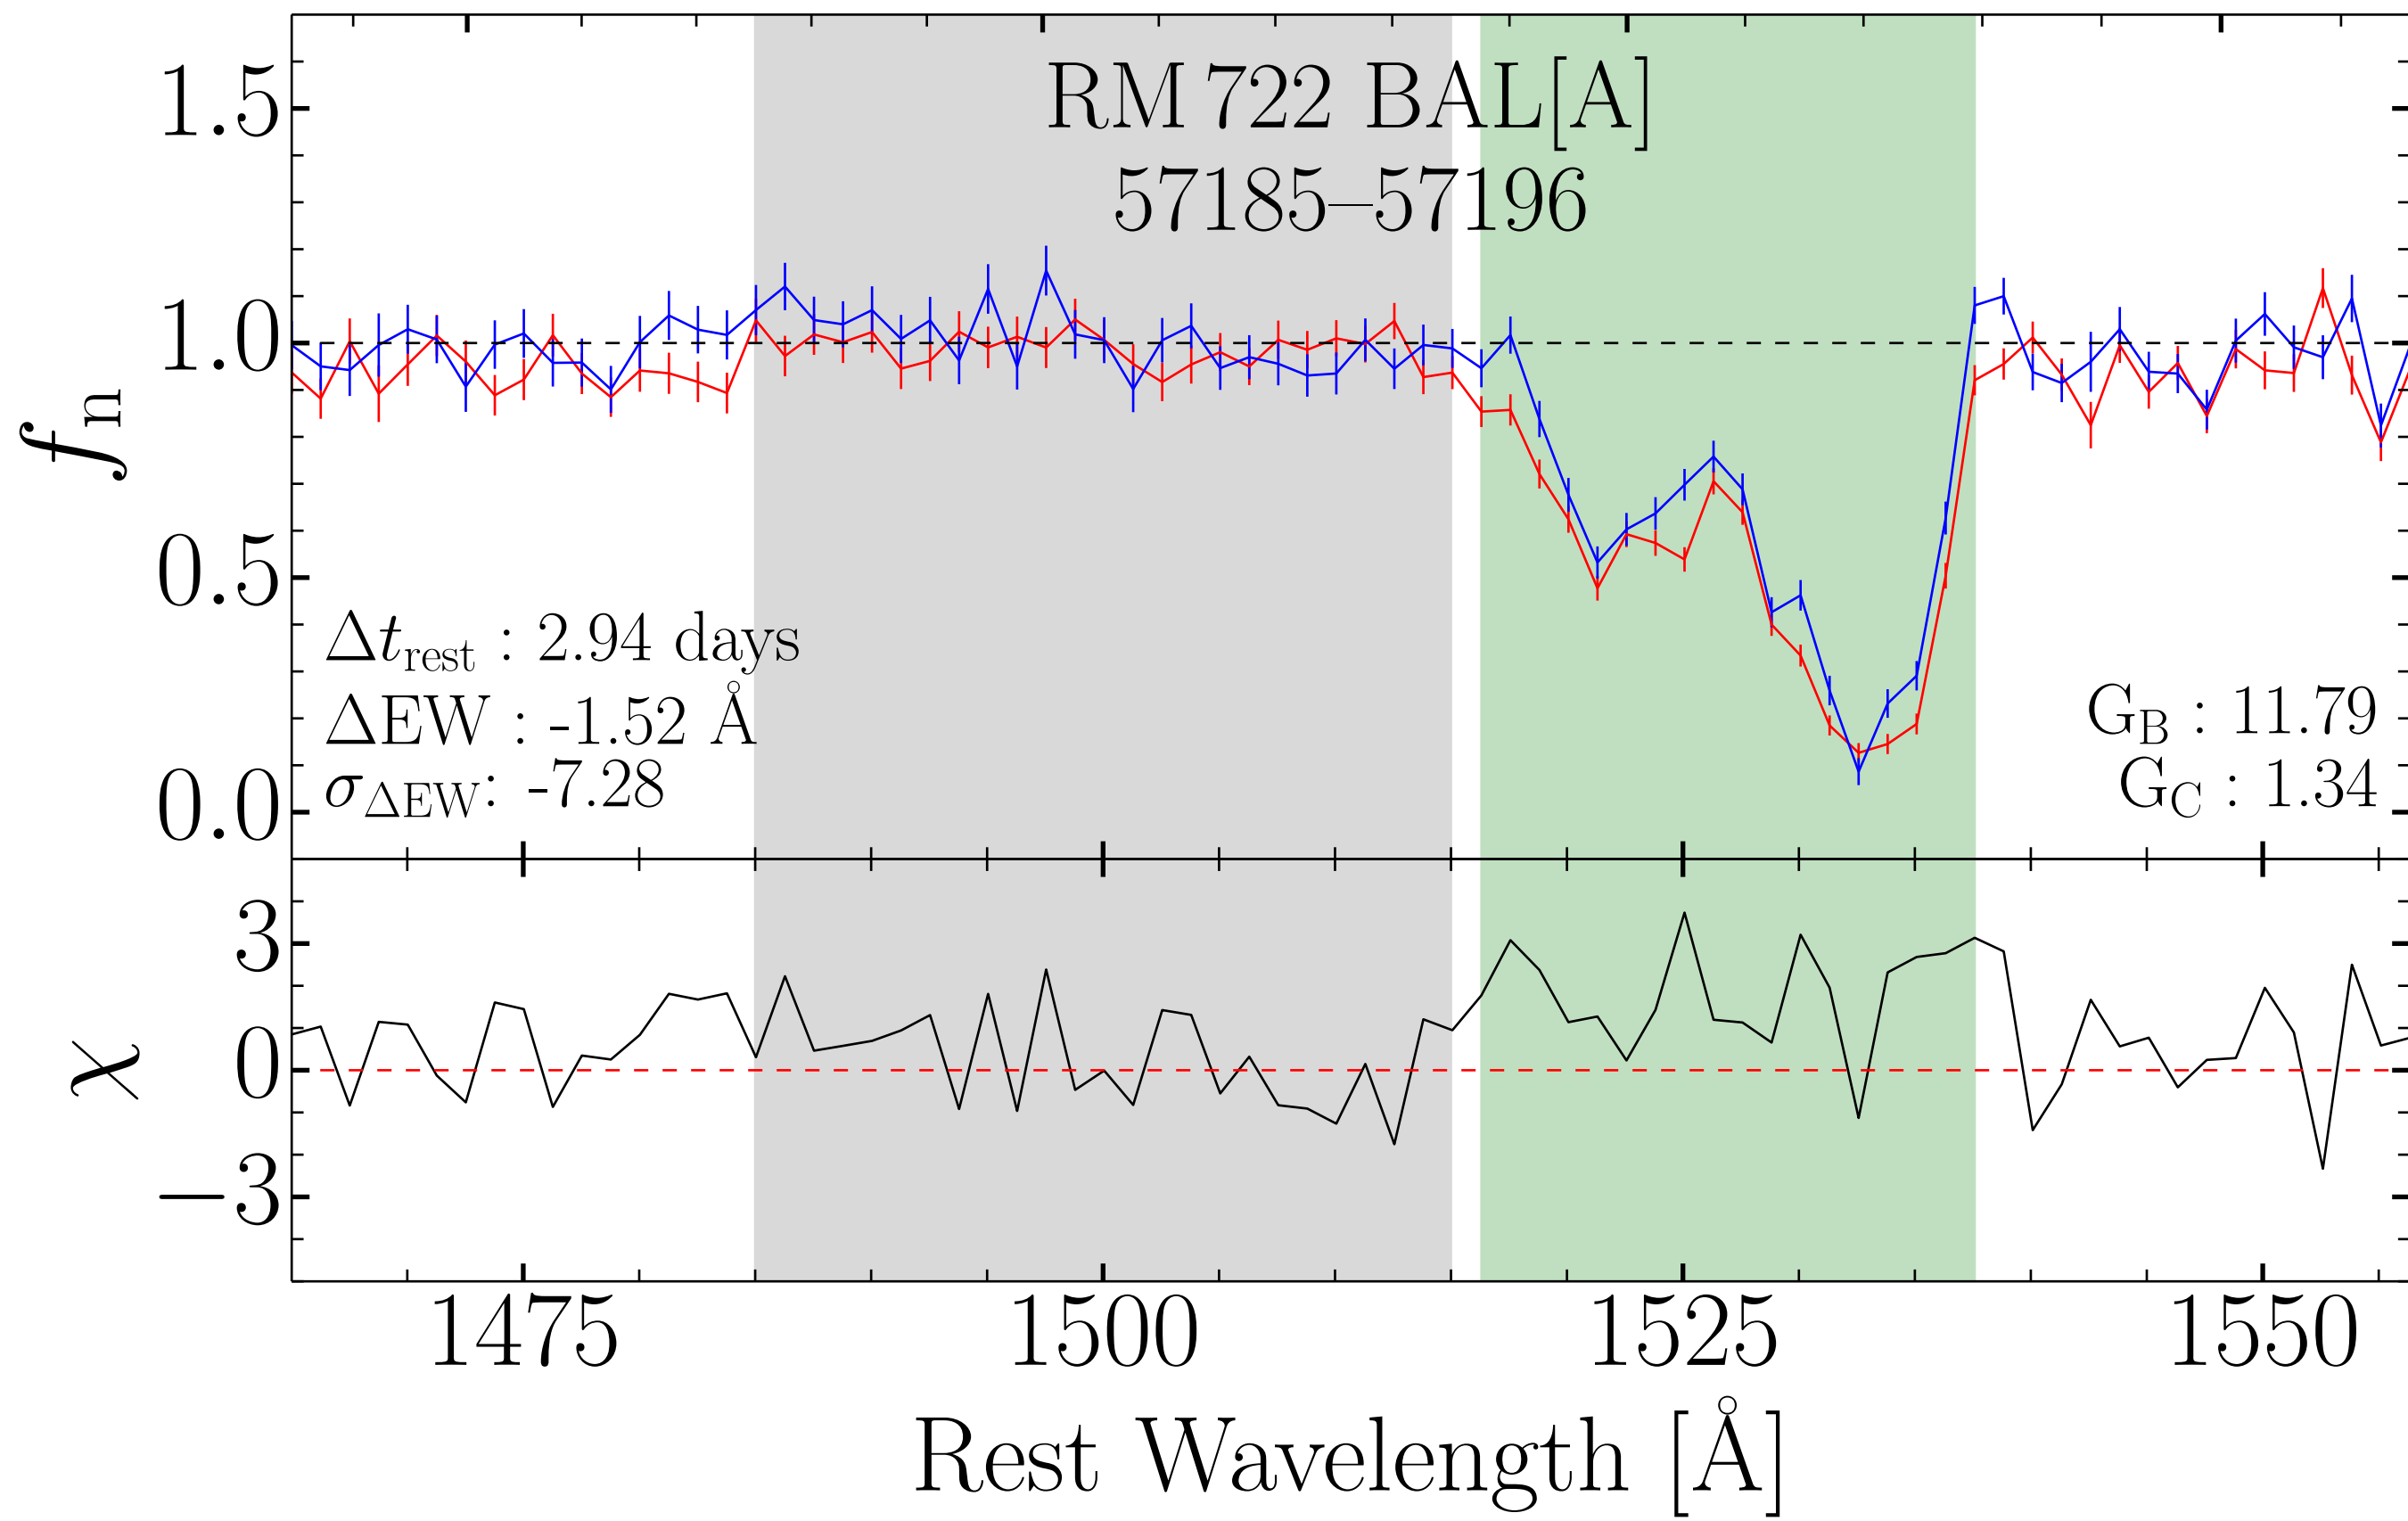

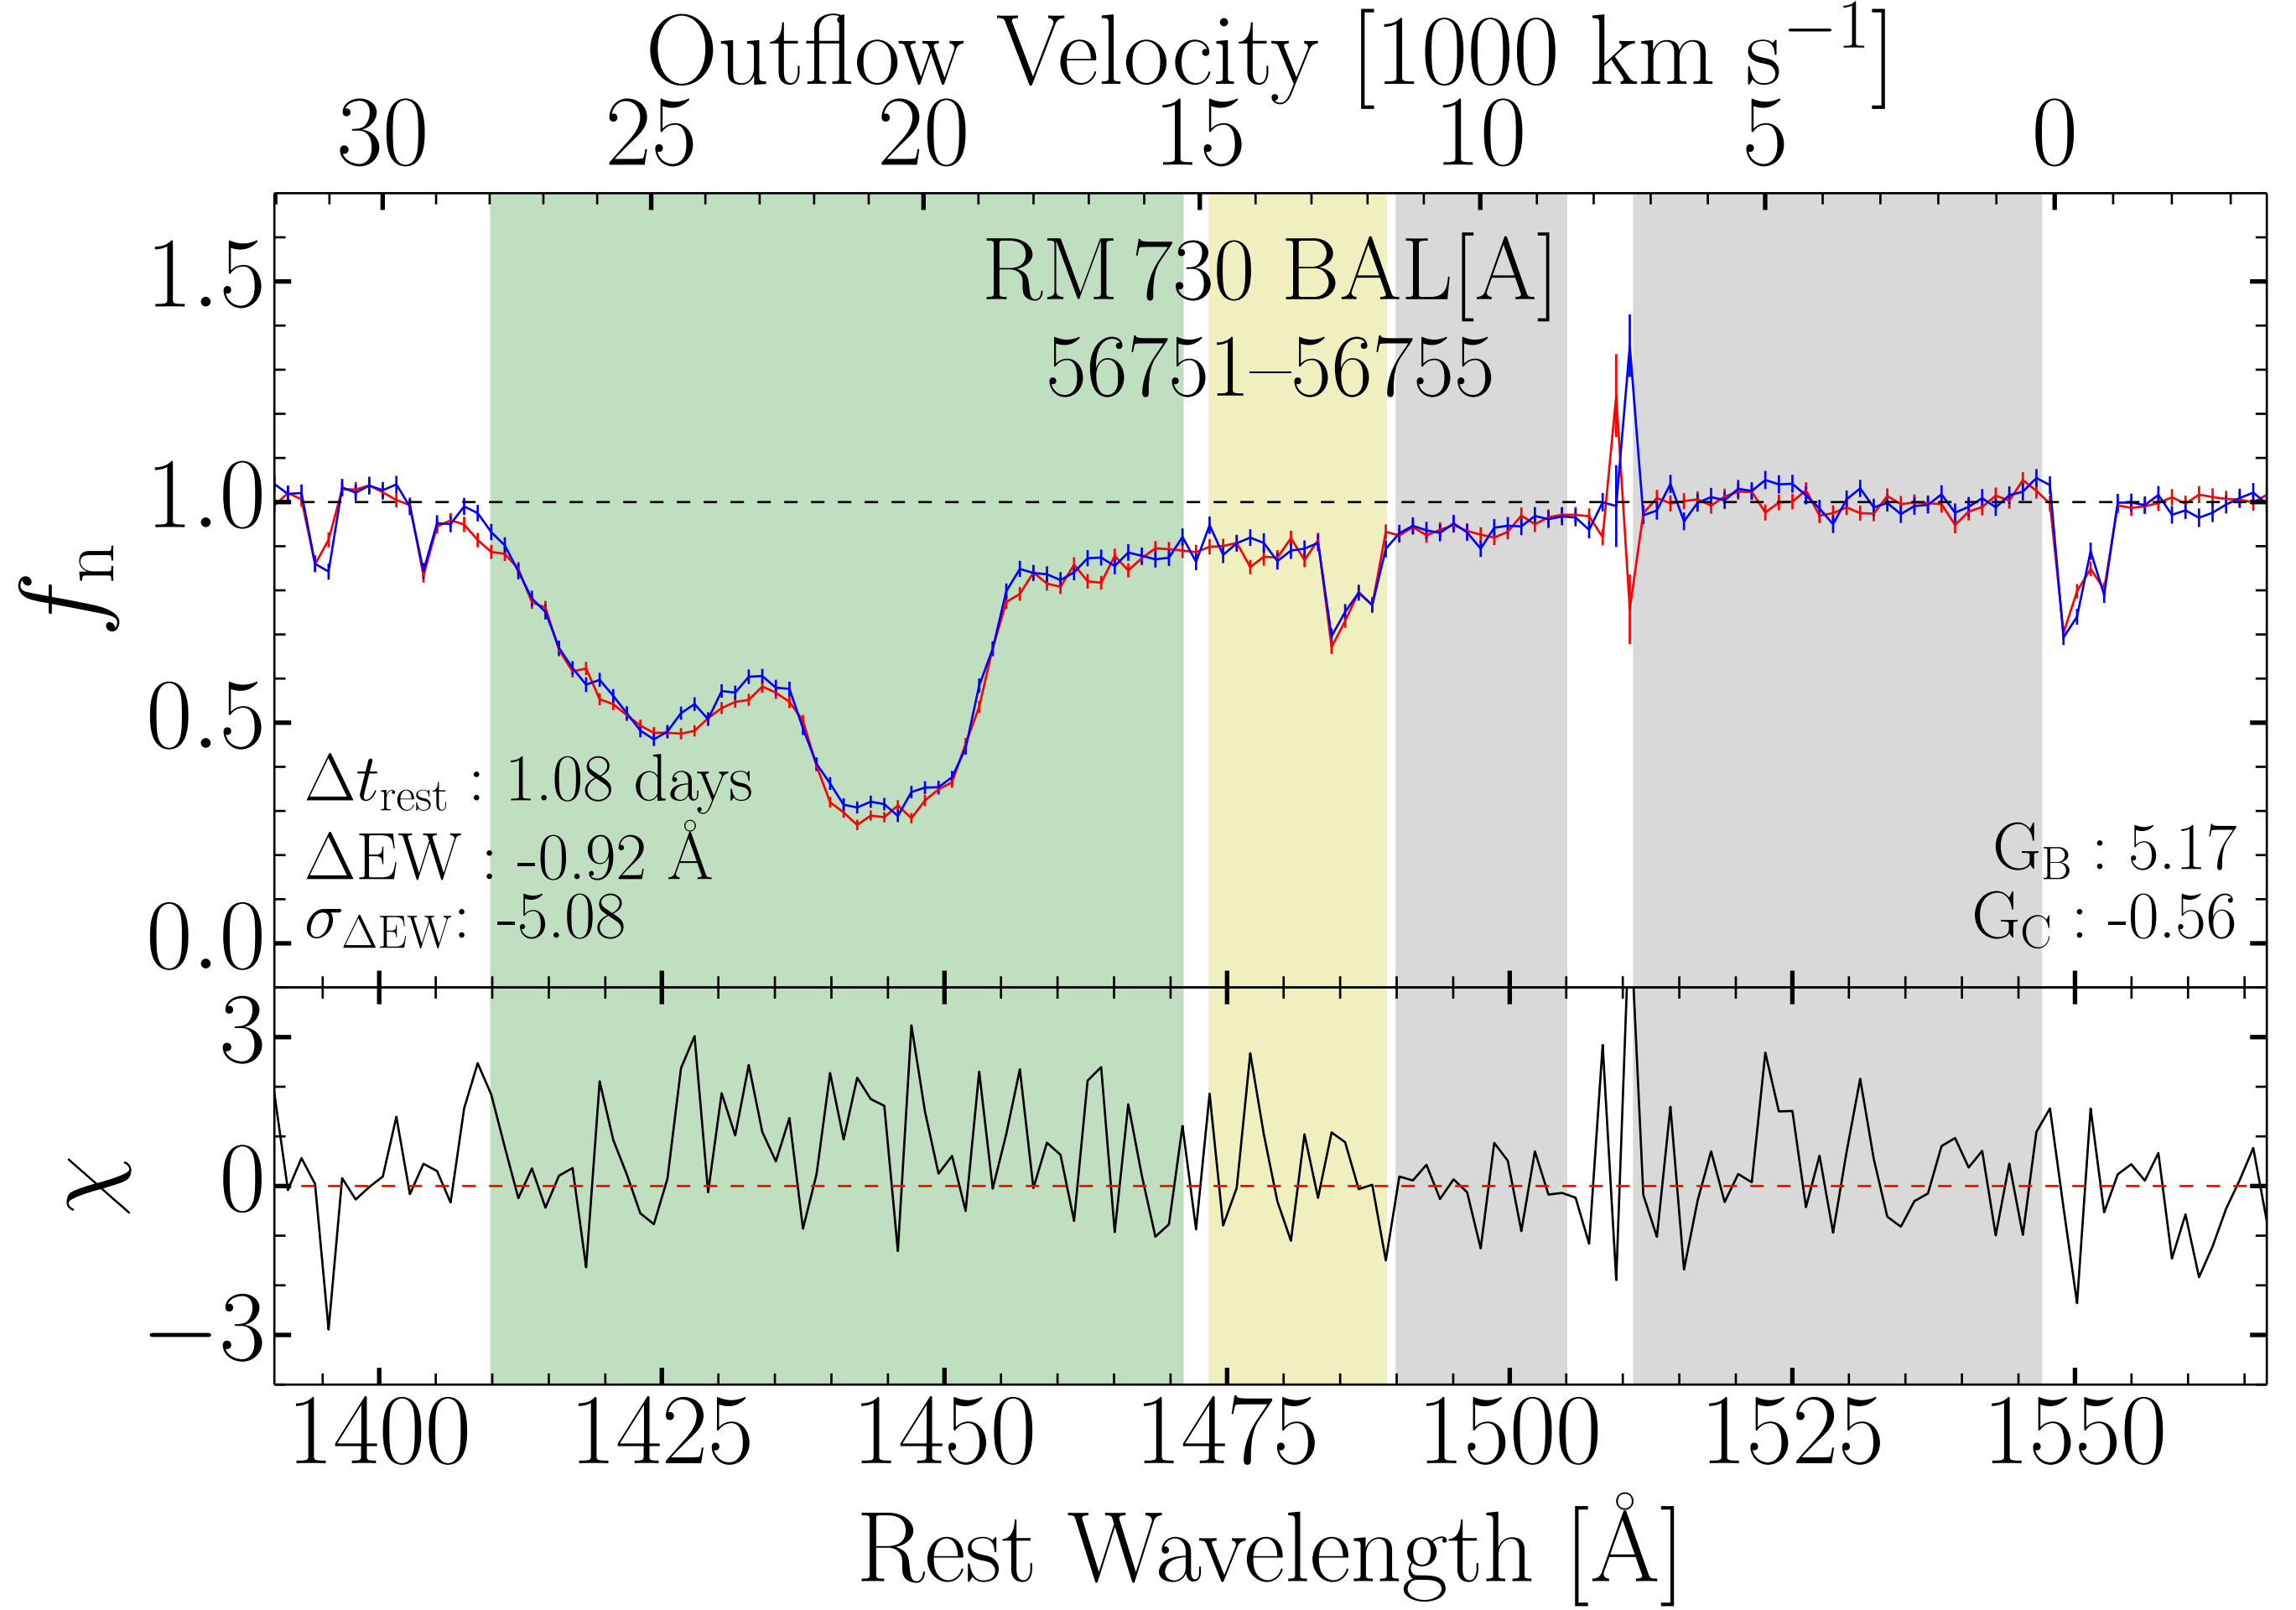



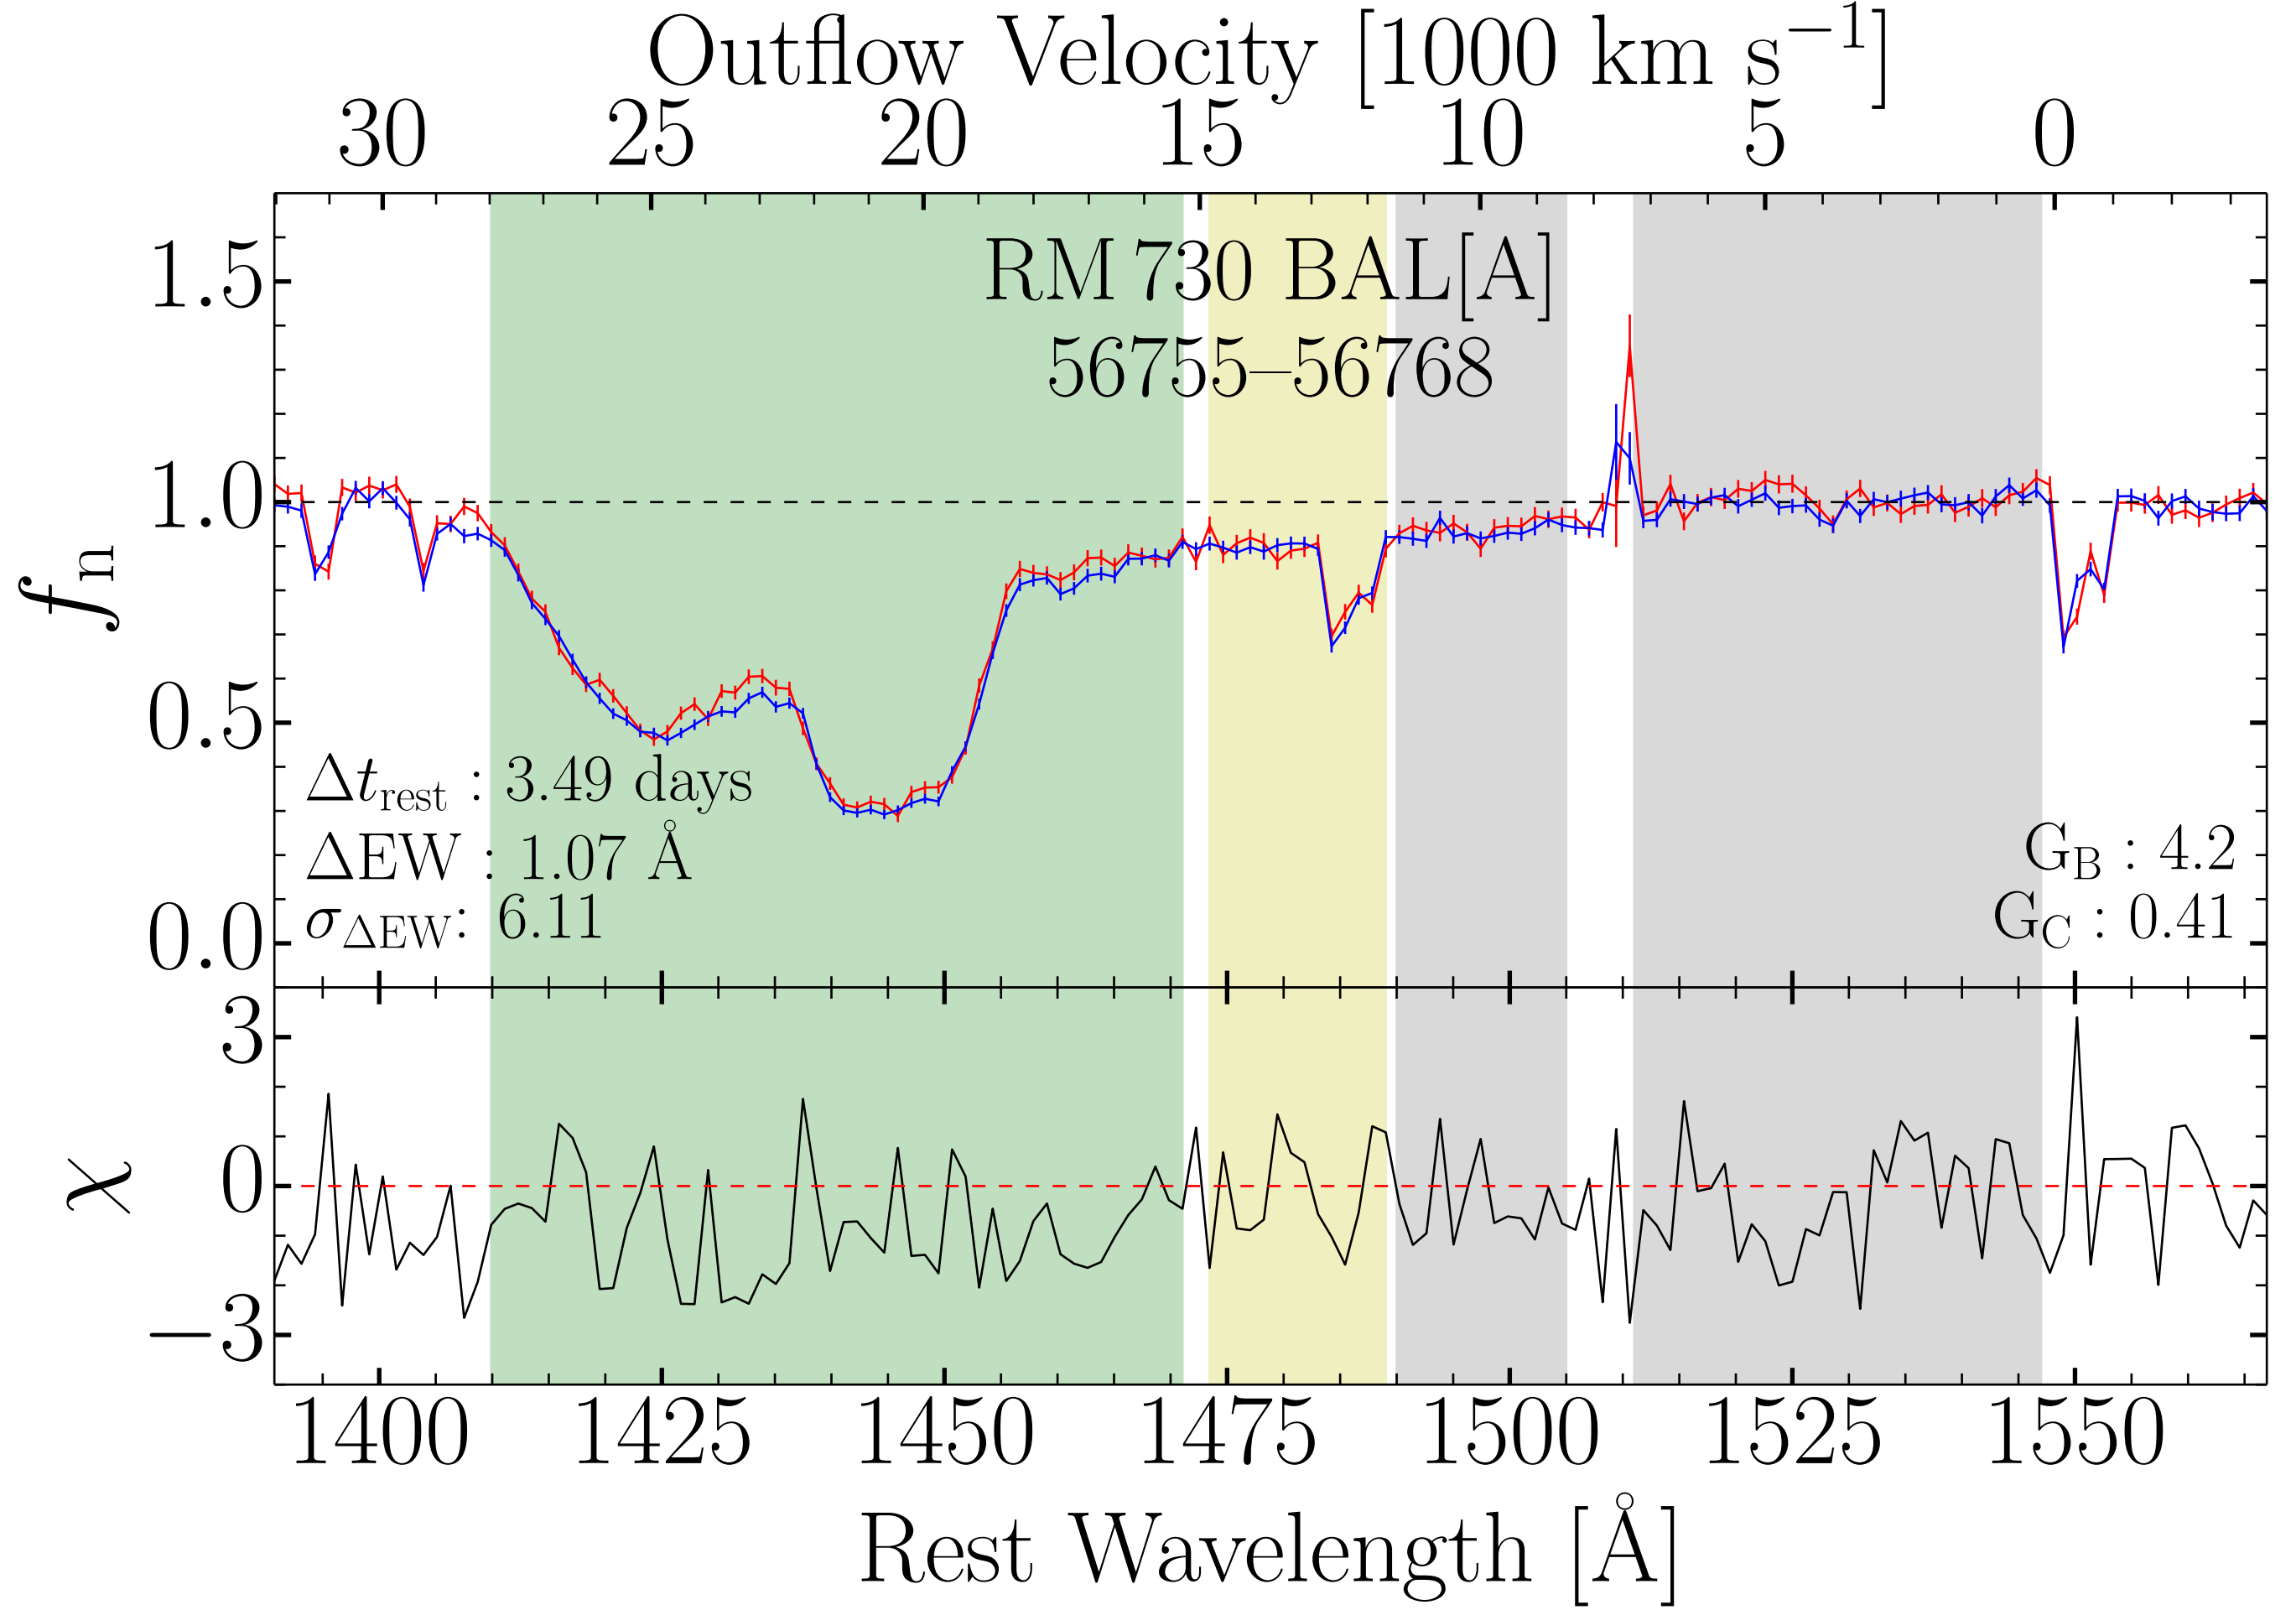

Outflow Velocity [ $1000 \text{ km s}^{-1}$ ]

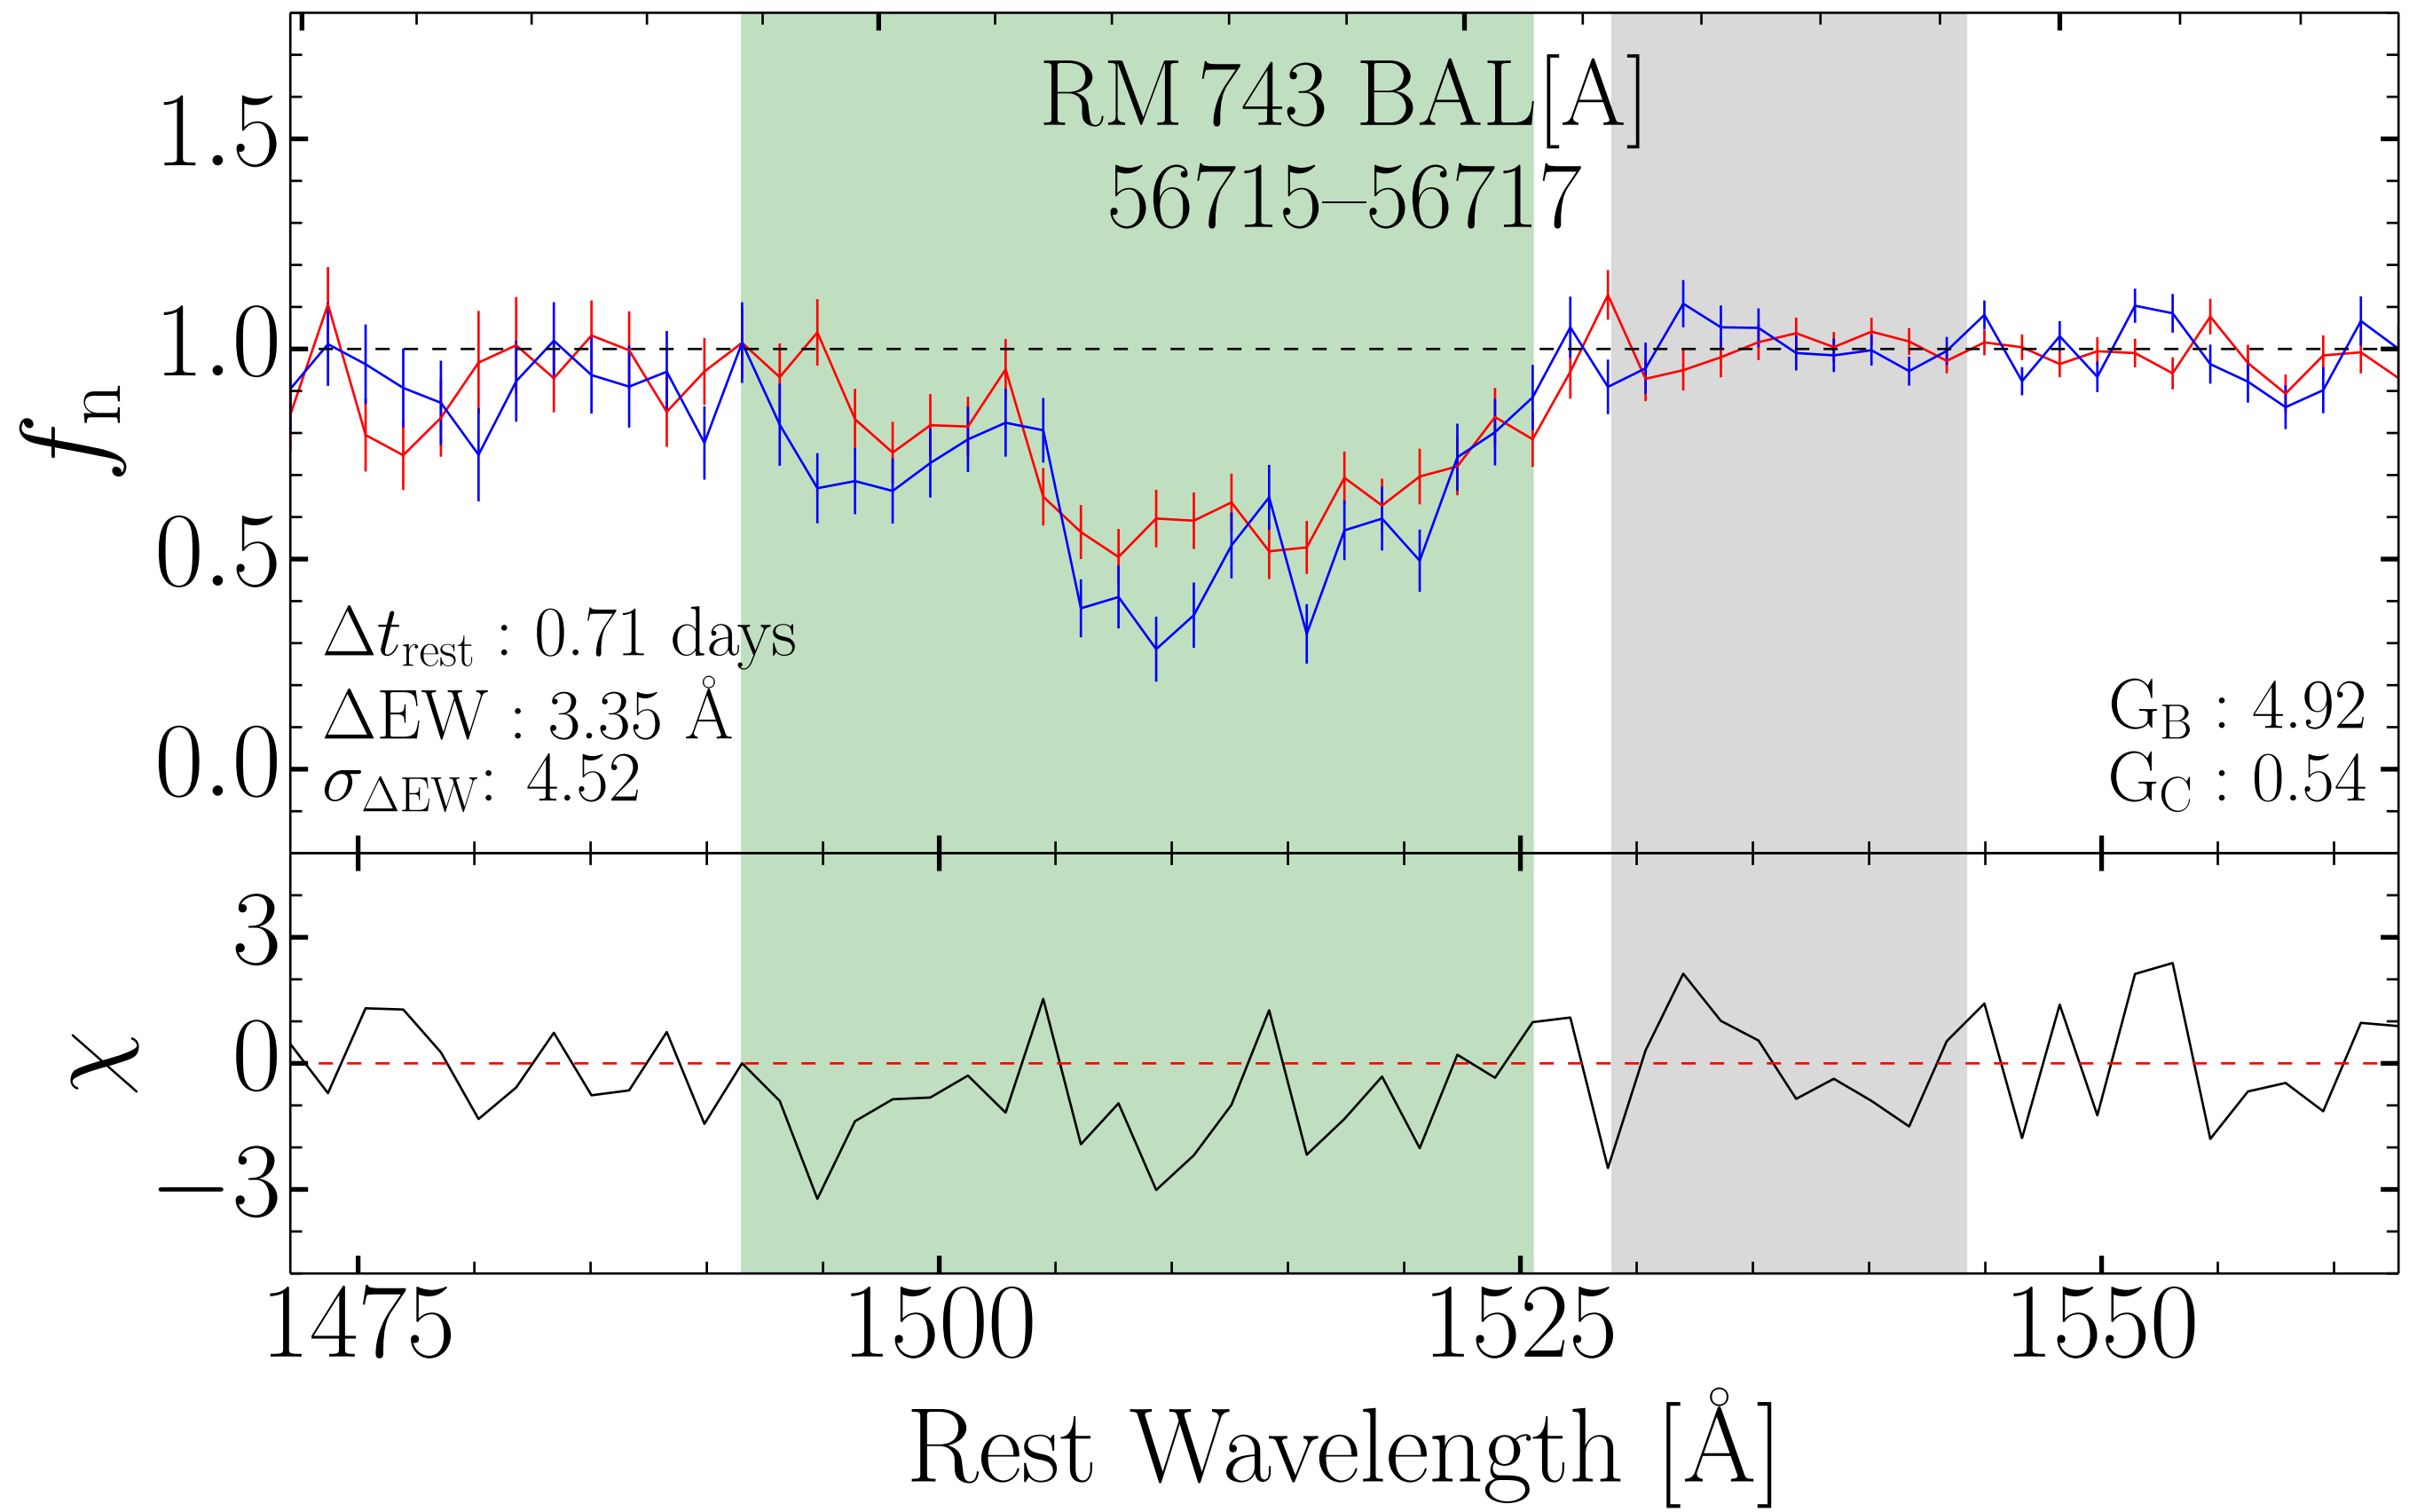

Outflow Velocity [1000 km s<sup>-1</sup>]

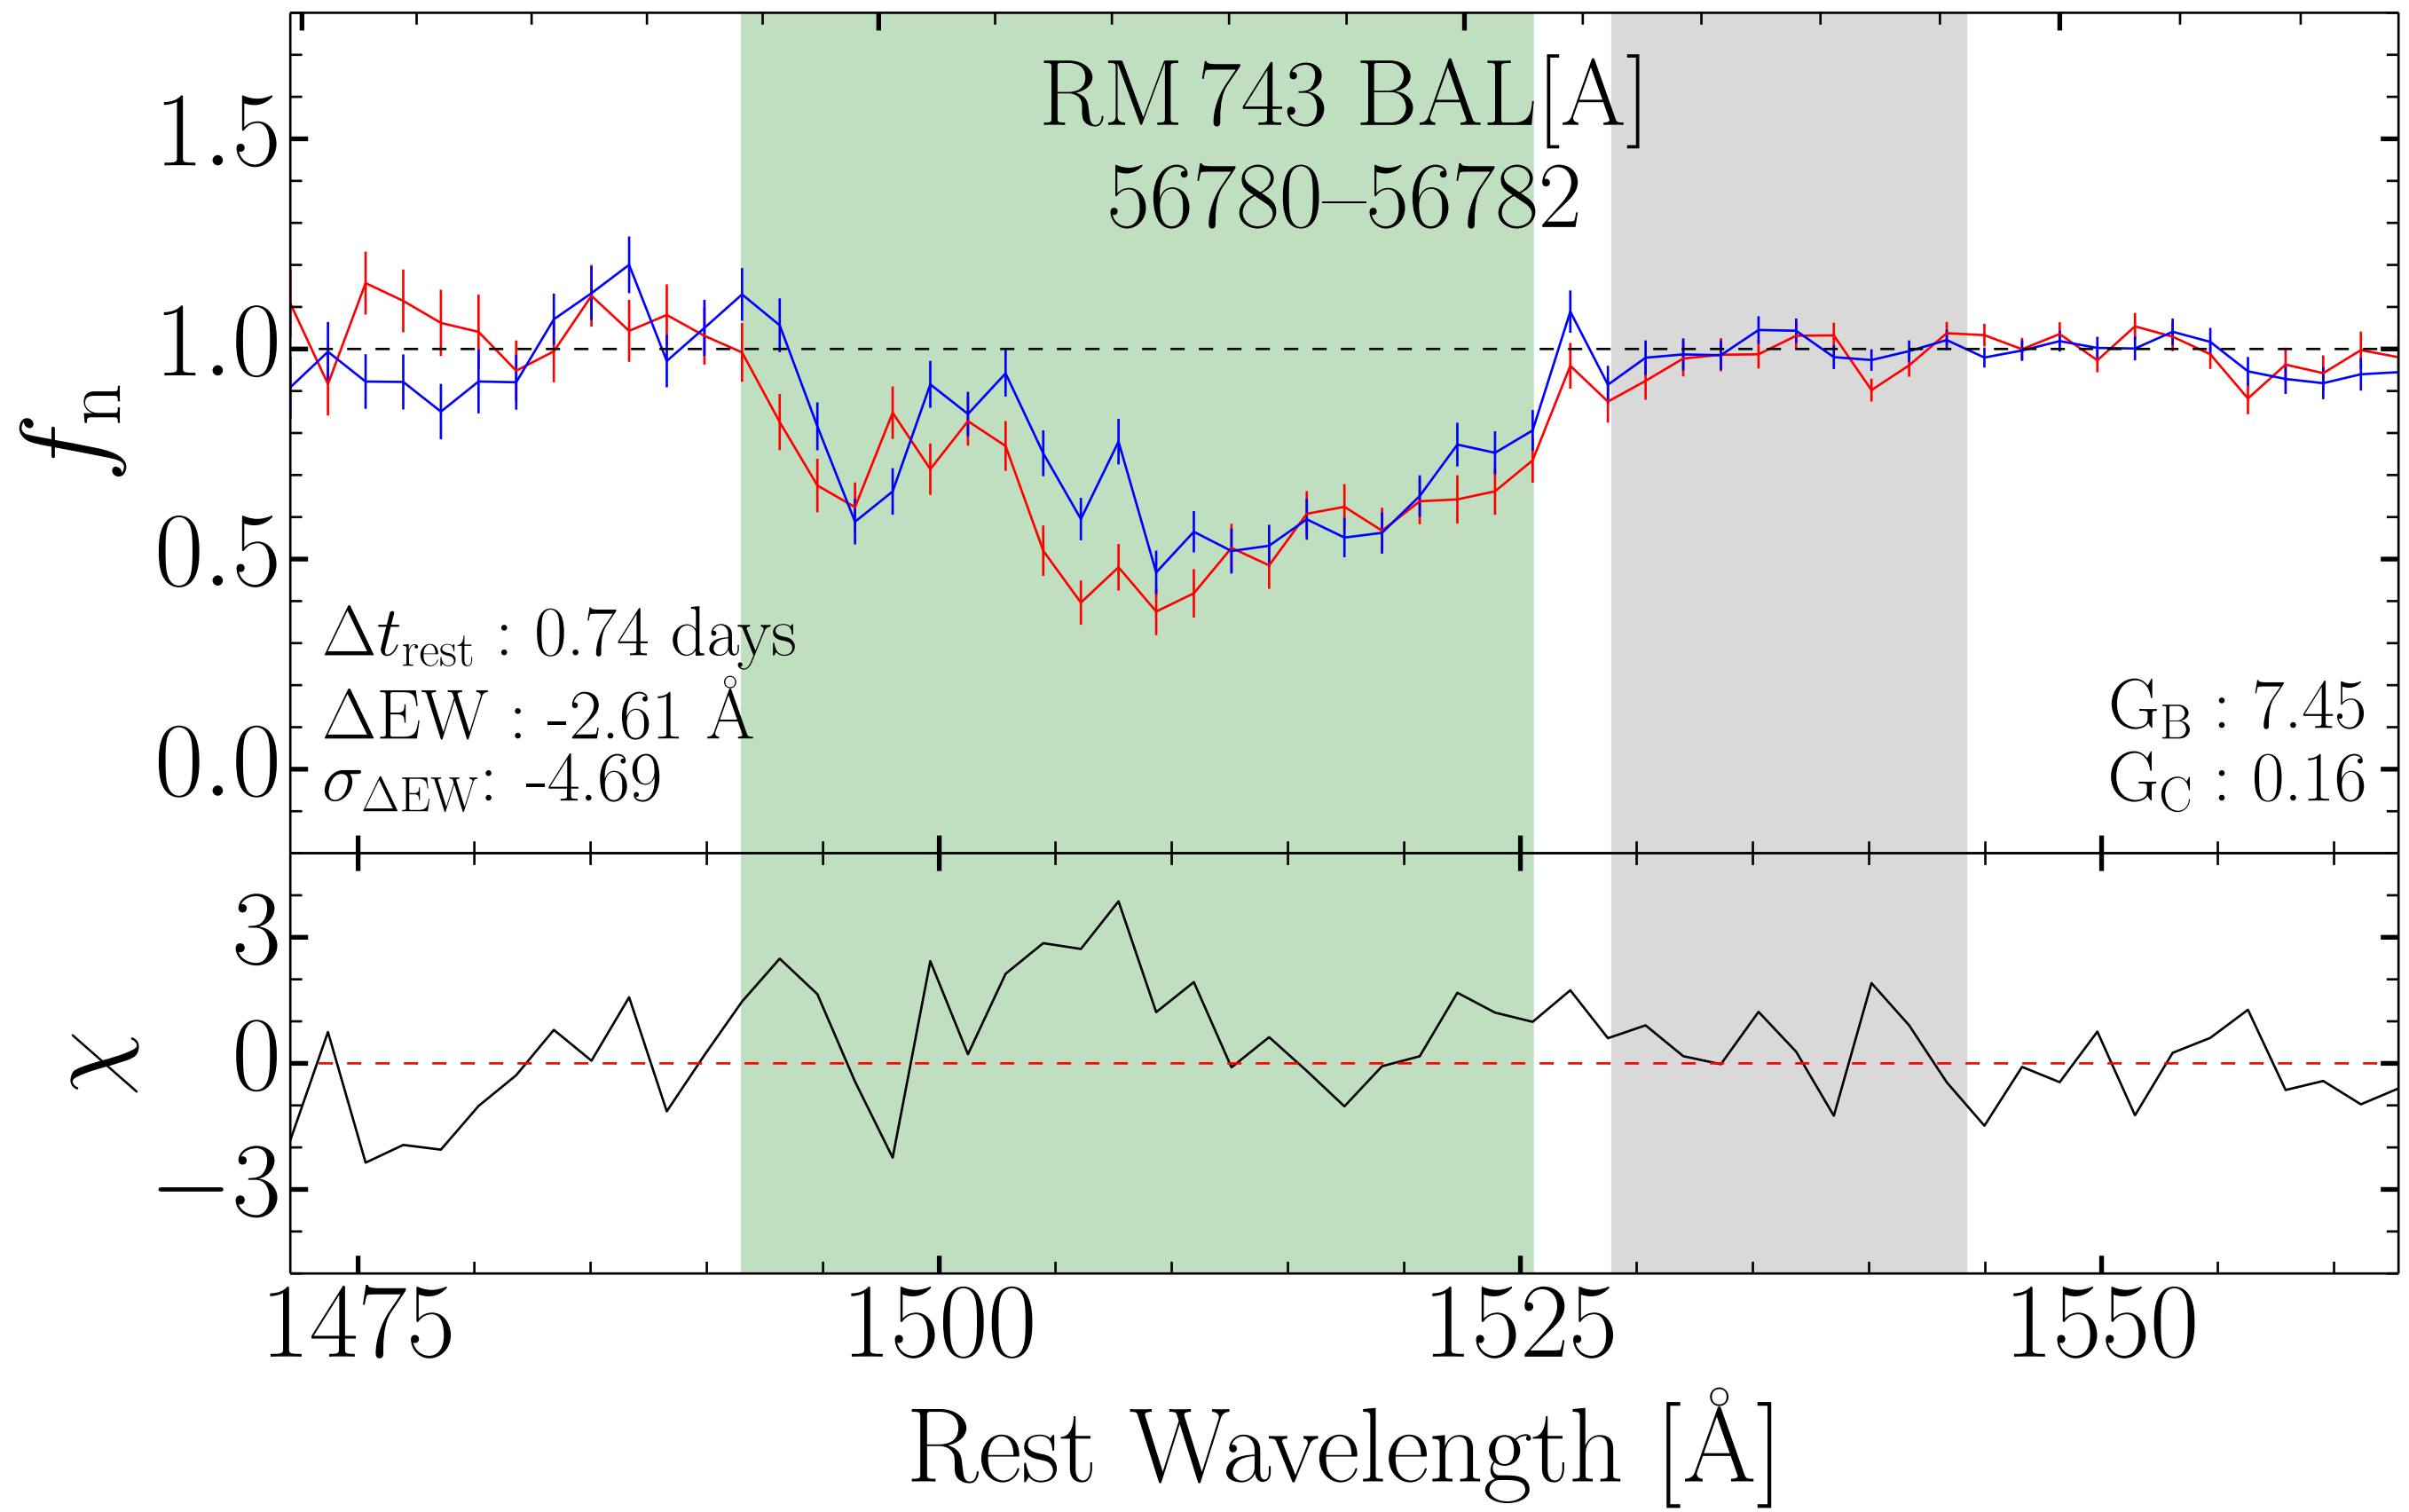

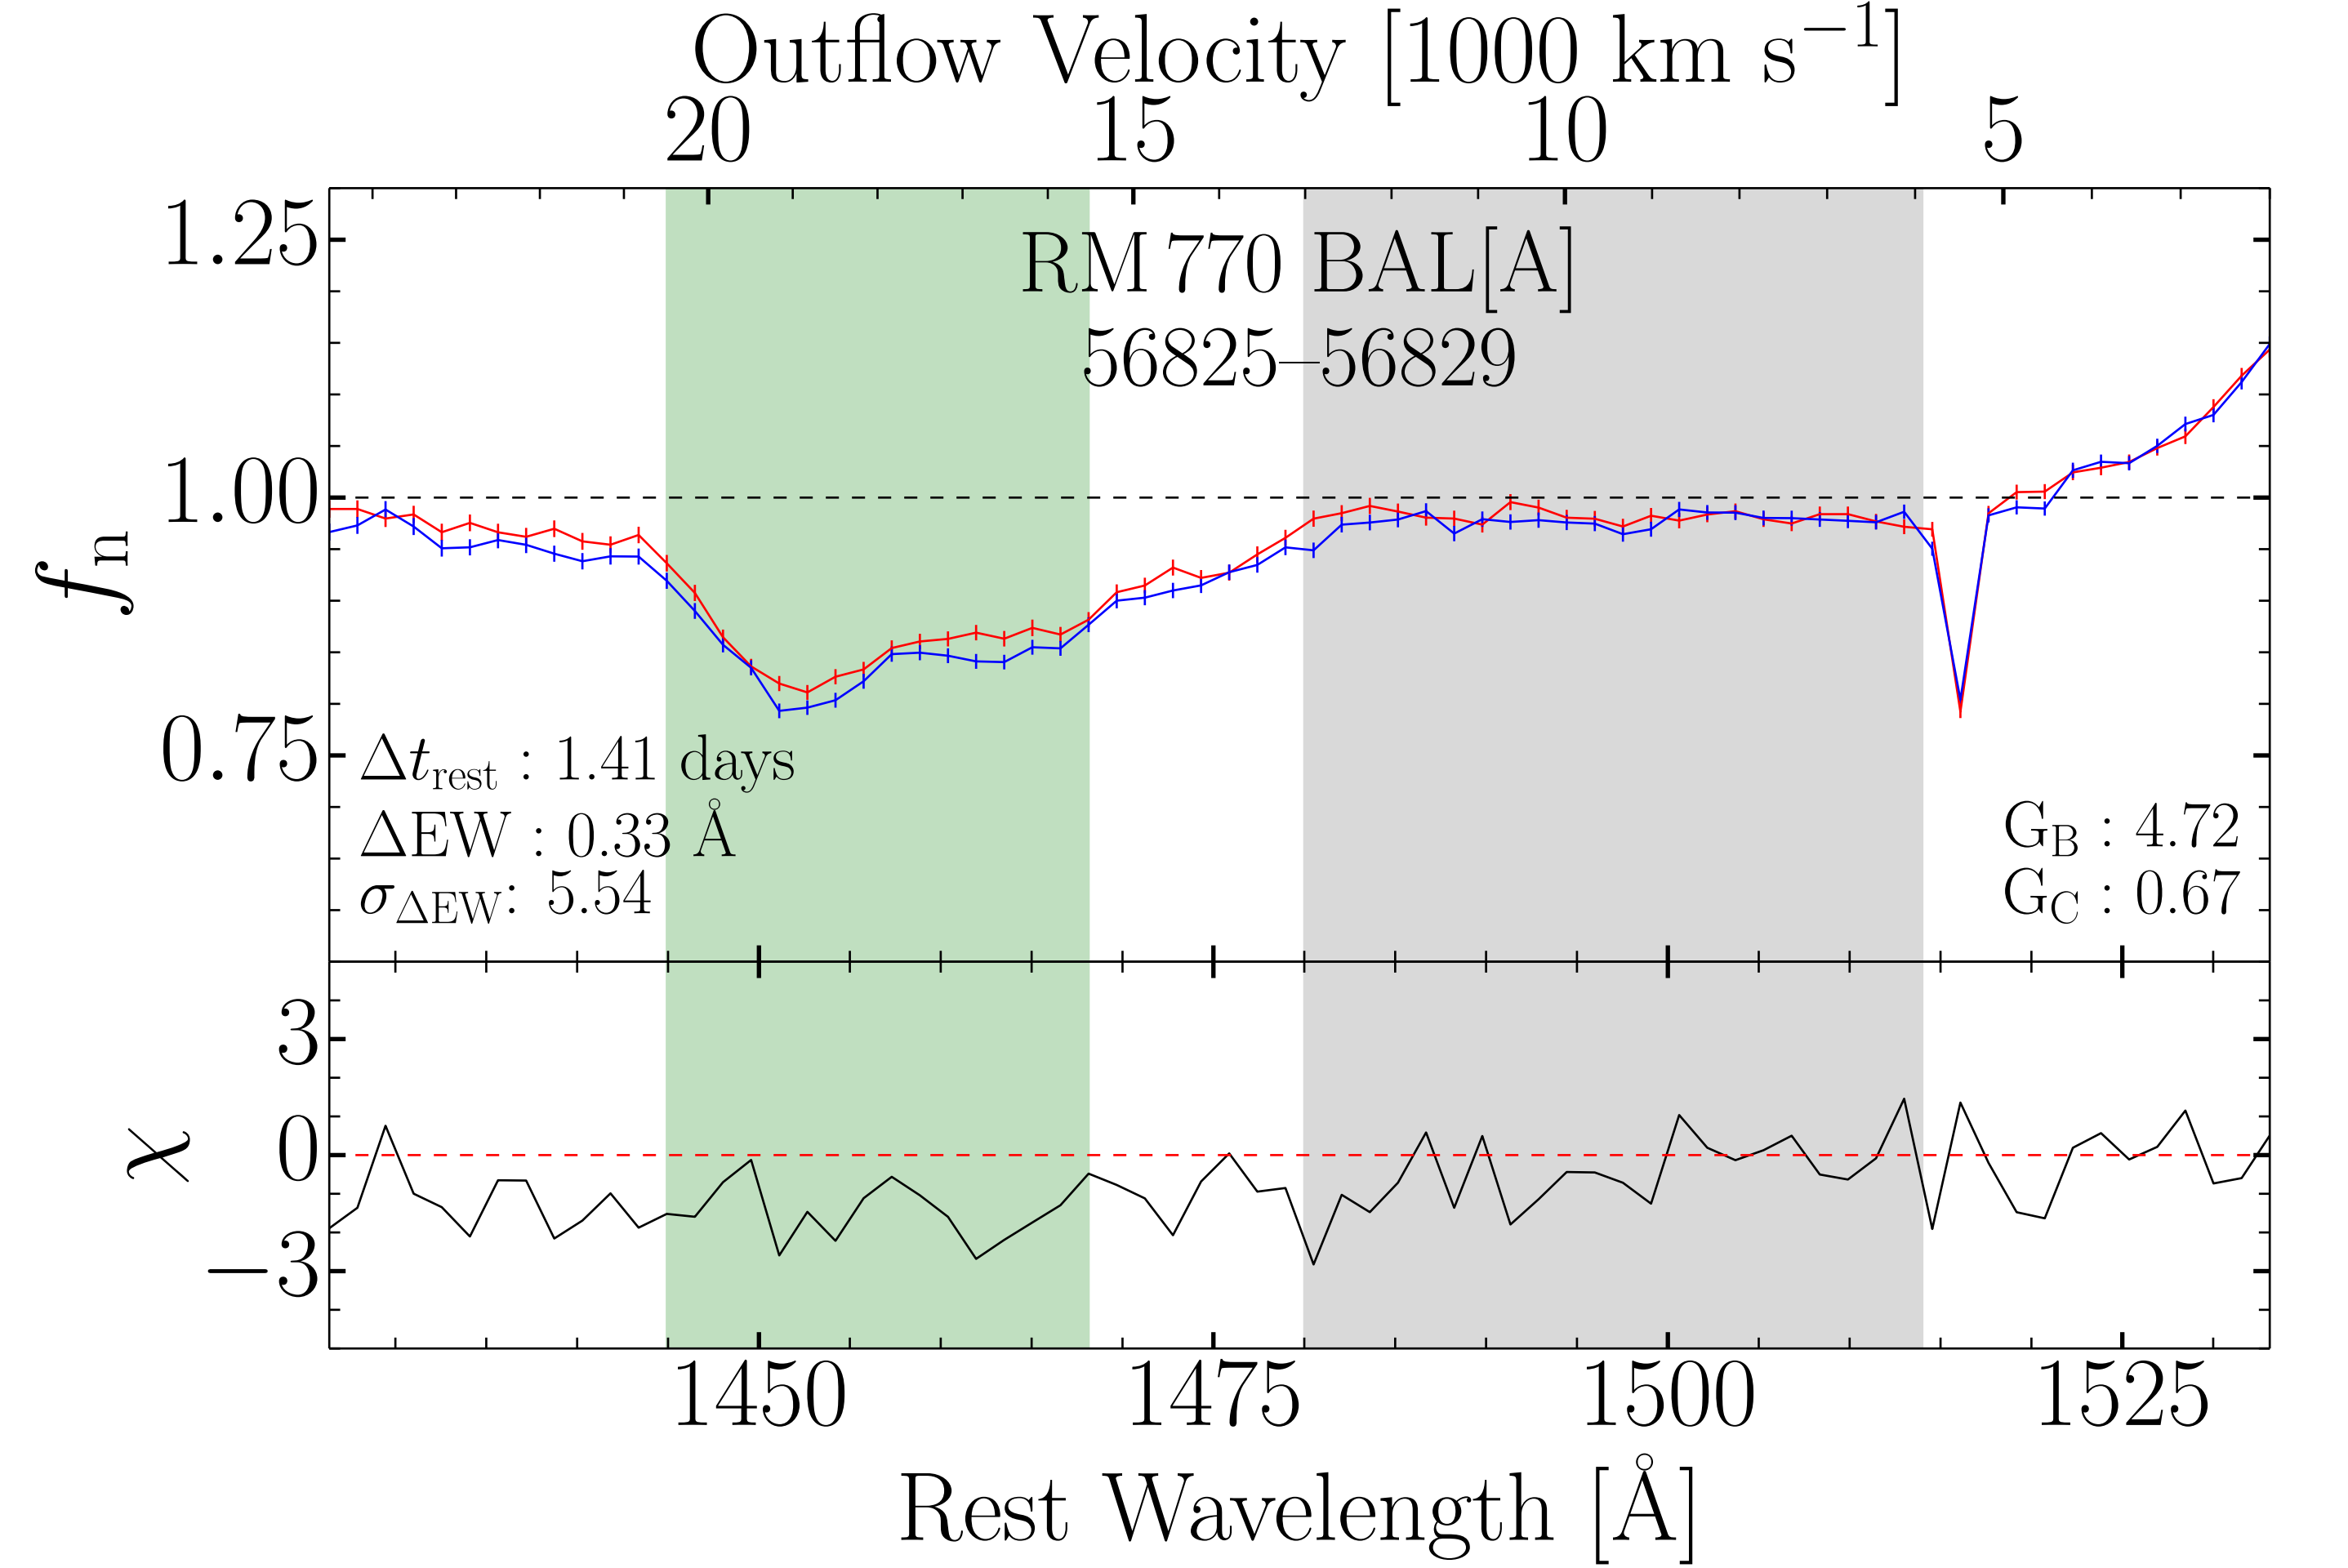

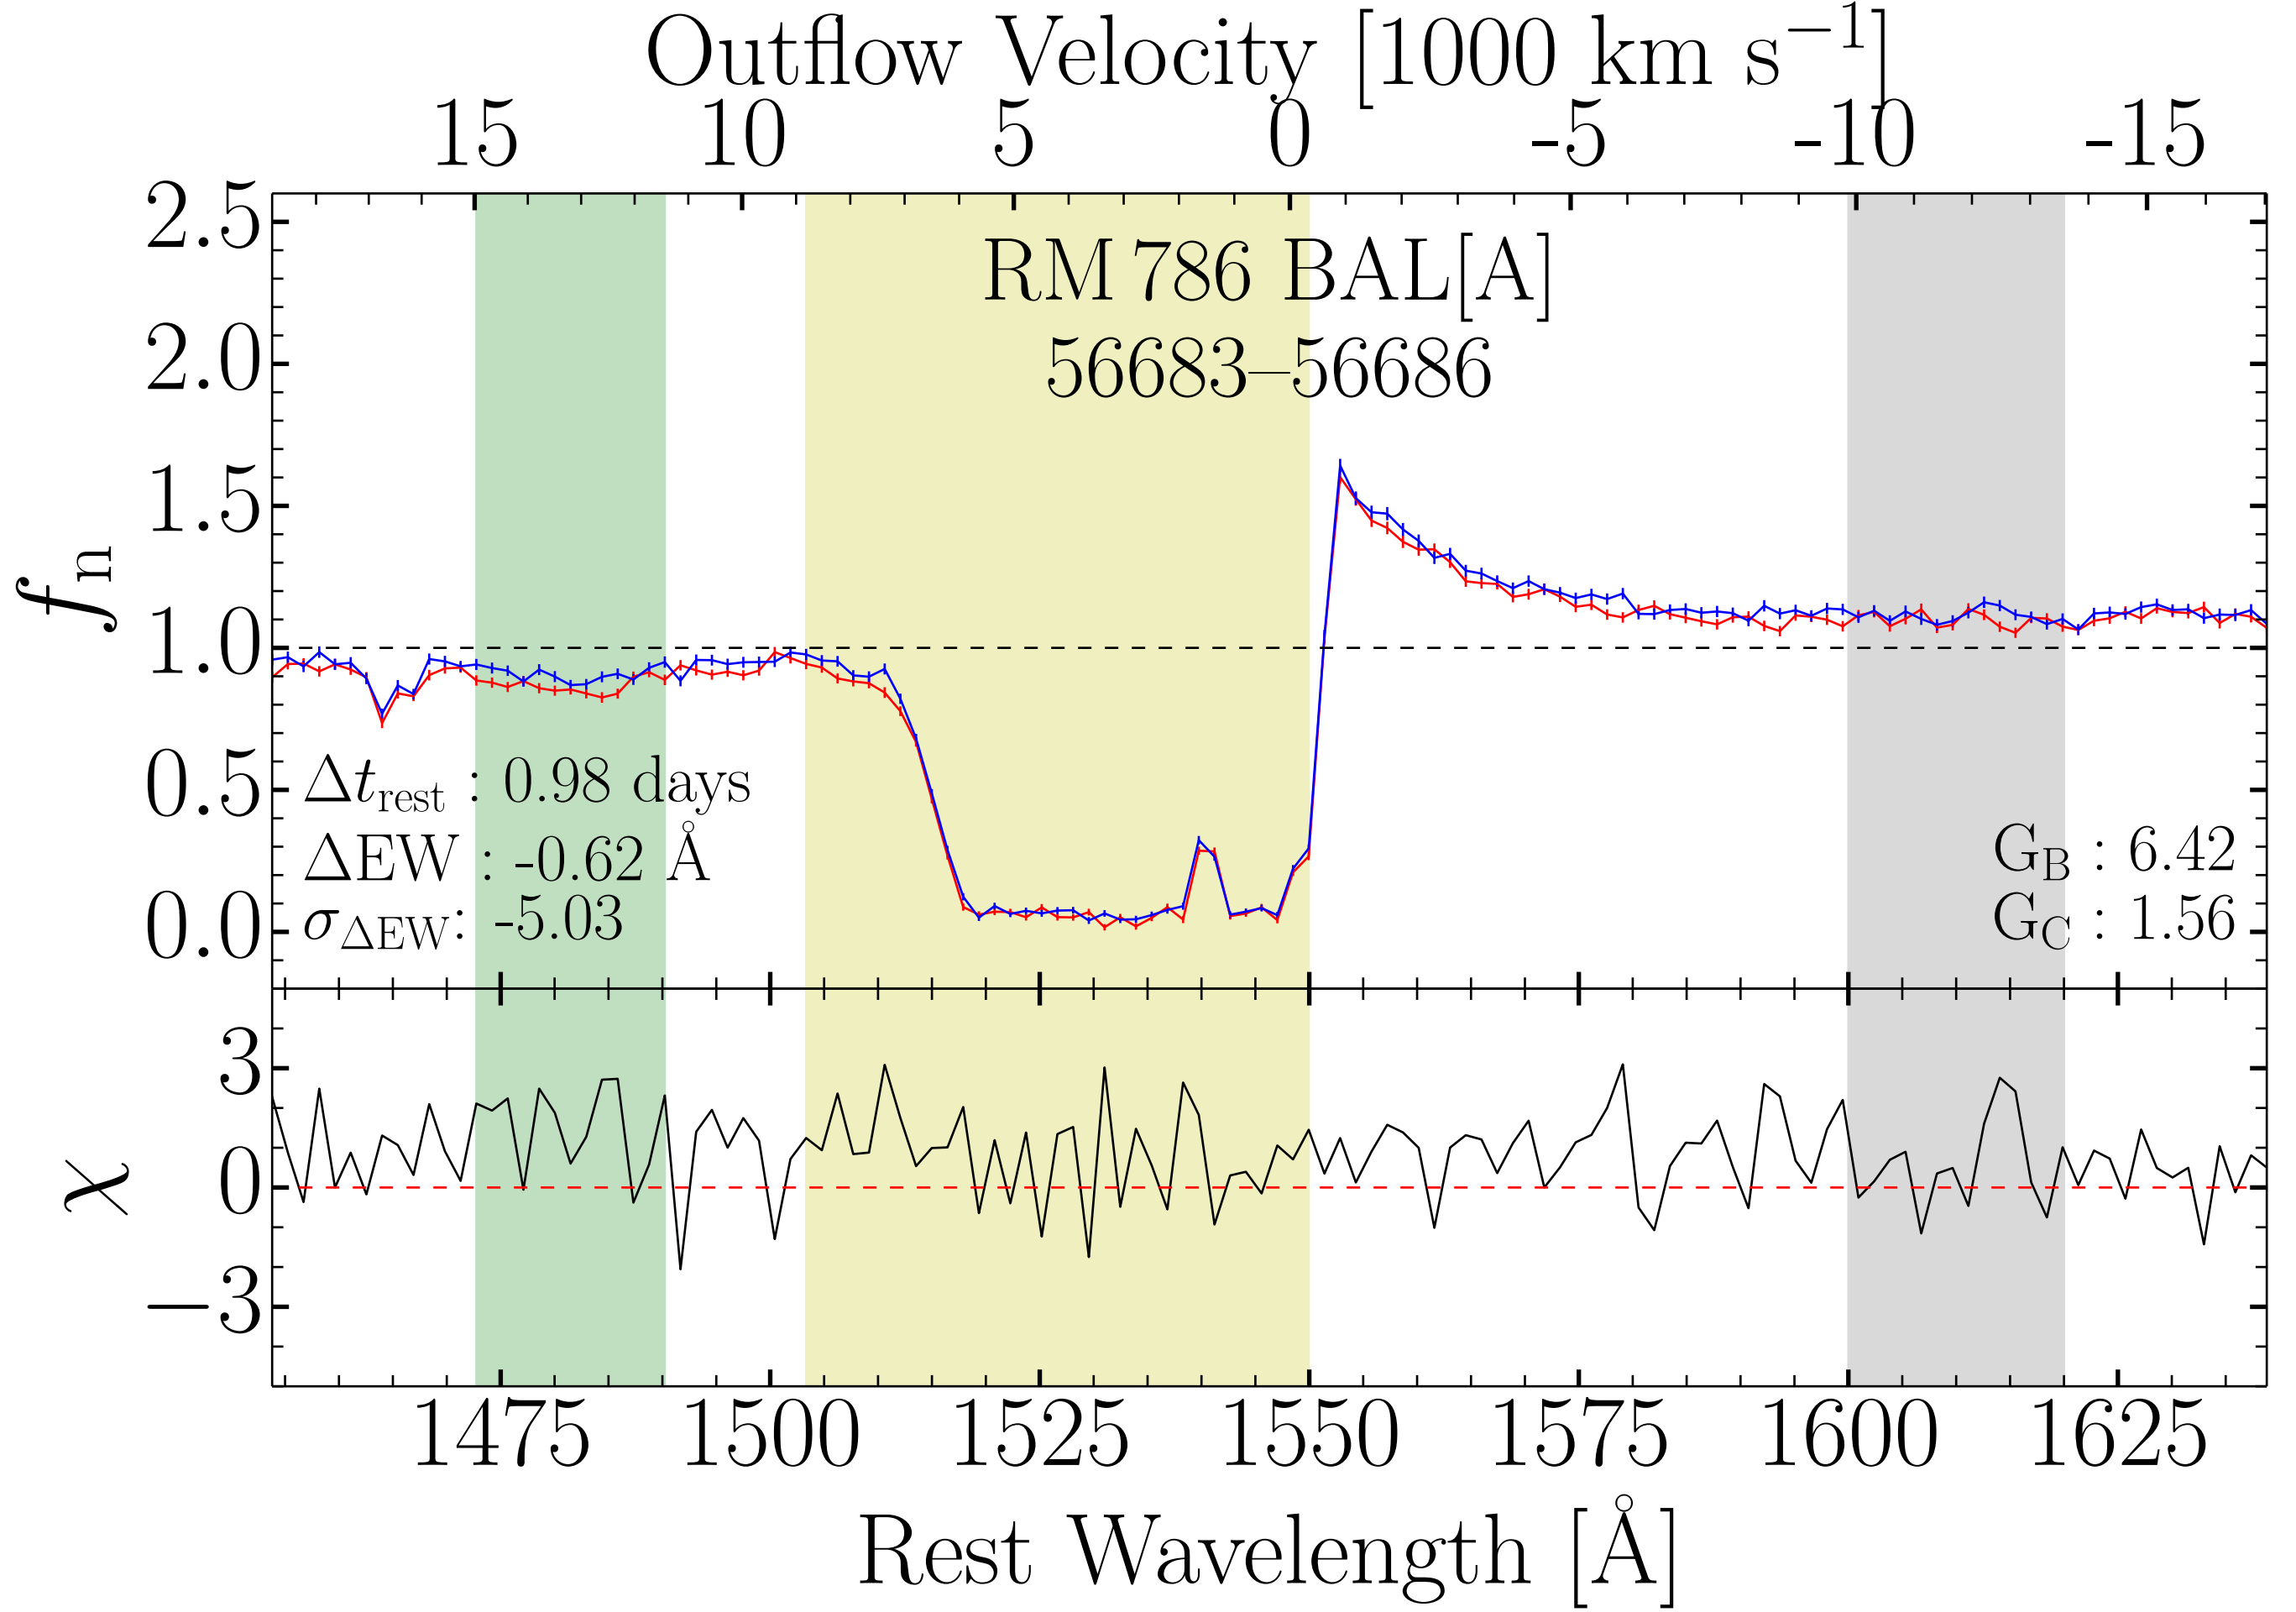

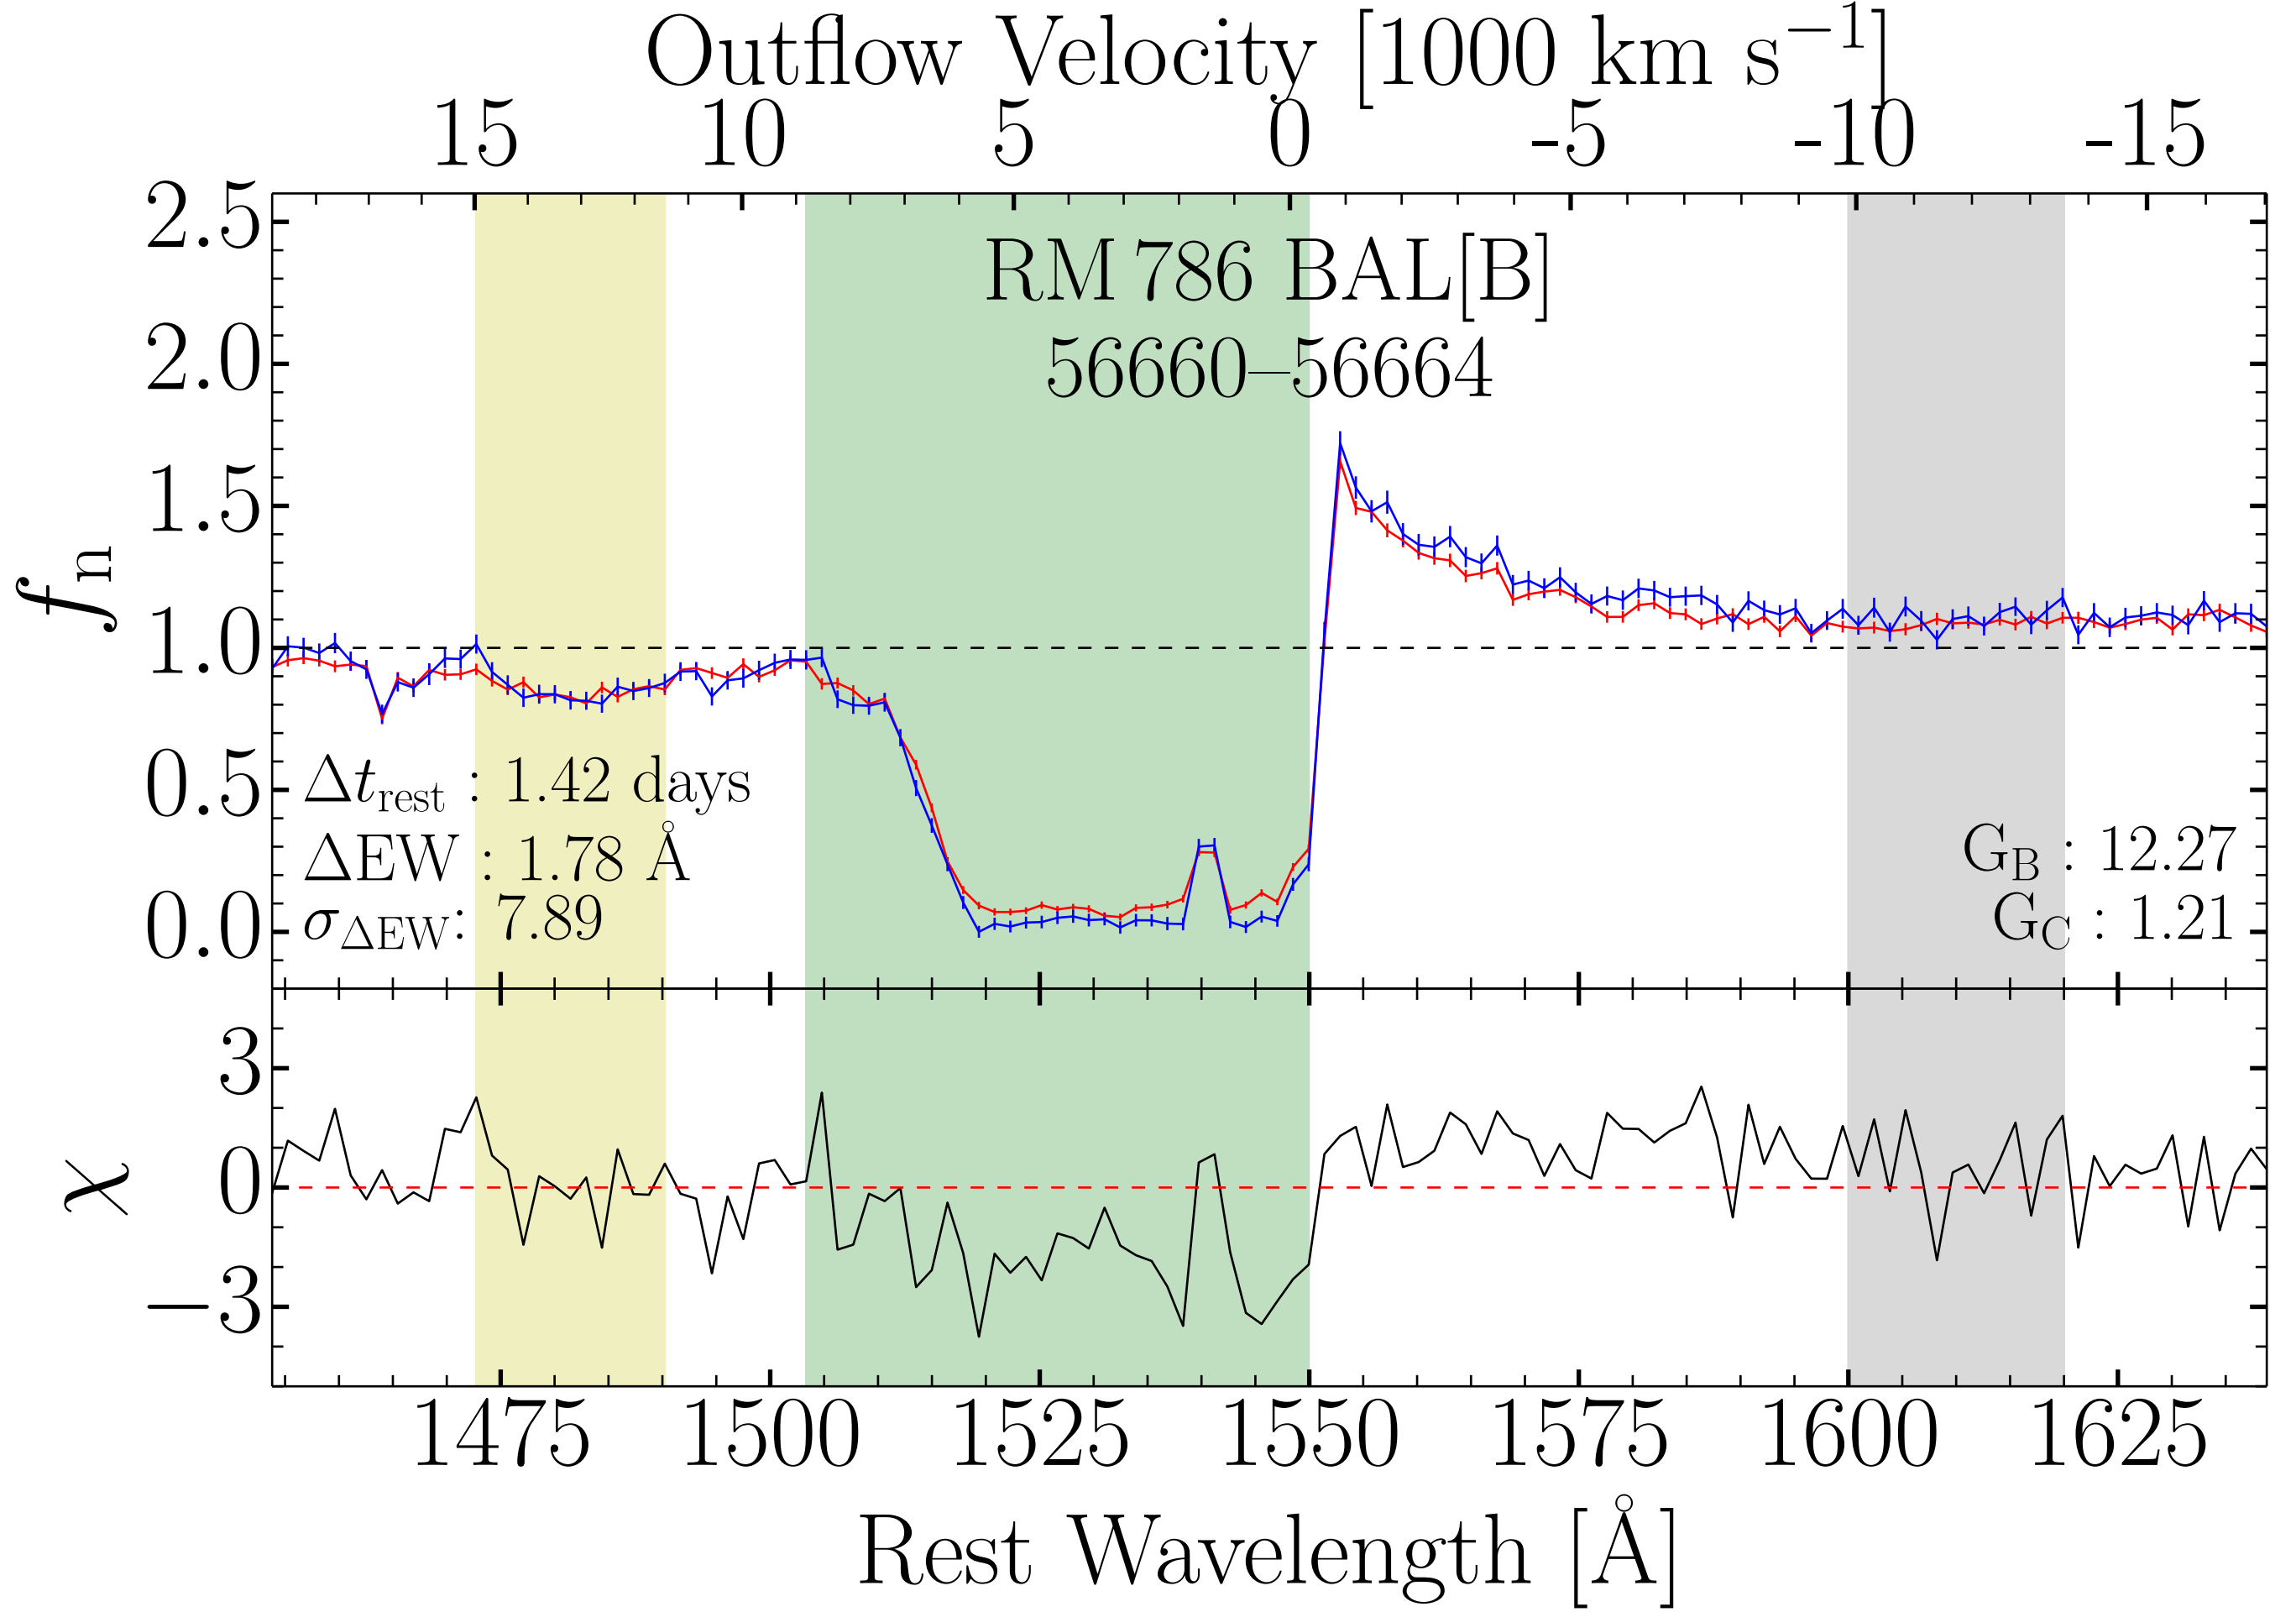

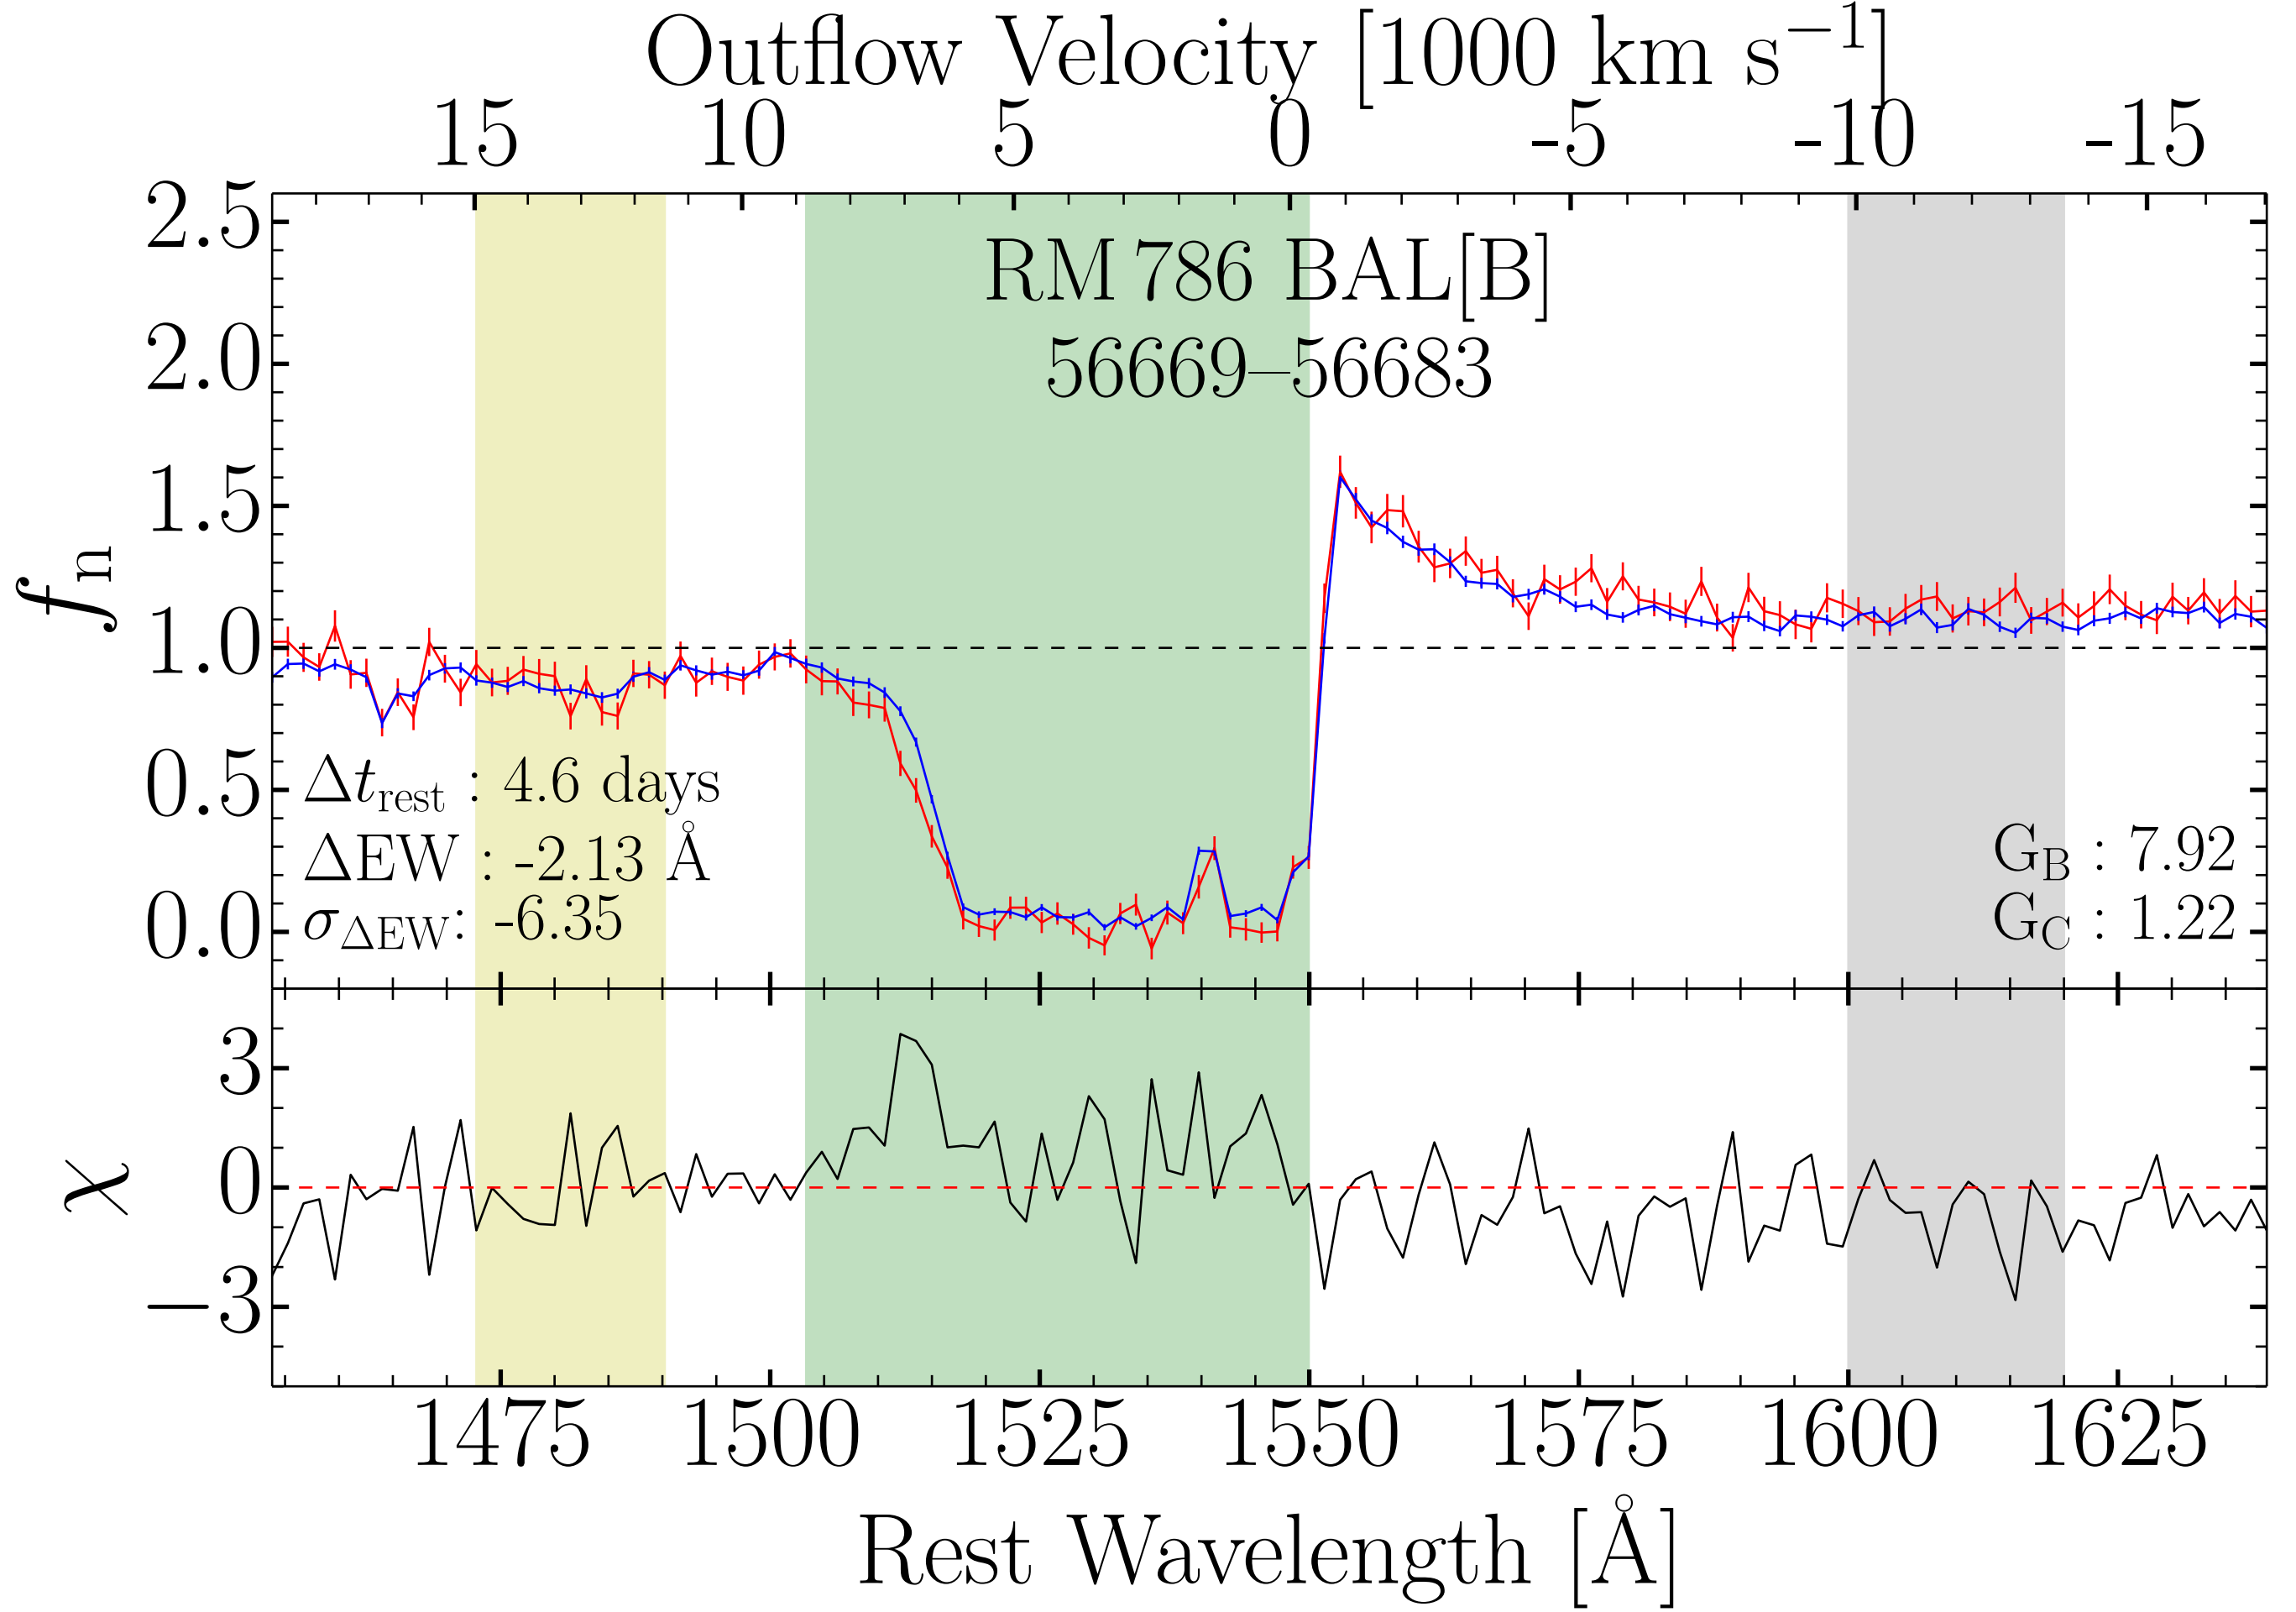

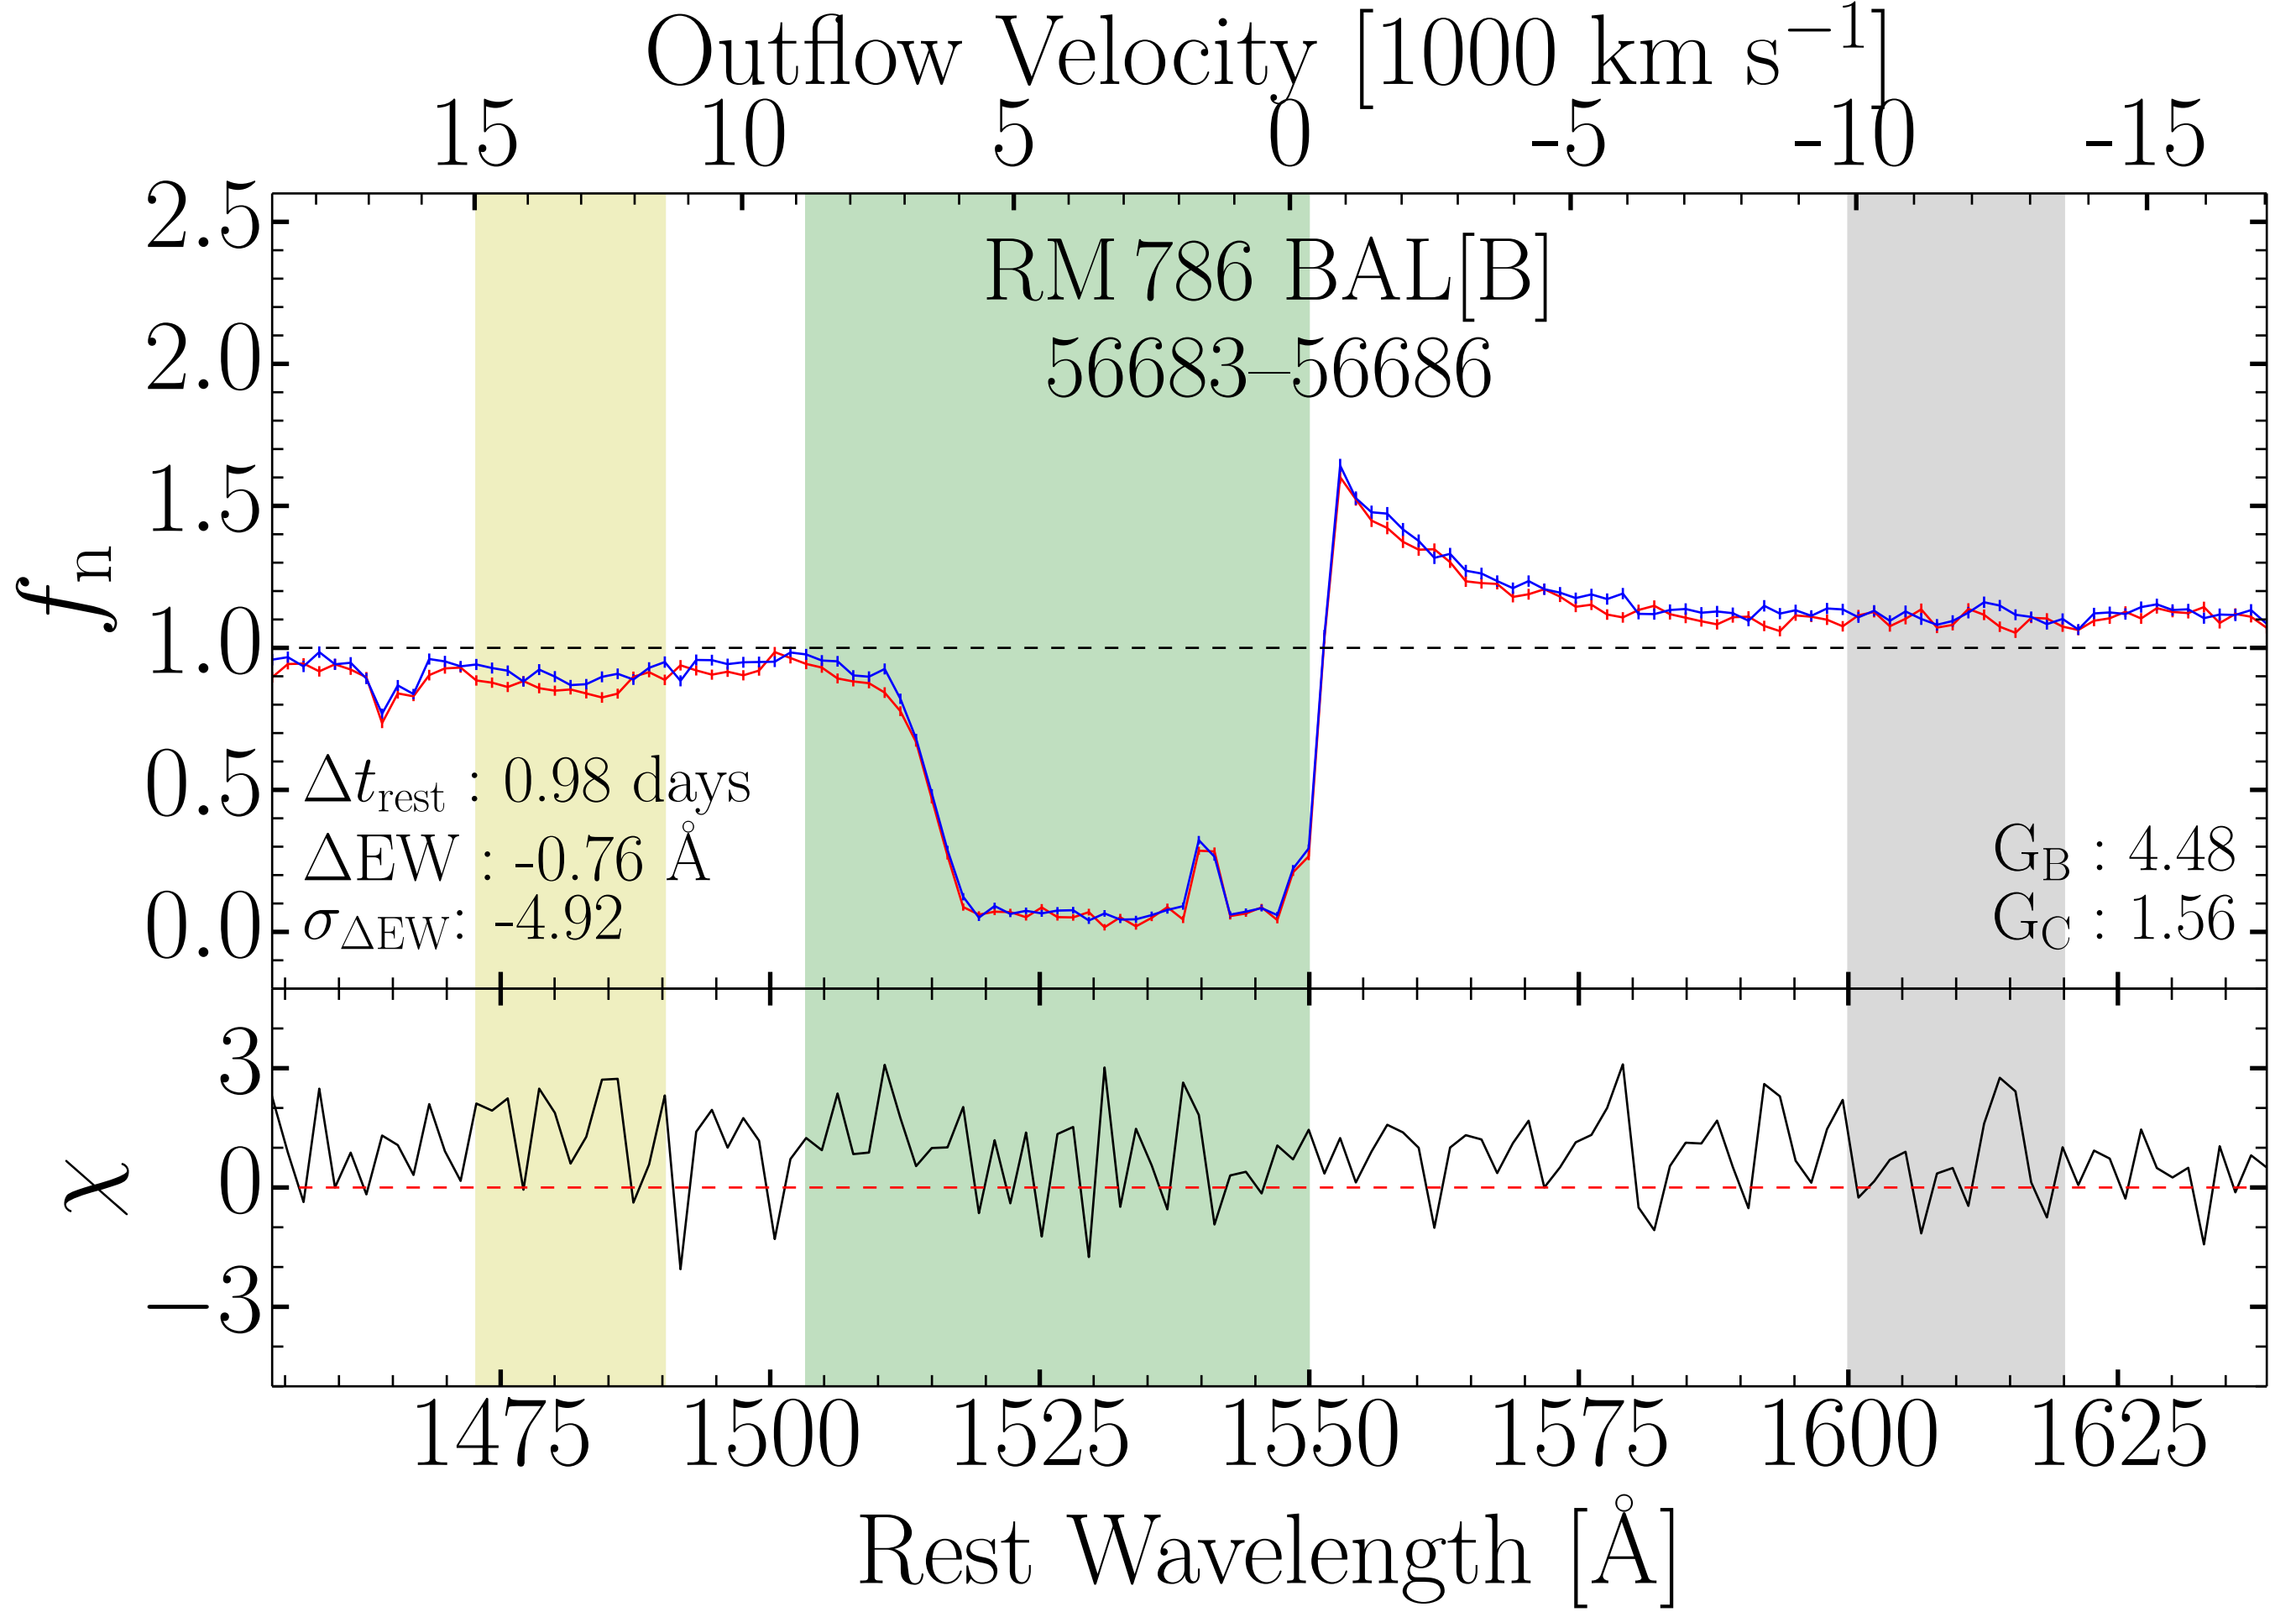



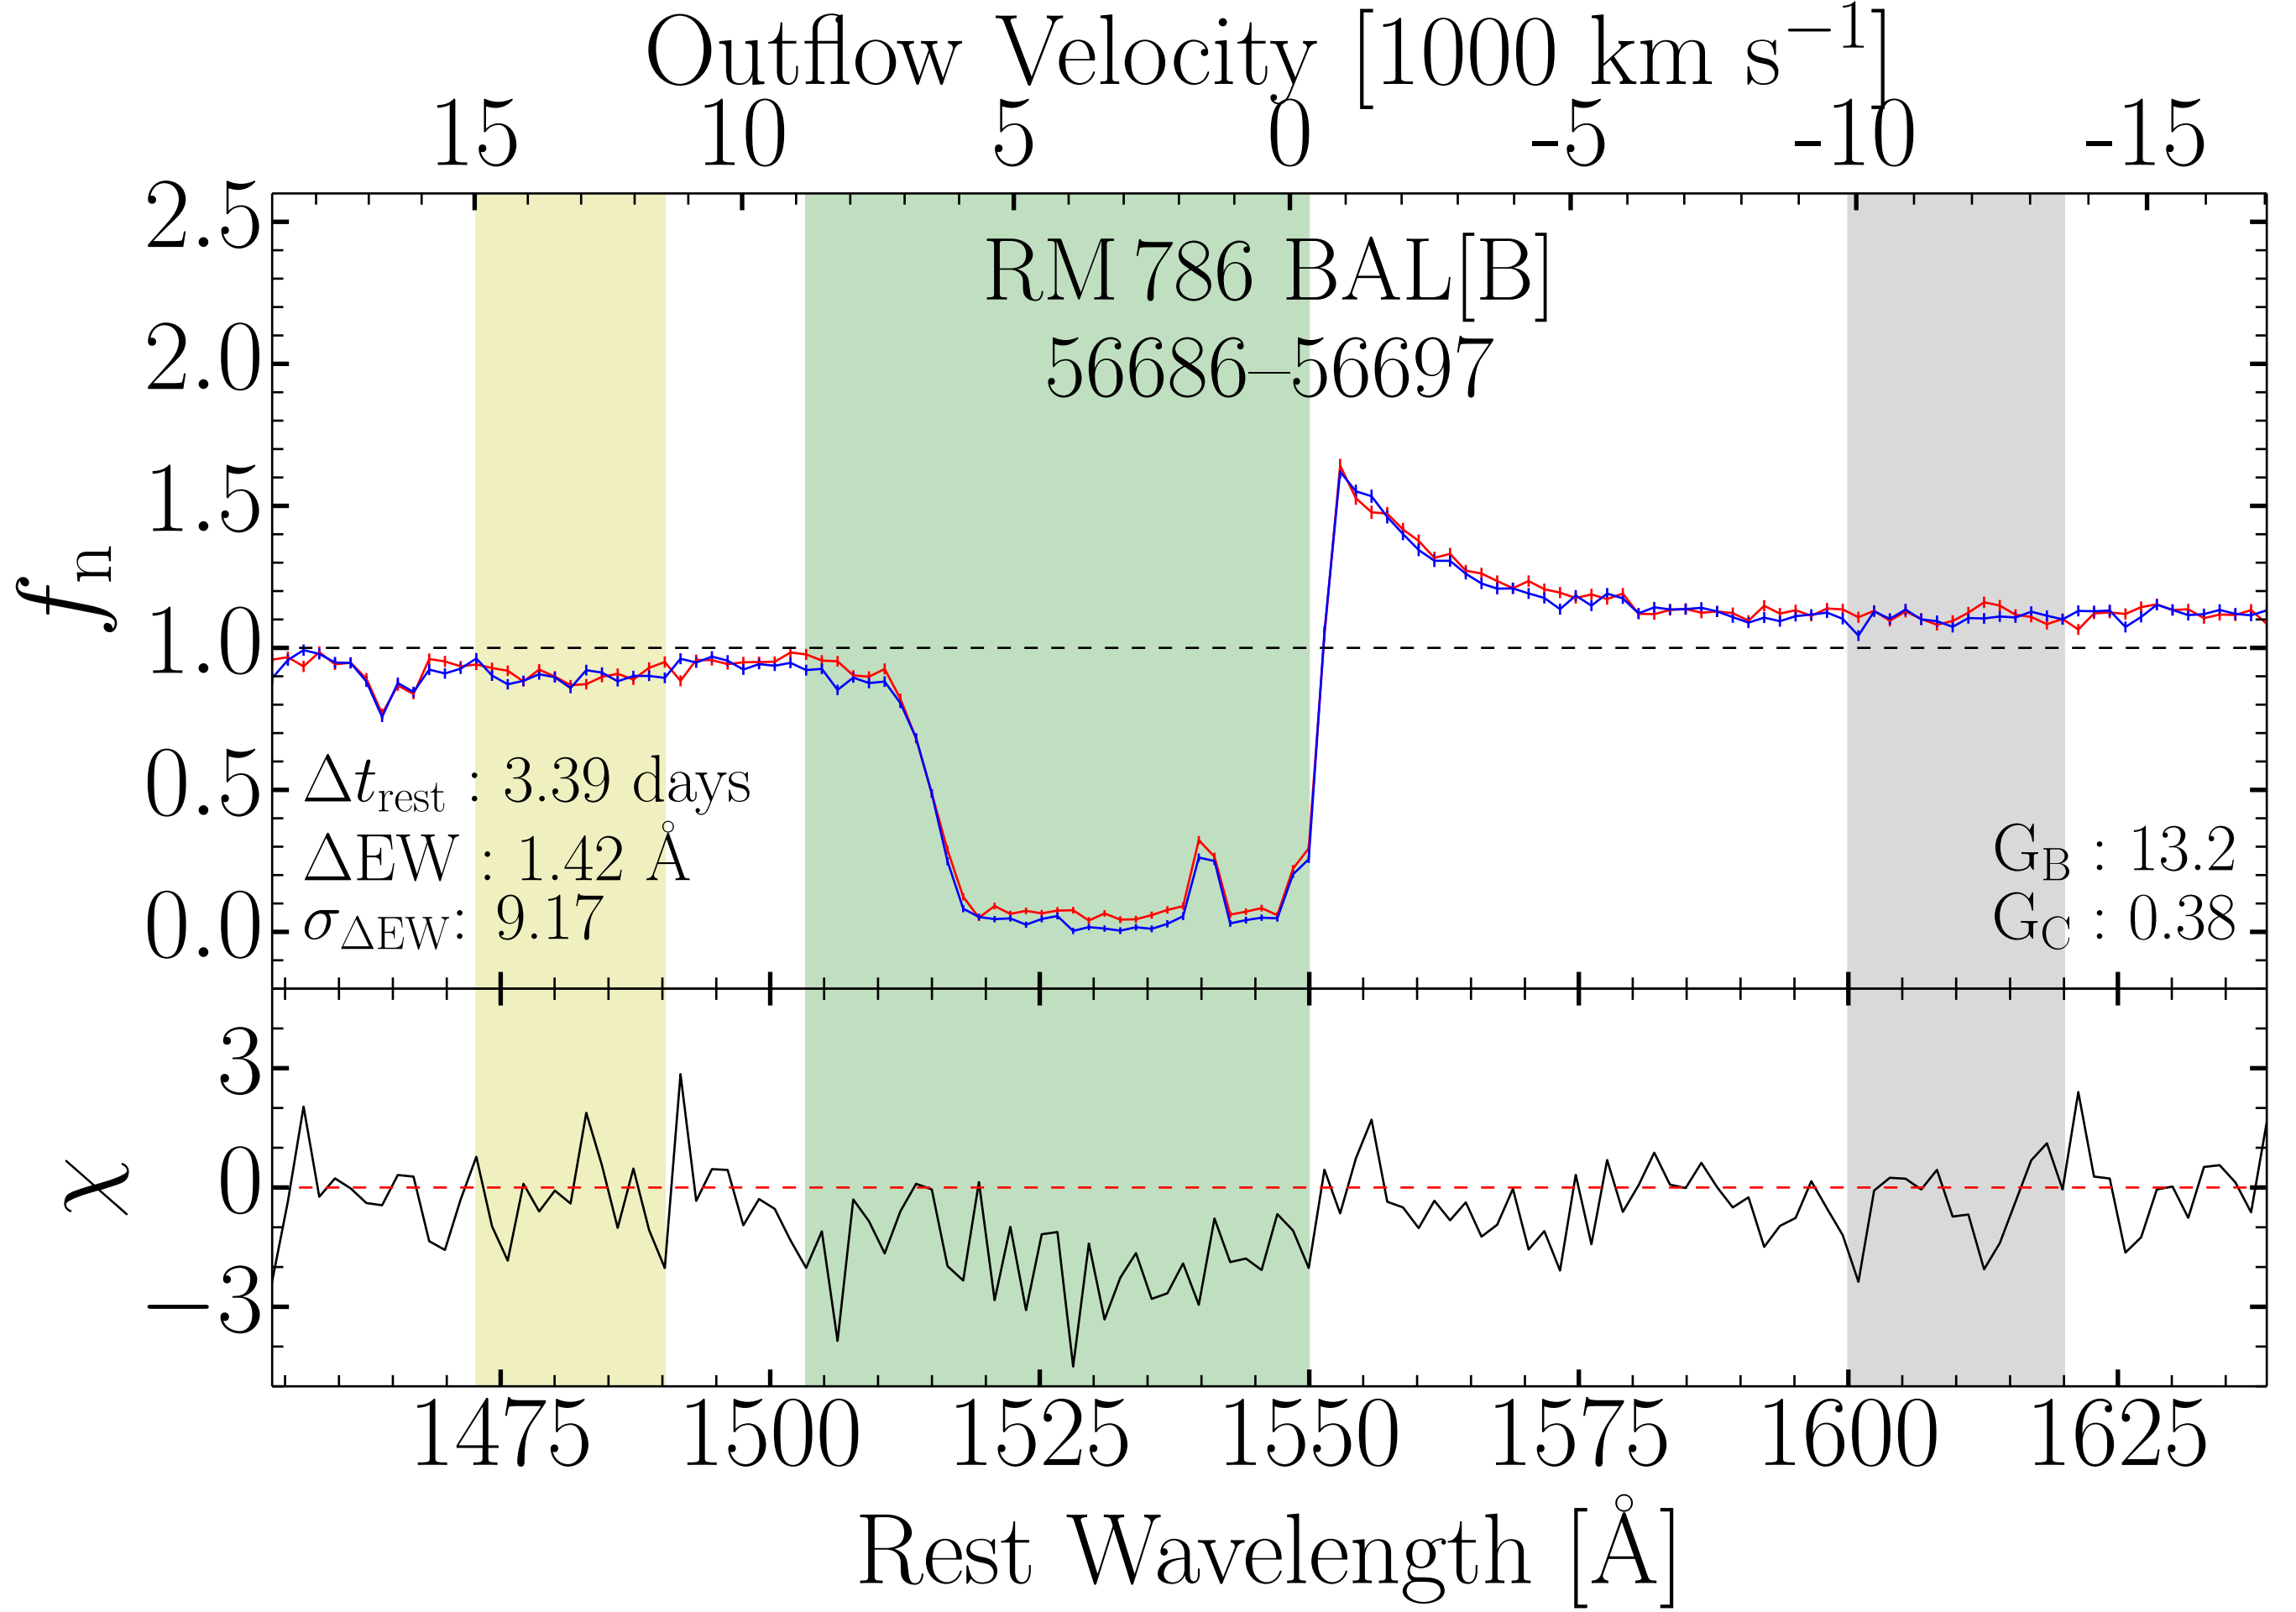

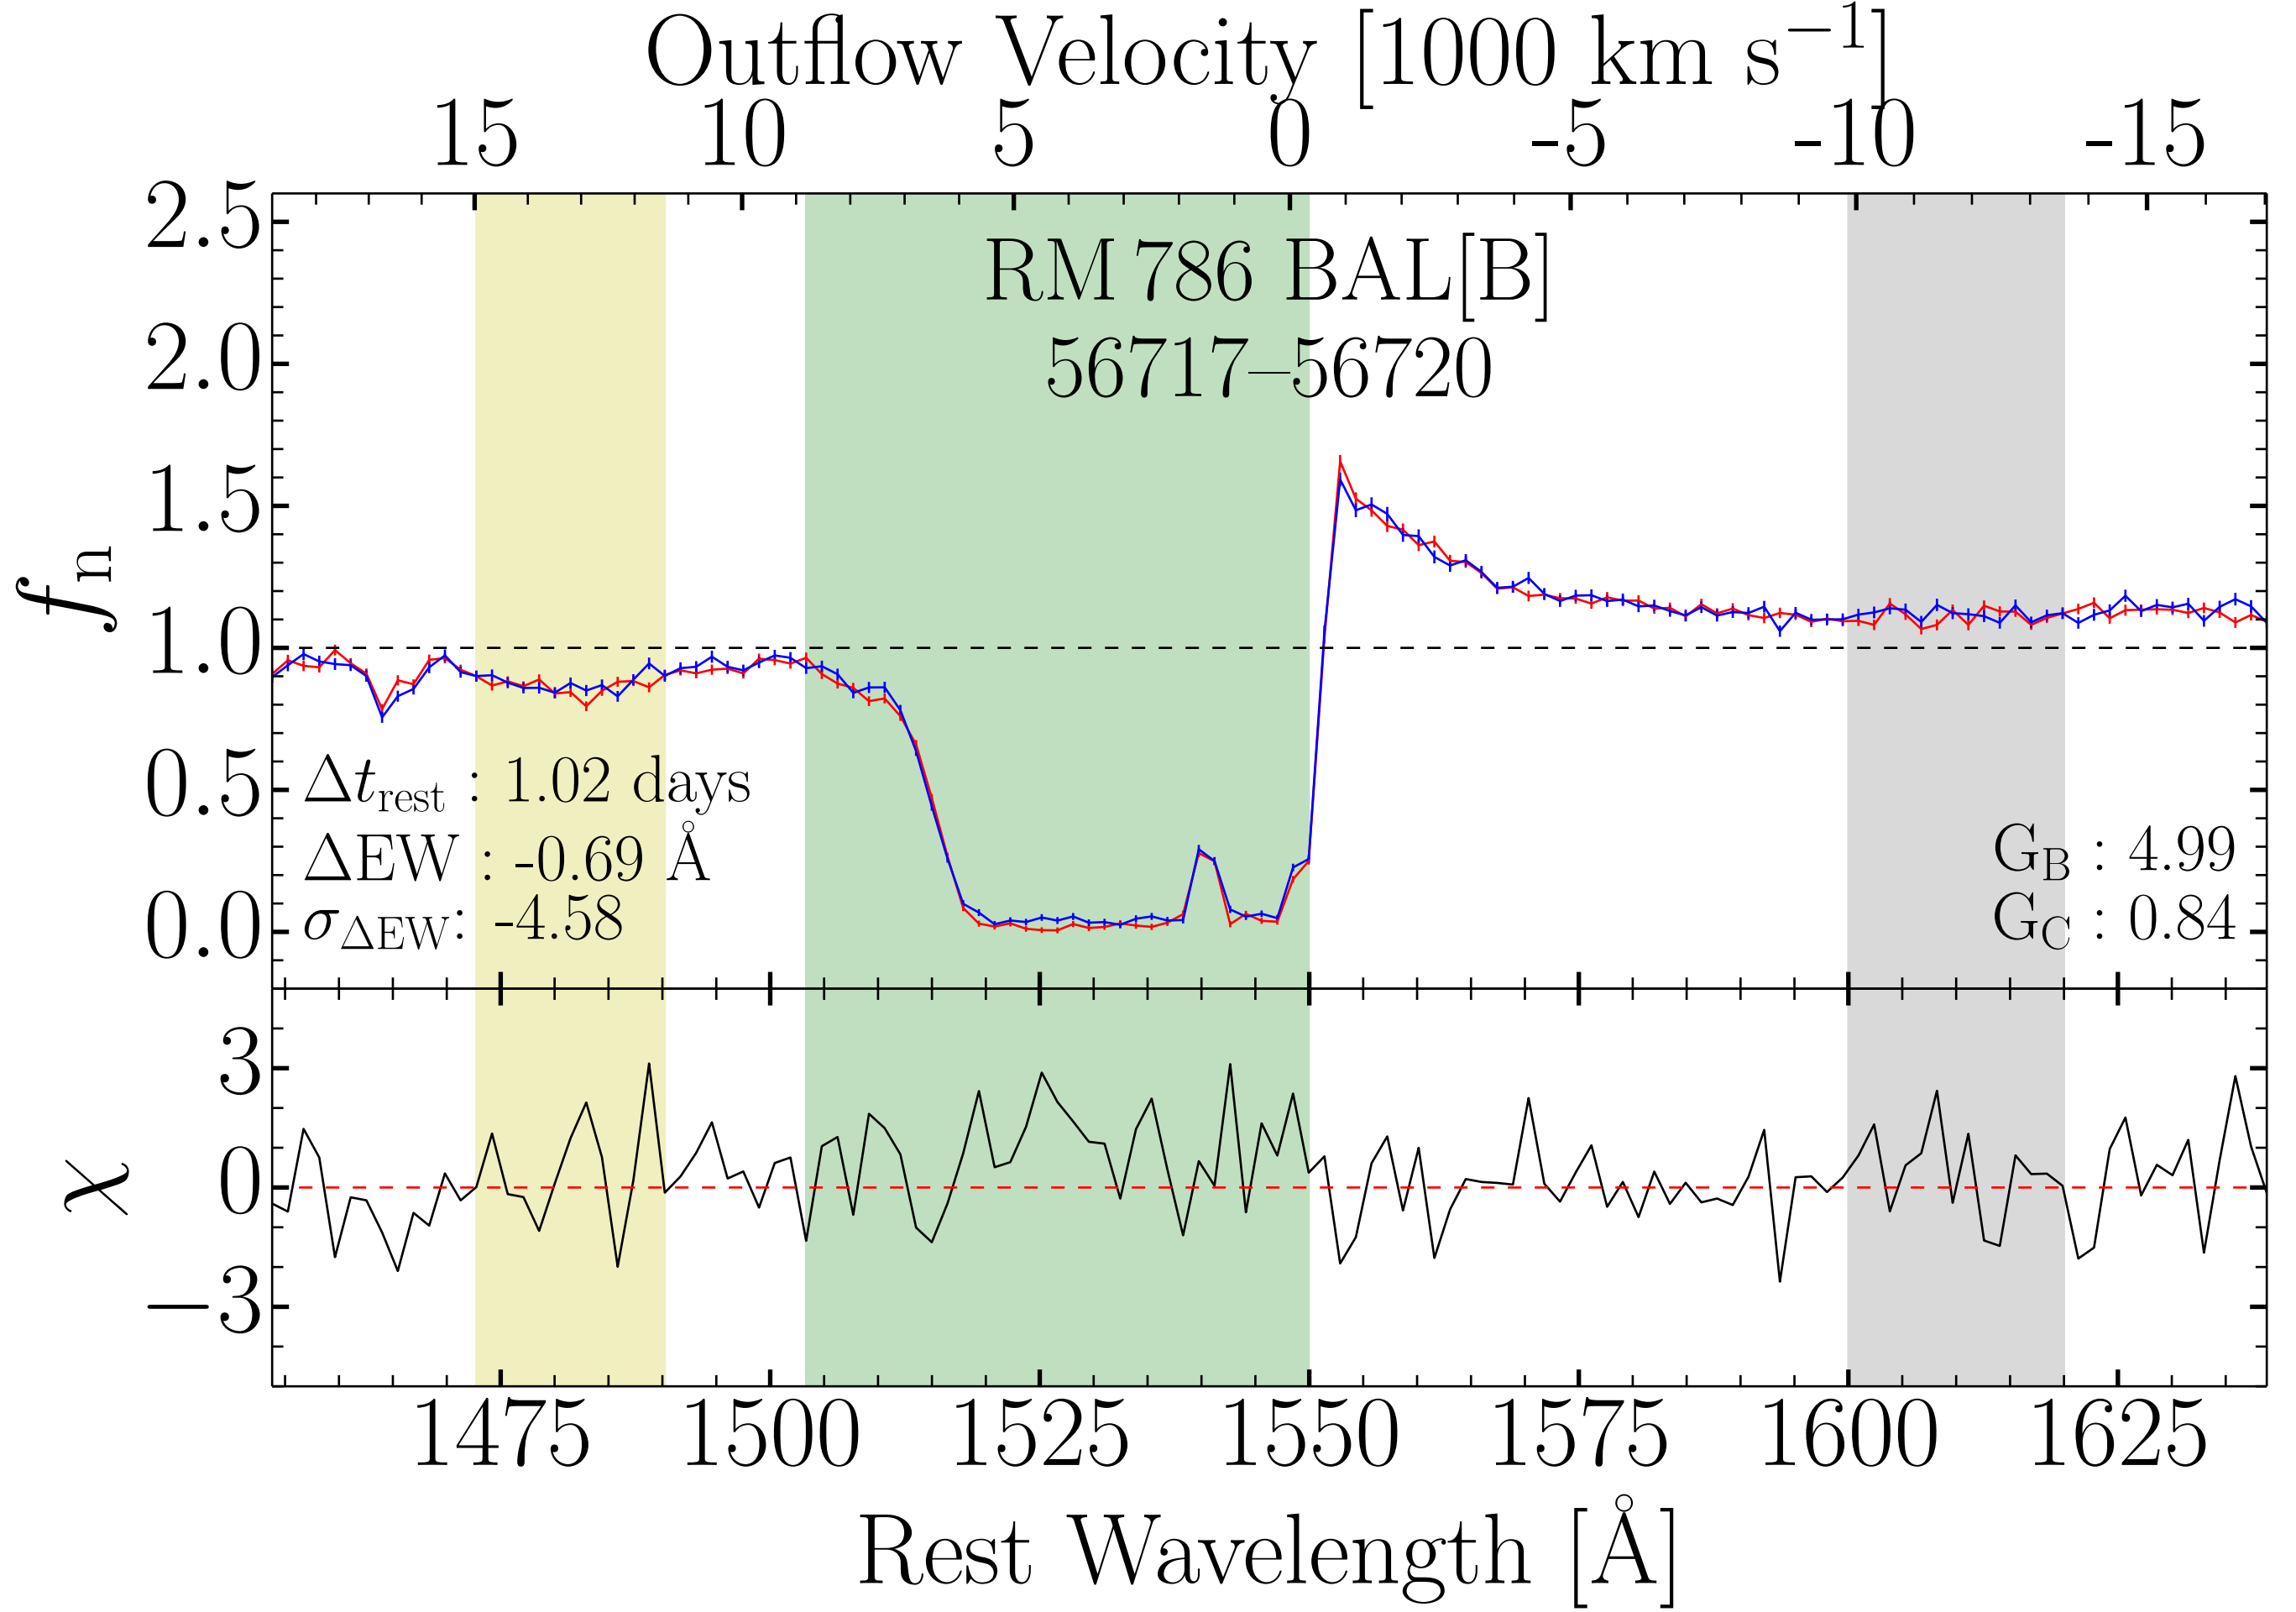

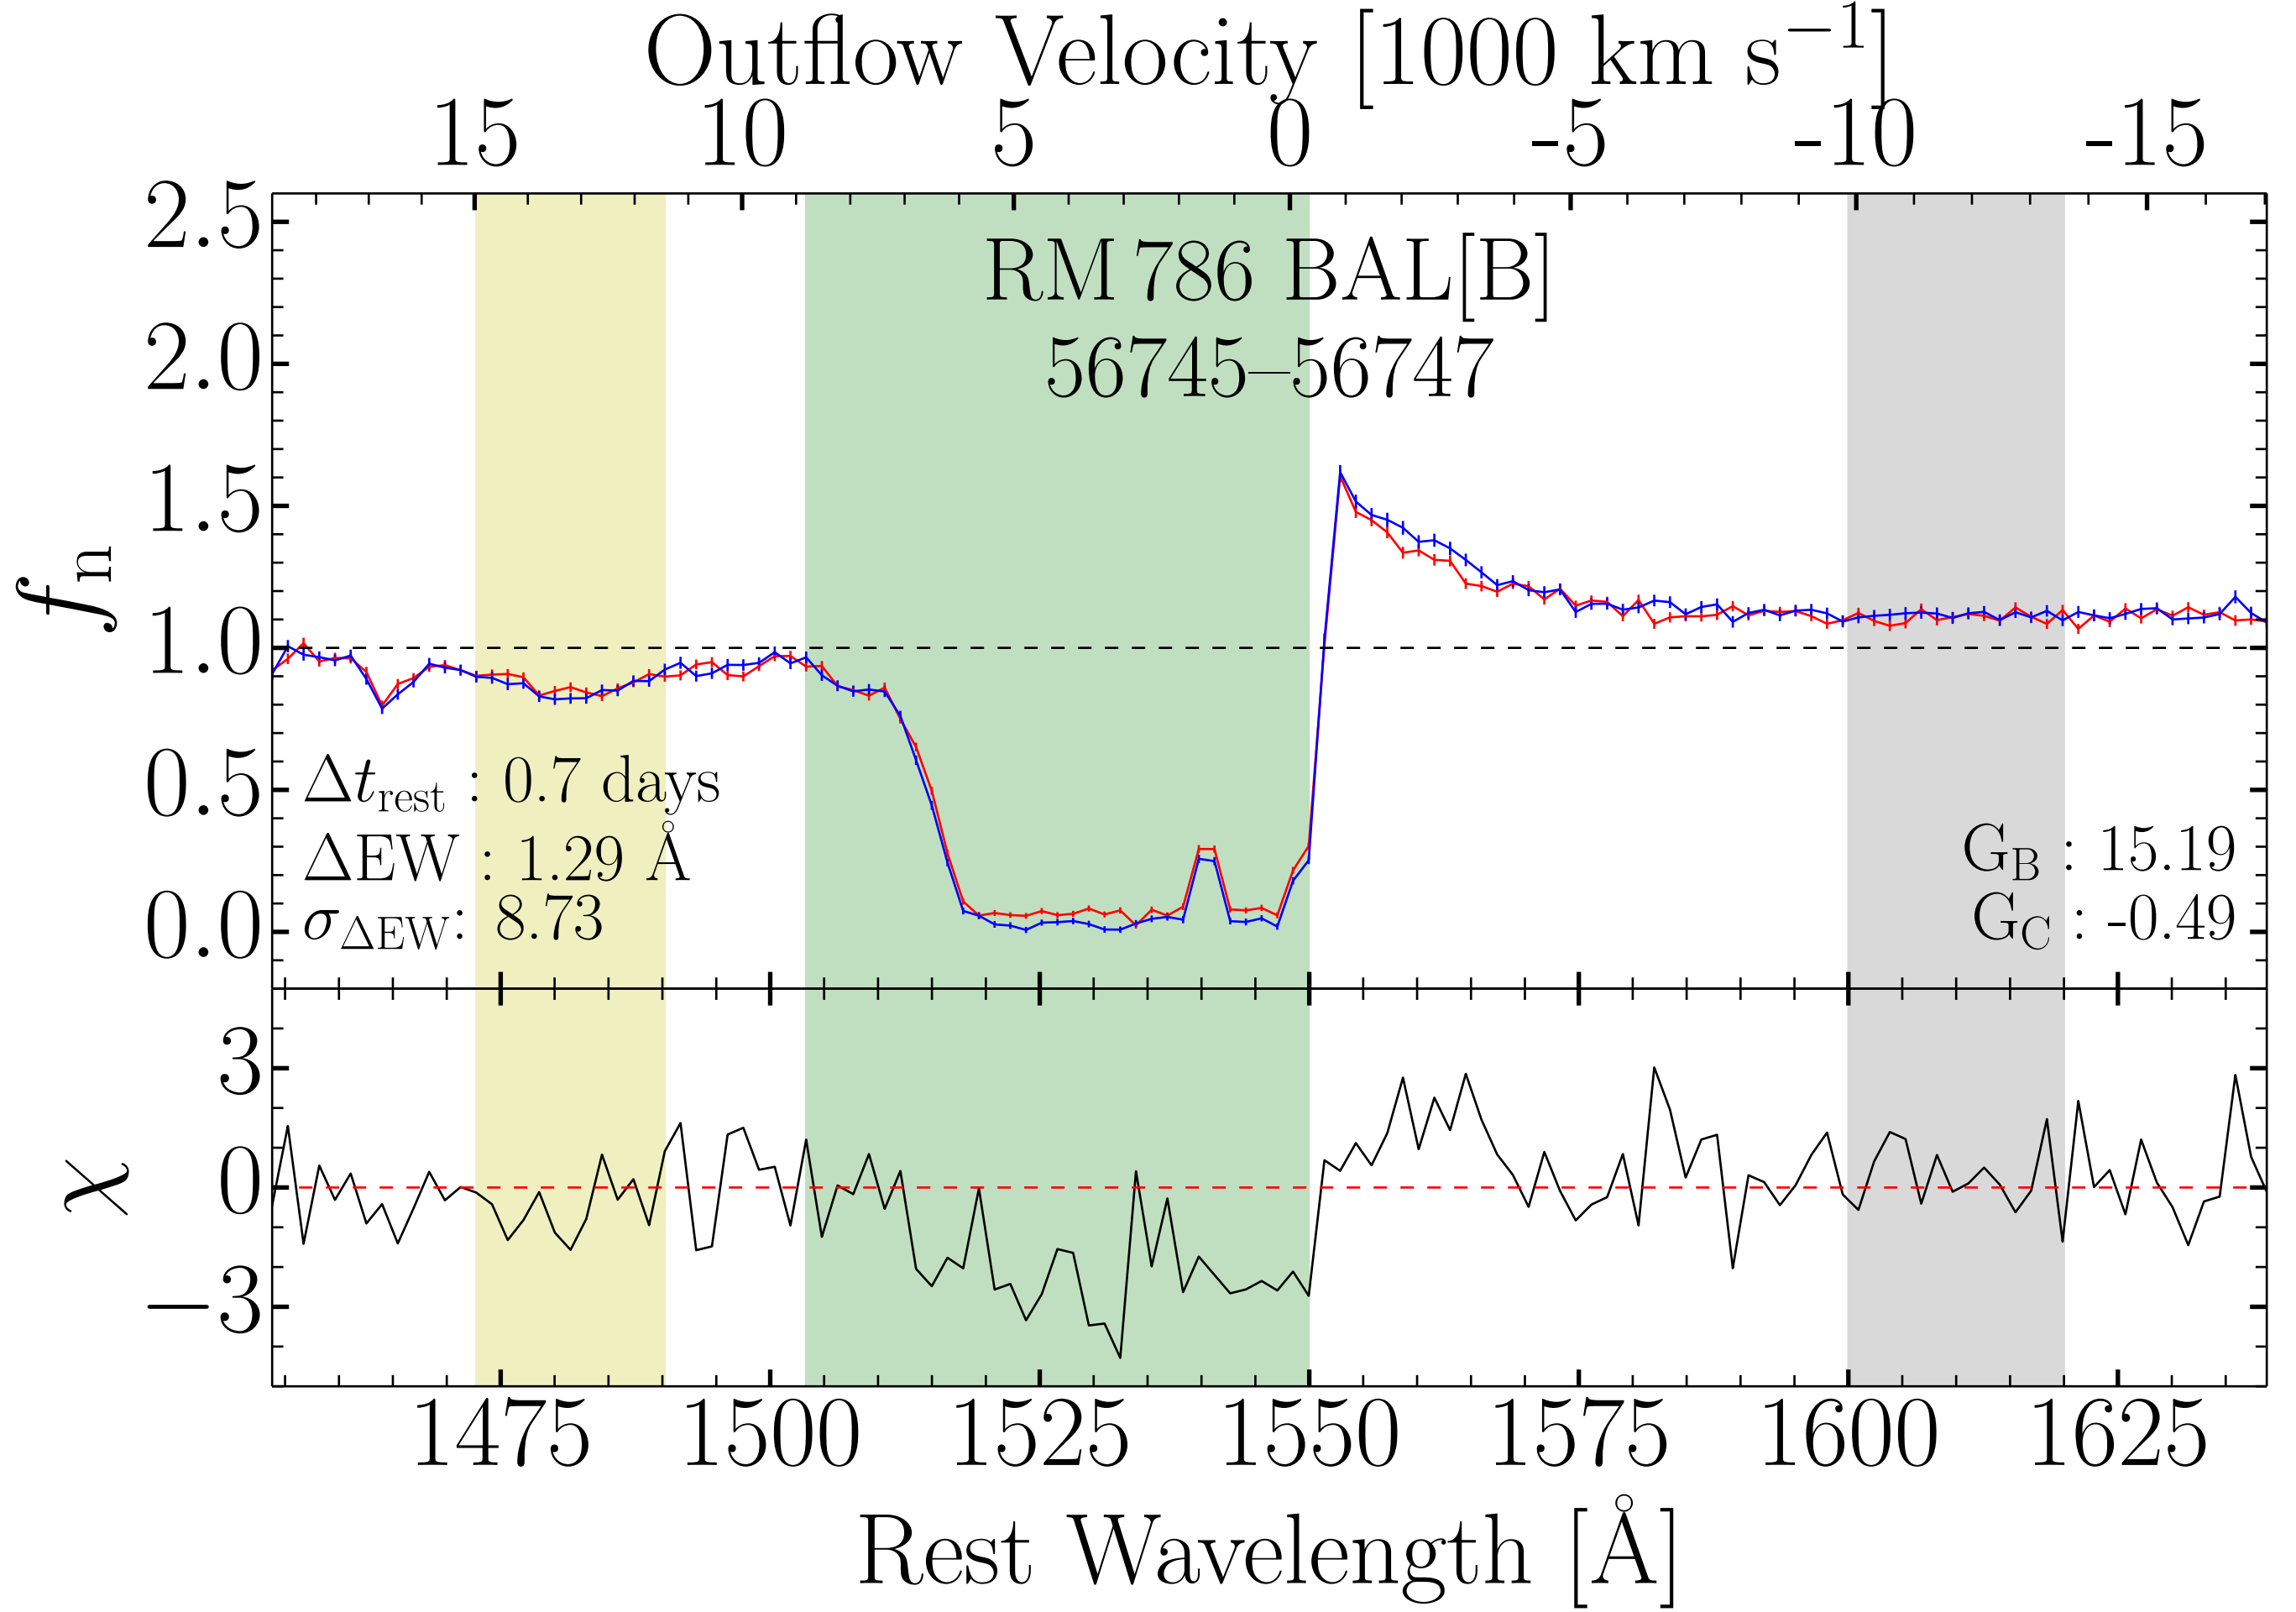

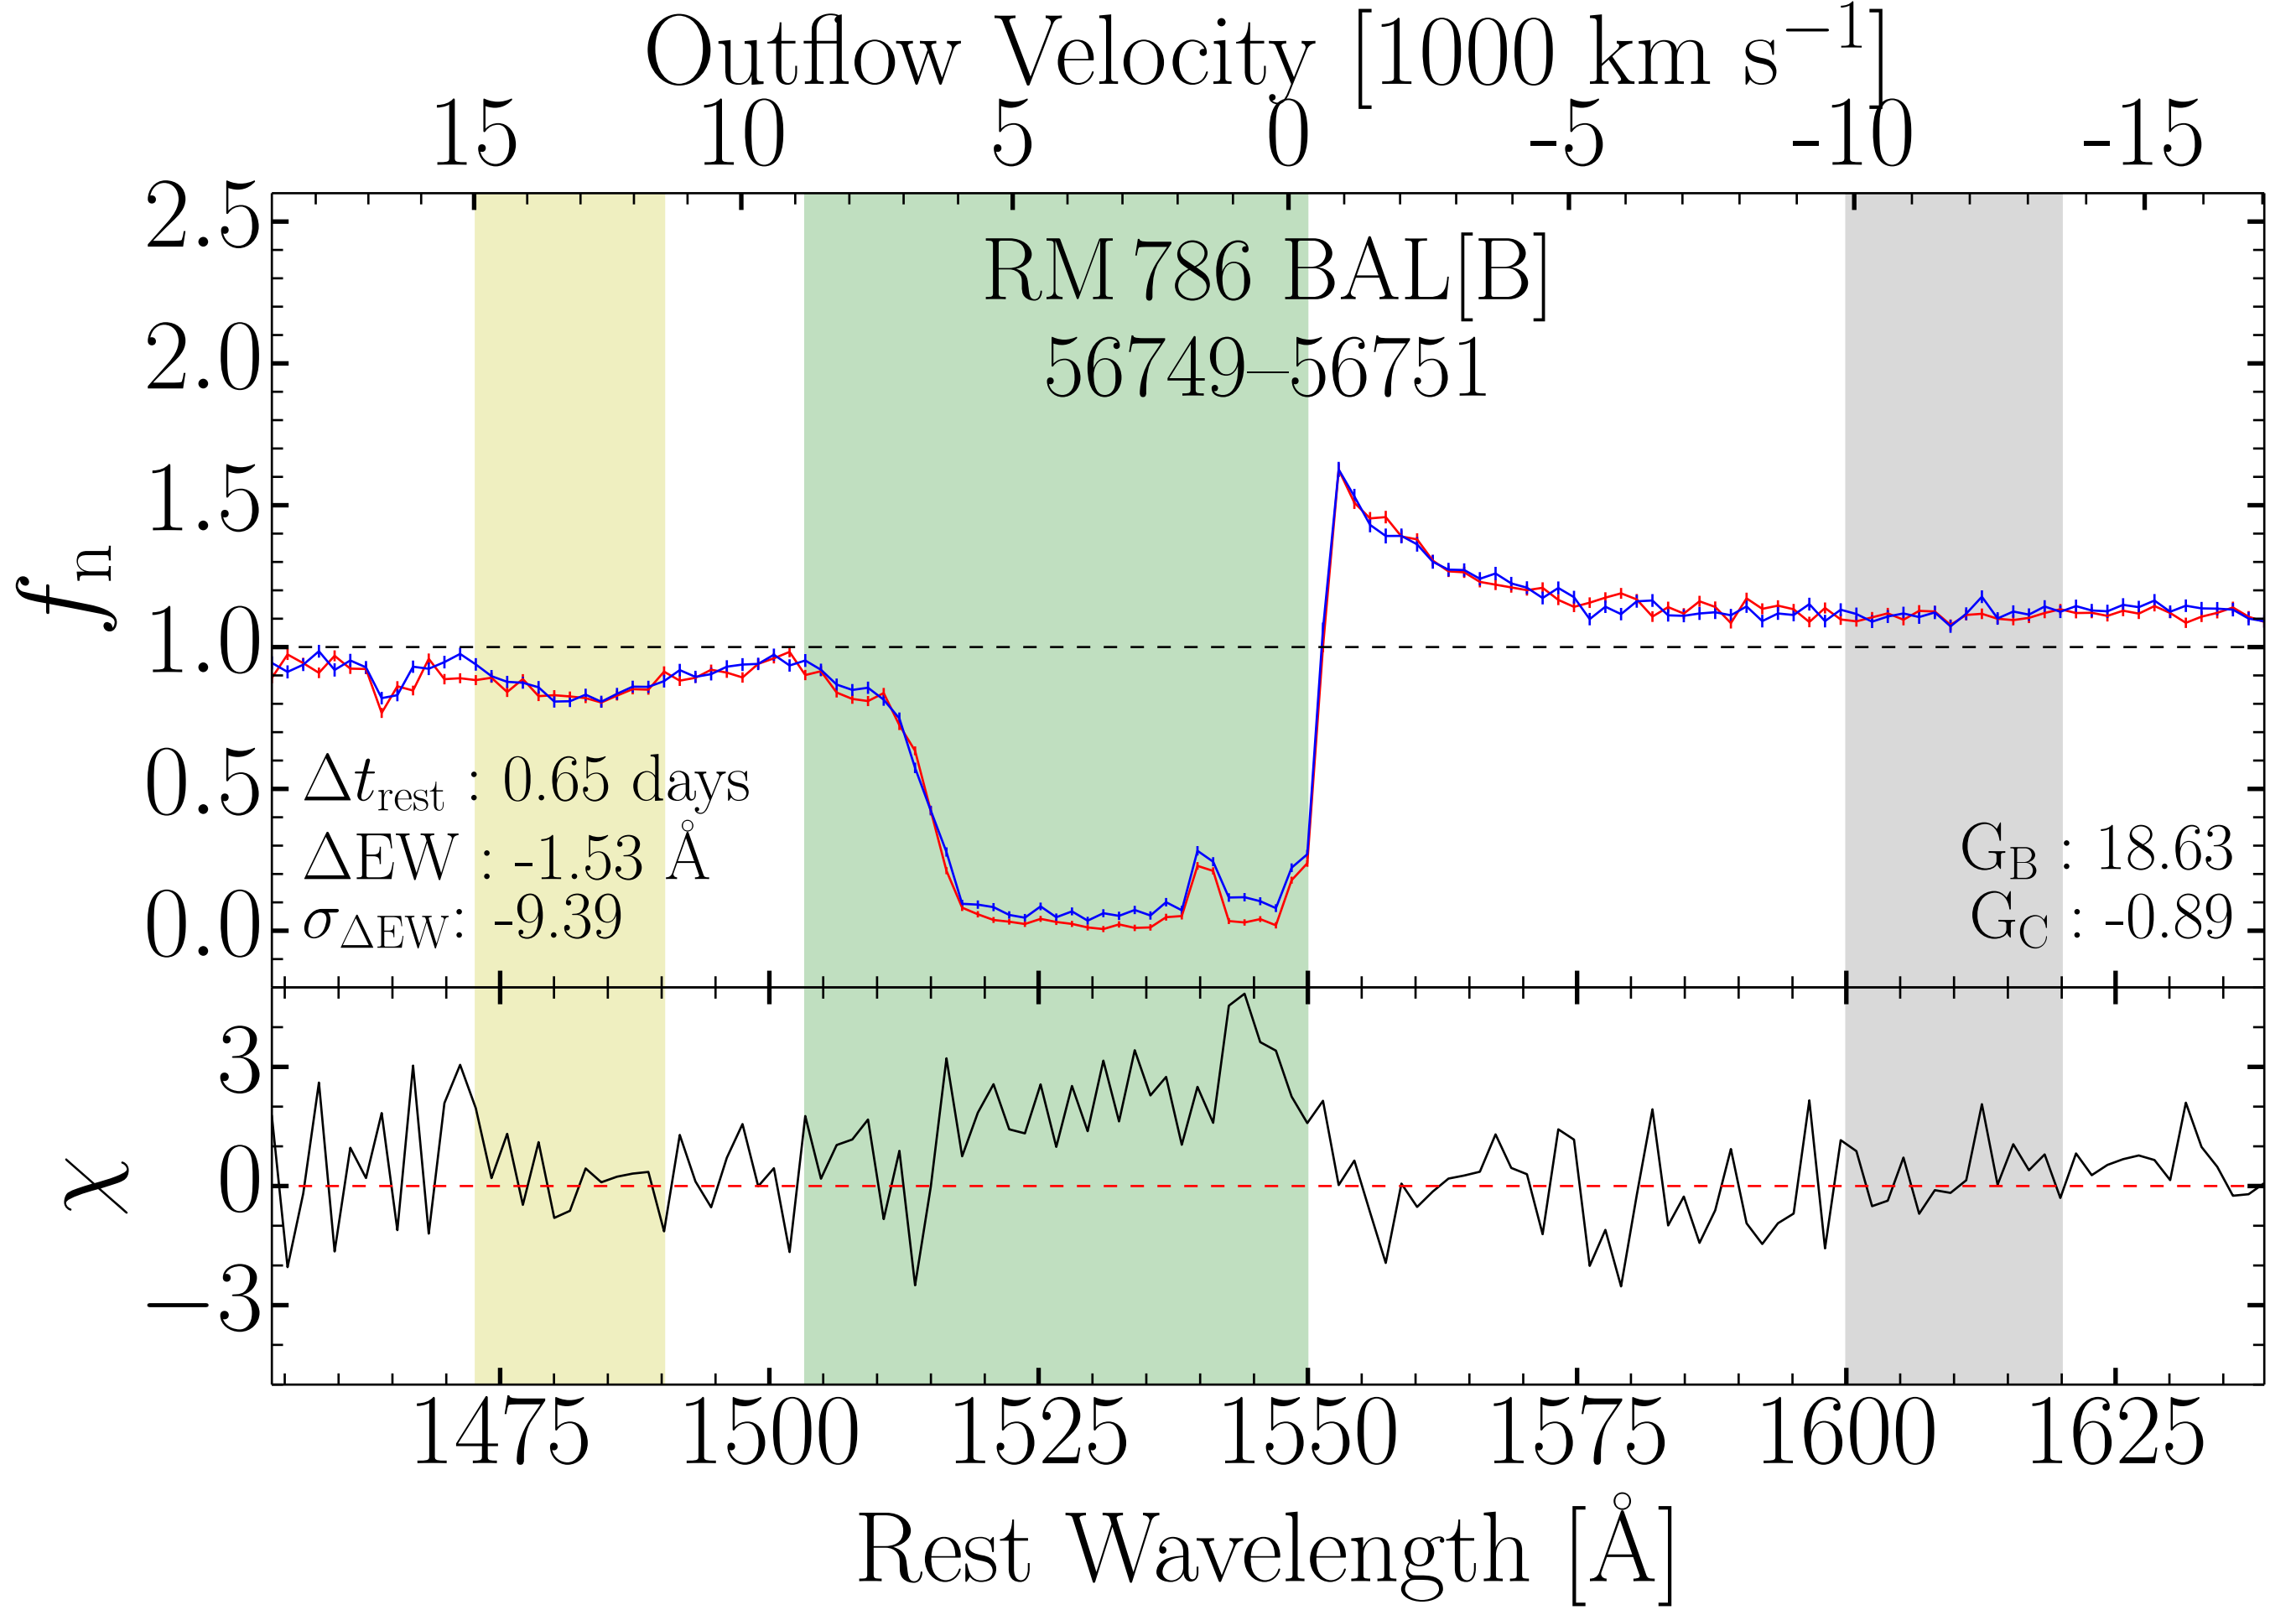

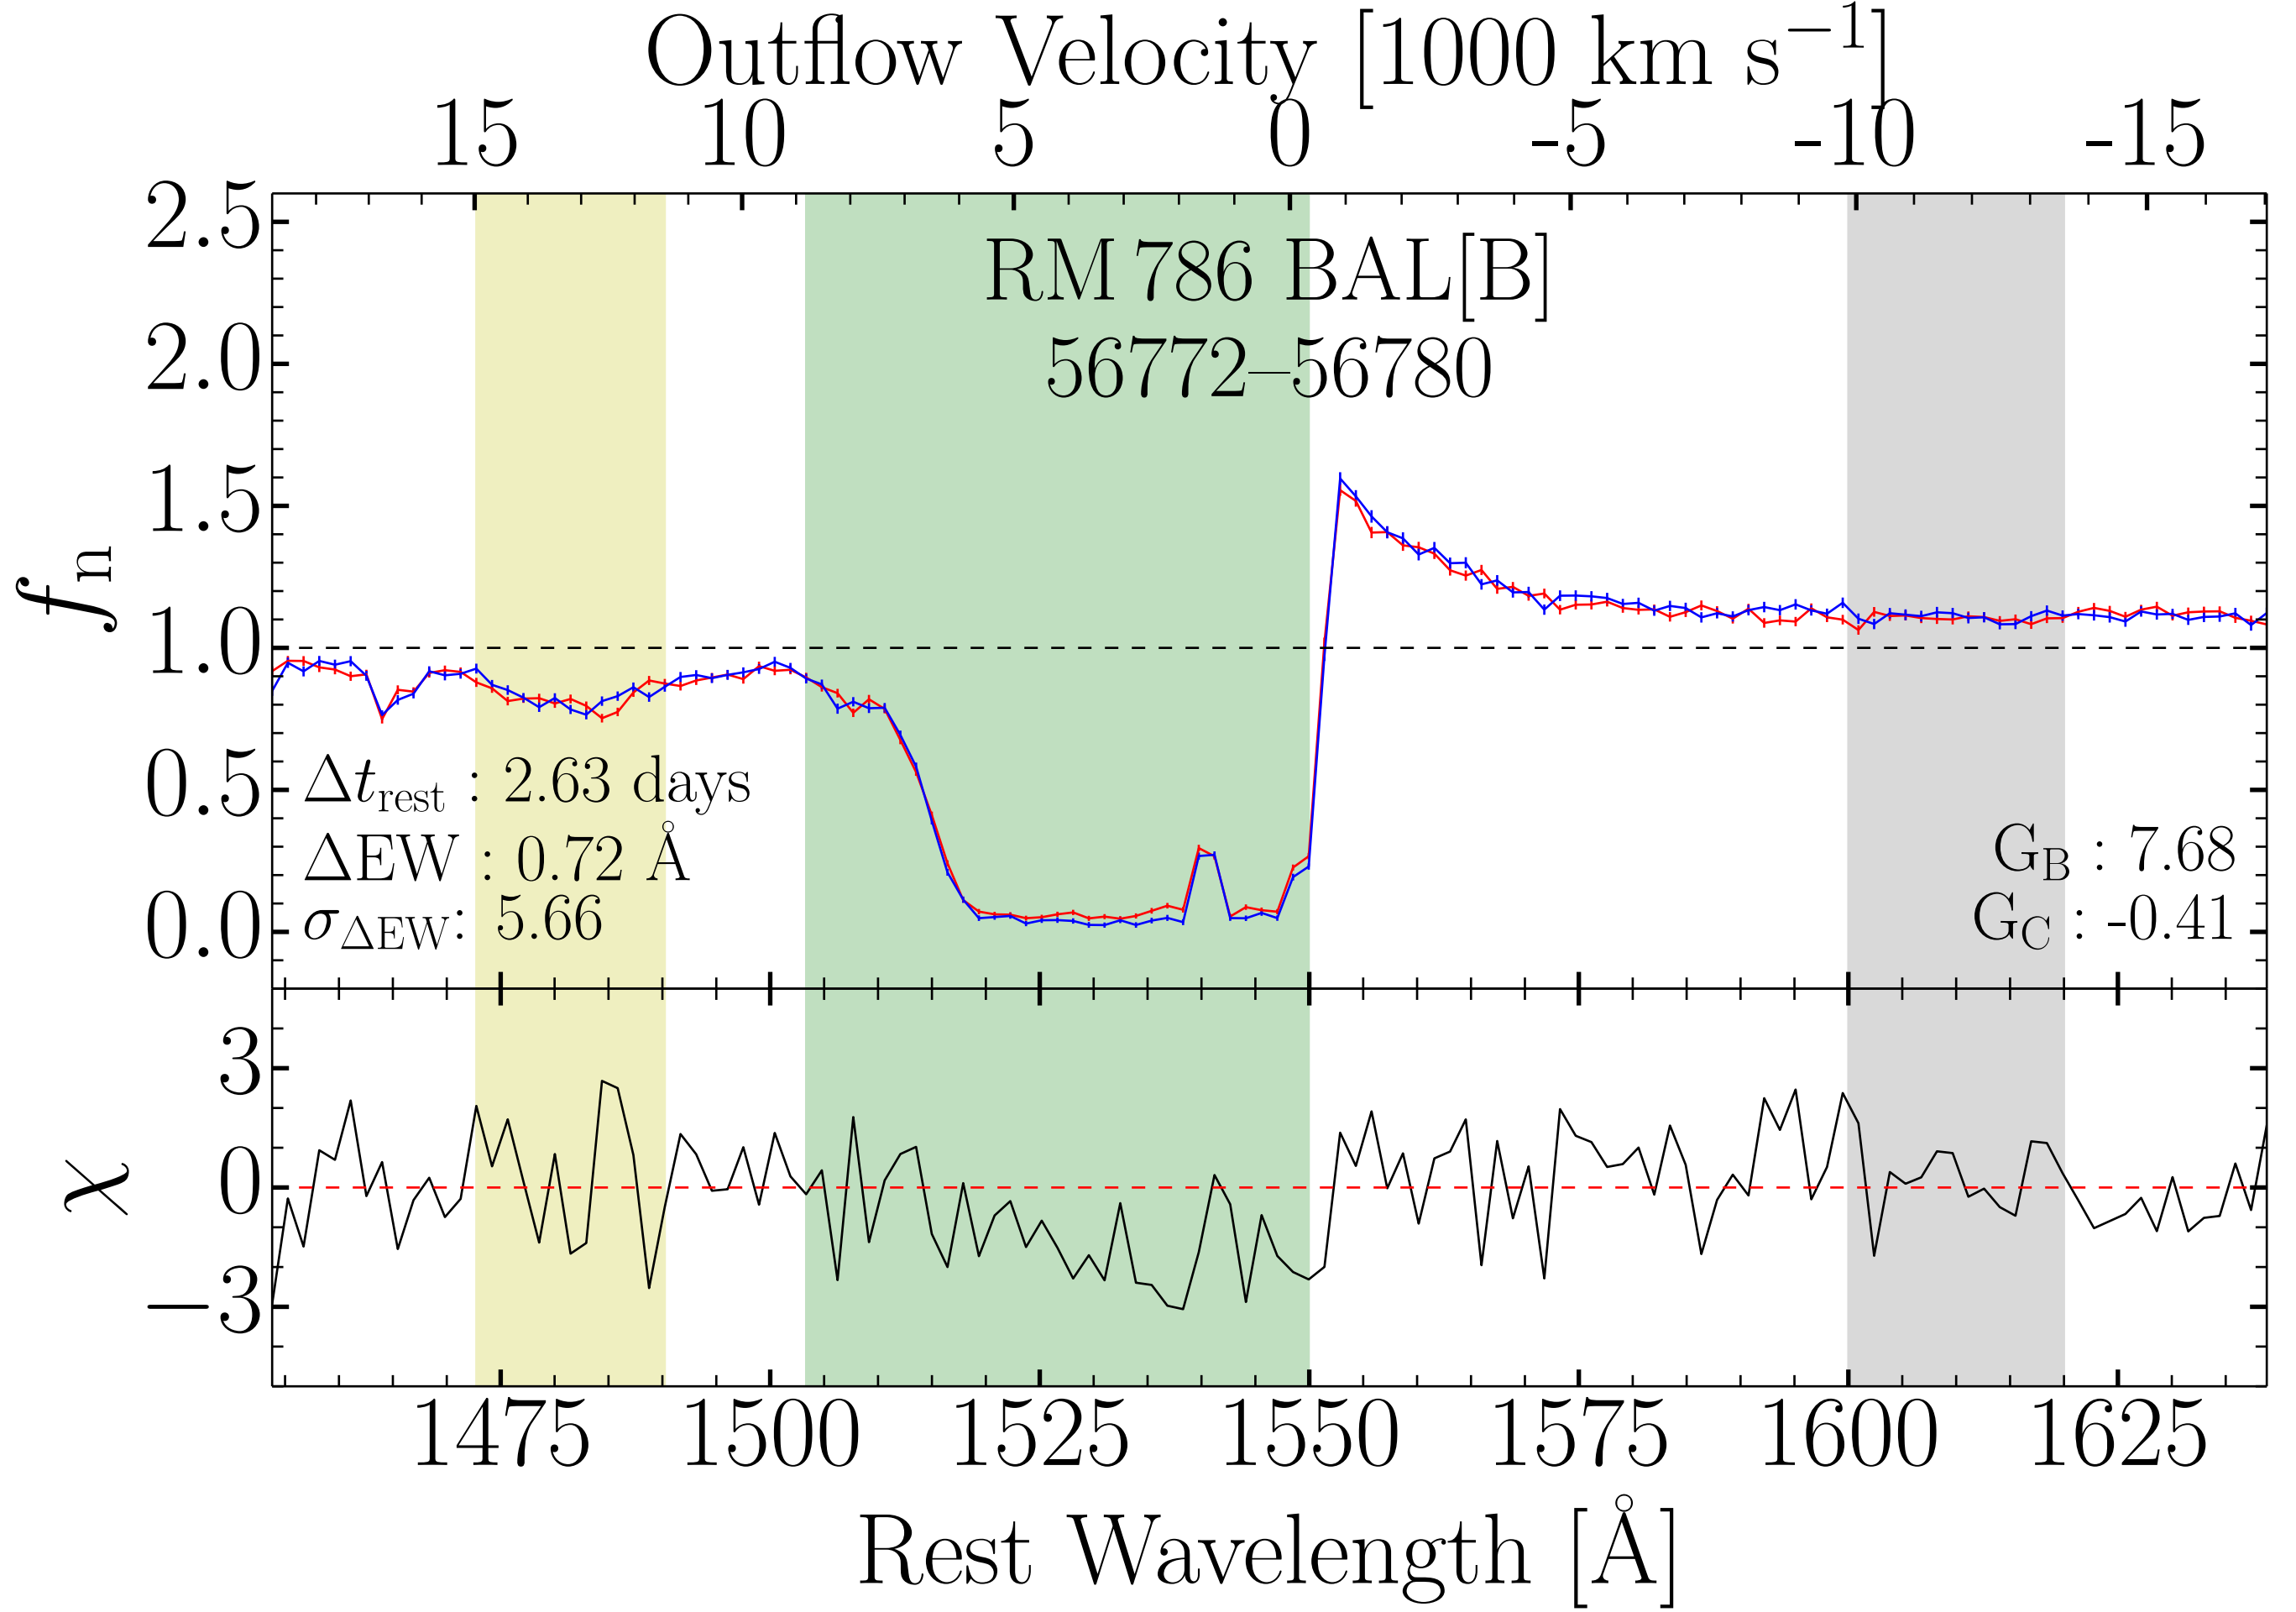

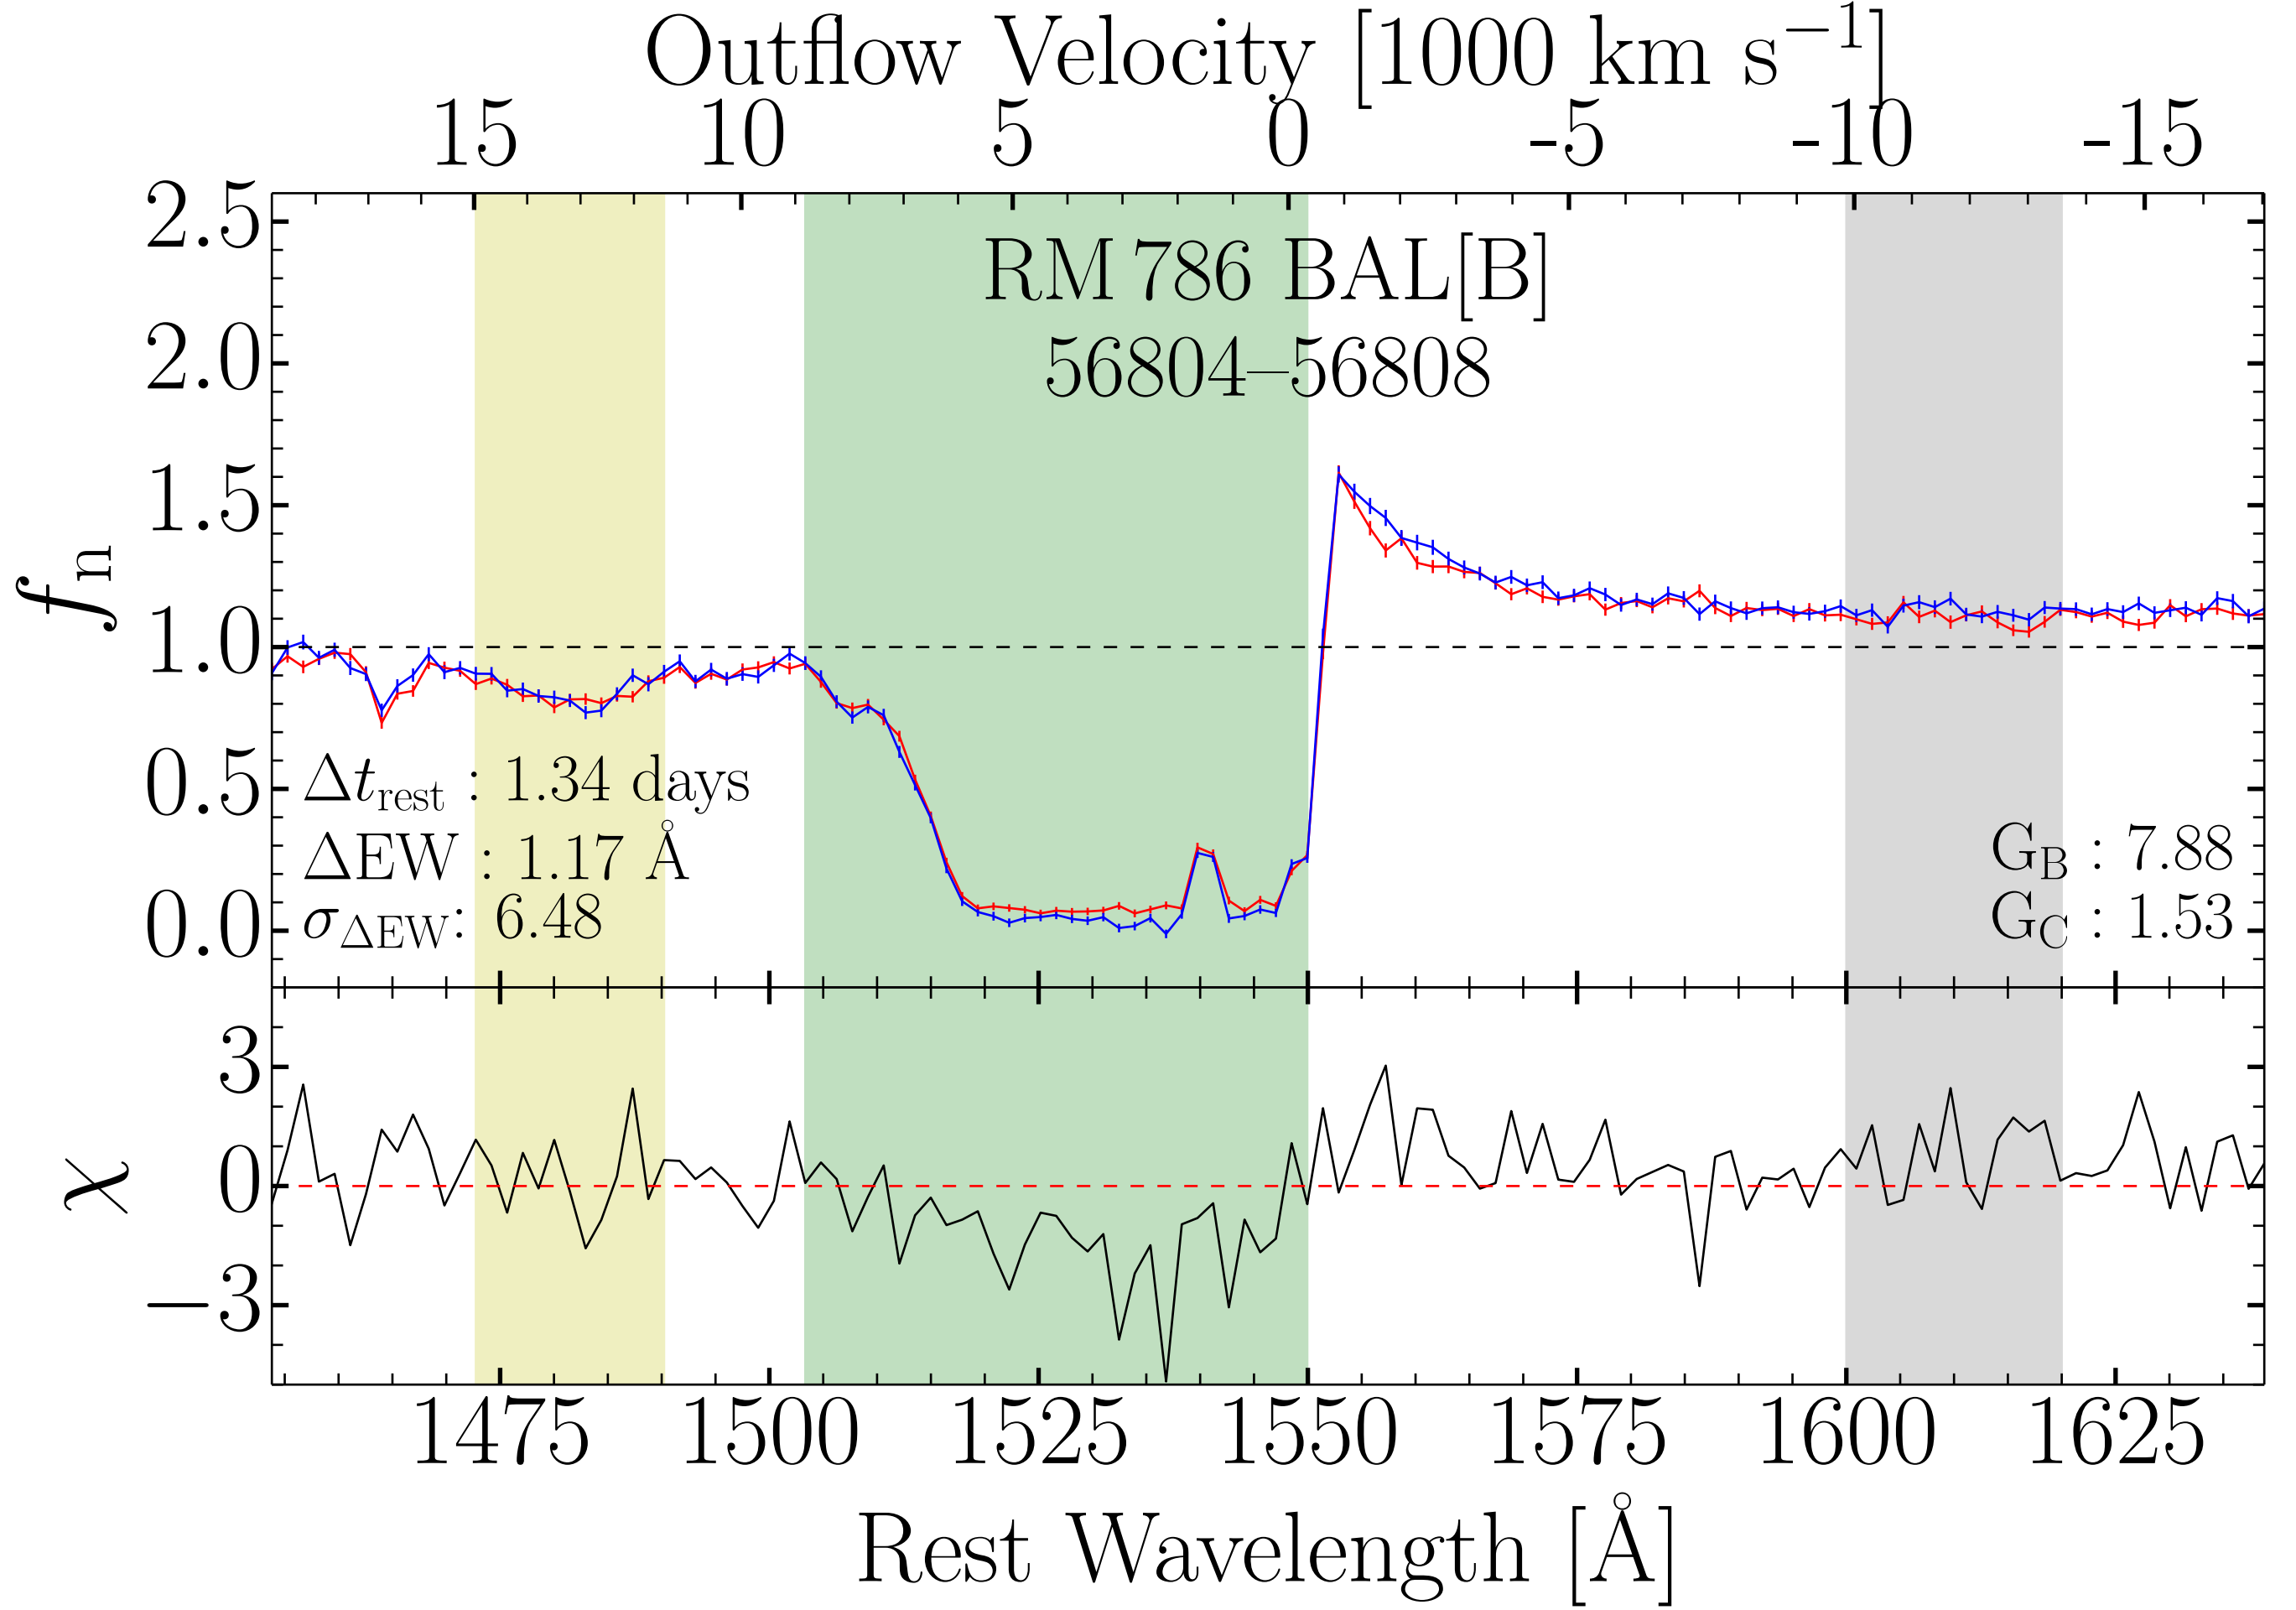

Supplement: Supplementary file 3 [file Figure8Set.pdf]
